# Supplementary material for: Linear congruence relations for exponents of Borcherds products
Source: arXiv:2301.11184 ancillary file (2026-06-08)
Supplement: Supplementary file 1 [file Mathem._f3_10000_coefficients.pdf]

In[1]:= N1 := 10001

In[2]:= N4 := 2501

In[3]:= sqrtN := 101

In[4]:= Eisen10[q\_, l\_] := 1 - 264 \* Sum[DivisorSigma[9, n] \* q^n, {n, 1, l}]  
[s... Teilerfunktion Sigma

In[5]:= Eisen104[q\_, l\_] := Eisen10[q^4, l]

In[6]:= theta[q\_, l\_] := 1 + 2 \* Sum[q^(n^2), {n, 1, l}]  
[summiere

In[7]:= thetaprime[q\_, l\_] := 2 \* Sum[n^2 \* q^(n^2), {n, 1, l}]  
[summiere

In[8]:= Eisen10prime[q\_, l\_] := D[Eisen10[q, l], q] /. q -> q^4  
[leite ab

In[9]:= Delta4[q\_, l\_] := q^4 \* Product[(1 - q^(4 \* n))^ (24), {n, 1, l}]  
[Produkt

In[10]:= Series[ ((-1) / 10) \* (Series[(theta[q, sqrtN] \* q^4 \* Eisen10prime[q, N1] -  
[Reihe [Reihe  
5 \* thetaprime[q, sqrtN] \* Eisen104[q, N4]) / Delta4[q, N4],  
{q, 0, N1}] + 304 \* theta[q, sqrtN]), {q, 0, N1}]

$$\frac{1}{q^3} - 248 q + 26752 q^4 - 85995 q^5 + 1707264 q^8 - 4096248 q^9 + 44330496 q^{12} - 91951146 q^{13} + 708938752 q^{16} - 1343913984 q^{17} + 8277534720 q^{20} - 14733025125 q^{21} + 77092288000 q^{24} - 130880766200 q^{25} + 604139268096 q^{28} - 988226335125 q^{29} + 4125992712192 q^{32} - 6548115718144 q^{33} + 25168873498752 q^{36} - 38948971203675 q^{37} + 139625296473600 q^{40} - 211482206208000 q^{41} + 714109061952000 q^{44} - 1061730839574405 q^{45} + 3403263881170944 q^{48} - 4978357936128248 q^{49} + 15242406059575296 q^{52} - 21978258495365367 q^{53} + 64601814211200000 q^{56} - 91959905058717696 q^{57} + 260587764136294400 q^{60} - 366670770751065375 q^{61} + 1005225129317834752 q^{64} - 1399658986148659200 q^{65} + 3723382942543724544 q^{68} - 513491009445157375 q^{69} + 13288900691444361984 q^{72} - 18166228425591128064 q^{73} + 45837862940390976000 q^{76} - 62155548894834991134 q^{77} + 153208405260561530880 q^{80} - 206195878414962688248 q^{81} + 497351599230700032000 q^{84} - 664712305249895086275 q^{85} + 1571268694728598728192 q^{88} - 2086403563729465344000 q^{89} + 4839811464525274957824 q^{92} - 6387584332011848220060 q^{93} + 14557905935137929728000 q^{96} - 19104303348255106695168 q^{97} + 42824436296045618358400 q^{100} - 55897900726628243067750 q^{101} + 123360098635392655680000 q^{104} - 160207720435903812403200 q^{105} + 348387441521711024498688 q^{108} - 450295048312241116461750 q^{109} + 965656482360879246852096 q^{112} - 1242491961502660359684096 q^{113} + 2629552536370095259392000 q^{116} - 3368913541363186297350723 q^{117} + 7040938644932617005388800 q^{120} - 8983966738037593190400248 q^{121} + 18553561298668351388160000 q^{124} - 23581937034763331475744675 q^{125} + 48150642600147147218436096 q^{128} - 60974372253512846929920000 q^{129} + 123157160007398448626286592 q^{132} - 155406973376229277138022853 q^{133} + 310657607063389715036544000 q^{136} - 390684010153976888520278016 q^{137} + 773269054153265448774374400 q^{140} - 969325246679971848864731625 q^{141} + 1900416270294787067711818752 q^{144} - 2374876395398403374388019200 q^{145} + 4613843375735732716149172224 q^{148} - 5748608250439912771997265000 q^{149} + 11070937433860986486083166720 q^{152} - 13754427746553619480458657792 q^{153} + 26267038925078650005742848000 q^{156} - 32544300922236617552772478542 q^{157} +$$

$61\ 649\ 313\ 622\ 264\ 569\ 913\ 547\ 673\ 600\ q^{160} - 76\ 180\ 226\ 508\ 602\ 745\ 601\ 572\ 864\ 000\ q^{161} +$   
 $143\ 188\ 980\ 687\ 460\ 115\ 250\ 425\ 856\ 000\ q^{164} - 176\ 488\ 162\ 490\ 358\ 926\ 884\ 134\ 751\ 425\ q^{165} +$   
 $329\ 244\ 504\ 886\ 316\ 348\ 511\ 942\ 609\ 920\ q^{168} - 404\ 814\ 256\ 845\ 771\ 786\ 255\ 876\ 096\ 248\ q^{169} +$   
 $749\ 736\ 798\ 089\ 782\ 167\ 224\ 187\ 167\ 232\ q^{172} - 919\ 632\ 701\ 548\ 867\ 846\ 884\ 213\ 141\ 405\ q^{173} +$   
 $1\ 691\ 318\ 574\ 740\ 888\ 229\ 187\ 763\ 712\ 000\ q^{176} - 2\ 069\ 827\ 978\ 936\ 775\ 624\ 688\ 320\ 675\ 840\ q^{177} +$   
 $3\ 780\ 986\ 491\ 833\ 507\ 418\ 367\ 897\ 671\ 680\ q^{180} - 4\ 616\ 897\ 414\ 660\ 710\ 370\ 439\ 986\ 327\ 625\ q^{181} +$   
 $8\ 378\ 711\ 970\ 614\ 255\ 456\ 425\ 908\ 864\ 000\ q^{184} - 10\ 209\ 156\ 174\ 770\ 896\ 986\ 607\ 602\ 892\ 800\ q^{185} +$   
 $18\ 410\ 441\ 241\ 798\ 577\ 736\ 100\ 686\ 278\ 656\ q^{188} - 22\ 385\ 862\ 948\ 323\ 527\ 221\ 703\ 821\ 584\ 625\ q^{189} +$   
 $40\ 121\ 935\ 725\ 405\ 104\ 263\ 736\ 625\ 168\ 384\ q^{192} - 48\ 687\ 403\ 563\ 100\ 565\ 745\ 406\ 365\ 302\ 784\ q^{193} +$   
 $86\ 744\ 167\ 089\ 111\ 545\ 378\ 556\ 727\ 322\ 752\ q^{196} - 105\ 057\ 418\ 446\ 920\ 848\ 727\ 861\ 875\ 851\ 642\ q^{197} +$   
 $186\ 098\ 915\ 592\ 551\ 097\ 775\ 453\ 929\ 004\ 800\ q^{200} - 224\ 961\ 024\ 243\ 594\ 293\ 439\ 998\ 373\ 888\ 000\ q^{201} +$   
 $396\ 270\ 585\ 150\ 064\ 390\ 750\ 754\ 014\ 848\ 000\ q^{204} - 478\ 141\ 371\ 948\ 932\ 597\ 445\ 583\ 400\ 583\ 975\ q^{205} +$   
 $837\ 681\ 120\ 945\ 800\ 891\ 528\ 864\ 700\ 874\ 752\ q^{208} - 1\ 008\ 944\ 243\ 488\ 924\ 926\ 781\ 901\ 377\ 536\ 000\ q^{209} +$   
 $1\ 758\ 306\ 141\ 903\ 149\ 724\ 176\ 343\ 005\ 165\ 568\ q^{212} - 2\ 114\ 115\ 506\ 340\ 393\ 417\ 361\ 586\ 612\ 410\ 703\ q^{213} +$   
 $3\ 665\ 429\ 852\ 251\ 110\ 050\ 954\ 237\ 803\ 776\ 000\ q^{216} - 4\ 399\ 727\ 023\ 295\ 523\ 926\ 828\ 375\ 819\ 747\ 328\ q^{217} +$   
 $7\ 590\ 175\ 878\ 929\ 963\ 739\ 700\ 468\ 766\ 054\ 400\ q^{220} - 9\ 095\ 763\ 067\ 156\ 221\ 635\ 467\ 130\ 806\ 944\ 000\ q^{221} +$   
 $15\ 615\ 412\ 027\ 323\ 168\ 914\ 368\ 363\ 699\ 200\ 000\ q^{224} -$   
 $18\ 682\ 983\ 206\ 912\ 292\ 758\ 478\ 168\ 650\ 187\ 000\ q^{225} +$   
 $31\ 923\ 056\ 063\ 148\ 842\ 036\ 766\ 167\ 740\ 268\ 544\ q^{228} -$   
 $38\ 134\ 747\ 767\ 586\ 090\ 724\ 436\ 924\ 140\ 004\ 000\ q^{229} +$   
 $64\ 859\ 912\ 432\ 069\ 455\ 571\ 554\ 766\ 005\ 507\ 584\ q^{232} -$   
 $77\ 363\ 089\ 388\ 943\ 624\ 303\ 142\ 631\ 279\ 394\ 816\ q^{233} +$   
 $130\ 989\ 828\ 235\ 652\ 005\ 143\ 521\ 203\ 577\ 280\ 000\ q^{236} -$   
 $156\ 010\ 094\ 888\ 301\ 480\ 536\ 306\ 458\ 695\ 521\ 877\ q^{237} +$   
 $262\ 998\ 740\ 190\ 003\ 422\ 083\ 903\ 535\ 410\ 790\ 400\ q^{240} -$   
 $312\ 782\ 495\ 823\ 950\ 257\ 950\ 232\ 204\ 357\ 632\ 000\ q^{241} +$   
 $525\ 034\ 092\ 495\ 479\ 989\ 100\ 799\ 377\ 569\ 536\ 000\ q^{244} -$   
 $623\ 541\ 312\ 140\ 383\ 572\ 505\ 839\ 003\ 639\ 807\ 630\ q^{245} +$   
 $1\ 042\ 315\ 972\ 865\ 220\ 487\ 316\ 625\ 330\ 120\ 787\ 968\ q^{248} -$   
 $1\ 236\ 177\ 322\ 751\ 259\ 150\ 473\ 309\ 169\ 856\ 512\ 000\ q^{249} +$   
 $2\ 058\ 008\ 844\ 893\ 949\ 568\ 377\ 740\ 449\ 376\ 741\ 376\ q^{252} -$   
 $2\ 437\ 509\ 871\ 262\ 785\ 082\ 562\ 742\ 751\ 789\ 448\ 753\ q^{253} +$   
 $4\ 041\ 910\ 245\ 296\ 841\ 649\ 131\ 619\ 604\ 791\ 754\ 752\ q^{256} -$   
 $4\ 780\ 982\ 401\ 236\ 996\ 364\ 622\ 847\ 495\ 386\ 824\ 704\ q^{257} +$   
 $7\ 897\ 163\ 983\ 926\ 156\ 984\ 121\ 510\ 088\ 562\ 278\ 400\ q^{260} -$   
 $9\ 329\ 234\ 644\ 723\ 843\ 442\ 136\ 177\ 091\ 163\ 920\ 500\ q^{261} +$   
 $15\ 351\ 547\ 153\ 294\ 714\ 922\ 231\ 399\ 401\ 293\ 312\ 000\ q^{264} -$   
 $18\ 112\ 731\ 382\ 145\ 988\ 049\ 450\ 593\ 467\ 326\ 464\ 000\ q^{265} +$   
 $29\ 694\ 715\ 001\ 269\ 905\ 779\ 217\ 615\ 041\ 573\ 681\ 664\ q^{268} -$   
 $34\ 992\ 903\ 625\ 159\ 269\ 662\ 856\ 037\ 141\ 593\ 912\ 000\ q^{269} +$   
 $57\ 161\ 006\ 881\ 968\ 969\ 259\ 846\ 859\ 691\ 124\ 457\ 472\ q^{272} -$   
 $67\ 279\ 283\ 689\ 860\ 872\ 399\ 465\ 010\ 341\ 521\ 195\ 008\ q^{273} +$   
 $109\ 511\ 625\ 034\ 192\ 179\ 132\ 052\ 510\ 641\ 138\ 688\ 000\ q^{276} -$   
 $128\ 745\ 959\ 241\ 786\ 239\ 083\ 115\ 357\ 629\ 244\ 156\ 016\ q^{277} +$   
 $208\ 835\ 592\ 384\ 080\ 353\ 217\ 306\ 066\ 820\ 671\ 155\ 200\ q^{280} -$   
 $245\ 233\ 967\ 280\ 581\ 613\ 365\ 677\ 197\ 318\ 574\ 080\ 000\ q^{281} +$   
 $396\ 438\ 190\ 958\ 302\ 292\ 346\ 912\ 411\ 084\ 170\ 496\ 000\ q^{284} -$   
 $465\ 012\ 641\ 475\ 750\ 012\ 920\ 378\ 908\ 580\ 805\ 540\ 175\ q^{285} +$   
 $749\ 228\ 629\ 899\ 430\ 341\ 461\ 878\ 542\ 741\ 118\ 961\ 664\ q^{288} -$   
 $877\ 863\ 297\ 674\ 224\ 564\ 728\ 293\ 881\ 862\ 258\ 688\ 248\ q^{289} +$   
 $1\ 409\ 811\ 263\ 459\ 841\ 311\ 193\ 821\ 680\ 786\ 005\ 245\ 952\ q^{292} -$   
 $1\ 650\ 085\ 693\ 867\ 116\ 628\ 056\ 191\ 936\ 222\ 432\ 752\ 500\ q^{293} +$   
 $2\ 641\ 519\ 310\ 056\ 710\ 858\ 427\ 457\ 995\ 084\ 228\ 032\ 000\ q^{296} -$   
 $3\ 088\ 458\ 158\ 909\ 547\ 338\ 291\ 702\ 421\ 165\ 435\ 125\ 760\ q^{297} +$   
 $4\ 928\ 672\ 803\ 506\ 715\ 937\ 101\ 596\ 109\ 904\ 243\ 366\ 400\ q^{300} -$

5 756 644 766 963 220 880 133 867 192 128 195 788 375  $q^{301} +$   
 9 158 524 758 887 023 459 879 507 728 182 969 856 000  $q^{304} -$   
 10 686 248 774 140 501 615 131 835 925 642 005 708 800  $q^{305} +$   
 16 950 213 742 498 165 030 309 709 457 050 611 605 504  $q^{308} -$   
 19 758 035 783 360 331 107 870 886 609 784 186 354 500  $q^{309} +$   
 31 247 308 541 835 707 098 013 425 790 525 769 843 712  $q^{312} -$   
 36 388 008 127 489 251 437 204 883 809 970 096 635 904  $q^{313} +$   
 57 381 305 741 993 790 941 471 044 404 033 341 952 000  $q^{316} -$   
 66 757 668 294 013 526 142 122 226 937 096 752 080 451  $q^{317} +$   
 104 973 621 911 077 290 593 857 013 148 799 400 017 920  $q^{320} -$   
 122 012 329 248 251 908 752 492 137 970 102 407 168 000  $q^{321} +$   
 191 325 331 238 931 341 449 726 260 650 672 777 242 752  $q^{324} -$   
 222 175 575 367 268 418 568 020 984 181 277 394 807 900  $q^{325} +$   
 347 437 713 682 552 115 080 522 536 996 800 253 809 664  $q^{328} -$   
 403 095 893 783 442 622 494 196 797 922 024 415 232 000  $q^{329} +$   
 628 669 506 202 413 596 954 346 025 812 120 240 360 960  $q^{332} -$   
 728 733 007 760 180 320 952 386 926 787 849 482 266 895  $q^{333} +$   
 1 133 539 569 017 465 362 775 613 747 097 158 217 728 000  $q^{336} -$   
 1 312 817 043 322 609 916 465 391 667 913 451 026 055 168  $q^{337} +$   
 2 036 793 049 687 780 460 635 500 560 352 653 852 774 400  $q^{340} -$   
 2 356 907 539 614 979 290 577 935 292 149 042 606 188 625  $q^{341} +$   
 3 647 365 963 524 870 382 677 817 823 848 506 786 240 000  $q^{344} -$   
 4 217 057 809 731 192 168 358 331 997 368 659 353 600 000  $q^{345} +$   
 6 509 678 263 743 402 059 113 426 820 203 381 716 195 328  $q^{348} -$   
 7 520 220 551 651 311 224 415 690 795 940 083 229 388 375  $q^{349} +$   
 11 580 098 572 261 705 195 677 512 756 501 334 690 877 440  $q^{352} -$   
 13 366 885 852 642 560 017 280 631 674 728 011 837 341 696  $q^{353} +$   
 20 533 436 494 782 926 610 921 045 211 828 522 948 608 000  $q^{356} -$   
 23 682 768 631 868 246 738 586 070 763 661 779 830 498 591  $q^{357} +$   
 36 293 688 308 130 586 789 012 176 183 035 983 116 480 000  $q^{360} -$   
 41 827 368 598 461 674 174 896 078 958 617 790 730 240 248  $q^{361} +$   
 63 950 425 607 599 924 276 159 659 728 757 999 328 896 000  $q^{364} -$   
 73 643 951 200 292 980 467 553 718 014 647 596 700 574 125  $q^{365} +$   
 112 336 478 597 212 527 169 793 447 524 004 423 090 356 224  $q^{368} -$   
 129 265 937 191 728 729 560 302 074 988 835 151 716 352 000  $q^{369} +$   
 196 736 423 721 117 896 196 413 377 182 074 676 118 523 904  $q^{372} -$   
 226 215 843 128 289 375 295 760 176 254 125 413 764 786 291  $q^{373} +$   
 343 523 404 003 882 393 619 734 641 002 224 670 078 208 000  $q^{376} -$   
 394 706 872 454 270 675 380 163 115 960 794 561 705 410 560  $q^{377} +$   
 598 075 370 423 985 742 519 602 371 954 820 788 647 065 600  $q^{380} -$   
 686 687 929 187 803 385 598 742 682 931 970 144 465 760 250  $q^{381} +$   
 1 038 253 583 262 493 248 398 492 621 428 453 871 284 224 000  $q^{384} -$   
 1 191 233 687 820 617 851 693 962 107 132 375 308 423 987 200  $q^{385} +$   
 1 797 290 515 073 352 398 951 438 909 244 233 411 412 049 920  $q^{388} -$   
 2 060 661 287 437 243 812 810 068 501 472 781 254 118 704 000  $q^{389} +$   
 3 102 553 955 651 630 688 104 868 788 776 503 403 306 487 040  $q^{392} -$   
 3 554 734 119 840 773 696 665 454 431 081 588 083 000 311 808  $q^{393} +$   
 5 341 030 224 720 860 528 461 811 969 109 896 789 930 688 000  $q^{396} -$   
 6 115 286 330 998 166 665 464 903 219 301 376 311 203 975 297  $q^{397} +$   
 9 169 661 720 342 319 102 294 128 468 092 677 058 473 856 000  $q^{400} -$   
 10 491 883 856 794 463 658 174 403 810 370 558 796 976 128 000  $q^{401} +$   
 15 700 796 595 273 930 688 964 623 439 980 303 790 540 544 000  $q^{404} -$   
 17 952 897 688 182 270 464 623 953 846 556 824 858 843 399 645  $q^{405} +$   
 26 813 112 647 595 007 769 687 009 898 310 102 221 438 262 272  $q^{408} -$   
 30 639 171 240 494 204 011 217 661 546 188 689 862 098 944 000  $q^{409} +$

45 671 640 681 928 318 798 024 795 745 619 576 805 770 455 040  $q^{412}$  -  
 52 155 175 282 182 184 531 597 618 245 573 670 646 263 948 251  $q^{413}$  +  
 77 595 420 308 678 298 029 121 721 264 723 712 694 382 080 000  $q^{416}$  -  
 88 554 758 917 075 203 719 946 001 579 893 120 505 198 510 080  $q^{417}$  +  
 131 501 751 043 635 322 323 017 435 137 959 396 121 196 134 400  $q^{420}$  -  
 149 981 011 837 572 566 355 784 930 148 781 649 558 423 531 500  $q^{421}$  +  
 222 304 599 736 703 084 889 569 776 929 311 984 539 807 296 000  $q^{424}$  -  
 253 387 938 233 282 154 832 661 303 067 145 877 090 296 627 200  $q^{425}$  +  
 374 888 366 738 313 878 849 177 227 652 908 144 587 461 113 344  $q^{428}$  -  
 427 047 247 299 021 023 333 491 797 701 184 189 016 423 347 375  $q^{429}$  +  
 630 676 813 818 468 241 603 106 221 315 348 602 165 005 107 200  $q^{432}$  -  
 717 994 213 490 704 370 074 043 172 583 939 235 023 307 636 736  $q^{433}$  +  
 1 058 467 666 126 468 991 356 194 534 864 941 963 245 348 608 000  $q^{436}$  -  
 1 204 301 842 111 794 583 388 129 632 273 158 162 742 688 650 524  $q^{437}$  +  
 1 772 263 412 316 919 268 451 375 232 893 195 878 213 148 748 800  $q^{440}$  -  
 2 015 269 725 638 691 655 883 951 344 520 696 909 695 922 176 248  $q^{441}$  +  
 2 960 551 970 188 950 069 780 176 114 670 020 093 402 774 784 000  $q^{444}$  -  
 3 364 559 035 226 489 919 323 410 568 642 039 362 715 373 628 500  $q^{445}$  +  
 4 934 286 201 567 974 104 989 857 242 261 661 696 772 088 135 680  $q^{448}$  -  
 5 604 458 781 514 643 653 499 370 068 002 152 908 256 497 664 000  $q^{449}$  +  
 8 205 336 600 278 434 066 418 656 354 078 409 006 058 659 414 016  $q^{452}$  -  
 9 314 571 397 925 486 493 356 355 951 340 121 849 153 020 912 674  $q^{453}$  +  
 13 614 502 760 460 066 261 369 581 542 102 249 042 040 150 016 000  $q^{456}$  -  
 15 446 446 006 262 849 510 755 987 940 708 051 560 414 872 797 184  $q^{457}$  +  
 22 539 958 026 394 545 437 245 257 103 733 011 594 816 518 681 600  $q^{460}$  -  
 25 558 967 911 585 531 136 216 548 111 102 668 665 862 621 394 875  $q^{461}$  +  
 37 235 972 692 729 121 537 676 778 510 179 866 715 658 119 168 000  $q^{464}$  -  
 42 200 673 406 215 055 258 713 394 517 447 355 030 005 150 515 200  $q^{465}$  +  
 61 382 230 580 130 657 749 481 096 058 514 524 713 997 813 942 272  $q^{468}$  -  
 69 529 449 771 746 757 106 361 548 775 375 372 399 428 228 333 125  $q^{469}$  +  
 100 972 897 174 349 211 430 775 088 613 462 591 426 005 142 202 880  $q^{472}$  -  
 114 315 023 272 677 237 631 685 949 446 071 489 423 022 793 916 416  $q^{473}$  +  
 165 752 746 325 607 528 540 563 613 999 151 961 767 319 649 792 000  $q^{476}$  -  
 187 557 504 570 275 687 097 131 078 351 151 423 341 167 179 198 810  $q^{477}$  +  
 271 532 455 560 309 422 479 487 687 600 255 570 979 664 992 460 800  $q^{480}$  -  
 307 095 518 104 268 545 206 239 264 559 528 044 612 945 117 184 000  $q^{481}$  +  
 443 914 120 925 912 075 081 964 764 919 489 090 223 944 652 826 752  $q^{484}$  -  
 501 800 914 555 266 120 105 929 196 121 146 447 217 205 904 851 850  $q^{485}$  +  
 724 274 582 171 773 400 759 330 529 729 696 430 433 523 678 002 688  $q^{488}$  -  
 818 312 477 052 847 131 520 716 402 293 626 921 911 643 262 976 000  $q^{489}$  +  
 1 179 356 894 335 702 895 178 152 340 855 834 538 926 702 369 416 192  $q^{492}$  -  
 1 331 825 262 007 482 943 236 878 165 225 334 729 382 039 990 972 758  $q^{493}$  +  
 1 916 617 343 579 750 796 328 024 247 638 673 095 822 922 280 960 000  $q^{496}$  -  
 2 163 346 360 275 518 848 261 171 169 823 727 355 427 958 897 704 960  $q^{497}$  +  
 3 108 736 853 638 401 360 465 583 520 189 431 139 267 818 588 876 800  $q^{500}$  -  
 3 507 242 339 166 591 134 303 014 361 662 597 969 085 167 816 800 000  $q^{501}$  +  
 5 032 698 547 954 972 554 802 597 252 901 606 057 633 696 956 800 000  $q^{504}$  -  
 5 675 137 338 284 960 026 802 641 724 502 756 137 400 098 276 966 400  $q^{505}$  +  
 8 131 976 352 220 035 300 283 370 741 733 849 177 406 777 163 710 464  $q^{508}$  -  
 9 165 742 171 171 168 739 387 276 510 487 897 115 550 559 589 316 250  $q^{509}$  +  
 13 115 328 233 265 215 421 739 153 954 185 842 241 575 784 811 462 656  $q^{512}$  -  
 14 775 736 704 820 701 821 302 994 169 590 471 206 513 082 809 319 424  $q^{513}$  +  
 21 113 466 094 468 121 638 880 206 779 078 972 873 154 774 333 440 000  $q^{516}$  -  
 23 775 534 981 703 567 483 241 672 343 309 199 525 121 385 637 871 487  $q^{517}$  +  
 33 927 080 189 150 150 560 979 038 439 920 613 558 660 031 183 283 200  $q^{520}$  -

38 187 420 157 589 053 261 401 739 386 113 096 924 645 038 866 432 000  $q^{521} +$   
 54 418 817 702 369 107 283 400 785 857 341 881 480 528 229 367 104 000  $q^{524} -$   
 61 224 923 723 545 642 746 909 926 233 259 022 366 230 167 632 324 975  $q^{525} +$   
 87 131 722 780 936 693 435 797 735 210 610 575 243 008 108 783 861 760  $q^{528} -$   
 97 985 761 131 283 482 657 869 486 938 288 907 966 112 503 095 296 248  $q^{529} +$   
 139 263 347 342 290 182 151 902 393 277 157 810 559 481 110 592 622 592  $q^{532} -$   
 156 542 829 395 986 645 885 356 044 221 651 495 791 434 314 039 015 977  $q^{533} +$   
 222 197 553 174 222 730 650 026 441 158 514 810 827 001 947 497 024 000  $q^{536} -$   
 249 659 112 668 005 989 904 405 775 406 871 038 541 275 988 856 635 392  $q^{537} +$   
 353 909 363 930 771 801 266 519 486 950 363 215 816 475 513 721 036 800  $q^{540} -$   
 397 478 906 963 708 421 672 544 377 173 040 548 779 401 093 310 776 000  $q^{541} +$   
 562 734 373 267 044 907 522 252 422 497 940 481 232 661 278 475 264 000  $q^{544} -$   
 631 744 404 051 187 873 963 834 135 238 328 041 828 811 938 217 984 000  $q^{545} +$   
 893 267 558 447 953 692 634 732 571 261 977 337 178 022 038 378 086 400  $q^{548} -$   
 1 002 391 683 118 703 511 534 568 790 899 502 725 611 798 276 537 050 625  $q^{549} +$   
 1 415 579 871 645 428 933 166 432 306 738 056 501 240 913 745 120 757 760  $q^{552} -$   
 1 587 852 565 911 568 353 811 250 945 065 926 063 261 124 547 381 624 832  $q^{553} +$   
 2 239 596 205 672 876 379 422 908 818 129 758 942 778 135 721 622 464 000  $q^{556} -$   
 2 511 119 369 471 661 604 804 172 816 631 970 214 619 013 053 241 835 454  $q^{557} +$   
 3 537 490 504 045 011 740 866 566 081 543 576 138 657 084 412 244 582 400  $q^{560} -$   
 3 964 757 749 896 016 802 722 144 432 453 051 951 677 959 526 531 072 000  $q^{561} +$   
 5 578 515 053 799 734 073 639 347 607 653 599 323 928 780 699 268 096 000  $q^{564} -$   
 6 249 792 368 062 178 474 171 683 061 724 959 436 762 083 909 433 390 900  $q^{565} +$   
 8 783 085 723 334 459 482 748 833 878 945 565 973 979 252 660 216 767 488  $q^{568} -$   
 9 836 068 435 389 722 649 350 279 825 700 218 535 232 526 987 280 384 000  $q^{569} +$   
 13 806 643 394 696 819 297 958 727 135 460 887 506 740 712 233 100 158 976  $q^{572} -$   
 15 455 810 008 337 095 979 801 543 526 725 042 066 272 250 180 133 251 949  $q^{573} +$   
 21 669 492 002 407 182 064 499 851 714 937 696 145 141 572 918 482 378 752  $q^{576} -$   
 24 248 417 812 346 738 090 749 371 297 825 676 627 989 344 106 646 142 976  $q^{577} +$   
 33 957 524 860 797 787 262 438 231 959 729 133 387 370 269 796 554 342 400  $q^{580} -$   
 37 984 241 436 780 351 668 769 718 841 766 181 981 304 253 383 314 149 375  $q^{581} +$   
 53 132 092 085 759 196 712 889 706 167 949 675 766 259 487 661 285 632 000  $q^{584} -$   
 59 409 898 750 279 489 901 153 213 968 743 433 283 499 978 197 036 236 800  $q^{585} +$   
 83 007 665 183 720 071 423 384 315 869 979 204 779 693 196 472 814 383 616  $q^{588} -$   
 92 780 400 079 645 625 623 325 899 331 220 178 083 582 204 138 789 097 875  $q^{589} +$   
 129 487 115 734 359 648 745 653 460 323 797 366 873 889 494 379 780 489 216  $q^{592} -$   
 144 677 968 010 486 615 337 328 464 166 116 971 054 889 174 278 325 338 112  $q^{593} +$   
 201 691 950 651 096 322 339 240 779 170 089 712 172 618 249 482 499 840 000  $q^{596} -$   
 225 270 247 435 082 396 609 238 757 868 864 950 785 219 050 755 489 522 230  $q^{597} +$   
 313 697 233 262 214 471 438 920 101 367 869 491 817 960 758 904 372 262 400  $q^{600} -$   
 350 240 999 579 480 552 917 316 283 973 402 615 282 631 072 146 477 056 000  $q^{601} +$   
 487 191 025 404 186 866 253 161 407 211 474 000 454 085 965 271 889 664 000  $q^{604} -$   
 543 748 626 506 858 226 239 157 736 343 096 874 669 034 034 722 007 818 620  $q^{605} +$   
 755 545 444 061 102 806 382 165 905 138 496 783 298 702 344 862 473 367 552  $q^{608} -$   
 842 953 521 716 310 460 003 483 867 496 149 165 062 872 417 992 753 152 000  $q^{609} +$   
 1 170 040 170 017 229 756 203 457 284 142 907 310 560 703 551 644 167 356 416  $q^{612} -$   
 1 304 936 794 931 378 397 859 972 854 796 010 875 452 244 963 460 286 579 303  $q^{613} +$   
 1 809 363 695 978 526 587 525 030 913 461 061 111 877 656 091 048 067 328 000  $q^{616} -$   
 2 017 259 364 588 328 172 825 119 741 333 118 132 058 224 482 185 388 720 128  $q^{617} +$   
 2 794 099 337 283 452 284 675 105 214 743 247 247 251 389 604 603 870 668 800  $q^{620} -$   
 3 114 055 487 001 697 984 116 640 127 574 815 635 154 522 289 046 157 327 250  $q^{621} +$   
 4 308 782 169 133 303 290 140 301 937 289 739 283 000 785 956 364 761 088 000  $q^{624} -$   
 4 800 529 344 979 696 756 943 341 988 400 458 760 327 154 970 225 107 403 000  $q^{625} +$   
 6 635 439 969 819 848 661 484 520 013 581 475 299 956 160 373 872 230 520 832  $q^{628} -$   
 7 390 193 782 950 497 273 469 880 925 724 215 617 309 391 812 918 109 863 125  $q^{629} +$

10 204 531 504 194 577 024 177 970 105 976 327 533 467 123 175 853 185 034 240  $q^{632}$  -  
 11 361 406 234 030 927 001 390 077 633 794 135 515 653 937 847 358 856 134 656  $q^{633}$  +  
 15 672 207 027 979 182 646 330 546 440 216 963 854 912 617 204 050 704 640 000  $q^{636}$  -  
 17 443 092 163 419 904 144 750 709 833 980 780 023 179 149 385 047 769 764 441  $q^{637}$  +  
 24 037 344 461 991 202 085 473 814 044 975 127 421 845 349 350 071 794 892 800  $q^{640}$  -  
 26 744 560 199 752 993 090 466 654 590 443 541 028 662 161 080 874 725 376 000  $q^{641}$  +  
 36 818 616 179 655 858 355 390 489 648 512 962 173 639 134 704 106 037 248 000  $q^{644}$  -  
 40 951 841 189 197 141 543 695 719 859 967 442 070 407 161 808 993 879 023 925  $q^{645}$  +  
 56 322 044 272 582 846 105 383 361 134 459 913 758 999 288 140 742 732 723 456  $q^{648}$  -  
 62 624 272 872 991 815 354 829 741 928 079 977 881 090 022 833 510 797 312 000  $q^{649}$  +  
 86 044 789 299 811 266 915 743 689 454 453 652 011 851 565 423 296 801 171 968  $q^{652}$  -  
 95 641 961 991 307 659 207 514 179 408 025 701 371 778 493 338 716 544 259 803  $q^{653}$  +  
 131 283 795 321 124 518 159 995 805 021 154 922 300 361 425 873 381 130 240 000  $q^{656}$  -  
 145 880 054 792 835 755 272 467 153 371 644 516 072 656 781 226 050 963 537 920  $q^{657}$  +  
 200 052 111 392 207 189 805 613 102 715 637 444 864 931 006 549 164 120 268 800  $q^{660}$  -  
 222 223 552 728 440 987 846 083 290 613 014 120 124 760 780 383 819 796 697 000  $q^{661}$  +  
 304 456 768 040 182 691 778 191 323 353 960 253 960 982 387 490 888 700 608 000  $q^{664}$  -  
 338 092 839 688 466 058 204 867 225 367 320 448 692 978 311 037 726 076 108 800  $q^{665}$  +  
 462 768 232 045 552 986 977 983 760 254 673 402 766 773 828 377 956 012 963 840  $q^{668}$  -  
 513 734 218 140 003 969 544 915 866 803 044 992 912 439 384 621 848 670 837 875  $q^{669}$  +  
 702 524 890 253 303 453 388 601 878 406 598 636 082 651 513 290 322 727 936 000  $q^{672}$  -  
 779 655 039 787 290 503 920 757 433 796 258 376 533 685 178 840 785 875 599 360  $q^{673}$  +  
 1 065 184 786 546 364 181 829 128 685 952 886 436 727 161 194 320 952 041 498 752  $q^{676}$  -  
 1 181 769 385 615 338 290 285 414 052 763 920 939 185 052 884 940 197 956 132 746  $q^{677}$  +  
 1 613 087 679 543 414 672 733 907 540 943 772 121 584 697 500 287 906 856 166 400  $q^{680}$  -  
 1 789 097 168 534 106 313 786 224 330 390 572 663 128 816 012 497 213 706 240 000  $q^{681}$  +  
 2 439 862 895 947 615 539 190 408 573 944 751 699 916 869 128 387 545 847 360 000  $q^{684}$  -  
 2 705 270 536 867 566 422 789 527 670 628 369 016 893 786 176 707 466 163 598 050  $q^{685}$  +  
 3 685 970 728 669 438 476 094 229 141 832 216 622 645 570 095 426 710 891 311 104  $q^{688}$  -  
 4 085 710 803 688 369 710 980 630 875 907 876 967 783 185 655 911 289 937 920 000  $q^{689}$  +  
 5 561 883 247 460 891 251 101 069 215 318 359 209 533 153 554 043 560 751 216 640  $q^{692}$  -  
 6 163 241 545 336 254 575 410 372 742 315 958 752 561 997 669 211 782 705 106 911  $q^{693}$  +  
 8 382 621 006 992 522 950 984 910 061 172 954 336 414 404 118 531 911 741 312 000  $q^{696}$  -  
 9 286 238 512 737 235 854 559 131 931 820 190 835 084 559 170 298 017 511 964 672  $q^{697}$  +  
 12 619 151 631 936 408 348 762 530 675 629 217 803 582 043 992 152 956 766 566 400  $q^{700}$  -  
 13 975 389 825 126 268 229 707 944 318 851 817 133 492 894 158 425 752 430 541 000  $q^{701}$  +  
 18 974 798 611 770 153 088 790 354 751 906 616 380 214 831 866 501 040 951 296 000  $q^{704}$  -  
 21 008 052 202 084 037 303 611 379 597 185 947 983 931 324 863 460 180 851 097 600  $q^{705}$  +  
 28 498 706 191 349 510 731 904 854 487 342 064 949 075 975 728 298 883 760 275 456  $q^{708}$  -  
 31 543 483 573 336 768 489 607 408 164 809 949 756 500 159 810 044 667 907 591 125  $q^{709}$  +  
 42 754 149 229 989 786 760 105 746 469 685 422 333 630 776 504 617 613 476 401 152  $q^{712}$  -  
 47 308 558 760 196 629 120 278 055 931 971 101 712 710 379 478 831 221 979 414 528  $q^{713}$  +  
 64 067 930 309 810 511 151 945 159 921 619 266 861 125 406 245 392 930 397 504 000  $q^{716}$  -  
 70 872 884 611 847 669 664 444 974 857 185 685 454 234 932 534 926 284 032 266 034  $q^{717}$  +  
 95 899 536 565 601 531 537 691 867 875 292 717 526 827 719 755 763 611 004 190 720  $q^{720}$  -  
 106 055 916 765 500 166 300 072 222 683 961 921 742 622 517 531 962 901 184 512 000  $q^{721}$  +  
 143 386 987 810 426 430 384 917 670 048 512 962 695 715 050 153 584 945 673 472 000  $q^{724}$  -  
 158 528 778 567 596 939 575 964 355 470 782 319 058 988 400 820 784 056 268 578 600  $q^{725}$  +  
 214 153 101 694 671 323 970 943 823 881 271 010 469 987 824 215 238 116 907 389 952  $q^{728}$  -  
 236 702 968 427 070 897 144 608 357 298 879 153 550 872 141 371 711 697 264 640 248  $q^{729}$  +  
 319 495 180 935 242 631 708 116 729 951 407 084 953 067 920 139 760 451 713 316 864  $q^{732}$  -  
 353 041 356 093 566 164 230 233 192 346 629 018 468 698 804 594 907 128 315 559 784  $q^{733}$  +  
 476 138 652 235 203 124 960 735 747 498 040 837 287 893 571 015 031 418 461 184 000  $q^{736}$  -  
 525 990 139 914 733 538 675 602 871 793 714 981 259 604 242 716 889 925 939 527 680  $q^{737}$  +  
 708 819 347 907 121 631 826 639 068 190 957 279 092 089 250 068 179 894 426 009 600  $q^{740}$  -

782 822 983 826 066 356 267 730 172 235 203 506 561 091 282 122 591 775 851 636 250 q<sup>741</sup> +  
1 054 082 132 631 193 822 663 593 525 165 573 818 883 767 348 304 111 432 365 696 000 q<sup>744</sup> -  
1 163 823 787 245 554 345 488 745 966 893 412 944 838 129 799 295 801 328 389 324 800 q<sup>745</sup> +  
1 565 863 197 644 635 904 606 466 600 264 725 764 818 876 273 076 180 838 620 812 288 q<sup>748</sup> -  
1 728 431 960 891 636 783 319 960 518 483 973 289 394 205 701 437 045 083 005 215 500 q<sup>749</sup> +  
2 323 685 369 855 249 360 214 934 288 665 971 056 612 233 296 221 986 078 576 377 856 q<sup>752</sup> -  
2 564 262 003 606 690 077 483 473 690 416 406 014 422 167 157 682 454 596 028 825 600 q<sup>753</sup> +  
3 444 677 652 683 602 165 891 479 366 952 519 242 686 422 942 024 308 549 924 864 000 q<sup>756</sup> -  
3 800 328 685 839 493 370 818 697 567 912 401 792 719 573 790 644 612 744 916 953 843 q<sup>757</sup> +  
5 101 186 212 763 466 953 734 092 929 712 586 243 239 027 112 770 758 682 365 056 000 q<sup>760</sup> -  
5 626 419 803 245 427 751 841 247 556 970 338 979 633 900 301 540 229 975 564 288 000 q<sup>761</sup> +  
7 546 552 787 390 583 847 398 643 160 479 863 199 541 283 087 361 267 485 872 640 000 q<sup>764</sup> -  
8 321 446 525 544 801 887 951 571 457 563 408 153 623 697 895 671 984 895 358 489 875 q<sup>765</sup> +  
11 152 811 818 122 308 208 532 593 831 475 047 003 387 066 723 664 059 175 116 472 320 q<sup>768</sup> -  
12 294 891 639 046 437 307 254 676 906 032 232 053 343 290 361 410 518 694 285 312 000 q<sup>769</sup> +  
16 465 764 074 005 411 472 182 976 307 250 716 538 048 679 589 574 275 573 644 476 416 q<sup>772</sup> -  
18 147 348 890 385 500 908 669 279 270 258 862 128 828 289 398 942 199 686 328 697 393 q<sup>773</sup> +  
24 285 359 840 046 874 307 333 794 780 708 180 157 560 777 662 852 899 837 275 008 000 q<sup>776</sup> -  
26 758 862 773 178 122 629 253 550 806 405 367 719 752 922 169 330 980 443 239 350 272 q<sup>777</sup> +  
35 782 912 033 198 726 847 707 318 602 547 423 940 905 575 397 336 061 335 606 528 000 q<sup>780</sup> -  
39 417 713 493 447 452 011 618 091 821 334 613 808 234 067 342 948 455 871 260 756 875 q<sup>781</sup> +  
52 671 853 667 885 914 867 910 671 066 200 778 310 535 281 351 124 914 119 528 778 752 q<sup>784</sup> -  
58 007 988 646 693 342 567 883 677 319 062 394 035 279 248 975 422 078 411 125 555 200 q<sup>785</sup> +  
77 456 267 821 645 758 853 947 470 508 061 106 253 515 339 939 746 546 742 437 103 616 q<sup>788</sup> -  
85 282 522 275 737 562 309 890 686 079 384 260 957 694 616 600 580 026 491 911 094 000 q<sup>789</sup> +  
113 792 277 872 504 634 800 360 567 625 006 462 945 062 343 234 258 254 450 804 436 480 q<sup>792</sup> -  
125 259 687 377 600 301 982 138 719 890 715 517 293 883 455 307 746 131 647 261 507 584 q<sup>793</sup> +  
167 013 067 269 876 134 552 474 569 797 878 049 583 186 419 556 559 978 182 483 200 000 q<sup>796</sup> -  
183 799 715 733 376 364 748 745 486 910 454 454 800 089 317 616 526 730 348 138 596 699 q<sup>797</sup> +  
244 890 922 461 587 172 862 523 939 836 752 610 295 268 541 222 583 178 926 343 628 800 q<sup>800</sup> -  
269 441 011 071 146 495 800 454 976 786 498 540 270 691 678 792 213 837 866 356 736 000 q<sup>801</sup> +  
358 742 305 126 004 894 915 264 012 045 979 642 493 326 497 077 936 850 198 255 616 000 q<sup>804</sup> -  
394 612 651 100 862 217 048 436 293 223 027 575 842 233 322 288 257 838 720 640 608 750 q<sup>805</sup> +  
525 028 929 200 240 425 455 429 644 687 530 402 364 318 837 206 881 380 070 103 620 096 q<sup>808</sup> -  
577 390 721 336 153 680 370 772 500 540 927 900 825 576 379 678 377 261 915 258 880 000 q<sup>809</sup> +  
767 675 406 126 968 144 839 243 857 770 211 188 086 543 015 452 610 145 067 635 066 880 q<sup>812</sup> -  
844 040 139 427 675 067 155 078 771 455 883 307 832 080 132 016 285 066 495 127 706 055 q<sup>813</sup> +  
1 121 421 195 990 054 157 847 874 852 369 338 181 808 734 040 075 711 155 078 233 088 000 q<sup>816</sup> -  
1 232 690 021 910 783 913 287 410 099 953 873 951 027 382 808 296 435 437 253 521 932 288 q<sup>817</sup> +  
1 636 664 195 081 194 825 881 917 026 492 037 870 157 984 491 509 779 482 926 386 585 600 q<sup>820</sup> -  
1 798 643 448 930 792 254 293 637 362 553 170 396 821 080 663 332 651 620 543 038 889 750 q<sup>821</sup> +  
2 386 453 649 028 193 408 510 540 207 206 802 831 861 681 146 572 163 943 072 749 696 000 q<sup>824</sup> -  
2 622 041 756 465 999 285 762 976 237 940 256 531 371 756 849 987 927 302 516 135 526 400 q<sup>825</sup> +  
3 476 577 415 237 079 665 037 311 438 711 256 810 272 041 425 804 705 718 074 540 587 008 q<sup>828</sup> -  
3 818 917 881 032 579 041 051 554 855 992 069 325 240 994 455 073 781 734 339 430 451 375 q<sup>829</sup> +  
5 060 100 322 042 020 880 584 084 452 114 777 332 269 434 611 470 205 870 148 980 703 232 q<sup>832</sup> -  
5 557 123 687 662 207 988 611 488 252 339 433 290 289 203 562 905 525 058 949 158 371 328 q<sup>833</sup> +  
7 358 299 845 140 520 276 878 918 777 804 875 923 600 003 186 350 773 990 290 327 552 000 q<sup>836</sup> -  
8 079 260 934 289 078 026 377 766 169 629 259 304 800 517 536 579 594 610 394 645 065 289 q<sup>837</sup> +  
10 690 788 589 110 547 997 893 997 720 644 630 585 292 875 903 025 778 046 442 794 752 000 q<sup>840</sup> -  
11 735 667 640 514 746 093 623 387 207 100 987 331 613 173 560 937 400 936 168 898 560 248 q<sup>841</sup> +  
15 518 818 407 968 441 629 728 571 073 424 990 487 945 450 814 687 494 535 780 244 672 000 q<sup>844</sup> -  
17 031 829 409 944 739 689 363 679 975 063 381 373 519 366 947 751 245 932 973 448 887 805 q<sup>845</sup> +  
22 507 482 495 552 509 162 875 502 175 132 458 814 573 346 616 607 411 181 226 545 594 368 q<sup>848</sup> -  
24 696 466 954 056 548 672 143 060 521 336 892 395 151 815 228 548 749 273 854 947 328 000 q<sup>849</sup> +

32 614 988 469 920 269 650 921 645 114 509 036 769 298 531 589 936 411 771 990 726 959 104  $q^{852}$  -  
 35 779 235 839 871 304 230 464 218 333 426 504 602 423 620 049 645 380 409 679 609 204 240  $q^{853}$  +  
 47 220 678 542 530 473 257 955 322 291 738 652 822 028 690 813 946 333 116 271 537 728 000  $q^{856}$  -  
 51 790 802 015 111 835 735 791 004 781 756 160 586 063 285 231 583 765 955 363 442 130 944  $q^{857}$  +  
 68 308 464 016 164 071 058 805 771 449 017 044 195 169 670 322 206 730 622 090 962 483 200  $q^{860}$  -  
 74 903 509 035 625 270 221 796 211 473 727 832 617 977 881 622 419 188 911 377 984 352 500  $q^{861}$  +  
 98 729 447 120 339 057 820 734 068 419 292 096 279 024 876 556 894 028 844 553 926 656 000  $q^{864}$  -  
 108 238 613 783 536 724 513 405 701 484 661 180 734 837 778 702 305 675 476 464 952 934 400  $q^{865}$  +  
 142 577 611 548 343 801 861 383 433 785 610 469 172 537 418 777 939 016 768 761 446 039 552  $q^{868}$  -  
 156 277 105 582 395 952 620 591 771 752 598 499 541 791 359 734 598 272 437 392 512 125 875  $q^{869}$  +  
 205 726 831 585 868 695 320 142 044 171 917 365 686 662 704 245 091 491 138 303 234 473 472  $q^{872}$  -  
 225 446 810 713 299 163 424 692 870 995 723 412 480 121 605 770 280 738 080 401 481 695 232  $q^{873}$  +  
 296 597 858 087 214 460 741 284 707 362 927 995 453 844 850 615 950 050 201 488 640 768 000  $q^{876}$  -  
 324 960 761 251 131 968 162 929 382 407 952 686 651 441 747 141 495 729 449 655 239 307 518  $q^{877}$  +  
 427 252 904 373 228 289 648 447 950 703 896 225 674 948 928 110 131 352 636 886 027 878 400  $q^{880}$  -  
 468 013 417 876 166 588 617 578 967 187 898 656 926 300 508 251 535 143 565 867 950 080 000  $q^{881}$  +  
 614 956 532 449 688 242 810 631 503 734 074 815 089 540 056 132 888 239 187 057 700 864 000  $q^{884}$  -  
 673 486 157 517 138 356 459 972 657 163 260 312 436 577 513 652 974 937 603 981 378 556 225  $q^{885}$  +  
 884 399 750 864 063 436 571 288 874 539 782 302 982 449 802 442 168 746 402 239 923 805 184  $q^{888}$  -  
 968 376 941 090 719 489 662 889 933 637 641 472 102 879 758 244 004 826 213 247 139 840 000  $q^{889}$  +  
 1 270 866 664 493 574 064 139 278 282 033 440 244 414 967 653 159 420 809 379 555 223 248 896  $q^{892}$  -  
 1 391 258 984 519 976 951 022 685 707 908 187 393 388 407 757 637 874 702 033 096 739 390 226  $q^{893}$  +  
 1 824 739 652 021 600 873 578 167 098 790 206 571 742 517 236 461 704 777 337 863 577 600 000  $q^{896}$  -  
 1 997 200 450 562 636 510 581 071 575 177 431 695 158 600 157 216 874 570 705 212 723 560 448  $q^{897}$  +  
 2 617 903 961 323 250 542 560 287 670 942 050 408 385 585 766 803 840 964 691 110 987 344 000  $q^{900}$  -  
 2 864 756 989 716 043 222 444 319 871 799 889 600 255 444 901 253 475 126 719 713 174 603 000  $q^{901}$  +  
 3 752 845 618 588 846 658 146 221 096 575 443 704 563 251 580 813 054 485 064 654 429 952 000  $q^{904}$  -  
 4 105 902 964 156 284 861 784 951 543 066 524 771 922 476 537 971 305 159 306 832 034 201 600  $q^{905}$  +  
 5 375 565 516 471 544 204 370 175 009 183 309 640 967 108 137 343 378 142 012 962 381 910 528  $q^{908}$  -  
 5 880 125 741 674 644 660 306 981 790 617 508 729 467 539 831 246 287 233 725 982 788 143 500  $q^{909}$  +  
 7 693 896 664 548 603 472 045 097 018 065 406 324 447 182 462 745 202 321 961 805 252 788 224  $q^{912}$  -  
 8 414 413 210 012 257 791 593 578 482 759 942 779 674 775 641 467 783 315 556 833 976 483 840  $q^{913}$  +  
 11 003 465 900 444 534 690 384 062 848 198 526 850 914 814 838 932 107 487 132 749 012 224 000  $q^{916}$  -  
 12 031 577 560 429 037 866 970 289 673 557 755 493 510 192 927 438 919 626 538 774 913 619 768  $q^{917}$  +  
 15 724 463 152 292 124 813 964 860 582 338 144 997 091 751 429 966 280 411 800 557 376 486 400  $q^{920}$  -  
 17 190 362 533 498 773 617 011 373 085 800 907 853 646 245 084 113 734 751 417 667 768 320 000  $q^{921}$  +  
 22 453 679 027 131 669 292 332 887 847 454 652 873 195 237 494 572 232 680 222 810 315 264 000  $q^{924}$  -  
 24 542 194 686 071 794 774 639 806 503 068 906 256 168 349 747 965 291 556 623 682 160 174 875  $q^{925}$  +  
 32 038 097 061 017 111 577 517 062 833 262 866 294 484 774 580 470 954 161 548 130 726 940 672  $q^{928}$  -  
 35 011 427 187 632 534 180 254 756 479 093 567 412 077 431 272 744 662 322 282 206 302 208 000  $q^{929}$  +  
 45 678 893 325 722 126 321 926 401 688 628 333 516 409 295 683 592 699 400 715 682 685 632 512  $q^{932}$  -  
 49 908 718 806 337 493 832 229 995 367 573 957 282 038 850 201 177 986 571 963 353 889 042 119  $q^{933}$  +  
 65 078 301 325 196 955 632 630 742 812 491 315 101 112 698 616 897 001 492 199 268 297 920 000  $q^{936}$  -  
 71 091 115 303 023 605 635 667 355 895 322 402 166 786 211 278 841 177 410 648 721 958 141 952  $q^{937}$  +  
 92 646 861 249 902 776 517 672 924 780 663 911 731 191 259 393 267 153 615 499 933 950 796 800  $q^{940}$  -  
 101 187 908 900 670 879 241 435 499 392 511 145 153 470 798 958 152 098 862 870 470 880 837 625  $q^{941}$  +  
 131 795 672 703 130 196 490 135 408 478 823 863 522 428 800 047 344 584 883 828 873 607 680 000  $q^{944}$  -  
 143 919 077 728 098 559 283 926 046 534 238 180 382 273 075 618 313 691 553 596 100 175 462 400  $q^{945}$  +  
 187 348 223 507 469 069 419 345 551 536 022 337 512 075 331 640 122 086 194 153 950 356 451 328  $q^{948}$  -  
 204 543 936 618 695 961 165 103 895 645 114 581 445 470 154 412 429 425 865 479 492 057 186 250  $q^{949}$  +  
 266 120 311 379 193 691 415 301 392 611 753 496 662 890 608 556 776 538 694 510 604 864 120 832  $q^{952}$  -  
 290 492 799 441 610 119 243 159 953 183 663 015 160 203 964 044 452 646 517 112 720 190 472 192  $q^{953}$  +  
 377 736 096 849 218 811 835 163 604 468 076 819 759 400 067 339 541 265 531 304 946 610 688 000  $q^{956}$  -  
 412 255 685 580 567 935 777 814 579 020 735 958 268 679 641 947 227 257 540 521 978 953 361 852  $q^{957}$  +  
 535 775 637 217 196 215 007 382 560 924 286 184 252 166 952 130 416 399 091 873 605 743 411 200  $q^{960}$  -

584 631 803 123 052 684 945 760 397 013 221 962 698 427 288 945 741 524 950 338 257 715 200 248  $q^{961} +$   
 759 387 435 323 705 548 448 322 448 089 211 832 812 798 837 118 336 561 063 319 917 697 024 000  $q^{964} -$   
 828 485 057 788 951 652 694 511 656 363 336 393 518 878 174 248 670 931 685 292 182 813 207 675  $q^{965} +$   
 1 075 552 886 249 625 290 737 424 779 143 852 410 110 683 388 883 651 739 009 614 063 444 564 736  $q^{968} -$   
 1 173 208 832 318 752 038 798 505 909 626 030 101 419 319 114 716 393 842 619 196 491 882 496 000  $q^{969} +$   
 1 522 263 993 409 519 267 388 829 208 725 292 014 688 465 136 590 500 146 988 342 562 465 408 512  $q^{972} -$   
 1 660 184 243 458 631 331 416 308 670 415 449 368 011 377 909 054 374 763 447 531 676 531 826 626  $q^{973} +$   
 2 152 979 660 446 473 236 693 908 622 301 155 341 438 939 285 913 629 899 951 794 312 914 944 000  $q^{976} -$   
 2 347 629 033 444 880 935 236 278 928 745 034 709 387 057 182 055 548 012 947 879 511 620 354 048  $q^{977} +$   
 3 042 870 792 621 637 524 176 218 054 185 166 837 612 484 614 638 969 516 459 304 106 697 185 280  $q^{980} -$   
 3 317 391 724 779 659 582 143 083 214 433 527 788 099 306 160 638 072 236 342 434 967 639 636 250  $q^{981} +$   
 4 297 566 396 973 588 333 797 547 687 360 042 962 911 209 435 616 373 337 234 980 328 766 592 000  $q^{984} -$   
 4 684 465 067 928 976 710 691 933 981 365 128 252 235 689 981 598 996 948 401 998 129 904 025 600  $q^{985} +$   
 6 065 394 112 643 035 072 603 546 922 806 075 852 583 998 120 151 358 122 277 352 987 491 612 672  $q^{988} -$   
 6 610 298 298 583 666 788 946 008 665 045 213 500 818 359 999 868 877 649 700 371 583 440 997 375  $q^{989} +$   
 8 554 500 006 825 516 141 263 720 163 030 100 060 347 844 828 441 771 390 159 643 220 759 724 032  $q^{992} -$   
 9 321 412 798 600 689 826 402 648 393 818 962 024 956 400 568 542 171 087 142 561 790 859 771 904  $q^{993} +$   
 12 056 776 839 609 405 053 486 015 370 097 969 143 975 532 152 562 808 972 223 147 951 069 184 000  
 $q^{996} -$   
 13 135 416 861 561 361 683 581 420 618 178 298 608 546 273 975 584 939 977 385 828 039 345 944 068  
 $q^{997} +$   
 16 981 286 630 453 755 651 997 267 867 542 689 200 760 606 560 645 603 401 049 935 819 434 624 000  
 $q^{1000} -$   
 18 497 336 726 881 443 475 829 220 098 146 187 409 690 839 476 488 378 940 785 924 863 729 664 000  
 $q^{1001} +$   
 23 900 914 351 243 377 546 923 902 822 212 056 178 523 526 258 750 153 043 390 503 952 355 008 000  
 $q^{1004} -$   
 26 030 321 915 509 069 322 095 409 533 524 958 294 521 622 354 547 725 818 813 137 466 890 115 775  
 $q^{1005} +$   
 33 617 448 528 489 051 606 908 473 055 516 195 109 562 556 287 235 244 312 353 380 929 050 099 712  
 $q^{1008} -$   
 36 606 366 374 493 883 207 491 117 164 430 921 526 285 531 841 356 844 845 415 254 189 953 024 000  
 $q^{1009} +$   
 47 252 308 555 553 452 589 247 401 094 379 223 668 900 382 695 447 316 340 726 480 846 321 831 936  
 $q^{1012} -$   
 51 444 883 356 497 060 917 286 162 117 303 660 454 129 357 111 407 709 513 913 722 425 077 276 242  
 $q^{1013} +$   
 66 372 944 700 992 174 490 528 366 863 520 648 889 577 864 080 745 866 991 611 248 602 439 168 000  
 $q^{1016} -$   
 72 250 016 697 565 777 095 575 238 661 220 684 225 744 051 023 101 458 243 914 417 273 161 842 688  
 $q^{1017} +$   
 93 168 825 010 930 689 890 132 704 270 769 336 684 157 563 662 851 472 205 362 521 819 322 368 000  
 $q^{1020} -$   
 101 401 789 253 586 774 057 963 736 031 496 655 300 646 446 140 309 748 119 084 014 737 904 892 375  
 $q^{1021} +$   
 130 696 307 448 284 597 077 493 759 641 792 351 404 634 076 303 260 824 906 440 789 142 970 826 752  
 $q^{1024} -$   
 142 222 029 310 878 147 216 718 537 894 068 083 727 609 967 855 829 811 161 656 494 470 514 278 400  
 $q^{1025} +$   
 183 219 146 676 086 815 502 159 404 561 648 589 395 808 777 872 354 485 486 877 140 161 596 686 336  
 $q^{1028} -$   
 199 344 096 550 873 044 622 681 389 007 373 825 412 871 491 523 379 392 648 084 971 304 806 769 500  
 $q^{1029} +$   
 256 681 690 086 287 753 424 944 469 730 019 210 084 966 059 576 125 684 020 672 508 519 200 350 208  
 $q^{1032} -$

279 226 603 559 027 205 524 354 769 905 504 907 935 825 394 561 907 338 310 301 930 007 267 606 528  
 $q^{1033} +$   
 359 366 061 670 115 511 223 327 817 402 604 299 824 618 206 370 063 825 308 243 432 492 778 752 000  
 $q^{1036} -$   
 390 866 771 983 313 451 351 726 093 784 149 804 125 217 474 535 412 839 095 683 062 153 892 872 137  
 $q^{1037} +$   
 502 804 308 773 411 009 982 340 393 026 977 731 235 697 921 433 957 750 434 449 180 498 755 584 000  
 $q^{1040} -$   
 546 790 392 152 193 281 037 260 766 212 231 901 504 909 348 010 951 607 953 019 381 190 381 568 000  
 $q^{1041} +$   
 703 043 651 316 643 381 307 878 741 033 645 295 112 077 925 231 583 100 437 165 120 655 010 048 000  
 $q^{1044} -$   
 764 424 797 541 511 117 352 964 270 939 730 786 709 950 176 812 123 619 807 266 893 095 491 113 575  
 $q^{1045} +$   
 982 400 453 102 744 478 497 442 191 610 454 195 520 393 791 191 023 993 324 197 370 349 738 398 208  
 $q^{1048} -$   
 1 068 001 882 627 062 492 863 851 209 512 402 249 087 078 425 068 433 910 043 606 788 273 516 544 000  
 $q^{1049} +$   
 1 371 890 217 096 129 561 707 257 796 210 825 737 714 492 448 202 577 814 728 445 704 426 219 100 160  
 $q^{1052} -$   
 1 491 194 192 522 077 665 348 409 999 953 754 466 926 466 375 012 700 577 139 223 646 843 791 459 948  
 $q^{1053} +$   
 1 914 592 130 819 184 347 699 117 037 025 870 394 134 458 585 398 694 735 780 609 334 343 503 872 000  
 $q^{1056} -$   
 2 080 764 275 942 099 974 831 079 123 061 254 209 370 795 979 960 901 398 560 937 823 055 655 075 840  
 $q^{1057} +$   
 2 670 304 786 180 290 474 012 157 459 015 812 529 623 966 015 143 353 398 135 746 669 002 469 376 000  
 $q^{1060} -$   
 2 901 613 755 454 128 506 840 798 533 364 982 473 990 932 106 697 550 604 021 635 027 584 261 595 500  
 $q^{1061} +$   
 3 721 984 731 601 497 541 211 107 364 132 923 894 096 654 047 788 771 436 673 964 726 028 887 424 000  
 $q^{1064} -$   
 4 043 764 819 570 306 307 799 357 059 744 647 377 225 024 843 540 380 484 093 059 928 868 247 961 600  
 $q^{1065} +$   
 5 184 645 282 679 331 749 559 189 461 710 480 265 095 151 355 991 530 936 791 894 970 492 144 784 384  
 $q^{1068} -$   
 5 632 008 012 192 503 706 435 562 396 012 060 826 982 325 482 615 893 247 296 432 965 087 561 248 750  
 $q^{1069} +$   
 7 217 648 436 174 909 182 668 414 926 869 675 460 031 144 153 151 928 909 325 806 712 267 621 330 944  
 $q^{1072} -$   
 7 839 226 751 387 103 185 044 658 732 400 054 375 375 616 409 373 302 287 343 861 771 888 368 877 568  
 $q^{1073} +$   
 10 041 673 714 379 077 207 913 008 931 532 358 843 403 184 628 618 602 883 800 931 154 706 915 072 000  
 $q^{1076} -$   
 10 904 788 984 217 491 348 411 201 624 045 503 710 826 298 691 162 313 995 343 759 629 740 019 519 055  
 $q^{1077} +$   
 13 962 129 793 715 616 876 893 056 840 642 095 769 062 121 228 800 645 426 805 746 351 901 966 233 600  
 $q^{1080} -$   
 15 159 918 154 633 026 534 152 974 530 691 278 612 053 385 321 619 407 665 115 838 411 617 386 496 000  
 $q^{1081} +$   
 19 401 436 396 493 110 872 579 417 632 900 210 693 106 815 672 311 065 437 627 048 261 786 030 592 000  
 $q^{1084} -$   
 21 062 671 737 133 865 584 624 001 086 729 973 920 270 492 830 066 966 893 830 024 367 501 135 265 375  
 $q^{1085} +$   
 26 943 511 554 403 893 609 672 273 566 681 816 513 219 273 517 319 127 019 802 453 980 177 025 204 224

$q^{1088} -$   
 29 246 137 777 586 341 144 579 706 590 669 788 649 155 365 884 156 054 276 591 816 385 785 348 096 248  
 $q^{1089} +$   
 37 395 043 760 325 827 791 757 614 433 751 482 379 190 047 739 986 599 929 917 245 788 958 448 058 368  
 $q^{1092} -$   
 40 584 806 327 313 638 242 865 100 981 974 289 561 925 654 747 119 655 800 557 363 457 739 238 112 900  
 $q^{1093} +$   
 51 869 833 725 679 185 578 438 701 016 899 293 462 180 136 760 762 131 592 334 520 521 177 296 256 000  
 $q^{1096} -$   
 56 285 917 421 883 207 211 658 718 679 378 434 337 916 434 546 255 212 037 274 830 867 988 661 043 200  
 $q^{1097} +$   
 71 904 825 790 007 265 093 736 355 880 596 036 141 365 001 163 646 119 327 748 009 982 796 342 489 600  
 $q^{1100} -$   
 78 015 113 375 857 765 815 045 023 834 065 304 141 835 403 107 213 624 561 950 856 959 627 139 595 500  
 $q^{1101} +$   
 99 619 645 583 150 121 607 906 549 964 146 865 638 383 369 694 411 620 969 175 224 878 324 785 152 000  
 $q^{1104} -$   
 108 069 180 395 039 678 524 312 133 114 826 104 949 898 029 131 273 911 021 639 591 008 873 214 771 200  
 $q^{1105} +$   
 137 935 833 528 875 732 282 689 249 713 196 095 570 516 036 103 300 647 048 546 711 606 408 823 928 832  
 $q^{1108} -$   
 149 613 393 465 680 324 949 012 737 846 652 515 964 792 065 191 614 817 072 997 180 944 036 028 658 375  
 $q^{1109} +$   
 190 877 942 914 351 275 197 836 025 799 621 337 030 499 942 183 706 172 401 386 715 575 644 200 866 304  
 $q^{1112} -$   
 207 007 443 452 030 783 326 855 200 866 472 443 539 987 871 217 870 437 435 103 626 399 079 277 658 112  
 $q^{1113} +$   
 263 986 842 028 335 866 034 521 028 075 463 563 520 512 939 205 621 903 249 685 685 785 172 441 600 000  
 $q^{1116} -$   
 286 252 758 839 853 906 535 043 440 122 627 378 959 076 883 345 307 282 999 885 059 399 421 089 588 251  
 $q^{1117} +$   
 364 886 719 626 773 761 346 402 533 056 511 127 122 715 039 545 045 666 193 083 870 770 085 553 971 200  
 $q^{1120} -$   
 395 606 097 863 267 372 237 989 102 602 467 301 174 125 862 232 462 445 780 844 965 133 673 328 640 000  
 $q^{1121} +$   
 504 062 526 964 530 834 818 300 840 090 314 376 549 582 194 536 294 374 219 638 402 799 128 258 560 000  
 $q^{1124} -$   
 546 420 751 946 601 217 975 473 202 889 038 532 294 610 430 330 689 653 600 323 555 281 844 680 279 450  
 $q^{1125} +$   
 695 925 374 186 784 693 224 096 016 534 782 267 474 874 503 037 220 796 054 811 171 059 406 208 997 376  
 $q^{1128} -$   
 754 299 162 779 117 942 856 827 362 018 032 961 554 820 046 831 866 515 841 386 644 101 417 205 760 000  
 $q^{1129} +$   
 960 271 741 358 410 715 370 161 294 251 523 313 271 622 543 669 437 000 498 557 933 931 210 721 748 480  
 $q^{1132} -$   
 1 040 671 380 361 914 832 760 385 544 861 409 442 869 642 114 159 958 850 915 119 375 296 465 056 089  
 $156 q^{1133} +$   
 1 324 280 992 760 504 271 432 146 165 371 224 660 193 497 475 087 962 801 161 451 856 977 182 078 976  
 $000 q^{1136} -$   
 1 434 955 523 133 853 571 331 737 927 764 160 511 043 051 332 208 465 203 216 723 302 557 000 338 407  
 $424 q^{1137} +$   
 1 825 248 302 573 788 907 694 241 535 394 749 730 691 114 269 841 553 200 128 720 942 902 602 218 700  
 $800 q^{1140} -$   
 1 977 513 243 539 340 633 252 302 725 355 510 697 913 144 916 845 349 251 726 387 709 818 476 543 082  
 $875 q^{1141} +$

2 514 321 740 882 902 028 470 595 071 137 134 508 394 222 743 527 645 316 889 499 105 978 773 558 656 000  $q^{1144}$  -  
 2 723 690 582 398 384 554 652 602 473 023 363 861 182 237 780 399 528 154 586 451 868 089 070 185 676 800  $q^{1145}$  +  
 3 461 609 756 439 234 845 060 735 344 438 943 663 405 920 819 667 047 030 699 219 469 633 858 683 256 832  $q^{1148}$  -  
 3 749 339 879 098 275 954 227 163 990 175 323 275 203 140 853 189 148 809 937 581 298 772 081 417 029 375  $q^{1149}$  +  
 4 763 157 883 331 499 374 804 542 451 686 333 158 598 342 873 250 476 481 246 426 698 728 218 871 644 160  $q^{1152}$  -  
 5 158 361 580 297 656 541 696 457 930 221 542 975 992 585 701 867 984 993 674 362 390 605 700 549 705 728  $q^{1153}$  +  
 6 550 473 739 929 445 768 647 009 067 073 825 872 947 164 056 935 442 311 891 781 034 500 258 185 242 752  $q^{1156}$  -  
 7 092 999 395 117 713 106 517 015 420 794 861 154 483 146 497 250 553 796 474 051 278 761 984 602 576 779  $q^{1157}$  +  
 9 003 524 279 625 260 840 612 662 419 887 437 350 587 748 551 958 856 408 794 941 825 295 546 944 025 600  $q^{1160}$  -  
 9 747 886 618 525 437 569 686 041 806 444 438 508 334 651 385 205 384 330 096 440 951 336 941 731 840 000  $q^{1161}$  +  
 12 368 461 813 819 819 617 155 575 688 732 432 528 790 529 189 599 371 822 920 526 186 376 492 516 096 000  $q^{1164}$  -  
 13 389 200 417 263 578 859 150 225 407 177 327 101 136 595 045 883 607 994 562 367 095 116 317 417 522 525  $q^{1165}$  +  
 16 981 786 715 124 952 452 905 484 042 473 729 179 492 675 245 711 486 850 534 868 172 634 225 120 247 808  $q^{1168}$  -  
 18 380 768 047 604 547 117 491 445 970 866 842 516 427 726 274 734 322 765 012 615 685 393 999 216 640 000  $q^{1169}$  +  
 23 303 267 072 138 619 440 318 256 405 504 975 290 960 650 429 020 965 396 588 516 217 173 800 409 720 832  $q^{1172}$  -  
 25 219 629 804 726 230 366 496 832 839 532 874 015 804 426 562 690 910 370 882 528 081 757 446 772 099 876  $q^{1173}$  +  
 31 960 765 898 248 101 007 621 501 150 556 705 045 190 133 864 964 492 688 651 456 143 989 283 368 512 000  $q^{1176}$  -  
 34 584 459 441 507 615 920 683 076 927 026 376 889 822 577 540 123 342 392 646 966 788 894 881 031 094 272  $q^{1177}$  +  
 43 811 251 819 154 698 273 574 014 904 142 847 362 913 434 741 176 385 103 395 168 742 750 153 561 958 400  $q^{1180}$  -  
 47 401 456 880 959 579 163 127 600 161 174 649 444 924 476 647 793 380 986 631 551 232 155 419 830 319 625  $q^{1181}$  +  
 60 023 793 522 201 516 325 021 983 704 844 561 860 133 808 476 147 738 325 000 190 038 600 363 080 192 000  $q^{1184}$  -  
 64 933 972 441 316 983 622 209 889 385 476 571 382 983 127 588 166 634 912 871 993 748 519 382 505 881 600  $q^{1185}$  +  
 82 192 402 123 358 825 774 915 589 092 631 281 595 284 653 958 829 299 330 987 181 166 315 512 891 899 904  $q^{1188}$  -  
 88 904 347 912 521 534 689 730 011 374 845 782 236 366 703 548 462 409 437 565 876 271 347 713 533 158 625  $q^{1189}$  +  
 112 489 378 572 575 503 069 310 661 713 500 804 382 412 403 574 611 028 853 809 548 504 153 914 380 573 184  $q^{1192}$  -  
 121 659 471 981 908 471 661 338 659 048 356 609 804 317 360 556 419 714 840 086 478 467 247 716 318 740 480  $q^{1193}$  +  
 153 873 600 990 536 827 972 796 297 966 776 053 101 444 446 133 656 248 811 681 567 192 366 229 856 768 000  $q^{1196}$  -  
 166 395 621 265 781 801 805 608 258 631 507 200 243 398 361 164 199 970 776 880 624 811 455 266 008

918 299  $q^{1197}$  +  
 210 373 294 171 343 943 526 068 058 139 027 738 343 798 009 330 896 502 206 692 670 535 093 012 970 0  
 598 400  $q^{1200}$  -  
 227 463 665 035 162 255 012 699 076 084 519 824 107 887 605 931 908 274 889 556 331 010 741 388 689 0  
 408 000  $q^{1201}$  +  
 287 469 724 991 244 860 988 907 532 163 267 306 327 878 563 665 128 000 775 882 614 658 347 830 017 0  
 024 000  $q^{1204}$  -  
 310 783 152 159 646 697 830 037 386 068 976 217 656 160 036 627 000 704 541 569 903 930 086 230 902 0  
 605 750  $q^{1205}$  +  
 392 617 588 917 443 557 001 550 961 573 939 079 072 919 813 410 766 054 839 060 487 982 808 715 707 0  
 796 480  $q^{1208}$  -  
 424 403 846 941 929 701 862 617 240 874 739 507 069 587 925 089 909 554 047 907 353 897 844 334 206 0  
 976 000  $q^{1209}$  +  
 535 950 436 713 447 284 588 198 555 353 599 834 986 219 313 648 989 206 030 400 623 737 454 103 171 0  
 336 192  $q^{1212}$  -  
 579 266 843 831 002 504 251 730 495 788 642 077 953 946 786 466 999 037 318 924 613 385 774 415 657 0  
 718 823  $q^{1213}$  +  
 731 236 470 524 481 027 322 563 756 603 455 051 427 278 460 285 489 573 374 991 507 833 579 077 275 0  
 648 000  $q^{1216}$  -  
 790 235 690 484 654 052 600 057 618 178 662 495 628 059 793 127 741 034 699 747 992 328 776 368 071 0  
 114 752  $q^{1217}$  +  
 997 172 939 733 205 674 957 968 668 442 657 726 658 844 280 603 011 332 204 451 229 429 271 266 367 0  
 897 600  $q^{1220}$  -  
 1 077 492 626 420 684 813 207 437 960 893 437 990 574 868 149 180 199 164 757 953 822 397 029 713 140 0  
 958 000  $q^{1221}$  +  
 1 359 138 239 468 603 670 677 678 980 290 861 424 764 382 228 436 203 622 348 659 354 055 324 965 779 0  
 840 000  $q^{1224}$  -  
 1 468 428 308 007 617 420 095 005 960 503 606 345 839 776 896 016 715 412 643 546 028 278 546 896 853 0  
 860 600  $q^{1225}$  +  
 1 851 562 413 458 576 125 613 674 717 925 882 181 196 614 421 638 336 475 528 831 178 602 063 369 154 0  
 772 480  $q^{1228}$  -  
 2 000 198 205 854 885 216 996 269 259 648 893 779 153 967 814 211 865 635 707 936 831 029 086 694 766 0  
 077 875  $q^{1229}$  +  
 2 521 132 788 566 857 948 902 365 894 446 789 780 410 634 036 249 588 073 851 192 031 429 371 833 866 0  
 846 208  $q^{1232}$  -  
 2 723 179 211 288 387 495 107 534 851 533 605 891 069 047 982 861 747 605 288 270 116 194 559 159 127 0  
 048 192  $q^{1233}$  +  
 3 431 126 889 084 174 625 106 561 438 661 244 474 563 504 137 444 839 501 283 265 202 965 169 968 164 0  
 352 000  $q^{1236}$  -  
 3 705 641 222 104 274 354 640 162 491 153 296 992 507 067 038 198 613 369 675 682 980 965 331 571 191 0  
 128 609  $q^{1237}$  +  
 4 667 266 261 847 301 417 085 673 014 866 416 604 039 281 791 698 584 541 860 536 295 815 542 126 874 0  
 368 000  $q^{1240}$  -  
 5 040 057 769 606 204 423 152 353 179 607 808 984 328 677 996 404 839 771 815 204 051 213 546 021 421 0  
 056 000  $q^{1241}$  +  
 6 345 621 331 618 988 456 640 597 941 931 855 944 007 299 485 361 183 801 678 756 640 940 882 065 267 0  
 456 000  $q^{1244}$  -  
 6 851 626 722 758 926 923 205 149 255 071 351 268 773 445 872 919 935 013 268 589 170 225 323 423 947 0  
 188 350  $q^{1245}$  +  
 8 623 280 890 319 548 479 520 383 307 495 639 806 433 711 405 224 530 463 043 117 026 437 543 975 774 0  
 150 656  $q^{1248}$  -  
 9 309 769 662 679 205 296 625 121 319 394 719 931 498 037 047 922 023 904 731 674 099 307 210 767 958 0  
 016 000  $q^{1249}$  +  
 11 712 746 372 635 193 864 587 586 139 359 801 667 938 025 606 369 571 668 701 605 200 059 768 104 0  
 305 524 736  $q^{1252}$  -

12 643 643 949 689 167 900 786 380 129 360 636 884 711 968 128 062 755 371 551 114 511 453 947 559 115 666 761  $q^{1253} +$   
 15 901 342 209 437 254 186 874 243 246 957 901 172 196 338 872 596 849 356 213 831 453 210 008 209 141 952 000  $q^{1256} -$   
 17 163 057 961 410 398 558 647 892 340 218 268 669 562 158 836 303 178 798 339 969 286 218 716 607 466 733 568  $q^{1257} +$   
 21 577 378 100 582 762 399 784 575 589 245 661 645 308 361 447 037 108 230 941 430 735 779 822 193 271 065 600  $q^{1260} -$   
 23 286 658 464 771 361 087 835 555 912 515 084 040 857 614 099 823 613 555 342 104 459 335 241 199 516 559 000  $q^{1261} +$   
 29 265 395 583 279 528 760 614 306 139 828 138 974 809 705 318 484 926 421 206 053 975 696 187 139 059 712 000  $q^{1264} -$   
 31 579 901 083 150 176 450 087 588 613 459 963 167 882 118 917 180 255 417 633 174 755 063 944 521 267 609 600  $q^{1265} +$   
 39 673 631 393 480 586 580 556 349 480 188 601 801 427 885 223 359 348 857 994 076 153 301 836 971 293 616 128  $q^{1268} -$   
 42 806 175 824 621 001 782 711 826 163 621 162 636 941 222 763 755 266 574 379 814 268 578 157 229 861 613 250  $q^{1269} +$   
 53 757 902 827 384 756 562 883 116 424 608 810 696 361 484 700 366 638 768 494 276 515 373 817 929 846 586 368  $q^{1272} -$   
 57 995 613 843 941 809 875 181 904 771 028 425 738 253 213 361 659 883 034 496 614 988 558 983 288 907 399 168  $q^{1273} +$   
 72 807 557 835 736 427 961 094 080 303 964 105 310 668 367 439 973 812 155 660 758 959 528 634 164 250 368 000  $q^{1276} -$   
 78 537 648 178 517 141 272 811 227 813 706 158 974 525 563 698 258 347 576 680 035 608 648 820 933 774 450 362  $q^{1277} +$   
 98 561 058 143 241 019 838 922 966 300 507 632 053 272 934 698 101 547 719 452 189 136 394 772 069 959 598 080  $q^{1280} -$   
 106 305 472 591 129 767 577 786 577 604 221 026 719 862 534 488 214 095 746 292 717 923 734 980 559 921 152 000  $q^{1281} +$   
 133 361 341 829 512 754 316 521 977 193 943 243 279 818 936 705 183 177 409 768 312 638 026 333 602 072 576 000  $q^{1284} -$   
 143 823 315 748 689 682 473 839 409 893 548 790 647 037 245 918 996 498 655 797 607 181 604 625 552 071 068 375  $q^{1285} +$   
 180 364 562 189 477 895 014 299 122 299 720 741 053 310 187 185 333 100 142 161 187 070 683 661 016 175 847 424  $q^{1288} -$   
 194 491 158 851 021 621 766 056 462 332 086 042 066 764 322 033 261 047 060 941 771 797 455 934 808 952 832 000  $q^{1289} +$   
 243 820 415 391 722 978 099 519 888 122 747 686 442 423 245 462 905 455 018 274 220 487 473 746 903 588 567 040  $q^{1292} -$   
 262 886 488 469 232 793 844 272 398 983 222 985 053 879 985 406 260 570 317 631 344 651 775 006 351 240 969 094  $q^{1293} +$   
 329 448 441 363 181 173 318 010 759 100 930 899 234 911 500 399 145 030 069 386 718 942 445 396 383 797 578 752  $q^{1296} -$   
 355 169 312 801 315 143 832 313 724 082 264 592 780 821 991 642 144 563 714 074 717 793 441 237 696 229 900 288  $q^{1297} +$   
 444 942 931 566 351 457 709 564 962 683 755 590 955 367 011 610 606 118 610 446 406 434 818 399 541 648 742 400  $q^{1300} -$   
 479 625 538 726 228 105 118 098 429 558 283 372 809 173 508 840 004 341 401 953 606 105 114 510 369 588 044 875  $q^{1301} +$   
 600 650 098 340 552 051 938 164 881 095 378 835 731 996 742 451 612 008 848 465 432 465 528 242 018 622 272 000  $q^{1304} -$   
 647 395 655 008 117 490 498 625 672 877 216 762 205 905 765 815 007 351 427 124 402 253 234 868 744 871 936 000  $q^{1305} +$   
 810 475 878 268 097 115 907 873 778 960 703 540 220 122 146 445 984 176 976 760 394 449 190 981 225

$100\ 711\ 936\ q^{1308} -$   
 $873\ 451\ 487\ 456\ 968\ 765\ 543\ 955\ 936\ 887\ 109\ 126\ 142\ 523\ 407\ 617\ 857\ 292\ 688\ 582\ 996\ 976\ 096\ 146\ 164\ 8$   
 $724\ 003\ 000\ q^{1309} +$   
 $1\ 093\ 102\ 388\ 235\ 983\ 671\ 497\ 436\ 866\ 479\ 875\ 688\ 282\ 111\ 881\ 757\ 675\ 941\ 646\ 888\ 763\ 644\ 804\ 255\ 821\ 8$   
 $343\ 809\ 536\ q^{1312} -$   
 $1\ 177\ 904\ 907\ 722\ 297\ 177\ 191\ 291\ 985\ 831\ 941\ 922\ 228\ 869\ 856\ 837\ 488\ 439\ 707\ 600\ 337\ 272\ 544\ 634\ 762\ 8$   
 $222\ 698\ 496\ q^{1313} +$   
 $1\ 473\ 617\ 266\ 701\ 875\ 247\ 473\ 525\ 814\ 324\ 408\ 016\ 053\ 471\ 323\ 776\ 230\ 636\ 423\ 014\ 999\ 285\ 659\ 762\ 986\ 8$   
 $676\ 224\ 000\ q^{1316} -$   
 $1\ 587\ 760\ 549\ 213\ 942\ 871\ 783\ 189\ 233\ 408\ 261\ 635\ 457\ 045\ 568\ 198\ 887\ 154\ 467\ 706\ 087\ 472\ 328\ 462\ 691\ 8$   
 $252\ 453\ 526\ q^{1317} +$   
 $1\ 985\ 695\ 094\ 886\ 952\ 150\ 600\ 420\ 023\ 783\ 993\ 550\ 552\ 869\ 600\ 433\ 465\ 641\ 616\ 186\ 292\ 819\ 079\ 364\ 364\ 8$   
 $054\ 579\ 200\ q^{1320} -$   
 $2\ 139\ 262\ 153\ 317\ 531\ 980\ 322\ 400\ 392\ 770\ 558\ 816\ 961\ 344\ 727\ 948\ 100\ 013\ 286\ 558\ 010\ 340\ 436\ 453\ 990\ 8$   
 $014\ 976\ 000\ q^{1321} +$   
 $2\ 674\ 516\ 703\ 199\ 621\ 517\ 269\ 244\ 971\ 420\ 131\ 043\ 366\ 626\ 156\ 341\ 300\ 472\ 598\ 569\ 901\ 581\ 109\ 884\ 880\ 8$   
 $878\ 016\ 000\ q^{1324} -$   
 $2\ 881\ 032\ 250\ 588\ 030\ 145\ 885\ 129\ 377\ 706\ 618\ 699\ 217\ 540\ 390\ 799\ 268\ 035\ 789\ 606\ 707\ 018\ 694\ 793\ 447\ 8$   
 $638\ 323\ 300\ q^{1325} +$   
 $3\ 600\ 674\ 282\ 010\ 449\ 001\ 821\ 549\ 279\ 446\ 449\ 574\ 216\ 432\ 154\ 057\ 403\ 358\ 262\ 120\ 988\ 519\ 247\ 594\ 814\ 8$   
 $900\ 391\ 936\ q^{1328} -$   
 $3\ 878\ 271\ 613\ 861\ 125\ 078\ 062\ 424\ 365\ 951\ 263\ 766\ 504\ 697\ 167\ 141\ 325\ 944\ 455\ 212\ 728\ 690\ 902\ 992\ 409\ 8$   
 $513\ 984\ 000\ q^{1329} +$   
 $4\ 845\ 392\ 955\ 001\ 739\ 101\ 112\ 726\ 691\ 377\ 705\ 905\ 466\ 424\ 824\ 926\ 770\ 647\ 006\ 212\ 378\ 115\ 586\ 640\ 823\ 8$   
 $744\ 489\ 472\ q^{1332} -$   
 $5\ 218\ 373\ 802\ 106\ 731\ 518\ 426\ 114\ 861\ 512\ 007\ 075\ 254\ 792\ 976\ 047\ 572\ 229\ 541\ 645\ 102\ 922\ 155\ 948\ 089\ 8$   
 $420\ 560\ 042\ q^{1333} +$   
 $6\ 517\ 509\ 640\ 716\ 006\ 282\ 782\ 781\ 993\ 299\ 508\ 496\ 811\ 840\ 570\ 514\ 707\ 348\ 651\ 607\ 297\ 687\ 652\ 334\ 925\ 8$   
 $270\ 912\ 000\ q^{1336} -$   
 $7\ 018\ 428\ 448\ 135\ 803\ 225\ 956\ 545\ 194\ 869\ 757\ 108\ 072\ 817\ 493\ 170\ 608\ 858\ 762\ 958\ 422\ 834\ 264\ 397\ 974\ 8$   
 $934\ 585\ 344\ q^{1337} +$   
 $8\ 762\ 796\ 655\ 582\ 960\ 525\ 495\ 296\ 710\ 103\ 300\ 342\ 788\ 318\ 295\ 633\ 950\ 790\ 140\ 179\ 643\ 247\ 459\ 874\ 615\ 8$   
 $458\ 662\ 400\ q^{1340} -$   
 $9\ 435\ 244\ 424\ 441\ 054\ 535\ 350\ 368\ 648\ 999\ 561\ 889\ 152\ 678\ 630\ 285\ 935\ 967\ 195\ 672\ 621\ 465\ 049\ 141\ 741\ 8$   
 $736\ 847\ 500\ q^{1341} +$   
 $11\ 776\ 412\ 585\ 959\ 192\ 402\ 793\ 273\ 527\ 187\ 421\ 715\ 207\ 434\ 004\ 055\ 601\ 213\ 854\ 341\ 369\ 877\ 110\ 590\ 8$   
 $688\ 100\ 352\ 000\ q^{1344} -$   
 $12\ 678\ 733\ 513\ 787\ 935\ 955\ 369\ 584\ 912\ 586\ 783\ 505\ 837\ 086\ 292\ 860\ 671\ 635\ 385\ 975\ 199\ 316\ 090\ 535\ 8$   
 $509\ 452\ 390\ 400\ q^{1345} +$   
 $15\ 819\ 522\ 378\ 283\ 828\ 943\ 026\ 769\ 129\ 813\ 556\ 889\ 959\ 644\ 833\ 047\ 988\ 668\ 847\ 919\ 039\ 797\ 493\ 178\ 8$   
 $710\ 492\ 479\ 488\ q^{1348} -$   
 $17\ 029\ 773\ 778\ 322\ 262\ 617\ 608\ 140\ 196\ 489\ 587\ 176\ 986\ 187\ 649\ 941\ 093\ 473\ 773\ 345\ 727\ 098\ 555\ 166\ 8$   
 $754\ 725\ 679\ 625\ q^{1349} +$   
 $21\ 241\ 473\ 450\ 274\ 677\ 412\ 303\ 498\ 947\ 650\ 891\ 929\ 693\ 607\ 554\ 406\ 066\ 205\ 725\ 527\ 188\ 149\ 348\ 611\ 8$   
 $793\ 671\ 425\ 792\ q^{1352} -$   
 $22\ 864\ 042\ 087\ 691\ 351\ 107\ 942\ 837\ 081\ 447\ 108\ 622\ 871\ 873\ 944\ 256\ 610\ 760\ 675\ 254\ 891\ 031\ 032\ 850\ 8$   
 $107\ 954\ 495\ 488\ q^{1353} +$   
 $28\ 509\ 372\ 860\ 404\ 251\ 058\ 218\ 667\ 125\ 186\ 231\ 918\ 463\ 134\ 111\ 915\ 170\ 603\ 188\ 589\ 940\ 563\ 876\ 425\ 8$   
 $734\ 582\ 656\ 000\ q^{1356} -$   
 $30\ 683\ 797\ 219\ 295\ 110\ 601\ 816\ 320\ 312\ 018\ 981\ 158\ 611\ 492\ 795\ 680\ 259\ 503\ 197\ 912\ 724\ 750\ 355\ 241\ 8$   
 $255\ 051\ 571\ 494\ q^{1357} +$   
 $38\ 247\ 519\ 218\ 573\ 033\ 185\ 513\ 094\ 853\ 444\ 319\ 505\ 683\ 866\ 609\ 641\ 401\ 856\ 672\ 299\ 498\ 634\ 955\ 938\ 8$   
 $733\ 885\ 849\ 600\ q^{1360} -$   
 $41\ 160\ 248\ 309\ 620\ 664\ 593\ 439\ 847\ 684\ 628\ 433\ 048\ 616\ 511\ 531\ 884\ 835\ 432\ 161\ 398\ 234\ 130\ 751\ 639\ 8$   
 $176\ 081\ 408\ 000\ q^{1361} +$

51 289 951 123 682 710 998 656 975 231 157 571 379 555 288 562 226 039 495 468 779 758 156 006 438  
 056 754 688 000  $q^{1364}$  -  
 55 190 010 826 557 892 181 368 930 005 363 717 293 092 045 635 563 563 971 921 831 677 136 060 930  
 038 785 154 650  $q^{1365}$  +  
 68 750 446 407 006 634 899 979 377 034 262 392 616 871 699 452 885 518 107 617 732 066 951 056 379  
 017 243 430 400  $q^{1368}$  -  
 73 970 303 296 435 564 196 638 843 658 190 654 689 513 693 325 213 201 141 942 232 534 282 669 871  
 907 422 208 248  $q^{1369}$  +  
 92 115 729 277 479 186 364 037 850 238 277 830 308 597 239 140 901 478 283 180 579 488 791 669 002  
 048 433 602 560  $q^{1372}$  -  
 99 099 064 920 076 285 065 048 760 088 950 109 122 025 944 124 598 041 086 980 513 884 154 992 116  
 923 879 057 123  $q^{1373}$  +  
 123 369 529 287 553 465 026 563 354 916 088 725 087 500 149 372 190 676 583 046 456 793 757 537 176  
 333 949 440 000  $q^{1376}$  -  
 132 708 198 860 736 088 154 866 248 022 686 838 608 076 880 060 937 892 382 654 149 557 879 756 502  
 357 534 212 096  $q^{1377}$  +  
 165 157 637 196 110 134 545 340 891 639 979 926 120 891 567 445 348 697 432 550 304 992 750 480 370  
 513 743 872 000  $q^{1380}$  -  
 177 640 829 580 949 465 291 353 968 876 225 900 655 152 752 825 407 144 662 967 898 736 565 794 136  
 975 941 526 000  $q^{1381}$  +  
 221 007 417 014 586 101 540 691 330 369 577 436 149 696 525 185 006 207 258 069 382 994 024 502 398  
 150 194 368 000  $q^{1384}$  -  
 237 687 018 206 503 065 354 406 266 128 975 602 410 070 763 324 703 987 821 838 384 604 248 218 386  
 867 991 347 200  $q^{1385}$  +  
 295 619 623 359 856 912 313 042 690 089 367 331 798 177 862 392 627 434 660 471 544 612 555 848 948  
 402 997 361 152  $q^{1388}$  -  
 317 897 089 007 515 961 740 896 109 056 466 146 620 913 425 380 724 680 154 587 572 259 469 562 736  
 266 888 191 250  $q^{1389}$  +  
 395 256 185 525 939 897 572 679 539 499 795 697 632 244 386 171 557 010 751 065 070 595 047 703 628  
 136 442 249 216  $q^{1392}$  -  
 424 997 954 497 399 704 109 955 584 506 994 282 621 942 630 073 779 165 716 719 725 554 824 805 167  
 239 028 146 176  $q^{1393}$  +  
 528 255 312 353 036 173 358 159 963 789 518 381 938 003 050 403 976 681 602 255 219 986 764 011 788  
 025 594 624 000  $q^{1396}$  -  
 567 946 077 202 623 715 055 731 737 820 273 032 912 491 596 538 125 472 547 492 522 132 006 996 453  
 656 609 099 076  $q^{1397}$  +  
 705 715 449 407 776 412 639 666 306 363 239 430 920 062 987 148 308 577 665 971 847 145 037 883 684  
 424 325 760 000  $q^{1400}$  -  
 758 661 620 622 473 127 150 952 625 144 878 702 653 869 076 385 486 462 922 800 389 880 627 741 525  
 219 471 360 000  $q^{1401}$  +  
 942 403 079 590 646 405 418 882 826 335 427 468 693 696 736 963 255 893 362 963 181 432 965 306 172  
 519 504 896 000  $q^{1404}$  -  
 1 013 002 774 830 693 349 662 321 119 589 761 676 513 432 869 401 923 670 909 414 812 509 713 138 248  
 469 987 075 275  $q^{1405}$  +  
 1 257 957 151 697 616 612 015 312 341 964 606 522 981 443 184 346 578 926 186 981 805 360 928 021 908  
 707 890 397 184  $q^{1408}$  -  
 1 352 058 320 483 752 128 430 264 788 658 805 236 117 860 538 656 338 299 626 304 773 016 558 514 969  
 759 748 096 000  $q^{1409}$  +  
 1 678 486 435 111 316 492 159 764 944 610 762 421 745 194 015 253 928 189 061 448 559 633 193 352 709  
 324 808 847 360  $q^{1412}$  -  
 1 803 861 704 216 195 427 745 149 033 341 446 574 071 797 719 976 006 691 709 160 407 574 334 899 176  
 516 972 839 014  $q^{1413}$  +  
 2 238 687 159 789 924 199 647 460 543 121 931 680 196 329 929 064 149 417 332 834 446 388 035 066 095  
 943 538 432 000  $q^{1416}$  -  
 2 405 663 196 038 281 951 337 749 342 576 606 893 249 370 254 211 896 098 371 973 535 822 154 051 516

883 269 582 848  $q^{1417} +$   
 2 984 649 316 017 283 020 540 083 688 973 817 378 161 218 119 356 221 974 906 929 415 604 853 281 178 9  
 769 505 331 200  $q^{1420} -$   
 3 206 940 663 918 037 226 573 197 725 175 713 132 590 679 576 179 878 033 225 681 038 813 752 528 204 9  
 590 603 612 875  $q^{1421} +$   
 3 977 574 127 627 063 093 875 686 009 889 515 968 448 752 189 630 880 458 453 360 052 075 305 606 176 9  
 474 808 320 000  $q^{1424} -$   
 4 273 387 527 481 785 307 925 310 574 038 218 965 438 860 486 168 576 536 612 051 968 587 643 946 918 9  
 018 061 926 400  $q^{1425} +$   
 5 298 696 648 091 578 442 714 580 181 647 684 165 978 144 080 233 964 296 327 680 562 130 782 805 341 9  
 527 861 108 736  $q^{1428} -$   
 5 692 193 010 743 556 592 876 094 233 762 683 338 074 738 195 044 209 488 862 155 609 989 316 095 692 9  
 675 335 092 750  $q^{1429} +$   
 7 055 801 651 520 542 142 834 514 540 714 727 292 356 622 258 588 917 096 136 337 355 288 857 054 736 9  
 552 760 439 296  $q^{1432} -$   
 7 579 030 783 231 221 878 431 357 059 592 539 800 656 670 751 884 545 879 056 925 171 352 379 331 090 9  
 389 250 768 896  $q^{1433} +$   
 9 391 845 222 592 018 675 218 100 404 521 307 035 794 551 973 325 344 303 194 940 842 625 888 778 159 9  
 498 395 392 000  $q^{1436} -$   
 10 087 305 194 080 668 771 084 239 911 544 915 523 771 430 540 637 897 121 832 950 316 784 171 527 9  
 503 751 708 229 799  $q^{1437} +$   
 12 496 358 187 638 689 897 623 678 516 457 660 606 321 220 528 345 102 349 990 327 778 423 708 294 9  
 027 645 911 552 000  $q^{1440} -$   
 13 420 379 733 732 746 771 607 401 744 576 474 411 528 162 501 294 080 083 089 752 952 742 503 258 9  
 064 153 391 104 000  $q^{1441} +$   
 16 620 523 256 779 988 315 065 585 304 870 381 396 597 418 893 859 390 317 826 930 879 738 384 668 9  
 745 075 271 706 752  $q^{1444} -$   
 17 847 743 468 411 973 091 850 558 256 350 663 665 606 388 488 456 657 030 669 069 960 749 317 059 9  
 964 278 011 009 330  $q^{1445} +$   
 22 097 101 866 824 115 665 841 724 369 009 262 933 373 949 848 092 802 025 866 722 697 138 181 005 9  
 840 202 182 151 680  $q^{1448} -$   
 23 726 375 544 126 833 218 718 274 804 882 909 790 694 032 043 456 533 603 253 663 935 602 458 449 9  
 888 817 135 616 000  $q^{1449} +$   
 29 366 760 771 654 253 720 520 052 386 930 187 586 811 937 316 413 098 019 585 064 540 917 156 494 9  
 143 077 267 893 760  $q^{1452} -$   
 31 528 968 513 242 558 641 800 106 338 236 500 606 511 135 690 518 100 098 366 266 311 432 165 854 9  
 523 209 719 323 943  $q^{1453} +$   
 39 012 840 710 182 359 216 741 721 772 406 965 696 596 777 964 801 468 488 659 737 622 326 031 817 9  
 673 535 077 376 000  $q^{1456} -$   
 41 881 198 478 397 938 737 584 304 409 997 441 203 288 743 520 687 144 735 968 035 691 563 548 172 9  
 829 508 275 470 336  $q^{1457} +$   
 51 807 257 122 990 867 994 376 706 538 065 666 473 173 395 357 423 306 982 381 629 292 200 558 466 9  
 696 798 943 744 000  $q^{1460} -$   
 55 610 923 617 284 913 037 546 763 785 284 725 878 227 154 401 711 702 867 611 711 022 020 755 587 9  
 454 828 072 611 000  $q^{1461} +$   
 68 771 074 607 120 165 027 011 960 659 531 720 241 165 111 375 956 409 768 986 437 038 864 421 172 9  
 393 186 343 808 000  $q^{1464} -$   
 73 813 104 687 561 910 780 652 830 459 079 509 159 690 309 112 666 362 121 774 003 596 233 759 010 9  
 437 572 571 955 200  $q^{1465} +$   
 91 254 416 495 966 895 575 124 818 311 256 203 832 895 467 973 913 564 071 905 899 195 974 948 862 9  
 757 306 741 993 472  $q^{1468} -$   
 97 935 439 995 944 077 135 258 486 143 673 077 743 282 406 210 185 838 249 278 936 624 043 734 506 9  
 101 905 450 555 250  $q^{1469} +$   
 121 041 842 413 520 352 422 181 546 674 087 796 112 878 293 279 923 338 589 475 982 068 662 861 622 9  
 139 261 367 222 272  $q^{1472} -$

129 891 282 701 161 325 604 805 799 404 869 467 641 857 073 500 759 775 865 043 353 652 297 555 888  
 094 618 469 236 736  $q^{1473} +$   
 160 491 259 696 758 076 757 162 671 573 306 444 850 372 024 370 243 733 554 431 691 112 071 481 059  
 602 434 904 064 000  $q^{1476} -$   
 172 208 477 703 146 289 370 286 853 629 472 884 380 641 509 033 382 664 755 721 858 216 645 232 443  
 723 056 477 472 830  $q^{1477} +$   
 212 716 973 094 032 661 654 196 171 064 944 884 425 040 919 577 656 459 236 417 413 715 966 613 974  
 983 896 775 961 600  $q^{1480} -$   
 228 225 472 684 855 487 151 461 248 973 920 966 232 721 268 669 779 761 242 948 927 253 777 350 037  
 758 005 792 768 000  $q^{1481} +$   
 281 830 809 590 969 659 244 194 558 290 232 894 664 534 715 443 470 868 809 369 592 694 878 862 282  
 118 659 887 616 000  $q^{1484} -$   
 302 349 624 720 893 522 232 106 769 694 596 448 328 737 281 472 019 132 145 445 393 859 962 547 861  
 201 789 727 364 225  $q^{1485} +$   
 373 259 628 343 993 177 543 189 538 427 117 982 523 982 060 405 298 106 744 905 666 483 446 691 657  
 868 798 367 989 760  $q^{1488} -$   
 400 397 304 188 126 791 921 172 908 311 165 347 079 441 240 512 283 270 257 799 745 997 623 821 595  
 475 856 543 744 000  $q^{1489} +$   
 494 163 262 485 083 488 827 732 442 535 078 184 994 052 188 030 379 217 945 229 955 240 247 518 341  
 705 226 009 757 696  $q^{1492} -$   
 530 041 536 939 778 294 847 586 216 496 030 635 233 315 800 237 947 954 855 833 445 660 625 369 168  
 083 206 704 429 707  $q^{1493} +$   
 653 984 462 578 591 526 195 029 345 610 482 281 017 537 293 772 138 132 336 601 550 790 251 833 872  
 203 660 392 576 000  $q^{1496} -$   
 701 400 975 765 645 328 788 520 994 468 418 060 298 766 805 358 434 226 775 202 671 057 271 225 584  
 885 334 792 241 152  $q^{1497} +$   
 865 172 273 480 034 692 432 081 053 401 027 155 208 286 577 647 124 707 341 713 187 073 068 322 109  
 265 270 524 416 000  $q^{1500} -$   
 927 814 544 114 135 462 853 839 059 337 532 985 992 806 603 833 012 602 150 123 528 517 029 472 478  
 342 935 696 232 250  $q^{1501} +$   
 1 144 133 199 955 483 457 507 111 722 533 898 232 185 602 427 714 408 087 837 659 279 001 546 252 915  
 638 415 669 248 000  $q^{1504} -$   
 1 226 859 921 647 078 052 451 900 089 182 781 018 611 584 143 217 195 420 319 326 546 191 142 485 745  
 633 716 923 596 800  $q^{1505} +$   
 1 512 481 446 271 070 311 266 380 016 081 495 535 404 290 830 447 034 625 507 952 044 087 101 735 947  
 136 806 111 150 080  $q^{1508} -$   
 1 621 692 152 387 557 863 032 734 902 248 984 518 419 383 884 555 409 120 555 982 490 764 240 240 053  
 721 503 367 294 375  $q^{1509} +$   
 1 998 681 685 295 770 880 953 534 489 398 330 240 534 682 811 556 560 580 112 275 365 103 962 264 798  
 100 137 332 051 968  $q^{1512} -$   
 2 142 802 371 519 526 942 292 913 188 428 373 356 592 190 196 697 511 246 367 394 377 873 681 235 416  
 607 822 562 852 864  $q^{1513} +$   
 2 640 206 835 618 186 728 745 928 886 632 651 291 740 356 236 100 283 328 180 411 653 470 262 787 055  
 579 704 211 904 000  $q^{1516} -$   
 2 830 327 689 685 385 529 918 229 425 704 133 555 808 009 875 748 099 652 896 949 877 293 402 326 802  
 671 421 070 630 747  $q^{1517} +$   
 3 486 371 305 796 322 302 392 105 742 971 156 853 167 526 554 719 733 914 722 795 048 791 123 696 033  
 390 182 883 737 600  $q^{1520} -$   
 3 737 083 893 999 633 366 632 601 239 267 461 717 599 933 375 364 495 113 674 031 969 770 328 751 765  
 099 912 646 656 248  $q^{1521} +$   
 4 602 049 850 843 199 889 522 246 257 470 494 076 635 811 777 623 718 657 988 423 946 197 834 477 049  
 842 888 589 824 000  $q^{1524} -$   
 4 932 545 759 756 782 391 461 740 193 925 918 434 586 347 594 703 603 157 650 956 275 369 601 871 891  
 665 418 542 489 425  $q^{1525} +$   
 6 072 557 162 778 137 585 213 763 534 132 480 967 811 621 954 578 350 903 861 013 811 406 234 155 782

737 188 445 308 928  $q^{1528}$  -  
 6 508 069 247 765 072 861 916 900 812 957 618 257 639 458 752 828 340 559 644 111 114 040 800 169 906  
 086 315 872 256 000  $q^{1529}$  +  
 8 010 048 261 406 625 383 949 417 855 962 505 076 238 647 689 171 980 005 703 613 835 951 922 270 488  
 576 287 336 878 080  $q^{1532}$  -  
 8 583 740 687 277 534 033 947 458 402 572 759 491 526 604 982 248 176 029 658 433 019 901 979 587 116  
 908 011 940 172 721  $q^{1533}$  +  
 10 561 910 762 027 559 789 448 576 038 427 878 058 767 124 560 585 934 601 445 343 095 992 970 323  
 976 924 446 228 480 000  $q^{1536}$  -  
 11 317 356 730 295 761 558 587 269 847 120 877 908 304 995 202 735 105 408 035 450 123 304 356 731  
 997 581 630 019 207 168  $q^{1537}$  +  
 13 921 765 123 396 954 217 384 703 843 527 161 030 968 807 339 900 150 659 066 801 709 137 801 624  
 297 331 384 628 838 400  $q^{1540}$  -  
 14 916 193 903 772 568 595 288 285 192 853 275 603 025 403 518 162 334 315 860 469 488 335 948 506  
 718 573 170 433 042 500  $q^{1541}$  +  
 18 343 878 381 748 724 538 837 439 729 897 793 197 125 994 765 446 377 174 780 044 027 578 208 578  
 109 074 700 301 184 000  $q^{1544}$  -  
 19 652 429 050 055 098 377 876 986 442 589 958 246 017 610 765 271 279 936 421 118 255 466 874 592  
 685 851 664 467 558 400  $q^{1545}$  +  
 24 162 044 150 647 696 242 356 102 079 609 189 657 227 723 581 246 581 452 019 591 458 593 149 785  
 794 200 697 727 230 464  $q^{1548}$  -  
 25 883 336 250 065 569 510 845 148 980 302 141 200 886 898 904 893 067 143 660 170 554 101 906 637  
 322 839 871 908 387 125  $q^{1549}$  +  
 31 814 304 386 992 358 164 540 290 083 402 231 177 742 897 755 241 019 164 767 233 904 115 190 056  
 378 088 110 672 445 440  $q^{1552}$  -  
 34 077 730 741 937 310 560 154 547 178 424 119 322 347 233 000 255 727 349 282 404 288 377 813 786  
 508 468 289 188 462 592  $q^{1553}$  +  
 41 875 309 470 694 078 249 648 164 002 624 107 473 654 521 765 355 056 618 462 631 920 792 122 859  
 750 599 289 543 424 000  $q^{1556}$  -  
 44 850 580 318 693 747 098 869 307 566 448 173 320 961 855 446 639 330 558 557 025 214 857 704 472  
 256 846 774 301 857 508  $q^{1557}$  +  
 55 098 662 296 207 698 666 766 405 953 678 181 757 154 957 577 873 843 171 659 775 503 880 394 931  
 971 486 913 803 980 800  $q^{1560}$  -  
 59 008 291 514 524 784 091 076 111 483 008 842 756 065 860 704 152 701 560 763 120 197 598 358 147  
 619 056 316 153 856 000  $q^{1561}$  +  
 72 472 308 067 908 599 512 116 189 196 346 628 295 432 773 092 118 771 017 597 357 777 780 103 470  
 421 049 881 592 320 000  $q^{1564}$  -  
 77 607 942 942 081 650 233 801 354 595 428 843 869 272 270 231 452 036 758 417 632 149 645 336 556  
 034 797 513 071 363 950  $q^{1565}$  +  
 95 290 964 712 627 712 409 353 678 614 315 068 533 813 618 372 787 126 697 638 090 659 272 055 626  
 618 942 098 315 704 320  $q^{1568}$  -  
 102 034 735 226 201 582 170 358 457 363 081 345 853 025 962 404 204 974 161 628 682 398 047 716 772  
 389 318 716 731 392 000  $q^{1569}$  +  
 125 250 804 779 505 975 607 258 954 288 409 750 214 686 820 389 755 812 895 483 092 064 144 555 567  
 227 529 196 322 144 256  $q^{1572}$  -  
 134 103 226 040 154 910 892 756 116 194 240 418 076 852 925 391 145 353 827 388 562 284 299 073 942  
 410 875 071 596 764 538  $q^{1573}$  +  
 164 573 183 533 819 961 979 832 024 009 297 078 319 074 086 838 022 711 379 822 978 133 090 685 672  
 603 166 430 246 848 000  $q^{1576}$  -  
 176 189 610 696 002 104 946 281 138 593 122 050 520 246 661 434 843 941 902 789 688 950 930 091 202  
 118 961 058 063 941 632  $q^{1577}$  +  
 216 166 270 298 339 492 893 289 724 477 439 873 061 482 909 365 919 072 428 509 033 943 069 631 837  
 240 890 164 619 571 200  $q^{1580}$  -  
 231 404 511 680 424 892 466 040 864 204 737 429 007 390 972 153 045 498 162 298 017 147 584 165 184  
 959 465 912 816 655 250  $q^{1581}$  +

283 836 124 653 920 517 598 488 928 570 861 908 261 199 129 332 402 067 383 531 033 406 259 845 579  
 422 704 628 208 128 000  $q^{1584}$  -  
 303 818 607 864 337 725 505 893 382 556 237 446 712 172 195 817 030 273 614 243 230 834 321 879 620  
 837 251 355 700 428 800  $q^{1585}$  +  
 372 562 252 477 510 767 819 298 298 550 988 480 284 370 054 390 775 753 635 070 996 255 893 814 589  
 864 318 816 429 398 016  $q^{1588}$  -  
 398 757 165 028 294 970 401 441 296 475 265 740 579 757 020 758 132 685 569 260 619 365 923 029 898  
 040 942 508 331 364 625  $q^{1589}$  +  
 488 857 221 192 473 124 761 437 048 817 007 411 031 614 401 024 611 853 784 057 816 729 745 869 271  
 241 108 923 558 106 112  $q^{1592}$  -  
 523 184 382 371 111 971 594 181 773 699 268 472 601 086 394 164 615 589 898 650 241 076 152 255 498  
 598 127 621 094 375 424  $q^{1593}$  +  
 641 235 823 362 806 630 649 061 408 083 686 636 198 589 326 964 212 802 569 723 527 710 207 408 156  
 393 432 952 470 528 000  $q^{1596}$  -  
 686 204 780 278 863 271 198 071 519 226 863 849 052 684 676 332 360 682 438 752 699 227 533 135 410  
 618 589 495 414 406 945  $q^{1597}$  +  
 840 826 960 655 112 591 367 800 430 426 477 712 308 687 945 325 193 221 779 386 001 791 853 927 250  
 832 479 140 954 316 800  $q^{1600}$  -  
 899 717 057 995 606 420 225 268 852 176 312 571 149 841 708 132 010 447 006 883 491 986 041 460 783  
 024 395 519 647 744 000  $q^{1601}$  +  
 1 102 171 405 056 683 228 931 112 186 957 550 708 305 990 675 379 235 248 031 041 874 058 157 878 079  
 138 701 374 007 296 000  $q^{1604}$  -  
 1 179 266 510 275 883 749 169 546 332 146 937 662 309 692 499 979 086 963 350 207 553 638 163 972 342  
 852 799 633 456 042 275  $q^{1605}$  +  
 1 444 261 566 700 034 320 495 479 115 729 930 122 151 118 899 550 188 872 571 326 540 669 683 435 532  
 573 400 954 872 715 264  $q^{1608}$  -  
 1 545 155 941 184 123 821 278 875 837 896 076 480 644 171 308 070 518 230 793 462 127 637 980 718 251  
 925 015 454 806 016 000  $q^{1609}$  +  
 1 891 896 246 326 074 943 287 399 566 782 284 860 500 601 142 789 130 301 608 575 965 744 159 683 264  
 941 010 653 540 193 280  $q^{1612}$  -  
 2 023 892 999 037 135 086 250 360 130 038 362 190 491 357 361 931 489 274 527 810 607 908 814 374 793  
 690 813 271 007 147 791  $q^{1613}$  +  
 2 477 445 226 686 871 833 415 535 414 964 241 295 087 568 278 776 228 869 372 772 230 963 836 339 816  
 844 533 877 221 376 000  $q^{1616}$  -  
 2 650 075 207 398 385 855 922 382 452 099 447 525 789 694 473 240 186 966 390 922 101 445 465 224 061  
 747 460 537 755 336 704  $q^{1617}$  +  
 3 243 146 952 384 339 599 453 265 911 376 626 992 385 534 380 977 352 087 651 222 810 194 621 924 227  
 375 914 742 856 837 120  $q^{1620}$  -  
 3 468 844 273 939 824 022 104 512 036 949 678 894 884 201 973 712 672 564 284 765 677 439 068 742 091  
 885 739 537 450 423 250  $q^{1621}$  +  
 4 244 099 392 869 793 923 543 002 697 906 724 217 154 548 462 542 562 269 623 015 881 037 125 186 216  
 640 274 678 654 464 000  $q^{1624}$  -  
 4 539 080 581 773 356 224 730 473 258 227 900 170 594 354 066 505 841 751 905 394 121 898 273 096 151  
 923 004 210 823 168 000  $q^{1625}$  +  
 5 552 151 978 379 566 897 145 773 580 875 543 699 240 144 745 971 880 316 827 122 675 123 579 384 261  
 229 996 041 031 415 808  $q^{1628}$  -  
 5 937 559 772 806 371 260 117 675 254 641 351 616 613 870 218 534 063 881 499 454 229 094 613 619 422  
 898 699 302 648 960 625  $q^{1629}$  +  
 7 260 968 478 407 425 366 057 673 350 678 285 822 751 157 236 412 301 975 426 892 435 106 699 451 122  
 751 171 476 695 654 400  $q^{1632}$  -  
 7 764 359 469 949 290 676 776 091 917 095 762 186 995 261 675 003 027 023 392 096 727 093 143 074 754  
 153 044 255 522 553 856  $q^{1633}$  +  
 9 492 611 041 970 131 493 501 000 974 821 637 290 886 299 059 829 158 526 508 933 679 859 605 514 402  
 984 386 683 895 808 000  $q^{1636}$  -  
 10 149 889 917 721 442 035 467 852 085 797 401 862 096 501 480 498 286 982 465 602 169 430 116 939

688 533 609 175 488 646 681  $q^{1637} +$   
 12 406 099 750 971 423 494 335 859 346 438 591 962 573 585 737 803 533 464 358 023 408 140 163 494  
 408 051 716 703 057 408 000  $q^{1640} -$   
 13 264 033 420 720 999 688 237 874 034 442 188 256 089 970 171 313 698 732 396 168 085 982 183 089  
 453 507 759 476 748 288 000  $q^{1641} +$   
 16 208 536 950 413 758 929 513 387 124 336 678 827 231 713 632 536 029 774 298 360 404 568 676 082  
 394 666 415 720 918 912 000  $q^{1644} -$   
 17 328 021 388 393 955 878 022 032 797 430 640 867 813 648 436 160 212 806 764 977 796 555 201 507  
 608 525 506 173 394 140 725  $q^{1645} +$   
 21 169 560 357 176 034 797 003 554 483 863 791 648 524 857 781 449 000 289 710 477 647 329 839 531  
 084 516 396 429 256 409 088  $q^{1648} -$   
 22 629 864 196 500 028 659 244 607 972 769 529 445 639 407 984 915 297 690 974 817 959 914 696 681  
 066 227 999 714 197 504 000  $q^{1649} +$   
 27 640 115 200 178 785 480 412 211 170 999 948 651 028 098 757 337 303 414 391 630 323 516 176 027  
 660 582 640 122 371 641 344  $q^{1652} -$   
 29 544 390 411 064 578 153 766 124 333 014 937 926 066 446 631 469 523 676 720 308 994 334 277 690  
 553 240 155 512 199 485 006  $q^{1653} +$   
 36 076 828 506 571 420 579 092 940 331 158 869 879 766 680 484 965 074 513 909 889 355 515 925 274  
 611 517 209 943 399 040 000  $q^{1656} -$   
 38 559 264 284 107 716 838 381 449 460 169 725 160 107 040 171 666 316 939 788 573 422 265 272 304  
 356 288 600 156 286 484 480  $q^{1657} +$   
 47 073 647 617 739 374 897 723 321 162 360 518 246 472 949 432 569 477 350 412 352 950 267 607 955  
 948 852 271 517 652 940 800  $q^{1660} -$   
 50 308 754 604 796 335 207 915 512 924 847 647 519 481 220 907 197 447 486 984 154 434 195 451 306  
 871 428 951 980 345 343 250  $q^{1661} +$   
 61 402 895 265 481 288 792 392 428 758 030 340 058 430 712 953 794 344 369 069 802 075 071 602 499  
 795 704 418 078 576 640 000  $q^{1664} -$   
 65 617 550 803 278 740 025 072 656 416 879 389 709 482 831 178 296 674 728 217 591 120 623 304 105  
 853 426 735 410 950 963 200  $q^{1665} +$   
 80 068 527 547 429 598 982 987 368 586 164 286 629 845 899 183 646 461 359 648 296 357 762 053 360  
 978 280 531 516 794 519 552  $q^{1668} -$   
 85 557 598 279 882 948 782 883 275 367 768 896 579 206 139 968 903 661 601 483 466 260 025 592 621  
 275 096 067 743 886 116 625  $q^{1669} +$   
 104 375 200 824 654 138 355 127 998 219 469 582 249 341 750 014 431 929 073 366 269 361 326 240 748  
 757 991 625 276 955 856 896  $q^{1672} -$   
 111 521 798 937 505 358 529 112 059 922 892 603 788 800 448 214 463 015 346 665 753 839 783 433 553  
 649 012 948 920 765 513 728  $q^{1673} +$   
 136 017 812 985 113 505 684 447 009 295 094 735 783 520 640 828 616 733 381 716 335 086 422 129 025  
 199 815 926 833 951 296 000  $q^{1676} -$   
 145 319 552 440 879 038 454 877 176 077 500 737 100 271 751 282 546 197 668 290 824 432 237 759 799  
 110 271 141 114 078 692 102  $q^{1677} +$   
 177 197 553 385 716 603 524 127 761 020 119 977 086 557 180 918 562 346 822 881 273 687 268 230 191  
 887 362 202 401 996 800 000  $q^{1680} -$   
 189 300 573 095 820 221 353 793 959 627 562 808 852 423 002 504 620 435 893 273 886 623 393 517 587  
 642 058 148 713 267 200 248  $q^{1681} +$   
 230 772 263 968 718 407 235 005 748 430 463 733 167 006 941 488 272 976 053 812 665 588 385 610 350  
 901 986 805 911 723 264 000  $q^{1684} -$   
 246 515 302 185 964 610 599 623 712 091 080 153 870 058 999 230 123 907 730 212 779 075 495 008 228  
 431 181 600 715 883 222 025  $q^{1685} +$   
 300 451 197 357 541 239 999 118 145 959 276 115 435 724 659 808 594 514 298 862 952 845 336 791 891  
 643 620 227 824 633 183 744  $q^{1688} -$   
 320 922 669 512 979 182 783 318 364 244 130 691 183 350 663 588 771 007 511 630 835 792 705 510 408  
 047 699 896 564 846 592 000  $q^{1689} +$   
 391 047 205 381 144 593 281 222 929 994 622 571 749 800 898 976 036 409 560 018 519 813 790 458 193  
 359 459 817 414 951 522 304  $q^{1692} -$

417 659 099 716 862 839 355 942 572 264 870 265 342 137 406 178 191 608 920 000 768 318 890 697 864 805 262 195 296 934 060 064  $q^{1693}$  +  
 508 803 195 633 440 133 356 387 237 175 906 566 586 807 393 540 207 009 761 589 659 911 192 816 998 681 627 668 824 843 776 000  $q^{1696}$  -  
 543 386 713 427 399 732 733 211 316 377 071 892 457 990 161 567 209 866 809 615 513 191 620 176 536 603 245 301 027 934 666 752  $q^{1697}$  +  
 661 814 601 798 141 360 308 275 650 231 522 652 109 694 867 710 667 235 221 208 682 634 248 062 527 928 069 665 615 707 750 400  $q^{1700}$  -  
 706 743 904 001 040 620 986 562 089 232 751 446 794 917 365 888 941 654 224 719 012 818 104 329 703 922 167 822 544 989 807 750  $q^{1701}$  +  
 860 575 944 094 583 527 866 605 438 710 796 758 668 448 804 852 014 367 402 052 051 027 329 620 576 080 773 234 704 326 400 000  $q^{1704}$  -  
 918 928 216 805 664 007 773 703 596 682 543 268 697 592 135 213 165 130 054 175 156 372 877 644 307 157 768 406 112 636 108 800  $q^{1705}$  +  
 1 118 687 719 244 375 014 222 113 949 636 565 633 604 106 048 492 152 699 866 733 640 200 275 287 959 618 775 717 465 350 718 464  $q^{1708}$  -  
 1 194 450 156 307 636 899 956 297 106 719 374 990 549 447 494 555 148 991 068 728 662 226 662 754 606 200 486 463 431 885 162 625  $q^{1709}$  +  
 1 453 770 382 190 281 488 168 306 854 479 598 087 674 262 222 526 049 947 444 740 796 290 442 571 897 257 025 897 273 715 822 592  $q^{1712}$  -  
 1 552 107 758 219 445 545 307 324 467 397 899 538 107 059 667 075 609 059 952 357 480 850 944 131 071 115 742 041 142 394 912 768  $q^{1713}$  +  
 1 888 645 742 695 752 795 057 913 843 736 304 858 439 161 008 241 094 372 677 239 760 642 025 296 566 123 575 269 740 515 328 000  $q^{1716}$  -  
 2 016 246 211 973 022 872 169 603 494 016 289 593 939 619 462 144 603 950 983 188 954 881 094 806 202 686 530 622 725 442 067 176  $q^{1717}$  +  
 2 452 863 571 042 718 771 466 865 607 315 412 829 882 358 424 192 443 213 914 181 620 424 748 599 957 335 247 942 454 733 900 800  $q^{1720}$  -  
 2 618 385 431 446 739 955 373 000 685 869 929 516 690 661 845 536 041 767 390 608 631 049 061 645 608 642 468 679 951 831 040 000  $q^{1721}$  +  
 3 184 673 709 387 965 092 052 835 074 662 780 686 451 385 332 019 783 934 995 077 759 290 053 332 471 526 458 347 597 433 344 000  $q^{1724}$  -  
 3 399 322 442 831 228 943 340 991 353 540 152 660 518 967 916 144 501 779 142 818 689 393 657 501 942 044 136 971 837 676 479 150  $q^{1725}$  +  
 4 133 572 959 581 416 928 855 547 943 442 114 802 514 134 173 537 328 990 530 294 086 382 947 200 532 915 306 566 640 666 804 224  $q^{1728}$  -  
 4 411 846 321 577 505 291 249 072 838 138 457 041 549 162 713 247 220 092 923 038 426 761 117 458 554 349 177 460 953 735 168 000  $q^{1729}$  +  
 5 363 593 315 214 744 313 701 258 657 696 362 326 669 081 722 331 318 723 244 479 192 709 166 813 271 095 408 054 720 928 399 360  $q^{1732}$  -  
 5 724 243 135 898 845 119 376 253 186 884 940 484 288 308 814 974 392 360 637 322 145 875 502 741 318 666 871 998 655 562 870 808  $q^{1733}$  +  
 6 957 546 102 474 819 087 571 984 539 359 001 608 719 990 775 890 535 109 373 646 308 551 038 511 248 487 711 340 759 166 208 000  $q^{1736}$  -  
 7 424 819 472 780 046 788 545 705 152 176 069 516 545 136 526 270 434 762 106 468 909 802 498 537 749 635 845 600 336 612 327 424  $q^{1737}$  +  
 9 022 498 343 251 324 905 834 771 955 906 904 183 711 487 216 126 218 135 780 474 126 884 122 142 885 239 179 547 653 838 489 600  $q^{1740}$  -  
 9 627 738 882 808 920 720 265 878 764 129 786 900 529 864 441 612 623 809 717 073 073 553 558 776 687 053 974 098 583 479 374 625  $q^{1741}$  +  
 11 696 837 072 878 377 433 620 536 802 391 363 691 885 245 185 882 200 490 958 398 709 470 144 040 065 357 541 051 466 360 832 000  $q^{1744}$  -  
 12 480 550 152 575 052 112 576 762 008 187 043 727 120 275 864 639 988 242 146 605 977 118 478 002 154 102 473 755 888 856 268 800  $q^{1745}$  +  
 15 159 379 461 810 454 468 366 760 264 225 614 033 414 683 414 177 274 354 433 259 046 757 390 702

423 016 152 985 721 344 675 840  $q^{1748}$  –  
 16 173 895 049 097 442 804 733 957 637 073 125 030 481 874 063 447 726 413 555 443 930 785 682 117 840 202 105 503 042 851 298 375  $q^{1749}$  +  
 19 641 117 855 997 573 208 017 933 314 324 700 168 398 231 829 762 975 077 542 767 752 670 311 950 397 506 920 357 522 021 607 424  $q^{1752}$  –  
 20 954 022 944 584 240 049 911 276 638 407 664 617 612 572 760 384 211 588 985 529 125 812 627 051 247 171 090 082 747 403 239 424  $q^{1753}$  +  
 25 440 357 538 166 970 625 768 067 086 908 617 077 637 439 436 759 240 190 722 522 770 250 695 692 764 880 337 933 718 387 968 000  $q^{1756}$  –  
 27 138 919 325 985 549 429 149 481 326 651 555 107 516 309 266 737 470 436 801 779 945 643 166 518 893 898 696 717 283 410 799 924  $q^{1757}$  +  
 32 942 221 730 192 865 921 673 608 788 015 315 643 532 872 961 317 008 534 185 971 517 789 374 287 801 383 057 301 319 024 844 800  $q^{1760}$  –  
 35 139 085 910 621 791 545 631 773 671 179 947 581 396 414 854 199 562 083 585 012 126 775 473 174 000 485 920 899 686 240 256 000  $q^{1761}$  +  
 42 643 776 704 296 399 178 757 184 246 303 436 539 540 010 845 777 664 974 719 397 258 905 072 154 746 212 807 247 479 724 058 752  $q^{1764}$  –  
 45 484 306 396 152 706 517 143 127 397 700 962 151 826 780 686 858 617 611 875 784 206 405 823 816 135 503 908 345 896 307 063 075  $q^{1765}$  +  
 55 186 387 275 808 816 682 789 452 512 304 900 508 666 275 083 553 526 550 783 566 753 196 411 271 992 415 853 478 160 943 351 808  $q^{1768}$  –  
 58 858 112 312 403 374 814 052 041 616 159 842 990 591 557 275 790 430 437 038 811 174 616 355 794 567 196 063 439 050 260 480 000  $q^{1769}$  +  
 71 397 371 741 252 361 410 904 391 476 789 046 844 239 051 684 471 283 059 732 404 859 197 307 166 963 181 248 729 517 330 860 544  $q^{1772}$  –  
 76 142 151 768 681 768 671 179 200 687 162 015 667 125 626 128 339 195 479 408 710 135 767 608 405 282 515 040 511 257 151 137 363  $q^{1773}$  +  
 92 343 614 102 316 297 917 952 190 535 225 326 932 514 183 357 755 365 593 243 479 574 702 792 830 938 331 540 327 313 864 704 000  $q^{1776}$  –  
 98 473 290 527 439 552 593 123 514 790 679 567 269 484 294 047 393 368 308 547 538 518 407 655 341 700 437 061 138 408 156 364 800  $q^{1777}$  +  
 119 400 546 801 368 049 373 313 781 023 982 301 975 586 759 775 857 436 574 542 356 085 465 886 558 719 906 937 600 170 826 752 000  $q^{1780}$  –  
 127 317 078 739 527 590 792 431 285 665 317 615 495 772 432 838 118 850 460 763 123 820 458 332 133 274 635 515 358 150 699 651 625  $q^{1781}$  +  
 154 340 886 070 502 435 061 207 432 581 848 393 924 603 526 183 526 693 015 970 561 699 724 794 655 315 067 749 323 237 416 960 000  $q^{1784}$  –  
 164 562 247 715 088 189 597 109 852 356 638 757 152 977 210 241 291 690 064 148 255 553 812 641 957 045 645 657 753 356 225 740 800  $q^{1785}$  +  
 199 448 744 366 255 471 709 320 389 934 815 145 341 297 853 329 447 822 387 076 261 131 617 887 978 026 574 677 390 926 872 619 008  $q^{1788}$  –  
 212 642 223 094 737 610 952 868 513 933 802 796 719 119 738 746 918 088 613 400 463 479 665 323 249 454 378 341 506 750 126 083 875  $q^{1789}$  +  
 257 666 336 998 712 781 342 508 105 041 685 751 450 254 944 472 303 631 588 352 408 910 765 861 051 433 558 806 599 439 431 499 776  $q^{1792}$  –  
 274 691 335 376 666 598 737 307 699 006 433 809 107 343 656 476 742 823 862 288 588 656 813 981 796 114 751 827 874 253 288 800 256  $q^{1793}$  +  
 332 782 541 170 999 433 188 188 875 989 875 359 395 119 948 235 271 434 462 776 250 748 852 517 966 383 987 654 967 646 414 848 000  $q^{1796}$  –  
 354 745 580 380 835 980 412 681 071 780 068 772 937 370 933 608 643 966 981 796 348 334 831 387 259 368 134 254 693 899 930 207 609  $q^{1797}$  +  
 429 675 180 808 254 396 534 667 772 884 022 629 260 954 233 647 827 969 746 703 218 563 018 253 287 591 507 936 112 913 861 331 200  $q^{1800}$  –  
 458 000 564 435 075 291 346 571 263 114 398 195 825 557 409 845 253 982 544 300 695 083 152 839 159 589 413 721 762 094 936 064 000  $q^{1801}$  +

554 622 260 332 527 207 905 329 575 174 072 859 581 046 059 395 287 051 828 912 464 157 010 391 114 846 987 820 074 328 056 192 000  $q^{1804}$  -  
 591 142 832 571 311 254 759 506 164 889 732 331 367 372 876 406 850 247 026 855 882 218 002 550 029 933 493 280 332 313 289 226 195  $q^{1805}$  +  
 715 701 660 148 722 549 092 306 418 645 598 675 711 144 574 966 770 408 594 771 243 427 181 252 457 377 924 058 879 843 583 655 936  $q^{1808}$  -  
 762 775 341 016 488 306 383 079 386 255 080 702 153 375 484 381 979 104 998 467 344 321 060 392 017 576 921 732 902 081 150 976 000  $q^{1809}$  +  
 923 304 298 275 904 755 074 750 678 624 378 542 366 032 835 393 401 168 597 609 290 208 434 959 877 789 300 770 372 904 376 053 760  $q^{1812}$  -  
 983 963 676 543 876 203 632 083 737 650 822 832 318 133 606 335 110 610 950 301 453 795 819 677 837 015 591 910 036 465 037 942 339  $q^{1813}$  +  
 1 190 792 791 280 622 669 446 690 560 806 380 675 490 353 452 343 132 893 164 803 464 708 605 722 218 735 066 550 115 905 905 728 000  $q^{1816}$  -  
 1 268 937 100 944 510 538 127 626 296 549 190 016 341 706 034 254 781 213 558 062 287 506 300 870 925 895 610 949 437 017 203 998 720  $q^{1817}$  +  
 1 535 346 641 280 105 802 893 385 390 083 337 752 012 931 509 793 066 735 262 354 032 755 021 427 301 994 630 090 446 576 649 830 400  $q^{1820}$  -  
 1 635 988 063 784 866 952 965 735 081 792 935 823 453 578 101 419 780 175 701 213 137 167 509 575 837 763 888 437 516 833 984 382 000  $q^{1821}$  +  
 1 979 046 480 552 061 500 119 381 620 502 453 097 932 545 250 801 951 385 064 420 030 500 554 167 708 683 732 360 742 321 668 096 000  $q^{1824}$  -  
 2 108 626 061 394 702 220 659 687 886 237 520 499 660 878 255 517 627 732 659 204 801 361 405 155 746 864 621 825 354 722 933 964 800  $q^{1825}$  +  
 2 550 264 618 521 258 119 445 596 332 333 498 606 645 108 915 122 693 377 821 064 219 153 223 441 710 557 709 043 366 178 525 511 680  $q^{1828}$  -  
 2 717 057 365 836 460 841 976 744 552 712 226 783 196 920 813 584 171 742 883 798 898 260 162 051 263 016 276 131 898 269 218 936 875  $q^{1829}$  +  
 3 285 447 947 467 995 698 166 968 446 428 384 711 415 664 470 039 041 006 937 020 373 947 396 890 063 534 959 376 164 229 373 163 008  $q^{1832}$  -  
 3 500 082 150 222 358 200 118 706 133 847 352 131 676 885 214 141 321 746 124 721 536 790 106 405 507 055 295 612 483 181 923 467 264  $q^{1833}$  +  
 4 231 403 308 556 706 714 844 932 712 586 090 763 079 780 695 232 124 815 563 639 127 023 827 828 756 083 112 289 337 110 928 896 000  $q^{1836}$  -  
 4 507 526 102 747 043 875 468 629 043 539 201 117 790 924 782 128 854 139 855 196 466 815 170 413 180 615 138 693 226 989 527 212 207  $q^{1837}$  +  
 5 448 226 146 847 915 423 587 930 207 510 277 951 295 498 831 598 260 571 830 979 902 547 990 084 715 881 291 625 371 630 863 769 600  $q^{1840}$  -  
 5 803 356 290 099 506 823 545 140 173 866 807 073 327 162 706 442 164 299 323 133 096 922 481 794 026 193 994 578 056 020 697 088 000  $q^{1841}$  +  
 7 013 052 539 472 959 897 132 965 143 076 636 827 018 243 916 758 754 592 820 316 175 708 080 759 677 069 293 223 398 305 567 488 000  $q^{1844}$  -  
 7 469 672 763 775 167 715 237 029 429 714 237 945 793 706 127 160 664 436 286 230 583 092 771 295 482 924 561 009 986 311 615 306 875  $q^{1845}$  +  
 9 024 864 819 329 313 183 672 290 317 317 944 679 143 035 254 641 383 172 040 682 197 544 616 296 804 218 284 088 925 872 937 740 288  $q^{1848}$  -  
 9 611 820 701 690 761 950 342 814 934 641 149 156 860 883 069 642 893 389 427 072 857 196 461 986 305 903 656 191 853 722 218 496 248  $q^{1849}$  +  
 11 610 645 038 031 588 646 269 509 643 431 675 263 550 047 152 394 353 120 617 812 361 642 012 605 261 808 975 838 696 465 555 738 624  $q^{1852}$  -  
 12 364 935 930 424 436 169 704 494 259 164 975 972 555 620 111 238 677 445 946 435 910 048 164 760 528 157 843 597 854 720 911 871 078  $q^{1853}$  +  
 14 933 252 239 770 163 322 594 021 698 291 254 172 693 390 169 293 559 654 705 584 620 435 677 231 287 510 876 980 647 931 789 312 000  $q^{1856}$  -  
 15 902 323 542 333 895 774 483 534 014 242 151 344 520 354 058 958 920 619 086 356 226 830 539 342

247 689 159 055 034 470 592 315 392  $q^{1857} +$   
 19 201 503 822 735 763 796 095 783 498 811 516 635 143 140 135 666 076 962 561 330 917 738 235 560  
 143 803 692 002 083 844 998 758 400  $q^{1860} -$   
 20 446 180 180 964 724 835 863 683 428 528 110 057 974 018 785 245 394 172 234 157 937 968 236 744  
 611 755 989 114 521 577 223 750 750  $q^{1861} +$   
 24 683 074 349 899 538 515 502 550 039 615 028 496 666 504 140 070 419 777 913 212 096 984 786 053  
 885 707 029 266 154 158 623 232 000  $q^{1864} -$   
 26 281 312 006 918 555 493 631 499 782 036 655 983 011 794 332 506 155 682 297 035 580 167 690 600  
 504 593 857 908 095 236 820 172 800  $q^{1865} +$   
 31 720 994 934 284 152 537 910 261 297 011 741 283 102 578 645 111 329 015 655 807 731 601 669 311  
 563 659 112 814 519 652 109 231 616  $q^{1868} -$   
 33 772 680 764 178 842 136 899 711 960 299 400 436 202 973 336 059 376 453 596 571 455 483 860 903  
 281 498 217 227 756 547 085 358 375  $q^{1869} +$   
 40 754 752 819 259 516 526 495 499 815 166 857 510 609 796 405 286 258 339 090 298 961 578 549 141  
 093 865 062 423 869 287 349 403 648  $q^{1872} -$   
 43 387 840 422 467 484 788 006 021 416 103 646 255 026 443 152 484 776 854 970 874 796 833 624 470  
 926 535 198 918 366 360 548 376 576  $q^{1873} +$   
 52 347 266 796 658 302 596 265 031 880 769 812 617 615 643 631 278 145 723 629 798 256 727 907 069  
 930 070 862 651 167 938 273 280 000  $q^{1876} -$   
 55 725 620 163 688 228 824 046 643 288 853 011 637 948 632 708 799 933 690 201 667 196 274 101 764  
 289 915 723 530 576 737 862 094 616  $q^{1877} +$   
 67 219 365 933 661 829 308 520 112 167 267 495 459 698 921 621 785 853 116 732 406 582 243 873 473  
 292 481 920 790 638 954 350 873 600  $q^{1880} -$   
 71 552 783 298 527 693 681 111 134 767 471 344 874 175 188 258 563 125 619 468 306 484 305 688 342  
 731 908 994 875 546 957 737 984 000  $q^{1881} +$   
 86 293 847 420 405 662 366 613 629 834 139 655 994 414 872 809 186 219 354 288 659 301 200 267 026  
 670 513 876 913 500 973 925 120 000  $q^{1884} -$   
 91 850 868 032 634 693 312 244 416 342 857 664 255 730 552 851 739 118 547 137 763 562 389 924 171  
 751 443 148 465 206 495 843 764 775  $q^{1885} +$   
 110 751 760 536 893 116 722 637 982 030 016 348 082 921 321 710 952 494 842 162 614 866 437 963 248  
 833 305 541 570 571 070 974 488 576  $q^{1888} -$   
 117 876 022 812 955 444 941 316 860 390 430 713 819 001 665 754 472 308 974 325 819 479 561 139 403  
 266 348 150 759 825 023 148 032 000  $q^{1889} +$   
 142 104 291 249 005 119 267 036 971 314 762 575 167 491 866 635 725 156 187 741 269 542 945 569 639  
 883 261 646 813 908 769 795 063 808  $q^{1892} -$   
 151 235 421 822 447 176 389 748 604 690 314 607 883 119 825 302 967 524 674 862 867 504 127 347 936  
 238 714 161 620 031 066 254 908 654  $q^{1893} +$   
 182 284 548 333 105 121 890 030 094 672 773 866 234 043 399 970 990 522 278 716 082 269 455 242 350  
 697 430 761 532 617 193 714 048 000  $q^{1896} -$   
 193 984 830 237 523 489 117 593 242 707 153 287 487 962 273 216 142 435 015 546 817 203 824 912 389  
 218 767 033 444 856 458 571 284 480  $q^{1897} +$   
 233 764 731 272 705 851 132 491 499 888 573 707 668 771 081 112 113 796 177 440 857 587 307 475 426  
 129 507 686 607 594 368 959 244 800  $q^{1900} -$   
 248 753 141 529 075 152 011 532 483 377 648 294 436 762 550 057 744 599 457 013 026 801 426 781 809  
 839 564 799 820 494 981 817 647 750  $q^{1901} +$   
 299 705 661 169 374 553 574 706 650 527 132 338 019 438 340 753 837 914 705 481 893 123 720 390 720  
 727 463 700 917 861 692 362 752 000  $q^{1904} -$   
 318 901 303 309 204 253 909 990 502 669 043 909 124 824 405 491 108 147 338 765 602 771 492 165 809  
 865 903 089 147 224 190 954 700 800  $q^{1905} +$   
 384 147 565 822 854 836 386 868 707 282 008 442 369 693 314 214 042 916 997 147 299 647 861 150 962  
 509 523 808 273 694 681 660 442 624  $q^{1908} -$   
 408 725 076 633 394 661 941 747 606 793 363 080 666 741 373 141 661 563 954 998 945 907 792 737 755  
 192 932 259 705 784 184 584 825 125  $q^{1909} +$   
 492 253 439 767 283 548 119 970 184 863 691 686 683 571 295 172 321 084 613 272 871 222 100 077 510  
 892 903 120 999 904 054 211 258 368  $q^{1912} -$

523 713 653 881 374 633 810 214 185 354 085 501 773 370 668 302 409 336 241 079 731 268 214 360 901  
 208 828 766 885 643 055 393 046 528  $q^{1913} +$   
 630 619 390 071 663 102 116 211 734 258 647 087 025 296 857 597 258 583 397 196 912 708 938 449 271  
 749 704 890 288 704 551 874 560 000  $q^{1916} -$   
 670 879 441 672 133 451 051 467 165 958 651 164 126 734 370 863 399 953 647 265 358 895 109 412 021  
 131 012 790 222 815 864 953 630 199  $q^{1917} +$   
 807 670 307 665 749 099 596 473 532 709 029 792 096 111 550 275 957 226 894 176 933 650 644 437 643  
 356 357 714 560 322 435 909 222 400  $q^{1920} -$   
 859 178 487 219 642 283 341 223 526 870 953 575 804 995 663 418 522 500 268 717 852 992 361 700 004  
 303 800 811 017 004 523 036 672 000  $q^{1921} +$   
 1 034 164 198 393 591 488 767 396 678 645 949 694 351 672 589 493 954 704 075 920 892 726 342 367 237  
 484 322 771 115 935 081 791 488 000  $q^{1924} -$   
 1 100 046 329 552 511 327 519 051 843 541 839 915 247 559 044 657 399 369 645 413 495 718 895 740 927  
 796 851 540 986 032 362 866 380 325  $q^{1925} +$   
 1 323 834 855 340 061 238 370 389 689 770 988 582 362 997 142 834 930 130 538 153 392 018 903 295 914  
 266 069 476 651 104 062 687 820 800  $q^{1928} -$   
 1 408 080 796 120 466 395 842 433 092 531 475 832 230 771 732 418 963 712 674 438 229 152 989 801 274  
 350 771 127 035 989 942 693 888 000  $q^{1929} +$   
 1 694 210 618 753 268 494 210 050 271 541 919 824 074 432 399 452 592 974 866 833 644 411 276 025 363  
 429 087 625 559 634 628 619 331 584  $q^{1932} -$   
 1 801 911 827 329 452 889 929 504 293 480 776 908 875 933 698 606 783 620 920 758 285 893 340 636 103  
 047 730 217 320 214 056 918 978 409  $q^{1933} +$   
 2 167 657 214 331 678 177 592 899 797 524 603 903 604 302 547 712 780 472 311 025 199 049 461 117 934  
 438 151 200 192 368 782 020 938 752  $q^{1936} -$   
 2 305 309 286 971 908 600 817 864 657 527 174 128 747 388 394 036 617 588 627 696 977 506 784 234 078  
 221 565 483 425 748 719 778 660 352  $q^{1937} +$   
 2 772 705 670 741 560 666 349 767 860 045 215 054 163 897 538 144 939 123 999 204 061 752 681 467 699  
 546 521 111 431 867 733 076 889 600  $q^{1940} -$   
 2 948 593 527 111 729 343 162 953 339 369 661 117 698 194 578 912 927 634 929 422 880 761 263 123 581  
 953 396 165 915 194 108 717 470 625  $q^{1941} +$   
 3 545 742 835 664 574 959 531 192 873 641 188 556 952 275 638 298 340 138 096 810 032 462 229 181 631  
 871 956 541 478 367 587 185 856 000  $q^{1944} -$   
 3 770 431 009 732 887 977 986 677 736 409 096 492 142 162 418 836 410 984 249 624 345 619 905 903 052  
 214 142 220 406 578 485 605 171 200  $q^{1945} +$   
 4 533 162 977 521 873 106 513 774 459 960 725 899 004 344 778 375 568 674 144 006 670 908 984 067 093  
 012 965 839 841 095 328 220 866 560  $q^{1948} -$   
 4 820 119 542 786 156 443 047 185 761 674 302 570 930 308 288 445 978 929 359 713 966 376 065 531 160  
 506 965 023 508 434 834 155 480 000  $q^{1949} +$   
 5 794 105 569 459 162 386 473 004 286 401 014 762 025 720 326 340 486 004 095 681 212 456 461 983 835  
 443 271 939 863 130 647 110 176 768  $q^{1952} -$   
 6 160 495 929 920 632 075 684 597 420 276 086 647 083 092 900 748 029 404 552 054 383 382 001 213 968  
 358 588 628 773 103 268 184 784 896  $q^{1953} +$   
 7 403 938 113 138 534 739 735 169 313 029 021 634 485 587 425 390 886 890 078 108 793 186 670 126 492  
 336 153 239 857 634 199 365 632 000  $q^{1956} -$   
 7 871 634 662 918 706 297 877 426 196 908 690 173 401 677 804 960 351 819 508 607 934 804 361 450 710  
 648 136 482 026 831 609 315 509 565  $q^{1957} +$   
 9 458 685 684 298 562 287 275 264 085 927 562 718 172 178 381 583 012 114 261 845 082 796 169 622 810  
 132 078 052 106 120 116 494 758 400  $q^{1960} -$   
 10 055 551 731 745 193 227 851 423 525 551 123 881 464 247 327 556 466 348 107 075 961 782 812 723  
 208 034 374 849 022 875 477 164 032 000  $q^{1961} +$   
 12 080 663 190 309 807 662 657 525 907 991 616 200 885 700 083 418 618 737 491 232 380 298 390 598  
 918 215 406 593 895 024 648 165 184 000  $q^{1964} -$   
 12 842 185 256 459 243 262 327 661 920 285 169 416 861 074 129 943 274 100 574 604 157 623 341 728  
 516 698 899 820 472 596 833 499 438 650  $q^{1965} +$   
 15 425 635 185 443 070 855 472 834 973 261 762 482 200 893 677 109 077 921 544 544 631 495 699 484

826 421 253 487 937 746 848 205 135 872  $q^{1968}$  -  
 16 396 997 707 119 937 927 563 003 049 898 065 815 673 941 267 825 143 591 221 502 715 458 125 872  
 888 290 079 632 748 319 611 359 232 000  $q^{1969}$  +  
 19 691 915 368 549 794 857 329 179 724 541 160 432 381 764 271 145 034 458 718 514 076 041 873 489  
 672 088 142 670 626 251 777 425 666 048  $q^{1972}$  -  
 20 930 637 083 281 451 670 053 130 203 744 919 033 493 004 310 273 814 782 055 689 347 684 757 244  
 074 080 918 909 719 393 784 841 678 873  $q^{1973}$  +  
 25 131 928 494 069 292 395 359 241 794 960 148 329 260 535 960 714 955 965 337 798 962 364 268 435  
 643 579 693 546 040 465 122 593 152 000  $q^{1976}$  -  
 26 711 211 774 165 504 493 528 198 584 971 805 106 887 903 697 094 232 512 746 353 734 977 778 427  
 899 028 200 949 850 090 749 256 171 520  $q^{1977}$  +  
 32 066 897 562 869 740 379 637 634 176 912 756 133 062 017 160 526 993 842 543 361 305 355 218 095  
 976 076 107 030 384 015 696 523 008 000  $q^{1980}$  -  
 34 079 882 491 148 649 225 487 550 019 904 388 876 593 069 175 723 683 112 466 226 396 208 420 854  
 904 755 390 094 926 251 965 894 229 000  $q^{1981}$  +  
 40 905 496 666 942 273 286 668 139 660 843 652 675 051 478 421 615 577 757 408 193 080 622 421 460  
 192 662 183 917 620 966 715 719 680 000  $q^{1984}$  -  
 43 470 662 971 919 460 503 989 422 969 438 038 519 327 274 123 672 482 602 455 846 968 414 783 369  
 220 777 803 100 560 125 033 871 769 600  $q^{1985}$  +  
 52 167 534 655 951 079 896 039 071 818 921 636 977 128 322 314 787 720 101 760 334 490 573 673 368  
 704 832 011 784 740 272 239 742 648 320  $q^{1988}$  -  
 55 435 559 613 182 888 613 144 735 964 934 739 739 391 200 750 665 976 749 638 634 240 861 113 012  
 428 148 016 281 766 204 059 923 479 750  $q^{1989}$  +  
 66 514 019 405 236 547 239 631 650 721 647 264 533 938 921 067 714 963 585 486 081 986 788 688 911  
 417 770 746 533 959 871 085 357 076 480  $q^{1992}$  -  
 70 676 482 082 431 337 803 285 461 010 814 230 510 307 485 635 884 618 736 304 589 658 213 379 912  
 597 950 305 161 454 252 816 468 606 976  $q^{1993}$  +  
 84 785 312 728 768 780 256 502 069 081 849 725 413 327 833 036 069 447 022 213 229 509 668 301 693  
 601 554 427 011 539 686 173 944 000 000  $q^{1996}$  -  
 90 085 739 077 072 720 637 256 103 447 902 141 332 032 328 589 457 464 651 099 828 258 855 904 657  
 158 497 614 875 108 339 445 251 353 244  $q^{1997}$  +  
 108 049 541 901 398 838 513 652 810 574 395 940 556 222 527 513 783 066 788 496 230 416 692 801 656  
 136 485 592 540 870 160 978 608 947 200  $q^{2000}$  -  
 114 797 416 948 913 907 080 069 325 683 795 750 999 931 246 499 001 130 257 746 719 610 569 995 523  
 830 757 016 045 145 684 114 718 720 000  $q^{2001}$  +  
 137 664 010 599 581 906 515 043 131 256 121 112 781 896 960 327 747 596 227 402 547 450 312 366 715  
 519 107 224 070 610 784 434 380 800 000  $q^{2004}$  -  
 146 252 550 678 833 899 715 122 688 576 265 802 828 869 404 203 699 825 549 891 971 928 671 163 289  
 178 911 852 470 456 912 580 229 765 000  $q^{2005}$  +  
 175 353 081 745 110 884 989 960 633 311 322 454 795 641 302 038 470 781 942 629 315 621 978 797 536  
 982 584 472 833 542 295 929 837 183 488  $q^{2008}$  -  
 186 281 770 492 208 580 211 932 707 719 486 239 818 976 548 598 133 193 521 509 803 471 967 669 319  
 618 899 458 784 445 445 445 230 592 000  $q^{2009}$  +  
 223 306 927 524 078 810 438 318 715 533 674 063 124 215 453 526 956 366 324 233 577 229 967 192 271  
 926 678 876 123 507 300 621 673 342 976  $q^{2012}$  -  
 237 210 085 947 590 416 986 232 808 314 304 788 204 736 768 569 991 957 782 189 233 143 761 225 732  
 566 656 598 852 633 415 087 918 270 561  $q^{2013}$  +  
 284 306 708 597 360 340 439 256 633 300 248 536 203 600 970 718 749 625 947 049 168 731 748 310 667  
 434 669 076 040 244 695 828 300 800 000  $q^{2016}$  -  
 301 989 706 499 302 031 940 159 125 849 180 870 909 341 608 005 042 269 438 571 899 881 134 824 561  
 847 983 002 179 553 001 056 136 298 496  $q^{2017}$  +  
 361 883 219 381 005 922 517 718 440 136 003 430 193 736 126 556 680 844 846 364 940 983 317 299 475  
 711 215 953 418 123 811 531 521 228 800  $q^{2020}$  -  
 384 368 361 330 576 576 650 696 492 943 972 316 837 335 770 661 227 935 886 636 190 819 870 764 871  
 202 343 723 673 626 947 831 285 209 000  $q^{2021}$  +

460 517 900 204 581 154 406 586 533 573 937 761 625 661 640 997 534 972 585 102 972 576 430 171 255 3  
 633 446 662 231 900 165 642 423 936 000  $q^{2024}$  -  
 489 102 557 467 114 582 502 907 559 713 628 280 954 534 305 108 827 316 125 059 060 839 298 209 292 3  
 386 236 747 831 708 925 854 894 948 600  $q^{2025}$  +  
 585 897 472 259 972 955 543 593 008 128 824 493 118 627 669 934 302 466 620 403 850 671 785 494 442 3  
 868 130 848 265 056 196 198 031 977 984  $q^{2028}$  -  
 622 227 712 017 724 974 516 986 797 096 264 806 673 061 393 580 195 009 160 064 336 445 177 976 083 3  
 526 061 668 982 894 820 856 241 289 375  $q^{2029}$  +  
 745 236 426 299 269 504 875 003 311 519 484 426 153 116 220 037 000 249 054 444 658 132 405 766 083 3  
 759 517 367 067 254 058 443 369 611 264  $q^{2032}$  -  
 791 400 248 299 693 598 761 932 306 927 577 310 051 986 646 955 472 556 908 181 959 539 043 772 481 3  
 182 714 333 276 107 952 344 349 245 440  $q^{2033}$  +  
 947 685 353 379 039 259 211 789 877 126 502 106 436 725 804 830 499 089 246 866 650 882 371 047 030 3  
 349 746 291 023 037 816 646 152 960 000  $q^{2036}$  -  
 1 006 330 728 621 208 754 979 462 862 963 910 236 111 561 112 500 892 451 642 630 882 050 750 154 533 3  
 554 414 040 714 702 911 762 246 507 128  $q^{2037}$  +  
 1 204 847 850 229 411 271 849 009 483 377 820 355 687 604 909 051 358 497 646 113 381 900 760 656 331 3  
 889 151 041 480 244 623 908 791 398 400  $q^{2040}$  -  
 1 279 332 125 449 544 197 670 196 477 832 813 113 483 324 529 456 758 361 139 158 202 980 373 376 799 3  
 413 903 036 454 680 305 305 337 856 000  $q^{2041}$  +  
 1 531 434 720 962 237 376 062 686 119 070 296 284 763 966 971 055 401 971 422 324 264 616 980 828 708 3  
 638 504 524 653 368 483 097 053 184 000  $q^{2044}$  -  
 1 626 013 680 849 683 166 542 213 512 537 171 915 415 069 597 217 580 511 936 979 465 460 160 470 418 3  
 893 646 172 800 869 327 995 130 326 450  $q^{2045}$  +  
 1 946 091 755 789 895 070 954 022 806 532 821 679 533 671 796 417 592 927 118 601 292 606 982 318 996 3  
 583 299 164 903 052 471 216 091 693 056  $q^{2048}$  -  
 2 066 158 815 716 653 024 017 818 518 169 505 774 958 429 982 214 883 352 642 419 420 417 310 052 974 3  
 728 205 524 014 350 489 080 680 448 000  $q^{2049}$  +  
 2 472 446 905 569 984 966 991 408 507 696 366 128 693 557 092 353 141 774 400 325 037 516 245 387 606 3  
 235 689 443 874 423 332 807 284 031 488  $q^{2052}$  -  
 2 624 835 659 120 646 498 093 936 477 759 453 336 253 044 150 497 357 352 464 199 228 439 641 707 632 3  
 499 750 293 324 485 340 974 874 764 927  $q^{2053}$  +  
 3 140 434 703 892 394 362 472 583 850 243 480 829 527 985 634 700 770 452 621 345 195 593 332 097 844 3  
 643 814 586 109 717 869 647 512 064 000  $q^{2056}$  -  
 3 333 801 520 195 096 658 148 846 761 629 820 630 059 785 306 652 635 546 766 504 119 892 680 652 207 3  
 603 921 058 995 676 011 676 346 974 208  $q^{2057}$  +  
 3 987 970 965 274 990 737 497 893 836 491 753 862 573 885 811 409 338 668 653 939 690 639 612 668 949 3  
 569 050 429 241 574 673 344 903 961 600  $q^{2060}$  -  
 4 233 278 708 092 342 966 394 637 250 967 805 836 849 554 825 071 696 367 496 103 239 201 471 580 617 3  
 926 763 317 330 801 555 794 638 705 625  $q^{2061}$  +  
 5 063 069 926 097 496 033 663 274 048 239 548 586 894 159 085 083 748 862 069 326 943 013 609 788 655 3  
 822 400 415 906 729 281 593 753 600 000  $q^{2064}$  -  
 5 374 199 385 266 372 678 097 022 579 983 102 972 680 343 223 781 241 595 375 652 116 879 166 737 356 3  
 033 005 449 868 061 697 848 100 454 400  $q^{2065}$  +  
 6 426 520 122 811 411 353 839 203 611 546 996 959 666 335 250 259 283 562 046 103 315 672 758 948 244 3  
 872 886 941 060 789 551 840 487 370 752  $q^{2068}$  -  
 6 821 042 705 198 001 797 067 272 369 738 796 889 474 119 703 870 756 522 171 789 018 432 037 310 246 3  
 849 717 352 481 986 566 446 012 393 250  $q^{2069}$  +  
 8 155 265 714 102 957 472 465 278 487 452 141 712 339 786 692 172 673 245 453 337 646 761 361 473 453 3  
 368 581 325 416 839 801 638 825 480 192  $q^{2072}$  -  
 8 655 419 708 537 102 570 022 256 866 698 337 054 966 170 642 893 654 162 509 434 806 467 371 534 213 3  
 074 909 762 595 668 070 647 013 081 088  $q^{2073}$  +  
 10 346 678 278 507 189 133 417 316 482 037 565 308 976 266 260 008 822 356 226 992 829 050 886 722 3  
 197 071 722 212 855 959 741 149 808 384 000  $q^{2076}$  -  
 10 980 602 056 097 858 986 311 985 854 724 634 137 586 351 226 740 696 065 157 099 644 878 709 412 3

$556\ 291\ 108\ 735\ 198\ 930\ 031\ 730\ 917\ 166\ 361\ q^{2077} +$   
 $13\ 123\ 952\ 404\ 773\ 360\ 106\ 299\ 528\ 224\ 139\ 027\ 696\ 469\ 903\ 182\ 201\ 544\ 125\ 879\ 696\ 143\ 552\ 421\ 516\ q^{2080} -$   
 $613\ 218\ 102\ 116\ 775\ 449\ 051\ 191\ 537\ 459\ 200\ q^{2081} +$   
 $13\ 927\ 241\ 832\ 325\ 971\ 286\ 939\ 447\ 131\ 932\ 748\ 955\ 270\ 347\ 660\ 438\ 509\ 094\ 660\ 679\ 461\ 760\ 938\ 693\ q^{2084} -$   
 $281\ 247\ 895\ 367\ 294\ 147\ 872\ 771\ 239\ 936\ 000\ q^{2085} +$   
 $16\ 642\ 919\ 214\ 907\ 709\ 575\ 118\ 469\ 560\ 076\ 380\ 849\ 413\ 915\ 970\ 276\ 388\ 917\ 812\ 148\ 882\ 181\ 283\ 721\ q^{2088} -$   
 $648\ 867\ 269\ 458\ 148\ 054\ 684\ 580\ 634\ 624\ 000\ q^{2089} +$   
 $17\ 660\ 594\ 086\ 398\ 529\ 891\ 355\ 696\ 083\ 247\ 524\ 288\ 808\ 094\ 575\ 379\ 752\ 677\ 153\ 711\ 081\ 702\ 512\ 655\ q^{2092} -$   
 $307\ 225\ 939\ 490\ 978\ 684\ 227\ 486\ 693\ 223\ 650\ q^{2093} +$   
 $21\ 100\ 648\ 557\ 842\ 507\ 927\ 048\ 005\ 273\ 621\ 842\ 553\ 243\ 786\ 542\ 611\ 157\ 239\ 753\ 104\ 873\ 275\ 470\ 860\ q^{2096} -$   
 $525\ 850\ 164\ 076\ 799\ 832\ 388\ 872\ 138\ 102\ 272\ q^{2097} +$   
 $22\ 389\ 634\ 919\ 257\ 261\ 953\ 699\ 027\ 689\ 986\ 112\ 170\ 785\ 797\ 553\ 977\ 412\ 980\ 385\ 317\ 407\ 861\ 365\ 576\ q^{2100} -$   
 $078\ 105\ 540\ 813\ 362\ 345\ 843\ 749\ 171\ 200\ 000\ q^{2101} +$   
 $26\ 746\ 307\ 056\ 051\ 337\ 896\ 887\ 658\ 505\ 080\ 838\ 666\ 870\ 169\ 771\ 204\ 144\ 085\ 595\ 305\ 889\ 407\ 499\ 366\ q^{2104} -$   
 $312\ 258\ 545\ 398\ 708\ 671\ 157\ 389\ 179\ 255\ 296\ q^{2105} +$   
 $28\ 378\ 570\ 084\ 010\ 798\ 548\ 913\ 655\ 331\ 770\ 354\ 360\ 511\ 570\ 624\ 257\ 650\ 484\ 154\ 803\ 262\ 221\ 519\ 044\ q^{2108} -$   
 $831\ 758\ 649\ 303\ 556\ 225\ 647\ 838\ 434\ 149\ 452\ q^{2109} +$   
 $33\ 894\ 860\ 594\ 341\ 826\ 380\ 087\ 895\ 608\ 530\ 570\ 529\ 946\ 676\ 588\ 090\ 713\ 202\ 237\ 633\ 557\ 699\ 213\ 947\ q^{2112} -$   
 $995\ 838\ 810\ 095\ 654\ 999\ 080\ 370\ 138\ 624\ 000\ q^{2113} +$   
 $35\ 961\ 357\ 661\ 101\ 938\ 512\ 313\ 742\ 335\ 859\ 158\ 378\ 179\ 645\ 898\ 111\ 991\ 050\ 653\ 674\ 985\ 221\ 955\ 621\ q^{2116} -$   
 $747\ 236\ 899\ 894\ 212\ 528\ 358\ 385\ 204\ 363\ 264\ q^{2117} +$   
 $42\ 944\ 362\ 637\ 959\ 759\ 984\ 546\ 339\ 446\ 564\ 882\ 013\ 442\ 373\ 085\ 445\ 766\ 607\ 539\ 069\ 295\ 845\ 240\ 960\ q^{2120} -$   
 $092\ 440\ 742\ 896\ 014\ 470\ 985\ 692\ 210\ 073\ 600\ q^{2121} +$   
 $45\ 560\ 030\ 204\ 266\ 096\ 763\ 112\ 304\ 211\ 037\ 695\ 024\ 734\ 141\ 068\ 116\ 991\ 811\ 911\ 348\ 410\ 093\ 231\ 491\ q^{2124} -$   
 $151\ 113\ 987\ 162\ 250\ 191\ 064\ 578\ 731\ 193\ 875\ q^{2125} +$   
 $54\ 397\ 762\ 031\ 634\ 712\ 785\ 183\ 337\ 417\ 492\ 194\ 973\ 777\ 792\ 239\ 742\ 360\ 924\ 256\ 935\ 324\ 848\ 038\ 018\ q^{2128} -$   
 $024\ 431\ 447\ 627\ 260\ 087\ 115\ 748\ 731\ 776\ 000\ q^{2129} +$   
 $57\ 707\ 805\ 377\ 853\ 954\ 476\ 315\ 502\ 082\ 096\ 362\ 477\ 241\ 304\ 907\ 924\ 942\ 410\ 067\ 102\ 362\ 322\ 264\ 067\ q^{2132} -$   
 $028\ 744\ 924\ 055\ 294\ 288\ 765\ 010\ 418\ 073\ 600\ q^{2133} +$   
 $68\ 890\ 405\ 804\ 966\ 135\ 984\ 231\ 621\ 530\ 382\ 478\ 219\ 188\ 098\ 810\ 988\ 826\ 751\ 715\ 445\ 788\ 042\ 836\ 401\ q^{2136} -$   
 $806\ 921\ 114\ 886\ 428\ 776\ 987\ 897\ 727\ 033\ 344\ q^{2137} +$   
 $73\ 078\ 230\ 257\ 555\ 448\ 160\ 847\ 611\ 878\ 410\ 310\ 719\ 259\ 851\ 830\ 105\ 506\ 018\ 457\ 414\ 757\ 551\ 033\ 161\ q^{2140} -$   
 $969\ 341\ 329\ 415\ 002\ 784\ 911\ 439\ 963\ 331\ 750\ q^{2141} +$   
 $87\ 224\ 716\ 728\ 792\ 856\ 811\ 972\ 251\ 919\ 171\ 952\ 226\ 422\ 353\ 264\ 678\ 374\ 571\ 827\ 711\ 870\ 282\ 622\ 161\ q^{2144} -$   
 $837\ 663\ 202\ 119\ 664\ 669\ 314\ 778\ 833\ 879\ 040\ q^{2145} +$   
 $92\ 521\ 926\ 626\ 736\ 871\ 318\ 624\ 024\ 633\ 219\ 102\ 632\ 619\ 032\ 501\ 918\ 423\ 860\ 405\ 063\ 856\ 525\ 097\ 958\ q^{2148} -$   
 $564\ 262\ 234\ 728\ 008\ 989\ 449\ 765\ 936\ 037\ 888\ q^{2149} +$   
 $110\ 413\ 907\ 921\ 484\ 866\ 662\ 324\ 376\ 691\ 499\ 230\ 378\ 446\ 925\ 214\ 379\ 629\ 464\ 613\ 978\ 174\ 943\ 654\ 724\ q^{2152} -$   
 $277\ 576\ 708\ 875\ 959\ 960\ 959\ 906\ 639\ 898\ 752\ q^{2153} +$   
 $117\ 112\ 909\ 694\ 233\ 533\ 839\ 048\ 732\ 610\ 742\ 558\ 999\ 565\ 828\ 802\ 608\ 021\ 225\ 859\ 830\ 470\ 873\ 727\ 958\ q^{2156} -$   
 $023\ 990\ 472\ 230\ 021\ 138\ 726\ 801\ 607\ 158\ 814\ q^{2157} +$   
 $139\ 737\ 077\ 763\ 286\ 925\ 791\ 855\ 390\ 281\ 577\ 680\ 207\ 847\ 505\ 464\ 040\ 103\ 794\ 384\ 785\ 426\ 898\ 349\ 014\ q^{2160} -$   
 $666\ 070\ 552\ 420\ 594\ 165\ 629\ 612\ 089\ 420\ 800\ q^{2161} +$   
 $148\ 206\ 961\ 929\ 078\ 946\ 723\ 657\ 242\ 986\ 705\ 175\ 429\ 612\ 513\ 064\ 995\ 341\ 269\ 064\ 283\ 728\ 174\ 678\ 940\ q^{2164} -$   
 $826\ 086\ 293\ 991\ 388\ 949\ 729\ 412\ 849\ 664\ 000\ q^{2165} +$   
 $176\ 808\ 632\ 927\ 045\ 666\ 981\ 088\ 094\ 872\ 293\ 668\ 844\ 008\ 683\ 020\ 007\ 652\ 958\ 852\ 807\ 211\ 706\ 106\ 727\ q^{2168} -$   
 $901\ 300\ 964\ 883\ 910\ 535\ 642\ 143\ 840\ 320\ 000\ q^{2169} +$   
 $187\ 515\ 183\ 809\ 699\ 776\ 853\ 139\ 055\ 716\ 788\ 360\ 713\ 237\ 925\ 276\ 748\ 429\ 284\ 628\ 232\ 751\ 782\ 409\ 690\ q^{2172} -$   
 $043\ 647\ 898\ 329\ 723\ 492\ 448\ 244\ 152\ 454\ 125\ q^{2173} +$   
 $223\ 665\ 747\ 075\ 000\ 967\ 852\ 643\ 542\ 836\ 774\ 862\ 075\ 620\ 552\ 282\ 082\ 461\ 551\ 167\ 438\ 861\ 861\ 927\ 693\ q^{2176} -$   
 $926\ 838\ 951\ 389\ 303\ 456\ 293\ 944\ 091\ 049\ 984\ q^{2177} +$   
 $237\ 196\ 647\ 662\ 694\ 021\ 925\ 410\ 940\ 058\ 783\ 841\ 089\ 654\ 436\ 820\ 074\ 936\ 747\ 597\ 379\ 168\ 415\ 384\ 811\ q^{2180} -$   
 $040\ 022\ 167\ 374\ 607\ 330\ 255\ 664\ 701\ 440\ 000\ q^{2181} +$   
 $282\ 878\ 517\ 343\ 249\ 200\ 364\ 314\ 249\ 690\ 672\ 501\ 502\ 803\ 834\ 954\ 911\ 587\ 528\ 226\ 481\ 508\ 551\ 688\ 343\ q^{2184} -$   
 $865\ 395\ 450\ 445\ 296\ 457\ 174\ 331\ 547\ 283\ 456\ q^{2185} +$

299 975 091 368 582 408 809 494 507 043 117 176 032 488 168 387 485 699 241 552 326 615 420 075 144 3  
 004 931 003 285 814 529 789 462 007 142 303  $q^{2133} +$   
 357 688 679 851 778 637 935 363 360 331 197 990 423 473 719 831 950 878 572 184 963 717 706 162 923 3  
 902 971 478 849 521 485 466 995 074 432 000  $q^{2136} -$   
 379 285 858 146 703 827 627 152 094 878 700 183 409 686 498 229 032 201 089 482 463 140 426 046 447 3  
 752 331 511 988 347 340 708 824 895 193 088  $q^{2137} +$   
 452 184 251 474 434 575 735 771 192 739 437 792 837 314 950 827 369 065 149 893 664 838 504 126 617 3  
 527 326 059 098 871 121 526 630 880 512 000  $q^{2140} -$   
 479 460 882 859 961 231 252 513 858 931 980 378 933 399 426 249 969 389 282 618 161 511 206 670 848 3  
 156 158 708 166 179 208 904 962 861 342 000  $q^{2141} +$   
 571 519 356 126 318 453 097 801 821 475 287 544 762 717 667 834 472 854 763 799 961 244 131 003 899 3  
 383 145 438 207 477 390 354 077 894 144 000  $q^{2144} -$   
 605 961 526 989 731 889 115 441 916 153 254 471 511 020 269 480 702 761 325 738 843 492 555 452 877 3  
 507 500 397 548 644 992 029 691 563 212 800  $q^{2145} +$   
 722 190 867 823 498 980 138 643 667 698 660 095 648 914 939 948 839 834 592 045 339 688 966 641 869 3  
 843 911 003 716 927 394 548 278 234 693 632  $q^{2148} -$   
 765 671 577 255 566 991 475 659 798 998 668 099 418 602 731 161 720 838 613 464 749 432 984 231 795 3  
 511 335 155 868 086 383 604 424 585 671 125  $q^{2149} +$   
 912 386 482 482 420 432 782 805 522 108 158 513 999 535 022 217 676 537 268 253 733 591 672 761 966 3  
 757 289 858 031 978 308 597 052 606 602 752  $q^{2152} -$   
 967 265 876 653 066 068 802 128 554 803 902 669 662 924 782 914 805 244 511 012 020 665 474 113 635 3  
 185 960 788 709 539 246 947 721 961 144 320  $q^{2153} +$   
 1 152 422 569 633 136 800 165 079 770 067 282 520 518 856 194 434 585 412 208 555 581 123 331 073 722 3  
 168 272 641 481 098 252 194 745 862 976 000  $q^{2156} -$   
 1 221 674 014 146 435 802 358 703 417 418 268 525 667 698 433 389 506 031 502 533 202 323 632 127 207 3  
 826 355 481 615 290 764 155 610 275 752 965  $q^{2157} +$   
 1 455 294 846 548 742 142 592 790 507 710 611 747 871 249 662 011 557 725 393 071 858 263 777 537 618 3  
 328 013 398 276 496 593 011 859 401 932 800  $q^{2160} -$   
 1 542 663 464 158 625 824 745 847 408 441 854 629 526 160 763 200 341 394 077 807 388 435 443 887 807 3  
 924 256 056 314 663 690 588 070 318 080 000  $q^{2161} +$   
 1 837 370 801 983 956 537 227 123 006 273 532 703 550 637 958 285 825 346 176 489 860 328 049 000 520 3  
 488 676 175 464 734 563 213 640 499 456 000  $q^{2164} -$   
 1 947 572 794 545 603 081 411 996 392 193 649 290 148 732 316 509 732 960 207 684 870 941 665 177 991 3  
 686 784 782 892 223 545 356 843 478 251 625  $q^{2165} +$   
 2 319 260 176 831 290 877 083 363 187 399 352 301 898 783 438 829 581 507 069 204 020 193 215 927 591 3  
 776 087 603 140 852 966 188 208 437 123 072  $q^{2168} -$   
 2 458 233 371 439 871 497 040 786 716 514 229 072 191 415 681 855 561 401 350 067 898 291 278 666 954 3  
 694 624 427 218 108 871 786 131 435 520 000  $q^{2169} +$   
 2 926 909 062 686 493 389 422 109 692 112 728 732 399 934 308 368 820 805 114 819 484 202 288 262 372 3  
 199 916 753 187 357 122 490 773 212 555 264  $q^{2172} -$   
 3 102 127 781 176 205 683 746 274 323 799 481 741 331 822 941 575 541 773 666 626 199 181 803 089 488 3  
 607 584 657 888 623 588 583 459 465 850 444  $q^{2173} +$   
 3 692 974 779 857 373 809 737 151 804 587 511 397 254 974 890 086 583 323 118 381 900 193 324 907 545 3  
 990 495 923 171 004 725 134 119 821 312 000  $q^{2176} -$   
 3 913 845 464 060 867 282 936 044 774 339 638 381 526 283 531 007 777 088 313 207 663 073 257 850 839 3  
 290 243 191 041 781 741 424 047 267 053 568  $q^{2177} +$   
 4 658 553 236 014 674 861 297 083 250 217 010 421 624 508 032 173 477 850 978 406 446 636 440 696 146 3  
 051 135 029 557 987 330 691 447 398 400 000  $q^{2180} -$   
 4 936 911 438 408 489 325 183 690 107 224 316 865 556 048 862 393 170 321 181 413 732 496 837 986 768 3  
 341 617 066 645 222 613 036 401 469 830 000  $q^{2181} +$   
 5 875 348 686 464 303 797 724 217 309 482 282 538 903 659 724 141 461 149 492 172 189 129 790 554 791 3  
 164 145 105 418 826 296 390 166 814 976 000  $q^{2184} -$   
 6 226 083 269 705 650 362 898 028 953 005 036 467 444 625 349 030 531 189 010 731 898 229 835 176 651 3  
 010 694 844 622 563 313 242 756 892 262 400  $q^{2185} +$   
 7 408 398 643 807 970 718 227 162 449 509 407 841 410 464 263 421 801 629 651 725 711 190 287 515 529 3

$033\ 028\ 104\ 286\ 458\ 327\ 610\ 609\ 275\ 162\ 112\ q^{2188} -$   
 $7\ 850\ 235\ 589\ 176\ 148\ 380\ 534\ 087\ 574\ 618\ 566\ 961\ 719\ 289\ 560\ 906\ 521\ 867\ 872\ 475\ 083\ 783\ 519\ 254\ 454\ q^{2189} +$   
 $9\ 339\ 495\ 277\ 750\ 519\ 525\ 563\ 333\ 794\ 377\ 959\ 019\ 614\ 851\ 450\ 197\ 486\ 191\ 593\ 475\ 591\ 543\ 666\ 456\ 301\ q^{2192} -$   
 $9\ 895\ 981\ 714\ 237\ 448\ 077\ 507\ 477\ 263\ 808\ 304\ 294\ 637\ 249\ 070\ 105\ 153\ 421\ 981\ 983\ 434\ 191\ 622\ 846\ 487\ q^{2193} +$   
 $11\ 771\ 480\ 454\ 445\ 896\ 416\ 287\ 811\ 253\ 798\ 832\ 897\ 303\ 017\ 271\ 545\ 637\ 781\ 516\ 788\ 661\ 802\ 457\ 640\ q^{2196} -$   
 $12\ 472\ 219\ 803\ 015\ 967\ 871\ 675\ 420\ 296\ 782\ 267\ 943\ 509\ 022\ 673\ 229\ 668\ 201\ 983\ 123\ 678\ 974\ 170\ 304\ q^{2197} +$   
 $14\ 833\ 636\ 401\ 047\ 169\ 451\ 664\ 117\ 819\ 648\ 199\ 240\ 408\ 852\ 561\ 034\ 151\ 319\ 470\ 347\ 879\ 125\ 525\ 176\ q^{2200} -$   
 $15\ 715\ 838\ 402\ 178\ 666\ 197\ 213\ 072\ 798\ 036\ 021\ 172\ 974\ 889\ 661\ 353\ 384\ 863\ 161\ 193\ 653\ 110\ 144\ 745\ q^{2201} +$   
 $18\ 688\ 450\ 109\ 841\ 126\ 708\ 465\ 306\ 757\ 181\ 294\ 414\ 970\ 132\ 437\ 727\ 197\ 731\ 804\ 881\ 429\ 008\ 353\ 129\ q^{2204} -$   
 $19\ 798\ 875\ 616\ 451\ 547\ 271\ 259\ 307\ 725\ 412\ 151\ 189\ 943\ 842\ 612\ 829\ 465\ 455\ 837\ 750\ 890\ 491\ 304\ 228\ q^{2205} +$   
 $23\ 540\ 099\ 847\ 710\ 857\ 370\ 546\ 809\ 755\ 490\ 720\ 344\ 754\ 929\ 369\ 439\ 968\ 538\ 034\ 308\ 409\ 035\ 174\ 035\ q^{2208} -$   
 $24\ 937\ 500\ 431\ 609\ 332\ 448\ 192\ 670\ 295\ 322\ 779\ 411\ 566\ 321\ 592\ 933\ 018\ 845\ 802\ 397\ 693\ 237\ 101\ 956\ q^{2209} +$   
 $29\ 645\ 100\ 046\ 754\ 516\ 010\ 894\ 212\ 281\ 160\ 145\ 330\ 357\ 870\ 597\ 085\ 772\ 462\ 114\ 671\ 460\ 090\ 196\ 370\ q^{2212} -$   
 $31\ 403\ 277\ 698\ 819\ 440\ 931\ 712\ 452\ 410\ 011\ 536\ 189\ 051\ 982\ 393\ 306\ 377\ 828\ 858\ 309\ 031\ 291\ 124\ 391\ q^{2213} +$   
 $37\ 325\ 650\ 837\ 826\ 690\ 213\ 970\ 182\ 491\ 331\ 958\ 353\ 089\ 657\ 573\ 341\ 768\ 788\ 681\ 716\ 874\ 198\ 582\ 330\ q^{2216} -$   
 $39\ 537\ 294\ 606\ 631\ 667\ 584\ 231\ 595\ 669\ 222\ 737\ 035\ 195\ 036\ 205\ 975\ 929\ 106\ 009\ 486\ 125\ 465\ 280\ 069\ q^{2217} +$   
 $46\ 986\ 376\ 067\ 207\ 287\ 871\ 946\ 708\ 108\ 004\ 525\ 676\ 811\ 100\ 888\ 030\ 550\ 363\ 785\ 273\ 550\ 556\ 931\ 362\ q^{2220} -$   
 $49\ 767\ 871\ 959\ 330\ 679\ 444\ 996\ 139\ 841\ 885\ 807\ 211\ 176\ 859\ 092\ 288\ 300\ 661\ 887\ 698\ 106\ 682\ 059\ 633\ q^{2221} +$   
 $59\ 135\ 305\ 696\ 065\ 220\ 610\ 666\ 150\ 021\ 796\ 240\ 632\ 605\ 650\ 561\ 760\ 678\ 189\ 124\ 809\ 255\ 326\ 073\ 507\ q^{2224} -$   
 $62\ 632\ 765\ 528\ 394\ 771\ 165\ 212\ 375\ 960\ 008\ 448\ 335\ 882\ 611\ 442\ 232\ 806\ 931\ 167\ 620\ 870\ 727\ 212\ 107\ q^{2225} +$   
 $74\ 410\ 173\ 622\ 771\ 338\ 602\ 912\ 977\ 726\ 418\ 445\ 787\ 426\ 624\ 413\ 031\ 153\ 595\ 839\ 933\ 429\ 079\ 865\ 310\ q^{2228} -$   
 $78\ 806\ 990\ 237\ 605\ 870\ 974\ 026\ 460\ 437\ 843\ 087\ 167\ 079\ 116\ 937\ 472\ 261\ 798\ 369\ 612\ 423\ 273\ 239\ 351\ q^{2229} +$   
 $93\ 611\ 370\ 923\ 815\ 411\ 209\ 548\ 898\ 871\ 712\ 206\ 537\ 662\ 018\ 284\ 673\ 602\ 824\ 196\ 298\ 771\ 503\ 366\ 132\ q^{2232} -$   
 $99\ 137\ 684\ 327\ 735\ 962\ 949\ 987\ 113\ 903\ 216\ 331\ 451\ 176\ 142\ 232\ 730\ 357\ 778\ 818\ 396\ 871\ 486\ 809\ 049\ q^{2233} +$   
 $117\ 743\ 230\ 676\ 181\ 522\ 998\ 507\ 153\ 884\ 575\ 649\ 057\ 834\ 357\ 591\ 400\ 001\ 639\ 241\ 221\ 772\ 022\ 619\ 749\ q^{2236} -$   
 $124\ 687\ 786\ 082\ 124\ 197\ 923\ 377\ 837\ 322\ 068\ 668\ 528\ 690\ 633\ 455\ 427\ 096\ 091\ 933\ 761\ 856\ 220\ 616\ 294\ q^{2237} +$   
 $148\ 065\ 740\ 617\ 118\ 121\ 583\ 625\ 382\ 630\ 118\ 412\ 577\ 412\ 810\ 549\ 654\ 726\ 408\ 111\ 473\ 582\ 335\ 294\ 373\ q^{2240} -$   
 $156\ 790\ 739\ 844\ 790\ 535\ 508\ 455\ 847\ 841\ 505\ 494\ 744\ 860\ 200\ 931\ 334\ 803\ 215\ 303\ 204\ 358\ 848\ 334\ 458\ q^{2241} +$   
 $323\ 389\ 829\ 894\ 343\ 046\ 862\ 796\ 261\ 965\ 824\ 000\ q^{2241} +$

186 159 304 767 470 515 920 174 996 424 082 317 553 681 745 406 449 065 662 758 112 749 726 654 416  
 238 897 918 136 930 098 795 118 913 839 104 000  $q^{2244}$  -  
 197 119 002 963 671 295 029 801 091 363 048 745 900 463 385 518 034 082 012 189 443 487 230 251 148  
 462 339 730 853 526 976 961 073 562 133 332 275  $q^{2245}$  +  
 234 005 830 798 668 007 578 264 425 665 758 658 604 162 234 380 916 706 139 496 074 950 026 009 100  
 363 777 778 661 307 786 335 716 276 711 464 960  $q^{2248}$  -  
 247 769 818 425 709 346 215 886 197 075 298 301 440 662 026 069 790 612 475 657 370 463 671 307 773  
 218 250 064 222 290 796 700 573 707 788 288 000  $q^{2249}$  +  
 294 090 238 791 491 280 666 528 521 689 227 310 732 982 932 021 553 677 266 760 774 986 095 132 850  
 500 859 587 865 810 822 900 722 474 515 806 720  $q^{2252}$  -  
 311 372 583 587 338 317 630 395 757 305 856 994 666 780 716 619 290 541 297 280 784 333 411 641 824  
 412 741 711 196 391 010 851 646 405 889 616 872  $q^{2253}$  +  
 369 527 509 550 289 224 465 409 511 360 028 795 651 034 654 171 204 995 621 198 964 499 958 082 837  
 471 988 364 932 274 523 044 880 134 365 184 000  $q^{2256}$  -  
 391 223 226 267 611 570 233 582 640 297 299 012 820 132 928 314 495 946 479 061 498 722 535 586 237  
 337 017 725 902 930 133 635 699 816 009 367 552  $q^{2257}$  +  
 464 221 667 201 173 500 383 257 333 663 010 279 861 392 743 102 188 259 975 411 052 379 277 904 919  
 951 434 350 432 449 068 094 597 953 436 774 400  $q^{2260}$  -  
 491 452 348 816 767 166 625 281 682 767 006 086 423 386 410 602 300 059 919 264 659 810 697 601 649  
 558 329 168 941 782 470 043 247 449 951 312 250  $q^{2261}$  +  
 583 064 684 232 882 198 687 733 438 960 694 693 124 272 780 673 384 447 542 347 238 582 692 976 560  
 627 707 060 181 762 378 012 993 080 543 552 000  $q^{2264}$  -  
 617 235 584 969 115 400 725 781 626 917 923 396 789 960 420 101 664 844 661 948 154 662 672 731 882  
 155 352 169 674 960 904 836 902 951 518 208 000  $q^{2265}$  +  
 732 185 285 707 617 792 484 977 907 183 514 797 378 990 649 353 197 241 102 535 529 036 534 857 761  
 056 515 343 721 804 310 460 080 616 340 039 680  $q^{2268}$  -  
 775 056 716 032 019 929 860 745 547 377 379 224 421 403 813 538 020 452 137 026 666 512 355 312 583  
 792 931 323 391 869 799 694 335 409 424 615 125  $q^{2269}$  +  
 919 260 110 591 829 443 126 597 677 161 173 766 108 866 584 837 506 688 547 704 713 217 714 735 670  
 158 334 636 934 634 619 239 596 044 728 688 640  $q^{2272}$  -  
 973 036 715 273 650 820 861 511 984 344 948 520 950 914 334 529 321 846 447 872 811 760 591 117 118  
 140 860 274 013 964 979 487 131 674 155 286 528  $q^{2273}$  +  
 1 153 902 783 499 509 966 520 382 414 748 376 384 697 022 541 986 998 965 742 954 937 723 944 790 046  
 992 579 200 821 388 366 560 151 111 589 888 000  $q^{2276}$  -  
 1 221 345 160 568 865 129 554 394 929 288 625 119 735 855 857 508 254 087 391 436 620 204 178 275 808  
 548 734 747 407 727 423 721 171 737 613 587 161  $q^{2277}$  +  
 1 448 150 310 873 410 657 544 106 481 943 175 024 921 385 547 437 207 606 801 625 858 267 126 846 432  
 911 681 375 487 996 075 948 080 708 023 296 000  $q^{2280}$  -  
 1 532 714 535 241 010 571 787 947 124 187 095 087 330 451 975 380 727 499 932 371 137 835 614 247 457  
 788 696 056 238 016 577 636 649 244 282 880 000  $q^{2281}$  +  
 1 817 071 030 105 553 721 172 422 168 928 513 065 327 581 910 585 693 909 089 689 423 246 158 493 051  
 389 532 972 997 657 352 635 843 831 424 576 000  $q^{2284}$  -  
 1 923 083 024 557 033 622 305 885 106 890 810 512 988 627 331 866 903 087 725 286 210 721 138 223 422  
 125 203 291 239 966 128 227 954 541 250 696 625  $q^{2285}$  +  
 2 279 524 342 800 105 819 923 301 733 711 165 283 070 377 377 215 724 426 562 341 971 486 080 535 752  
 645 018 838 200 676 626 883 424 261 296 734 208  $q^{2288}$  -  
 2 412 397 758 169 226 513 438 548 649 014 445 620 300 647 624 341 669 333 502 315 688 716 274 726 809  
 790 590 933 907 518 641 612 233 519 202 304 000  $q^{2289}$  +  
 2 859 109 946 164 994 031 337 741 183 088 072 233 263 084 717 689 554 369 572 958 689 566 085 142 349  
 630 999 532 145 611 942 814 725 880 351 965 184  $q^{2292}$  -  
 3 025 618 355 211 623 538 259 098 858 122 688 096 634 761 409 245 891 654 196 290 456 724 858 808 587  
 031 738 529 313 708 215 631 300 047 848 416 227  $q^{2293}$  +  
 3 585 353 602 584 093 413 054 892 211 491 950 167 400 847 855 453 221 089 964 669 880 031 060 494 999  
 967 582 818 863 475 194 550 077 093 829 120 000  $q^{2296}$  -  
 3 793 970 482 352 305 731 935 968 330 895 783 694 059 918 071 232 269 708 624 484 757 088 584 426 137

740 968 689 266 013 023 727 687 211 394 990 080  $q^{2297} +$   
 4 495 188 108 671 645 895 031 740 269 908 842 010 938 266 192 474 101 210 620 746 396 694 893 987 194  
 320 667 263 049 687 828 776 412 737 777 408 000  $q^{2300} -$   
 4 756 511 413 136 382 219 421 772 632 259 054 820 231 397 898 654 045 051 590 642 181 206 790 600 419  
 673 145 195 512 815 868 596 334 401 464 147 250  $q^{2301} +$   
 5 634 802 603 708 665 899 810 886 804 106 658 371 962 181 571 126 011 119 057 118 392 213 707 885 526  
 036 413 278 427 798 468 897 170 144 133 578 752  $q^{2304} -$   
 5 962 084 873 111 890 911 942 643 537 066 624 726 720 925 576 463 460 729 855 406 814 866 489 319 818  
 791 873 698 506 146 901 479 689 113 234 636 800  $q^{2305} +$   
 7 061 951 392 508 282 973 925 144 122 522 594 444 718 188 501 163 435 441 622 076 787 599 235 978 534  
 440 682 040 663 111 995 726 323 740 387 082 240  $q^{2308} -$   
 7 471 761 507 882 735 922 877 610 910 707 921 821 369 667 925 562 037 320 786 557 388 223 070 867 565  
 053 685 314 715 678 512 196 357 070 704 077 125  $q^{2309} +$   
 8 848 835 918 937 479 308 646 113 024 351 234 236 459 337 131 678 621 253 540 513 158 563 396 446 327  
 543 797 745 401 971 047 683 860 623 184 497 920  $q^{2312} -$   
 9 361 885 038 530 421 712 607 134 493 814 666 078 668 754 097 284 367 322 475 947 323 191 872 757 257  
 198 039 532 882 183 894 016 748 445 951 983 616  $q^{2313} +$   
 11 085 701 494 578 163 816 458 462 981 944 350 981 167 904 809 965 499 805 388 823 962 845 832 388  
 356 127 588 185 586 848 792 539 927 700 391 936 000  $q^{2316} -$   
 11 727 873 712 288 107 901 741 894 217 609 507 789 331 768 848 560 108 954 434 647 279 617 842 994  
 627 752 132 316 413 395 364 383 909 209 243 286 787  $q^{2317} +$   
 13 885 325 206 170 978 585 186 111 406 013 502 997 654 702 557 020 003 223 737 246 605 352 578 907  
 694 578 407 657 121 294 747 870 714 043 727 872 000  $q^{2320} -$   
 14 688 963 434 855 088 442 417 430 004 135 066 288 778 042 580 720 213 686 057 908 653 861 448 550  
 156 314 590 170 166 494 914 016 633 605 894 144 000  $q^{2321} +$   
 17 388 614 765 747 259 086 985 850 286 451 793 288 333 722 958 281 023 967 957 480 218 052 465 316  
 690 121 307 276 427 585 063 545 101 614 794 240 000  $q^{2324} -$   
 18 394 124 747 749 066 673 939 404 499 424 994 454 824 418 013 817 075 324 798 701 655 962 723 790  
 325 520 719 669 142 451 667 937 113 210 096 673 450  $q^{2325} +$   
 21 771 592 004 168 889 435 641 379 180 860 934 059 936 886 271 159 486 236 698 282 987 083 315 367  
 504 119 564 973 188 095 684 607 621 891 095 977 984  $q^{2328} -$   
 23 029 442 780 829 666 869 031 590 795 169 236 614 708 806 159 267 605 990 641 640 221 606 003 966  
 391 624 152 165 351 492 606 149 206 007 644 160 000  $q^{2329} +$   
 27 254 101 820 732 974 060 302 545 383 380 808 458 405 208 588 154 777 666 011 762 046 899 646 943  
 442 729 965 144 794 774 705 347 720 805 168 646 144  $q^{2332} -$   
 28 827 320 188 873 728 525 524 100 472 184 400 616 598 335 508 420 437 441 356 143 084 882 133 442  
 384 349 937 701 200 850 845 781 554 764 057 511 539  $q^{2333} +$   
 34 110 670 891 636 739 746 522 267 496 074 521 771 694 287 797 476 640 761 237 181 809 573 817 295  
 235 157 199 187 181 939 865 071 278 296 225 792 000  $q^{2336} -$   
 36 077 951 253 287 753 994 587 992 932 964 470 552 260 018 961 668 360 243 683 409 052 810 512 992  
 903 431 613 276 891 612 626 397 456 154 880 114 688  $q^{2337} +$   
 42 684 044 286 561 624 793 714 013 834 125 191 862 575 520 783 770 989 010 449 018 189 378 200 387  
 007 456 683 965 234 407 505 223 062 794 283 417 600  $q^{2340} -$   
 45 143 624 995 169 062 567 859 065 019 076 787 653 082 359 876 829 484 208 302 645 922 146 642 912  
 018 402 573 778 938 845 288 764 467 269 283 501 250  $q^{2341} +$   
 53 402 057 285 246 687 735 913 065 411 954 708 079 225 060 624 635 211 109 803 711 586 127 534 377  
 136 697 637 723 899 872 869 151 788 574 295 744 000  $q^{2344} -$   
 56 476 551 518 412 737 697 123 599 129 389 705 865 303 676 481 715 072 701 356 041 033 931 450 012  
 990 229 597 786 590 021 090 546 199 485 053 337 600  $q^{2345} +$   
 66 798 660 257 595 500 646 921 780 428 878 821 379 871 027 646 396 785 418 021 838 600 397 483 178  
 058 437 645 419 965 301 546 628 429 936 165 453 312  $q^{2348} -$   
 70 641 075 354 975 386 405 163 812 131 396 005 885 904 512 316 568 446 430 511 257 967 318 751 031  
 781 318 612 568 054 363 814 204 323 713 912 653 250  $q^{2349} +$   
 83 540 114 084 413 209 532 375 065 643 303 063 517 474 004 674 262 128 542 631 969 684 178 578 771  
 210 215 557 030 533 525 605 895 408 503 400 706 048  $q^{2352} -$

88 341 350 354 063 019 280 885 652 244 320 360 877 299 508 807 372 383 745 863 646 031 844 307 005  
 882 460 022 945 119 537 713 680 238 009 997 066 240  $q^{2353} +$   
 104 457 621 699 447 442 935 923 194 340 520 253 212 537 005 818 713 714 171 888 325 697 061 734 280  
 546 114 369 717 445 660 776 208 617 217 529 856 000  $q^{2356} -$   
 110 455 812 614 969 335 698 564 850 544 875 754 563 626 114 007 334 556 509 786 080 789 054 263 917  
 301 806 779 171 357 284 898 895 354 683 095 032 364  $q^{2357} +$   
 130 587 969 650 878 507 446 589 911 190 492 490 358 065 499 656 396 625 516 928 882 748 833 659 459  
 131 139 357 071 563 729 199 248 190 609 507 251 200  $q^{2360} -$   
 138 080 113 482 982 693 924 621 819 186 653 965 935 876 719 680 664 300 005 073 782 831 972 561 078  
 901 661 034 454 504 043 153 129 260 443 209 728 000  $q^{2361} +$   
 163 224 136 656 938 423 940 822 294 690 962 418 620 222 125 708 262 965 328 917 013 295 178 759 112  
 291 470 850 199 761 634 424 102 192 660 238 080 000  $q^{2364} -$   
 172 580 579 059 569 888 837 208 068 839 038 000 808 223 512 362 499 250 752 054 269 763 963 902 429  
 948 551 232 465 506 116 843 791 889 699 147 057 250  $q^{2365} +$   
 203 978 302 008 154 338 192 731 767 474 434 568 975 395 045 116 347 328 155 313 252 885 249 904 263  
 678 475 262 040 845 497 156 071 959 949 963 034 624  $q^{2368} -$   
 215 660 765 062 103 381 706 317 658 659 512 978 467 440 222 210 925 707 291 442 616 417 407 986 928  
 698 602 186 623 493 517 019 795 004 554 190 848 000  $q^{2369} +$   
 254 860 277 723 935 301 047 453 575 867 711 312 566 191 227 147 514 512 484 218 446 585 387 153 635  
 632 498 019 963 573 048 399 714 399 632 879 747 072  $q^{2372} -$   
 269 444 299 817 484 225 426 238 765 295 961 758 921 624 239 761 969 596 378 020 136 762 893 877 943  
 297 230 651 080 833 542 596 677 347 206 243 262 296  $q^{2373} +$   
 318 375 122 350 064 741 266 705 453 376 272 943 777 528 557 397 653 441 358 575 194 986 116 095 633  
 794 549 625 591 472 066 464 604 999 971 047 424 000  $q^{2376} -$   
 336 577 982 966 471 630 419 080 312 995 515 809 281 346 172 019 450 454 438 238 580 188 118 008 060  
 712 059 147 441 918 107 038 908 351 114 108 993 536  $q^{2377} +$   
 397 644 605 585 185 718 911 542 960 419 019 031 724 673 893 364 154 234 059 809 901 700 769 181 524  
 793 842 391 255 490 042 850 430 170 736 654 796 800  $q^{2380} -$   
 420 360 069 388 340 533 336 129 488 714 235 918 298 316 910 660 991 681 977 086 195 295 642 744 798  
 346 210 805 270 432 154 013 724 837 483 789 821 250  $q^{2381} +$   
 496 558 324 188 233 385 464 063 845 990 350 332 431 450 721 907 970 102 580 712 902 166 359 642 932  
 424 544 648 254 827 683 655 285 830 634 383 360 000  $q^{2384} -$   
 524 899 861 918 933 120 007 070 395 998 922 617 438 648 749 409 582 332 766 382 083 859 049 060 826  
 673 890 986 223 097 117 681 054 341 514 747 904 000  $q^{2385} +$   
 619 961 673 690 154 191 726 715 216 336 279 498 703 213 476 089 238 530 982 462 252 015 976 071 570  
 750 273 894 681 334 938 896 212 695 531 222 216 704  $q^{2388} -$   
 655 316 218 385 229 603 704 244 740 500 417 487 842 906 017 933 985 893 713 595 915 311 846 321 510  
 734 350 465 546 591 898 743 710 646 937 028 390 250  $q^{2389} +$   
 773 889 622 794 099 635 307 875 306 713 363 394 039 348 755 307 632 684 788 839 327 560 884 020 336  
 313 527 886 730 634 465 938 003 557 148 090 890 240  $q^{2392} -$   
 817 984 417 402 051 276 469 134 726 624 522 823 840 404 061 060 784 776 650 251 545 997 535 838 772  
 785 961 431 068 714 306 750 010 686 658 110 390 272  $q^{2393} +$   
 965 857 399 125 071 840 931 389 077 622 418 830 778 510 261 409 794 087 570 727 946 299 757 955 119  
 738 021 886 324 021 478 249 911 060 094 249 728 000  $q^{2396} -$   
 1 020 843 108 859 086 280 188 474 866 284 297 669 624 797 720 243 625 366 857 399 014 576 378 142 496  
 220 514 308 163 389 567 964 546 390 520 849 585 122  $q^{2397} +$   
 1 205 221 876 674 077 757 113 600 871 320 838 159 885 016 574 876 864 264 632 957 310 821 602 344 747  
 341 410 429 411 811 559 206 531 320 430 518 374 400  $q^{2400} -$   
 1 273 775 905 081 941 149 098 163 767 085 377 381 458 250 856 578 205 225 185 443 702 053 154 766 715  
 798 332 576 520 876 456 928 020 222 500 970 496 248  $q^{2401} +$   
 1 503 630 781 330 386 087 839 407 212 827 866 491 266 392 701 390 037 018 024 151 618 112 271 037 385  
 217 894 698 341 356 036 032 211 912 627 464 192 000  $q^{2404} -$   
 1 589 085 678 569 189 738 105 992 863 712 743 588 199 063 215 072 718 520 905 825 235 692 690 701 505  
 290 736 331 727 986 796 629 985 117 453 099 577 575  $q^{2405} +$   
 1 875 580 955 420 499 474 700 805 826 906 115 742 819 951 529 013 604 428 894 058 591 089 446 983 748

127 411 773 657 595 325 041 811 085 034 557 388 800  $q^{2408}$  -  
 1 982 083 984 554 159 040 001 303 998 002 687 458 545 932 401 983 558 383 053 415 859 154 404 307 941 9  
 651 571 425 877 589 840 442 120 048 599 179 264 000  $q^{2409}$  +  
 2 339 112 035 974 090 480 693 733 248 034 669 302 419 329 007 668 671 005 597 390 817 866 569 419 616 9  
 137 409 775 258 597 192 506 329 211 959 845 911 040  $q^{2412}$  -  
 2 471 823 422 673 207 029 165 591 455 509 566 680 564 803 807 459 775 696 371 528 757 612 006 566 351 9  
 983 662 279 275 988 599 255 003 202 683 920 572 752  $q^{2413}$  +  
 2 916 668 240 697 282 374 659 625 319 530 299 413 674 342 504 873 317 387 659 040 590 968 608 455 668 9  
 445 957 372 952 482 884 768 254 360 953 513 984 000  $q^{2416}$  -  
 3 082 007 440 857 706 594 874 183 378 219 877 403 704 576 181 095 434 025 962 808 846 949 252 638 426 9  
 873 850 600 859 123 384 436 204 817 111 808 114 688  $q^{2417}$  +  
 3 636 168 812 660 066 736 102 481 473 086 834 987 581 705 007 114 900 965 667 355 369 001 981 573 805 9  
 578 297 391 209 007 328 841 061 358 393 478 686 720  $q^{2420}$  -  
 3 842 120 374 507 513 427 385 541 044 869 987 136 154 913 281 259 465 258 017 521 032 767 427 524 986 9  
 571 921 901 342 234 477 868 886 030 888 712 881 125  $q^{2421}$  +  
 4 532 337 411 207 139 497 581 755 642 296 462 654 203 066 662 635 905 319 974 973 538 645 027 950 640 9  
 107 029 527 649 071 354 925 800 401 346 541 952 000  $q^{2424}$  -  
 4 788 830 786 535 468 357 345 146 189 912 891 969 832 842 293 118 187 719 213 416 935 827 278 467 307 9  
 936 001 807 701 508 323 730 255 659 075 901 030 400  $q^{2425}$  +  
 5 648 352 800 093 818 558 503 555 332 166 826 654 784 954 669 143 817 856 131 768 769 684 578 878 996 9  
 398 048 520 805 395 454 524 271 520 778 825 052 160  $q^{2428}$  -  
 5 967 733 900 956 874 560 555 963 399 974 915 091 212 076 318 157 251 096 923 346 481 897 014 959 971 9  
 638 916 811 487 191 425 555 140 142 413 405 554 250  $q^{2429}$  +  
 7 037 898 127 909 289 102 883 973 961 806 710 552 415 285 854 488 952 911 512 385 885 334 997 311 498 9  
 556 516 045 778 875 882 558 289 479 365 156 175 872  $q^{2432}$  -  
 7 435 514 688 130 405 024 582 799 386 525 446 399 279 818 188 441 916 687 106 655 056 721 581 845 159 9  
 609 280 636 746 039 398 207 233 160 195 529 932 800  $q^{2433}$  +  
 8 767 704 605 143 500 092 670 099 542 958 743 750 915 445 836 579 008 467 293 747 431 252 253 092 121 9  
 494 856 137 324 186 655 957 402 397 495 025 664 000  $q^{2436}$  -  
 9 262 632 685 544 990 107 444 840 546 484 432 295 089 406 232 509 805 524 664 611 789 139 132 104 049 9  
 563 921 495 937 333 904 000 340 526 820 317 054 395  $q^{2437}$  +  
 10 920 708 303 432 490 701 031 464 374 132 171 528 133 036 878 282 358 019 722 002 809 431 944 901 9  
 151 963 310 410 297 976 416 929 322 746 757 424 102 400  $q^{2440}$  -  
 11 536 653 816 981 208 942 251 082 276 020 681 338 553 486 212 528 547 045 996 696 311 265 380 357 9  
 848 201 952 238 699 527 909 168 410 062 539 501 568 000  $q^{2441}$  +  
 13 599 967 182 364 539 775 500 533 942 637 107 515 999 945 427 636 810 009 398 395 536 619 227 377 9  
 019 357 291 151 458 540 586 150 049 424 544 405 120 000  $q^{2444}$  -  
 14 366 384 408 740 007 571 990 869 807 072 250 533 194 195 487 709 659 142 227 838 158 617 500 311 9  
 894 459 888 278 789 742 979 402 239 664 035 937 054 625  $q^{2445}$  +  
 16 933 520 581 756 179 474 195 578 763 892 129 996 014 976 219 088 614 648 442 158 892 845 947 106 9  
 038 634 396 035 736 208 546 363 019 645 998 391 754 752  $q^{2448}$  -  
 17 886 999 658 840 536 200 137 568 731 354 095 901 348 498 041 275 346 431 160 262 637 371 852 833 9  
 565 269 007 326 775 317 568 640 178 837 916 262 400 000  $q^{2449}$  +  
 21 080 416 901 868 679 989 040 792 315 690 864 234 857 037 491 588 356 898 309 590 777 677 753 519 9  
 821 429 355 226 081 696 198 109 098 456 710 110 726 144  $q^{2452}$  -  
 22 266 404 679 945 717 327 383 764 114 071 358 753 689 028 846 239 926 779 629 507 313 684 783 842 9  
 878 198 568 196 653 638 649 649 139 461 665 695 153 667  $q^{2453}$  +  
 26 238 189 007 056 191 004 700 051 638 842 799 489 736 363 791 139 028 685 606 531 001 353 035 200 9  
 960 511 628 852 861 527 542 860 916 840 450 378 176 000  $q^{2456}$  -  
 27 713 122 993 062 301 669 324 314 384 003 284 094 690 752 075 396 635 677 060 122 926 215 654 033 9  
 336 952 517 461 546 132 045 083 075 111 528 964 030 464  $q^{2457}$  +  
 32 652 123 471 800 497 761 343 963 642 078 525 703 170 901 688 970 545 092 793 149 699 548 341 740 9  
 634 055 001 366 050 706 811 112 221 703 333 328 179 200  $q^{2460}$  -  
 34 486 077 571 307 407 009 101 677 332 188 002 645 634 963 057 022 662 294 920 405 330 426 762 071 9  
 486 720 275 846 942 712 467 345 199 638 444 543 984 000  $q^{2461}$  +

40 626 752 158 703 212 143 660 301 175 302 292 847 927 305 581 464 161 932 754 516 632 316 173 441 9  
 125 289 619 100 039 115 811 597 919 345 592 915 968 000  $q^{2464}$  -  
 42 906 716 401 548 325 336 998 162 631 618 810 705 579 699 044 750 982 405 991 630 711 650 616 847 9  
 905 497 929 854 423 992 656 206 654 196 714 445 209 600  $q^{2465}$  +  
 50 540 096 501 852 546 512 234 377 234 516 327 680 397 856 922 381 130 743 274 904 686 629 413 069 9  
 645 009 052 299 551 711 333 796 711 454 825 783 476 224  $q^{2468}$  -  
 53 374 041 974 497 008 799 541 512 705 484 222 764 452 438 467 631 777 249 347 448 772 403 492 857 9  
 811 163 723 162 009 819 763 553 531 890 673 861 870 250  $q^{2469}$  +  
 62 861 320 867 551 571 265 752 882 772 483 746 728 145 644 076 840 281 872 386 614 880 278 074 536 9  
 404 042 977 781 411 069 012 651 707 001 925 990 417 408  $q^{2472}$  -  
 66 383 236 981 517 482 179 743 530 885 958 659 257 908 923 597 314 540 001 416 734 575 331 633 934 9  
 543 017 667 294 280 382 916 203 211 840 614 294 913 024  $q^{2473}$  +  
 78 172 607 159 330 541 952 762 957 020 792 749 584 621 321 720 210 633 402 346 068 217 878 759 222 9  
 891 694 685 607 273 149 177 369 855 005 953 839 168 000  $q^{2476}$  -  
 82 548 742 778 013 865 358 413 696 503 245 991 538 046 609 732 920 857 868 478 594 501 096 564 433 9  
 593 847 527 229 756 774 585 627 889 504 086 493 565 790  $q^{2477}$  +  
 97 196 255 439 658 397 379 508 514 911 816 240 754 525 476 596 330 162 220 995 376 484 911 106 292 9  
 018 199 959 029 323 606 350 053 512 027 401 561 292 800  $q^{2480}$  -  
 102 632 850 262 177 250 839 673 272 647 460 765 782 248 875 249 823 704 065 733 488 810 746 035 556 9  
 097 502 572 500 798 115 646 835 555 760 125 153 280 000  $q^{2481}$  +  
 120 828 253 414 666 014 609 794 076 784 932 671 520 972 543 581 324 663 314 488 023 851 177 584 796 9  
 793 779 527 423 409 197 987 437 111 334 379 032 576 000  $q^{2484}$  -  
 127 581 113 839 587 040 185 350 372 660 421 558 535 239 404 268 580 567 882 760 777 117 534 983 571 9  
 180 432 644 565 444 258 871 682 197 714 458 691 730 875  $q^{2485}$  +  
 150 179 851 855 414 900 524 292 667 046 193 035 274 169 738 589 632 052 820 723 183 542 994 103 579 9  
 637 297 404 587 800 491 672 552 027 093 820 902 255 616  $q^{2488}$  -  
 158 566 209 360 295 370 474 720 580 542 218 879 395 481 719 358 714 323 545 057 414 515 146 881 859 9  
 633 910 679 358 261 270 192 817 567 604 614 410 240 000  $q^{2489}$  +  
 186 629 046 594 224 499 041 166 130 624 898 158 206 262 888 778 186 018 688 515 984 742 502 316 075 9  
 889 329 746 971 497 024 015 164 376 081 983 383 871 488  $q^{2492}$  -  
 197 042 240 221 034 997 029 440 941 425 176 217 198 546 545 298 164 098 041 887 645 144 819 279 201 9  
 636 251 951 413 421 041 947 630 698 138 842 482 625 481  $q^{2493}$  +  
 231 884 316 903 318 734 246 079 391 628 057 443 462 131 264 405 563 666 228 296 606 691 486 946 451 9  
 078 685 509 683 544 595 326 793 605 108 704 559 104 000  $q^{2496}$  -  
 244 811 969 363 609 043 885 898 534 718 616 835 983 273 156 853 014 805 813 170 634 043 461 205 434 9  
 275 115 104 238 853 923 657 750 302 293 871 722 987 520  $q^{2497}$  +  
 288 063 524 900 139 954 960 201 295 713 159 018 907 059 123 944 274 701 293 366 597 373 889 861 223 9  
 427 029 475 699 271 044 550 141 534 855 987 478 096 000  $q^{2500}$  -  
 304 110 039 816 268 405 439 485 332 383 785 969 110 655 707 382 180 792 851 222 660 075 408 023 979 9  
 185 347 579 239 049 307 862 182 308 761 272 330 204 250  $q^{2501}$  +  
 357 791 565 875 295 126 618 760 746 689 101 453 075 766 410 287 480 306 615 505 641 276 483 994 894 9  
 388 703 043 332 721 956 991 707 524 555 323 958 400 000  $q^{2504}$  -  
 377 705 968 795 518 595 842 106 047 591 961 815 218 802 641 903 040 264 502 315 443 204 377 696 060 9  
 527 279 828 885 513 824 861 053 781 681 729 478 656 000  $q^{2505}$  +  
 444 321 205 620 461 398 768 390 097 349 547 263 056 031 855 460 237 758 047 742 674 953 340 980 358 9  
 063 719 730 004 979 795 642 829 930 890 325 483 075 584  $q^{2508}$  -  
 469 031 592 366 989 554 491 160 892 295 577 246 870 764 021 970 071 562 519 967 520 580 873 833 020 9  
 584 928 531 532 481 390 258 404 410 409 534 198 174 375  $q^{2509}$  +  
 551 682 585 567 775 529 559 856 568 666 633 068 075 698 268 557 308 945 925 510 614 116 057 325 966 9  
 181 968 704 195 857 903 588 443 400 751 868 575 236 096  $q^{2512}$  -  
 582 338 738 899 799 491 283 490 982 067 756 405 986 049 407 365 522 349 999 163 416 834 142 025 913 9  
 015 839 917 528 699 764 105 109 825 714 630 504 742 912  $q^{2513}$  +  
 684 868 166 218 382 665 181 451 968 920 670 102 570 279 748 177 600 619 573 367 834 437 417 279 703 9  
 441 602 949 537 136 266 101 347 789 528 529 512 960 000  $q^{2516}$  -  
 722 894 268 907 699 832 611 141 738 567 566 716 801 438 568 723 662 132 189 860 382 120 783 374 285 9

908 827 009 704 584 317 069 530 901 717 414 564 080 530  $q^{2517} +$   
 850 061 471 099 676 479 791 234 227 499 346 354 458 595 349 129 442 007 277 921 792 654 241 783 847  $q^{2518} -$   
 919 117 738 891 116 835 565 396 919 485 443 322 752 000  $q^{2520} -$   
 897 221 296 581 721 905 652 863 300 533 263 403 248 563 642 167 786 444 157 999 485 784 844 461 446  $q^{2521} +$   
 401 731 510 507 173 081 673 393 579 095 286 300 672 000  $q^{2521} +$   
 1 054 919 957 793 186 363 280 463 285 386 981 227 598 934 667 491 282 094 176 067 504 787 342 368 105  $q^{2522} -$   
 913 136 229 768 444 990 054 437 457 382 787 063 040 000  $q^{2524} -$   
 1 113 397 478 602 998 662 118 588 090 470 569 342 101 411 938 958 975 205 515 850 542 505 914 983 244  $q^{2525} +$   
 550 763 798 601 477 618 888 878 775 163 382 410 774 575  $q^{2525} +$   
 1 308 924 766 215 802 706 629 053 706 376 288 401 866 805 668 326 502 241 554 762 425 699 271 021 173  $q^{2526} -$   
 149 636 794 819 717 178 270 466 113 670 151 621 033 984  $q^{2528} -$   
 1 381 423 810 126 415 774 461 073 091 426 194 606 007 285 169 997 431 992 323 457 610 472 164 972 239  $q^{2529} +$   
 336 646 348 061 324 681 665 384 913 144 606 699 520 000  $q^{2529} +$   
 1 623 813 084 245 752 701 700 852 185 822 675 683 840 438 450 413 724 535 244 573 784 385 462 464 346  $q^{2530} -$   
 542 433 068 053 347 967 736 160 054 716 958 907 711 488  $q^{2532} -$   
 1 713 680 518 796 712 322 225 373 075 107 985 605 114 966 956 275 214 084 970 787 130 547 495 307 523  $q^{2533} +$   
 142 760 802 008 145 409 084 614 783 123 825 143 011 410  $q^{2533} +$   
 2 014 112 558 671 490 232 909 940 225 966 106 363 771 582 567 307 180 321 327 159 343 035 609 539 296  $q^{2534} -$   
 247 260 417 402 096 760 642 782 464 323 213 450 304 000  $q^{2536} -$   
 2 125 490 534 050 288 368 790 086 078 267 415 741 911 454 402 805 651 762 034 757 823 190 072 123 366  $q^{2537} +$   
 893 941 633 126 022 329 857 822 217 454 589 905 829 888  $q^{2537} +$   
 2 497 801 727 513 802 251 125 732 954 759 967 993 764 407 806 133 747 973 870 258 316 447 233 117 820  $q^{2540} -$   
 258 427 266 682 794 119 286 887 508 210 820 511 872 000  $q^{2540} -$   
 2 635 815 801 640 993 214 041 777 585 765 321 116 148 346 462 644 576 514 373 710 936 611 462 873 878  $q^{2541} +$   
 101 708 862 331 482 334 292 247 650 505 143 597 376 000  $q^{2541} +$   
 3 097 126 057 763 591 732 187 247 528 407 576 484 163 094 701 791 439 732 207 621 875 898 033 986 513  $q^{2544} -$   
 832 197 223 568 240 678 052 923 476 400 607 139 840 000  $q^{2544} -$   
 3 268 117 622 702 981 595 706 489 668 843 219 005 004 940 937 464 268 072 008 608 161 002 415 464 852  $q^{2545} +$   
 410 002 519 430 275 522 367 067 788 171 277 049 856 000  $q^{2545} +$   
 3 839 606 086 395 064 111 353 523 499 022 194 527 059 374 799 592 138 633 558 522 136 313 073 729 343  $q^{2548} -$   
 946 495 616 659 891 320 715 188 898 128 588 075 661 312  $q^{2548} -$   
 4 051 419 481 749 554 838 783 421 347 469 509 378 064 999 676 148 714 391 292 213 216 149 045 409 734  $q^{2549} +$   
 336 462 515 214 403 343 862 492 807 738 323 828 633 000  $q^{2549} +$   
 4 759 282 684 856 926 836 569 174 219 895 816 268 793 284 682 654 737 583 111 576 744 477 724 386 074  $q^{2552} -$   
 054 989 075 341 620 377 335 198 246 527 961 084 666 880  $q^{2552} -$   
 5 021 619 807 637 192 406 202 908 095 035 725 796 965 666 998 088 175 818 375 317 786 306 294 248 837  $q^{2553} +$   
 584 628 677 317 491 282 463 406 208 382 686 648 532 992  $q^{2553} +$   
 5 898 254 970 667 729 470 955 796 641 853 571 917 508 739 042 541 771 246 585 440 589 862 985 467 711  $q^{2556} -$   
 541 310 001 251 839 197 254 934 705 803 702 932 224 000  $q^{2556} -$   
 6 223 113 178 094 276 424 824 370 301 605 871 280 282 674 656 029 553 677 832 992 463 645 611 648 170  $q^{2557} +$   
 670 064 630 629 107 948 832 396 935 729 427 004 295 842  $q^{2557} +$   
 7 308 579 332 703 552 284 430 775 316 928 808 787 923 080 477 900 837 212 167 401 698 573 357 867 382  $q^{2560} -$   
 528 477 968 370 303 799 027 989 252 898 013 085 696 000  $q^{2560} -$   
 7 710 792 114 778 631 506 147 399 286 562 569 756 722 146 243 921 699 238 172 934 810 693 139 344 917  $q^{2561} +$   
 323 247 608 096 531 369 064 555 106 722 849 931 264 000  $q^{2561} +$   
 9 054 613 983 346 645 413 266 852 782 160 090 318 899 230 249 950 567 268 443 920 023 643 353 628 578  $q^{2564} -$   
 888 109 395 976 074 128 378 850 142 669 751 826 432 000  $q^{2564} -$   
 9 552 518 416 060 405 817 033 148 152 776 792 089 750 799 692 431 331 305 115 541 054 831 457 518 479  $q^{2565} +$   
 076 115 478 843 707 342 053 333 035 608 403 427 485 225  $q^{2565} +$   
 11 215 913 094 789 100 739 857 569 388 772 588 735 901 046 217 741 736 190 925 114 898 940 377 172  $q^{2568} -$   
 964 302 971 489 395 772 703 595 155 386 119 732 978 595 840  $q^{2568} -$   
 11 832 173 669 623 302 235 550 664 048 644 483 433 482 277 064 398 387 155 194 703 214 390 350 707  $q^{2569} +$   
 051 125 779 715 446 554 202 666 959 575 019 320 999 936 000  $q^{2569} +$   
 13 890 798 771 986 700 171 918 061 276 662 124 103 237 862 585 803 242 850 130 189 836 216 076 408  $q^{2572} -$   
 091 486 386 655 200 527 688 478 669 270 456 508 277 911 040  $q^{2572} -$

14 653 424 075 382 772 086 255 154 099 969 627 070 462 999 945 968 900 365 383 994 907 931 421 115 9  
 717 776 025 026 517 962 185 266 567 549 228 064 571 353 205  $q^{2573} +$   
 17 200 768 910 714 581 536 771 888 687 823 367 271 691 586 088 762 248 082 578 457 719 559 483 595 9  
 782 484 376 918 494 636 829 388 872 861 897 807 953 920 000  $q^{2576} -$   
 18 144 366 096 499 678 877 588 701 721 983 946 620 874 623 515 398 980 556 482 558 975 294 504 108 9  
 534 005 766 868 438 340 115 837 890 836 481 474 579 824 640  $q^{2577} +$   
 21 295 935 676 594 082 709 485 973 401 076 278 874 037 139 791 665 047 236 119 308 915 294 354 099 9  
 295 049 028 574 274 702 536 496 962 599 229 619 358 924 800  $q^{2580} -$   
 22 463 258 101 546 929 418 602 696 515 710 377 897 898 117 114 763 249 684 312 002 739 948 895 304 9  
 063 826 774 493 116 644 208 377 629 419 471 918 408 720 625  $q^{2581} +$   
 26 361 734 506 668 982 889 586 329 506 518 244 899 432 090 971 411 744 516 261 347 819 708 066 249 9  
 430 649 687 873 086 591 029 950 196 048 626 272 314 368 000  $q^{2584} -$   
 27 805 590 735 046 218 946 730 693 053 842 331 136 804 468 064 679 665 824 388 038 184 374 189 542 9  
 842 441 067 233 161 734 665 869 238 165 621 676 331 827 200  $q^{2585} +$   
 32 627 199 129 701 111 454 546 241 373 495 636 996 216 561 005 403 071 932 832 063 157 550 610 788 9  
 534 425 945 881 090 597 450 265 154 137 306 007 706 859 520  $q^{2588} -$   
 34 412 807 310 464 343 019 113 923 774 423 470 604 865 049 715 012 936 869 128 740 784 181 894 060 9  
 587 015 574 893 854 943 131 082 301 441 213 070 718 536 500  $q^{2589} +$   
 40 375 166 522 201 902 406 294 988 670 300 361 508 923 978 804 429 051 580 908 547 601 609 222 107 9  
 003 995 653 938 195 046 066 572 435 563 947 468 551 763 968  $q^{2592} -$   
 42 583 057 583 505 558 313 458 574 524 629 692 557 959 432 428 535 627 323 103 073 386 294 077 975 9  
 428 257 599 497 704 541 453 444 349 693 705 986 896 756 736  $q^{2593} +$   
 49 954 859 910 351 195 357 011 429 512 707 048 800 076 358 209 741 966 439 889 877 369 108 122 265 9  
 556 984 124 543 228 534 069 873 782 551 496 306 550 784 000  $q^{2596} -$   
 52 684 456 935 879 576 780 128 113 208 961 376 576 311 289 984 846 462 856 490 457 106 218 637 466 9  
 164 622 751 341 352 106 230 942 586 947 456 047 215 243 727  $q^{2597} +$   
 61 797 401 513 082 657 113 461 187 567 106 293 238 193 335 096 786 792 285 678 822 542 862 553 682 9  
 242 324 807 987 688 783 814 935 314 253 193 399 968 064 000  $q^{2600} -$   
 65 171 432 091 512 573 313 705 741 797 467 944 963 072 358 368 437 534 490 256 350 094 124 329 015 9  
 877 746 607 635 533 693 191 648 856 029 298 577 739 776 248  $q^{2601} +$   
 76 434 934 145 481 911 256 380 232 422 472 517 995 050 832 919 691 197 353 174 579 160 547 484 065 9  
 752 969 438 579 490 374 288 451 387 862 605 874 832 896 000  $q^{2604} -$   
 80 604 868 679 783 720 852 518 690 591 873 480 059 936 127 534 043 922 661 003 063 536 073 513 307 9  
 873 435 163 076 593 020 136 919 699 620 693 340 180 910 025  $q^{2605} +$   
 94 524 187 526 163 841 757 201 350 380 299 975 359 381 448 514 728 197 213 574 710 293 001 097 408 9  
 744 840 146 288 840 198 524 578 954 022 399 794 301 333 504  $q^{2608} -$   
 99 676 941 003 711 806 146 190 514 867 183 601 152 002 471 383 019 402 869 308 055 801 787 155 105 9  
 254 423 172 306 830 958 479 258 646 075 411 770 200 064 000  $q^{2609} +$   
 116 875 517 865 289 762 986 791 589 203 742 098 112 786 963 857 907 065 415 886 552 189 203 203 219 9  
 448 819 150 851 212 147 811 726 291 084 024 714 482 415 616  $q^{2612} -$   
 123 241 707 326 312 889 614 295 389 721 062 344 698 884 964 247 077 513 434 780 791 392 990 857 455 9  
 467 741 020 263 014 715 249 826 211 890 567 437 367 334 852  $q^{2613} +$   
 144 488 686 288 026 148 059 830 386 445 878 950 667 656 040 124 379 146 788 120 276 918 302 686 056 9  
 202 042 364 397 924 624 804 857 742 160 892 812 328 320 000  $q^{2616} -$   
 152 352 803 525 900 616 448 856 626 646 393 229 500 182 415 224 021 167 573 121 924 973 819 873 952 9  
 083 988 222 195 553 431 862 952 789 022 075 928 427 495 424  $q^{2617} +$   
 178 596 932 983 982 675 466 005 975 956 825 157 971 390 974 662 768 362 701 771 847 334 077 199 770 9  
 319 554 848 284 670 795 622 251 678 633 552 450 896 025 600  $q^{2620} -$   
 188 309 874 735 329 417 807 811 359 955 604 364 924 464 720 386 523 434 995 116 598 382 792 393 027 9  
 090 090 573 759 097 829 640 415 347 608 633 895 391 488 375  $q^{2621} +$   
 220 721 262 080 021 109 168 028 925 872 288 635 018 638 565 782 673 655 702 784 046 279 238 078 860 9  
 805 365 596 168 931 356 274 659 265 022 288 284 352 512 000  $q^{2624} -$   
 232 715 761 637 141 873 503 797 923 591 748 945 022 654 207 800 618 407 375 071 570 262 575 410 123 9  
 275 873 999 004 009 336 878 660 802 794 854 567 559 168 000  $q^{2625} +$   
 272 737 292 347 699 090 501 519 282 254 580 588 754 807 384 137 797 799 130 767 879 565 961 957 584 9

060 546 373 763 782 587 441 881 983 020 691 441 774 968 832  $q^{2628}$  -  
 287 546 921 472 464 671 337 142 953 676 216 779 262 104 927 353 940 994 608 944 058 414 803 674 717 3  
 700 411 867 321 558 035 871 687 633 847 915 507 881 357 125  $q^{2629}$  +  
 336 957 569 674 670 019 183 650 514 747 457 616 395 165 533 595 329 049 484 366 878 184 699 145 889 3  
 084 871 781 992 516 099 863 293 267 429 535 397 316 433 920  $q^{2632}$  -  
 355 240 133 214 824 704 362 224 856 123 387 895 569 088 941 768 296 242 278 381 211 631 749 994 065 3  
 184 802 362 201 902 505 834 388 168 859 817 532 869 443 584  $q^{2633}$  +  
 416 232 901 692 904 909 358 340 180 171 474 802 469 967 310 775 059 682 332 006 836 108 640 791 364 3  
 764 251 138 607 556 688 978 879 556 558 428 954 288 832 000  $q^{2636}$  -  
 438 799 235 905 341 908 800 150 228 145 228 662 203 823 163 239 564 683 623 484 412 063 042 317 950 3  
 668 016 410 770 333 649 644 961 519 616 672 501 038 784 517  $q^{2637}$  +  
 514 077 091 210 242 512 398 131 433 070 399 490 845 654 241 550 515 155 334 330 449 532 814 422 705 3  
 136 512 050 155 965 521 463 177 240 894 135 339 078 451 200  $q^{2640}$  -  
 541 926 508 462 607 288 865 189 473 187 906 613 358 083 470 421 034 659 592 580 030 577 966 852 275 3  
 522 724 635 226 843 027 612 014 697 393 750 710 030 336 000  $q^{2641}$  +  
 634 820 447 658 411 841 533 056 841 704 112 794 328 134 455 562 638 103 370 799 241 731 627 562 011 3  
 900 748 606 523 049 909 831 458 167 930 658 636 364 032 000  $q^{2644}$  -  
 669 184 354 699 790 579 815 865 430 864 441 857 798 949 935 201 481 702 496 617 375 795 431 346 570 3  
 355 040 005 251 801 172 892 580 381 452 208 864 262 072 455  $q^{2645}$  +  
 783 798 686 990 660 723 526 575 374 463 359 363 523 855 629 942 057 718 525 618 214 512 898 894 202 3  
 982 079 859 794 655 998 373 523 032 461 976 320 786 233 856  $q^{2648}$  -  
 826 194 253 359 138 867 663 924 404 929 120 159 782 615 152 352 108 446 639 739 191 716 800 810 870 3  
 447 771 027 332 968 983 154 340 622 224 593 114 312 704 000  $q^{2649}$  +  
 967 585 342 255 734 123 448 831 517 701 904 935 042 984 226 121 355 599 460 338 128 510 125 992 326 3  
 268 405 588 428 960 775 946 477 173 319 050 094 108 930 048  $q^{2652}$  -  
 1 019 881 524 345 213 667 492 882 207 592 340 735 834 712 566 265 042 312 733 609 609 879 652 554 985 3  
 885 378 079 125 344 288 468 479 617 650 962 848 189 417 033  $q^{2653}$  +  
 1 194 277 663 100 438 578 753 145 422 973 472 932 627 626 407 188 894 289 197 681 147 899 132 307 786 3  
 518 885 749 127 089 419 516 792 774 259 060 490 203 648 000  $q^{2656}$  -  
 1 258 776 415 987 444 662 067 781 450 451 217 367 656 238 606 456 641 977 581 598 062 835 030 896 104 3  
 793 293 745 185 860 605 062 878 466 540 486 231 274 815 488  $q^{2657}$  +  
 1 473 848 260 748 768 325 746 857 464 528 929 670 248 227 386 367 357 923 703 289 255 131 148 604 529 3  
 104 655 320 115 188 877 918 725 359 630 541 010 700 697 600  $q^{2660}$  -  
 1 553 384 416 202 764 236 726 463 281 636 965 885 920 083 225 174 697 978 424 800 129 105 278 511 814 3  
 758 420 204 581 492 593 777 218 093 270 149 349 203 378 500  $q^{2661}$  +  
 1 818 577 551 224 251 517 333 979 517 649 814 294 587 935 617 742 572 745 522 547 547 229 202 243 223 3  
 133 960 350 955 378 995 849 269 001 441 110 866 310 208 000  $q^{2664}$  -  
 1 916 641 633 503 431 545 817 732 447 301 280 040 530 034 586 215 840 972 486 853 161 100 129 878 995 3  
 856 192 072 895 503 774 812 948 675 168 762 648 736 563 200  $q^{2665}$  +  
 2 243 585 480 949 304 193 023 384 992 857 855 735 851 732 533 432 717 054 128 731 123 146 415 980 784 3  
 884 459 183 168 807 048 537 383 246 408 613 994 452 019 200  $q^{2668}$  -  
 2 364 474 705 240 639 376 887 579 528 035 388 979 182 120 427 937 250 175 234 900 214 236 236 162 311 3  
 787 513 684 538 974 540 259 652 998 814 194 433 549 148 750  $q^{2669}$  +  
 2 767 485 229 013 454 961 841 977 950 847 083 475 524 985 535 544 538 512 961 256 581 562 666 737 561 3  
 069 552 401 270 501 168 501 555 849 367 616 451 969 761 280  $q^{2672}$  -  
 2 916 489 121 416 769 937 556 244 532 913 942 578 255 534 006 229 937 745 492 131 155 737 634 426 773 3  
 994 226 856 070 182 817 259 102 714 223 971 561 346 334 720  $q^{2673}$  +  
 3 413 186 745 338 049 333 911 818 706 484 919 461 820 540 865 010 822 694 655 995 051 390 232 742 564 3  
 122 972 195 017 174 676 396 457 907 269 486 759 415 296 000  $q^{2676}$  -  
 3 596 815 287 986 292 958 005 432 831 416 203 348 648 754 945 003 084 874 179 126 628 438 233 729 275 3  
 211 503 419 921 662 374 954 958 584 795 586 579 390 380 386  $q^{2677}$  +  
 4 208 884 319 260 763 136 093 625 660 729 775 120 758 751 615 091 642 398 029 217 115 283 974 355 315 3  
 707 805 383 822 933 716 821 030 673 267 875 314 917 760 000  $q^{2680}$  -  
 4 435 148 320 593 841 491 894 881 733 548 529 948 420 044 219 522 641 476 111 464 914 157 232 515 438 3  
 155 971 888 701 812 202 753 412 313 104 864 740 155 392 000  $q^{2681}$  +

5 189 270 142 766 835 219 447 007 188 572 943 801 801 823 498 102 869 659 488 669 925 626 606 508 308  
 877 799 785 534 533 123 422 691 865 456 292 483 107 584 000  $q^{2684}$  -  
 5 468 025 735 941 045 824 946 930 698 115 165 119 252 452 999 877 875 017 571 296 450 906 554 803 883  
 936 531 286 502 957 160 447 677 528 389 360 329 146 226 875  $q^{2685}$  +  
 6 397 025 360 067 238 556 088 375 994 976 334 257 566 951 653 612 881 085 221 498 039 085 282 164 737  
 044 213 677 799 050 779 984 541 764 154 646 502 624 657 408  $q^{2688}$  -  
 6 740 397 233 589 051 348 412 736 564 774 130 255 420 657 502 479 854 924 658 521 506 669 965 904 496  
 578 452 910 743 290 969 247 671 997 067 096 281 341 952 000  $q^{2689}$  +  
 7 884 651 776 409 051 563 715 882 217 376 943 839 177 063 859 380 115 674 921 918 484 220 584 081 994  
 442 881 256 534 622 755 467 035 944 187 157 495 836 426 240  $q^{2692}$  -  
 8 307 553 052 483 990 558 101 320 505 192 094 309 131 580 403 397 020 087 481 514 046 691 234 941 861  
 300 243 113 603 284 003 778 526 267 166 769 823 743 603 580  $q^{2693}$  +  
 9 716 721 718 642 630 882 307 213 975 631 153 709 937 381 982 837 177 377 539 576 733 751 017 413 871  
 855 916 799 192 328 099 949 189 021 599 393 711 480 064 000  $q^{2696}$  -  
 10 237 492 453 721 794 561 871 199 344 103 450 704 427 483 809 616 985 456 000 301 433 639 068 778  
 766 949 153 541 758 435 213 130 137 498 335 333 516 192 710 656  $q^{2697}$  +  
 11 972 641 091 536 671 467 661 969 953 003 917 902 191 804 493 260 303 226 066 535 473 460 824 405  
 190 360 381 108 874 776 479 985 908 177 018 666 657 695 692 800  $q^{2700}$  -  
 12 613 832 348 172 165 809 031 704 060 149 943 523 780 960 043 385 121 496 524 388 783 198 817 809  
 871 028 997 914 021 422 759 241 948 807 814 995 072 710 870 250  $q^{2701}$  +  
 14 750 042 183 367 704 518 473 543 375 152 816 052 521 832 422 379 127 491 712 012 779 886 524 766  
 522 020 329 366 346 593 171 567 031 175 713 193 326 399 818 752  $q^{2704}$  -  
 15 539 378 718 412 390 376 353 041 505 075 278 167 620 105 356 544 646 759 015 849 427 583 244 357  
 692 254 335 314 620 569 607 461 322 004 352 705 708 384 256 000  $q^{2705}$  +  
 18 168 949 130 649 588 517 615 684 249 473 077 697 280 961 614 025 261 192 180 764 629 914 763 856  
 632 945 107 579 784 636 650 731 384 255 815 912 818 209 658 880  $q^{2708}$  -  
 19 140 511 213 707 350 526 772 940 614 371 388 191 138 241 570 438 492 197 225 987 021 700 981 174  
 770 509 241 950 175 661 063 544 683 960 686 641 697 782 611 875  $q^{2709}$  +  
 22 376 891 242 438 376 922 112 903 662 698 664 202 548 972 137 613 917 852 791 905 147 306 132 814  
 064 294 024 596 589 789 908 732 862 106 734 106 964 036 058 112  $q^{2712}$  -  
 23 572 565 268 174 079 517 538 659 564 867 261 466 802 978 767 682 236 660 759 441 144 826 414 388  
 562 926 541 528 887 581 893 711 054 836 884 541 427 682 443 264  $q^{2713}$  +  
 27 555 178 939 798 455 182 133 267 863 006 315 960 173 727 794 936 769 827 151 352 305 393 047 910  
 474 755 881 591 273 597 191 268 707 364 431 072 550 074 880 000  $q^{2716}$  -  
 29 026 437 704 883 516 358 530 534 511 418 935 476 041 376 044 066 035 697 926 610 977 786 047 671  
 044 970 850 454 322 474 139 447 314 114 080 914 832 438 671 636  $q^{2717}$  +  
 33 926 605 513 052 674 233 152 141 611 411 030 191 824 552 298 505 417 487 763 632 346 157 110 175  
 613 148 393 840 268 469 521 600 844 469 372 338 611 692 134 400  $q^{2720}$  -  
 35 736 692 753 814 490 413 644 774 347 523 043 432 338 553 481 921 774 179 271 985 362 624 580 503  
 203 725 699 320 687 233 689 662 147 074 155 386 537 119 744 000  $q^{2721}$  +  
 41 764 897 228 623 905 239 483 141 775 233 722 771 981 038 730 644 071 220 679 900 815 244 216 338  
 613 281 713 930 980 508 154 122 213 669 991 058 534 983 680 000  $q^{2724}$  -  
 43 991 507 822 244 271 268 325 437 037 217 558 743 548 291 673 364 781 015 542 338 509 718 231 928  
 492 894 798 311 076 194 366 462 412 213 047 913 506 807 783 900  $q^{2725}$  +  
 51 406 306 962 431 388 666 741 450 073 062 501 979 299 347 999 465 207 653 335 870 267 673 759 881  
 669 390 031 129 722 213 517 505 784 101 436 571 888 360 952 832  $q^{2728}$  -  
 54 144 874 771 653 359 271 189 055 787 263 340 982 342 324 301 333 330 355 820 249 211 950 166 700  
 532 540 901 792 327 584 059 322 098 423 580 567 896 457 216 000  $q^{2729}$  +  
 63 263 835 473 747 898 867 069 108 011 206 340 066 695 494 904 907 076 555 500 624 594 743 220 232  
 907 081 533 089 095 979 357 472 077 336 311 067 928 951 925 248  $q^{2732}$  -  
 66 631 566 004 683 639 715 290 251 187 264 434 540 644 306 462 632 998 639 182 045 351 988 374 578  
 987 600 762 747 014 586 949 640 984 966 829 870 168 144 529 712  $q^{2733}$  +  
 77 844 673 300 139 615 009 887 537 817 086 728 427 479 157 665 678 123 950 321 372 736 855 311 866  
 455 581 406 946 322 216 173 179 299 859 449 375 694 620 160 000  $q^{2736}$  -  
 81 985 489 174 416 032 081 527 835 178 897 234 515 814 264 469 985 015 585 881 913 438 879 459 893

470 772 649 281 546 423 299 672 750 620 763 583 162 563 035 136  $q^{2737} +$   
 95 771 589 497 470 032 310 506 132 994 830 213 796 145 615 962 813 994 265 886 014 541 840 308 691  
 920 785 129 502 274 495 888 016 321 318 980 987 429 001 932 800  $q^{2740} -$   
 100 862 194 471 889 174 310 033 570 315 510 166 765 527 262 165 140 278 670 189 287 004 583 987 171  
 050 097 663 702 222 718 661 679 525 094 512 217 109 673 504 125  $q^{2741} +$   
 117 809 156 503 786 128 260 102 624 146 629 174 644 204 090 768 696 302 388 909 710 626 049 423 342  
 968 180 040 917 369 449 402 781 054 092 783 832 281 779 200 000  $q^{2744} -$   
 124 066 469 940 619 505 496 388 560 774 298 295 275 251 718 252 112 302 396 614 751 169 777 839 305  
 452 722 782 189 980 824 207 043 317 217 633 653 784 130 355 200  $q^{2745} +$   
 144 895 899 913 573 360 231 117 016 697 202 246 857 438 890 305 787 324 574 185 989 793 690 630 212  
 723 164 953 282 900 725 546 175 142 054 726 691 827 490 867 200  $q^{2748} -$   
 152 586 170 091 464 721 179 936 709 356 466 252 326 593 148 790 881 713 538 263 868 452 688 385 103  
 613 677 093 375 208 261 795 624 130 012 107 334 383 480 590 875  $q^{2749} +$   
 178 183 706 023 939 046 700 855 369 118 889 440 662 522 593 882 757 796 377 829 345 627 244 368 497  
 959 765 188 360 562 182 548 343 082 965 974 421 708 601 327 616  $q^{2752} -$   
 187 633 679 778 662 635 129 131 011 933 708 512 122 596 428 726 711 465 052 329 045 338 602 488 784  
 667 408 813 232 941 971 245 467 248 533 774 734 145 756 692 480  $q^{2753} +$   
 219 086 118 569 953 830 981 711 332 071 377 317 367 319 660 400 477 734 056 471 178 353 814 113 852  
 991 973 738 687 026 375 401 153 988 631 715 619 018 813 440 000  $q^{2756} -$   
 230 696 729 270 033 489 266 118 533 889 032 695 752 942 488 543 604 804 588 330 607 396 738 542 753  
 122 175 671 937 927 727 696 091 224 815 690 477 589 697 997 721  $q^{2757} +$   
 269 337 521 211 427 256 553 137 036 992 264 357 382 349 666 200 606 894 313 254 092 544 420 031 755  
 281 948 399 050 818 842 969 605 114 793 004 081 268 455 628 800  $q^{2760} -$   
 283 600 660 430 690 488 270 405 944 057 883 834 729 189 830 938 632 509 391 857 171 268 210 466 238  
 749 652 507 529 267 523 374 554 413 625 437 703 720 824 832 000  $q^{2761} +$   
 331 065 648 856 388 075 453 762 752 006 810 230 068 476 664 019 498 978 693 855 815 452 894 705 545  
 151 454 552 119 881 756 521 833 226 411 668 274 154 376 512 000  $q^{2764} -$   
 348 584 713 486 323 577 511 485 950 558 398 679 955 828 674 748 118 426 410 925 965 919 157 376 247  
 919 986 955 625 168 059 599 409 914 549 010 554 912 224 934 475  $q^{2765} +$   
 406 880 416 866 384 671 044 130 945 564 191 391 484 838 605 454 508 206 114 102 445 051 246 287 964  
 354 595 317 723 696 507 538 911 181 949 077 774 841 026 527 232  $q^{2768} -$   
 428 395 477 922 567 226 767 129 753 665 532 780 308 819 369 108 934 723 235 103 400 655 763 279 728  
 304 951 548 192 179 177 624 265 010 511 818 048 639 934 464 000  $q^{2769} +$   
 499 982 724 634 764 929 930 548 808 429 570 381 436 290 366 611 328 488 005 804 384 760 994 832 238  
 308 478 545 607 582 641 424 957 018 699 866 197 123 395 952 640  $q^{2772} -$   
 526 401 352 888 411 527 450 263 581 122 349 239 303 373 521 735 820 139 526 737 906 687 627 332 523  
 646 024 383 507 404 563 523 211 880 012 874 885 301 826 243 711  $q^{2773} +$   
 614 297 705 879 144 773 318 917 538 947 999 719 726 870 587 970 313 438 946 223 646 874 839 283 147  
 717 775 974 814 752 051 011 054 777 658 301 455 653 160 896 000  $q^{2776} -$   
 646 732 720 297 862 197 062 480 966 338 195 932 189 009 881 531 369 007 164 668 269 923 986 073 231  
 438 161 161 587 918 842 507 550 530 086 605 305 685 015 724 032  $q^{2777} +$   
 754 637 895 099 971 348 020 358 368 040 492 608 048 582 644 417 516 775 734 570 072 155 765 441 694  
 587 732 355 140 405 656 613 092 551 676 632 181 212 947 712 000  $q^{2780} -$   
 794 453 582 200 111 165 479 186 428 605 926 784 414 488 636 384 581 698 985 330 315 348 817 657 369  
 804 310 188 678 892 826 722 681 641 366 431 598 710 374 087 125  $q^{2781} +$   
 926 902 998 128 615 532 460 435 686 545 809 870 231 588 387 197 868 174 666 837 666 609 916 197 644  
 658 517 387 760 906 142 362 825 710 489 967 959 525 839 872 000  $q^{2784} -$   
 975 771 695 061 452 835 585 216 281 361 346 055 116 568 227 258 869 685 857 332 975 136 392 413 376  
 392 962 899 701 940 307 345 075 789 484 712 105 455 494 758 400  $q^{2785} +$   
 1 138 324 443 454 644 691 486 008 122 424 469 119 360 809 981 751 937 009 819 719 988 831 942 454 889  
 745 167 644 048 806 246 905 795 434 615 836 839 882 027 073 536  $q^{2788} -$   
 1 198 295 798 801 988 356 879 398 457 713 072 679 127 977 678 895 247 909 022 787 518 418 272 240 904  
 173 771 557 586 376 982 133 392 515 516 869 700 199 120 106 625  $q^{2789} +$   
 1 397 764 709 788 074 127 780 854 794 406 395 182 401 375 610 851 013 978 509 693 709 728 314 070 924  
 963 210 755 786 924 719 257 738 716 094 418 082 104 802 311 680  $q^{2792} -$

1 471 350 450 505 376 676 341 306 323 749 532 066 429 621 280 507 316 813 101 193 129 493 744 818 347 901 467 190 321 407 155 639 742 328 789 988 467 108 040 310 784  $q^{2793} +$   
 1 716 083 646 916 072 156 959 777 781 497 837 359 344 540 146 463 040 398 422 907 240 249 370 485 754 807 082 968 428 705 727 694 742 289 864 967 888 110 748 288 000  $q^{2796} -$   
 1 806 361 308 218 200 543 027 783 852 958 398 459 479 747 209 472 641 291 873 675 746 641 499 533 819 831 224 183 013 183 206 034 334 344 295 349 643 633 234 054 747  $q^{2797} +$   
 2 106 586 720 201 024 385 460 411 611 006 067 110 466 745 502 211 629 273 050 328 256 838 394 330 672 432 435 997 229 671 778 633 857 194 022 132 952 238 583 398 400  $q^{2800} -$   
 2 217 326 562 545 442 989 139 227 627 724 203 356 296 675 758 904 215 163 188 460 617 227 405 118 358 016 112 567 230 107 318 327 348 248 355 485 451 389 005 824 000  $q^{2801} +$   
 2 585 573 422 396 476 874 190 574 093 039 618 056 439 763 304 423 387 401 285 311 644 504 350 904 411 009 529 534 259 798 033 313 899 059 328 940 861 582 167 296 000  $q^{2804} -$   
 2 721 393 696 700 116 493 761 192 830 575 148 337 203 580 087 406 722 564 838 221 144 904 297 583 303 774 314 137 675 882 610 551 915 419 685 993 729 604 360 128 900  $q^{2805} +$   
 3 173 008 141 967 023 080 128 527 552 736 038 141 956 406 870 233 240 528 251 282 287 819 807 754 516 981 899 668 237 800 611 659 188 623 592 847 185 261 300 330 496  $q^{2808} -$   
 3 339 565 008 132 338 986 638 098 389 415 286 640 693 573 698 658 842 550 583 718 097 304 129 886 327 574 737 741 803 149 474 558 320 293 880 269 673 776 234 496 248  $q^{2809} +$   
 3 893 340 715 901 090 218 209 042 810 159 640 943 631 762 824 201 064 466 790 880 509 410 906 061 576 110 915 157 394 660 939 605 611 479 406 065 301 136 226 355 200  $q^{2812} -$   
 4 097 560 516 142 863 872 908 334 731 789 642 662 772 856 785 246 616 735 650 798 877 527 544 346 745 624 148 790 389 752 910 054 504 798 321 593 358 814 737 328 239  $q^{2813} +$   
 4 776 509 923 517 983 583 203 648 130 573 359 515 792 850 022 617 122 074 500 143 569 262 459 947 222 050 148 651 596 456 376 856 343 318 360 897 572 628 561 920 000  $q^{2816} -$   
 5 026 873 216 363 832 981 545 775 220 907 296 557 015 816 515 075 378 661 176 837 626 296 832 560 715 474 836 948 112 903 117 586 039 229 135 162 856 775 182 385 152  $q^{2817} +$   
 5 859 170 535 414 218 031 469 568 627 456 617 867 008 823 922 897 698 181 358 457 245 401 346 129 310 309 462 943 553 697 005 615 460 559 692 575 839 841 035 059 200  $q^{2820} -$   
 6 166 059 376 230 772 311 718 012 050 290 524 099 988 576 454 244 931 736 920 244 226 291 316 164 654 715 896 479 303 131 910 530 919 318 218 593 224 660 714 352 500  $q^{2821} +$   
 7 186 193 510 272 919 396 401 131 168 222 771 275 378 263 708 945 602 827 217 934 438 467 214 765 757 032 324 271 419 746 971 089 738 713 759 009 905 135 917 824 000  $q^{2824} -$   
 7 562 316 002 168 551 518 292 811 107 495 489 192 834 676 657 769 539 006 821 053 800 792 830 374 681 842 158 481 892 196 815 976 045 672 400 968 010 448 848 486 400  $q^{2825} +$   
 8 812 499 887 372 003 575 386 999 664 209 517 675 297 776 578 426 539 099 898 799 368 729 924 250 761 334 211 870 291 614 764 416 196 459 321 737 199 525 094 366 208  $q^{2828} -$   
 9 273 409 122 779 189 579 713 865 043 127 403 838 017 692 005 897 140 698 157 444 673 679 054 058 568 988 044 681 406 149 227 788 131 804 686 072 525 033 927 160 000  $q^{2829} +$   
 10 805 302 287 552 383 273 889 409 182 071 338 912 486 773 769 932 531 341 030 690 276 814 541 730 023 336 081 648 660 335 943 711 246 707 698 216 329 506 822 946 816  $q^{2832} -$   
 11 370 030 578 061 580 663 637 089 726 765 700 735 424 164 901 868 745 410 087 586 298 570 584 571 550 998 111 590 491 622 878 664 144 015 379 084 309 250 017 853 440  $q^{2833} +$   
 13 246 844 238 008 252 697 036 158 351 662 060 032 730 414 205 978 740 103 416 030 822 268 109 647 993 371 728 023 948 876 657 672 192 140 315 998 547 774 825 728 000  $q^{2836} -$   
 13 938 678 137 172 646 158 172 161 455 522 061 995 253 231 708 382 867 874 905 924 235 835 457 347 080 847 012 810 958 929 751 107 810 048 413 778 306 505 741 347 735  $q^{2837} +$   
 16 237 747 419 539 939 179 670 049 048 913 609 461 722 418 592 067 711 850 045 238 317 980 918 483 281 393 261 616 080 381 939 159 233 624 939 893 557 048 340 275 200  $q^{2840} -$   
 17 085 174 661 957 980 203 706 749 149 260 608 941 204 680 735 866 290 557 467 819 815 275 601 749 042 196 866 659 548 137 531 605 987 286 750 921 797 399 982 080 000  $q^{2841} +$   
 19 901 101 182 018 936 119 474 622 691 913 265 238 071 780 092 336 198 262 485 491 159 889 611 989 954 796 563 231 964 593 531 253 543 404 974 642 346 264 414 720 000  $q^{2844} -$   
 20 938 967 513 146 361 693 213 844 174 082 265 493 301 806 034 868 981 517 171 735 464 948 737 304 975 238 201 080 729 171 873 535 828 483 617 263 448 074 933 262 775  $q^{2845} +$   
 24 387 458 238 477 881 900 786 586 087 168 340 114 339 291 672 138 119 043 978 756 098 602 028 139

650 950 896 418 755 701 842 727 884 679 410 044 699 998 746 148 864  $q^{2848}$  -  
 25 658 380 462 577 063 879 681 142 487 350 429 811 447 533 984 580 423 420 208 165 126 724 345 987  
 714 755 850 559 597 831 837 741 432 031 476 843 834 499 530 752 000  $q^{2849}$  +  
 29 880 936 491 743 599 653 363 711 693 914 641 646 402 496 130 227 369 706 067 343 643 471 894 784  
 325 878 918 328 986 293 181 361 541 048 398 871 329 094 862 602 240  $q^{2852}$  -  
 31 437 028 247 972 646 481 821 490 602 657 265 921 812 941 963 024 457 551 478 350 985 703 384 803  
 633 888 135 874 673 190 992 163 932 045 159 276 211 807 335 316 345  $q^{2853}$  +  
 36 606 670 883 716 514 402 195 643 560 218 001 204 963 864 023 953 113 942 696 549 052 183 444 588  
 598 217 120 961 594 397 877 673 622 766 741 147 623 694 118 144 000  $q^{2856}$  -  
 38 511 650 071 681 746 090 930 419 137 411 832 050 490 720 841 676 855 047 442 217 844 648 445 211  
 407 913 235 891 331 082 383 732 341 409 765 574 908 931 385 360 384  $q^{2857}$  +  
 44 839 912 707 345 174 301 956 535 504 176 390 135 115 858 357 456 030 665 633 788 181 402 292 604  
 678 647 697 302 338 940 464 402 721 287 023 834 685 374 044 416 000  $q^{2860}$  -  
 47 171 674 609 263 524 090 286 083 610 570 923 535 654 942 569 893 919 349 384 801 645 720 282 648  
 489 334 990 967 085 158 643 297 293 589 034 860 861 784 624 178 250  $q^{2861}$  +  
 54 917 139 079 861 662 717 731 906 359 398 129 399 001 862 752 792 224 144 536 373 974 374 424 909  
 604 184 061 825 310 094 878 734 568 601 960 264 066 860 609 024 000  $q^{2864}$  -  
 57 770 897 658 017 052 361 985 849 020 100 093 924 900 285 580 646 646 720 166 654 655 680 287 490  
 386 377 830 143 465 143 147 551 576 949 064 620 195 397 625 446 400  $q^{2865}$  +  
 67 249 614 792 291 591 217 717 132 329 687 810 809 918 230 094 277 964 163 407 338 802 503 379 010  
 091 555 279 399 789 365 051 585 377 140 450 968 754 055 720 157 184  $q^{2868}$  -  
 70 741 737 097 161 775 646 335 812 044 780 524 163 947 762 663 296 073 436 016 938 392 878 615 135  
 539 492 266 799 412 669 336 504 994 907 956 908 667 832 294 822 625  $q^{2869}$  +  
 82 339 945 626 757 899 240 591 793 833 133 869 583 162 871 476 533 663 383 224 184 239 742 567 792  
 348 702 417 556 957 944 949 311 576 608 150 457 660 235 008 093 184  $q^{2872}$  -  
 86 612 631 608 398 872 836 691 182 512 588 639 731 058 282 052 669 377 286 437 967 919 538 328 162  
 824 844 434 020 341 121 531 434 783 638 087 939 572 764 897 869 824  $q^{2873}$  +  
 100 802 280 243 910 282 855 584 471 062 061 193 918 245 159 890 071 128 583 143 040 646 361 531 059  
 450 730 842 655 875 338 239 469 865 465 402 149 589 548 756 992 000  $q^{2876}$  -  
 106 029 273 581 852 159 022 736 316 352 721 346 285 508 695 255 654 916 338 775 955 261 226 756 632  
 154 970 873 852 817 792 943 652 583 655 840 714 075 295 792 526 885  $q^{2877}$  +  
 123 386 961 479 323 051 769 544 883 882 808 100 378 817 386 989 352 530 968 670 140 717 129 782 688  
 873 014 960 950 163 387 704 093 334 890 188 777 370 112 060 948 480  $q^{2880}$  -  
 129 780 517 629 752 172 948 283 441 332 743 544 712 159 646 234 810 727 506 815 850 042 171 288 806  
 451 319 320 436 659 267 924 460 725 560 037 564 630 289 199 104 000  $q^{2881}$  +  
 151 010 602 934 625 724 523 594 138 586 205 682 888 407 814 452 586 653 224 528 766 685 795 330 026  
 190 690 967 317 215 871 077 600 327 686 423 379 227 771 101 184 000  $q^{2884}$  -  
 158 829 990 013 525 830 591 105 606 674 288 950 231 263 618 064 669 015 876 572 354 426 535 109 207  
 235 457 498 548 453 207 424 025 761 510 921 712 153 638 347 379 350  $q^{2885}$  +  
 184 792 779 898 501 693 676 048 773 338 503 469 022 516 154 539 998 672 939 967 272 827 430 971 764  
 899 447 048 005 761 797 650 650 518 686 687 398 587 730 026 253 056  $q^{2888}$  -  
 194 354 648 191 675 383 681 642 499 145 130 210 805 574 592 805 242 827 805 516 940 771 321 716 416  
 207 322 161 981 721 391 945 680 044 894 393 088 944 298 049 536 000  $q^{2889}$  +  
 226 100 783 143 797 727 973 388 665 971 940 276 820 983 698 593 924 741 932 533 639 920 309 980 744  
 624 780 046 335 270 024 498 567 859 198 295 802 625 931 155 781 632  $q^{2892}$  -  
 237 791 812 288 972 609 522 028 945 490 478 129 624 137 414 510 803 748 257 585 212 190 916 191 930  
 315 754 929 940 456 436 424 952 844 842 863 039 335 699 877 924 394  $q^{2893}$  +  
 276 604 200 062 012 241 714 692 961 317 441 328 450 714 906 090 486 255 964 413 032 648 980 778 978  
 679 432 807 922 861 290 657 555 566 938 036 023 205 003 327 488 000  $q^{2896}$  -  
 290 896 522 116 910 942 581 457 961 187 950 534 008 243 418 629 462 925 163 891 603 789 283 046 636  
 814 716 609 310 122 375 354 537 007 503 045 135 522 557 507 043 328  $q^{2897}$  +  
 338 341 472 123 718 415 180 371 003 779 043 039 107 771 111 648 335 874 284 618 977 089 858 088 412  
 207 599 605 584 664 299 932 352 930 501 115 571 413 655 656 601 600  $q^{2900}$  -  
 355 811 477 260 078 746 787 112 557 156 642 985 279 936 534 060 435 661 465 895 880 953 238 111 886  
 867 086 168 373 527 483 326 941 575 904 830 378 509 496 996 459 250  $q^{2901}$  +

413 801 045 632 858 555 024 801 162 638 123 558 141 318 916 765 296 750 585 839 452 619 928 843 598  
 376 934 892 726 556 691 215 407 111 610 692 887 674 467 133 504 000  $q^{2904}$  -  
 435 152 309 264 778 328 464 200 224 315 037 596 425 784 382 024 611 142 621 281 139 747 000 987 118  
 136 127 332 539 127 779 841 437 216 918 466 129 069 127 294 976 000  $q^{2905}$  +  
 506 020 302 210 494 682 628 600 833 915 175 060 064 815 422 153 036 694 244 338 005 164 635 012 885  
 802 205 403 931 423 230 666 339 330 733 637 043 066 748 323 387 392  $q^{2908}$  -  
 532 111 533 061 964 151 542 697 250 606 894 060 241 376 783 286 159 715 291 470 842 714 568 534 746  
 596 490 992 183 327 065 184 933 927 740 358 793 053 957 936 427 000  $q^{2909}$  +  
 618 706 148 317 653 239 545 016 606 826 645 485 857 193 817 821 444 849 545 615 016 259 341 053 814  
 152 453 366 698 327 449 614 513 515 211 601 077 443 815 560 372 224  $q^{2912}$  -  
 650 585 252 438 687 571 961 788 353 911 489 774 900 798 141 177 277 656 911 725 573 891 489 147 436  
 354 388 214 400 461 214 897 188 045 143 217 809 946 356 567 736 320  $q^{2913}$  +  
 756 381 986 039 523 446 777 150 072 033 386 070 554 302 074 934 013 156 741 975 237 467 093 514 320  
 174 627 075 093 678 823 409 730 567 491 109 684 822 263 828 506 752  $q^{2916}$  -  
 795 327 579 601 436 883 662 320 717 523 223 119 579 653 868 163 949 689 602 145 778 368 186 935 758  
 778 747 462 599 660 594 667 812 021 016 447 767 927 691 020 133 508  $q^{2917}$  +  
 924 566 812 660 332 118 614 076 043 092 572 238 758 464 954 965 726 293 542 754 226 550 065 313 778  
 025 131 162 398 068 087 626 574 802 725 257 967 716 624 969 446 400  $q^{2920}$  -  
 972 138 805 619 914 162 564 380 541 172 584 650 633 132 932 243 626 909 644 413 116 842 697 620 057  
 137 272 159 006 544 864 121 188 314 250 120 345 394 420 547 584 000  $q^{2921}$  +  
 1 129 993 443 564 351 535 852 267 929 650 968 263 506 926 651 680 749 202 884 248 762 798 776 783 637  
 597 427 499 398 397 737 984 253 578 571 028 539 328 784 276 736 000  $q^{2924}$  -  
 1 188 094 668 063 589 972 768 022 765 211 941 855 880 218 697 910 004 728 916 383 469 455 398 675 018  
 172 134 216 534 608 793 365 584 052 770 409 642 253 502 556 619 000  $q^{2925}$  +  
 1 380 874 369 443 250 875 446 927 446 309 826 491 727 014 936 120 650 492 014 163 636 950 625 884 872  
 900 413 790 769 392 552 924 682 068 382 377 253 494 960 580 149 248  $q^{2928}$  -  
 1 451 825 654 562 035 704 262 523 007 046 652 433 257 789 950 031 374 817 919 106 845 152 311 701 787  
 338 341 642 700 152 153 669 260 707 479 070 701 995 366 965 248 000  $q^{2929}$  +  
 1 687 225 602 650 554 939 067 155 137 258 215 834 666 994 941 670 570 748 922 153 148 795 212 936 626  
 343 279 853 560 123 377 794 552 704 765 503 502 631 206 172 702 720  $q^{2932}$  -  
 1 773 857 217 195 108 301 160 122 108 438 446 427 773 398 945 490 378 246 389 110 640 331 923 083 312  
 771 825 185 193 125 100 024 607 668 536 727 114 574 174 349 863 706  $q^{2933}$  +  
 2 061 261 109 221 534 004 880 866 258 622 555 624 710 811 057 186 610 995 448 901 303 039 828 822 252  
 128 549 972 239 916 783 270 363 972 405 862 507 505 984 989 440 000  $q^{2936}$  -  
 2 167 024 126 451 868 758 900 835 078 415 084 374 348 985 400 188 235 620 362 728 352 867 690 766 783  
 256 209 949 124 642 594 927 592 354 260 937 906 978 173 498 359 808  $q^{2937}$  +  
 2 517 873 148 048 068 198 066 194 175 266 495 632 799 298 938 207 991 074 497 429 853 430 183 318 596  
 490 014 315 410 775 269 733 179 707 293 993 764 845 725 222 451 200  $q^{2940}$  -  
 2 646 975 054 711 044 684 460 535 639 988 065 557 108 012 239 633 335 545 798 896 899 724 182 558 527  
 721 378 297 622 922 227 125 086 002 010 885 839 414 051 904 080 250  $q^{2941}$  +  
 3 075 217 150 729 939 327 187 808 137 908 254 394 154 239 863 142 079 825 750 852 394 455 548 530 413  
 532 459 382 433 197 110 190 305 811 623 444 629 274 344 988 672 000  $q^{2944}$  -  
 3 232 786 956 709 911 582 498 730 422 785 278 613 414 502 137 952 710 267 021 607 435 413 478 226 415  
 525 953 183 091 083 643 112 272 579 756 963 221 488 557 948 928 000  $q^{2945}$  +  
 3 755 423 800 671 734 156 258 500 619 204 378 685 064 563 727 797 993 883 949 240 111 524 896 791 486  
 147 096 384 867 071 262 341 041 889 175 348 389 892 170 778 099 712  $q^{2948}$  -  
 3 947 713 040 487 198 632 372 825 936 596 898 647 733 029 282 212 347 839 720 634 375 199 997 130 116  
 275 410 000 077 484 744 727 111 423 976 886 147 621 990 290 721 250  $q^{2949}$  +  
 4 585 465 860 926 258 964 629 104 844 087 384 757 042 630 384 382 919 817 137 949 468 830 022 184 829  
 005 403 566 218 801 737 707 297 323 554 209 468 089 068 685 382 656  $q^{2952}$  -  
 4 820 093 257 256 804 057 472 218 686 240 329 562 005 830 792 631 234 464 925 732 642 249 575 335 425  
 907 897 775 679 831 503 239 832 617 948 456 544 095 668 039 647 232  $q^{2953}$  +  
 5 598 213 242 609 237 829 754 500 452 386 375 395 544 798 025 445 286 349 938 786 680 280 360 484 305  
 056 236 448 747 393 805 934 564 865 849 789 887 027 001 163 584 000  $q^{2956}$  -  
 5 884 462 477 292 725 461 442 513 803 084 690 963 073 743 894 531 354 454 583 194 213 573 488 209 449

643 150 201 857 439 667 422 941 036 783 193 308 551 113 194 839 840  $q^{2957} +$   
 6 833 717 024 514 939 183 991 847 223 209 734 104 068 617 366 068 795 705 833 001 839 498 989 068 397  
 013 061 942 294 289 805 511 592 166 388 544 430 357 874 868 224 000  $q^{2960} -$   
 7 182 899 097 416 054 111 668 578 258 355 179 809 198 968 284 795 815 747 053 162 025 951 875 160 157  
 702 195 390 714 812 951 425 768 520 244 956 811 781 528 363 008 000  $q^{2961} +$   
 8 340 771 902 928 266 984 221 248 992 625 727 368 610 499 096 653 896 757 704 675 578 443 722 610 824  
 619 291 763 081 763 383 360 921 945 784 234 793 547 673 338 880 000  $q^{2964} -$   
 8 766 666 030 664 991 705 430 635 099 115 159 236 512 621 676 891 969 062 173 013 563 691 458 848 840  
 272 582 274 501 876 785 281 707 730 408 205 482 856 447 451 631 075  $q^{2965} +$   
 10 178 817 199 817 312 862 885 121 181 703 300 319 664 345 196 783 048 028 908 345 129 633 703 584  
 045 072 510 526 668 144 095 661 213 218 536 695 225 324 778 544 437 248  $q^{2968} -$   
 10 698 207 207 841 027 771 483 604 730 341 151 604 770 473 212 053 603 308 503 512 960 980 049 732  
 011 506 213 045 561 353 460 884 213 477 626 514 688 899 324 628 992 000  $q^{2969} +$   
 12 420 249 489 389 782 573 483 539 845 845 788 267 765 039 737 048 328 553 718 278 183 487 909 834  
 174 221 648 488 449 396 521 421 501 717 932 014 442 188 644 346 808 320  $q^{2972} -$   
 13 053 576 295 502 184 112 026 211 822 036 543 948 020 055 794 374 005 033 656 731 256 580 078 101  
 049 282 193 089 295 824 325 439 757 161 562 099 238 138 906 680 372 494  $q^{2973} +$   
 15 153 235 604 676 436 684 562 620 047 786 437 910 690 931 399 870 533 749 194 424 498 256 013 902  
 916 715 564 900 497 743 390 162 634 367 366 064 057 886 911 282 176 000  $q^{2976} -$   
 15 925 390 816 950 211 890 092 821 653 493 560 942 434 281 018 669 996 302 772 675 802 376 608 583  
 387 462 451 570 150 672 557 507 157 005 345 518 080 129 631 759 695 872  $q^{2977} +$   
 18 485 133 848 227 022 143 973 841 646 285 418 830 371 647 142 767 673 265 801 379 451 672 238 460  
 068 883 326 584 699 156 638 207 406 656 823 594 619 510 855 768 473 600  $q^{2980} -$   
 19 426 424 871 854 773 425 845 389 651 133 856 505 779 580 314 082 699 758 691 424 035 669 115 184  
 343 265 649 604 133 372 953 497 050 688 038 702 965 435 318 717 752 375  $q^{2981} +$   
 22 546 654 370 558 337 093 565 835 926 491 250 616 221 375 887 758 877 478 826 395 497 844 481 844  
 092 463 691 629 868 450 536 836 030 568 457 233 422 373 373 593 024 000  $q^{2984} -$   
 23 693 977 938 094 189 058 384 406 435 857 645 997 114 930 946 554 734 455 042 205 973 846 524 191  
 586 596 112 527 957 597 228 066 687 096 903 981 728 114 405 736 448 000  $q^{2985} +$   
 27 496 917 765 155 395 561 717 322 286 939 136 890 315 042 877 289 943 644 459 089 133 503 973 620  
 021 132 242 838 608 210 133 229 652 786 828 052 016 352 713 625 715 200  $q^{2988} -$   
 28 895 186 717 447 777 114 177 399 816 159 567 357 877 586 923 542 292 420 771 522 878 449 161 561  
 463 981 178 141 362 494 570 617 580 200 236 621 917 439 785 349 175 250  $q^{2989} +$   
 33 529 605 012 312 347 741 494 236 804 099 796 948 651 843 815 966 016 202 646 709 977 088 340 518  
 338 239 074 138 170 479 534 323 378 753 203 182 564 682 214 725 574 656  $q^{2992} -$   
 35 233 482 759 515 547 745 824 330 162 999 710 128 816 454 135 887 214 330 158 253 515 820 055 670  
 862 972 323 590 067 677 939 762 493 848 935 212 425 885 104 356 589 568  $q^{2993} +$   
 40 880 433 261 795 813 070 912 684 122 744 836 752 175 641 718 325 487 962 416 973 685 442 262 861  
 708 262 423 270 062 897 717 384 997 183 398 248 695 536 340 973 568 000  $q^{2996} -$   
 42 956 442 004 352 180 851 477 022 325 457 293 509 413 206 489 251 665 063 621 368 043 139 718 625  
 040 703 107 575 145 024 970 114 370 768 444 133 767 125 754 191 506 520  $q^{2997} +$   
 49 836 242 122 392 261 023 008 510 807 188 305 767 249 767 830 053 158 430 463 366 805 902 559 590  
 122 783 864 489 934 810 356 167 679 728 574 788 576 119 309 528 832 000  $q^{3000} -$   
 52 365 325 046 008 862 991 756 029 366 447 319 727 075 973 347 521 726 444 037 589 441 938 227 261  
 770 830 743 794 398 850 632 522 092 259 214 242 178 794 993 803 264 000  $q^{3001} +$   
 60 746 035 998 348 099 533 793 004 425 023 553 383 471 482 654 883 996 426 951 946 782 780 350 877  
 595 483 057 004 689 576 091 432 223 434 680 772 573 488 569 181 696 000  $q^{3004} -$   
 63 826 670 802 054 902 618 120 022 642 753 848 425 376 473 878 005 097 249 406 288 565 591 430 819  
 535 047 256 013 847 465 889 176 120 646 044 723 029 938 285 105 008 150  $q^{3005} +$   
 74 034 401 848 331 985 282 895 601 467 218 947 137 389 077 323 860 551 399 808 887 528 404 203 730  
 412 947 834 699 747 775 512 248 520 877 995 802 319 766 225 001 644 032  $q^{3008} -$   
 77 786 383 759 505 526 985 401 180 362 794 194 052 143 586 956 605 157 415 795 415 193 902 543 723  
 746 546 433 782 224 953 441 451 480 586 399 222 325 411 733 233 664 000  $q^{3009} +$   
 90 217 811 291 468 627 509 401 660 589 186 266 298 177 894 496 214 204 186 397 046 539 994 801 525  
 895 008 701 489 832 269 297 319 263 523 278 193 584 895 275 307 548 672  $q^{3012} -$

94 786 848 940 017 540 870 502 161 282 910 732 045 590 348 275 578 294 279 308 374 054 363 241 691 3  
 783 284 245 966 119 552 899 903 069 031 643 703 393 084 602 283 187 653  $q^{3013} +$   
 109 924 424 577 675 577 532 955 942 411 523 451 266 176 685 977 424 960 240 621 391 855 212 497 014 3  
 009 983 334 091 144 064 447 396 041 788 968 983 455 931 204 739 200 000  $q^{3016} -$   
 115 487 722 680 579 578 199 675 075 470 735 826 263 056 208 773 688 674 866 922 828 420 161 958 009 3  
 766 861 448 999 899 630 673 479 477 897 593 732 066 635 661 093 502 976  $q^{3017} +$   
 133 918 145 609 482 535 468 323 878 770 540 244 042 072 199 182 518 685 709 606 932 767 221 101 825 3  
 060 120 329 988 857 615 915 483 522 034 034 230 544 905 359 210 649 600  $q^{3020} -$   
 140 691 185 491 466 828 673 864 063 666 688 170 011 321 663 923 547 557 804 603 821 859 318 976 630 3  
 598 348 808 200 800 536 005 791 022 472 119 334 400 334 748 266 330 500  $q^{3021} +$   
 163 127 836 834 076 744 442 776 023 168 313 642 375 186 777 681 741 293 297 274 752 740 966 132 142 3  
 825 237 243 612 274 117 874 680 858 826 843 248 240 985 150 406 656 000  $q^{3024} -$   
 171 372 610 754 602 599 817 119 526 441 041 759 303 130 883 610 314 872 721 726 120 519 522 672 079 3  
 938 913 301 710 559 003 796 848 637 325 690 943 428 778 403 218 686 200  $q^{3025} +$   
 198 682 796 331 451 518 483 158 533 155 170 689 280 665 784 551 978 767 291 926 532 806 112 324 811 3  
 104 516 223 497 294 256 198 237 886 898 276 530 360 924 176 356 870 144  $q^{3028} -$   
 208 717 806 066 179 182 419 541 979 866 684 772 184 211 478 927 279 364 864 782 502 173 760 538 623 3  
 307 726 710 076 567 771 554 082 649 892 407 839 009 872 258 869 259 000  $q^{3029} +$   
 241 955 833 966 954 758 042 074 976 446 188 285 675 059 012 637 689 844 050 838 091 825 146 736 026 3  
 885 023 284 787 969 419 416 028 938 903 398 554 890 015 732 570 937 856  $q^{3032} -$   
 254 168 230 117 474 648 395 756 670 290 880 702 737 355 474 443 785 162 181 100 154 953 147 471 976 3  
 764 100 611 657 115 221 417 799 966 728 114 443 416 891 712 354 189 312  $q^{3033} +$   
 294 615 567 721 079 739 050 389 374 732 788 225 411 262 838 952 303 723 707 545 108 086 854 878 931 3  
 552 974 114 230 371 852 617 597 627 859 731 692 706 464 986 959 360 000  $q^{3036} -$   
 309 475 886 237 884 297 572 195 607 549 915 124 925 039 842 825 127 958 098 318 491 831 480 122 724 3  
 559 656 564 929 152 352 568 492 257 351 883 166 886 428 130 695 955 179  $q^{3037} +$   
 358 689 905 745 943 792 288 372 459 614 557 298 393 326 114 321 280 920 647 116 380 958 708 209 864 3  
 881 905 149 852 196 336 739 753 297 225 733 691 599 877 426 662 400 000  $q^{3040} -$   
 376 769 955 096 791 588 137 429 509 248 029 104 339 285 239 162 422 438 686 001 932 651 474 249 703 3  
 336 802 296 984 952 436 492 677 645 548 608 120 022 199 034 236 928 000  $q^{3041} +$   
 436 643 097 021 534 520 042 902 957 907 905 112 796 074 489 462 051 059 542 339 998 558 734 344 336 3  
 904 988 257 677 986 446 741 106 049 652 134 759 850 216 610 492 416 000  $q^{3044} -$   
 458 637 666 890 945 563 570 963 287 620 720 118 430 072 271 674 534 278 980 010 772 040 630 562 784 3  
 670 590 896 242 953 297 832 964 808 806 127 022 874 528 571 420 102 275  $q^{3045} +$   
 531 469 239 057 126 805 667 731 027 754 418 162 067 512 434 767 506 068 774 942 506 411 184 076 275 3  
 942 219 394 415 760 203 478 252 769 078 607 141 610 105 053 179 110 400  $q^{3048} -$   
 558 222 443 742 822 971 342 185 058 625 597 741 741 338 023 659 209 630 234 987 722 073 851 408 112 3  
 111 625 363 178 064 222 643 424 623 345 654 921 165 534 695 288 832 000  $q^{3049} +$   
 646 805 743 490 538 701 321 960 730 962 655 594 065 639 188 729 708 880 011 754 016 342 436 298 138 3  
 150 491 200 513 684 435 109 577 474 055 944 089 442 135 156 475 758 592  $q^{3052} -$   
 679 342 985 495 734 525 729 808 642 301 458 378 752 286 814 972 614 830 169 864 166 496 214 493 551 3  
 464 442 930 695 585 261 288 945 540 330 022 710 022 260 060 480 371 951  $q^{3053} +$   
 787 071 002 165 104 057 653 938 473 229 887 464 040 192 125 216 237 665 903 924 732 636 058 173 577 3  
 440 748 297 115 473 458 968 799 972 761 691 116 983 793 782 435 840 000  $q^{3056} -$   
 826 637 750 194 068 551 966 392 810 964 368 575 999 329 633 789 118 692 889 389 176 117 603 847 518 3  
 873 220 166 438 926 427 891 765 920 835 554 290 686 482 644 791 689 216  $q^{3057} +$   
 957 631 394 509 688 945 722 193 702 183 220 641 008 720 194 982 679 730 148 618 497 641 989 198 553 3  
 958 473 942 137 896 386 274 451 773 854 487 829 692 620 550 068 736 000  $q^{3060} -$   
 1 005 740 222 805 082 017 960 410 988 355 609 397 816 708 473 481 269 033 804 208 145 012 616 964 846 3  
 317 587 666 671 085 037 531 513 800 555 026 132 407 361 245 776 957 375  $q^{3061} +$   
 1 165 003 864 706 384 464 934 887 605 060 128 794 567 938 063 558 980 784 756 466 575 598 234 911 029 3  
 224 947 734 883 237 895 365 688 527 438 111 770 369 753 528 421 120 000  $q^{3064} -$   
 1 223 491 506 668 860 583 580 461 427 322 285 904 824 803 550 067 791 855 072 470 149 240 192 181 352 3  
 474 949 337 688 561 348 459 799 131 896 131 508 883 319 800 101 273 600  $q^{3065} +$   
 1 417 101 613 985 262 360 828 986 628 942 757 779 470 271 587 734 728 529 554 656 921 630 499 345 216 3

561 368 275 152 664 619 506 124 043 006 462 302 811 515 969 173 149 696  $q^{3068}$  -  
 1 488 198 153 472 184 556 006 140 188 305 695 824 380 922 825 728 765 093 506 444 166 869 536 597 665  
 583 046 587 484 050 923 522 395 540 923 446 403 941 968 490 120 030 750  $q^{3069}$  +  
 1 723 532 047 539 000 844 838 074 569 206 290 059 870 568 962 324 090 732 112 402 917 586 463 442 073  
 408 575 475 328 475 745 755 607 747 418 455 884 596 922 979 480 240 128  $q^{3072}$  -  
 1 809 944 819 671 673 266 141 721 579 889 084 058 317 673 301 613 688 031 111 702 718 679 289 163 905  
 504 550 511 795 751 942 338 519 382 994 139 785 857 823 806 757 470 208  $q^{3073}$  +  
 2 095 958 045 160 893 895 926 125 697 020 827 602 093 338 597 758 957 287 835 447 505 038 865 354 705  
 451 482 940 355 447 682 350 722 658 696 440 418 213 133 721 462 784 000  $q^{3076}$  -  
 2 200 973 361 225 741 175 949 586 775 015 762 641 803 837 875 796 861 576 900 599 246 646 295 724 518  
 565 687 773 542 916 232 687 429 665 147 476 298 117 377 933 309 905 026  $q^{3077}$  +  
 2 548 535 960 085 315 505 240 312 094 712 160 847 582 585 382 155 351 712 558 099 143 362 487 189 845  
 573 120 277 863 498 516 033 300 034 162 256 835 473 599 292 585 676 800  $q^{3080}$  -  
 2 676 142 427 954 542 296 700 917 301 447 310 165 300 124 633 259 266 098 546 551 733 276 945 897 114  
 267 750 360 945 858 131 868 537 651 550 037 260 466 456 347 426 816 000  $q^{3081}$  +  
 3 098 446 576 634 327 275 294 451 792 932 121 685 018 802 182 788 520 649 138 573 675 047 103 701 288  
 414 437 945 147 448 107 450 756 977 546 703 715 778 210 425 805 184 000  $q^{3084}$  -  
 3 253 484 582 939 687 474 046 992 405 077 341 865 518 402 076 548 894 000 218 887 756 359 945 337 405  
 332 310 884 939 068 374 812 064 633 690 439 995 945 170 503 687 548 875  $q^{3085}$  +  
 3 766 538 676 860 135 298 991 005 086 577 688 238 597 909 003 840 001 557 120 441 609 254 714 343 059  
 172 839 921 108 461 256 523 693 680 691 551 466 277 972 398 031 372 288  $q^{3088}$  -  
 3 954 881 558 793 641 493 976 068 811 567 905 943 627 419 461 272 722 903 519 751 977 143 736 712 385  
 019 163 926 517 314 321 950 881 651 794 123 272 950 858 511 327 232 000  $q^{3089}$  +  
 4 578 109 003 544 414 557 662 597 829 416 199 612 027 055 907 713 162 445 541 196 021 461 748 276 258  
 799 647 637 468 447 756 958 206 782 202 619 249 988 083 788 196 595 712  $q^{3092}$  -  
 4 806 882 601 510 762 326 052 646 751 099 873 732 781 654 178 749 725 601 480 330 388 444 145 328 943  
 198 405 903 820 181 916 552 555 011 771 239 159 129 770 465 890 114 162  $q^{3093}$  +  
 5 563 847 411 653 251 068 037 035 677 659 289 657 904 851 963 426 904 033 506 167 755 875 713 414 456  
 552 014 676 520 935 261 910 780 116 771 328 240 044 838 887 274 560 000  $q^{3096}$  -  
 5 841 696 101 201 855 033 112 879 111 733 098 587 969 165 568 812 482 649 781 695 299 300 536 323 419  
 140 087 842 938 739 385 035 096 836 645 199 197 828 524 917 364 719 616  $q^{3097}$  +  
 6 760 982 053 854 015 607 836 884 819 414 516 262 182 266 569 569 398 311 372 654 039 625 132 953 869  
 231 879 031 721 330 667 161 619 579 603 347 652 732 256 424 032 768 000  $q^{3100}$  -  
 7 098 391 057 284 398 245 051 625 839 816 016 363 725 844 447 960 004 729 840 218 729 575 048 372 582  
 022 781 875 382 330 957 208 661 534 624 736 655 394 472 129 799 087 125  $q^{3101}$  +  
 8 214 666 766 877 384 962 696 685 870 740 690 366 807 780 340 038 812 800 852 178 275 624 465 685 417  
 075 199 910 296 572 404 955 743 996 000 309 943 159 764 585 346 048 000  $q^{3104}$  -  
 8 624 352 603 137 355 617 423 457 459 450 888 946 693 643 761 733 171 096 243 568 574 936 370 893 769  
 869 583 003 652 005 226 569 308 485 493 596 969 940 592 257 499 136 000  $q^{3105}$  +  
 9 979 661 678 760 353 853 052 447 475 888 841 408 254 440 204 531 711 930 214 905 025 741 530 647 924  
 908 883 692 837 066 774 889 133 089 063 129 393 549 336 788 764 655 616  $q^{3108}$  -  
 10 477 045 099 018 352 275 147 531 616 339 342 335 163 344 743 651 614 355 598 418 840 809 701 506  
 264 918 905 568 130 017 008 980 116 312 413 056 241 456 498 182 729 823 875  $q^{3109}$  +  
 12 122 368 761 670 477 386 720 883 062 208 164 334 176 871 287 186 197 420 988 656 159 241 829 821  
 845 174 273 902 575 215 726 335 731 916 067 319 891 251 408 030 970 278 400  $q^{3112}$  -  
 12 726 147 526 942 285 374 340 919 054 951 257 295 997 752 651 469 806 179 346 509 092 197 111 810  
 272 702 334 194 871 501 809 704 753 763 512 506 925 358 603 116 578 832 384  $q^{3113}$  +  
 14 723 296 996 719 586 724 470 405 470 523 566 100 714 223 146 198 190 078 286 000 583 251 595 578  
 285 452 727 400 310 890 572 796 640 198 836 429 993 695 488 457 502 848 000  $q^{3116}$  -  
 15 456 139 491 480 537 219 979 096 837 870 699 457 880 126 558 477 635 340 134 429 480 897 196 723  
 619 620 792 000 347 904 438 774 305 895 725 396 668 180 551 152 504 718 720  $q^{3117}$  +  
 17 880 047 461 563 157 899 278 007 640 446 515 771 805 764 542 090 083 274 095 900 154 634 875 819  
 638 924 504 885 371 953 761 029 989 870 505 385 461 164 490 230 118 400 000  $q^{3120}$  -  
 18 769 432 534 157 284 387 162 368 458 055 073 108 941 342 847 724 153 308 337 748 568 501 279 152  
 497 191 148 909 999 217 482 321 835 030 994 695 608 861 813 945 671 680 000  $q^{3121}$  +

21 710 927 560 822 358 693 693 250 823 636 286 194 198 821 949 750 703 462 153 379 241 068 043 528  
 444 774 117 706 997 657 692 885 338 909 540 040 823 154 196 592 437 760 000  $q^{3124}$  -  
 22 790 161 295 568 656 846 921 496 558 645 598 404 932 416 230 771 355 366 427 926 587 107 370 534  
 769 588 138 849 020 540 523 343 892 380 758 596 659 372 591 231 151 478 875  $q^{3125}$  +  
 26 359 326 472 103 994 345 302 390 969 991 795 458 662 524 186 969 198 281 434 401 307 801 811 851  
 726 498 744 680 047 618 732 628 187 272 768 608 604 618 684 703 747 553 280  $q^{3128}$  -  
 27 668 773 019 872 071 378 792 241 482 507 453 795 977 444 951 308 233 226 409 591 180 024 491 087  
 862 853 238 373 111 152 919 090 244 031 402 835 551 980 605 833 297 920 000  $q^{3129}$  +  
 31 999 011 495 780 099 387 418 884 578 784 679 804 728 850 506 930 157 660 245 803 898 655 506 508  
 771 043 367 797 855 725 548 567 519 824 862 205 747 922 804 040 985 092 096  $q^{3132}$  -  
 33 587 582 849 478 201 740 340 151 102 374 789 801 440 280 040 375 619 650 136 370 749 127 026 509  
 848 323 566 384 149 372 204 851 029 158 924 798 725 667 438 301 955 483 430  $q^{3133}$  +  
 38 840 538 363 356 616 648 409 281 844 092 207 925 137 109 715 545 117 649 859 196 297 860 627 954  
 164 652 370 160 841 963 584 428 197 634 289 470 442 966 194 230 433 226 752  $q^{3136}$  -  
 40 767 497 339 829 903 233 018 435 923 849 081 157 312 244 845 476 525 491 722 169 896 232 323 518  
 355 288 104 548 313 320 786 870 813 204 402 695 383 541 431 504 607 576 064  $q^{3137}$  +  
 47 139 008 870 251 156 112 870 572 578 358 238 141 829 256 373 947 763 734 999 202 597 166 968 561  
 122 428 349 712 854 795 471 033 649 526 805 652 860 532 179 465 872 998 400  $q^{3140}$  -  
 49 476 150 885 482 282 734 429 535 497 223 348 560 952 825 831 038 337 758 148 095 238 894 386 274  
 475 686 509 607 308 251 733 006 315 599 214 274 534 710 904 496 468 408 750  $q^{3141}$  +  
 57 203 457 893 660 132 385 026 406 378 242 466 970 646 961 840 351 595 866 673 426 890 880 666 612  
 037 822 046 440 683 745 238 400 687 715 409 138 299 056 732 578 801 408 000  $q^{3144}$  -  
 60 037 750 798 032 446 836 529 910 966 686 057 010 752 947 309 593 988 710 065 527 064 392 745 932  
 575 701 643 511 182 765 200 778 578 629 876 521 071 026 283 731 255 296 000  $q^{3145}$  +  
 69 408 210 671 709 269 698 363 689 725 175 949 365 947 140 857 189 228 359 271 518 902 361 364 163  
 579 752 307 893 903 241 990 347 167 820 524 072 553 185 952 893 285 196 288  $q^{3148}$  -  
 72 844 988 433 980 963 685 718 718 580 516 105 328 131 617 054 686 310 939 227 026 150 344 273 120  
 070 084 710 526 167 967 544 194 239 388 308 439 167 031 947 302 440 917 625  $q^{3149}$  +  
 84 206 622 251 399 943 879 872 299 509 290 114 497 419 764 619 673 907 904 800 640 993 167 747 124  
 131 296 404 853 044 326 670 683 683 025 067 877 533 078 383 513 964 036 096  $q^{3152}$  -  
 88 373 448 232 049 857 336 496 574 267 736 588 761 850 334 700 616 834 776 935 724 589 720 570 061  
 876 745 313 333 454 557 381 109 283 791 693 971 089 064 325 387 281 268 736  $q^{3153}$  +  
 102 147 696 787 160 249 838 174 323 269 554 420 415 489 233 497 883 671 028 982 415 854 229 245 471  
 879 049 263 305 423 370 776 010 007 191 470 306 086 366 235 082 635 264 000  $q^{3156}$  -  
 107 199 036 433 224 851 302 352 160 226 145 832 148 633 474 705 336 925 210 298 465 170 294 344 456  
 725 008 573 785 494 735 770 446 542 279 373 808 461 589 615 600 033 112 168  $q^{3157}$  +  
 123 896 187 937 011 087 226 558 110 842 996 707 573 200 529 704 811 423 225 286 391 744 873 557 831  
 503 748 959 809 521 737 832 019 701 337 876 188 223 377 729 182 605 004 800  $q^{3160}$  -  
 130 019 059 816 863 803 482 983 972 713 269 543 102 923 617 376 837 680 474 227 585 147 817 494 317  
 726 835 798 464 866 204 604 265 350 592 580 684 382 088 568 805 236 736 000  $q^{3161}$  +  
 150 256 906 635 029 844 907 607 938 070 537 522 188 456 552 483 467 786 342 721 614 768 085 007 330  
 743 224 570 232 144 807 426 033 871 925 019 493 004 059 134 077 613 056 000  $q^{3164}$  -  
 157 677 715 844 264 567 055 053 935 852 611 781 147 030 199 393 142 520 948 128 569 252 310 718 415  
 285 973 954 787 581 204 026 333 713 359 924 991 261 357 854 005 345 233 550  $q^{3165}$  +  
 182 204 113 448 879 036 087 262 185 444 110 325 426 789 804 606 536 718 003 953 551 337 425 840 238  
 957 397 436 222 686 147 279 562 688 425 506 019 505 032 802 510 215 303 168  $q^{3168}$  -  
 191 196 913 801 236 808 216 442 826 948 399 848 830 270 762 751 394 385 227 637 880 718 306 502 714  
 045 696 102 550 591 805 710 381 666 784 489 666 525 733 728 856 903 680 000  $q^{3169}$  +  
 220 917 054 903 020 447 432 291 157 264 527 901 434 002 107 210 381 388 901 569 584 791 393 876 308  
 322 049 076 619 967 955 968 874 135 973 649 093 633 357 157 485 166 166 016  $q^{3172}$  -  
 231 813 537 472 485 183 515 268 234 681 888 951 175 404 477 213 912 184 217 602 020 556 690 535 492  
 942 610 325 997 815 230 242 150 168 217 740 317 813 706 373 583 585 452 519  $q^{3173}$  +  
 267 822 923 003 320 339 457 102 665 576 869 075 934 470 953 494 972 208 435 085 628 611 451 363 756  
 446 983 573 336 768 918 957 035 518 350 527 895 330 944 876 933 114 560 000  $q^{3176}$  -  
 281 024 490 312 451 508 186 705 587 968 487 597 709 388 129 102 817 933 583 958 804 710 639 266 182

729 186 745 121 905 317 529 348 435 381 152 075 345 750 911 038 271 913 984  $q^{3177} +$   
 324 648 782 501 423 554 786 570 138 340 389 067 329 817 298 631 186 768 474 379 677 650 539 716 076  $q^{3178} -$   
 752 146 787 256 402 535 154 174 706 992 760 804 579 720 328 079 565 875 200  $q^{3180} -$   
 340 641 142 135 062 267 377 933 447 978 495 458 135 182 525 721 801 371 747 457 597 394 358 243 530  $q^{3181} +$   
 608 755 627 038 872 531 636 251 772 748 262 411 594 931 588 487 498 280 375  $q^{3181} +$   
 393 484 330 545 400 287 810 452 054 294 277 414 368 772 243 554 781 780 041 589 016 510 706 503 228  $q^{3182} -$   
 651 667 158 906 661 213 314 652 835 017 084 869 838 259 281 350 195 200 000  $q^{3184} -$   
 412 855 131 833 345 071 892 393 127 879 058 867 105 914 938 515 417 567 819 996 826 031 201 907 374  $q^{3185} +$   
 777 886 626 200 587 680 242 495 838 620 337 520 877 835 540 793 358 745 600  $q^{3185} +$   
 476 857 739 553 886 319 476 582 731 585 921 229 477 436 346 042 366 304 132 196 207 895 932 130 597  $q^{3186} -$   
 690 521 152 230 123 762 592 217 715 647 438 179 960 342 755 338 846 976 000  $q^{3188} -$   
 500 317 885 374 466 040 835 991 662 383 017 699 461 493 749 326 810 161 188 101 929 872 718 274 488  $q^{3189} +$   
 820 322 246 535 641 467 427 409 889 579 380 465 933 503 108 136 821 710 250  $q^{3189} +$   
 577 827 300 012 749 682 107 440 944 974 228 215 537 989 665 450 267 937 866 818 651 699 529 235 399  $q^{3190} -$   
 400 973 762 919 246 633 502 218 281 830 449 570 854 668 592 804 478 316 544  $q^{3192} -$   
 606 236 696 533 027 947 348 033 655 250 145 249 194 597 353 450 291 028 313 061 042 151 816 164 622  $q^{3193} +$   
 113 127 979 738 031 918 640 247 202 568 156 185 151 351 822 759 605 960 704  $q^{3193} +$   
 700 092 141 797 978 479 148 551 154 498 523 609 661 763 796 655 392 608 791 558 116 952 377 584 805  $q^{3194} -$   
 130 207 968 647 338 424 265 414 017 243 619 112 828 104 783 891 597 312 000  $q^{3196} -$   
 734 490 806 677 601 421 603 632 556 641 545 373 017 482 040 573 964 932 389 719 667 458 866 195 813  $q^{3197} +$   
 034 894 280 464 297 588 833 240 756 496 305 008 774 457 245 944 593 576 242  $q^{3197} +$   
 848 125 990 298 847 388 897 971 828 341 732 380 614 253 235 983 058 215 263 795 389 664 794 392 845  $q^{3200} -$   
 487 014 840 255 058 646 147 797 555 678 159 532 843 769 227 152 506 470 400  $q^{3200} -$   
 889 771 630 074 833 713 185 072 653 155 373 449 638 549 555 964 940 079 755 820 301 221 546 828 114  $q^{3201} +$   
 900 729 874 999 569 123 691 060 560 511 050 220 956 645 424 055 123 968 000  $q^{3201} +$   
 1 027 338 730 808 679 990 242 003 422 004 019 161 632 316 147 383 175 593 319 346 941 872 092 643 443  $q^{3204} -$   
 450 587 775 551 448 524 990 211 213 702 552 394 995 685 809 884 669 952 000  $q^{3204} -$   
 1 077 752 127 510 314 942 857 749 523 123 417 714 994 485 911 338 754 803 044 831 307 580 047 536 130  $q^{3205} +$   
 467 523 625 929 643 940 154 658 932 813 849 295 176 796 476 910 317 179 725  $q^{3205} +$   
 1 244 271 539 980 229 720 994 994 122 256 417 382 125 931 947 462 342 873 708 695 928 021 049 201 310  $q^{3208} -$   
 428 842 987 553 063 114 970 937 822 868 672 055 702 904 043 503 825 560 576  $q^{3208} -$   
 1 305 291 363 520 614 559 965 163 192 747 488 470 623 806 748 016 855 741 977 493 202 274 416 992 496  $q^{3209} +$   
 610 854 921 224 615 514 859 550 194 530 406 965 945 564 500 625 063 936 000  $q^{3209} +$   
 1 506 832 531 067 599 239 072 428 930 495 094 961 641 571 016 937 626 001 998 566 575 500 999 890 784  $q^{3212} -$   
 150 511 651 773 129 701 095 028 251 953 614 236 102 223 554 747 291 079 680  $q^{3212} -$   
 1 580 681 527 283 752 175 491 691 192 276 485 430 309 891 583 702 869 733 914 808 109 217 175 888 966  $q^{3213} +$   
 482 092 593 104 755 220 448 809 383 370 787 395 155 097 442 232 083 148 062  $q^{3213} +$   
 1 824 581 291 690 051 324 251 379 916 865 270 648 670 505 846 188 382 772 418 429 194 127 436 965 985  $q^{3216} -$   
 777 510 167 785 007 229 299 118 618 118 638 394 517 547 556 955 504 640 000  $q^{3216} -$   
 1 913 946 197 690 927 812 619 829 559 235 767 332 951 403 932 546 615 765 678 984 375 965 136 610 207  $q^{3217} +$   
 961 147 093 819 904 538 326 756 345 717 080 743 164 636 870 014 742 429 696  $q^{3217} +$   
 2 209 072 418 913 465 013 629 765 629 264 504 973 533 732 231 753 634 069 054 853 616 680 995 124 774  $q^{3220} -$   
 342 702 270 841 397 084 188 133 558 962 970 230 564 399 933 274 384 384 000  $q^{3220} -$   
 2 317 200 441 651 576 632 577 911 377 456 766 343 279 572 828 855 306 831 531 084 258 737 925 218 023  $q^{3221} +$   
 125 348 007 952 596 288 768 300 271 122 717 071 669 762 320 408 892 613 000  $q^{3221} +$   
 2 674 270 236 696 317 471 887 138 753 717 887 231 029 729 483 238 237 335 265 230 434 305 510 022 118  $q^{3224} -$   
 186 618 276 392 432 377 282 147 265 393 901 597 556 357 256 509 214 848 000  $q^{3224} -$   
 2 805 085 514 264 975 238 045 881 927 584 757 325 216 736 892 834 469 908 345 620 705 306 584 023 559  $q^{3225} +$   
 257 867 035 691 958 640 758 552 211 461 203 785 920 559 949 836 578 816 000  $q^{3225} +$   
 3 237 049 387 586 476 445 187 366 716 636 588 791 788 780 134 066 021 031 677 244 536 845 749 654 750  $q^{3228} -$   
 825 945 870 127 724 314 608 668 379 403 364 566 068 028 489 194 046 773 248  $q^{3228} -$   
 3 395 293 555 956 209 748 617 977 060 231 138 463 077 681 220 514 151 758 134 105 083 910 251 018 807  $q^{3229} +$   
 939 116 392 493 035 619 244 009 163 835 510 010 377 724 809 986 715 877 125  $q^{3229} +$   
 3 917 799 011 121 013 834 014 362 860 845 563 145 627 940 195 599 582 037 316 352 905 416 412 926 766  $q^{3232} -$   
 409 978 284 281 249 515 320 255 819 335 086 051 541 979 371 995 395 321 856  $q^{3232} -$

4 109 200 846 291 150 294 964 923 451 377 404 051 719 880 623 240 240 130 063 555 724 847 256 913 673  
 116 759 637 187 613 136 230 578 746 463 072 659 715 752 056 233 050 308 608  $q^{3233} +$   
 4 741 151 860 542 289 083 879 510 012 466 572 545 943 637 033 712 886 302 942 052 238 726 631 372 488  
 387 643 094 851 614 996 578 788 685 698 867 197 659 045 380 272 988 160 000  $q^{3236} -$   
 4 972 631 986 790 755 956 701 204 742 971 699 453 429 762 051 806 092 680 483 833 972 990 565 129 098  
 293 338 198 578 943 793 737 643 066 818 835 770 032 133 263 431 939 269 937  $q^{3237} +$   
 5 736 864 093 392 292 634 550 799 672 832 397 928 066 162 372 499 093 558 778 902 929 696 315 298 456  
 390 256 516 283 632 434 040 912 331 660 901 971 152 906 864 669 787 532 800  $q^{3240} -$   
 6 016 781 977 826 682 834 372 777 529 664 492 501 708 962 046 444 513 432 165 448 412 089 038 956 633  
 618 948 063 337 749 795 187 409 241 440 061 868 533 745 544 230 707 200 000  $q^{3241} +$   
 6 940 876 752 119 477 301 157 395 504 067 910 404 884 871 126 147 797 173 489 360 213 311 121 029 804  
 205 987 573 670 924 087 501 273 620 729 716 936 236 275 703 677 591 232 000  $q^{3244} -$   
 7 279 328 686 617 778 450 555 483 319 111 963 403 968 546 094 908 213 638 903 081 473 160 348 607 926  
 691 864 228 623 310 589 905 394 358 713 865 296 078 259 266 578 736 586 200  $q^{3245} +$   
 8 396 596 310 697 704 523 283 717 716 875 052 608 246 710 099 725 231 790 837 458 146 576 997 918 873  
 742 820 183 810 134 033 479 244 654 171 541 502 922 146 423 985 497 489 408  $q^{3248} -$   
 8 805 774 865 768 122 375 933 751 680 052 734 159 584 500 889 014 266 277 799 644 198 103 244 056 711  
 627 471 209 229 879 351 036 057 051 757 459 817 141 731 130 677 354 496 248  $q^{3249} +$   
 10 156 439 322 156 322 588 095 657 967 142 294 306 843 184 023 330 381 264 004 639 806 977 278 518  
 985 617 293 385 984 965 923 340 779 994 396 193 645 605 607 425 935 922 704 384  $q^{3252} -$   
 10 651 066 904 817 112 025 123 862 386 149 391 610 435 122 349 180 337 894 799 809 488 013 121 278  
 864 636 605 649 009 700 952 936 172 599 838 190 087 771 458 184 589 914 694 741  $q^{3253} +$   
 12 283 695 424 159 900 773 845 988 932 445 041 444 191 530 821 811 614 811 611 224 485 492 712 184  
 883 244 662 247 574 492 697 007 916 267 132 309 296 214 349 464 169 740 160 000  $q^{3256} -$   
 12 881 547 157 699 726 625 581 338 712 110 561 008 726 142 134 346 390 045 220 319 123 972 046 009  
 484 036 644 153 916 783 135 335 027 177 187 765 751 503 596 590 956 429 344 768  $q^{3257} +$   
 14 854 774 063 230 438 970 138 945 783 375 906 547 624 317 397 319 827 361 918 525 570 822 631 230  
 428 478 593 151 883 180 624 042 633 087 747 406 739 104 954 976 349 938 124 800  $q^{3260} -$   
 15 577 308 319 718 954 287 415 704 235 249 049 401 246 236 067 270 594 499 980 140 781 678 134 259  
 975 284 285 753 602 328 333 913 112 369 716 582 555 130 056 495 218 500 859 125  $q^{3261} +$   
 17 961 913 665 132 267 580 814 171 710 699 952 040 378 397 997 975 255 715 942 730 273 487 704 680  
 919 846 740 454 829 188 160 302 458 305 580 769 219 435 275 994 816 815 104 000  $q^{3264} -$   
 18 835 032 328 902 443 972 684 334 058 311 794 741 731 963 799 084 092 487 986 930 214 536 167 736  
 802 866 696 129 314 514 102 491 690 657 227 373 041 669 004 361 889 941 094 400  $q^{3265} +$   
 21 716 448 068 972 443 770 105 549 485 183 079 884 822 790 798 804 238 855 825 252 673 983 126 865  
 449 993 302 682 228 084 864 760 031 552 068 792 611 247 790 403 286 799 925 248  $q^{3268} -$   
 22 771 413 119 752 202 550 165 049 640 585 254 625 937 590 809 846 008 353 727 827 049 175 352 229  
 930 593 907 830 143 448 886 260 564 380 463 663 937 712 676 408 202 121 816 125  $q^{3269} +$   
 26 252 744 408 314 064 471 558 491 834 288 514 106 356 557 537 798 063 112 549 215 875 561 468 139  
 336 656 832 107 772 332 597 482 112 212 242 182 141 970 902 522 525 918 575 616  $q^{3272} -$   
 27 527 282 841 042 067 819 997 042 168 551 085 808 828 635 301 469 984 840 465 886 191 650 752 044  
 317 180 001 466 551 362 876 602 638 031 786 231 269 783 507 006 757 548 228 608  $q^{3273} +$   
 31 732 949 928 372 558 922 963 998 370 468 263 585 181 315 155 762 516 385 837 599 951 301 182 203  
 241 330 388 532 187 717 696 329 788 510 281 775 610 481 955 528 753 618 560 000  $q^{3276} -$   
 33 272 585 559 068 521 575 622 138 979 507 982 529 384 049 110 564 382 524 988 845 483 026 723 127  
 456 832 940 374 878 173 546 186 147 927 599 199 596 517 877 465 686 886 284 672  $q^{3277} +$   
 38 352 713 272 685 775 163 162 219 916 316 537 112 271 344 978 147 652 732 641 192 782 862 348 590  
 430 325 093 237 171 643 912 075 712 771 720 054 393 095 598 263 245 031 014 400  $q^{3280} -$   
 40 212 371 839 712 337 429 183 794 895 561 726 642 411 668 300 994 682 460 517 013 612 934 576 358  
 940 039 993 928 908 325 457 863 918 543 371 024 023 400 107 978 989 617 152 000  $q^{3281} +$   
 46 348 079 515 248 951 052 082 457 829 705 139 964 886 489 794 899 358 440 964 761 166 718 071 285  
 739 276 184 024 695 129 590 367 691 160 302 563 990 644 586 658 262 648 576 000  $q^{3284} -$   
 48 594 022 941 687 937 825 384 214 620 934 797 360 836 857 321 289 714 261 800 337 979 174 682 410  
 015 582 906 192 785 731 593 509 826 794 476 011 137 819 822 355 620 103 983 000  $q^{3285} +$   
 56 003 798 808 349 499 454 779 699 117 735 003 758 358 018 125 427 178 598 418 598 240 294 517 876

342 645 724 943 964 371 740 475 791 128 085 854 866 045 303 219 634 651 819 008  $q^{3288}$  -  
 58 715 955 867 016 676 518 275 845 970 109 620 810 460 125 702 470 090 333 816 472 095 583 486 708  
 395 239 891 595 724 108 177 478 860 955 788 452 583 914 079 468 982 714 368 000  $q^{3289}$  +  
 67 663 337 348 137 079 595 153 388 475 508 398 262 752 476 971 792 669 797 316 576 042 790 755 587  
 753 541 002 439 295 145 900 862 868 135 111 324 324 391 845 706 457 416 349 696  $q^{3292}$  -  
 70 938 111 654 071 774 619 123 960 217 054 670 302 574 495 021 105 728 542 108 707 716 689 391 349  
 657 837 355 167 864 208 171 798 410 422 120 811 766 430 469 410 887 751 274 265  $q^{3293}$  +  
 81 740 938 094 491 811 125 024 688 371 369 089 229 469 441 154 452 449 860 101 530 854 468 846 904  
 994 815 780 279 773 470 634 125 848 625 026 084 556 056 688 022 378 802 176 000  $q^{3296}$  -  
 85 694 590 806 845 657 988 746 421 746 660 739 840 962 775 083 078 422 834 783 281 812 374 329 269  
 818 902 650 163 974 349 814 245 701 820 648 528 284 872 630 902 171 279 360 000  $q^{3297}$  +  
 98 736 149 319 488 088 885 626 329 287 978 411 269 361 222 431 775 614 265 468 058 252 903 023 031  
 534 857 589 180 848 014 775 418 029 039 799 374 922 473 408 149 416 985 804 800  $q^{3300}$  -  
 103 508 873 725 718 733 257 723 099 723 382 340 586 742 746 596 878 714 881 567 461 858 864 877 683  
 106 564 837 261 951 245 105 887 113 028 248 947 205 550 960 404 482 813 328 250  $q^{3301}$  +  
 119 251 324 002 745 111 606 973 199 195 001 737 117 382 030 316 188 962 316 045 371 098 886 839 311  
 908 653 729 311 351 009 795 687 393 503 467 796 166 836 425 458 820 813 952 000  $q^{3304}$  -  
 125 012 152 955 686 481 558 943 871 359 228 262 584 013 355 097 941 082 170 517 909 234 920 684 710  
 872 685 770 843 233 668 645 528 620 327 311 837 463 245 384 763 138 952 396 800  $q^{3305}$  +  
 144 012 695 228 532 937 964 144 328 736 639 738 519 406 493 973 399 658 921 220 673 269 707 262 811  
 012 736 218 131 911 105 492 022 022 298 541 634 192 284 652 113 902 778 576 384  $q^{3308}$  -  
 150 965 411 019 304 687 806 018 223 856 589 828 654 052 071 821 270 001 212 353 412 840 446 365 880  
 076 847 801 709 464 636 217 380 792 938 628 792 221 417 359 135 688 120 931 125  $q^{3309}$  +  
 173 895 755 535 080 383 226 712 091 409 896 922 407 240 837 586 905 163 617 623 341 005 295 851 043  
 537 455 980 215 662 295 813 599 647 329 851 151 140 276 732 026 977 949 401 088  $q^{3312}$  -  
 182 286 006 182 292 109 427 323 438 273 284 331 684 260 078 541 343 298 355 945 654 867 875 743 080  
 496 447 266 893 812 846 763 095 508 453 743 894 327 689 965 109 693 031 841 792  $q^{3313}$  +  
 209 955 815 783 754 403 423 697 522 246 692 880 736 333 859 688 485 044 205 843 731 635 588 599 055  
 271 419 302 995 103 926 548 338 894 888 173 719 795 319 257 766 610 321 152 000  $q^{3316}$  -  
 220 079 683 067 256 078 142 144 947 932 048 182 883 160 917 168 590 361 364 050 575 171 021 056 281  
 617 918 827 010 370 443 959 740 231 590 569 918 731 910 649 840 424 163 568 938  $q^{3317}$  +  
 253 464 796 552 828 844 521 620 891 961 643 463 290 918 604 320 609 449 945 787 460 211 644 870 773  
 712 860 981 151 658 225 212 589 405 276 798 376 251 001 208 891 979 536 614 400  $q^{3320}$  -  
 265 679 110 817 348 111 426 369 244 396 682 576 657 264 751 433 461 482 748 991 738 570 280 416 779  
 762 880 349 338 320 029 073 009 120 790 443 114 236 404 700 598 029 344 768 000  $q^{3321}$  +  
 305 955 518 318 213 727 763 224 350 372 165 479 280 043 553 371 793 798 304 563 084 268 149 060 326  
 266 977 638 804 511 739 312 358 359 702 963 753 971 820 667 798 520 563 456 000  $q^{3324}$  -  
 320 690 274 798 112 336 640 091 955 960 404 095 391 345 350 441 062 606 426 012 458 660 072 742 884  
 895 475 540 599 179 420 897 551 736 781 593 899 459 624 850 821 908 287 752 100  $q^{3325}$  +  
 369 275 012 965 502 216 012 323 691 915 778 854 281 429 347 348 042 326 635 533 494 417 685 536 609  
 753 364 859 158 661 872 247 944 495 183 341 392 810 096 771 368 481 754 972 160  $q^{3328}$  -  
 387 048 316 152 638 888 140 210 954 788 830 725 568 310 191 331 949 352 472 860 116 742 913 582 063  
 885 519 158 384 545 786 798 404 361 278 436 642 887 997 029 143 514 329 088 000  $q^{3329}$  +  
 445 648 687 130 914 144 424 789 457 474 198 601 154 332 302 907 722 763 484 879 272 842 869 424 440  
 650 409 248 453 307 220 948 731 047 496 407 215 317 161 076 921 063 177 895 936  $q^{3332}$  -  
 467 084 735 943 015 541 524 754 678 919 905 796 066 667 353 913 243 235 078 185 367 851 751 783 461  
 297 048 292 889 488 878 681 033 838 666 286 949 852 443 441 594 120 661 250 125  $q^{3333}$  +  
 537 757 537 871 269 450 772 271 454 424 471 208 827 224 445 288 563 447 293 849 451 601 602 867 563  
 812 405 087 699 877 336 762 660 367 604 306 111 002 522 786 349 088 865 536 000  $q^{3336}$  -  
 563 608 267 982 358 928 362 935 679 735 787 535 432 551 820 833 023 266 759 593 972 631 020 250 620  
 466 249 227 770 559 955 189 371 566 700 870 973 569 533 721 455 667 755 810 816  $q^{3337}$  +  
 648 831 065 669 582 661 218 148 264 888 809 814 656 178 119 387 768 233 868 304 172 503 451 842 185  
 748 423 329 967 872 869 152 785 232 525 622 882 079 619 864 533 850 891 033 600  $q^{3340}$  -  
 680 002 189 821 800 678 296 020 155 009 753 029 573 752 101 263 545 687 970 439 720 785 920 937 859  
 472 014 150 902 272 039 071 555 007 086 425 570 394 112 182 107 990 253 241 750  $q^{3341}$  +

782 759 063 738 157 315 763 265 052 166 579 173 181 977 054 078 054 887 198 870 848 785 952 946 610  
 953 124 196 052 075 353 463 392 719 994 146 661 231 136 373 905 997 742 080 000  $q^{3344} -$   
 820 341 400 347 184 368 998 682 703 447 094 791 565 336 476 262 182 706 284 013 772 941 259 093 622  
 925 648 614 712 442 276 699 368 335 167 470 028 070 110 311 612 492 049 612 800  $q^{3345} +$   
 944 226 103 916 522 252 343 261 230 150 577 775 444 176 418 171 960 756 244 184 517 281 144 598 958  
 577 706 278 827 269 215 689 993 236 328 822 485 828 676 481 336 583 791 624 192  $q^{3348} -$   
 989 533 263 827 491 223 987 078 523 259 147 417 117 869 627 006 815 201 097 883 022 679 901 522 877  
 529 903 596 423 741 590 741 351 488 463 432 162 042 995 523 796 217 971 144 625  $q^{3349} +$   
 1 138 873 309 689 453 863 604 311 930 859 477 529 450 000 162 862 161 889 201 710 917 499 822 375 154  
 404 918 958 232 046 064 953 103 532 427 417 415 156 837 951 460 853 475 953 152  $q^{3352} -$   
 1 193 487 026 554 876 630 909 934 042 734 931 630 970 182 751 127 032 932 373 710 818 154 519 990 440  
 597 689 894 718 979 000 835 622 380 654 810 870 875 327 446 524 692 514 275 328  $q^{3353} +$   
 1 373 492 931 776 247 428 086 229 299 530 787 286 271 213 109 548 142 803 114 307 224 229 675 985 902  
 875 693 628 137 741 403 598 232 650 440 392 306 927 256 030 244 777 975 040 000  $q^{3356} -$   
 1 439 317 580 430 855 190 892 190 119 766 179 127 339 638 436 618 403 224 671 416 664 558 239 298 044  
 210 345 941 045 057 195 007 270 770 239 176 027 227 249 977 147 824 665 649 824  $q^{3357} +$   
 1 656 262 352 318 810 063 385 994 661 260 599 612 269 949 786 337 014 583 766 475 970 314 897 674 089  
 008 895 085 317 079 404 394 649 499 277 731 277 549 986 080 205 770 467 328 000  $q^{3360} -$   
 1 735 590 510 376 314 377 169 158 429 470 372 897 788 369 767 512 925 084 290 477 622 747 173 364 276  
 849 194 360 406 558 825 488 881 554 175 240 426 091 568 173 517 399 973 888 000  $q^{3361} +$   
 1 997 025 477 045 061 742 342 661 443 556 443 807 115 513 333 748 728 875 377 781 431 264 166 389 497  
 067 418 323 935 756 595 161 319 079 592 025 979 010 924 096 370 736 209 946 752  $q^{3364} -$   
 2 092 616 758 121 752 653 747 831 725 358 964 757 007 296 426 357 968 334 587 105 658 596 549 579 252  
 219 073 164 463 764 574 482 875 570 857 101 875 555 415 143 276 292 228 928 250  $q^{3365} +$   
 2 407 631 075 422 167 528 046 832 474 307 531 473 933 152 430 835 426 881 756 352 581 140 998 936 672  
 010 992 627 242 097 757 477 313 229 941 750 443 142 616 306 815 384 312 526 336  $q^{3368} -$   
 2 522 806 910 352 528 301 220 955 983 706 550 112 995 323 168 635 197 256 189 363 545 359 229 898 425  
 588 190 529 816 260 436 389 013 330 465 405 577 034 957 581 587 466 186 752 000  $q^{3369} +$   
 2 902 339 550 119 904 938 091 839 191 650 140 673 872 654 595 200 833 216 837 249 808 900 440 211 289  
 120 697 498 950 259 251 742 301 826 652 829 003 805 190 669 097 764 826 258 432  $q^{3372} -$   
 3 041 097 130 198 191 952 532 567 309 198 948 450 438 547 776 553 736 259 203 797 211 955 813 189 501  
 364 026 464 300 367 018 750 102 994 763 043 524 718 942 018 440 348 719 346 059  $q^{3373} +$   
 3 498 311 923 076 107 563 086 298 237 242 095 811 693 171 113 087 792 775 904 513 076 514 591 210 872  
 813 135 890 938 733 682 841 593 646 320 137 072 745 900 716 929 524 204 032 000  $q^{3376} -$   
 3 665 461 164 632 034 740 448 849 540 358 253 362 078 196 599 237 535 649 667 893 578 079 050 319 202  
 439 581 867 684 463 017 900 346 328 830 527 446 609 315 656 833 792 826 966 016  $q^{3377} +$   
 4 216 197 592 815 932 414 017 994 692 671 198 773 096 030 906 615 546 629 567 068 708 486 283 665 371  
 696 501 230 642 163 494 902 987 604 743 846 768 107 626 257 095 709 649 582 080  $q^{3380} -$   
 4 417 525 756 766 054 168 505 600 913 700 697 028 939 769 503 865 768 843 444 077 213 997 590 880 359  
 954 072 150 784 736 821 788 912 424 251 618 200 748 135 987 996 685 492 142 625  $q^{3381} +$   
 5 080 840 738 391 456 336 104 940 999 387 188 119 311 793 259 312 062 991 913 748 297 781 430 176 816  
 399 991 272 222 660 741 328 424 176 420 309 965 909 949 423 027 486 618 880 000  $q^{3384} -$   
 5 323 310 267 515 577 887 248 037 438 625 585 826 678 488 533 876 961 852 932 955 767 521 026 742 404  
 720 749 977 194 480 582 450 523 649 765 433 642 043 006 859 859 854 545 715 200  $q^{3385} +$   
 6 122 129 229 606 637 574 399 195 628 657 685 574 333 109 730 972 196 278 154 895 984 672 666 588 945  
 841 610 167 744 781 783 875 798 701 353 442 571 107 722 763 813 589 423 331 328  $q^{3388} -$   
 6 414 115 480 999 944 065 785 328 476 382 489 087 852 323 554 543 265 698 226 825 433 090 118 769 296  
 752 593 139 149 595 175 631 472 470 045 777 154 845 485 689 952 656 682 645 375  $q^{3389} +$   
 7 376 014 683 178 468 339 773 611 396 584 912 464 131 887 791 297 796 327 744 487 709 650 678 519 198  
 189 346 630 067 449 309 789 239 491 093 884 435 953 993 933 424 408 616 894 464  $q^{3392} -$   
 7 727 591 570 558 095 468 249 349 711 203 724 711 519 603 297 391 024 493 625 941 599 205 201 069 536  
 462 237 551 089 357 014 416 942 863 617 598 116 288 764 044 349 631 444 811 776  $q^{3393} +$   
 8 885 738 038 460 926 770 837 254 667 538 340 635 023 926 375 260 003 321 635 988 620 110 729 630 960  
 834 233 038 552 048 312 641 660 425 754 729 925 753 478 438 646 498 973 696 000  $q^{3396} -$   
 9 309 021 203 015 336 152 969 083 595 815 046 868 567 746 810 452 103 453 781 472 950 789 624 301 008

450 035 806 445 149 700 248 115 152 110 848 915 913 944 782 904 638 773 278 674  $q^{3397} +$   
 10 703 301 904 002 412 930 715 867 647 011 592 833 423 160 580 508 279 224 193 349 357 291 232 577  $q^{3400} -$   
 429 695 899 397 882 989 778 217 067 374 302 067 888 991 185 258 883 670 224 051 200  $q^{3401} +$   
 11 212 860 956 286 100 737 984 476 087 709 367 166 441 643 372 387 191 780 479 045 618 596 675 750  $q^{3404} -$   
 173 559 335 088 920 733 071 799 874 544 400 903 191 090 683 824 041 956 503 552 000  $q^{3405} +$   
 12 891 239 174 768 766 846 387 631 590 100 402 149 463 347 831 297 470 663 633 696 419 486 895 533  $q^{3408} -$   
 716 271 603 380 646 482 870 911 664 593 273 954 703 696 206 684 025 702 702 720 000  $q^{3409} +$   
 13 504 592 857 285 013 431 334 249 120 420 824 335 268 115 145 363 648 271 546 116 600 470 226 900  $q^{3412} -$   
 146 349 523 516 899 013 367 235 543 725 840 169 381 035 157 432 950 838 489 947 700  $q^{3413} +$   
 15 524 737 311 576 320 501 325 510 249 417 499 205 969 284 103 449 958 128 165 056 221 420 548 231  $q^{3416} -$   
 256 623 248 024 315 587 817 359 625 751 778 567 732 271 533 306 621 567 345 164 288  $q^{3417} +$   
 16 262 948 198 247 837 454 212 158 460 195 749 089 252 494 062 897 071 838 876 939 582 070 147 931  $q^{3420} -$   
 386 467 893 625 562 186 388 275 537 137 898 861 740 715 361 837 110 544 711 680 000  $q^{3421} +$   
 18 694 189 535 232 167 748 568 939 931 235 392 525 058 398 584 132 816 583 298 778 521 611 489 437  $q^{3424} -$   
 787 802 224 233 578 109 541 073 481 885 105 666 994 132 103 340 550 873 887 623 168  $q^{3425} +$   
 19 582 578 201 071 888 111 900 793 311 293 505 004 044 074 526 663 071 525 678 500 488 832 680 844  $q^{3428} -$   
 160 616 089 177 751 865 624 131 839 341 177 244 313 055 698 698 192 015 483 610 991  $q^{3432} +$   
 22 508 258 408 631 387 849 602 281 747 160 755 892 273 050 507 017 873 157 324 037 687 389 950 363  $q^{3433} +$   
 138 202 582 926 773 743 595 798 877 432 271 544 980 224 937 398 135 715 112 064 000  $q^{3437} +$   
 23 577 260 979 743 337 460 860 311 006 845 432 351 316 042 493 138 662 003 837 155 694 008 312 959  $q^{3440} -$   
 176 175 766 339 510 888 836 285 397 710 944 415 622 417 009 569 063 406 688 993 280  $q^{3441} +$   
 27 097 554 328 340 971 374 096 876 811 027 258 118 925 835 048 833 282 485 553 589 269 053 602 741  $q^{3442} -$   
 144 945 964 494 257 254 886 085 621 473 179 368 054 405 741 222 252 167 287 654 400  $q^{3445} +$   
 28 383 752 089 612 321 313 912 449 889 292 707 782 958 868 154 131 356 969 496 660 968 551 546 826  $q^{3448} -$   
 976 155 315 633 694 961 378 652 963 226 048 706 062 619 987 333 082 704 575 387 750  $q^{3452} -$   
 32 619 051 883 093 384 559 310 025 052 007 303 814 702 352 433 395 714 355 623 339 122 136 374 080  $q^{3455} +$   
 762 573 025 944 271 266 666 623 667 835 277 947 711 728 920 382 017 631 610 368 000  $q^{3456} -$   
 34 166 407 335 091 606 213 244 603 257 739 582 573 358 673 418 256 815 023 835 317 095 984 662 068  $q^{3459} +$   
 371 197 889 569 227 691 965 627 604 362 105 616 705 388 148 476 823 631 359 180 800  $q^{3462} -$   
 39 261 391 530 731 489 098 303 750 796 721 414 511 065 939 438 911 960 340 572 928 358 379 380 893  $q^{3465} +$   
 127 701 293 375 143 655 379 539 254 295 582 184 188 124 522 453 197 093 567 791 104  $q^{3468} -$   
 41 122 732 135 776 681 386 372 856 954 121 842 550 483 083 754 938 689 345 945 666 804 292 934 470  $q^{3471} +$   
 163 565 611 184 066 308 898 440 644 670 442 286 964 786 986 884 140 639 234 354 875  $q^{3474} -$   
 47 251 243 400 359 382 192 356 010 095 540 413 081 428 935 295 576 830 744 398 595 628 920 353 960  $q^{3477} +$   
 937 611 608 484 144 115 360 068 614 302 711 079 869 323 476 731 721 933 785 227 264  $q^{3480} -$   
 49 490 042 464 823 842 621 947 775 786 673 597 192 191 327 559 489 892 536 436 273 583 560 694 097  $q^{3483} +$   
 530 891 292 116 614 013 312 964 017 475 308 893 013 406 374 342 795 890 969 083 904  $q^{3486} -$   
 56 860 945 203 870 443 646 591 816 060 491 403 146 665 035 174 068 931 394 963 125 025 750 562 621  $q^{3489} +$   
 034 865 054 566 004 500 498 860 334 213 893 781 001 504 344 173 218 016 577 216 000  $q^{3492} -$   
 59 553 459 177 984 100 254 168 245 960 476 368 910 473 541 747 269 405 301 247 895 238 903 887 987  $q^{3495} +$   
 515 555 540 471 550 217 776 769 897 802 470 976 965 866 790 647 433 404 156 062 454  $q^{3498} -$   
 68 417 668 391 067 272 109 962 088 484 980 487 590 725 157 999 566 086 988 940 542 279 379 559 504  $q^{3501} +$   
 275 047 171 945 963 626 377 221 133 869 635 057 316 147 155 027 114 098 768 691 200  $q^{3504} -$   
 71 655 501 650 268 460 645 329 334 216 642 005 317 578 471 948 414 595 342 247 611 587 210 786 348  $q^{3507} +$   
 669 823 962 155 533 365 695 803 851 043 545 889 970 320 180 497 373 656 817 664 000  $q^{3510} -$   
 82 314 417 182 143 975 761 059 946 792 427 230 598 557 607 392 894 142 998 832 788 024 239 313 772  $q^{3513} +$   
 468 488 291 342 399 647 806 908 137 100 709 964 243 464 700 317 066 699 402 240 000  $q^{3516} -$   
 86 207 599 469 942 392 895 785 530 659 941 291 612 191 762 803 115 309 059 658 688 643 702 232 782  $q^{3519} +$   
 503 558 731 313 526 272 850 726 765 139 780 670 952 929 490 184 747 844 106 054 700  $q^{3522} -$   
 99 023 225 608 130 858 112 444 476 407 431 399 858 045 664 295 136 785 927 891 104 126 528 059 535  $q^{3525} +$   
 289 822 371 163 091 619 346 069 722 610 193 577 209 622 285 019 705 704 913 823 744  $q^{3528} -$   
 103 703 904 229 816 013 275 854 497 417 087 594 563 756 863 149 898 558 621 051 502 700 785 998 678  $q^{3531} +$   
 288 158 544 728 714 155 816 860 198 186 832 173 261 043 888 129 810 049 372 160 000  $q^{3534} -$   
 119 110 990 155 732 215 082 313 916 736 214 500 551 921 105 250 771 781 690 268 511 884 662 960 363  $q^{3537} +$   
 367 513 682 013 140 934 026 468 679 834 985 070 740 197 819 341 517 274 597 978 112  $q^{3540} -$

124 737 859 265 799 108 668 671 276 063 061 115 768 147 166 216 298 007 466 767 761 236 082 738 118 \
 343 416 704 120 059 363 183 433 549 192 459 552 252 038 550 050 606 953 675 127 773  $q^{3453} +$  \
 143 258 462 406 969 678 105 721 640 352 665 327 678 145 076 112 098 029 570 400 542 496 465 388 868 \
 034 060 426 825 649 265 013 308 295 307 263 601 904 373 815 268 224 348 930 048 000  $q^{3456} -$  \
 150 022 075 989 748 843 451 059 379 711 547 548 906 136 899 554 923 895 258 308 757 355 011 908 792 \
 939 865 758 154 637 447 809 522 668 443 108 670 595 485 647 363 904 939 295 604 736  $q^{3457} +$  \
 172 283 030 008 588 760 429 889 043 959 662 759 786 681 123 888 436 346 192 279 247 237 049 342 628 \
 406 326 304 110 035 813 157 506 607 324 947 040 875 792 140 120 806 142 282 956 800  $q^{3460} -$  \
 180 412 174 199 504 989 958 737 931 414 638 599 004 614 465 710 134 493 158 304 071 861 534 768 941 \
 386 468 854 525 714 982 992 390 779 380 456 432 489 713 703 390 974 457 559 212 625  $q^{3461} +$  \
 207 166 038 777 600 474 221 092 425 301 486 159 619 473 678 357 284 429 191 979 902 680 715 304 481 \
 563 496 724 535 123 615 413 583 269 549 450 058 390 702 167 339 553 005 977 728 000  $q^{3464} -$  \
 216 935 373 954 621 921 286 532 283 677 396 019 133 130 374 781 769 353 917 251 290 562 010 389 526 \
 239 215 588 029 825 881 696 558 904 318 154 938 729 843 216 195 462 578 610 176 000  $q^{3465} +$  \
 249 085 557 786 106 500 481 278 595 094 857 307 157 808 678 978 905 888 713 832 978 543 508 682 022 \
 094 544 257 147 529 669 851 250 005 490 611 403 518 566 701 267 642 115 434 973 696  $q^{3468} -$  \
 260 824 782 505 017 543 393 872 119 144 059 777 548 909 562 264 328 767 184 229 532 686 165 699 803 \
 042 436 307 362 263 577 927 390 837 950 328 926 543 853 748 272 109 927 454 495 125  $q^{3469} +$  \
 299 455 667 700 766 133 635 212 441 390 990 232 948 790 647 558 955 934 694 216 407 073 810 226 442 \
 481 215 919 067 444 670 679 353 322 380 597 122 643 911 972 363 730 548 580 679 680  $q^{3472} -$  \
 313 560 506 402 600 028 977 941 830 524 320 623 186 954 017 976 909 801 474 136 709 562 332 821 139 \
 723 821 611 556 585 717 786 057 211 525 899 846 965 330 554 842 912 654 901 968 896  $q^{3473} +$  \
 359 973 566 256 131 591 473 466 305 495 607 797 540 251 764 255 376 050 604 560 531 200 675 071 748 \
 655 015 824 770 205 212 788 800 988 059 999 351 629 889 327 163 374 828 007 424 000  $q^{3476} -$  \
 376 918 942 353 224 665 834 408 933 449 419 260 437 583 414 523 158 318 781 277 377 301 327 045 240 \
 899 778 084 051 973 615 467 352 309 976 499 244 386 131 837 780 162 933 881 138 044  $q^{3477} +$  \
 432 676 040 423 636 241 152 854 670 941 221 369 357 746 008 021 558 787 568 512 723 768 239 934 580 \
 037 995 393 650 063 374 600 846 689 837 284 843 646 747 345 440 033 629 318 041 600  $q^{3480} -$  \
 453 031 867 800 723 318 038 530 577 850 904 908 830 404 715 481 790 998 603 312 343 148 172 610 857 \
 446 371 676 437 144 439 055 740 191 918 640 924 988 969 708 556 234 014 289 920 248  $q^{3481} +$  \
 520 007 160 857 657 158 850 342 105 345 935 078 754 747 580 321 104 178 808 658 649 287 549 482 550 \
 327 215 137 087 831 018 488 423 492 685 835 772 145 709 208 285 995 194 649 344 000  $q^{3484} -$  \
 544 457 272 311 779 520 935 748 828 612 785 133 154 343 529 180 917 004 071 711 406 165 894 759 538 \
 765 454 618 622 842 041 104 041 188 636 955 895 167 783 114 894 319 049 525 895 475  $q^{3485} +$  \
 624 899 420 429 946 640 965 789 925 297 362 172 391 781 474 922 131 746 368 161 205 234 817 369 448 \
 757 652 818 218 597 132 519 422 811 460 773 000 350 201 729 318 723 763 661 393 920  $q^{3488} -$  \
 654 264 253 873 890 926 967 103 059 961 296 831 623 005 555 427 573 464 917 544 998 703 752 417 023 \
 269 736 586 777 207 701 112 328 912 637 606 978 305 582 718 447 613 708 849 152 000  $q^{3489} +$  \
 750 870 976 906 325 809 596 717 432 877 583 043 356 469 216 142 206 827 707 926 678 795 696 812 368 \
 219 456 266 451 658 485 337 526 139 981 775 581 702 029 182 990 423 280 881 713 152  $q^{3492} -$  \
 786 134 762 569 451 208 325 266 211 572 007 099 032 319 783 447 188 793 414 431 394 488 423 627 703 \
 823 234 178 395 965 872 621 882 708 282 068 751 593 204 447 362 696 710 718 636 023  $q^{3493} +$  \
 902 142 184 182 292 103 516 166 374 701 190 929 293 106 738 231 632 547 732 042 282 997 780 013 910 \
 559 578 340 098 690 995 715 370 968 797 358 236 094 814 157 090 921 507 053 952 000  $q^{3496} -$  \
 944 485 522 497 704 181 269 120 337 233 496 972 933 068 542 896 525 883 530 050 993 671 483 439 779 \
 069 408 079 800 245 152 530 750 929 478 706 073 100 190 135 693 928 239 760 801 792  $q^{3497} +$  \
 1 083 775 223 837 961 719 143 736 395 597 401 734 919 716 345 493 383 904 949 586 982 481 045 409 178 \
 610 280 931 550 827 123 126 917 409 597 407 139 738 684 655 821 985 302 617 856 000  $q^{3500} -$  \
 1 134 614 118 912 093 297 899 576 786 309 052 173 778 337 433 789 148 265 398 131 479 514 829 619 984 \
 288 682 277 095 059 877 399 200 343 828 274 671 797 716 394 855 223 171 968 091 625  $q^{3501} +$  \
 1 301 841 399 247 218 719 837 578 232 315 531 840 169 399 105 447 508 594 265 071 509 957 917 926 204 \
 574 511 281 581 062 591 549 403 402 245 941 730 230 392 785 395 323 182 532 608 000  $q^{3504} -$  \
 1 362 874 022 390 625 075 480 620 588 485 191 799 846 055 912 717 567 824 749 012 404 648 010 782 518 \
 262 846 511 334 937 401 706 012 205 566 166 914 547 281 784 568 015 869 847 142 400  $q^{3505} +$  \
 1 563 621 552 158 694 426 808 468 522 651 614 394 635 786 332 528 229 524 032 827 709 428 788 723 077 \

707 130 086 047 012 165 446 570 898 153 685 147 254 037 790 043 002 263 623 657 472  $q^{3508}$  -  
 1 636 884 260 634 765 809 094 603 490 516 569 615 534 564 071 070 088 461 051 013 955 971 644 891 484  
 004 713 690 702 407 333 471 474 485 539 278 273 125 980 390 636 217 388 855 746 625  $q^{3509}$  +  
 1 877 846 135 325 696 168 576 262 737 811 146 712 864 397 480 350 719 536 508 194 247 260 161 633 637  
 547 258 729 610 631 420 084 363 295 306 803 525 025 060 943 135 807 895 900 746 752  $q^{3512}$  -  
 1 965 780 571 275 155 933 581 891 291 144 771 819 511 456 316 709 084 016 185 646 685 994 907 855 863  
 474 088 376 013 807 039 288 228 159 349 240 308 293 067 080 084 913 519 972 220 928  $q^{3513}$  +  
 2 254 982 758 768 196 273 081 432 906 310 219 465 492 483 543 604 260 574 548 572 377 585 842 229 832  
 880 547 201 340 001 342 452 534 694 493 592 297 034 805 444 559 167 409 280 768 000  $q^{3516}$  -  
 2 360 516 211 782 333 964 998 925 551 223 141 603 660 147 486 345 316 402 830 591 046 856 145 410 612  
 620 064 843 519 458 793 817 620 785 067 497 506 572 597 490 307 551 040 016 132 013  $q^{3517}$  +  
 2 707 580 562 660 103 755 718 256 948 247 867 536 286 150 614 279 890 299 544 351 384 378 687 203 454  
 049 707 366 541 704 431 681 207 585 913 319 854 721 585 297 970 423 049 941 811 200  $q^{3520}$  -  
 2 834 222 208 160 853 479 337 282 613 876 217 078 820 128 798 576 423 549 434 840 463 241 198 689 211  
 164 105 813 463 866 408 659 333 938 827 346 943 699 727 580 868 363 168 669 696 000  $q^{3521}$  +  
 3 250 682 605 691 322 445 797 389 964 904 054 838 721 743 501 597 683 735 728 160 304 097 496 109 194  
 914 446 703 513 907 752 257 344 849 800 362 230 439 774 030 773 401 685 954 560 000  $q^{3524}$  -  
 3 402 638 743 814 749 405 488 215 946 679 168 011 975 482 908 153 615 376 818 415 124 690 444 322 429  
 701 627 130 668 792 219 190 652 711 813 755 058 752 940 401 720 358 661 869 390 550  $q^{3525}$  +  
 3 902 319 652 630 013 737 485 953 616 923 617 957 231 524 877 377 558 177 358 319 894 376 011 293 669  
 113 355 140 337 598 056 760 387 023 035 753 806 571 308 065 857 235 521 483 762 432  $q^{3528}$  -  
 4 084 631 685 043 108 449 790 959 471 480 278 708 917 358 593 567 749 702 387 013 079 046 757 158 438  
 375 970 405 340 310 144 238 793 724 907 496 294 830 029 171 373 829 811 302 400 000  $q^{3529}$  +  
 4 684 101 368 656 517 220 647 998 187 188 888 626 190 324 815 821 257 998 339 253 432 223 235 038 202  
 691 036 375 941 867 910 820 815 064 529 931 743 933 229 732 697 433 193 880 428 032  $q^{3532}$  -  
 4 902 810 983 179 957 221 869 423 396 682 071 734 464 037 941 761 134 132 070 807 120 893 455 052 539  
 399 594 881 405 418 064 918 002 637 848 424 351 326 107 099 165 789 127 875 963 139  $q^{3533}$  +  
 5 621 924 064 385 716 360 110 026 540 303 534 042 989 818 313 438 157 079 338 071 566 845 566 447 119  
 264 469 536 339 939 037 610 032 020 670 532 987 231 819 358 822 901 177 286 656 000  $q^{3536}$  -  
 5 884 270 972 748 726 039 352 416 474 835 313 656 672 984 081 530 421 116 133 897 122 312 926 624 749  
 666 698 476 550 872 854 758 483 844 382 738 876 398 075 202 476 042 362 764 787 712  $q^{3537}$  +  
 6 746 817 884 073 298 477 962 110 335 283 633 902 220 366 262 139 505 633 863 014 916 901 016 076 247  
 841 705 619 330 579 854 167 532 150 316 639 709 313 228 955 449 215 962 951 065 600  $q^{3540}$  -  
 7 061 476 504 411 054 265 226 902 909 250 491 026 693 491 648 248 133 615 322 309 946 241 652 692 591  
 095 920 004 983 475 986 698 522 659 697 028 732 872 084 806 355 398 480 365 824 750  $q^{3541}$  +  
 8 095 960 809 384 426 480 797 777 425 894 065 527 894 358 707 884 511 770 444 003 893 823 042 901 512  
 206 505 360 950 422 621 952 816 920 697 480 199 567 416 377 412 529 848 714 432 000  $q^{3544}$  -  
 8 473 323 535 415 720 001 740 521 919 612 998 370 700 624 417 777 608 657 487 635 444 072 673 046 391  
 117 166 443 614 811 676 547 047 740 494 259 437 991 033 840 833 867 420 341 043 200  $q^{3545}$  +  
 9 713 892 204 434 325 222 957 117 549 771 178 306 310 353 271 032 440 113 400 162 994 439 307 901 134  
 773 177 475 940 313 924 446 509 741 420 708 955 222 906 311 390 234 873 737 693 184  $q^{3548}$  -  
 10 166 408 397 272 682 167 776 111 707 076 184 189 001 230 867 338 701 939 281 990 203 036 875 308  
 392 322 714 164 271 743 982 728 274 125 044 835 357 131 610 017 932 017 830 096 961 125  $q^{3549}$  +  
 11 653 965 024 259 436 816 886 213 981 454 089 036 833 839 265 289 678 746 749 011 529 830 498 756  
 383 656 447 642 532 843 820 293 109 602 460 306 165 642 081 212 402 180 458 791 280 640  $q^{3552}$  -  
 12 196 546 647 834 552 237 167 805 127 810 475 334 018 686 808 641 582 932 106 746 151 150 481 649  
 152 117 867 671 166 685 285 399 942 793 857 664 605 857 489 175 444 154 088 829 157 376  $q^{3553}$  +  
 13 980 083 450 953 183 246 486 427 932 322 204 056 386 491 373 858 317 412 129 126 035 542 937 907  
 189 392 758 716 782 392 886 160 229 554 083 784 624 947 364 058 207 441 784 954 880 000  $q^{3556}$  -  
 14 630 590 404 526 256 202 182 227 393 488 866 501 530 906 999 257 479 114 260 601 692 541 327 760  
 994 071 321 601 241 190 343 550 702 742 066 548 972 376 310 917 157 795 393 583 021 907  $q^{3557}$  +  
 16 768 781 851 079 926 406 741 244 777 017 689 526 007 382 580 607 102 319 644 374 277 491 066 390  
 792 176 867 661 665 593 630 015 982 646 015 993 431 395 726 610 848 449 178 752 563 200  $q^{3560}$  -  
 17 548 602 599 720 748 059 824 458 684 701 526 278 171 898 241 607 478 321 439 625 503 872 731 699  
 118 327 285 078 200 660 321 393 099 330 012 709 716 025 063 182 884 675 786 911 744 000  $q^{3561}$  +

20 111 711 853 060 804 358 173 886 669 517 231 677 190 445 732 467 821 201 641 754 190 711 792 882 \
 395 452 211 214 906 637 075 474 158 861 284 548 658 170 786 518 093 793 195 062 592 000 q<sup>3564</sup> - \
 21 046 457 999 633 965 967 684 685 410 451 333 133 993 830 583 532 596 767 902 981 114 417 275 922 \
 127 339 462 822 164 635 680 672 143 605 210 487 132 703 779 609 789 415 470 684 754 975 q<sup>3565</sup> + \
 24 118 617 368 118 492 396 892 947 534 207 185 511 111 242 310 533 033 930 662 301 691 591 148 284 \
 272 384 587 935 392 654 884 546 551 267 720 163 079 458 497 920 802 895 572 732 149 760 q<sup>3568</sup> - \
 25 238 954 444 249 080 538 382 082 021 190 694 014 593 384 075 243 040 059 234 848 680 811 157 072 \
 972 040 498 869 394 621 605 294 975 010 869 619 674 573 711 527 194 591 810 998 272 000 q<sup>3569</sup> + \
 28 920 892 933 628 294 271 170 951 309 138 759 572 496 222 371 865 689 347 901 840 909 454 012 702 \
 128 720 581 323 533 644 494 991 499 861 380 630 703 301 197 803 888 281 231 084 875 776 q<sup>3572</sup> - \
 30 263 534 026 751 055 960 346 948 504 917 025 748 559 807 399 987 556 350 540 755 385 509 153 784 \
 854 284 678 659 198 600 413 534 018 442 886 689 461 217 531 738 829 900 770 815 553 231 q<sup>3573</sup> + \
 34 675 839 333 126 330 280 298 785 252 279 020 555 509 766 663 928 918 790 370 396 061 082 192 146 \
 300 452 727 095 569 057 883 212 293 695 435 922 774 483 677 156 967 801 223 920 512 000 q<sup>3576</sup> - \
 36 284 733 348 613 743 777 114 751 320 968 004 510 871 113 716 405 191 262 151 204 384 688 488 549 \
 610 220 666 242 398 671 529 177 825 298 703 680 127 641 349 418 242 884 543 948 357 632 q<sup>3577</sup> + \
 41 571 752 627 001 402 567 760 179 742 542 013 938 548 277 385 344 251 004 591 979 315 343 844 514 \
 001 758 647 764 226 274 822 075 086 618 020 036 165 556 403 898 138 056 225 990 195 200 q<sup>3580</sup> - \
 43 499 505 171 386 243 330 542 793 481 948 284 702 352 332 641 816 763 000 856 931 007 325 467 854 \
 738 663 669 898 971 757 779 256 852 664 703 764 354 298 597 250 024 063 305 060 830 750 q<sup>3581</sup> + \
 49 834 009 208 876 969 150 627 011 512 430 318 387 136 411 444 331 383 145 155 753 773 307 417 396 \
 784 664 893 860 788 584 673 315 526 735 779 787 872 671 488 223 935 147 630 592 000 000 q<sup>3584</sup> - \
 52 143 581 466 584 437 414 352 340 799 166 005 067 956 975 032 908 349 219 593 156 141 336 502 019 \
 491 078 742 971 398 089 643 245 978 169 455 761 127 877 501 272 429 440 647 754 547 200 q<sup>3585</sup> + \
 59 732 341 115 930 404 623 056 551 623 763 736 048 423 117 718 231 285 042 437 727 466 046 809 426 \
 949 790 524 223 346 072 611 057 285 389 458 945 574 546 677 317 397 151 665 020 272 640 q<sup>3588</sup> - \
 62 499 080 909 367 790 789 032 638 474 377 383 308 465 531 184 033 809 551 252 120 132 661 486 720 \
 887 239 111 567 104 000 424 998 628 918 554 096 825 944 161 841 875 337 852 995 931 875 q<sup>3589</sup> + \
 71 589 533 557 940 778 249 247 313 190 034 130 775 113 699 160 133 847 891 111 008 800 550 618 429 \
 212 771 800 858 086 667 670 058 848 267 804 938 618 663 018 519 887 556 883 135 636 480 q<sup>3592</sup> - \
 74 903 603 305 492 412 219 518 227 959 182 090 768 723 805 541 085 138 416 662 752 639 868 860 800 \
 786 767 629 937 662 917 654 863 487 621 038 145 514 323 303 656 726 208 620 830 851 072 q<sup>3593</sup> + \
 85 791 821 671 417 803 574 565 955 797 932 256 982 316 421 863 064 774 540 438 552 434 383 567 425 \
 022 696 388 231 141 487 123 531 125 907 970 149 577 378 242 921 617 329 006 175 104 000 q<sup>3596</sup> - \
 89 761 100 519 219 894 886 982 309 264 639 786 420 707 016 322 534 614 651 716 599 330 040 398 812 \
 401 831 602 940 684 501 650 825 282 437 878 097 277 763 966 609 459 711 553 998 801 357 q<sup>3597</sup> + \
 102 801 317 260 679 509 089 486 648 950 742 555 497 521 839 092 161 922 077 025 582 174 914 384 514 \
 342 409 979 172 865 999 502 321 637 833 021 199 495 071 750 740 077 656 446 660 480 000 q<sup>3600</sup> - \
 107 554 869 654 670 842 395 775 013 661 189 326 448 348 202 016 667 672 746 559 717 070 233 501 330 \
 834 419 577 188 837 107 019 417 480 136 584 750 481 212 811 032 881 394 881 355 776 000 q<sup>3601</sup> + \
 123 170 860 436 903 966 461 982 935 989 682 622 408 003 343 060 044 920 367 385 795 347 523 966 102 \
 570 805 086 754 487 215 382 841 070 943 367 268 924 272 702 649 876 192 935 072 768 000 q<sup>3604</sup> - \
 128 863 081 289 662 919 401 438 225 683 283 308 411 780 866 209 503 972 290 994 642 153 565 955 994 \
 604 846 091 052 009 859 271 404 627 895 412 362 458 566 635 134 472 253 108 845 858 925 q<sup>3605</sup> + \
 147 561 767 611 264 458 472 122 699 315 096 664 088 463 778 228 381 997 870 990 531 244 461 005 801 \
 143 313 331 209 242 927 846 756 172 807 057 225 709 504 755 835 573 237 018 660 754 432 q<sup>3608</sup> - \
 154 377 335 561 517 854 718 556 008 540 534 679 288 493 230 872 213 068 732 752 163 368 932 628 196 \
 855 477 249 262 357 337 268 319 780 266 187 517 263 295 782 235 396 832 814 968 832 000 q<sup>3609</sup> + \
 176 765 038 625 875 397 668 935 687 389 655 326 692 613 969 204 751 545 003 565 013 699 411 948 286 \
 050 075 345 005 174 146 715 058 135 290 580 977 985 014 804 373 159 419 500 675 813 376 q<sup>3612</sup> - \
 184 924 834 352 327 228 574 031 812 040 194 240 616 640 981 867 433 977 210 052 471 415 850 032 450 \
 692 845 554 111 915 219 273 275 193 855 736 500 280 687 040 971 323 007 759 980 937 820 q<sup>3613</sup> + \
 211 726 694 760 859 790 904 846 842 913 480 495 972 280 018 866 818 471 929 485 024 055 175 417 582 \
 798 772 312 669 595 946 878 743 940 256 279 500 753 094 081 627 527 448 442 611 712 000 q<sup>3616</sup> - \
 221 494 871 688 691 504 120 307 706 428 587 435 319 662 665 735 301 918 355 517 086 200 759 047 320 \

706 029 109 197 916 678 164 753 045 888 821 637 728 130 861 766 335 563 398 082 560 000 q<sup>3617</sup> +  
 253 578 049 327 158 879 443 028 720 157 062 169 446 835 377 317 641 021 245 809 729 833 682 413 109 q<sup>3618</sup> -  
 932 320 922 247 221 376 280 573 356 495 949 057 601 065 818 043 590 364 213 920 563 200 q<sup>3620</sup> -  
 265 270 480 299 643 964 657 342 165 270 139 441 975 151 088 470 611 139 600 970 769 275 168 461 993 q<sup>3621</sup> +  
 107 250 714 256 827 481 104 811 501 261 786 184 585 761 437 233 505 370 771 105 311 500 q<sup>3621</sup> +  
 303 671 867 582 000 041 344 628 217 398 597 654 007 105 824 703 635 734 311 234 492 369 318 789 920 q<sup>3624</sup> -  
 332 670 589 955 204 349 664 518 659 091 347 138 266 649 966 671 782 699 694 573 696 000 q<sup>3624</sup> -  
 317 666 234 286 497 157 463 150 306 270 095 660 253 269 289 237 754 526 769 250 691 627 683 867 709 q<sup>3625</sup> +  
 593 736 312 780 624 927 111 429 748 855 164 094 468 633 224 805 198 956 685 836 288 000 q<sup>3625</sup> +  
 363 625 557 599 973 488 732 573 810 928 627 284 734 954 464 143 825 142 654 522 655 151 314 279 962 q<sup>3628</sup> -  
 344 998 934 357 578 998 525 159 655 672 274 836 851 063 397 133 539 965 640 063 550 976 q<sup>3628</sup> -  
 380 373 401 077 877 078 641 835 668 281 369 519 787 058 527 037 218 872 029 776 725 075 774 330 331 q<sup>3629</sup> +  
 410 963 035 487 736 617 993 037 672 440 215 885 144 778 317 984 118 678 684 468 447 750 q<sup>3629</sup> +  
 435 372 754 231 270 853 756 839 454 279 510 133 060 242 365 453 840 711 133 924 185 973 039 884 219 q<sup>3632</sup> -  
 073 193 412 724 947 876 243 898 575 507 110 434 830 975 552 127 778 072 414 264 176 640 q<sup>3632</sup> -  
 455 413 866 262 575 541 839 795 489 866 593 135 766 261 936 281 024 671 284 414 982 812 911 155 712 q<sup>3633</sup> +  
 672 885 627 684 654 856 438 612 077 556 903 249 150 568 959 114 627 339 851 766 104 064 q<sup>3633</sup> +  
 521 224 921 210 352 226 656 617 168 187 864 429 524 955 877 475 792 191 673 795 652 879 519 990 925 q<sup>3636</sup> -  
 098 113 212 279 805 774 232 648 169 036 532 359 499 410 470 819 346 057 885 409 536 000 q<sup>3636</sup> -  
 545 204 529 647 998 842 439 838 920 079 979 794 768 058 000 907 757 153 823 431 062 771 573 605 553 q<sup>3637</sup> +  
 044 216 067 863 479 662 802 061 698 047 668 642 301 569 169 090 647 128 156 525 627 349 q<sup>3637</sup> +  
 623 944 909 979 397 539 232 539 484 643 604 934 178 451 676 943 040 865 346 490 024 847 704 242 824 q<sup>3640</sup> -  
 120 363 364 610 594 885 816 304 270 071 968 420 938 933 093 756 296 672 811 978 854 400 q<sup>3640</sup> -  
 652 634 198 482 769 996 937 858 172 228 135 260 958 733 631 415 961 995 522 030 890 075 020 529 528 q<sup>3641</sup> +  
 064 897 521 761 810 168 157 248 293 686 400 527 110 850 258 107 805 330 548 011 008 000 q<sup>3641</sup> +  
 746 834 787 552 046 897 762 256 444 904 899 572 015 436 485 856 972 398 762 289 037 262 190 277 121 q<sup>3644</sup> -  
 152 785 057 552 962 354 642 596 836 614 526 613 736 428 577 460 404 558 285 409 280 000 q<sup>3644</sup> -  
 781 155 394 331 946 185 796 584 746 907 661 286 694 504 762 170 234 014 637 984 582 271 221 523 166 q<sup>3645</sup> +  
 912 028 425 322 594 433 571 254 393 914 866 633 251 804 880 137 989 274 326 599 756 405 q<sup>3645</sup> +  
 893 840 691 305 137 903 752 041 325 789 296 094 748 739 429 998 909 239 162 192 917 049 430 488 899 q<sup>3648</sup> -  
 810 195 355 323 582 656 224 076 114 225 721 031 989 758 920 105 753 076 337 237 557 248 q<sup>3648</sup> -  
 934 893 955 658 507 010 493 272 385 737 194 854 897 672 164 102 413 011 248 310 739 935 820 139 984 q<sup>3649</sup> +  
 114 397 181 064 902 934 416 198 743 470 138 870 395 962 095 743 231 444 838 948 864 000 q<sup>3649</sup> +  
 1 069 677 999 692 727 897 028 623 008 841 858 602 559 997 201 834 960 866 643 710 104 762 398 230 054 q<sup>3652</sup> -  
 861 280 902 994 107 672 711 370 828 749 108 857 763 654 235 070 309 389 736 253 898 752 q<sup>3652</sup> -  
 1 118 779 873 101 717 895 272 401 035 440 490 561 584 704 486 236 616 829 132 788 741 300 355 548 627 q<sup>3653</sup> +  
 697 582 943 572 678 009 995 643 143 410 418 064 946 065 264 807 676 401 915 725 760 390 q<sup>3653</sup> +  
 1 279 980 740 892 035 348 430 321 056 716 658 080 074 872 955 871 181 421 678 703 162 280 322 448 308 q<sup>3656</sup> -  
 456 687 244 854 711 802 832 184 926 995 548 710 305 301 287 650 569 910 471 295 104 000 q<sup>3656</sup> -  
 1 338 703 455 845 749 254 386 232 538 882 836 190 911 779 663 693 586 063 202 936 760 172 699 267 536 q<sup>3657</sup> +  
 651 874 711 007 512 277 835 161 824 848 402 100 493 307 693 964 079 618 403 432 202 240 q<sup>3657</sup> +  
 1 531 479 915 798 577 476 163 471 921 261 049 188 657 276 343 368 059 223 847 401 258 374 852 089 396 q<sup>3660</sup> -  
 420 183 151 852 541 713 580 404 223 480 575 371 650 766 125 316 964 699 495 037 440 000 q<sup>3660</sup> -  
 1 601 701 715 692 359 029 052 699 711 524 191 392 797 246 106 330 958 108 811 318 460 478 183 215 070 q<sup>3661</sup> +  
 116 266 877 042 041 332 516 287 334 322 258 712 736 398 803 990 115 418 139 946 807 750 q<sup>3661</sup> +  
 1 832 216 310 782 767 965 581 744 079 963 367 614 084 667 249 971 277 122 675 674 453 552 387 047 037 q<sup>3664</sup> -  
 129 253 136 267 605 135 576 845 286 109 423 845 299 816 398 460 132 201 052 420 096 000 q<sup>3664</sup> -  
 1 916 180 794 717 709 532 623 747 992 345 064 479 588 024 918 438 172 422 641 923 706 263 148 808 033 q<sup>3665</sup> +  
 199 681 412 535 249 229 934 160 231 182 513 615 247 253 773 192 390 033 309 905 715 200 q<sup>3665</sup> +  
 2 191 794 446 813 607 407 188 798 404 942 973 982 334 186 885 626 642 866 404 203 076 430 113 682 746 q<sup>3668</sup> -  
 959 090 189 956 376 157 203 737 345 117 150 913 820 086 235 487 840 164 599 674 982 400 q<sup>3668</sup> -  
 2 292 181 381 545 693 683 419 656 685 273 375 225 545 390 694 643 496 913 269 922 534 712 030 817 354 q<sup>3669</sup> +  
 504 211 724 488 158 858 680 665 406 570 508 980 894 153 488 637 634 815 684 804 108 625 q<sup>3669</sup> +  
 2 621 685 587 811 583 527 141 074 909 479 352 928 833 679 433 435 429 790 801 440 330 279 341 648 559 q<sup>3672</sup> -  
 692 584 697 829 603 815 203 342 917 276 971 386 389 774 285 637 193 556 096 703 582 208 q<sup>3672</sup> -

2 741 695 394 635 479 569 176 642 160 859 509 488 256 920 956 714 640 103 334 350 743 074 719 039 976 \
 006 004 863 583 398 057 299 407 884 606 416 672 600 090 525 472 567 140 892 801 073 152 q<sup>3673</sup> +  
 3 135 589 251 526 971 686 312 303 604 750 906 129 803 020 067 317 462 196 678 931 427 821 922 482 014 \
 148 204 804 003 723 021 385 937 992 519 749 371 409 569 800 078 212 047 465 792 256 000 q<sup>3676</sup> -  
 3 279 043 799 413 204 526 186 592 997 358 742 937 466 695 987 170 977 717 034 258 783 074 966 267 169 \
 230 850 406 239 727 473 514 072 582 007 549 307 763 149 222 348 784 909 911 872 671 533 q<sup>3677</sup> +  
 3 749 864 477 399 803 495 381 822 998 814 509 036 356 089 605 559 450 085 850 327 838 939 392 121 285 \
 265 895 317 041 433 101 929 170 661 616 456 164 114 304 802 522 574 354 206 558 822 400 q<sup>3680</sup> -  
 3 921 327 318 194 124 616 596 006 832 851 559 754 999 636 341 043 104 286 314 523 801 327 986 851 320 \
 107 051 571 943 318 784 668 785 501 944 258 622 848 584 987 549 946 935 677 091 840 000 q<sup>3681</sup> +  
 4 484 044 263 133 987 187 161 099 669 079 548 819 081 502 689 444 040 803 321 101 424 678 949 683 479 \
 063 051 192 446 895 627 807 987 367 937 693 831 480 395 839 648 846 966 136 842 240 000 q<sup>3684</sup> -  
 4 688 964 045 492 680 077 884 048 308 717 410 266 697 992 361 988 026 550 261 676 729 625 164 075 575 \
 830 840 238 648 618 003 333 472 702 600 446 452 761 437 631 664 147 199 818 852 423 425 q<sup>3685</sup> +  
 5 361 449 151 015 683 107 740 569 555 415 672 933 847 493 271 339 089 323 320 721 220 176 506 212 170 \
 308 707 799 808 350 679 538 326 871 310 780 679 815 589 536 378 711 108 810 590 467 584 q<sup>3688</sup> -  
 5 606 330 665 335 148 237 920 275 715 486 436 706 340 660 750 817 915 596 637 471 039 574 407 939 969 \
 004 019 954 806 678 542 682 838 914 107 012 546 460 534 297 545 505 624 961 466 368 000 q<sup>3689</sup> +  
 6 409 919 004 734 445 941 353 905 613 319 162 719 031 537 076 227 540 038 355 860 507 352 402 294 505 \
 469 007 832 135 645 125 778 953 504 830 124 060 857 927 208 250 082 126 958 608 315 392 q<sup>3692</sup> -  
 6 702 527 163 461 493 488 862 195 570 600 701 163 811 284 067 335 493 175 498 876 334 267 498 794 506 \
 077 422 879 183 383 443 856 570 859 294 773 903 834 418 624 673 303 642 777 077 401 230 q<sup>3693</sup> +  
 7 662 685 660 902 208 730 808 625 603 465 217 502 995 936 000 151 903 898 364 588 331 731 686 965 802 \
 374 121 050 077 403 730 887 137 817 466 734 573 709 191 173 285 466 388 422 979 584 000 q<sup>3696</sup> -  
 8 012 288 733 243 860 219 155 444 861 981 513 627 619 333 863 689 707 792 154 099 748 525 319 413 772 \
 051 548 005 237 261 225 718 991 529 342 660 610 078 209 076 460 019 139 396 648 599 552 q<sup>3697</sup> +  
 9 159 413 477 564 389 954 692 431 337 306 317 507 851 582 804 436 938 421 326 683 936 332 660 064 276 \
 708 420 107 270 119 910 855 455 384 850 062 927 221 028 594 249 257 002 157 312 768 000 q<sup>3700</sup> -  
 9 577 073 105 631 511 256 511 700 557 705 440 866 331 566 187 085 437 793 791 475 957 423 653 227 489 \
 502 814 944 271 364 591 214 013 730 600 308 046 348 691 260 201 764 261 604 955 354 625 q<sup>3701</sup> +  
 10 947 439 966 728 851 850 491 003 013 608 749 381 604 554 377 744 718 542 167 352 276 735 224 320 \
 669 568 373 106 075 412 246 551 967 093 431 106 488 956 446 406 800 072 402 005 536 000 000 q<sup>3704</sup> -  
 11 446 356 928 271 996 873 927 799 141 795 060 610 466 713 678 538 146 941 860 802 904 876 498 611 \
 079 519 797 957 946 323 111 690 122 472 144 789 862 337 077 193 469 387 486 935 311 974 400 q<sup>3705</sup> +  
 13 083 254 846 252 879 312 288 826 826 777 035 673 901 327 129 544 090 042 213 105 591 025 963 383 \
 222 994 238 664 273 118 028 545 779 401 776 318 657 339 973 300 164 984 530 809 360 541 696 q<sup>3708</sup> -  
 13 679 181 241 056 198 004 424 747 652 444 522 831 545 010 313 768 150 825 895 344 918 337 773 259 \
 687 179 638 421 724 528 787 128 890 463 846 365 929 389 385 491 485 585 409 614 654 618 875 q<sup>3709</sup> +  
 15 634 263 164 969 541 366 041 395 443 727 770 395 852 973 728 302 527 244 639 080 007 011 945 659 \
 076 154 260 086 078 853 281 029 457 115 739 274 906 416 135 403 767 947 522 132 748 369 920 q<sup>3712</sup> -  
 16 345 993 739 594 207 330 001 390 687 752 472 869 492 955 194 563 561 011 369 061 680 426 492 569 \
 305 557 785 191 500 841 958 467 560 130 487 535 672 704 774 291 376 236 299 566 680 899 584 q<sup>3713</sup> +  
 18 680 886 865 636 898 129 463 409 005 106 006 020 526 239 904 639 555 212 791 488 782 103 392 092 \
 538 160 186 132 047 927 702 004 201 422 633 259 858 180 244 427 490 099 310 558 201 856 000 q<sup>3716</sup> -  
 19 530 844 616 300 288 331 714 933 459 938 569 988 936 905 894 044 169 355 184 252 073 198 190 401 \
 419 659 355 715 250 928 252 890 722 953 771 555 336 211 694 372 137 092 642 356 905 043 337 q<sup>3717</sup> +  
 22 319 069 517 029 858 730 906 416 361 122 124 081 769 460 256 577 948 523 752 417 579 009 462 742 \
 960 490 812 839 037 953 687 019 267 040 676 543 454 297 434 773 859 835 459 036 065 536 000 q<sup>3720</sup> -  
 23 334 003 596 386 831 769 778 804 401 252 036 198 642 864 637 255 023 179 744 236 444 356 918 876 \
 635 232 405 586 801 977 269 567 535 044 543 280 447 605 813 017 959 899 644 684 288 000 248 q<sup>3721</sup> +  
 26 663 261 282 974 528 397 342 674 368 728 350 567 394 699 933 185 987 818 726 648 342 878 522 000 \
 615 555 507 804 570 367 606 132 048 275 798 627 552 683 312 726 162 267 189 983 282 624 000 q<sup>3724</sup> -  
 27 875 078 670 709 594 535 902 650 171 547 502 550 759 266 540 092 655 835 353 867 779 391 479 352 \
 479 410 407 539 359 221 744 420 241 022 534 425 921 828 089 702 865 645 526 513 285 272 000 q<sup>3725</sup> +  
 31 849 975 875 272 745 900 758 028 551 846 215 400 698 135 912 853 495 699 572 931 167 596 613 022 \

281 090 723 773 992 783 767 478 726 844 586 526 724 026 275 208 042 570 798 292 723 695 616 q<sup>3728</sup> -  
 33 296 732 358 462 076 685 849 181 981 234 069 022 512 166 694 347 946 023 727 287 542 103 266 158 \\  
 771 344 686 653 704 737 826 717 558 072 748 351 457 433 972 721 873 746 158 959 861 760 000 q<sup>3729</sup> +  
 38 042 028 702 556 246 880 377 738 899 718 326 089 705 681 846 994 456 099 243 297 207 989 965 172 \\  
 405 392 566 609 161 960 129 481 488 327 267 557 327 061 493 428 433 329 048 087 386 554 368 q<sup>3732</sup> -  
 39 769 109 573 026 421 308 831 003 731 323 840 381 857 600 683 678 687 817 425 735 188 900 331 015 \\  
 209 974 744 461 820 824 286 190 710 472 640 253 689 979 953 109 894 013 613 351 475 332 957 q<sup>3733</sup> +  
 45 433 586 204 997 873 460 465 329 760 948 252 052 290 304 221 076 112 719 645 063 023 250 712 547 \\  
 945 755 139 563 925 322 263 535 749 945 444 028 755 730 044 071 260 547 317 407 750 848 000 q<sup>3736</sup> -  
 47 495 112 863 945 216 310 052 708 105 010 383 480 871 096 073 662 316 425 751 235 713 376 531 878 \\  
 559 239 539 249 162 776 480 721 594 879 197 367 091 788 638 557 948 354 076 892 651 716 608 q<sup>3737</sup> +  
 54 256 181 081 621 640 654 252 879 618 030 780 177 235 811 297 124 098 579 277 792 467 654 239 401 \\  
 949 833 192 153 047 935 671 853 304 109 524 758 943 448 726 311 343 620 947 285 187 788 800 q<sup>3740</sup> -  
 56 716 686 620 719 110 470 048 377 907 395 206 717 215 520 066 214 163 146 217 272 195 844 493 737 \\  
 655 512 407 469 670 381 587 820 834 299 798 259 177 307 079 940 754 921 635 240 611 737 125 q<sup>3741</sup> +  
 64 785 877 516 742 932 588 971 471 151 295 822 771 574 053 304 757 134 164 747 309 688 066 077 308 \\  
 663 223 716 496 880 358 965 877 707 390 134 218 749 170 563 235 110 034 419 327 787 520 000 q<sup>3744</sup> -  
 67 722 302 526 795 410 042 081 047 601 075 265 319 450 294 775 468 907 093 290 937 365 534 647 434 \\  
 173 803 273 219 143 207 659 835 394 813 841 518 458 696 431 074 114 453 924 834 605 465 600 q<sup>3745</sup> +  
 77 351 805 478 930 128 963 533 234 127 162 988 865 214 709 236 517 715 344 904 481 760 115 195 942 \\  
 468 989 353 719 476 958 221 041 348 804 666 548 297 065 272 222 191 465 351 448 519 917 568 q<sup>3748</sup> -  
 80 855 875 067 726 513 143 337 829 400 039 091 199 991 032 444 992 811 525 363 108 017 484 627 041 \\  
 554 275 576 397 982 998 855 367 912 011 079 679 281 261 121 353 487 524 993 881 356 264 750 q<sup>3749</sup> +  
 92 346 324 750 217 941 070 217 863 178 377 704 238 469 883 703 111 364 004 777 904 887 609 124 900 \\  
 764 768 024 356 988 558 276 219 371 887 134 439 532 931 551 850 090 991 809 276 977 700 864 q<sup>3752</sup> -  
 96 527 379 322 691 210 042 551 684 769 483 517 326 691 450 147 538 228 233 633 229 797 476 229 192 \\  
 912 347 087 545 943 854 406 318 488 395 058 026 693 842 810 680 887 646 720 508 950 609 920 q<sup>3753</sup> +  
 110 237 128 793 016 737 452 155 756 785 444 629 047 255 909 126 026 784 858 139 631 829 207 613 464 \\  
 124 999 240 082 177 880 010 883 406 957 376 842 954 392 862 137 731 671 156 031 895 040 000 q<sup>3756</sup> -  
 115 225 494 906 185 556 132 624 304 728 986 075 329 128 800 819 512 891 713 978 432 350 230 537 334 \\  
 655 405 601 032 695 987 483 735 604 284 213 448 323 985 679 186 319 190 087 898 889 679 675 q<sup>3757</sup> +  
 131 581 657 359 632 525 901 997 541 655 562 586 752 319 161 898 422 041 725 947 701 935 812 523 200 \\  
 557 165 279 477 281 674 473 291 280 841 403 486 385 138 541 749 817 434 331 988 183 244 800 q<sup>3760</sup> -  
 137 532 661 324 269 597 037 584 308 803 526 935 067 826 254 076 449 603 383 553 081 143 953 170 271 \\  
 172 447 399 676 974 585 964 518 614 638 146 870 040 073 709 852 476 527 989 151 809 536 000 q<sup>3761</sup> +  
 157 044 256 655 309 840 243 610 439 134 865 263 347 177 543 608 905 328 352 543 949 540 602 500 787 \\  
 625 596 094 153 624 896 916 854 704 369 027 187 649 497 994 859 693 791 182 409 100 032 000 q<sup>3764</sup> -  
 164 143 003 005 458 339 109 051 797 776 660 079 385 179 947 578 944 457 581 474 618 876 426 771 624 \\  
 723 697 389 227 093 447 524 834 926 359 656 069 091 499 845 363 377 645 002 003 438 673 375 q<sup>3765</sup> +  
 187 416 608 971 490 205 566 522 939 914 137 148 187 314 710 300 136 103 458 352 844 130 447 016 173 \\  
 636 272 162 045 781 174 032 987 351 033 748 657 046 632 519 751 617 343 242 591 227 292 672 q<sup>3768</sup> -  
 195 883 669 043 287 857 142 083 734 905 038 957 470 053 714 158 020 561 304 725 986 757 971 664 330 \\  
 547 737 346 555 055 185 587 500 906 012 535 212 294 911 680 860 861 831 890 902 876 160 000 q<sup>3769</sup> +  
 223 642 052 495 092 072 523 674 072 443 712 973 122 743 828 335 952 772 376 022 326 475 211 200 790 \\  
 539 863 849 295 832 913 929 969 112 491 053 038 237 822 290 453 553 295 568 146 410 594 304 q<sup>3772</sup> -  
 233 740 235 838 357 255 789 564 197 915 352 058 774 414 023 723 833 562 072 963 405 267 968 656 751 \\  
 259 712 891 171 307 306 395 423 404 278 084 942 051 508 427 123 419 788 820 659 005 501 614 q<sup>3773</sup> +  
 266 844 529 421 236 821 559 583 252 106 446 957 227 890 137 224 490 271 332 442 595 771 133 118 210 \\  
 053 716 310 827 311 856 938 603 005 367 676 037 179 977 124 415 293 950 284 009 533 440 000 q<sup>3776</sup> -  
 278 886 943 430 828 499 502 117 585 814 719 713 852 919 844 192 754 122 489 315 914 003 419 502 420 \\  
 232 584 491 101 928 668 693 137 952 038 662 657 290 007 480 964 396 406 839 769 870 860 288 q<sup>3777</sup> +  
 318 363 040 052 751 645 761 658 874 722 118 888 505 586 168 181 180 691 261 317 635 563 008 458 775 \\  
 998 798 398 686 698 247 072 611 596 990 771 890 415 469 285 139 576 097 152 264 342 732 800 q<sup>3780</sup> -  
 332 722 682 025 320 437 590 594 714 227 321 758 872 144 276 730 950 435 882 102 334 161 842 355 740 \\  
 242 690 549 419 168 824 911 689 968 141 360 615 478 406 838 036 321 247 201 215 915 415 000 q<sup>3781</sup> +

379 792 646 417 544 710 378 487 823 381 401 184 447 314 919 812 469 796 414 204 618 616 698 640 688 \\  
 025 959 990 398 952 013 564 494 369 017 899 173 774 184 718 913 538 511 901 134 585 600 000 q<sup>3784</sup> - \\  
 396 913 818 368 676 678 847 749 753 521 960 043 459 762 014 204 649 580 092 034 748 350 753 821 363 \\  
 117 761 117 740 897 886 520 193 512 512 158 459 637 763 547 408 990 640 844 476 173 516 800 q<sup>3785</sup> + \\  
 453 033 266 010 307 074 565 057 077 082 984 141 334 880 230 981 891 332 187 989 764 310 905 093 402 \\  
 757 464 186 267 657 400 331 017 075 183 641 635 837 733 566 113 498 801 790 644 729 459 200 q<sup>3788</sup> - \\  
 473 445 157 399 197 612 640 866 818 543 336 187 728 548 277 818 210 899 231 474 011 784 733 040 263 \\  
 528 341 334 789 276 420 811 801 764 319 380 997 968 868 046 500 194 713 774 127 437 230 625 q<sup>3789</sup> + \\  
 540 347 730 426 982 886 346 136 750 793 845 802 293 770 112 087 985 168 737 784 412 035 569 970 913 \\  
 344 950 169 483 863 080 880 264 276 448 178 594 128 152 777 339 757 218 999 155 183 353 856 q<sup>3792</sup> - \\  
 564 680 579 059 197 083 829 721 199 549 501 966 070 427 757 209 728 013 278 395 873 148 456 665 456 \\  
 004 840 139 824 746 543 763 271 798 258 091 725 254 644 654 807 303 579 771 857 252 024 320 q<sup>3793</sup> + \\  
 644 430 861 863 499 353 819 592 067 748 690 982 487 461 307 290 831 381 411 712 901 311 321 965 372 \\  
 565 399 521 970 630 411 507 756 537 389 163 123 989 751 047 180 869 391 701 673 991 680 000 q<sup>3796</sup> - \\  
 673 435 180 609 974 614 241 572 137 881 258 377 930 676 943 025 141 261 504 470 720 622 364 559 374 \\  
 497 995 580 926 122 970 007 527 494 762 265 175 594 764 664 260 309 435 859 134 827 453 492 q<sup>3797</sup> + \\  
 768 491 650 948 268 959 525 777 881 817 024 103 286 723 106 703 729 618 498 934 479 616 296 199 657 \\  
 584 822 257 369 599 893 136 456 651 081 065 609 549 548 261 639 691 022 671 248 687 142 400 q<sup>3800</sup> - \\  
 803 061 099 824 441 725 902 283 430 128 315 280 556 378 438 095 757 751 445 770 890 899 197 237 849 \\  
 234 101 631 396 836 491 950 062 051 771 323 359 442 586 581 607 803 435 168 735 305 728 000 q<sup>3801</sup> + \\  
 916 351 011 966 304 500 698 039 537 753 336 143 415 824 082 195 199 224 932 750 301 050 206 863 119 \\  
 315 106 219 309 564 811 213 691 060 582 790 295 405 539 515 155 683 525 389 165 761 792 000 q<sup>3804</sup> - \\  
 957 549 604 281 293 824 966 333 553 157 101 904 931 866 084 707 394 529 131 904 882 317 508 729 958 \\  
 108 151 568 743 577 678 788 974 967 154 085 061 645 308 632 659 402 826 268 489 800 389 375 q<sup>3805</sup> + \\  
 1 092 558 057 835 034 093 660 112 904 757 141 206 878 062 807 534 553 330 079 623 422 155 430 904 182 \\  
 018 412 132 697 423 846 205 309 956 070 960 783 804 644 884 550 596 257 966 880 735 608 832 q<sup>3808</sup> - \\  
 1 141 652 518 777 307 407 753 198 073 494 909 521 166 975 190 926 197 804 922 377 512 061 227 359 833 \\  
 607 251 647 977 753 699 665 987 949 459 746 789 420 420 515 637 152 788 058 138 394 624 000 q<sup>3809</sup> + \\  
 1 302 528 390 999 993 051 087 103 996 778 071 263 502 026 020 781 340 267 468 940 085 099 647 915 928 \\  
 157 143 953 185 814 409 935 569 717 763 355 781 442 821 232 661 873 714 018 770 858 606 592 q<sup>3812</sup> - \\  
 1 361 026 641 005 344 857 321 801 903 174 267 881 286 279 388 157 182 755 468 879 488 294 641 751 281 \\  
 960 915 015 512 811 343 011 664 504 672 138 738 317 681 391 700 536 577 468 037 147 300 936 q<sup>3813</sup> + \\  
 1 552 708 564 095 799 391 352 437 777 630 195 965 006 252 976 663 196 277 998 055 746 682 671 903 555 \\  
 832 984 215 932 045 242 451 963 140 565 336 807 246 979 418 044 087 496 771 946 794 560 000 q<sup>3816</sup> - \\  
 1 622 405 482 192 547 887 985 594 117 563 086 518 306 400 454 920 391 013 048 513 226 246 004 696 520 \\  
 819 367 680 708 508 479 246 817 499 056 528 820 598 392 864 005 368 929 045 003 110 481 920 q<sup>3817</sup> + \\  
 1 850 771 645 176 576 003 654 782 948 254 309 145 358 041 822 839 161 081 320 029 912 620 671 134 368 \\  
 952 446 245 157 513 537 838 045 601 537 185 347 007 434 057 419 923 792 381 600 500 992 000 q<sup>3820</sup> - \\  
 1 933 803 484 615 324 587 815 564 352 712 187 667 929 425 183 147 984 843 844 486 302 494 490 205 047 \\  
 478 410 006 841 613 581 924 745 037 707 005 551 236 273 483 165 422 948 602 351 778 498 250 q<sup>3821</sup> + \\  
 2 205 849 749 587 897 518 395 398 995 779 737 147 001 905 175 226 774 261 190 263 036 953 563 753 958 \\  
 650 912 973 316 385 860 510 336 091 346 296 535 854 457 661 786 834 152 535 584 944 128 000 q<sup>3824</sup> - \\  
 2 304 758 835 836 866 513 984 507 673 892 297 704 134 448 734 901 571 323 832 851 159 539 566 875 198 \\  
 874 943 383 662 783 538 858 908 914 687 682 321 997 705 072 890 667 421 013 137 104 076 800 q<sup>3825</sup> + \\  
 2 628 810 501 443 202 793 061 659 215 338 562 995 102 146 277 296 803 631 605 486 462 167 094 465 297 \\  
 675 096 289 024 817 820 005 779 457 606 418 738 540 682 036 705 396 076 770 501 125 931 008 q<sup>3828</sup> - \\  
 2 746 622 148 653 296 187 403 989 591 706 783 045 594 394 666 733 749 764 492 309 660 510 288 458 871 \\  
 534 320 197 003 840 555 278 054 601 779 221 068 599 199 026 363 699 034 359 108 013 297 875 q<sup>3829</sup> + \\  
 3 132 585 694 576 349 465 639 367 642 246 768 444 147 086 764 664 116 783 829 151 147 112 592 921 698 \\  
 817 500 570 763 776 608 682 490 808 522 636 456 584 889 122 147 698 583 140 114 136 641 536 q<sup>3832</sup> - \\  
 3 272 899 639 892 225 033 218 381 114 092 701 539 955 986 370 685 159 338 313 852 429 643 688 689 099 \\  
 445 520 337 673 657 900 305 041 481 480 900 679 248 456 777 980 110 496 425 411 121 217 536 q<sup>3833</sup> + \\  
 3 732 561 974 186 565 969 360 003 612 694 003 842 777 757 387 954 913 986 570 783 419 835 460 397 719 \\  
 117 216 866 045 340 945 258 403 764 354 089 955 533 820 617 105 391 728 499 556 507 648 000 q<sup>3836</sup> - \\  
 3 899 661 060 473 130 652 854 335 201 563 232 258 311 539 322 066 260 609 740 152 236 417 288 023 102 \

455 440 148 475 414 300 676 767 366 877 320 625 089 207 488 739 488 869 708 405 571 776 510  $q^{3837} +$   
 4 447 045 201 729 397 452 664 560 033 494 922 642 039 082 427 520 161 760 758 959 487 750 992 851 593  $\setminus$   
 966 044 762 485 282 021 354 689 640 204 462 712 247 395 681 630 500 558 155 082 235 904 000  $q^{3840} -$   
 4 646 024 551 051 915 150 393 537 435 079 149 205 254 500 916 581 603 411 824 409 258 173 215 704 614  $\setminus$   
 057 323 921 342 492 205 250 834 621 300 563 958 743 610 391 998 356 947 801 872 285 696 000  $q^{3841} +$   
 5 297 812 350 955 133 444 713 457 032 188 497 692 978 020 245 811 622 460 587 415 174 650 680 934 447  $\setminus$   
 937 134 886 992 633 072 175 942 580 710 907 108 752 793 571 804 473 827 576 344 166 426 752  $q^{3844} -$   
 5 534 732 878 499 496 378 669 058 655 803 880 543 123 193 953 565 525 652 525 723 094 681 989 704 608  $\setminus$   
 740 404 976 062 053 266 171 525 388 086 724 137 977 304 296 608 275 165 176 659 293 031 925  $q^{3845} +$   
 6 310 767 376 399 147 727 191 205 056 882 339 452 315 365 679 252 889 929 275 935 495 538 447 559 469  $\setminus$   
 419 178 874 975 435 914 011 504 408 260 560 495 628 300 307 794 227 766 695 554 190 691 328  $q^{3848} -$   
 6 592 838 215 234 896 920 785 086 603 402 798 823 268 563 336 517 929 073 734 071 272 357 805 600 756  $\setminus$   
 528 040 101 195 933 429 496 068 870 807 023 507 123 295 134 111 107 999 036 027 531 264 000  $q^{3849} +$   
 7 516 720 573 012 403 611 214 386 004 692 256 902 640 437 417 754 794 859 108 914 074 742 459 177 317  $\setminus$   
 703 095 001 287 958 444 761 515 887 590 465 086 615 775 319 560 675 448 041 065 737 050 624  $q^{3852} -$   
 7 852 515 835 271 737 454 816 593 636 106 058 723 164 493 269 188 555 153 413 073 142 715 819 047 911  $\setminus$   
 769 977 928 610 652 895 892 566 253 114 756 871 368 680 486 854 497 827 686 650 694 010 394  $q^{3853} +$   
 8 952 314 596 988 693 885 936 697 942 894 141 258 005 948 380 309 932 067 700 946 173 939 534 839 136  $\setminus$   
 031 479 292 169 272 513 344 612 516 718 894 341 600 150 135 908 691 004 041 741 352 960 000  $q^{3856} -$   
 9 352 030 911 655 449 226 826 177 921 407 439 610 053 829 481 858 024 705 243 284 861 536 514 195 272  $\setminus$   
 586 663 866 491 795 702 915 749 906 049 794 033 931 229 004 520 700 460 909 252 289 757 184  $q^{3857} +$   
 10 661 124 649 880 475 982 822 812 987 749 588 930 737 146 709 989 579 457 982 459 859 902 742 442  $\setminus$   
 730 784 850 195 601 006 313 364 806 821 292 051 095 442 001 671 258 556 274 211 620 281 036 800  
 $q^{3860} -$   
 11 136 887 121 079 818 550 551 379 356 699 944 475 398 798 236 854 386 274 720 210 430 565 309 329  $\setminus$   
 095 024 002 878 054 645 737 439 729 628 485 053 141 578 269 894 719 090 355 081 768 265 582 250  
 $q^{3861} +$   
 12 694 965 467 238 771 430 540 149 061 347 436 897 276 729 854 152 379 832 171 342 246 153 613 114  $\setminus$   
 190 662 022 211 723 767 185 809 777 434 595 843 753 803 254 878 710 379 561 954 428 093 696 000  
 $q^{3864} -$   
 13 261 191 124 802 240 448 476 939 930 812 908 834 430 831 666 793 997 095 168 758 688 717 557 602  $\setminus$   
 078 240 785 306 817 300 790 778 799 122 906 856 087 717 565 349 208 458 418 663 086 510 899 200  
 $q^{3865} +$   
 15 115 443 849 111 492 423 610 374 781 394 493 487 413 005 611 435 417 416 029 743 779 683 788 648  $\setminus$   
 193 858 974 615 398 592 211 188 713 756 926 472 563 202 399 915 500 253 579 379 400 847 280 128  
 $q^{3868} -$   
 15 789 273 356 871 527 291 739 270 099 267 577 915 271 240 211 982 372 801 461 595 627 704 710 503  $\setminus$   
 348 592 281 535 570 494 029 756 276 847 269 170 726 306 588 261 911 938 404 691 092 504 756 625  
 $q^{3869} +$   
 17 995 802 700 358 803 311 340 970 278 947 595 648 593 416 228 372 301 205 783 055 421 008 268 826  $\setminus$   
 722 017 060 546 471 734 603 199 249 893 824 786 981 080 513 277 343 899 451 133 142 631 008 256  
 $q^{3872} -$   
 18 797 613 096 405 735 000 420 101 883 093 224 971 431 946 504 433 712 025 482 906 366 051 741 270  $\setminus$   
 910 326 615 958 144 921 072 018 101 986 256 438 532 140 771 689 636 203 293 843 727 572 762 624  
 $q^{3873} +$   
 21 423 111 124 297 987 704 831 517 908 172 708 186 032 933 849 241 117 808 224 249 507 614 891 338  $\setminus$   
 510 237 180 100 444 282 259 119 659 608 325 967 453 157 275 187 756 440 612 813 232 566 272 000  
 $q^{3876} -$   
 22 377 124 749 728 145 811 767 005 585 147 348 977 932 831 068 433 454 199 915 503 232 841 087 600  $\setminus$   
 684 198 538 920 299 098 616 974 823 291 713 932 994 470 322 983 851 471 902 846 132 756 053 714  
 $q^{3877} +$   
 25 500 865 282 962 347 519 065 969 988 303 477 595 074 869 925 426 754 591 148 114 734 092 957 318  $\setminus$   
 066 151 727 734 868 942 694 870 990 937 577 247 313 606 170 601 066 492 090 136 611 503 539 200  
 $q^{3880} -$   
 26 635 872 880 668 246 306 305 078 336 374 074 766 676 131 340 980 172 862 181 510 515 161 047 211  $\setminus$

373 274 026 779 891 580 041 193 462 519 573 299 749 926 356 346 337 060 125 730 433 359 872 000  
 $q^{3881} +$   
 30 352 076 796 582 814 670 174 177 829 054 659 900 965 818 850 648 604 645 366 566 226 936 422 744  
 659 075 133 924 611 953 420 933 345 980 512 529 341 013 864 830 574 215 018 927 542 801 088 000  
 $q^{3884} -$   
 31 702 296 111 374 447 983 417 462 274 622 548 380 761 029 416 732 198 243 908 966 877 978 980 608  
 978 379 399 732 900 510 977 794 073 112 274 063 568 156 904 117 235 039 623 346 940 899 614 725  
 $q^{3885} +$   
 36 122 939 753 631 659 273 986 754 499 606 841 612 047 334 377 687 076 065 242 472 996 220 520 586  
 457 469 989 922 402 690 591 193 855 418 919 120 244 487 742 546 413 018 534 160 146 555 736 064  
 $q^{3888} -$   
 37 729 034 936 551 548 928 697 834 944 670 642 578 412 010 654 484 566 568 377 842 129 503 427 552  
 127 636 322 889 730 547 668 674 543 006 378 171 175 732 459 816 369 591 612 654 138 691 584 000  
 $q^{3889} +$   
 42 987 184 355 309 665 250 169 213 715 496 046 915 661 004 003 143 115 558 874 595 168 222 946 096  
 064 222 469 070 954 992 311 753 988 120 057 990 004 801 893 649 856 581 131 366 210 912 088 064  
 $q^{3892} -$   
 44 897 476 183 446 505 651 382 116 068 417 531 157 635 729 749 153 940 897 851 066 455 412 781 017  
 092 756 393 181 325 244 310 134 467 671 052 493 154 475 408 729 463 661 330 801 298 114 158 847  
 $q^{3893} +$   
 51 151 245 315 534 845 219 357 897 687 342 775 715 015 665 801 223 716 033 182 917 928 802 999 099  
 565 965 858 890 711 053 070 586 374 764 487 238 205 998 094 882 346 826 594 263 749 772 928 000  
 $q^{3896} -$   
 53 423 147 820 190 137 534 328 775 530 138 139 728 793 607 321 338 726 524 188 089 789 955 123 679  
 004 018 754 171 801 148 941 553 566 113 252 207 673 223 202 438 641 230 906 355 972 826 431 488  
 $q^{3897} +$   
 60 860 396 960 587 278 023 180 196 632 945 643 567 550 205 552 628 779 324 265 993 130 785 831 589  
 083 245 002 112 189 219 695 492 056 334 291 140 855 831 781 643 065 312 332 155 117 128 550 400  
 $q^{3900} -$   
 63 562 122 672 646 305 146 487 588 173 132 586 275 242 382 211 397 943 616 356 615 517 253 398 876  
 808 375 851 380 543 596 094 653 517 225 759 540 819 231 253 841 338 345 003 166 412 205 627 375  
 $q^{3901} +$   
 72 406 035 209 942 314 141 165 183 714 398 371 841 160 077 956 863 923 770 646 621 412 568 752 011  
 699 134 458 601 233 953 187 342 093 576 314 579 063 857 244 052 476 371 706 456 242 896 896 000  
 $q^{3904} -$   
 75 618 619 072 795 200 733 026 951 682 826 932 306 415 384 455 011 459 980 372 766 177 709 533 882  
 354 281 499 223 567 126 378 827 186 855 071 399 225 323 260 530 321 806 162 233 431 221 862 400  
 $q^{3905} +$   
 86 134 320 086 576 257 602 992 181 048 076 707 020 229 720 034 193 070 166 703 067 614 024 918 145  
 002 212 646 649 423 519 652 972 463 629 297 924 249 607 221 620 170 582 754 541 056 656 424 960  
 $q^{3908} -$   
 89 954 021 380 138 604 202 297 330 892 269 467 793 612 749 317 881 097 482 513 984 481 521 454 989  
 339 060 395 150 259 287 061 790 236 486 721 741 579 324 444 420 031 904 987 549 854 466 666 750  
 $q^{3909} +$   
 102 456 432 066 230 443 303 236 916 869 245 694 987 810 055 263 505 259 666 859 805 379 993 676 311  
 093 176 771 946 075 831 763 080 112 758 889 697 458 270 492 369 916 659 473 545 680 031 903 744  
 $q^{3912} -$   
 106 997 584 698 348 816 325 670 760 600 238 283 428 850 465 168 217 967 565 348 753 298 354 575 825  
 574 697 424 809 178 503 674 658 978 808 410 019 255 349 334 211 169 815 614 228 988 749 086 720  
 $q^{3913} +$   
 121 860 742 573 331 759 625 980 351 640 255 534 703 368 218 390 098 608 321 382 992 620 203 059 657  
 524 234 743 986 537 561 343 063 976 585 045 787 714 902 485 684 139 029 914 050 786 992 128 000  
 $q^{3916} -$   
 127 259 137 144 188 183 054 734 539 825 020 902 003 487 564 417 203 528 427 811 089 563 438 026 334  
 455 536 809 127 276 263 150 620 980 202 216 267 196 453 448 133 564 838 618 358 232 660 475 535

$q^{3917} +$   
 144 927 254 619 062 501 002 374 243 659 161 412 909 262 439 683 049 775 336 910 038 240 112 921 722 014 870 854 024 700 702 082 406 451 934 065 572 185 925 565 562 918 438 436 063 440 900 997 120  
 $q^{3920} -$   
 151 344 151 125 434 257 182 067 768 485 399 668 179 806 653 579 894 704 492 821 490 340 787 807 635 397 495 886 824 157 389 037 260 216 758 139 761 478 406 230 347 266 377 222 278 824 873 984 000  
 $q^{3921} +$   
 172 344 735 555 502 312 955 733 454 173 896 428 870 174 741 896 671 162 429 091 265 237 945 733 828 756 978 592 051 014 024 612 326 975 283 426 925 331 410 949 320 108 928 628 333 271 770 880 000  
 $q^{3924} -$   
 179 971 623 919 136 093 263 925 835 091 739 229 656 666 916 592 548 398 830 407 685 156 205 728 416 607 774 579 250 607 213 262 005 996 092 648 637 434 076 216 180 486 248 467 438 469 151 717 300  
 $q^{3925} +$   
 204 931 042 083 851 903 093 495 601 819 319 555 059 491 278 708 397 723 497 543 400 454 730 579 072 421 286 346 266 535 455 191 772 418 701 019 128 223 231 712 495 491 019 589 259 397 230 523 904  
 $q^{3928} -$   
 213 995 289 387 563 438 116 985 322 302 443 078 052 582 658 004 156 197 432 716 133 756 966 486 363 012 778 489 423 133 246 716 191 705 340 660 844 410 851 530 042 489 004 274 351 480 676 352 000  
 $q^{3929} +$   
 243 657 230 247 272 489 360 814 334 518 110 455 141 474 608 428 633 382 861 227 084 414 700 741 590 385 100 633 628 385 194 448 449 914 912 571 216 139 341 996 605 415 833 120 690 093 556 508 672  
 $q^{3932} -$   
 254 428 779 265 929 584 265 954 671 505 676 827 343 529 915 519 350 807 714 228 839 599 540 971 815 472 598 878 226 539 907 994 889 702 937 978 665 775 837 971 864 197 953 935 109 949 848 585 268  
 $q^{3933} +$   
 289 676 152 813 971 902 596 147 830 878 236 330 191 010 091 743 189 343 167 208 112 434 283 733 207 293 476 145 954 079 718 761 314 069 823 666 084 690 649 715 374 922 625 342 338 704 919 552 000  
 $q^{3936} -$   
 302 475 466 871 596 006 489 130 590 406 234 751 646 113 552 359 181 109 743 067 240 898 575 936 332 727 607 509 587 330 136 462 273 158 201 951 696 756 568 016 428 907 456 299 757 221 052 350 464  
 $q^{3937} +$   
 344 356 376 354 514 562 820 912 050 331 563 804 196 750 477 252 468 664 452 904 570 481 773 989 102 751 189 305 829 065 608 874 797 837 840 056 824 514 815 941 543 193 728 908 540 242 969 395 200  
 $q^{3940} -$   
 359 563 861 594 616 015 866 692 106 549 482 057 514 035 275 201 803 095 607 307 547 265 478 440 252 157 625 971 139 130 742 336 589 924 459 977 009 109 079 375 493 734 385 404 875 872 167 331 625  
 $q^{3941} +$   
 409 322 404 155 027 789 314 216 298 609 163 374 370 370 038 259 202 187 351 698 724 043 047 161 334 018 254 242 067 515 064 447 177 357 443 488 479 873 076 294 866 666 754 530 161 664 489 600 000  
 $q^{3944} -$   
 427 389 583 009 824 015 250 038 781 575 356 478 539 648 089 325 798 645 271 913 797 237 755 162 478 525 573 262 865 453 049 715 709 903 872 351 842 556 781 707 402 638 794 267 755 580 792 832 000  
 $q^{3945} +$   
 486 502 373 281 605 684 356 922 680 691 978 834 829 765 313 654 798 462 366 269 509 883 411 288 669 089 305 455 633 237 236 660 832 727 668 267 404 119 620 931 291 313 157 306 272 699 341 058 048  
 $q^{3948} -$   
 507 965 133 486 516 814 982 886 117 840 020 260 832 954 734 070 111 387 713 528 874 951 371 636 241 682 365 319 329 554 043 476 267 093 183 229 459 951 390 887 718 485 154 419 240 820 715 661 500  
 $q^{3949} +$   
 578 184 609 822 022 136 771 280 446 802 735 413 661 171 782 010 277 866 570 571 590 171 877 970 736 748 491 889 648 231 738 938 743 007 353 625 659 772 909 951 980 930 141 274 221 549 551 042 560  
 $q^{3952} -$   
 603 678 913 187 482 282 662 370 871 173 506 210 117 526 439 893 165 331 971 001 842 401 309 316 315 354 991 546 154 321 475 175 727 477 618 444 215 924 999 843 312 663 764 889 018 426 220 576 768  
 $q^{3953} +$

687 084 681 731 528 501 176 533 000 942 843 405 129 964 732 944 567 891 081 888 881 883 482 152 525 843 221 415 960 461 378 922 649 855 600 965 353 244 435 532 712 248 444 997 601 090 441 728 000  
 $q^{3956} -$   
 717 365 187 761 193 968 975 781 703 620 327 965 188 404 217 518 909 705 092 912 853 951 626 960 194 760 447 376 131 412 417 442 893 628 527 499 498 800 338 895 310 043 200 497 809 496 716 106 615  
 $q^{3957} +$   
 816 424 891 077 561 384 832 904 918 505 597 313 658 154 038 208 442 981 248 413 058 388 831 156 924 714 320 651 261 485 415 093 958 192 557 794 292 126 111 958 347 410 122 422 979 124 794 291 200  
 $q^{3960} -$   
 852 387 034 428 828 953 262 374 733 618 073 431 255 366 232 876 387 381 657 317 058 550 085 364 807 727 232 661 057 090 764 642 836 927 610 311 431 148 703 169 308 484 796 585 031 961 460 736 000  
 $q^{3961} +$   
 970 028 505 420 956 332 075 762 294 522 156 462 985 365 892 885 872 809 339 422 574 359 294 812 335 584 225 082 426 016 351 128 937 710 926 549 506 190 308 368 723 441 259 316 156 530 758 144 000  
 $q^{3964} -$   
 1 012 734 665 527 408 778 919 379 095 667 121 845 660 820 294 952 439 541 183 555 219 279 100 370 478 250 751 756 565 564 221 972 688 288 774 685 415 094 076 451 218 076 808 534 757 670 778 681 025  
 $q^{3965} +$   
 1 152 431 451 768 044 081 227 398 135 382 662 658 204 196 617 773 424 856 083 691 779 432 894 347 170 482 419 422 039 526 977 642 410 291 347 210 003 032 653 638 517 266 314 065 173 435 016 937 472  
 $q^{3968} -$   
 1 203 141 970 506 910 490 670 274 543 302 651 014 659 654 740 028 993 263 227 280 893 526 196 359 780 186 958 429 296 889 308 540 452 921 844 587 032 602 467 176 014 600 989 961 717 763 305 472 248  
 $q^{3969} +$   
 1 369 014 698 016 139 313 174 948 566 408 095 920 621 741 772 052 501 676 885 631 551 321 170 519 804 593 514 780 237 685 733 487 957 720 356 145 542 844 883 581 799 776 224 439 933 992 052 506 624  
 $q^{3972} -$   
 1 429 224 640 445 090 606 910 005 426 215 057 475 409 333 885 606 655 415 600 422 405 518 955 916 262 697 228 568 669 294 363 833 533 021 338 827 509 245 997 015 406 047 439 018 377 910 784 543 277  
 $q^{3973} +$   
 1 626 161 140 327 797 712 052 843 288 807 081 847 009 973 949 912 536 544 483 596 213 222 289 982 453 314 878 153 767 232 441 562 511 984 293 832 871 565 967 726 730 411 341 685 583 558 218 752 000  
 $q^{3976} -$   
 1 697 643 858 181 160 676 051 498 316 192 000 918 227 270 961 763 155 649 388 820 108 298 343 531 555 464 163 989 731 322 515 909 724 077 457 296 729 987 470 362 087 446 528 776 848 650 037 035 008  
 $q^{3977} +$   
 1 931 441 517 235 490 624 570 037 969 377 620 919 446 733 221 669 260 340 547 103 763 203 257 600 525 399 784 634 592 742 757 384 539 956 810 392 590 097 938 815 945 473 450 789 363 049 927 577 600  
 $q^{3980} -$   
 2 016 300 269 726 438 052 461 003 691 028 314 780 625 296 493 760 662 923 591 057 428 322 805 330 493 826 291 548 174 050 461 839 412 866 512 816 299 312 662 770 435 774 215 971 443 631 795 660 250  
 $q^{3981} +$   
 2 293 834 702 393 591 369 363 893 461 126 980 193 829 223 077 773 495 669 514 820 512 310 761 032 304 839 395 429 631 734 668 287 902 936 125 255 442 277 082 052 595 417 136 702 824 360 591 360 000  
 $q^{3984} -$   
 2 394 563 819 432 331 046 266 039 165 548 138 849 322 486 189 351 454 977 422 154 689 503 818 421 006 167 598 459 231 960 965 133 373 976 664 726 865 526 674 926 657 224 864 239 735 188 424 294 400  
 $q^{3985} +$   
 2 723 988 711 278 229 480 878 875 903 322 601 965 829 307 607 733 305 697 760 084 737 373 920 500 516 178 124 678 504 269 646 259 133 872 235 580 093 484 348 013 507 006 232 339 632 768 602 658 816  
 $q^{3988} -$   
 2 843 546 057 007 388 183 149 900 986 584 734 219 457 400 733 396 634 982 727 798 483 212 272 833 075 355 652 536 092 279 893 226 147 150 681 638 171 609 763 107 802 887 423 156 392 207 312 004 625  
 $q^{3989} +$   
 3 234 529 920 588 782 055 043 466 282 485 544 218 057 325 217 500 960 265 866 436 989 417 836 089 699

445 255 626 372 909 166 318 640 800 318 086 135 039 201 579 861 533 685 938 777 354 542 370 304  
 $q^{3992} -$   
 3 376 422 737 863 484 557 191 639 310 622 290 103 575 440 809 519 518 986 262 521 951 572 474 198 683  
 965 253 154 509 983 919 998 467 635 255 488 587 306 423 615 428 386 628 363 898 795 818 352 640  
 $q^{3993} +$   
 3 840 429 375 487 153 905 422 704 210 505 201 920 158 069 802 074 526 307 988 416 871 731 281 602 774  
 981 005 537 358 597 220 638 885 168 237 588 114 991 741 699 394 387 034 962 315 131 911 168 000  
 $q^{3996} -$   
 4 008 815 973 698 084 259 447 702 380 240 959 820 855 797 634 134 932 150 513 561 076 210 678 278 604  
 611 788 297 844 462 280 006 751 189 102 189 102 789 403 883 570 910 977 304 149 427 666 063 025  
 $q^{3997} +$   
 4 559 436 687 957 900 072 524 153 248 744 701 027 453 477 645 167 927 427 461 608 893 358 476 205 180  
 399 627 763 238 869 881 471 620 981 682 004 904 306 662 266 439 287 090 176 977 589 279 744 000  
 $q^{4000} -$   
 4 759 246 888 176 314 669 568 522 151 163 354 569 126 893 471 349 470 527 611 836 474 687 707 329 357  
 872 710 026 982 092 110 223 377 398 987 095 166 832 225 847 580 878 688 030 435 484 868 608 000  
 $q^{4001} +$   
 5 412 593 955 377 742 103 814 445 647 181 898 701 070 614 274 373 352 705 127 201 808 140 091 856 182  
 623 668 739 235 581 685 193 528 419 362 981 510 966 255 351 733 244 351 046 971 320 782 848 000  
 $q^{4004} -$   
 5 649 671 740 913 486 118 038 669 364 835 725 569 354 273 561 644 694 931 449 421 283 232 282 056 324  
 686 416 042 936 309 104 286 268 939 050 762 279 878 436 588 074 782 189 535 481 183 572 056 750  
 $q^{4005} +$   
 6 424 844 406 078 525 183 461 570 351 027 399 260 975 657 196 902 169 780 411 436 958 559 814 964 027  
 258 022 161 614 604 392 224 876 871 352 690 044 087 604 269 389 384 889 915 733 129 406 029 824  
 $q^{4008} -$   
 6 706 116 858 217 391 431 063 515 700 113 627 849 531 616 502 985 811 442 357 113 854 588 296 231 512  
 006 430 317 986 930 354 168 191 251 839 608 001 383 400 156 509 876 810 319 763 615 813 632 000  
 $q^{4009} +$   
 7 625 753 172 351 289 496 715 760 579 928 017 078 152 876 570 421 092 905 836 661 063 835 698 544 793  
 341 930 092 503 484 631 191 331 455 335 833 275 771 847 527 095 503 814 073 558 543 210 895 360  
 $q^{4012} -$   
 7 959 430 518 036 784 725 222 313 204 383 726 359 243 293 189 165 349 252 272 040 142 732 981 678 470  
 874 086 327 300 399 889 634 135 559 100 049 249 258 960 436 468 187 168 735 200 576 525 660 490  
 $q^{4013} +$   
 9 050 360 776 677 486 612 856 061 745 909 356 499 975 106 999 189 592 255 029 173 671 509 186 946 776  
 937 062 812 307 628 292 165 603 119 381 162 427 357 916 761 182 526 606 311 038 447 170 048 000  
 $q^{4016} -$   
 9 446 173 258 206 438 024 793 808 347 433 130 637 863 052 627 796 323 363 906 337 179 167 776 552 836  
 966 620 576 144 564 509 776 414 951 098 600 027 900 826 843 856 936 439 899 433 275 809 726 464  
 $q^{4017} +$   
 10 740 193 683 424 561 417 116 827 663 629 507 806 554 938 166 091 554 211 751 202 958 062 747 437  
 869 767 286 772 106 450 825 934 405 586 117 470 822 558 394 910 116 959 987 286 450 962 814 566 400  
 $q^{4020} -$   
 11 209 672 004 622 692 454 933 008 348 038 317 384 167 619 311 135 776 207 180 515 138 650 167 767  
 109 208 721 654 870 998 602 441 067 057 010 522 752 653 009 980 555 780 441 134 695 317 973 123 875  
 $q^{4021} +$   
 12 744 460 721 458 814 910 299 563 962 095 960 086 961 931 702 418 906 375 872 526 606 853 682 809  
 847 684 400 510 305 347 817 672 875 351 083 825 066 271 983 069 306 433 229 607 172 863 378 560 000  
 $q^{4024} -$   
 13 301 268 059 570 082 279 332 768 969 094 712 856 892 146 457 913 806 162 570 704 180 922 690 080  
 593 865 617 246 153 898 060 213 322 441 158 846 598 742 842 656 329 850 282 357 929 362 977 587 200  
 $q^{4025} +$   
 15 121 469 447 903 097 112 046 498 464 211 495 644 878 237 056 070 330 463 236 265 705 280 736 743  
 523 674 227 708 926 301 115 803 012 109 029 440 477 579 726 777 604 731 292 819 045 122 943 383 552

$q^{4028} -$   
 15 781 794 480 147 069 721 820 424 632 126 743 642 636 082 933 148 686 562 964 804 996 418 494 226 \
 892 709 038 434 225 178 929 388 079 351 165 449 166 583 499 066 013 319 196 945 597 134 728 129 750  
 $q^{4029} +$   
 17 940 302 746 994 225 982 808 388 235 858 314 152 128 018 560 211 653 759 444 313 631 869 737 552 \
 261 311 683 829 343 279 434 508 850 229 380 055 346 192 948 019 835 940 585 085 776 555 582 029 824  
 $q^{4032} -$   
 18 723 324 866 261 468 746 579 536 361 158 024 407 555 335 471 546 505 788 775 197 104 501 586 516 \
 345 624 016 182 063 214 278 815 381 730 959 485 488 946 714 876 573 613 190 836 678 140 888 678 400  
 $q^{4033} +$   
 21 282 803 314 746 797 202 245 282 047 468 252 523 483 543 595 666 361 001 195 540 045 747 594 444 \
 449 596 153 401 396 186 378 444 249 464 423 094 507 801 854 977 724 055 392 977 552 196 282 368 000  
 $q^{4036} -$   
 22 211 243 248 445 474 101 727 203 200 281 959 490 386 062 108 086 163 443 708 558 941 227 118 179 \
 157 601 128 083 406 257 821 105 618 915 113 691 611 645 402 182 071 533 314 914 188 113 461 422 269  
 $q^{4037} +$   
 25 245 922 375 468 052 223 469 053 726 313 747 874 298 136 604 832 726 547 843 291 105 296 878 705 \
 826 190 984 509 269 191 169 476 992 477 884 033 342 560 163 496 321 541 864 574 735 156 584 320 000  
 $q^{4040} -$   
 26 346 693 832 060 751 540 526 070 253 658 320 626 056 947 983 850 468 153 489 851 672 030 105 869 \
 855 882 438 047 638 029 727 594 206 014 930 124 355 991 046 129 573 597 668 831 546 534 178 816 000  
 $q^{4041} +$   
 29 944 499 252 821 846 404 933 057 509 414 804 628 531 413 592 117 506 773 721 123 804 136 927 325 \
 651 843 485 751 316 419 094 958 859 527 174 395 661 678 787 118 992 342 300 751 886 660 769 536 000  
 $q^{4044} -$   
 31 249 480 069 349 576 638 479 130 561 136 281 409 694 220 416 837 949 631 072 077 261 675 198 399 \
 279 588 918 806 150 232 691 069 767 861 038 522 987 019 405 705 135 023 695 983 675 317 422 984 700  
 $q^{4045} +$   
 35 514 550 562 702 231 002 473 142 350 579 540 077 052 246 295 816 628 861 257 332 612 223 292 438 \
 746 159 549 247 004 788 648 632 223 876 639 932 502 145 797 331 665 264 849 496 141 956 639 588 352  
 $q^{4048} -$   
 37 061 495 192 981 336 077 727 178 079 137 770 128 149 710 118 874 946 871 174 447 253 378 891 183 \
 094 319 164 841 856 761 847 024 164 581 289 149 168 073 283 052 582 063 259 358 346 806 075 392 000  
 $q^{4049} +$   
 42 117 162 146 006 990 416 200 366 820 446 487 928 419 924 470 339 706 006 570 980 522 748 391 020 \
 694 429 040 314 818 735 539 280 278 119 487 094 416 350 143 545 807 982 031 013 377 868 271 699 968  
 $q^{4052} -$   
 43 950 781 306 939 496 043 306 779 762 258 822 920 868 315 021 151 074 389 950 181 661 023 828 978 \
 207 448 947 207 968 344 341 521 983 497 096 648 662 036 240 634 689 570 789 468 519 912 228 871 098  
 $q^{4053} +$   
 49 943 093 815 939 318 920 503 549 041 402 794 211 773 859 357 856 811 622 445 096 662 191 513 592 \
 043 170 241 199 871 190 181 215 725 776 192 544 537 935 843 955 586 115 966 543 699 192 500 032 000  
 $q^{4056} -$   
 52 116 331 809 149 272 596 714 217 552 036 816 080 986 727 770 261 158 658 049 306 991 332 039 751 \
 205 877 328 933 777 164 124 313 623 360 632 420 182 617 743 728 561 491 690 536 943 605 653 471 232  
 $q^{4057} +$   
 59 218 227 028 224 165 614 101 021 051 463 128 850 912 626 147 272 652 543 143 093 421 121 183 516 \
 783 759 999 417 852 363 253 578 213 999 496 624 133 025 912 385 578 986 811 497 748 673 507 225 600  
 $q^{4060} -$   
 61 793 772 806 631 865 787 280 680 936 975 202 292 472 135 977 269 837 009 571 213 545 418 195 367 \
 090 642 412 347 230 564 008 406 655 432 324 226 635 454 430 897 463 186 961 118 385 817 895 439 250  
 $q^{4061} +$   
 70 210 009 250 148 762 485 115 331 975 958 824 118 191 269 280 745 633 923 762 586 339 103 903 301 \
 068 996 460 245 774 136 748 075 444 301 385 414 351 313 136 928 402 292 122 913 291 983 147 008 000  
 $q^{4064} -$

73 262 083 858 277 847 777 193 136 146 037 761 523 835 360 508 623 887 904 077 167 453 320 693 924 :  
 940 529 358 997 829 661 728 733 357 422 781 887 261 673 470 272 853 734 067 532 573 047 855 513 600  
 $q^{4065} +$   
 83 235 076 762 482 592 102 798 651 126 725 089 394 680 256 347 943 290 104 604 211 946 223 377 420 :  
 941 287 144 546 291 857 479 227 410 096 632 163 999 748 030 063 908 989 975 793 837 787 296 530 432  
 $q^{4068} -$   
 86 851 547 527 195 253 606 206 196 788 404 931 816 481 881 154 233 573 737 486 206 837 961 971 163 :  
 293 739 594 440 868 880 015 878 850 191 804 944 135 040 982 406 236 936 985 462 318 324 555 674 875  
 $q^{4069} +$   
 98 668 270 652 292 244 507 809 095 520 147 673 834 789 886 950 632 575 530 264 669 878 154 606 511 :  
 547 484 358 313 350 075 511 283 196 837 430 095 508 770 407 101 684 251 989 357 355 540 095 489 536  
 $q^{4072} -$   
 102 953 151 651 963 885 582 151 119 074 908 657 224 497 658 607 045 651 111 090 338 213 054 895 711 :  
 192 863 545 591 177 296 665 798 758 047 587 616 755 874 770 890 758 193 731 370 142 624 198 230 016  
 $q^{4073} +$   
 116 953 299 759 212 056 708 343 716 335 182 776 489 865 226 401 707 658 721 495 415 961 380 706 849 :  
 421 061 076 539 776 328 906 531 682 561 533 291 341 155 207 482 452 639 922 626 034 044 308 544 000  
 $q^{4076} -$   
 122 029 708 907 432 943 324 281 356 991 206 214 545 168 739 410 430 352 869 618 745 733 976 907 573 :  
 364 002 439 599 899 904 587 707 091 042 854 839 010 078 060 813 527 174 764 432 891 427 814 876 338  
 $q^{4077} +$   
 138 615 350 402 259 011 470 071 804 192 840 325 436 615 963 893 377 828 339 251 076 257 421 423 582 :  
 237 660 538 002 573 683 756 281 641 534 863 229 018 227 021 410 012 710 488 124 979 990 511 616 000  
 $q^{4080} -$   
 144 629 006 245 909 725 788 464 380 124 603 498 309 644 736 583 786 392 521 655 231 480 590 920 879 :  
 448 096 037 244 479 612 176 009 089 112 998 660 506 413 257 124 072 266 481 431 826 376 802 304 000  
 $q^{4081} +$   
 164 275 997 112 339 414 926 054 551 658 374 029 703 645 144 490 901 815 119 059 908 870 526 061 341 :  
 501 428 116 152 768 326 892 564 273 092 999 451 937 025 514 638 872 461 127 224 784 951 342 848 000  
 $q^{4084} -$   
 171 399 353 516 002 751 403 196 463 395 269 739 567 233 093 833 137 180 337 639 566 484 652 132 423 :  
 401 292 544 215 667 166 202 565 957 818 191 103 701 320 106 931 533 625 247 235 329 720 833 041 250  
 $q^{4085} +$   
 194 670 832 829 691 190 705 724 239 899 004 611 059 130 931 716 783 950 849 884 648 935 944 722 641 :  
 000 550 034 070 691 822 185 368 939 883 914 583 263 749 290 023 403 296 398 963 220 428 807 618 560  
 $q^{4088} -$   
 203 107 967 514 892 015 720 333 487 632 478 988 049 327 482 816 839 378 203 285 359 015 257 025 330 :  
 069 752 339 106 055 617 666 384 867 297 795 393 629 326 869 671 521 768 582 719 839 203 270 656 000  
 $q^{4089} +$   
 230 670 312 868 123 498 598 000 014 074 461 153 534 970 362 492 231 721 317 411 673 647 076 045 553 :  
 704 527 770 448 490 961 730 782 227 711 052 061 050 815 340 040 399 124 951 073 910 303 254 577 152  
 $q^{4092} -$   
 240 662 706 787 622 228 930 150 129 934 100 528 134 256 604 601 735 074 346 307 391 779 087 133 449 :  
 936 436 996 395 263 432 897 842 476 060 291 706 156 245 569 625 724 459 456 959 160 778 400 553 655  
 $q^{4093} +$   
 273 304 396 489 864 509 551 710 950 054 187 728 119 502 650 561 916 580 003 087 670 560 549 064 699 :  
 782 086 616 883 050 154 538 774 188 948 474 060 119 645 512 834 591 014 437 410 854 810 788 298 752  
 $q^{4096} -$   
 285 137 765 823 076 391 523 306 862 235 621 340 560 154 978 919 937 210 092 055 286 031 231 532 607 :  
 121 942 741 070 589 338 461 992 654 734 400 086 416 827 338 568 541 316 514 367 588 293 801 934 848  
 $q^{4097} +$   
 323 791 675 642 219 182 672 665 734 439 974 829 318 454 370 947 559 214 577 218 812 589 749 291 636 :  
 331 993 069 097 748 641 966 477 983 871 408 684 153 484 610 850 076 659 767 411 737 829 899 468 800  
 $q^{4100} -$   
 337 804 047 480 578 859 312 157 645 922 279 606 059 492 182 393 358 053 641 953 202 794 801 000 266 :

603 394 183 855 861 697 656 311 227 399 433 889 060 310 047 077 417 412 988 084 948 547 797 582 625  
 $q^{4101} +$   
 383 573 805 188 622 167 256 197 319 284 378 130 980 568 218 119 175 883 755 295 629 309 395 793 846  
 669 386 966 638 178 648 364 584 059 409 863 577 903 681 039 190 640 840 209 385 283 630 866 432 000  
 $q^{4104} -$   
 400 165 062 544 608 557 875 213 070 388 928 694 890 059 856 560 546 780 719 611 878 470 129 126 561  
 621 382 185 485 359 524 121 550 633 607 867 259 879 370 376 612 943 644 035 191 303 800 546 918 400  
 $q^{4105} +$   
 454 356 196 252 145 500 279 333 814 745 479 446 807 817 956 374 353 299 743 607 796 122 697 974 825  
 354 614 044 739 277 294 878 627 302 171 473 257 533 330 042 657 702 597 689 769 872 597 950 867 456  
 $q^{4108} -$   
 473 999 358 822 321 301 440 307 480 101 754 993 710 428 176 189 998 312 910 348 563 818 489 214 720  
 327 125 300 909 837 593 578 315 672 802 780 263 299 123 989 325 274 926 077 494 563 039 388 381 750  
 $q^{4109} +$   
 538 156 108 123 940 145 994 414 525 305 361 888 972 899 080 090 179 573 993 305 214 453 495 922 364  
 027 246 300 430 312 789 083 816 127 804 482 515 256 632 218 231 989 039 886 799 138 144 402 276 352  
 $q^{4112} -$   
 561 410 663 384 475 223 027 429 763 370 664 066 142 991 137 107 184 457 619 930 930 146 494 310 781  
 904 854 296 835 794 378 868 812 403 592 537 669 021 561 178 990 236 625 278 799 691 915 654 004 736  
 $q^{4113} +$   
 637 359 479 341 869 264 005 983 525 334 448 594 181 186 747 993 059 492 841 903 209 555 519 818 685  
 897 826 106 191 491 181 501 464 855 335 322 315 677 241 588 473 041 880 508 855 223 234 670 592 000  
 $q^{4116} -$   
 664 887 135 374 856 171 197 911 830 605 012 702 813 896 350 773 473 510 831 414 295 443 358 908 969  
 020 175 662 159 392 123 431 857 333 428 849 516 379 778 475 891 964 301 059 235 538 274 743 395 674  
 $q^{4117} +$   
 754 788 080 639 058 942 944 332 531 784 418 845 239 994 253 417 199 500 089 347 294 462 295 214 048  
 302 132 206 103 864 040 735 459 766 910 989 978 354 054 381 667 026 891 472 195 099 079 521 510 400  
 $q^{4120} -$   
 787 371 379 136 042 956 556 644 051 941 843 590 073 789 146 130 383 302 727 220 657 911 774 031 725  
 476 803 599 671 199 413 287 462 006 732 113 562 495 166 786 046 241 034 060 071 915 013 545 984 000  
 $q^{4121} +$   
 893 778 858 127 862 614 953 636 052 234 288 204 783 278 991 333 110 022 978 013 680 574 493 719 110  
 831 010 374 474 276 872 659 175 328 620 250 669 566 815 353 491 478 372 954 600 946 399 598 336 000  
 $q^{4124} -$   
 932 343 165 128 403 746 437 106 146 356 787 672 142 962 520 780 979 623 573 972 703 305 106 492 586  
 286 755 046 353 950 489 489 757 276 198 252 599 439 165 438 505 785 482 321 841 325 877 195 100 125  
 $q^{4125} +$   
 1 058 277 672 137 171 845 909 986 721 919 686 559 078 076 619 610 615 927 961 620 708 556 276 948 020  
 885 549 478 862 935 014 226 838 725 273 465 371 753 062 237 997 861 002 440 300 235 710 386 995 200  
 $q^{4128} -$   
 1 103 917 157 398 038 145 835 039 463 684 719 298 207 069 385 450 795 082 265 983 896 715 994 923 416  
 422 589 702 141 355 279 513 909 670 206 834 794 172 628 109 809 535 325 586 279 713 673 547 776 000  
 $q^{4129} +$   
 1 252 950 034 772 586 514 385 629 360 727 325 435 512 928 014 140 752 833 824 909 716 131 244 146 373  
 271 347 992 447 750 655 223 279 995 365 584 334 157 807 271 061 155 175 312 043 222 788 698 521 600  
 $q^{4132} -$   
 1 306 958 360 777 019 395 499 672 798 952 435 130 982 598 140 887 358 851 265 608 472 721 181 967 347  
 088 839 721 931 287 124 474 314 546 683 932 838 981 152 609 838 555 183 865 511 380 418 349 986 392  
 $q^{4133} +$   
 1 483 311 918 378 188 362 072 938 854 688 731 750 346 600 369 865 034 027 792 158 548 069 856 464 162  
 244 166 875 976 850 099 722 071 052 918 223 463 691 012 189 192 858 951 308 489 794 173 166 720 000  
 $q^{4136} -$   
 1 547 218 489 889 672 062 022 147 078 947 229 456 217 034 367 688 063 862 865 073 912 743 429 849 689  
 907 839 363 645 775 509 909 945 280 711 573 174 665 009 560 459 688 099 760 454 237 931 648 319 488

$q^{4137} +$   
 1 755 884 260 443 192 077 310 709 055 220 973 265 425 759 952 476 359 026 812 873 011 267 579 860 933 3  
 420 022 615 976 381 110 750 391 728 083 862 632 089 460 999 718 692 489 984 007 236 219 281 536 000  
 $q^{4140} -$   
 1 831 497 038 725 880 916 002 957 428 089 512 918 572 355 865 602 738 487 766 677 346 138 538 727 707 3  
 609 583 199 349 151 783 478 050 467 097 410 535 186 529 283 088 611 319 613 196 640 073 308 533 250  
 $q^{4141} +$   
 2 078 375 443 198 500 427 819 547 770 377 248 742 206 215 914 229 622 428 854 411 702 682 764 534 498 3  
 707 675 868 980 954 605 861 047 308 147 541 035 592 362 693 360 056 819 961 023 213 747 648 512 000  
 $q^{4144} -$   
 2 167 831 509 740 435 055 050 993 708 595 939 071 517 850 047 165 838 586 279 783 687 453 108 641 662 3  
 096 910 338 602 930 496 622 442 212 669 568 644 833 642 448 864 786 103 237 399 601 168 560 947 200  
 $q^{4145} +$   
 2 459 896 795 959 715 592 094 232 878 159 438 357 503 956 443 906 982 887 936 638 449 361 155 839 059 3  
 717 429 231 949 278 906 802 704 149 031 660 268 648 955 113 393 040 103 684 786 475 911 627 182 080  
 $q^{4148} -$   
 2 565 722 063 663 047 577 885 241 104 447 236 051 944 690 137 434 304 696 766 612 087 335 007 053 580 3  
 104 217 075 987 134 316 082 775 329 555 600 854 768 405 289 976 450 994 130 399 307 820 806 918 250  
 $q^{4149} +$   
 2 911 217 076 136 034 972 839 925 759 528 006 452 590 988 126 877 835 862 225 289 692 546 831 372 032 3  
 731 998 569 025 973 489 603 827 599 467 435 612 887 998 264 499 618 883 799 411 066 742 033 026 048  
 $q^{4152} -$   
 3 036 396 797 275 162 994 715 184 074 899 932 037 950 654 539 750 918 219 382 959 343 773 200 163 545 3  
 796 808 232 914 681 520 335 502 974 723 224 616 379 509 071 264 523 953 085 691 283 530 114 433 024  
 $q^{4153} +$   
 3 445 062 955 412 462 172 346 344 083 693 174 980 478 874 475 817 846 010 057 457 774 204 859 975 403 3  
 843 822 968 642 821 599 508 606 169 438 684 121 891 065 351 390 559 813 623 801 968 098 627 072 000  
 $q^{4156} -$   
 3 593 124 972 033 117 387 499 355 052 163 528 683 264 206 657 961 911 874 444 864 930 332 333 405 075 3  
 475 490 304 609 967 508 102 054 370 337 305 790 440 742 059 927 060 605 801 603 055 740 700 000 169  
 $q^{4157} +$   
 4 076 473 799 994 785 698 467 203 428 628 082 928 840 765 064 974 570 712 544 161 467 731 931 648 193 3  
 762 811 859 210 859 836 781 955 604 567 916 686 202 709 178 725 045 147 166 451 667 726 552 268 800  
 $q^{4160} -$   
 4 251 586 831 877 227 200 094 708 152 411 315 420 461 711 849 710 378 976 582 184 015 474 005 531 241 3  
 540 363 412 596 149 745 211 158 920 722 505 479 861 303 570 044 886 982 050 362 721 567 997 952 000  
 $q^{4161} +$   
 4 823 220 522 227 102 912 350 594 207 926 663 186 555 473 619 144 224 602 535 123 395 586 313 302 307 3  
 680 034 861 347 493 275 626 552 776 994 306 890 585 708 023 115 713 477 779 421 801 818 597 376 000  
 $q^{4164} -$   
 5 030 310 199 538 674 561 017 673 929 924 827 214 638 674 422 048 503 655 341 937 793 040 007 803 983 3  
 335 792 398 615 197 480 213 580 671 741 896 193 281 594 854 036 651 910 967 410 849 727 040 413 575  
 $q^{4165} +$   
 5 706 300 035 688 300 536 954 536 113 095 914 015 782 476 621 270 988 702 991 014 708 155 282 709 093 3  
 985 036 490 095 536 367 223 038 938 875 778 476 113 880 052 629 284 203 925 520 375 774 810 311 680  
 $q^{4168} -$   
 5 951 185 869 163 994 660 971 427 703 539 062 712 509 137 532 175 507 294 530 956 683 223 780 445 337 3  
 709 933 043 071 351 023 774 511 859 723 725 130 521 617 727 366 417 008 155 136 516 031 565 824 000  
 $q^{4169} +$   
 6 750 518 914 559 310 713 472 487 890 694 647 833 771 400 681 087 005 610 060 858 787 721 534 579 731 3  
 675 590 111 175 862 606 809 852 478 585 990 503 593 040 584 441 073 297 550 876 052 214 061 297 664  
 $q^{4172} -$   
 7 040 075 968 617 187 827 852 988 467 553 627 545 971 414 091 718 053 067 956 783 621 917 088 824 412 3  
 406 152 307 435 170 817 286 894 574 637 694 387 655 226 504 547 504 295 518 029 316 287 983 474 238  
 $q^{4173} +$

7 985 182 296 585 834 121 927 541 903 578 969 816 265 217 480 565 879 388 248 417 729 180 792 605 900 \\  
 771 533 261 257 213 635 585 423 952 039 614 437 292 191 919 854 740 110 410 114 488 297 838 592 000 \\  
 $q^{4176} -$

8 327 532 005 686 446 885 819 167 021 870 158 766 409 324 861 055 450 465 947 630 108 242 682 300 182 \\  
 055 071 156 242 337 553 139 048 896 489 627 349 358 043 455 913 078 567 481 616 922 901 173 829 632 \\  
 $q^{4177} +$

9 444 906 943 242 926 110 356 804 725 966 769 760 570 856 829 785 042 564 971 675 922 446 121 165 734 \\  
 971 540 921 824 966 733 177 296 370 942 065 700 469 204 778 883 813 360 143 966 231 139 021 619 200 \\  
 $q^{4180} -$

9 849 642 307 267 068 062 210 773 132 726 527 516 522 445 507 097 846 378 793 246 720 610 693 430 813 \\  
 011 276 979 929 638 726 414 172 388 782 856 383 681 619 890 095 345 709 358 993 682 165 958 112 625 \\  
 $q^{4181} +$

11 170 580 758 343 116 558 799 926 431 695 144 738 441 537 099 997 855 530 479 371 449 387 512 092 \\  
 318 573 565 220 599 617 184 256 245 113 731 970 456 978 738 874 841 636 200 092 562 017 776 938 944 \\  
 000  $q^{4184} -$

11 649 032 090 255 274 354 827 067 210 534 301 202 401 695 908 795 419 308 780 057 128 097 181 027 \\  
 113 914 150 465 034 446 591 017 897 203 272 481 693 383 099 974 857 556 332 385 520 247 593 199 206 \\  
 400  $q^{4185} +$

13 210 495 058 698 134 904 032 641 668 144 384 236 650 894 792 668 075 474 546 142 199 221 232 625 \\  
 081 369 579 202 823 294 527 014 511 711 875 212 247 312 349 157 890 183 943 611 048 632 960 698 316 \\  
 800  $q^{4188} -$

13 776 043 562 557 837 486 623 135 340 153 748 893 711 066 234 914 631 381 836 212 125 917 549 864 \\  
 633 779 514 895 127 674 848 663 238 177 640 136 243 244 214 366 537 373 048 659 319 588 874 872 262 \\  
 500  $q^{4189} +$

15 621 680 595 137 069 182 068 495 753 657 852 881 804 089 569 997 187 682 278 148 560 665 343 551 \\  
 351 476 773 619 762 225 050 938 025 542 950 029 531 500 425 488 195 169 792 066 751 772 589 764 259 \\  
 840  $q^{4192} -$

16 290 128 354 373 232 832 394 854 276 558 906 049 370 172 345 600 517 092 523 451 475 703 749 706 \\  
 109 518 030 915 265 968 550 302 410 151 078 617 542 572 433 459 795 114 027 874 493 067 787 928 797 \\  
 184  $q^{4193} +$

18 471 483 865 870 324 086 663 819 546 076 280 645 462 999 776 143 189 517 877 031 657 935 165 206 \\  
 739 467 535 610 564 811 467 820 778 776 805 800 693 637 516 794 457 110 297 412 962 376 793 643 008 \\  
 000  $q^{4196} -$

19 261 490 355 675 823 556 046 942 915 197 298 844 886 190 864 619 928 319 744 872 314 530 802 321 \\  
 343 960 018 572 266 903 527 458 199 571 012 551 197 324 526 592 075 430 958 446 422 468 589 881 143 \\  
 355  $q^{4197} +$

21 839 426 795 988 347 756 218 612 384 169 421 182 023 510 351 200 506 306 158 412 943 915 845 078 \\  
 890 671 854 649 791 368 519 647 365 172 055 197 335 571 696 016 100 446 710 409 909 743 143 704 806 \\  
 400  $q^{4200} -$

22 773 023 840 961 262 353 070 842 222 012 718 166 878 944 118 610 535 921 027 977 537 402 397 958 \\  
 310 308 630 105 157 371 325 855 361 289 286 720 853 057 745 093 128 845 211 354 832 042 686 517 248 \\  
 000  $q^{4201} +$

25 819 400 552 331 492 389 647 737 250 323 701 714 446 127 888 641 087 249 725 081 577 654 034 355 \\  
 433 843 595 833 342 337 379 771 687 799 126 570 912 703 882 289 833 883 008 805 720 656 388 859 968 \\  
 000  $q^{4204} -$

26 922 599 779 626 396 328 506 437 519 535 173 009 157 803 955 404 768 579 506 073 179 541 707 686 \\  
 818 397 513 639 323 199 771 335 793 480 153 507 996 658 587 532 264 610 618 098 598 795 060 571 726 \\  
 045  $q^{4205} +$

30 522 253 328 676 425 166 954 757 904 039 474 313 656 517 698 669 841 760 054 624 784 082 887 587 \\  
 002 417 546 997 025 019 527 051 284 476 381 830 084 576 615 545 254 793 673 115 620 020 307 505 856 \\  
 512  $q^{4208} -$

31 825 762 675 066 005 189 909 951 882 129 591 514 504 072 296 225 032 514 066 532 417 439 975 427 \\  
 150 647 620 965 117 591 458 096 717 584 496 913 040 678 969 983 446 906 498 166 812 685 754 523 648 \\  
 000  $q^{4209} +$

36 078 842 615 332 580 511 459 260 611 486 673 258 342 111 024 259 953 948 989 952 715 112 755 721 \

552 011 422 173 847 724 796 375 643 787 428 893 698 083 989 932 455 721 674 964 065 812 080 154 380 \
 288  $q^{4212}$  -

37 618 911 400 956 400 000 624 423 306 044 395 163 240 815 313 673 579 314 355 426 828 168 883 606 \
 421 243 276 834 833 202 364 984 366 535 261 463 919 235 895 432 983 815 405 473 605 920 970 302 262 \
 526  $q^{4213}$  +

42 643 635 046 019 042 304 924 574 179 768 386 212 855 768 331 627 061 885 255 184 566 311 307 214 \
 984 943 354 773 524 736 183 614 472 764 428 965 881 823 268 170 737 720 455 432 707 263 954 190 848 \
 000  $q^{4216}$  -

44 463 050 607 341 545 690 856 765 003 879 117 926 397 651 389 587 402 536 531 138 690 879 582 841 \
 971 884 844 543 581 085 182 507 615 954 256 556 180 455 773 935 018 730 491 510 299 145 642 639 654 \
 912  $q^{4217}$  +

50 398 951 730 082 782 274 466 737 003 949 527 645 980 895 521 448 370 877 506 356 922 850 995 879 \
 718 429 219 123 372 290 153 118 781 763 294 361 704 756 909 198 985 456 709 079 224 175 592 382 720 \
 000  $q^{4220}$  -

52 548 214 702 810 585 529 547 924 451 038 250 354 487 908 088 686 060 301 387 203 689 732 195 406 \
 875 213 089 228 691 544 732 901 636 638 576 823 217 528 590 599 714 550 207 160 228 833 138 564 643 \
 750  $q^{4221}$  +

59 559 974 426 018 052 959 014 727 288 705 260 843 600 925 843 169 668 869 152 439 628 723 202 339 \
 876 399 607 272 420 943 820 215 611 887 719 740 085 854 983 540 897 311 712 305 096 850 273 304 576 \
 000  $q^{4224}$  -

62 098 684 594 999 336 999 836 121 239 092 809 133 242 150 529 422 866 861 444 967 326 833 168 739 \
 628 664 682 473 458 727 192 595 960 992 841 716 132 962 012 692 823 527 214 921 473 286 715 875 787 \
 000  $q^{4225}$  +

70 380 648 459 138 954 564 448 546 327 449 981 448 205 587 822 157 829 597 614 287 286 858 961 166 \
 035 108 733 655 582 421 473 380 408 069 462 246 679 347 897 216 496 281 111 951 081 319 592 409 104 \
 384  $q^{4228}$  -

73 379 138 775 491 566 782 515 209 748 341 081 963 753 659 147 586 861 870 514 696 098 226 479 275 \
 857 933 999 679 548 052 396 285 164 325 207 817 427 429 442 798 078 875 431 478 579 504 380 013 730 \
 000  $q^{4229}$  +

83 160 642 480 738 148 616 041 191 056 103 844 133 930 369 343 418 471 130 230 063 340 707 729 599 \
 698 939 378 729 516 210 477 864 274 187 959 203 205 195 240 398 927 107 117 851 570 880 562 930 453 \
 760  $q^{4232}$  -

86 701 905 538 282 080 890 924 971 381 648 421 060 814 717 644 010 513 038 278 120 694 739 864 259 \
 310 538 608 504 779 064 295 038 910 186 004 722 217 754 364 104 412 281 678 374 773 446 576 358 359 \
 040  $q^{4233}$  +

98 253 553 653 521 620 651 658 943 714 345 259 109 292 888 009 022 975 519 552 705 936 730 858 387 \
 551 794 929 990 841 030 080 987 997 981 642 383 640 207 831 910 090 173 900 280 845 647 976 355 200 \
 000  $q^{4236}$  -

102 435 512 795 429 208 585 541 754 028 397 426 972 501 279 746 216 734 665 051 586 675 009 845 313 \
 564 655 034 456 964 737 445 508 836 096 917 563 895 510 170 083 057 741 857 080 220 200 846 620 622 \
 171  $q^{4237}$  +

116 076 580 387 742 276 261 341 171 151 342 643 085 569 807 387 533 800 537 090 617 151 093 777 747 \
 329 527 400 216 638 081 738 293 563 069 118 702 124 746 320 980 824 828 517 575 549 318 380 158 976 \
 000  $q^{4240}$  -

121 014 766 890 020 577 998 709 134 878 061 046 259 966 412 831 051 161 159 389 587 727 521 624 289 \
 653 243 560 719 875 138 219 717 319 197 737 478 755 657 965 816 929 596 349 059 843 574 117 609 472 \
 000  $q^{4241}$  +

137 121 924 237 280 776 248 431 928 359 148 098 343 600 103 314 150 741 598 146 260 606 164 560 181 \
 819 962 614 685 989 737 323 206 184 209 385 979 212 350 676 729 449 361 116 705 476 789 065 710 848 \
 000  $q^{4244}$  -

142 952 632 935 097 781 637 729 740 751 713 369 186 565 905 356 534 262 442 050 546 215 966 846 607 \
 827 756 965 005 246 309 893 552 799 769 052 957 080 515 331 599 158 911 348 270 065 631 261 002 704 \
 300  $q^{4245}$  +

161 970 229 045 282 375 449 181 395 366 398 354 718 207 001 211 311 049 581 679 343 988 037 341 616 \
 367 727 371 972 895 074 360 509 720 475 601 435 503 645 293 534 772 238 751 813 106 621 610 927 778

$304 q^{4248} -$   
 168 854 237 621 546 571 951 647 328 750 156 273 024 138 285 758 293 570 562 843 789 639 088 909 521 1  
 708 724 536 998 593 796 862 499 726 167 713 544 967 632 721 992 257 731 458 093 686 691 017 359 360 1  
 $000 q^{4249} +$   
 191 306 420 140 145 419 300 206 685 074 370 112 219 391 159 178 106 027 601 278 244 096 194 605 409 1  
 746 182 850 556 062 646 959 508 661 994 015 186 900 684 505 856 776 897 799 629 831 860 115 385 636 1  
 $864 q^{4252} -$   
 199 433 372 424 554 255 986 456 914 874 928 141 825 821 467 026 329 398 533 663 385 555 039 486 014 1  
 714 845 378 045 705 556 754 157 074 178 717 846 457 121 220 826 084 879 470 885 014 900 101 038 542 1  
 $177 q^{4253} +$   
 225 938 370 777 371 263 231 622 303 086 036 590 013 918 554 915 622 896 566 606 643 715 438 839 725 1  
 875 362 722 789 135 244 057 944 018 689 178 508 109 515 075 474 124 605 292 290 552 831 368 684 544 1  
 $000 q^{4256} -$   
 235 531 942 209 834 466 379 527 854 772 076 882 555 722 787 157 086 540 814 464 711 454 994 242 755 1  
 707 547 694 564 412 498 823 036 156 542 602 260 106 494 170 077 047 747 751 637 279 890 240 015 728 1  
 $640 q^{4257} +$   
 266 818 898 809 273 198 392 503 838 882 364 490 780 265 058 680 247 376 216 382 321 523 539 870 919 1  
 248 117 093 498 425 573 397 233 462 340 584 469 348 268 339 626 143 742 654 222 070 665 904 280 371 1  
 $200 q^{4260} -$   
 278 142 883 176 270 576 985 310 381 157 155 337 822 087 811 668 388 887 031 388 123 839 534 720 129 1  
 223 923 550 467 197 988 651 983 397 915 558 133 150 865 943 222 182 643 418 623 667 951 103 048 888 1  
 $750 q^{4261} +$   
 315 071 685 751 400 355 105 613 840 760 772 218 183 791 173 535 857 031 935 536 839 602 746 841 290 1  
 578 514 697 865 277 737 860 911 025 726 155 255 313 941 669 996 173 485 837 548 802 551 658 244 992 1  
 $000 q^{4264} -$   
 328 437 166 962 507 130 003 889 709 415 481 179 301 591 150 792 924 610 458 744 524 927 441 907 900 1  
 516 941 666 840 484 788 190 936 092 382 861 624 276 364 247 682 049 354 461 135 005 403 998 170 316 1  
 $800 q^{4265} +$   
 372 021 815 363 342 909 597 712 850 168 420 081 434 109 832 988 068 634 060 581 642 619 120 285 220 1  
 688 035 768 191 171 695 874 440 645 316 522 661 052 584 467 025 472 497 117 878 357 970 101 306 107 1  
 $904 q^{4268} -$   
 387 795 617 050 419 517 070 680 859 127 089 267 629 241 165 661 471 932 933 552 762 518 850 220 736 1  
 367 496 679 263 551 398 465 794 932 685 754 871 532 278 881 094 030 648 996 509 175 155 485 894 960 1  
 $750 q^{4269} +$   
 439 231 752 348 740 605 018 823 838 021 435 183 123 919 056 620 380 086 007 182 991 042 709 506 781 1  
 801 445 079 006 447 460 765 716 824 260 409 980 750 490 134 130 545 378 857 395 919 881 280 421 158 1  
 $912 q^{4272} -$   
 457 846 392 209 298 646 055 946 406 821 993 466 854 356 013 806 684 492 695 711 369 212 766 511 756 1  
 212 630 426 409 739 018 303 141 603 579 178 598 230 755 676 496 005 673 208 703 062 912 649 762 111 1  
 $488 q^{4273} +$   
 518 543 727 068 644 087 346 582 416 467 456 231 927 116 087 986 528 270 806 614 677 392 805 396 822 1  
 055 145 377 795 378 513 651 115 103 600 777 382 881 593 541 566 019 040 291 485 048 812 359 719 680 1  
 $000 q^{4276} -$   
 540 509 143 039 470 511 905 421 145 772 569 751 383 949 597 714 436 647 379 683 842 053 159 111 491 1  
 218 557 691 323 234 306 226 367 167 186 371 499 399 826 605 847 551 338 997 547 400 797 270 751 303 1  
 $008 q^{4277} +$   
 612 129 663 090 430 403 516 443 873 497 856 186 668 936 671 038 810 274 871 948 167 610 874 349 818 1  
 071 932 078 938 470 929 603 666 668 741 394 792 179 501 086 615 883 449 942 328 974 419 925 463 680 1  
 $000 q^{4280} -$   
 638 047 025 687 681 194 821 628 989 545 160 938 817 834 014 369 950 088 539 064 221 030 200 969 096 1  
 239 774 746 267 188 943 616 665 796 124 574 269 899 436 646 673 720 702 821 720 835 782 389 805 056 1  
 $000 q^{4281} +$   
 722 549 985 470 697 499 740 261 795 091 753 720 807 223 732 743 956 500 770 570 729 976 981 861 585 1  
 763 025 570 631 094 116 664 412 484 657 676 815 263 298 963 420 797 774 721 514 848 381 535 195 648 1  
 $000 q^{4284} -$

753 127 966 214 221 515 200 090 198 242 184 566 242 445 407 299 471 682 239 287 559 814 612 231 966  
 847 274 517 247 664 012 677 084 433 370 039 199 699 485 609 974 376 965 207 468 075 427 057 313 802  
 250  $q^{4285} +$

852 822 884 194 929 919 185 483 053 870 216 518 487 261 843 628 712 391 881 534 828 823 284 320 867  
 782 496 687 321 196 213 666 700 806 285 058 704 858 780 159 172 280 897 321 398 232 170 243 056 631  
 808  $q^{4288} -$

888 896 815 411 753 561 741 410 157 730 236 216 840 473 925 043 371 563 345 911 149 400 972 694 857  
 275 329 437 782 490 403 649 498 042 210 875 035 963 485 948 931 051 730 437 962 101 828 470 489 088  
 000  $q^{4289} +$

1 006 505 885 397 861 955 702 760 648 822 909 397 414 894 730 923 780 160 740 833 517 734 435 350 312  
 908 114 899 855 308 841 835 414 550 958 736 282 906 363 070 430 024 673 048 700 566 626 476 589 875  
 200  $q^{4292} -$

1 049 060 323 593 233 511 556 119 330 310 152 610 312 845 661 756 208 851 270 461 154 800 929 755 012  
 224 685 674 532 741 560 492 832 527 091 356 347 996 288 758 823 712 276 725 816 168 594 543 680 849  
 986  $q^{4293} +$

1 187 791 910 185 819 107 961 471 802 678 225 796 102 545 332 247 798 398 736 489 856 895 552 127 541  
 649 636 547 871 571 509 124 941 356 002 631 430 652 633 130 433 849 045 693 077 836 902 765 701 376  
 000  $q^{4296} -$

1 237 987 205 601 910 497 393 204 489 536 838 542 717 457 665 953 207 835 029 124 094 606 739 842 023  
 625 810 430 404 642 338 837 380 239 250 121 871 984 346 385 995 576 389 229 370 824 195 363 576 381  
 440  $q^{4297} +$

1 401 622 385 676 589 179 423 355 682 979 431 411 144 101 113 137 286 862 846 642 817 275 216 541 852  
 583 592 659 737 602 925 996 945 703 067 198 414 082 450 307 148 659 059 181 962 738 146 410 720 499  
 200  $q^{4300} -$

1 460 825 967 004 640 196 523 081 001 879 469 295 497 080 284 591 576 070 420 093 404 392 519 780 024  
 987 168 146 447 690 595 487 462 403 458 307 724 186 729 001 631 905 550 638 884 918 359 116 344 187  
 125  $q^{4301} +$

1 653 820 425 369 036 145 350 661 403 841 353 143 825 562 328 759 971 006 398 830 355 028 065 449 271  
 066 968 102 065 022 095 126 698 984 957 921 393 057 038 823 595 834 024 648 273 481 759 833 253 888  
 000  $q^{4304} -$

1 723 643 633 631 698 195 036 241 982 288 603 417 010 244 309 304 296 961 964 648 285 097 586 579 641  
 307 437 797 736 631 254 836 024 088 868 324 135 759 338 767 498 984 296 850 972 796 598 312 363 622  
 400  $q^{4305} +$

1 951 247 628 026 389 308 095 874 567 751 538 528 505 792 799 268 769 329 794 532 328 450 078 317 882  
 408 676 936 043 073 796 528 791 481 358 347 058 870 943 049 314 205 703 998 753 023 918 689 613 914  
 112  $q^{4308} -$

2 033 589 080 682 558 897 079 200 252 332 674 898 302 113 033 771 070 210 042 352 054 160 454 479 631  
 876 277 910 373 232 912 055 693 599 323 827 834 081 333 038 320 732 694 603 799 449 760 835 125 600  
 750  $q^{4309} +$

2 301 988 669 851 795 824 258 280 038 010 101 256 317 389 051 124 959 109 732 756 726 608 247 354 204  
 746 525 394 127 787 532 540 776 632 080 888 680 937 405 500 218 527 367 240 422 419 321 074 718 060  
 032  $q^{4312} -$

2 399 085 309 048 609 420 391 345 825 595 116 075 061 139 789 907 719 974 219 665 732 407 459 673 917  
 188 741 113 998 998 210 386 730 843 433 121 287 907 166 761 114 335 916 931 898 211 845 644 726 992  
 896  $q^{4313} +$

2 715 568 600 236 940 103 204 207 871 917 650 983 224 073 902 852 018 535 586 432 241 698 886 292 943  
 209 281 648 222 962 082 360 531 606 170 463 292 388 170 429 908 621 278 089 166 485 332 771 351 808  
 000  $q^{4316} -$

2 830 055 782 367 925 454 305 168 264 552 873 249 855 212 688 463 961 722 232 549 334 218 981 223 217  
 727 167 935 727 424 240 634 157 741 427 322 712 017 935 274 261 863 403 346 074 972 062 623 690 657  
 032  $q^{4317} +$

3 203 208 616 019 988 385 121 906 306 110 451 594 558 554 569 770 061 366 058 697 067 594 182 609 815  
 947 059 081 144 682 017 786 834 986 006 713 158 261 350 476 236 591 840 060 644 888 954 055 469 465  
 600  $q^{4320} -$

3 338 190 838 659 655 281 967 712 275 765 207 081 509 247 260 871 262 588 916 424 774 767 194 848 904

881 160 714 207 079 161 777 355 160 780 204 660 983 896 105 836 380 446 405 564 495 873 666 236 416 000  $q^{4321}$  +  
 3 778 127 105 602 499 996 297 069 471 253 257 414 774 633 863 740 561 486 459 433 309 062 779 024 934 293 245 526 945 446 049 989 326 596 370 955 473 857 347 118 687 654 318 438 050 393 758 609 334 272 000  $q^{4324}$  -  
 3 937 261 248 718 298 804 529 072 578 983 358 339 697 898 966 962 191 283 293 819 230 649 362 633 128 512 843 310 567 676 599 376 491 837 419 314 951 996 624 841 590 560 202 054 878 563 756 012 460 267 225  $q^{4325}$  +  
 4 455 893 948 994 292 785 810 407 165 545 052 280 264 451 880 357 422 022 053 377 398 790 604 597 491 268 782 566 252 423 589 568 356 533 079 844 853 661 756 815 996 777 528 953 186 918 105 237 609 431 552  $q^{4328}$  -  
 4 643 487 237 417 913 786 678 177 153 719 280 580 404 440 211 592 961 079 003 710 436 795 508 484 170 382 310 971 218 315 717 814 650 983 106 704 485 532 197 071 608 220 033 164 337 302 769 743 626 240 000  $q^{4329}$  +  
 5 254 847 464 057 593 433 370 982 592 503 089 955 737 361 110 758 266 926 021 399 771 464 053 330 782 643 412 385 263 894 161 537 814 405 991 961 967 565 765 494 733 451 086 075 024 444 822 738 703 131 136  $q^{4332}$  -  
 5 475 972 746 137 948 957 358 747 849 496 833 083 900 598 387 356 090 187 844 347 353 833 044 288 613 239 583 084 827 982 472 035 279 822 180 091 032 019 652 975 168 693 820 421 763 675 453 545 081 603 224  $q^{4333}$  +  
 6 196 585 039 517 661 099 857 253 741 516 132 726 562 270 088 081 554 469 003 310 843 675 580 208 353 187 763 786 414 775 828 071 083 806 983 187 162 534 335 423 495 803 296 051 147 120 863 792 279 552 000  $q^{4336}$  -  
 6 457 216 432 786 413 264 741 237 168 712 589 647 592 942 905 215 480 101 116 840 255 132 498 059 008 989 059 337 247 844 772 269 622 239 586 867 585 357 266 633 537 155 863 595 525 980 233 571 857 235 968  $q^{4337}$  +  
 7 306 540 434 684 283 960 196 377 316 647 807 136 066 049 325 877 696 738 376 735 726 046 443 812 842 457 226 561 814 894 697 428 673 079 586 316 990 904 152 981 914 743 921 263 746 489 910 818 037 760 000  $q^{4340}$  -  
 7 613 712 925 110 651 465 087 392 899 689 470 089 137 161 931 416 531 535 950 209 207 879 562 189 728 698 282 726 388 641 833 749 858 080 336 415 859 766 228 540 226 660 303 984 570 181 036 294 666 624 625  $q^{4341}$  +  
 8 614 663 004 759 526 354 448 054 186 881 796 708 416 848 190 926 632 693 022 786 024 602 326 347 810 413 930 182 935 447 040 428 677 628 787 160 685 984 741 014 502 742 962 315 097 803 245 625 664 384 000  $q^{4344}$  -  
 8 976 660 215 689 443 784 529 230 522 807 306 523 786 645 379 386 985 149 007 813 876 082 451 219 590 594 817 012 937 153 968 391 778 024 376 752 001 539 342 684 556 652 720 828 344 901 778 153 979 904 000  $q^{4345}$  +  
 10 156 216 788 347 709 369 777 929 665 650 220 828 923 735 551 927 230 133 061 940 154 136 838 830 934 643 796 540 864 723 304 336 966 072 503 378 864 410 596 332 490 918 876 298 592 666 626 255 438 757 888  $q^{4348}$  -  
 10 582 791 874 872 676 215 440 500 181 661 096 622 298 793 734 272 415 377 542 820 513 153 726 972 661 605 206 742 364 969 933 419 925 093 820 103 219 896 633 525 429 055 570 861 116 748 975 956 657 157 875  $q^{4349}$  +  
 11 972 720 539 896 685 026 992 022 862 754 436 182 245 410 069 364 035 476 548 530 775 307 855 368 961 272 886 554 984 080 113 976 844 232 495 175 914 891 757 250 271 885 675 333 850 217 083 295 456 296 960  $q^{4352}$  -  
 12 475 356 033 384 008 894 138 057 332 204 463 136 944 470 459 655 836 271 594 498 569 082 512 055 167 188 689 820 629 145 048 740 475 571 347 541 400 601 380 113 932 150 390 712 132 856 279 103 332 515 840  $q^{4353}$  +  
 14 113 053 485 941 788 337 191 337 831 369 944 357 367 009 880 244 581 601 222 462 465 987 697 095 947 189 301 745 136 703 495 389 890 321 674 082 286 231 341 803 718 019 593 227 673 557 602 267 881 498 752  $q^{4356}$  -  
 14 705 266 934 322 352 945 798 544 158 633 782 387 046 681 509 733 895 295 375 248 241 504 350 628 380 982 859 385 172 821 562 284 953 717 087 107 116 686 373 306 350 188 853 995 795 727 711 361 993

$866\,458 q^{4357} +$   
 16 634 755 926 041 863 886 203 888 422 414 965 877 659 249 719 721 512 993 582 815 706 989 086 717 \ \backslash  
 513 985 041 152 834 734 035 064 361 107 470 313 697 465 346 359 292 823 230 757 365 862 078 506 468 \ \backslash  
 $121\,600 q^{4360} -$   
 17 332 459 374 651 995 410 970 991 349 904 646 502 815 902 237 198 757 664 254 410 166 222 191 847 \ \backslash  
 000 592 893 125 935 633 189 006 024 024 281 704 068 351 682 683 203 258 952 441 461 509 199 975 469 \ \backslash  
 $056\,000 q^{4361} +$   
 19 605 558 899 684 293 295 111 929 089 787 683 815 109 140 552 573 386 566 648 799 751 695 640 350 \ \backslash  
 706 302 644 071 080 147 846 304 651 126 753 654 400 482 824 990 438 299 629 325 978 150 417 690 403 \ \backslash  
 $392\,000 q^{4364} -$   
 20 427 481 666 046 789 923 658 233 116 378 719 150 690 486 123 814 968 365 054 424 064 819 619 371 \ \backslash  
 468 323 455 476 668 767 345 140 198 025 289 766 047 078 309 261 020 380 072 416 942 553 159 145 352 \ \backslash  
 $723\,775 q^{4365} +$   
 23 105 183 131 216 234 686 197 924 693 919 735 932 963 673 891 304 947 483 113 964 751 720 988 829 \ \backslash  
 095 346 082 482 950 352 643 967 272 650 617 309 463 419 919 969 898 692 196 120 075 578 140 736 668 \ \backslash  
 $565\,504 q^{4368} -$   
 24 073 368 981 563 367 703 185 732 340 090 711 213 422 357 764 304 320 042 353 474 737 302 803 246 \ \backslash  
 698 478 929 592 249 295 598 391 575 162 853 890 379 322 965 359 561 387 721 614 310 426 142 083 891 \ \backslash  
 $200\,000 q^{4369} +$   
 27 227 454 500 964 306 848 913 290 607 681 482 872 269 761 980 712 441 251 148 591 460 844 315 897 \ \backslash  
 714 604 023 376 489 313 655 331 581 915 991 533 114 665 069 210 426 789 306 219 176 024 547 333 143 \ \backslash  
 $021\,568 q^{4372} -$   
 28 367 846 279 315 231 504 941 843 595 505 682 595 537 799 459 351 911 954 152 540 768 876 880 598 \ \backslash  
 184 955 162 111 155 855 013 137 258 780 916 418 447 929 445 896 250 400 281 790 766 739 069 424 166 \ \backslash  
 $147\,508 q^{4373} +$   
 32 082 791 553 937 619 224 283 052 899 136 746 195 555 407 189 033 904 264 943 772 653 092 437 146 \ \backslash  
 000 995 873 525 254 416 883 628 092 198 659 889 861 239 117 808 868 764 001 508 905 727 505 648 088 \ \backslash  
 $256\,000 q^{4376} -$   
 33 425 918 596 321 217 319 273 118 142 904 393 640 280 203 029 405 619 387 662 552 714 549 676 837 \ \backslash  
 943 332 858 037 406 668 191 738 844 614 726 967 212 383 312 295 159 197 275 960 891 315 445 834 807 \ \backslash  
 $214\,080 q^{4377} +$   
 37 801 130 261 188 435 887 781 447 084 867 478 153 547 457 151 486 087 792 979 092 335 480 567 966 \ \backslash  
 599 202 581 170 929 655 793 259 341 845 457 232 290 244 672 357 108 799 543 991 665 216 211 330 727 \ \backslash  
 $014\,400 q^{4380} -$   
 39 382 916 607 023 021 096 321 135 609 237 966 298 570 856 854 164 057 206 340 555 044 658 266 817 \ \backslash  
 662 221 817 997 027 989 461 058 354 700 320 333 929 584 955 517 547 523 902 473 131 510 934 168 584 \ \backslash  
 $526\,500 q^{4381} +$   
 44 535 362 643 311 752 127 304 819 994 478 230 577 037 207 305 589 113 005 962 854 783 206 123 516 \ \backslash  
 273 585 500 548 125 820 746 985 692 708 529 084 676 196 243 307 351 102 548 260 523 171 887 779 521 \ \backslash  
 $536\,000 q^{4384} -$   
 46 398 077 202 086 079 409 076 242 228 732 538 737 583 843 570 773 532 722 196 969 708 273 984 577 \ \backslash  
 989 391 785 025 021 409 385 654 495 689 373 546 716 260 970 248 204 178 210 397 170 320 053 115 686 \ \backslash  
 $092\,800 q^{4385} +$   
 52 465 379 244 325 893 943 236 803 042 182 302 346 756 496 339 701 481 525 948 349 497 716 886 023 \ \backslash  
 332 214 283 356 491 394 277 730 647 250 317 049 192 101 596 752 264 014 848 616 820 598 608 402 556 \ \backslash  
 $993\,536 q^{4388} -$   
 54 658 752 769 600 932 024 571 745 319 731 689 065 466 554 756 456 476 802 321 468 888 119 922 957 \ \backslash  
 925 645 329 079 691 758 720 243 590 523 096 155 209 583 060 115 706 040 784 753 577 952 427 617 731 \ \backslash  
 $694\,875 q^{4389} +$   
 61 802 821 151 744 949 436 816 441 205 416 648 337 070 316 952 125 308 922 091 809 631 491 651 097 \ \backslash  
 660 609 669 158 031 914 372 551 238 000 315 907 139 347 072 319 405 198 851 807 208 230 221 789 759 \ \backslash  
 $738\,368 q^{4392} -$   
 64 385 359 211 164 674 465 362 577 975 638 210 062 015 796 189 011 135 521 039 421 132 736 354 625 \ \backslash  
 645 635 650 166 724 363 003 752 844 743 264 409 203 739 534 682 937 444 435 795 913 498 383 180 345 \ \backslash  
 $573\,376 q^{4393} +$

72 796 665 699 082 102 906 054 748 664 267 433 031 040 920 475 921 227 203 663 543 630 018 502 901  
 392 212 850 177 275 028 219 599 307 581 019 723 969 891 414 626 633 972 227 721 260 112 269 091 134  
 336 000  $q^{4396}$  -

75 837 191 920 037 020 666 439 881 939 691 361 947 750 892 149 777 735 005 015 833 309 336 772 304  
 514 757 695 805 719 409 084 212 989 814 300 423 023 086 833 981 609 746 781 202 010 351 884 822 579  
 043 772  $q^{4397}$  +

85 739 791 634 238 269 170 775 457 476 991 807 149 830 634 298 436 245 075 833 155 509 251 188 941  
 706 610 683 450 869 901 935 714 454 839 210 441 737 802 980 283 299 935 711 647 295 651 637 064 816  
 537 600  $q^{4400}$  -

89 319 261 480 836 015 618 860 721 228 762 285 776 891 791 698 534 504 942 920 983 522 886 366 480  
 466 161 804 092 454 915 613 534 853 878 316 652 873 095 129 478 087 400 821 629 857 051 519 193 956  
 352 000  $q^{4401}$  +

100 976 694 947 081 058 982 433 329 519 665 635 033 274 497 316 252 715 547 525 207 042 493 763 257  
 267 916 035 358 914 645 980 104 422 656 263 112 365 870 142 275 490 071 221 529 270 645 288 933 774  
 848 000  $q^{4404}$  -

105 190 327 298 510 180 224 464 490 208 722 894 813 362 331 952 091 683 532 895 826 066 488 880 819  
 404 080 295 946 530 453 288 496 785 787 760 759 970 198 165 622 124 477 170 880 492 366 427 244 943  
 713 250  $q^{4405}$  +

118 912 556 373 888 489 358 764 053 767 023 104 042 088 557 650 844 650 327 997 342 875 746 885 134  
 906 982 291 895 437 944 478 326 866 273 627 964 286 595 250 137 707 338 827 659 663 610 697 267 627  
 332 608  $q^{4408}$  -

123 872 338 406 969 908 830 521 502 756 160 398 556 013 519 402 553 547 661 761 205 945 832 490 082  
 284 351 456 848 392 216 254 335 165 668 781 956 397 549 308 923 367 696 965 859 877 533 741 708 120  
 064 000  $q^{4409}$  +

140 023 896 599 677 044 449 787 057 368 577 491 916 205 974 500 611 935 800 716 151 850 005 354 792  
 899 349 713 137 964 461 562 677 552 620 625 585 802 893 479 919 841 176 980 530 754 366 069 910 720  
 823 296  $q^{4412}$  -

145 861 527 140 288 465 072 363 230 358 930 516 795 752 338 149 965 148 462 503 326 612 003 814 780  
 783 428 653 569 913 200 558 259 079 563 659 489 097 545 898 237 963 053 289 278 214 581 607 260 957  
 717 146  $q^{4413}$  +

164 871 096 258 162 667 256 606 158 255 206 688 565 807 753 098 164 884 498 083 623 324 141 178 983  
 684 186 957 205 932 758 213 974 651 391 792 968 505 714 295 518 890 741 630 091 975 577 653 959 917  
 568 000  $q^{4416}$  -

171 741 444 104 593 141 746 611 330 701 620 090 363 898 393 709 436 854 159 871 987 453 956 454 055  
 171 256 556 050 692 906 345 936 110 725 945 662 223 557 999 581 994 169 266 207 381 060 355 165 312  
 974 848  $q^{4417}$  +

194 113 106 034 276 820 082 614 847 916 868 188 038 892 866 785 291 639 208 275 072 482 196 739 447  
 417 043 566 436 189 125 169 125 748 275 925 872 290 575 058 278 698 443 114 341 111 712 391 760 627  
 302 400  $q^{4420}$  -

202 198 273 060 373 664 332 072 943 287 822 655 897 005 162 777 843 513 336 524 872 933 774 620 583  
 567 971 950 365 027 157 215 257 131 500 765 418 214 799 234 616 178 158 689 376 001 883 362 564 129  
 598 375  $q^{4421}$  +

228 524 728 738 086 606 032 756 973 725 142 378 289 162 414 761 789 473 208 703 283 748 161 188 438  
 172 971 785 672 991 866 063 364 648 600 248 759 404 174 473 754 601 132 980 947 145 355 203 590 118  
 400 000  $q^{4424}$  -

238 038 823 195 231 952 357 835 016 908 330 162 476 779 755 299 490 576 626 293 645 051 310 033 409  
 950 882 521 365 166 501 732 363 162 921 467 479 972 418 711 732 456 515 171 101 869 762 251 931 794  
 636 800  $q^{4425}$  +

269 016 921 586 358 475 592 619 654 621 879 408 690 766 257 900 983 157 733 985 290 141 449 979 429  
 529 151 707 220 192 822 298 634 190 483 226 530 034 143 088 330 088 414 993 449 881 024 261 520 887  
 132 160  $q^{4428}$  -

280 211 665 339 370 051 223 382 988 019 317 141 826 185 617 115 600 851 774 117 611 467 314 304 144  
 813 207 812 326 594 746 299 508 795 702 061 590 687 986 412 871 362 853 350 177 975 737 563 923 321  
 302 875  $q^{4429}$  +

316 660 644 792 462 588 417 171 514 690 736 973 889 363 421 609 991 622 068 379 760 703 361 928 215



$059456 q^{4468} -$   
1 426 012 575 560 988 881 891 951 205 318 831 245 272 042 558 772 869 544 097 184 223 984 740 840 270 651 590 611 737 976 281 616 909 297 835 485 879 563 595 578 115 122 919 608 746 131 277 424 704 245 238 750  $q^{4469} +$   
1 610 622 515 143 011 686 931 572 065 809 374 472 975 250 534 526 396 825 671 914 298 594 102 419 856 838 374 944 632 144 475 600 037 408 771 443 848 823 338 059 419 840 956 263 376 323 684 583 942 232 364 032  $q^{4472} -$   
1 677 309 882 536 645 120 256 074 717 837 495 248 033 637 665 217 203 226 005 483 016 578 525 391 020 509 303 831 412 594 788 146 300 351 147 836 971 524 864 242 084 092 762 264 067 473 640 578 776 512 659 456  $q^{4473} +$   
1 894 349 659 280 515 098 317 298 757 180 996 787 764 468 999 927 194 713 473 833 778 702 461 007 804 074 664 271 756 308 002 523 117 322 133 933 047 702 309 326 959 292 773 846 640 478 469 258 291 098 880 000  $q^{4476} -$   
1 972 749 000 597 760 053 631 118 286 526 958 469 418 657 569 072 816 051 484 734 843 458 887 289 264 934 100 487 683 543 399 188 761 732 124 815 010 777 383 421 521 954 444 216 911 510 960 124 995 461 955 767  $q^{4477} +$   
2 227 897 108 890 874 496 677 979 783 312 693 079 954 786 507 147 713 800 486 453 219 075 422 900 815 246 061 734 668 888 596 962 786 856 424 843 335 907 256 073 523 698 725 092 494 514 649 893 046 221 209 600  $q^{4480} -$   
2 320 058 716 139 379 350 739 920 773 083 259 939 396 491 509 971 290 935 215 205 862 445 619 779 215 685 973 418 129 802 840 828 724 290 032 104 491 463 970 447 002 413 699 025 844 409 297 618 167 201 792 000  $q^{4481} +$   
2 619 984 759 314 194 911 393 094 045 792 105 440 050 807 089 467 736 271 091 576 381 445 232 898 702 482 844 184 991 351 327 281 403 045 862 054 847 132 551 272 570 324 161 295 788 744 694 787 207 444 480 000  $q^{4484} -$   
2 728 316 692 470 512 225 963 968 073 496 240 421 047 670 565 146 101 820 869 866 253 038 401 629 882 958 262 625 674 955 152 149 807 150 544 024 110 812 731 301 668 721 088 844 801 700 355 803 500 925 757 050  $q^{4485} +$   
3 080 853 811 831 367 611 556 170 490 290 025 790 541 655 246 691 751 937 982 944 040 071 512 272 636 140 169 011 456 820 344 816 480 493 099 246 090 956 250 659 864 268 976 400 078 493 179 993 921 275 088 896  $q^{4488} -$   
3 208 184 127 197 362 195 757 991 227 251 518 869 008 494 145 712 177 409 105 942 655 200 514 646 775 424 175 519 101 098 081 631 284 206 328 441 846 003 796 962 076 660 015 302 514 259 720 203 845 439 488 248  $q^{4489} +$   
3 622 531 333 111 965 994 548 238 188 482 618 431 464 797 984 282 322 288 469 096 541 420 185 867 225 007 995 565 936 919 767 029 193 568 108 136 586 703 241 287 600 561 633 187 647 160 101 478 679 033 221 632  $q^{4492} -$   
3 772 181 100 576 364 681 589 459 247 362 997 356 797 125 268 193 116 075 882 714 192 180 965 232 491 150 205 148 609 628 905 524 248 619 491 912 701 090 517 693 662 546 497 520 168 329 607 309 667 262 353 267  $q^{4493} +$   
4 259 140 674 492 699 867 835 871 395 556 901 375 255 164 884 700 891 989 203 937 099 172 935 189 431 007 439 190 867 678 266 572 965 637 600 991 958 937 922 728 661 287 153 044 223 266 913 891 630 694 400 000  $q^{4496} -$   
4 435 009 648 228 860 530 046 959 789 131 826 468 031 767 883 657 326 970 359 590 234 611 763 734 596 689 741 499 390 601 235 044 486 805 641 734 631 240 971 158 235 970 551 566 889 825 773 795 492 950 212 608  $q^{4497} +$   
5 007 265 675 098 150 833 757 097 654 188 143 619 706 416 698 219 371 147 389 109 830 436 873 085 490 629 014 378 718 733 429 650 398 184 442 614 042 601 367 478 979 751 305 076 833 036 754 616 272 930 099 200  $q^{4500} -$   
5 213 932 803 422 172 070 899 144 557 026 328 697 792 260 045 037 556 674 042 935 715 985 170 186 022 916 122 035 208 290 966 033 318 316 363 773 556 547 012 573 920 812 788 114 636 883 182 122 608 296 566 875  $q^{4501} +$   
5 886 377 937 594 448 005 193 885 150 940 991 214 093 527 213 791 915 566 518 300 620 736 796 406 249 130 001 930 053 213 561 318 296 475 268 270 383 271 783 556 236 666 956 903 552 783 485 679 464 988 480 000  $q^{4504} -$

6 129 219 274 053 632 590 032 725 559 605 182 309 084 192 482 050 149 216 193 393 230 989 854 925 186 \
 522 477 384 026 767 878 606 825 305 651 513 967 919 367 989 300 838 805 121 023 024 919 194 597 280 \
 972 800  $q^{4505} +$

6 919 338 064 452 393 294 196 983 135 851 837 156 659 014 408 841 274 602 575 044 139 334 406 059 464 \
 054 225 398 335 276 524 491 904 208 952 416 392 438 924 179 416 800 499 245 644 254 250 976 204 480 \
 595 968  $q^{4508} -$

7 204 665 083 152 907 467 891 424 409 242 015 248 537 241 553 053 784 369 986 639 010 377 457 379 596 \
 381 726 178 687 101 737 797 569 619 412 337 757 767 247 542 859 381 784 034 787 829 141 323 864 468 \
 912 500  $q^{4509} +$

8 132 983 616 086 554 989 591 096 544 229 245 555 992 410 836 946 282 632 919 336 477 674 502 234 504 \
 386 825 433 475 379 314 836 832 364 048 241 571 483 255 338 646 408 856 619 198 087 589 684 591 298 \
 625 536  $q^{4512} -$

8 468 205 450 851 596 638 356 034 534 709 991 787 496 948 452 121 244 097 070 312 963 868 925 971 906 \
 303 720 076 177 341 281 329 112 578 800 961 842 783 458 202 587 065 531 201 442 215 582 859 662 252 \
 244 992  $q^{4513} +$

9 558 818 747 068 193 940 947 588 032 753 448 078 325 958 113 253 643 376 053 590 568 311 579 981 821 \
 845 025 157 551 530 424 258 156 156 740 696 212 692 850 126 202 758 958 470 850 539 109 589 462 712 \
 320 000  $q^{4516} -$

9 952 632 479 179 330 090 856 092 394 700 394 941 655 448 955 354 044 244 979 505 964 453 795 172 832 \
 509 486 830 277 039 567 296 968 267 309 686 240 114 160 749 630 314 210 053 454 436 256 872 600 821 \
 760 920  $q^{4517} +$

11 233 823 047 722 723 792 225 293 689 974 423 884 841 087 103 727 840 692 449 426 397 472 285 658 \
 856 957 490 934 180 443 534 623 567 881 098 365 627 479 781 571 863 851 956 070 962 443 356 060 951 \
 928 550 400  $q^{4520} -$

11 696 436 875 877 396 686 078 551 549 161 049 233 457 435 314 082 672 049 685 007 865 068 156 840 \
 907 520 124 858 173 919 705 979 960 462 950 233 875 987 402 565 261 519 578 655 949 248 989 115 987 \
 664 896 000  $q^{4521} +$

13 201 400 130 120 047 848 506 177 835 380 061 872 275 578 902 788 121 625 588 844 125 421 824 121 \
 532 402 100 023 002 363 694 304 474 306 879 904 853 343 711 133 221 892 811 803 369 375 788 457 485 \
 294 080 000  $q^{4524} -$

13 744 795 086 557 207 207 309 155 448 919 665 511 518 584 344 878 507 277 173 101 510 709 722 561 \
 016 717 401 396 249 782 427 620 619 022 672 310 742 685 910 972 358 984 832 951 510 255 796 479 337 \
 432 811 350  $q^{4525} +$

15 512 490 025 005 644 424 226 663 782 994 506 136 218 617 494 698 461 051 244 652 880 323 413 752 \
 584 119 670 817 443 631 908 325 291 794 459 311 437 539 479 225 128 637 539 538 448 394 207 072 552 \
 180 256 768  $q^{4528} -$

16 150 726 874 246 266 124 685 224 281 972 392 214 225 659 527 748 205 194 887 211 243 648 123 980 \
 557 026 423 942 929 550 629 715 423 909 489 744 338 529 631 274 409 914 014 304 642 679 609 524 473 \
 675 776 000  $q^{4529} +$

18 226 873 587 672 511 341 016 207 541 307 430 908 022 497 459 346 609 990 118 871 177 835 195 388 \
 542 248 313 747 607 548 298 201 988 300 067 538 534 796 673 175 149 335 878 110 270 206 138 884 253 \
 928 304 640  $q^{4532} -$

18 976 452 683 259 477 780 148 370 286 342 351 768 270 670 544 016 333 062 953 333 062 717 147 022 \
 383 780 386 551 904 275 281 703 466 797 564 639 887 415 653 925 065 127 385 816 502 399 180 225 025 \
 368 457 745  $q^{4533} +$

21 414 701 949 198 370 068 493 444 337 146 162 602 621 878 036 756 976 413 660 958 726 876 445 871 \
 571 135 830 145 658 154 141 604 260 785 739 018 267 618 440 341 211 504 122 965 525 695 045 636 060 \
 483 200 000  $q^{4536} -$

22 294 985 157 596 651 172 037 581 684 168 980 337 555 398 164 304 654 080 066 860 835 913 602 753 \
 704 958 210 584 055 115 147 281 404 626 801 914 191 885 555 778 379 429 161 816 354 790 688 974 853 \
 715 329 024  $q^{4537} +$

25 158 289 715 459 447 903 667 838 921 783 735 870 876 943 668 710 464 397 317 439 752 541 616 892 \
 536 187 881 538 981 614 412 493 161 806 561 630 878 800 105 588 573 677 028 047 201 130 046 399 613 \
 170 124 800  $q^{4540} -$

26 191 995 078 117 561 509 490 668 673 047 248 421 840 119 837 046 029 657 183 094 734 910 114 993 \

363 943 336 006 131 280 642 821 650 238 877 061 064 789 281 580 774 740 263 530 301 983 178 117 895 \
 852 056 375  $q^{4541}$  +

29 554 217 250 976 212 806 527 759 931 314 382 739 687 551 446 628 500 710 793 983 119 093 910 095 \
 084 567 767 871 777 820 946 380 092 426 324 661 000 790 897 115 878 707 065 404 048 920 447 278 180 \
 548 608 000  $q^{4544}$  -

30 767 998 884 325 977 452 415 665 078 948 276 298 394 643 701 881 508 233 252 822 167 451 583 831 \
 993 753 754 932 554 797 904 980 198 694 475 477 876 588 684 946 370 426 815 202 093 073 713 678 621 \
 106 176 000  $q^{4545}$  +

34 715 795 153 021 232 792 038 505 844 934 068 227 433 299 310 859 614 631 200 059 995 914 211 265 \
 126 656 374 949 931 632 457 338 124 480 816 293 149 200 329 699 770 077 345 368 488 729 786 619 667 \
 766 788 096  $q^{4548}$  -

36 140 923 027 381 789 188 294 658 262 531 108 006 813 181 829 057 531 278 162 669 108 168 955 907 \
 576 115 877 261 918 789 602 316 553 877 056 809 319 030 298 510 301 670 034 876 510 828 106 023 123 \
 254 474 250  $q^{4549}$  +

40 775 953 116 639 844 956 631 785 093 940 618 645 827 435 043 819 374 733 241 043 351 765 712 631 \
 638 095 251 886 132 626 740 728 796 337 975 398 268 755 912 054 556 919 312 757 181 546 677 012 542 \
 767 754 240  $q^{4552}$  -

42 449 109 861 793 814 779 225 576 962 190 665 009 867 064 740 513 365 031 917 802 845 436 599 039 \
 465 378 191 763 959 955 430 461 246 958 581 918 432 318 551 749 348 885 103 557 144 820 517 549 879 \
 350 001 664  $q^{4553}$  +

47 890 626 039 205 172 087 313 202 619 374 447 852 316 568 242 083 271 988 523 897 891 156 737 280 \
 098 430 941 771 784 960 754 431 782 813 160 731 915 851 327 652 394 003 789 825 272 580 528 871 484 \
 876 288 000  $q^{4556}$  -

49 854 840 859 060 096 108 685 240 090 652 854 918 148 023 499 802 295 310 862 422 706 616 568 069 \
 357 542 765 609 492 067 024 650 854 303 705 944 403 507 950 522 905 943 164 165 528 512 472 623 671 \
 953 065 239  $q^{4557}$  +

56 242 722 678 094 240 219 151 443 901 514 073 063 084 235 768 624 291 741 111 863 925 173 268 200 \
 237 562 802 479 913 990 892 727 935 064 133 738 636 585 772 352 646 590 409 656 622 619 295 256 851 \
 100 467 200  $q^{4560}$  -

58 548 465 892 119 996 715 937 335 641 495 510 843 611 474 647 909 697 149 619 732 342 967 357 516 \
 266 299 649 128 595 674 218 367 940 138 920 036 805 398 088 420 397 457 843 685 271 442 790 363 577 \
 126 912 000  $q^{4561}$  +

66 046 776 766 101 026 297 994 173 819 017 267 148 388 076 247 815 979 774 183 364 791 205 393 980 \
 985 355 125 641 940 095 705 739 351 493 453 904 560 188 155 272 763 454 874 787 971 100 593 219 740 \
 374 016 000  $q^{4564}$  -

68 753 242 516 276 857 167 354 070 110 355 798 604 992 995 088 737 293 957 985 324 381 984 088 454 \
 306 894 498 868 487 222 613 860 744 776 705 513 995 358 644 549 941 540 566 954 167 648 146 751 189 \
 705 807 725  $q^{4565}$  +

77 554 397 567 770 046 056 450 491 707 297 572 244 641 920 160 854 346 864 239 034 464 202 194 871 \
 818 081 765 100 399 771 343 527 289 862 477 785 425 731 393 467 636 436 683 271 744 707 021 015 527 \
 124 921 856  $q^{4568}$  -

80 731 006 936 147 152 315 062 992 549 925 111 479 936 471 033 919 140 560 134 922 700 625 367 796 \
 058 263 261 692 375 404 936 386 710 397 079 239 880 169 117 843 720 267 579 520 982 839 585 476 445 \
 073 408 000  $q^{4569}$  +

91 060 656 848 678 307 503 758 530 879 615 960 721 988 700 352 670 244 352 243 562 865 134 351 253 \
 899 709 478 281 306 029 237 761 327 190 313 095 453 006 091 147 321 586 632 625 995 949 512 384 110 \
 019 674 112  $q^{4572}$  -

94 788 819 138 799 146 430 333 314 917 569 840 920 243 781 918 454 898 123 878 323 266 623 279 319 \
 717 979 704 489 472 354 045 668 246 804 100 590 976 275 008 742 496 799 876 138 691 108 065 458 020 \
 585 752 469  $q^{4573}$  +

106 911 572 623 164 601 623 617 815 045 347 528 939 080 366 179 278 798 260 354 050 635 840 734 249 \
 085 104 625 656 483 042 273 617 219 123 508 256 122 651 302 261 324 132 574 240 043 181 279 477 763 \
 367 936 000  $q^{4576}$  -

111 286 749 004 629 991 143 844 938 193 101 998 268 480 118 108 106 615 082 909 152 341 512 919 546 \
 477 699 621 887 833 267 589 814 611 506 976 548 422 893 755 484 727 877 700 617 679 146 086 886 769 \

$106\ 354\ 176\ q^{4577} +$   
 $125\ 512\ 877\ 422\ 159\ 308\ 832\ 272\ 581\ 209\ 930\ 886\ 410\ 928\ 673\ 265\ 947\ 578\ 009\ 223\ 978\ 958\ 923\ 820\ 845\ \dots$   
 $814\ 960\ 602\ 030\ 341\ 501\ 989\ 835\ 367\ 947\ 796\ 383\ 746\ 017\ 361\ 446\ 870\ 427\ 514\ 697\ 928\ 387\ 288\ 536\ 689\ \dots$   
 $322\ 393\ 600\ q^{4580} -$   
 $130\ 646\ 998\ 680\ 798\ 554\ 023\ 381\ 237\ 094\ 690\ 751\ 354\ 630\ 913\ 232\ 225\ 169\ 132\ 996\ 501\ 442\ 405\ 397\ 241\ \dots$   
 $267\ 466\ 389\ 332\ 105\ 064\ 686\ 731\ 255\ 073\ 787\ 297\ 634\ 034\ 631\ 662\ 214\ 498\ 693\ 294\ 407\ 066\ 816\ 381\ 291\ \dots$   
 $374\ 149\ 375\ q^{4581} +$   
 $147\ 340\ 290\ 857\ 495\ 377\ 674\ 501\ 942\ 093\ 609\ 438\ 538\ 079\ 618\ 757\ 211\ 531\ 393\ 320\ 126\ 898\ 680\ 819\ 003\ \dots$   
 $063\ 343\ 934\ 792\ 823\ 103\ 160\ 334\ 650\ 670\ 696\ 880\ 298\ 781\ 797\ 118\ 637\ 525\ 413\ 796\ 838\ 925\ 982\ 406\ 535\ \dots$   
 $840\ 768\ 000\ q^{4584} -$   
 $153\ 364\ 589\ 820\ 008\ 590\ 319\ 969\ 664\ 130\ 550\ 842\ 724\ 549\ 387\ 117\ 273\ 454\ 076\ 453\ 347\ 740\ 336\ 006\ 343\ \dots$   
 $893\ 592\ 899\ 749\ 592\ 877\ 676\ 365\ 301\ 126\ 694\ 253\ 211\ 456\ 232\ 749\ 167\ 545\ 268\ 345\ 352\ 534\ 512\ 477\ 223\ \dots$   
 $536\ 230\ 400\ q^{4585} +$   
 $172\ 951\ 553\ 742\ 611\ 761\ 413\ 861\ 418\ 645\ 042\ 765\ 671\ 515\ 412\ 828\ 898\ 630\ 157\ 854\ 511\ 872\ 428\ 368\ 617\ \dots$   
 $409\ 132\ 457\ 267\ 372\ 110\ 118\ 138\ 135\ 067\ 379\ 191\ 735\ 323\ 332\ 808\ 977\ 724\ 326\ 782\ 944\ 717\ 771\ 106\ 179\ \dots$   
 $749\ 760\ 000\ q^{4588} -$   
 $180\ 019\ 883\ 271\ 832\ 597\ 455\ 161\ 206\ 976\ 257\ 625\ 173\ 770\ 000\ 778\ 238\ 453\ 925\ 740\ 580\ 904\ 990\ 100\ 352\ \dots$   
 $043\ 888\ 107\ 717\ 806\ 911\ 047\ 652\ 292\ 268\ 203\ 507\ 155\ 116\ 541\ 355\ 292\ 979\ 121\ 557\ 053\ 446\ 684\ 187\ 972\ \dots$   
 $084\ 386\ 250\ q^{4589} +$   
 $203\ 000\ 524\ 885\ 745\ 354\ 084\ 309\ 610\ 188\ 656\ 256\ 143\ 735\ 147\ 029\ 955\ 297\ 482\ 329\ 945\ 548\ 965\ 249\ 533\ \dots$   
 $826\ 026\ 124\ 346\ 054\ 914\ 620\ 383\ 348\ 392\ 514\ 912\ 774\ 811\ 711\ 348\ 114\ 027\ 450\ 981\ 514\ 904\ 543\ 446\ 724\ \dots$   
 $996\ 890\ 624\ q^{4592} -$   
 $211\ 293\ 244\ 425\ 218\ 334\ 563\ 311\ 023\ 103\ 718\ 998\ 399\ 775\ 131\ 493\ 894\ 726\ 673\ 963\ 565\ 663\ 549\ 956\ 816\ \dots$   
 $917\ 467\ 202\ 177\ 544\ 323\ 386\ 471\ 814\ 718\ 070\ 379\ 695\ 721\ 913\ 183\ 125\ 912\ 976\ 035\ 353\ 503\ 370\ 067\ 439\ \dots$   
 $084\ 601\ 344\ q^{4593} +$   
 $238\ 253\ 692\ 980\ 541\ 030\ 805\ 205\ 904\ 803\ 496\ 938\ 725\ 609\ 956\ 846\ 105\ 404\ 394\ 282\ 796\ 553\ 191\ 348\ 408\ \dots$   
 $795\ 243\ 968\ 100\ 285\ 871\ 449\ 118\ 861\ 262\ 240\ 412\ 485\ 863\ 809\ 693\ 481\ 731\ 180\ 984\ 299\ 977\ 194\ 575\ 125\ \dots$   
 $227\ 520\ 000\ q^{4596} -$   
 $247\ 982\ 220\ 762\ 307\ 614\ 918\ 071\ 312\ 285\ 890\ 513\ 316\ 493\ 572\ 216\ 542\ 729\ 911\ 721\ 608\ 455\ 768\ 728\ 727\ \dots$   
 $427\ 129\ 804\ 886\ 776\ 451\ 106\ 414\ 216\ 238\ 989\ 735\ 094\ 340\ 573\ 599\ 085\ 161\ 195\ 674\ 414\ 863\ 299\ 865\ 280\ \dots$   
 $698\ 694\ 223\ q^{4597} +$   
 $279\ 609\ 516\ 042\ 937\ 063\ 400\ 090\ 637\ 397\ 512\ 905\ 087\ 474\ 600\ 618\ 659\ 268\ 607\ 570\ 264\ 910\ 264\ 567\ 605\ \dots$   
 $986\ 059\ 543\ 866\ 115\ 262\ 224\ 221\ 143\ 146\ 195\ 185\ 878\ 657\ 738\ 396\ 974\ 881\ 454\ 933\ 950\ 988\ 974\ 217\ 759\ \dots$   
 $870\ 387\ 200\ q^{4600} -$   
 $291\ 021\ 660\ 607\ 891\ 372\ 213\ 574\ 525\ 528\ 801\ 834\ 097\ 723\ 520\ 425\ 101\ 484\ 787\ 075\ 690\ 379\ 722\ 667\ 342\ \dots$   
 $834\ 317\ 833\ 017\ 478\ 554\ 601\ 283\ 848\ 807\ 787\ 740\ 420\ 977\ 847\ 663\ 252\ 170\ 518\ 911\ 023\ 545\ 450\ 378\ 733\ \dots$   
 $162\ 496\ 000\ q^{4601} +$   
 $328\ 121\ 071\ 057\ 825\ 908\ 003\ 330\ 573\ 563\ 834\ 411\ 460\ 955\ 497\ 973\ 277\ 537\ 662\ 879\ 116\ 554\ 447\ 158\ 843\ \dots$   
 $184\ 160\ 272\ 344\ 292\ 573\ 732\ 112\ 594\ 339\ 264\ 791\ 566\ 520\ 266\ 625\ 677\ 856\ 075\ 750\ 391\ 040\ 843\ 051\ 481\ \dots$   
 $416\ 704\ 000\ q^{4604} -$   
 $341\ 507\ 275\ 080\ 028\ 316\ 831\ 577\ 347\ 009\ 654\ 840\ 467\ 593\ 765\ 515\ 672\ 015\ 546\ 046\ 085\ 497\ 059\ 387\ 539\ \dots$   
 $508\ 809\ 769\ 631\ 268\ 769\ 412\ 983\ 957\ 900\ 278\ 218\ 402\ 272\ 414\ 468\ 101\ 703\ 728\ 178\ 954\ 363\ 706\ 196\ 320\ \dots$   
 $237\ 812\ 200\ q^{4605} +$   
 $385\ 022\ 578\ 629\ 027\ 606\ 560\ 429\ 843\ 592\ 361\ 674\ 214\ 520\ 120\ 092\ 162\ 981\ 060\ 644\ 722\ 552\ 323\ 900\ 220\ \dots$   
 $064\ 995\ 123\ 576\ 923\ 742\ 357\ 600\ 969\ 250\ 541\ 948\ 154\ 623\ 690\ 961\ 156\ 546\ 335\ 318\ 526\ 399\ 233\ 439\ 641\ \dots$   
 $291\ 063\ 296\ q^{4608} -$   
 $400\ 723\ 230\ 658\ 802\ 162\ 580\ 045\ 407\ 677\ 104\ 455\ 199\ 773\ 660\ 627\ 148\ 602\ 474\ 973\ 498\ 358\ 470\ 099\ 601\ \dots$   
 $488\ 518\ 817\ 742\ 270\ 892\ 173\ 545\ 029\ 990\ 851\ 379\ 159\ 070\ 557\ 533\ 691\ 522\ 082\ 594\ 118\ 938\ 536\ 411\ 395\ \dots$   
 $092\ 480\ 000\ q^{4609} +$   
 $451\ 760\ 463\ 487\ 186\ 514\ 332\ 513\ 309\ 890\ 221\ 667\ 159\ 009\ 823\ 052\ 259\ 763\ 731\ 150\ 727\ 861\ 957\ 614\ 871\ \dots$   
 $419\ 671\ 407\ 715\ 169\ 755\ 408\ 392\ 427\ 419\ 641\ 048\ 451\ 487\ 661\ 060\ 109\ 323\ 340\ 297\ 446\ 404\ 842\ 531\ 162\ \dots$   
 $509\ 606\ 912\ q^{4612} -$   
 $470\ 174\ 459\ 687\ 613\ 317\ 850\ 636\ 066\ 441\ 557\ 835\ 460\ 661\ 852\ 671\ 495\ 136\ 682\ 576\ 709\ 326\ 930\ 054\ 717\ \dots$   
 $429\ 029\ 834\ 075\ 051\ 960\ 309\ 501\ 894\ 036\ 045\ 847\ 009\ 225\ 443\ 562\ 732\ 185\ 059\ 521\ 212\ 018\ 058\ 555\ 258\ \dots$   
 $049\ 155\ 309\ q^{4613} +$

530 029 724 057 847 426 723 084 444 740 685 473 869 710 664 195 516 122 713 162 354 607 711 718 841 3  
 894 037 657 749 293 479 764 673 800 274 312 014 004 721 654 417 717 918 131 659 073 783 818 578 618 3  
 401 024 000  $q^{4616}$  -  
 551 624 492 953 882 632 193 913 878 291 288 634 850 299 579 565 039 039 604 601 999 758 639 250 732 3  
 369 763 339 017 662 167 308 235 878 509 864 385 502 390 363 452 234 375 980 458 348 952 660 954 417 3  
 953 275 904  $q^{4617}$  +  
 621 816 515 678 748 737 644 200 965 578 710 507 499 219 889 134 817 639 294 798 412 549 748 079 793 3  
 557 287 992 789 332 271 797 423 083 299 338 107 325 402 968 763 698 954 725 675 938 477 193 971 643 3  
 714 662 400  $q^{4620}$  -  
 647 139 755 125 424 724 406 257 019 496 680 776 400 008 760 518 332 450 137 326 798 401 402 846 792 3  
 286 651 694 666 881 560 799 310 001 717 734 717 610 845 101 080 741 240 063 362 828 649 569 563 472 3  
 721 455 500  $q^{4621}$  +  
 729 448 005 697 589 425 449 480 463 888 456 624 019 469 301 193 189 091 886 877 358 486 770 175 615 3  
 417 266 966 140 618 885 372 719 300 526 018 746 243 117 013 519 195 755 392 068 163 411 560 957 444 3  
 149 578 752  $q^{4624}$  -  
 759 141 423 588 956 032 824 171 953 773 492 421 240 461 286 611 814 077 686 025 513 483 363 296 181 3  
 795 825 608 178 502 872 871 229 320 479 347 434 751 441 875 242 657 139 504 194 600 361 993 607 016 3  
 415 232 000  $q^{4625}$  +  
 855 650 738 337 103 351 438 695 668 695 449 917 247 392 330 099 643 670 520 928 764 025 419 163 868 3  
 905 665 670 030 186 098 107 890 510 215 326 371 434 222 685 044 594 393 799 098 096 340 624 875 044 3  
 662 276 096  $q^{4628}$  -  
 890 466 138 055 214 258 252 503 212 690 642 818 883 623 001 585 952 564 339 525 224 869 912 007 609 3  
 766 349 910 505 436 456 839 288 246 569 525 677 625 057 168 399 784 817 092 562 710 699 629 709 140 3  
 890 332 875  $q^{4629}$  +  
 1 003 618 957 273 666 820 261 033 007 273 125 186 335 187 553 036 717 538 783 574 368 297 621 594 720 3  
 395 416 253 096 106 988 575 795 604 099 088 617 160 506 710 729 801 783 069 483 033 578 071 688 874 3  
 913 191 936  $q^{4632}$  -  
 1 044 437 066 725 510 552 606 223 210 996 982 650 955 668 666 780 169 145 458 513 297 230 326 925 485 3  
 390 927 941 146 960 930 424 743 375 730 520 137 101 385 221 749 381 174 813 302 525 347 528 935 622 3  
 358 859 776  $q^{4633}$  +  
 1 177 094 579 468 004 321 829 224 588 564 474 789 913 239 857 038 354 904 118 541 745 035 954 015 107 3  
 202 054 721 003 541 648 313 322 304 965 275 069 428 639 304 638 170 795 209 749 020 142 022 719 641 3  
 157 888 000  $q^{4636}$  -  
 1 224 947 090 189 614 777 358 042 368 848 973 146 012 799 339 549 754 132 695 648 042 782 433 254 176 3  
 447 059 305 211 276 326 640 953 949 656 514 683 277 040 646 960 402 116 476 239 444 754 222 215 037 3  
 021 954 719  $q^{4637}$  +  
 1 380 460 800 903 532 464 457 074 759 476 823 656 596 997 822 323 800 908 584 858 711 453 895 911 089 3  
 452 747 921 421 573 330 107 555 301 726 325 489 939 286 797 329 138 038 832 789 263 672 325 638 817 3  
 858 969 600  $q^{4640}$  -  
 1 436 556 162 773 729 465 169 126 935 509 589 512 914 030 687 081 922 411 102 789 793 241 009 418 979 3  
 878 287 899 032 242 991 614 474 314 367 153 783 376 007 335 682 725 803 048 626 790 270 776 322 153 3  
 054 208 000  $q^{4641}$  +  
 1 618 851 650 528 340 410 481 107 403 634 114 011 395 788 522 455 466 214 240 339 078 127 818 820 982 3  
 320 998 333 107 171 569 631 927 321 909 365 776 931 412 452 902 439 505 466 927 736 146 803 646 478 3  
 458 880 000  $q^{4644}$  -  
 1 684 605 260 055 917 821 791 467 042 174 791 479 237 527 089 612 470 206 098 067 592 650 408 415 837 3  
 291 039 915 059 594 798 244 820 448 179 275 998 277 388 959 008 076 773 782 790 450 205 070 830 534 3  
 076 172 550  $q^{4645}$  +  
 1 898 280 201 035 513 910 251 662 980 943 258 327 892 683 406 556 151 266 483 180 819 703 933 821 451 3  
 661 616 900 130 577 881 764 289 944 215 700 932 438 457 128 903 195 968 751 789 604 951 418 553 188 3  
 210 271 232  $q^{4648}$  -  
 1 975 349 729 213 037 588 198 086 187 846 490 715 312 020 473 729 375 757 867 750 302 663 503 883 563 3  
 217 263 459 948 294 974 913 931 316 178 937 585 689 726 733 559 585 283 129 117 217 002 213 636 301 3  
 791 232 000  $q^{4649}$  +  
 2 225 788 603 701 108 967 217 289 225 414 298 940 295 189 674 776 451 737 846 678 276 837 108 268 861 3

831 994 530 761 180 695 625 155 415 220 436 349 927 898 392 486 421 389 150 180 038 646 676 893 437 5  
 622 070 784  $q^{4652}$  -  
 2 316 115 335 683 367 160 136 784 165 596 194 457 416 744 868 288 282 911 084 161 166 623 291 552 030 5  
 879 917 859 300 846 527 762 306 930 774 912 856 544 991 229 356 967 800 082 041 390 152 864 702 405 5  
 441 355 745  $q^{4653}$  +  
 2 609 623 650 479 917 933 746 692 918 436 509 438 941 761 468 207 553 837 476 117 237 865 061 917 552 5  
 504 382 555 277 655 754 323 164 632 907 637 408 089 333 845 165 437 975 327 929 899 986 006 271 756 5  
 568 576 000  $q^{4656}$  -  
 2 715 480 856 913 991 781 584 069 571 037 666 804 226 567 409 276 918 743 353 226 342 558 710 262 359 5  
 880 020 908 067 796 135 465 744 978 585 372 748 269 581 676 432 964 514 300 383 650 601 470 054 986 5  
 106 470 400  $q^{4657}$  +  
 3 059 442 192 957 493 134 761 345 607 689 695 598 422 773 139 269 537 047 914 483 588 678 463 890 789 5  
 551 394 934 052 164 834 797 862 043 369 370 640 940 332 672 721 509 797 374 580 884 186 021 950 153 5  
 535 590 400  $q^{4660}$  -  
 3 183 491 725 247 611 631 668 553 457 881 785 162 718 205 024 980 909 508 669 701 938 130 784 104 377 5  
 873 126 033 133 345 594 334 790 112 752 279 338 845 577 528 551 944 896 148 921 506 002 195 397 471 5  
 655 914 000  $q^{4661}$  +  
 3 586 551 479 777 778 144 020 625 020 860 874 078 806 552 101 649 954 498 699 777 233 089 039 844 090 5  
 833 013 090 135 445 106 905 195 460 103 306 965 376 965 845 654 350 592 087 575 028 483 509 416 449 5  
 243 776 000  $q^{4664}$  -  
 3 731 909 983 095 604 205 243 795 989 605 901 467 498 749 518 785 957 840 279 394 113 363 767 582 977 5  
 181 803 053 330 590 071 157 372 166 072 058 585 206 002 797 197 891 819 539 659 672 498 566 774 839 5  
 230 464 000  $q^{4665}$  +  
 4 204 190 329 563 157 533 463 532 177 656 758 200 499 244 915 063 319 364 281 699 289 941 682 392 820 5  
 967 098 751 646 784 123 188 123 996 516 473 467 347 435 298 463 873 686 075 055 169 663 845 494 215 5  
 576 012 800  $q^{4668}$  -  
 4 374 506 702 898 135 886 712 026 649 420 007 376 618 619 966 073 036 537 041 611 829 583 033 552 680 5  
 917 137 407 196 445 451 909 693 327 634 529 309 059 443 827 327 312 662 672 353 123 744 330 257 257 5  
 763 603 875  $q^{4669}$  +  
 4 927 858 055 846 676 438 864 625 224 747 473 503 129 501 429 772 176 956 175 028 201 623 071 454 809 5  
 349 140 481 173 523 659 187 608 273 106 563 781 714 788 654 002 322 513 107 114 991 446 094 615 572 5  
 124 794 880  $q^{4672}$  -  
 5 127 404 063 535 125 054 669 893 347 426 852 801 529 812 951 919 954 819 364 254 004 079 266 461 188 5  
 578 752 434 443 365 434 456 952 099 972 459 756 463 089 097 432 217 164 684 269 432 220 092 334 368 5  
 587 546 624  $q^{4673}$  +  
 5 775 699 228 345 311 199 253 895 972 561 668 305 391 953 061 527 637 078 191 974 315 711 366 288 325 5  
 196 512 508 745 829 765 280 501 025 818 372 359 435 833 650 250 037 078 364 195 647 140 988 392 948 5  
 244 480 000  $q^{4676}$  -  
 6 009 475 488 979 626 049 237 549 241 101 334 122 257 833 097 308 714 596 664 400 983 512 833 996 578 5  
 504 842 657 414 155 929 806 118 312 514 937 719 122 352 260 270 297 203 747 386 365 452 142 550 994 5  
 740 811 044  $q^{4677}$  +  
 6 768 953 719 270 663 250 469 108 798 078 370 895 680 740 488 908 729 967 219 837 680 445 895 409 158 5  
 987 779 465 254 819 049 975 739 302 295 440 476 293 515 774 131 647 409 693 728 504 430 374 872 036 5  
 345 472 000  $q^{4680}$  -  
 7 042 813 673 444 311 488 180 090 586 234 828 632 980 539 315 606 821 277 143 813 101 569 201 232 438 5  
 656 599 946 729 319 771 134 776 584 222 957 654 865 410 649 327 781 415 435 422 409 752 624 605 919 5  
 985 664 000  $q^{4681}$  +  
 7 932 483 077 279 067 685 703 138 887 225 610 344 237 728 031 064 851 417 005 096 351 699 994 253 939 5  
 645 171 113 231 388 977 152 546 039 736 393 500 085 911 891 684 431 909 489 633 301 661 612 368 526 5  
 753 728 000  $q^{4684}$  -  
 8 253 277 974 342 285 748 022 029 220 538 400 312 088 549 645 914 724 323 159 348 086 275 056 884 565 5  
 645 238 940 783 730 546 596 482 396 078 757 538 665 259 079 454 773 510 564 176 459 180 418 820 548 5  
 972 320 350  $q^{4685}$  +  
 9 295 386 133 602 836 222 188 972 549 730 569 313 245 002 993 960 053 319 192 362 682 865 345 707 956 5  
 962 463 395 309 281 269 063 390 465 287 159 791 199 578 067 631 975 716 405 092 691 739 482 610 521 5

$742\,622\,720\,q^{4688} -$   
 $9\,671\,134\,590\,078\,636\,508\,853\,810\,964\,419\,073\,869\,319\,331\,465\,267\,211\,856\,661\,501\,273\,501\,154\,034\,700\,408\,293\,919\,635\,503\,446\,529\,084\,417\,152\,809\,788\,411\,214\,344\,083\,963\,245\,273\,708\,097\,482\,380\,546\,407\,415\,808\,000\,q^{4689} +$   
 $10\,891\,718\,919\,810\,142\,719\,564\,577\,574\,809\,579\,953\,720\,294\,230\,357\,182\,940\,833\,290\,450\,266\,248\,155\,429\,172\,114\,253\,796\,563\,421\,190\,714\,779\,324\,235\,722\,185\,112\,901\,348\,638\,360\,882\,947\,294\,834\,084\,633\,633\,291\,624\,448\,q^{4692} -$   
 $11\,331\,805\,200\,710\,968\,333\,427\,669\,598\,709\,852\,349\,769\,540\,897\,562\,066\,937\,655\,557\,837\,403\,251\,744\,171\,042\,932\,355\,968\,574\,261\,783\,854\,469\,148\,240\,327\,986\,013\,542\,218\,578\,803\,643\,767\,031\,985\,801\,220\,236\,661\,286\,276\,q^{4693} +$   
 $12\,761\,336\,516\,953\,463\,550\,980\,220\,091\,527\,605\,472\,380\,549\,474\,136\,952\,923\,969\,394\,470\,814\,284\,924\,263\,880\,355\,633\,887\,252\,398\,619\,395\,550\,591\,990\,601\,720\,613\,763\,796\,600\,254\,607\,194\,440\,119\,515\,399\,980\,672\,832\,000\,q^{4696} -$   
 $13\,276\,742\,390\,371\,238\,499\,445\,778\,578\,201\,520\,928\,441\,533\,099\,653\,583\,324\,226\,199\,211\,063\,258\,625\,010\,311\,231\,806\,573\,773\,962\,753\,945\,488\,004\,315\,593\,272\,763\,019\,230\,507\,624\,178\,402\,398\,505\,230\,383\,520\,181\,583\,872\,q^{4697} +$   
 $14\,950\,877\,422\,785\,508\,848\,054\,839\,842\,024\,276\,366\,288\,541\,095\,651\,204\,115\,653\,683\,544\,635\,625\,760\,163\,226\,998\,267\,037\,400\,658\,434\,911\,484\,232\,908\,721\,147\,616\,286\,130\,984\,790\,564\,367\,783\,608\,645\,370\,511\,950\,745\,600\,q^{4700} -$   
 $15\,554\,453\,254\,636\,468\,582\,161\,568\,241\,209\,544\,734\,754\,200\,282\,063\,740\,620\,636\,570\,788\,420\,415\,067\,514\,427\,480\,379\,646\,806\,414\,431\,366\,236\,572\,762\,249\,397\,335\,018\,235\,990\,487\,204\,329\,124\,196\,007\,973\,244\,238\,261\,125\,q^{4701} +$   
 $17\,514\,914\,488\,665\,243\,726\,681\,495\,630\,040\,021\,983\,445\,424\,789\,643\,987\,971\,536\,454\,073\,478\,587\,730\,176\,129\,930\,977\,682\,969\,683\,460\,992\,103\,573\,538\,189\,658\,294\,583\,592\,160\,242\,595\,382\,076\,417\,103\,104\,502\,851\,072\,000\,q^{4704} -$   
 $18\,221\,696\,198\,000\,300\,216\,841\,790\,522\,566\,797\,687\,566\,232\,751\,533\,648\,403\,486\,281\,974\,000\,525\,460\,408\,065\,354\,028\,724\,608\,940\,045\,365\,928\,289\,792\,264\,139\,404\,681\,855\,350\,789\,466\,273\,762\,656\,378\,579\,505\,353\,523\,200\,q^{4705} +$   
 $20\,517\,300\,524\,081\,617\,596\,693\,083\,774\,944\,499\,933\,458\,611\,424\,756\,485\,947\,863\,590\,504\,851\,975\,685\,607\,515\,417\,100\,754\,773\,035\,687\,591\,493\,625\,746\,152\,248\,218\,947\,092\,875\,803\,311\,579\,986\,932\,498\,719\,930\,995\,556\,352\,q^{4708} -$   
 $21\,344\,880\,132\,845\,119\,294\,596\,394\,050\,082\,874\,427\,251\,834\,743\,330\,378\,500\,414\,052\,271\,551\,940\,878\,562\,516\,439\,068\,517\,390\,707\,689\,161\,563\,925\,638\,999\,843\,099\,654\,269\,670\,625\,878\,346\,304\,710\,529\,781\,197\,100\,038\,125\,q^{4709} +$   
 $24\,032\,741\,391\,627\,265\,290\,336\,550\,874\,061\,407\,550\,392\,481\,504\,000\,408\,338\,018\,882\,897\,396\,626\,350\,786\,750\,589\,658\,889\,445\,411\,984\,566\,676\,063\,190\,887\,151\,336\,201\,959\,811\,120\,926\,074\,460\,773\,428\,265\,540\,613\,410\,816\,q^{4712} -$   
 $25\,001\,700\,202\,906\,476\,859\,000\,085\,409\,656\,306\,112\,994\,510\,496\,808\,916\,279\,553\,658\,295\,385\,456\,476\,937\,499\,557\,945\,956\,608\,565\,545\,985\,377\,388\,014\,873\,277\,476\,687\,276\,300\,178\,886\,593\,050\,660\,178\,954\,927\,747\,465\,216\,q^{4713} +$   
 $28\,148\,634\,932\,210\,247\,701\,631\,876\,053\,867\,172\,266\,734\,018\,888\,743\,210\,571\,454\,359\,516\,085\,294\,223\,489\,306\,573\,397\,030\,582\,732\,034\,509\,327\,783\,193\,888\,486\,325\,768\,086\,901\,747\,314\,929\,672\,558\,816\,619\,722\,666\,176\,000\,q^{4716} -$   
 $29\,283\,049\,889\,067\,429\,784\,947\,560\,606\,066\,269\,838\,810\,149\,319\,766\,814\,744\,685\,475\,794\,737\,700\,123\,398\,818\,958\,698\,359\,684\,790\,995\,500\,936\,344\,422\,516\,347\,609\,491\,286\,775\,976\,306\,358\,072\,279\,187\,357\,921\,832\,724\,749\,q^{4717} +$   
 $32\,967\,220\,501\,658\,579\,051\,377\,290\,695\,760\,011\,409\,026\,428\,147\,418\,543\,284\,479\,951\,373\,459\,045\,389\,509\,049\,561\,599\,002\,154\,243\,025\,641\,017\,738\,503\,087\,153\,287\,176\,101\,663\,926\,183\,231\,680\,823\,785\,765\,270\,896\,230\,400\,q^{4720} -$   
 $34\,295\,256\,050\,978\,851\,283\,601\,857\,530\,656\,830\,560\,290\,568\,068\,490\,820\,295\,288\,824\,899\,839\,256\,797\,595\,447\,487\,442\,519\,002\,138\,194\,827\,629\,986\,273\,115\,965\,852\,483\,764\,230\,037\,198\,670\,593\,879\,411\,054\,130\,126\,848\,000\,q^{4721} +$   
 $38\,608\,091\,420\,059\,216\,594\,981\,847\,510\,634\,568\,178\,517\,347\,384\,738\,958\,370\,859\,942\,045\,145\,150\,161\,626\,908\,908\,050\,196\,188\,875\,096\,512\,495\,344\,171\,423\,911\,654\,889\,270\,834\,437\,628\,352\,692\,662\,345\,157\,074\,273\,024\,000\,q^{4724} -$

40 162 691 274 944 550 509 928 788 434 124 336 570 490 605 132 325 554 543 424 575 772 398 894 854 \
 314 229 764 608 151 947 747 020 932 335 601 753 258 801 282 700 688 236 977 213 523 225 645 654 122 \
 181 712 418 075  $q^{4725} +$

45 211 131 414 301 176 960 081 472 825 214 451 106 652 336 095 409 233 832 050 350 454 293 984 835 \
 829 224 062 201 299 994 698 012 652 162 602 771 171 614 082 842 835 645 387 541 651 154 240 127 134 \
 726 790 243 328  $q^{4728} -$

47 030 827 023 926 975 239 372 661 083 461 675 828 482 713 787 254 821 769 361 704 001 488 759 034 \
 016 649 013 456 143 838 068 930 136 924 719 729 631 229 183 526 807 900 521 549 936 037 669 953 458 \
 651 947 008 000  $q^{4729} +$

52 939 946 382 461 735 114 376 556 878 220 010 034 061 703 461 855 278 458 153 942 563 509 699 732 \
 623 734 499 748 842 047 726 119 068 401 442 027 173 215 901 779 002 343 131 972 082 609 768 414 932 \
 919 851 563 008  $q^{4732} -$

55 069 801 737 762 670 977 892 358 196 585 832 621 501 290 094 831 234 303 811 929 802 532 729 442 \
 712 858 713 069 710 963 098 073 643 084 794 103 616 596 924 021 712 876 321 357 640 317 820 209 251 \
 858 766 609 016  $q^{4733} +$

61 985 874 770 939 196 549 392 377 534 621 542 053 891 989 194 678 633 608 682 505 011 044 708 949 \
 476 516 263 786 271 514 882 264 533 025 056 658 293 344 522 103 037 009 275 719 401 850 522 267 349 \
 336 027 136 000  $q^{4736} -$

64 478 590 465 389 723 147 931 123 080 054 568 231 332 823 132 210 960 867 114 302 421 876 639 602 \
 923 074 834 780 296 925 091 746 319 517 756 847 814 484 163 121 844 386 468 375 594 838 201 652 727 \
 449 620 873 216  $q^{4737} +$

72 572 673 817 400 181 829 519 982 062 302 354 856 651 171 327 567 144 864 785 710 082 795 006 409 \
 459 905 047 602 634 889 797 015 150 005 188 610 229 961 551 727 688 762 075 863 162 077 557 306 586 \
 643 895 091 200  $q^{4740} -$

75 489 877 123 089 289 600 093 759 572 415 225 634 742 453 987 736 246 502 654 593 071 183 351 806 \
 875 100 849 021 163 783 559 505 571 933 892 709 343 595 137 199 734 609 098 277 006 968 727 087 329 \
 179 269 600 375  $q^{4741} +$

84 961 995 207 984 607 689 890 184 963 047 958 784 425 773 361 668 740 978 495 795 095 930 424 520 \
 869 577 207 505 317 179 145 491 919 652 665 185 994 116 696 343 387 033 649 272 224 926 444 164 005 \
 956 755 712 000  $q^{4744} -$

88 375 747 409 800 022 207 008 489 398 672 363 450 877 011 975 381 410 871 408 894 372 877 670 340 \
 608 499 194 720 659 951 163 893 476 068 709 950 348 681 834 423 955 193 916 646 063 638 964 443 581 \
 562 162 380 800  $q^{4745} +$

99 459 782 714 486 576 782 649 234 907 145 534 527 127 941 559 397 128 293 120 658 037 616 156 264 \
 473 503 190 760 537 203 129 056 584 975 861 606 483 701 575 084 515 569 257 505 479 008 637 876 617 \
 624 445 475 328  $q^{4748} -$

103 454 340 176 389 104 412 619 101 790 628 508 942 905 290 557 891 293 270 089 119 688 452 636 253 \
 847 206 799 347 022 308 654 740 052 486 244 748 427 998 931 681 227 114 230 415 083 151 025 458 370 \
 312 528 064 625  $q^{4749} +$

116 423 746 569 643 521 028 485 818 997 197 985 998 909 914 693 272 653 254 716 247 400 324 681 773 \
 721 888 149 892 124 906 112 808 624 619 951 768 989 130 407 509 574 737 122 811 112 417 996 635 491 \
 683 799 662 592  $q^{4752} -$

121 097 618 111 339 156 126 696 253 192 141 217 065 396 978 675 667 561 937 005 144 200 394 693 792 \
 417 783 651 251 966 703 878 372 642 038 853 092 049 093 242 622 667 213 633 894 397 928 644 536 989 \
 269 343 436 800  $q^{4753} +$

136 272 095 234 695 542 946 823 681 277 677 254 424 863 464 571 264 804 160 803 591 289 729 742 858 \
 752 425 315 701 156 194 839 655 789 560 188 591 126 204 827 723 489 647 171 082 474 937 222 576 909 \
 600 619 008 000  $q^{4756} -$

141 740 445 519 792 452 189 962 955 624 653 840 037 379 750 796 301 887 524 149 537 168 671 550 447 \
 551 855 239 381 164 758 658 679 396 688 166 596 517 714 202 240 865 738 015 647 585 264 490 593 747 \
 500 604 658 656  $q^{4757} +$

159 493 735 429 185 828 607 402 421 250 239 172 218 762 014 200 452 870 535 254 628 369 171 752 649 \
 859 691 959 695 814 167 429 228 465 657 887 121 092 694 677 811 567 006 486 205 480 249 146 604 600 \
 905 520 896 000  $q^{4760} -$

165 891 192 376 547 560 893 901 694 411 211 190 411 068 679 892 259 042 692 302 200 325 599 550 795 \

667 004 312 067 257 975 216 410 423 919 457 080 368 587 238 706 565 660 393 339 391 355 545 904 132 5  
 653 510 656 248  $q^{4761} +$   
 186 660 186 546 917 042 182 871 259 649 703 233 015 195 727 907 107 672 808 638 023 360 468 851 057 5  
 668 563 491 857 654 281 858 498 090 672 917 323 119 419 396 131 862 994 514 077 869 589 889 198 210 5  
 375 108 352 000  $q^{4764} -$   
 194 144 120 472 870 809 179 938 996 502 953 162 406 130 563 635 976 740 286 886 702 105 774 964 097 5  
 176 374 104 591 060 168 656 664 631 056 420 773 439 651 988 228 023 199 827 386 181 140 634 526 027 5  
 483 661 843 975  $q^{4765} +$   
 218 439 496 711 501 598 361 361 828 712 292 429 253 457 930 284 986 523 290 760 807 257 180 232 673 5  
 222 339 654 994 021 284 612 947 300 001 633 329 812 437 644 841 147 856 008 782 361 479 800 335 041 5  
 586 700 939 264  $q^{4768} -$   
 227 193 850 222 038 642 729 320 977 578 274 618 897 737 641 732 781 490 086 840 643 480 396 226 398 5  
 616 721 452 066 824 501 385 582 687 716 053 065 935 877 033 329 207 830 243 287 008 370 698 628 346 5  
 466 897 920 000  $q^{4769} +$   
 255 612 495 706 258 614 453 308 157 162 166 884 196 812 561 555 404 784 460 109 083 614 647 877 072 5  
 631 203 401 909 205 449 076 898 484 294 557 788 307 275 698 148 094 773 474 370 889 955 662 726 906 5  
 847 342 968 832  $q^{4772} -$   
 265 852 256 553 716 293 269 205 883 488 811 576 476 888 396 932 844 756 074 425 911 994 395 203 580 5  
 895 066 247 032 262 302 581 217 485 375 935 783 125 425 361 183 060 168 297 090 510 629 029 487 259 5  
 699 467 817 199  $q^{4773} +$   
 299 091 775 984 222 835 868 642 232 596 631 696 635 016 326 363 548 894 698 598 766 863 908 721 388 5  
 144 074 564 224 708 956 554 207 836 936 976 702 338 680 732 592 607 816 309 616 587 487 964 866 785 5  
 170 123 904 000  $q^{4776} -$   
 311 068 200 494 943 341 017 332 957 682 267 769 404 820 126 023 700 812 641 068 205 399 140 369 409 5  
 445 857 025 563 245 331 891 778 213 675 150 837 232 088 084 412 918 826 437 561 792 779 687 464 641 5  
 270 299 230 208  $q^{4777} +$   
 349 943 858 251 037 911 918 670 697 864 295 649 954 067 321 841 433 769 912 687 728 989 610 124 829 5  
 459 211 351 053 357 610 981 179 810 907 307 411 381 841 306 615 025 129 826 332 777 790 519 325 047 5  
 515 287 449 600  $q^{4780} -$   
 363 950 570 883 704 286 821 988 983 796 444 665 247 495 974 009 763 873 945 536 967 386 890 892 407 5  
 969 220 946 406 341 562 953 107 121 005 069 957 972 876 030 650 378 827 549 974 239 493 421 440 609 5  
 367 118 148 250  $q^{4781} +$   
 409 415 074 262 289 884 606 279 310 751 929 920 271 002 263 641 621 862 676 665 050 980 818 341 595 5  
 489 242 673 409 203 255 045 293 884 254 373 111 172 180 540 793 445 838 759 730 544 763 627 740 335 5  
 713 988 608 000  $q^{4784} -$   
 425 795 189 795 905 570 078 807 233 514 063 588 586 148 511 388 873 114 046 309 841 160 508 717 926 5  
 433 064 792 980 825 605 434 623 763 550 370 886 897 133 591 390 178 033 864 978 310 224 709 183 555 5  
 227 153 203 200  $q^{4785} +$   
 478 961 788 288 872 742 073 761 227 179 496 776 444 600 485 602 603 467 452 966 631 636 381 177 612 5  
 230 977 596 904 499 308 583 032 790 869 116 120 944 890 766 410 404 913 202 181 852 973 473 981 126 5  
 672 188 575 744  $q^{4788} -$   
 498 116 227 559 794 552 612 956 409 624 576 525 675 379 907 920 303 842 691 324 984 900 569 530 096 5  
 566 882 584 221 122 205 369 455 424 753 084 927 610 612 666 080 844 076 664 268 186 496 460 956 495 5  
 226 437 901 375  $q^{4789} +$   
 560 285 682 278 601 442 437 731 611 615 609 261 388 477 597 685 251 017 268 366 688 195 154 938 739 5  
 441 524 630 662 737 637 179 367 011 210 550 599 195 366 677 067 691 413 466 698 195 478 543 066 208 5  
 397 016 706 048  $q^{4792} -$   
 582 682 880 864 617 530 381 635 737 094 694 527 456 238 112 932 158 345 593 177 219 956 790 453 055 5  
 689 369 200 032 228 956 484 303 447 656 490 077 674 249 948 099 379 329 735 366 395 629 751 022 566 5  
 680 140 644 352  $q^{4793} +$   
 655 374 950 525 789 206 488 748 838 220 423 192 771 494 019 830 608 249 086 141 861 554 176 246 906 5  
 668 913 749 748 559 415 429 492 636 806 711 727 399 439 463 125 914 679 559 706 649 063 825 123 996 5  
 984 265 472 000  $q^{4796} -$   
 681 562 192 984 241 124 770 040 808 401 506 804 346 884 197 407 592 458 487 496 914 998 803 614 943 5  
 650 433 336 186 935 524 817 904 048 970 055 888 735 788 143 951 651 857 804 502 854 817 241 461 422 5

$514\ 516\ 665\ 860\ q^{4797} +$   
 766 552 390 503 294 410 587 107 482 699 270 965 325 622 665 183 677 322 262 386 155 009 847 738 776  
 $777\ 878\ 178\ 597\ 228\ 932\ 835\ 638\ 178\ 404\ 266\ 467\ 527\ 412\ 587\ 590\ 811\ 590\ 977\ 366\ 565\ 227\ 678\ 596\ 757$   
 $165\ 785\ 907\ 200\ q^{4800} -$   
 797 169 041 492 993 655 213 546 823 295 930 275 400 616 387 512 278 991 780 634 430 706 322 276 950  
 $705\ 832\ 236\ 222\ 279\ 606\ 214\ 858\ 726\ 305\ 907\ 024\ 084\ 293\ 983\ 819\ 911\ 192\ 317\ 051\ 593\ 510\ 746\ 434\ 378$   
 $281\ 279\ 488\ 000\ q^{4801} +$   
 896 531 540 734 699 375 966 429 180 861 442 466 397 039 153 371 761 171 014 440 707 200 829 727 829  
 $514\ 816\ 607\ 624\ 555\ 920\ 817\ 553\ 934\ 697\ 093\ 523\ 728\ 802\ 462\ 191\ 819\ 665\ 996\ 886\ 918\ 714\ 940\ 944\ 103$   
 $199\ 072\ 256\ 000\ q^{4804} -$   
 932 324 489 500 511 745 281 823 020 756 352 032 060 684 034 315 061 953 642 461 609 756 644 782 546  
 $561\ 942\ 077\ 851\ 740\ 279\ 757\ 650\ 933\ 701\ 083\ 713\ 011\ 317\ 738\ 803\ 061\ 683\ 509\ 060\ 953\ 439\ 796\ 405\ 986$   
 $595\ 826\ 513\ 245\ q^{4805} +$   
 1 048 482 208 057 041 547 590 346 769 081 246 606 516 672 523 324 580 277 859 322 768 004 628 101 036  
 $222\ 588\ 258\ 974\ 038\ 135\ 216\ 726\ 434\ 319\ 244\ 173\ 160\ 529\ 282\ 136\ 356\ 670\ 099\ 767\ 779\ 002\ 024\ 535\ 193$   
 $834\ 148\ 728\ 832\ q^{4808} -$   
 1 090 323 895 394 726 070 489 169 936 050 323 980 524 346 125 419 633 017 539 027 034 463 305 382 029  
 $230\ 254\ 732\ 300\ 717\ 896\ 601\ 320\ 669\ 652\ 463\ 149\ 079\ 720\ 018\ 024\ 603\ 322\ 080\ 312\ 294\ 858\ 756\ 994\ 534$   
 $909\ 059\ 072\ 000\ q^{4809} +$   
 1 226 106 949 854 455 737 313 332 901 663 923 826 032 818 454 269 056 453 712 955 897 219 989 198 015  
 $116\ 866\ 934\ 272\ 491\ 154\ 392\ 381\ 267\ 127\ 178\ 361\ 890\ 368\ 992\ 858\ 497\ 450\ 082\ 059\ 173\ 990\ 406\ 681\ 946$   
 $613\ 704\ 190\ 976\ q^{4812} -$   
 1 275 016 408 040 230 405 490 076 521 923 612 692 276 751 550 157 084 515 380 572 936 039 011 164 927  
 $473\ 805\ 093\ 623\ 473\ 837\ 074\ 006\ 042\ 326\ 731\ 838\ 792\ 559\ 263\ 377\ 676\ 992\ 178\ 330\ 905\ 162\ 403\ 981\ 918$   
 $941\ 839\ 463\ 256\ q^{4813} +$   
 1 433 730 337 081 118 525 601 247 669 415 389 425 701 182 007 590 299 441 445 495 490 870 292 129 086  
 $709\ 068\ 475\ 707\ 652\ 361\ 388\ 214\ 050\ 350\ 998\ 730\ 392\ 880\ 071\ 508\ 214\ 336\ 709\ 029\ 314\ 601\ 548\ 326\ 443$   
 $715\ 895\ 296\ 000\ q^{4816} -$   
 1 490 897 744 788 261 502 596 736 164 746 508 140 205 036 623 101 029 064 779 127 351 053 378 652 051  
 $606\ 717\ 486\ 838\ 607\ 595\ 186\ 600\ 261\ 524\ 750\ 417\ 784\ 170\ 004\ 599\ 019\ 556\ 453\ 837\ 157\ 342\ 800\ 642\ 260$   
 $159\ 449\ 989\ 120\ q^{4817} +$   
 1 676 403 127 254 466 426 670 431 728 459 845 492 879 503 917 713 588 187 755 083 223 437 213 034 588  
 $592\ 480\ 909\ 053\ 691\ 137\ 674\ 747\ 064\ 500\ 119\ 172\ 766\ 863\ 904\ 879\ 651\ 265\ 115\ 022\ 700\ 099\ 099\ 838\ 002$   
 $540\ 063\ 744\ 000\ q^{4820} -$   
 1 743 218 464 868 585 973 051 865 891 522 889 629 448 443 569 353 082 551 864 316 199 753 099 470 227  
 $014\ 235\ 489\ 618\ 646\ 972\ 344\ 619\ 936\ 961\ 029\ 001\ 605\ 197\ 405\ 824\ 028\ 324\ 817\ 593\ 988\ 112\ 333\ 917\ 876$   
 $183\ 658\ 223\ 125\ q^{4821} +$   
 1 960 023 830 211 014 010 388 825 278 541 048 971 806 695 712 022 154 918 544 043 339 559 321 406 441  
 $732\ 226\ 005\ 544\ 329\ 735\ 050\ 927\ 704\ 836\ 735\ 541\ 572\ 562\ 493\ 964\ 116\ 814\ 511\ 793\ 866\ 224\ 106\ 568\ 718$   
 $991\ 262\ 656\ 000\ q^{4824} -$   
 2 038 110 318 153 788 492 541 991 904 539 703 629 520 684 762 634 854 881 359 285 613 138 270 206 046  
 $674\ 203\ 025\ 667\ 878\ 540\ 409\ 398\ 960\ 785\ 473\ 185\ 192\ 858\ 763\ 167\ 556\ 220\ 922\ 618\ 065\ 770\ 119\ 003\ 886$   
 $893\ 654\ 835\ 200\ q^{4825} +$   
 2 291 480 561 574 758 352 568 905 904 448 278 677 492 340 512 821 498 713 067 295 879 603 125 310 870  
 $951\ 232\ 664\ 619\ 419\ 823\ 103\ 640\ 712\ 035\ 284\ 127\ 442\ 847\ 602\ 606\ 056\ 475\ 806\ 172\ 003\ 378\ 979\ 013\ 870$   
 $548\ 938\ 731\ 520\ q^{4828} -$   
 2 382 733 677 532 590 248 996 595 477 055 792 308 866 799 127 538 968 912 721 009 828 330 571 074 982  
 $896\ 160\ 759\ 440\ 471\ 745\ 069\ 233\ 077\ 565\ 100\ 969\ 318\ 789\ 317\ 657\ 573\ 804\ 134\ 443\ 771\ 315\ 254\ 691\ 758$   
 $089\ 926\ 435\ 750\ q^{4829} +$   
 2 678 816 559 255 598 696 946 023 306 847 876 386 506 137 515 960 908 622 623 789 880 916 412 805 101  
 $267\ 641\ 729\ 643\ 175\ 623\ 568\ 811\ 217\ 176\ 198\ 712\ 069\ 127\ 816\ 131\ 214\ 084\ 331\ 382\ 684\ 119\ 267\ 153\ 261$   
 $464\ 708\ 325\ 376\ q^{4832} -$   
 2 785 449 562 239 548 623 370 193 504 769 064 888 971 776 194 573 958 531 887 032 268 512 792 882 896  
 $244\ 479\ 781\ 898\ 443\ 966\ 986\ 586\ 744\ 171\ 444\ 527\ 297\ 462\ 865\ 841\ 267\ 925\ 347\ 380\ 480\ 204\ 595\ 651\ 768$   
 $839\ 182\ 090\ 240\ q^{4833} +$

3 131 423 298 126 018 101 278 227 094 261 425 626 750 343 794 523 992 732 244 627 298 535 220 020 846  
 055 742 439 839 283 003 753 168 639 371 886 236 674 682 077 911 218 887 216 713 823 848 963 827 488  
 428 101 632 000  $q^{4836}$  -

3 256 020 341 154 121 050 996 440 001 129 709 579 903 915 110 148 840 458 157 521 550 770 308 092 166  
 556 127 803 343 309 247 734 452 082 406 232 176 766 577 041 961 742 252 598 742 180 421 871 026 951  
 551 172 213 952  $q^{4837}$  +

3 660 265 790 423 024 089 763 938 723 409 514 426 029 851 402 202 776 215 013 408 761 558 282 391 346  
 726 926 234 831 710 688 110 360 894 515 885 263 887 073 157 213 331 554 507 354 165 408 545 224 801  
 897 826 828 800  $q^{4840}$  -

3 805 843 882 915 527 619 510 014 684 832 969 519 242 150 673 234 012 937 600 460 746 829 156 957 701  
 689 861 288 246 727 947 433 957 387 503 093 111 168 808 089 000 456 413 897 185 850 194 959 943 583  
 678 529 536 000  $q^{4841}$  +

4 278 145 419 648 055 285 360 882 389 009 517 982 210 714 035 842 565 156 040 346 561 937 007 054 303  
 480 149 065 194 345 048 356 643 396 387 285 174 499 392 059 737 120 644 977 828 102 582 863 633 531  
 625 129 344 000  $q^{4844}$  -

4 448 226 709 551 831 891 466 145 871 477 321 020 793 982 017 317 807 561 053 420 071 656 947 843 676  
 577 778 690 140 930 711 123 689 519 074 676 869 172 120 579 452 220 612 101 403 636 849 212 415 125  
 535 504 918 925  $q^{4845}$  +

5 000 006 541 556 848 503 481 283 484 996 853 778 249 005 614 767 401 730 471 375 881 933 174 754 412  
 173 344 611 338 500 832 889 689 772 588 968 956 341 263 386 408 615 410 740 596 456 304 139 810 228  
 008 504 705 024  $q^{4848}$  -

5 198 702 630 647 434 235 310 144 135 921 105 442 027 589 570 400 498 364 872 112 968 290 108 760 177  
 949 741 085 588 593 657 766 373 213 948 547 780 695 003 687 430 448 293 787 910 771 187 505 219 184  
 975 020 032 000  $q^{4849}$  +

5 843 294 117 929 153 507 505 296 096 965 217 148 394 540 886 900 633 107 620 613 234 607 364 501 119  
 265 715 953 762 787 789 298 030 230 727 024 167 308 622 883 810 232 072 505 142 147 827 322 072 394  
 822 414 198 784  $q^{4852}$  -

6 075 404 407 359 192 935 154 794 787 726 113 509 011 408 605 266 420 481 789 857 720 506 899 957 099  
 443 109 524 412 006 225 991 547 884 680 065 972 183 356 226 491 710 517 054 797 804 279 268 012 682  
 278 424 695 105  $q^{4853}$  +

6 828 370 851 266 035 428 983 533 618 444 460 991 746 044 426 066 256 695 361 800 789 968 091 826 911  
 312 219 701 875 053 043 971 777 693 727 527 304 237 971 510 408 868 047 000 179 252 547 853 024 455  
 285 191 936 000  $q^{4856}$  -

7 099 497 244 851 645 917 351 694 282 180 193 524 403 533 073 252 982 886 663 229 987 778 695 029 221  
 684 426 747 680 317 776 950 874 748 696 660 555 062 891 861 214 698 755 492 887 365 163 690 262 826  
 807 258 939 392  $q^{4857}$  +

7 979 003 689 413 940 758 486 138 015 636 358 830 826 793 979 216 688 920 236 339 850 977 671 698 356  
 880 306 215 691 031 305 795 213 612 121 154 931 164 620 221 126 709 588 659 997 048 526 774 121 755  
 732 839 372 800  $q^{4860}$  -

8 295 684 367 075 180 282 340 138 821 692 899 087 142 727 922 744 939 091 247 742 245 526 419 636 535  
 521 550 932 042 547 821 055 556 544 809 577 349 996 312 753 197 454 202 384 087 757 617 785 170 678  
 881 903 461 250  $q^{4861}$  +

9 322 931 200 992 276 285 356 870 873 711 569 516 775 407 842 700 144 932 031 748 686 833 872 097 305  
 937 080 407 482 274 688 792 175 670 257 082 577 118 922 011 820 369 981 668 224 091 023 238 702 167  
 936 040 960 000  $q^{4864}$  -

9 692 796 623 152 820 605 240 636 429 712 723 021 256 552 892 394 037 298 547 448 054 715 162 336 306  
 755 070 051 492 058 565 472 249 552 206 300 213 778 154 096 215 179 265 004 745 378 291 017 548 116  
 474 008 371 200  $q^{4865}$  +

10 892 525 223 388 592 383 276 654 426 114 583 093 191 268 583 006 454 839 146 288 789 911 219 454  
 143 430 816 994 734 788 276 397 862 784 148 654 144 749 708 266 727 450 902 310 788 771 773 127 961  
 005 085 868 556 288  $q^{4868}$  -

11 324 480 049 424 459 362 737 415 458 917 025 057 806 450 451 206 996 967 215 178 151 211 087 581  
 120 761 959 500 938 248 829 111 221 137 394 913 564 907 741 873 017 360 580 076 260 204 682 012 424  
 765 727 405 313 125  $q^{4869}$  +

12 725 562 399 192 060 079 339 729 629 357 442 701 941 424 776 351 154 412 889 941 356 044 259 810

011 270 552 359 301 189 919 034 078 559 740 735 823 010 515 394 821 462 424 027 072 227 324 233 194 \
 642 242 362 079 232  $q^{4872}$  -

13 229 997 611 340 695 039 781 738 283 836 687 577 574 575 798 124 610 795 814 964 888 633 273 831 \
 943 003 264 174 049 471 245 393 287 922 284 403 179 775 699 879 470 384 179 939 459 205 416 038 231 \
 124 223 966 085 120  $q^{4873}$  +

14 866 123 795 714 478 360 999 791 449 165 527 245 530 384 227 969 540 348 799 225 917 266 813 480 \
 732 620 538 565 355 354 759 007 753 078 559 576 997 018 748 310 299 701 023 086 198 368 655 190 601 \
 837 700 798 848 000  $q^{4876}$  -

15 455 164 028 343 292 251 284 273 524 831 507 246 292 872 332 767 825 437 458 439 836 592 705 960 \
 388 974 242 000 844 992 023 099 165 044 088 542 284 476 489 815 279 262 959 577 940 019 970 766 469 \
 426 455 770 780 325  $q^{4877}$  +

17 365 643 805 577 524 954 880 816 606 038 619 842 925 766 631 444 946 831 673 693 036 205 517 234 \
 774 174 821 824 900 812 775 674 328 055 766 037 051 270 972 841 968 400 982 027 888 601 668 550 004 \
 658 319 917 056 000  $q^{4880}$  -

18 053 435 704 807 968 198 428 338 378 029 528 628 009 749 488 933 329 771 062 124 815 694 983 672 \
 703 329 957 165 448 873 120 714 142 271 005 906 785 520 361 121 685 787 965 978 865 994 688 346 972 \
 643 952 603 136 000  $q^{4881}$  +

20 284 133 023 906 371 302 903 228 223 180 766 818 562 850 494 185 222 984 343 504 679 294 605 616 \
 355 556 653 804 814 526 453 736 817 772 091 788 340 418 601 499 188 989 419 667 088 612 054 863 222 \
 574 025 115 648 000  $q^{4884}$  -

21 087 181 423 429 690 030 813 572 778 765 061 738 447 248 566 447 456 942 272 114 383 279 619 535 \
 269 264 977 133 683 531 964 705 914 495 248 506 789 328 113 855 320 401 581 600 050 492 207 391 796 \
 499 535 428 722 525  $q^{4885}$  +

23 691 603 870 545 798 814 905 498 046 411 893 250 348 804 612 073 910 995 956 105 782 465 359 219 \
 489 890 465 328 867 624 227 603 927 123 722 210 595 089 337 399 009 896 122 654 104 349 770 865 273 \
 981 546 174 448 640  $q^{4888}$  -

24 629 163 688 313 602 767 874 820 960 458 164 794 310 579 677 357 360 509 488 879 243 691 613 789 \
 218 622 351 693 989 636 455 726 688 301 457 824 261 860 059 571 150 386 909 834 121 694 641 125 293 \
 010 354 905 088 000  $q^{4889}$  +

27 669 732 468 249 852 162 783 856 720 542 049 314 997 240 369 886 625 097 223 513 465 170 324 234 \
 315 950 780 954 836 583 864 190 863 502 635 110 686 677 254 636 818 633 508 945 417 619 043 697 315 \
 511 636 512 028 672  $q^{4892}$  -

28 764 265 531 480 807 480 355 457 871 090 403 829 843 418 862 784 643 113 585 127 749 406 023 745 \
 085 850 657 955 033 341 389 043 943 156 326 628 496 877 075 112 298 708 973 355 848 705 672 421 243 \
 217 120 322 290 880  $q^{4893}$  +

32 313 795 809 758 109 071 522 526 335 749 205 392 945 257 237 641 459 353 621 858 945 772 879 629 \
 050 132 592 649 121 567 660 210 147 921 541 972 826 523 120 208 712 990 377 087 092 027 239 406 809 \
 573 746 263 040 000  $q^{4896}$  -

33 591 503 332 509 616 074 221 891 091 721 599 577 359 106 471 222 894 000 733 796 241 797 198 083 \
 890 968 388 451 829 087 786 515 025 808 316 753 246 943 743 727 015 340 863 284 503 810 447 903 172 \
 836 266 605 838 336  $q^{4897}$  +

37 734 929 675 766 997 355 551 233 503 183 708 811 970 860 584 114 770 676 192 644 658 445 466 187 \
 894 770 476 117 667 759 344 524 221 724 672 333 415 045 082 474 171 079 840 248 755 142 254 720 942 \
 490 243 531 139 200  $q^{4900}$  -

39 226 372 879 239 550 317 071 761 267 878 959 556 372 068 939 579 710 873 640 299 243 295 656 638 \
 945 053 550 261 589 750 499 361 585 284 813 393 841 489 844 500 275 456 782 255 404 860 900 219 718 \
 620 923 160 426 250  $q^{4901}$  +

44 062 760 250 599 706 899 291 719 605 868 896 776 127 456 712 775 043 990 534 534 044 413 543 965 \
 096 881 115 003 526 330 175 680 512 911 668 704 526 736 532 250 856 294 766 349 218 715 160 756 594 \
 828 202 492 864 000  $q^{4904}$  -

45 803 583 672 159 408 928 910 542 598 202 554 611 222 898 724 672 278 843 872 820 102 073 564 682 \
 333 614 050 335 728 676 836 818 933 697 209 999 903 309 339 674 771 391 460 214 851 957 453 271 353 \
 093 955 633 152 000  $q^{4905}$  +

51 448 471 095 696 932 978 748 935 015 606 825 083 750 910 906 909 902 884 812 572 463 411 570 227 \
 241 955 470 475 009 440 363 138 887 642 371 967 042 233 252 475 647 630 285 848 443 908 502 295 668 \

540 134 606 096 384  $q^{4908}$  -  
 53 480 245 525 763 902 813 820 081 444 240 738 531 107 389 683 101 772 749 305 609 356 576 343 662 \ \backslash  
 991 221 845 548 227 228 137 865 286 015 763 904 818 843 716 333 650 139 811 234 710 892 612 820 630 \ \backslash  
 294 368 647 013 125  $q^{4909}$  +  
 60 068 377 283 922 670 633 361 516 008 903 744 754 286 365 900 368 155 269 984 974 630 510 519 691 \ \backslash  
 586 549 400 378 453 767 091 157 621 991 080 999 618 479 101 988 211 046 611 136 575 963 801 897 647 \ \backslash  
 920 659 964 776 448  $q^{4912}$  -  
 62 439 582 055 566 754 434 848 666 863 453 037 141 690 047 260 757 772 178 634 447 377 465 962 242 \ \backslash  
 477 257 147 750 202 439 208 751 027 175 734 247 482 204 889 183 417 601 137 325 220 953 449 500 213 \ \backslash  
 146 232 613 044 224  $q^{4913}$  +  
 70 128 090 303 929 548 940 361 881 898 843 014 962 006 379 764 836 445 872 047 410 619 403 630 312 \ \backslash  
 929 660 737 749 168 084 159 994 335 801 432 270 470 773 735 898 982 590 155 600 628 153 743 482 013 \ \backslash  
 351 995 092 736 000  $q^{4916}$  -  
 72 895 257 902 427 401 906 323 876 290 054 630 016 459 725 522 829 115 811 036 075 143 848 343 407 \ \backslash  
 859 948 184 806 559 276 058 369 757 180 380 919 672 854 858 625 668 270 011 633 061 841 991 718 417 \ \backslash  
 855 761 079 549 170  $q^{4917}$  +  
 81 867 371 085 410 814 102 313 667 561 131 445 535 317 090 612 807 054 193 280 409 868 441 480 343 \ \backslash  
 146 528 565 858 653 035 597 996 027 244 140 527 474 197 868 558 858 173 071 323 236 896 870 601 214 \ \backslash  
 569 277 655 193 600  $q^{4920}$  -  
 85 096 420 818 801 721 150 520 654 456 308 503 957 137 522 781 240 410 213 463 506 080 264 140 203 \ \backslash  
 919 335 768 180 972 645 390 078 494 850 037 883 760 409 278 666 955 405 813 726 944 445 316 989 788 \ \backslash  
 457 761 980 416 000  $q^{4921}$  +  
 95 565 784 489 262 832 500 029 357 497 852 933 062 073 108 320 061 115 252 719 747 332 349 664 793 \ \backslash  
 622 079 093 935 317 236 430 675 474 963 855 495 392 425 217 518 710 357 297 423 866 246 702 155 248 \ \backslash  
 245 716 403 200 000  $q^{4924}$  -  
 99 333 576 352 911 095 689 978 517 843 924 890 464 251 223 798 593 918 261 055 950 926 129 547 054 \ \backslash  
 628 967 377 516 696 570 671 773 376 429 279 745 613 281 342 772 889 451 685 423 185 381 890 231 066 \ \backslash  
 974 232 010 949 275  $q^{4925}$  +  
 111 549 287 219 305 709 383 726 390 686 840 502 358 971 348 613 184 759 271 362 885 741 119 239 804 \ \backslash  
 726 155 574 716 765 305 303 776 425 885 808 845 826 544 236 920 718 607 832 322 570 189 034 281 490 \ \backslash  
 494 321 866 571 776  $q^{4928}$  -  
 115 945 432 198 592 648 735 347 944 097 413 119 403 483 012 012 822 938 125 873 473 537 619 620 674 \ \backslash  
 158 655 719 467 151 276 133 808 893 431 287 629 961 073 490 941 229 901 507 273 649 760 442 716 508 \ \backslash  
 342 247 284 736 000  $q^{4929}$  +  
 130 197 902 771 974 441 828 847 099 421 289 494 884 392 209 964 807 937 536 410 665 575 113 035 515 \ \backslash  
 164 127 219 089 057 088 903 002 971 567 374 762 252 936 777 707 830 143 982 718 174 532 993 883 996 \ \backslash  
 213 452 926 910 464  $q^{4932}$  -  
 135 326 871 774 898 116 938 278 397 047 410 158 300 103 384 209 373 423 114 097 205 606 889 315 433 \ \backslash  
 743 477 385 081 107 379 613 305 869 719 781 087 045 262 797 244 340 743 200 461 621 797 500 218 620 \ \backslash  
 024 868 427 848 400  $q^{4933}$  +  
 151 954 662 244 640 154 986 233 142 540 468 424 006 042 080 842 371 842 195 964 520 317 995 825 138 \ \backslash  
 532 923 004 412 359 460 597 720 472 092 327 672 399 587 270 836 122 429 213 581 225 069 504 681 005 \ \backslash  
 756 521 291 776 000  $q^{4936}$  -  
 157 938 242 776 796 515 837 228 225 212 096 624 106 094 911 302 801 243 361 344 336 067 239 841 636 \ \backslash  
 302 426 304 499 998 677 456 081 705 792 306 636 563 886 012 817 829 660 663 239 085 923 651 889 570 \ \backslash  
 536 078 442 987 520  $q^{4937}$  +  
 177 336 019 150 218 752 382 364 254 087 808 574 366 655 221 020 910 656 388 518 900 561 934 910 820 \ \backslash  
 508 215 187 198 904 285 696 663 027 575 867 140 345 326 693 408 377 889 464 798 805 229 695 667 819 \ \backslash  
 168 411 526 092 800  $q^{4940}$  -  
 184 316 176 897 080 306 868 624 079 240 438 089 649 815 084 850 094 725 932 805 819 611 563 296 530 \ \backslash  
 693 518 091 485 526 452 130 234 242 746 318 455 295 211 391 228 064 884 331 130 424 544 085 828 539 \ \backslash  
 676 695 335 855 500  $q^{4941}$  +  
 206 943 980 507 796 648 568 452 027 330 397 455 227 456 864 514 427 766 015 177 224 097 968 560 792 \ \backslash  
 038 522 386 297 712 701 401 374 856 704 558 974 092 771 608 727 291 887 894 317 632 651 096 515 261 \ \backslash  
 294 237 995 008 000  $q^{4944}$  -

215 086 192 357 907 031 868 349 883 031 618 959 190 451 837 306 383 230 860 558 197 922 776 105 386  
 824 937 377 481 633 143 975 315 931 278 373 665 261 081 000 765 700 554 350 691 418 568 970 993 927  
 118 537 439 641 600  $q^{4945} +$   
 241 480 236 177 781 334 147 795 919 929 006 557 722 677 319 844 206 601 346 967 702 040 681 418 306  
 272 741 320 177 284 737 859 330 644 191 813 555 522 739 855 690 587 170 306 066 005 155 381 526 126  
 816 905 001 015 296  $q^{4948} -$   
 250 977 372 119 950 095 079 583 904 161 802 421 504 387 112 698 230 157 082 434 667 390 372 701 650  
 452 973 596 875 251 171 243 928 860 765 878 723 727 101 673 550 320 345 928 875 540 103 109 961 105  
 679 038 713 488 500  $q^{4949} +$   
 281 762 614 594 224 207 379 471 135 075 681 248 879 738 807 430 379 637 078 053 330 906 957 546 775  
 270 504 947 015 135 714 460 094 740 429 079 461 719 016 341 824 065 088 911 670 809 854 439 349 139  
 223 550 796 318 208  $q^{4952} -$   
 292 839 458 601 389 823 593 261 940 583 725 136 782 671 844 160 521 207 078 734 901 610 711 569 155  
 051 035 967 252 217 039 081 451 465 600 463 655 714 600 876 974 214 675 209 208 049 807 210 318 878  
 452 901 825 478 656  $q^{4953} +$   
 328 744 246 772 725 371 719 667 555 378 101 936 639 549 205 991 273 852 584 511 519 688 296 718 314  
 111 145 555 542 307 294 433 542 638 630 255 727 233 541 322 214 074 782 302 617 330 532 758 328 506  
 252 922 507 264 000  $q^{4956} -$   
 341 662 761 534 705 501 325 205 945 432 812 521 997 780 431 021 539 683 027 262 347 737 011 124 285  
 062 086 902 232 787 370 341 222 523 595 970 980 151 517 275 348 088 281 217 697 783 496 133 129 232  
 416 719 279 203 818  $q^{4957} +$   
 383 535 882 967 485 817 116 230 239 793 421 288 843 971 376 894 651 868 532 815 796 666 436 489 866  
 167 666 256 374 833 106 135 602 213 145 491 685 197 107 762 187 482 766 684 321 099 734 323 667 936  
 753 738 655 744 000  $q^{4960} -$   
 398 601 340 491 253 583 986 071 685 000 179 302 330 629 725 342 546 018 504 811 461 430 514 950 599  
 233 185 482 568 943 399 473 848 179 277 181 109 853 835 797 488 721 793 567 876 618 939 780 208 368  
 605 375 012 864 000  $q^{4961} +$   
 447 431 879 042 666 782 444 233 452 319 807 712 547 107 157 070 058 727 470 710 910 901 882 499 085  
 567 807 244 012 077 567 599 063 286 385 950 659 317 135 881 987 319 444 077 473 380 232 695 320 442  
 766 509 064 192 000  $q^{4964} -$   
 464 999 999 093 648 848 759 006 104 291 522 019 588 525 910 365 896 602 656 401 431 003 815 579 267  
 296 071 416 857 624 214 145 250 317 946 555 279 719 234 848 539 828 692 853 383 711 465 702 908 981  
 944 179 259 901 525  $q^{4965} +$   
 521 940 454 169 814 086 489 772 435 270 015 440 925 139 042 767 799 545 254 578 973 204 628 264 114  
 247 815 940 376 289 475 785 265 814 503 162 753 424 211 248 839 711 647 992 234 601 899 193 088 578  
 018 933 007 147 008  $q^{4968} -$   
 542 425 715 736 079 225 887 595 503 276 705 606 096 812 523 697 513 747 469 857 415 766 737 367 251  
 090 479 446 591 852 609 346 373 857 875 790 709 609 434 565 842 935 738 222 102 510 692 442 606 688  
 779 974 811 648 000  $q^{4969} +$   
 608 818 919 792 238 880 369 722 621 832 136 699 107 051 864 080 161 244 302 973 818 357 858 942 495  
 828 883 056 139 780 354 876 782 620 346 890 145 065 193 365 192 239 991 291 075 387 772 712 814 600  
 844 336 679 118 848  $q^{4972} -$   
 632 704 237 744 193 932 903 597 633 717 146 494 052 077 941 171 724 761 081 425 130 113 924 478 271  
 233 345 255 741 514 500 165 667 394 178 737 377 137 124 309 796 203 770 408 501 039 311 459 368 785  
 648 354 819 966 251  $q^{4973} +$   
 710 114 694 148 900 803 771 314 334 984 859 569 544 198 958 613 225 022 144 912 422 935 684 081 184  
 334 190 851 115 342 300 895 556 552 815 188 987 332 228 656 924 982 345 384 418 737 149 148 321 857  
 533 902 964 736 000  $q^{4976} -$   
 737 962 684 654 799 408 412 686 136 838 415 275 253 204 208 114 832 265 207 318 872 586 966 844 993  
 255 472 040 193 923 605 465 411 164 845 282 028 677 066 291 732 958 514 034 601 830 307 516 740 031  
 862 461 780 787 200  $q^{4977} +$   
 828 213 049 627 448 699 426 542 587 159 087 267 758 874 916 199 756 055 476 722 568 056 957 206 780  
 081 976 520 570 775 660 645 443 396 892 825 773 582 967 161 665 119 880 745 927 219 834 014 405 057  
 447 887 712 665 600  $q^{4980} -$   
 860 679 144 383 765 473 339 503 987 717 236 737 841 103 886 329 637 290 960 009 017 051 143 815 904

544 864 044 114 273 872 003 621 636 753 919 478 769 803 534 161 841 898 050 044 318 737 434 343 581 3  
 627 771 389 024 125  $q^{4981} +$   
 965 892 694 843 151 580 125 435 425 949 437 923 752 315 634 796 113 759 746 148 954 843 669 364 466 3  
 654 765 484 359 776 486 889 929 327 346 558 905 126 432 334 942 988 706 883 060 099 718 167 035 765 3  
 651 863 909 888 000  $q^{4984} -$   
 1 003 740 406 618 429 998 048 972 167 937 025 832 429 737 748 772 280 349 772 105 141 334 373 564 652 3  
 858 418 899 565 436 942 221 325 957 324 667 908 080 766 764 219 481 998 296 900 782 081 356 808 945 3  
 330 916 709 171 200  $q^{4985} +$   
 1 126 390 473 131 666 274 364 294 844 840 617 133 151 216 752 177 413 924 970 560 647 213 334 691 227 3  
 965 046 768 923 419 958 039 465 439 533 100 995 239 878 982 133 797 620 348 604 151 796 928 002 227 3  
 800 394 003 167 232  $q^{4988} -$   
 1 170 509 164 466 859 686 950 168 353 987 402 076 706 385 710 214 627 786 121 216 873 920 149 675 633 3  
 018 644 679 506 076 546 403 637 202 684 703 273 896 944 197 639 909 997 047 808 850 245 636 820 201 3  
 854 160 455 407 750  $q^{4989} +$   
 1 313 476 668 181 793 175 124 687 271 994 978 395 296 810 991 480 769 474 377 070 310 268 791 529 116 3  
 944 134 618 918 916 315 200 569 273 897 951 695 094 038 849 208 206 874 858 267 903 054 406 461 070 3  
 719 461 638 602 752  $q^{4992} -$   
 1 364 902 232 459 401 115 183 041 788 986 579 396 062 743 740 848 448 811 246 769 014 473 886 489 679 3  
 408 696 763 962 419 090 898 551 151 755 690 596 420 652 114 145 582 952 243 704 491 530 862 698 687 3  
 739 120 242 393 088  $q^{4993} +$   
 1 531 542 650 562 861 182 054 761 870 167 811 241 410 560 247 851 585 606 380 568 666 947 995 397 200 3  
 874 907 666 039 531 269 470 233 699 444 698 852 073 009 446 330 517 504 815 605 538 797 076 218 795 3  
 141 785 894 912 000  $q^{4996} -$   
 1 591 481 581 352 459 151 773 612 387 772 631 837 906 806 277 352 149 375 921 494 399 740 186 616 672 3  
 149 063 044 928 679 843 323 339 887 565 618 739 292 359 521 151 865 212 756 393 839 824 629 751 957 3  
 612 489 056 029 808  $q^{4997} +$   
 1 785 702 881 430 398 366 085 753 653 500 969 052 563 423 866 594 461 557 918 643 062 278 945 839 475 3  
 877 414 304 742 641 404 246 556 665 583 647 508 158 689 055 608 679 667 968 141 504 230 384 129 091 3  
 955 231 428 512 000  $q^{5000} -$   
 1 855 560 283 550 939 171 991 393 695 722 957 788 615 576 591 738 861 862 463 551 820 670 893 708 079 3  
 108 729 891 996 543 173 576 408 261 736 612 662 019 256 556 219 461 332 564 991 886 242 091 878 211 3  
 294 848 561 152 000  $q^{5001} +$   
 2 081 913 618 124 109 328 115 184 406 611 886 298 995 926 160 166 519 196 755 824 876 354 956 509 785 3  
 882 231 895 794 370 630 064 624 862 073 367 918 562 868 128 392 616 530 007 568 794 351 095 126 712 3  
 199 157 423 040 000  $q^{5004} -$   
 2 163 325 803 989 333 866 193 603 348 134 229 451 169 648 874 504 780 105 058 092 012 944 394 901 604 3  
 056 359 062 794 657 181 844 503 110 687 320 148 480 062 153 739 873 368 690 925 717 047 650 695 775 3  
 360 918 676 674 575  $q^{5005} +$   
 2 427 111 048 138 803 628 255 123 729 539 991 452 507 848 707 849 301 653 833 599 337 922 199 751 738 3  
 026 833 257 419 253 095 522 511 969 203 345 752 818 020 799 493 624 015 657 082 363 071 702 118 141 3  
 053 856 558 350 336  $q^{5008} -$   
 2 521 983 467 710 503 968 912 422 193 357 666 002 820 897 849 833 017 485 552 117 968 451 495 896 825 3  
 781 376 804 007 044 999 823 350 391 622 143 031 967 019 420 089 785 458 615 970 181 966 436 559 184 3  
 249 506 230 272 000  $q^{5009} +$   
 2 829 372 021 687 357 359 954 844 917 428 050 463 791 346 165 194 090 671 262 056 694 882 148 971 875 3  
 018 639 482 353 208 788 170 982 672 601 450 124 538 643 632 079 237 807 875 830 911 031 780 557 882 3  
 293 837 976 780 800  $q^{5012} -$   
 2 939 923 396 120 581 494 268 864 256 472 501 102 137 693 130 498 015 325 282 196 545 858 401 109 116 3  
 232 589 525 782 158 456 294 914 397 666 181 206 538 971 499 836 051 365 148 088 128 982 513 628 142 3  
 122 178 959 192 302  $q^{5013} +$   
 3 298 101 068 814 547 808 373 621 261 235 878 263 472 003 743 116 856 549 644 929 033 678 845 025 185 3  
 580 729 557 254 796 518 317 142 098 094 433 010 401 422 299 971 828 060 338 437 455 504 750 116 915 3  
 779 295 968 000 000  $q^{5016} -$   
 3 426 914 739 389 844 259 761 666 953 699 999 338 434 203 335 020 741 701 948 396 254 161 763 513 993 3  
 051 606 868 975 497 982 810 525 273 340 040 926 481 186 204 827 756 918 970 229 247 500 682 028 237 3

$280\ 539\ 823\ 702\ 016\ q^{5017} +$   
 $3\ 844\ 247\ 986\ 409\ 469\ 397\ 783\ 280\ 181\ 059\ 150\ 331\ 009\ 753\ 066\ 056\ 440\ 741\ 536\ 400\ 073\ 060\ 432\ 957\ 570\ 641\ 521\ 594\ 429\ 104\ 989\ 675\ 419\ 228\ 916\ 900\ 437\ 934\ 103\ 818\ 469\ 835\ 747\ 551\ 273\ 006\ 903\ 856\ 317\ 193\ 361\ 775\ 923\ 046\ 400\ q^{5020} -$   
 $3\ 994\ 331\ 654\ 804\ 383\ 240\ 608\ 616\ 850\ 473\ 769\ 614\ 591\ 500\ 597\ 170\ 029\ 060\ 139\ 142\ 975\ 931\ 011\ 370\ 226\ 489\ 582\ 040\ 700\ 298\ 193\ 755\ 282\ 384\ 978\ 286\ 440\ 006\ 594\ 877\ 126\ 124\ 487\ 288\ 844\ 310\ 415\ 312\ 224\ 687\ 652\ 985\ 254\ 259\ 375\ q^{5021} +$   
 $4\ 480\ 560\ 977\ 028\ 620\ 471\ 003\ 169\ 984\ 845\ 144\ 196\ 135\ 757\ 074\ 520\ 967\ 399\ 974\ 495\ 005\ 653\ 374\ 923\ 142\ 755\ 400\ 997\ 598\ 639\ 178\ 647\ 345\ 127\ 939\ 662\ 128\ 631\ 155\ 353\ 459\ 033\ 752\ 404\ 023\ 117\ 634\ 531\ 169\ 531\ 552\ 525\ 107\ 712\ 000\ q^{5024} -$   
 $4\ 655\ 416\ 204\ 093\ 395\ 438\ 941\ 265\ 256\ 191\ 052\ 901\ 874\ 184\ 843\ 959\ 303\ 477\ 662\ 767\ 610\ 439\ 100\ 298\ 616\ 968\ 226\ 669\ 872\ 897\ 790\ 130\ 097\ 491\ 716\ 594\ 584\ 598\ 366\ 646\ 629\ 686\ 136\ 797\ 287\ 241\ 910\ 457\ 788\ 670\ 888\ 041\ 059\ 942\ 400\ q^{5025} +$   
 $5\ 221\ 881\ 130\ 888\ 740\ 211\ 439\ 862\ 341\ 991\ 909\ 295\ 063\ 520\ 246\ 377\ 786\ 352\ 661\ 790\ 982\ 853\ 830\ 533\ 067\ 786\ 383\ 488\ 209\ 214\ 063\ 433\ 392\ 406\ 055\ 835\ 027\ 964\ 152\ 127\ 298\ 560\ 917\ 259\ 612\ 385\ 484\ 787\ 853\ 927\ 809\ 835\ 528\ 896\ 512\ q^{5028} -$   
 $5\ 425\ 584\ 183\ 166\ 967\ 010\ 488\ 333\ 978\ 069\ 931\ 895\ 831\ 504\ 962\ 922\ 087\ 683\ 666\ 490\ 005\ 750\ 976\ 134\ 272\ 422\ 096\ 835\ 337\ 483\ 343\ 920\ 646\ 688\ 108\ 533\ 831\ 519\ 286\ 764\ 277\ 177\ 401\ 262\ 788\ 078\ 085\ 465\ 511\ 522\ 623\ 307\ 864\ 810\ 000\ q^{5029} +$   
 $6\ 085\ 484\ 982\ 956\ 369\ 869\ 656\ 984\ 973\ 226\ 639\ 752\ 499\ 250\ 629\ 495\ 219\ 226\ 154\ 705\ 038\ 783\ 626\ 487\ 763\ 343\ 640\ 220\ 895\ 439\ 233\ 349\ 981\ 291\ 111\ 250\ 117\ 783\ 632\ 117\ 705\ 065\ 439\ 780\ 549\ 386\ 340\ 438\ 871\ 275\ 669\ 324\ 994\ 962\ 432\ q^{5032} -$   
 $6\ 322\ 780\ 874\ 231\ 523\ 680\ 628\ 607\ 014\ 425\ 008\ 239\ 130\ 476\ 258\ 742\ 809\ 692\ 679\ 592\ 167\ 416\ 088\ 289\ 151\ 990\ 422\ 352\ 251\ 106\ 581\ 978\ 697\ 082\ 679\ 433\ 275\ 594\ 433\ 747\ 016\ 954\ 076\ 337\ 159\ 325\ 096\ 756\ 116\ 419\ 067\ 132\ 822\ 224\ 896\ q^{5033} +$   
 $7\ 091\ 482\ 969\ 926\ 087\ 856\ 525\ 132\ 760\ 675\ 337\ 683\ 468\ 241\ 306\ 874\ 085\ 175\ 058\ 415\ 989\ 123\ 715\ 184\ 508\ 117\ 163\ 445\ 175\ 692\ 039\ 889\ 121\ 463\ 125\ 865\ 532\ 107\ 747\ 205\ 687\ 435\ 473\ 106\ 599\ 564\ 056\ 121\ 380\ 717\ 032\ 459\ 570\ 368\ 000\ q^{5036} -$   
 $7\ 367\ 894\ 844\ 886\ 323\ 758\ 496\ 435\ 491\ 823\ 510\ 533\ 092\ 734\ 118\ 623\ 842\ 160\ 186\ 960\ 643\ 890\ 158\ 344\ 065\ 190\ 093\ 686\ 928\ 241\ 491\ 779\ 311\ 271\ 543\ 222\ 953\ 413\ 821\ 990\ 619\ 165\ 023\ 857\ 026\ 034\ 649\ 169\ 558\ 017\ 935\ 554\ 296\ 467\ 967\ q^{5037} +$   
 $8\ 263\ 282\ 881\ 627\ 298\ 920\ 708\ 754\ 027\ 258\ 874\ 487\ 288\ 823\ 861\ 344\ 234\ 619\ 479\ 204\ 163\ 435\ 222\ 575\ 889\ 651\ 038\ 779\ 785\ 713\ 391\ 485\ 822\ 202\ 505\ 973\ 945\ 519\ 995\ 918\ 445\ 000\ 235\ 418\ 365\ 820\ 148\ 550\ 084\ 702\ 915\ 700\ 747\ 673\ 600\ q^{5040} -$   
 $8\ 585\ 239\ 237\ 065\ 076\ 657\ 366\ 412\ 159\ 263\ 851\ 381\ 446\ 768\ 766\ 534\ 739\ 886\ 283\ 184\ 929\ 232\ 749\ 030\ 395\ 716\ 382\ 046\ 027\ 190\ 056\ 207\ 162\ 103\ 721\ 551\ 604\ 876\ 117\ 465\ 845\ 680\ 657\ 502\ 043\ 912\ 905\ 235\ 669\ 898\ 718\ 209\ 024\ 000\ 248\ q^{5041} +$   
 $9\ 628\ 128\ 876\ 573\ 284\ 321\ 085\ 535\ 685\ 349\ 823\ 220\ 885\ 813\ 038\ 963\ 867\ 938\ 133\ 773\ 779\ 091\ 979\ 850\ 227\ 586\ 964\ 703\ 649\ 259\ 542\ 442\ 895\ 158\ 717\ 077\ 161\ 395\ 394\ 639\ 855\ 629\ 152\ 157\ 524\ 928\ 209\ 943\ 039\ 903\ 392\ 751\ 266\ 304\ 000\ q^{5044} -$   
 $10\ 003\ 111\ 520\ 199\ 695\ 282\ 423\ 080\ 722\ 799\ 195\ 700\ 020\ 634\ 294\ 206\ 124\ 776\ 339\ 153\ 925\ 514\ 924\ 385\ 229\ 582\ 429\ 997\ 138\ 856\ 191\ 306\ 832\ 555\ 945\ 522\ 503\ 110\ 966\ 510\ 710\ 241\ 778\ 868\ 719\ 623\ 573\ 995\ 013\ 307\ 252\ 044\ 229\ 251\ 100\ q^{5045} +$   
 $11\ 217\ 728\ 345\ 100\ 922\ 686\ 747\ 752\ 471\ 421\ 363\ 271\ 578\ 925\ 766\ 193\ 509\ 936\ 625\ 278\ 589\ 321\ 790\ 886\ 061\ 402\ 078\ 207\ 220\ 617\ 393\ 680\ 034\ 339\ 878\ 765\ 144\ 152\ 616\ 634\ 638\ 573\ 307\ 523\ 409\ 956\ 686\ 445\ 424\ 323\ 894\ 660\ 142\ 097\ 408\ q^{5048} -$   
 $11\ 654\ 444\ 462\ 142\ 105\ 422\ 273\ 004\ 193\ 759\ 475\ 154\ 630\ 536\ 942\ 450\ 273\ 403\ 472\ 220\ 789\ 445\ 135\ 876\ 126\ 409\ 577\ 311\ 670\ 034\ 601\ 720\ 650\ 421\ 423\ 445\ 599\ 286\ 301\ 566\ 713\ 079\ 828\ 999\ 487\ 860\ 117\ 449\ 687\ 107\ 539\ 070\ 418\ 944\ 000\ q^{5049} +$   
 $13\ 068\ 980\ 894\ 308\ 648\ 408\ 865\ 968\ 895\ 952\ 610\ 827\ 139\ 843\ 341\ 539\ 198\ 573\ 154\ 998\ 964\ 180\ 984\ 019\ 654\ 437\ 401\ 449\ 085\ 620\ 683\ 228\ 564\ 682\ 573\ 534\ 105\ 909\ 367\ 864\ 211\ 309\ 083\ 355\ 792\ 032\ 246\ 466\ 958\ 394\ 167\ 699\ 349\ 686\ 272\ q^{5052} -$   
 $13\ 577\ 563\ 138\ 109\ 166\ 741\ 132\ 632\ 469\ 238\ 003\ 796\ 665\ 240\ 325\ 822\ 333\ 805\ 366\ 900\ 062\ 031\ 265\ 537\ 943\ 196\ 808\ 114\ 904\ 899\ 120\ 217\ 961\ 460\ 745\ 458\ 491\ 728\ 781\ 593\ 075\ 403\ 759\ 631\ 557\ 282\ 348\ 170\ 042\ 816\ 436\ 931\ 676\ 609\ 730\ q^{5053} +$

15 224 826 041 430 350 573 549 720 441 029 197 574 173 088 151 346 159 635 070 342 489 179 895 945 \\  
 446 849 515 368 094 104 699 988 102 420 594 383 122 332 239 125 629 549 161 603 016 496 104 410 324 \\  
 604 956 907 831 296 000  $q^{5056}$  -

15 817 065 198 556 412 037 459 214 030 382 271 488 617 517 027 994 588 608 561 170 365 386 249 970 \\  
 264 361 965 757 935 445 524 861 275 698 017 437 039 088 164 532 875 620 816 262 971 360 540 692 422 \\  
 852 023 947 695 751 168  $q^{5057}$  +

17 735 228 888 204 419 138 230 931 148 413 534 567 065 817 641 336 322 838 431 824 292 278 680 549 \\  
 118 925 067 887 271 183 319 787 254 768 688 420 318 045 202 464 634 448 458 185 393 262 867 811 887 \\  
 947 554 053 030 707 200  $q^{5060}$  -

18 424 844 405 225 198 836 384 666 093 897 818 281 659 632 091 222 831 025 739 402 505 413 376 218 \\  
 087 023 289 005 834 160 884 660 703 486 469 464 305 888 374 446 382 771 032 672 427 939 726 161 244 \\  
 834 469 071 742 327 250  $q^{5061}$  +

20 658 326 168 353 521 072 885 285 579 879 832 621 406 896 463 989 708 557 771 143 471 906 439 913 \\  
 205 689 955 415 847 714 633 259 524 212 030 294 268 304 956 741 779 298 744 552 609 408 245 419 015 \\  
 714 044 543 575 808 000  $q^{5064}$  -

21 461 280 683 069 746 514 188 480 670 214 489 345 192 366 276 802 361 364 819 321 868 615 858 103 \\  
 647 255 694 791 356 300 361 757 384 440 533 232 631 783 025 023 928 561 105 908 108 557 531 213 950 \\  
 734 737 444 144 742 400  $q^{5065}$  +

24 061 758 683 281 369 915 183 908 104 245 857 174 177 208 580 865 059 296 584 704 254 770 375 810 \\  
 130 838 275 144 516 752 081 800 385 057 731 811 277 868 565 542 881 640 982 328 476 323 738 770 793 \\  
 899 464 888 578 718 720  $q^{5068}$  -

24 996 623 696 801 299 633 973 639 149 555 961 138 303 923 578 929 266 468 180 963 759 733 485 985 \\  
 370 591 576 742 613 180 354 818 825 586 752 547 466 072 236 147 999 942 756 904 202 187 836 550 125 \\  
 193 613 920 406 142 125  $q^{5069}$  +

28 024 220 348 518 698 150 312 111 357 192 723 585 601 003 487 207 700 786 323 702 114 751 587 584 \\  
 797 985 966 082 515 869 475 615 188 234 816 630 055 801 400 142 766 188 039 918 674 968 960 582 431 \\  
 764 386 943 879 331 840  $q^{5072}$  -

29 112 601 328 457 244 491 560 377 191 659 414 531 560 884 107 463 675 501 084 429 628 791 811 476 \\  
 159 578 789 258 465 381 019 650 508 707 828 084 893 280 501 607 591 652 373 116 348 063 946 643 333 \\  
 939 216 800 308 396 032  $q^{5073}$  +

32 637 258 959 306 602 639 569 519 709 509 288 420 972 886 460 392 947 432 533 198 651 282 065 566 \\  
 287 543 476 357 426 660 792 202 652 620 853 511 839 282 836 946 662 163 062 626 719 400 184 426 055 \\  
 991 697 418 350 592 000  $q^{5076}$  -

33 904 289 504 269 206 007 833 642 339 643 056 242 788 123 522 413 185 987 586 276 140 056 661 041 \\  
 826 449 645 736 092 835 746 280 682 887 039 910 952 512 529 779 917 969 631 276 849 665 437 899 454 \\  
 781 097 616 035 150 552  $q^{5077}$  +

38 007 369 457 058 115 588 048 997 114 893 225 964 296 446 788 091 699 141 091 373 443 496 193 666 \\  
 995 337 434 900 442 520 417 269 319 487 951 246 490 600 544 693 035 612 234 160 416 852 708 973 011 \\  
 791 109 871 983 692 800  $q^{5080}$  -

39 482 285 708 363 111 502 271 560 898 955 281 013 797 713 941 791 382 661 103 408 572 946 224 743 \\  
 260 825 527 708 140 897 645 513 040 090 125 053 866 892 948 353 360 563 177 720 048 540 720 924 839 \\  
 060 543 777 787 904 000  $q^{5081}$  +

44 258 427 065 836 468 142 737 717 663 800 935 833 926 777 815 667 069 224 854 601 320 137 610 956 \\  
 401 870 643 517 511 830 576 866 387 762 319 351 785 042 614 766 275 365 812 641 685 383 233 121 996 \\  
 420 470 842 467 328 000  $q^{5084}$  -

45 975 235 358 814 740 912 478 936 451 404 888 834 437 281 653 360 910 252 680 404 793 637 849 349 \\  
 806 221 524 993 050 234 555 788 841 810 883 686 904 381 307 262 464 235 238 412 756 334 108 653 062 \\  
 160 829 946 165 362 875  $q^{5085}$  +

51 534 515 316 254 385 623 418 845 086 714 468 687 835 567 645 240 051 917 896 865 018 433 444 602 \\  
 592 736 482 294 368 488 610 555 776 867 826 430 726 585 107 039 835 758 935 325 548 660 710 090 716 \\  
 075 688 073 568 100 352  $q^{5088}$  -

53 532 768 160 685 681 244 154 689 023 559 717 570 725 380 575 831 611 344 282 517 305 131 978 165 \\  
 846 851 269 095 186 003 119 696 802 364 666 463 360 674 547 765 065 737 755 079 593 224 601 748 953 \\  
 141 269 007 302 656 000  $q^{5089}$  +

60 003 212 853 670 027 738 800 141 419 463 207 673 747 890 229 125 810 982 360 221 259 162 570 852 \

569 684 050 267 290 886 443 248 008 427 826 039 457 302 784 826 740 449 945 209 338 939 113 635 978 \
 506 689 987 268 198 400  $q^{5092}$  -

62 328 910 767 657 253 235 645 968 591 009 620 775 093 677 341 612 548 349 360 043 049 851 327 228 \
 657 937 160 865 585 038 714 377 711 820 836 794 455 057 226 896 278 867 585 666 311 320 256 642 712 \
 592 601 396 555 792 891  $q^{5093}$  +

69 859 413 235 837 335 567 099 665 564 977 475 646 553 323 896 873 333 555 771 888 463 135 629 082 \
 400 472 492 785 012 292 039 147 028 367 145 977 469 193 061 942 665 915 845 639 379 754 397 637 408 \
 426 526 935 280 320 000  $q^{5096}$  -

72 566 052 783 841 141 763 176 503 937 605 721 027 305 090 751 360 347 940 839 221 523 371 694 968 \
 826 910 415 908 274 567 611 346 813 971 032 545 669 412 885 599 738 639 334 940 031 870 809 641 344 \
 090 817 980 158 869 504  $q^{5097}$  +

81 329 763 891 487 576 351 593 360 222 129 810 675 944 688 653 091 202 176 280 804 485 288 232 932 \
 011 684 469 461 125 528 249 267 229 353 622 584 167 480 179 200 069 434 564 897 582 457 963 766 956 \
 372 933 247 954 150 400  $q^{5100}$  -

84 479 555 558 165 182 514 689 477 034 997 492 722 171 414 099 662 585 604 273 480 356 532 979 163 \
 633 024 302 032 183 879 114 985 187 056 010 235 280 375 494 712 949 118 502 685 895 022 903 146 818 \
 071 698 005 708 425 750  $q^{5101}$  +

94 677 824 301 566 108 176 983 558 082 599 737 366 304 251 910 230 196 048 992 411 152 864 800 263 \
 429 647 500 247 022 053 561 422 817 471 109 685 245 039 190 612 404 507 683 471 847 953 512 012 396 \
 852 884 986 718 208 000  $q^{5104}$  -

98 343 107 641 348 317 469 645 270 480 243 044 229 272 712 127 572 524 773 420 384 461 088 866 158 \
 567 841 600 782 330 836 354 548 246 443 200 190 108 508 908 236 176 291 899 568 540 753 149 857 470 \
 458 511 647 734 169 600  $q^{5105}$  +

110 210 059 587 427 684 616 117 282 173 680 431 229 606 072 699 355 531 367 441 197 640 438 601 517 \
 295 528 167 311 664 627 623 901 207 544 728 704 743 372 240 029 507 292 831 707 167 601 620 747 294 \
 848 534 974 982 129 664  $q^{5108}$  -

114 474 947 509 941 641 385 195 505 138 453 353 385 605 948 332 828 565 467 807 617 130 497 994 403 \
 335 363 686 054 445 269 370 859 884 800 213 663 270 129 267 966 729 911 393 759 374 961 338 857 847 \
 481 739 359 734 526 000  $q^{5109}$  +

128 282 804 402 898 337 816 929 678 230 052 718 729 951 313 670 234 912 799 954 363 457 992 169 546 \
 133 285 492 108 224 874 070 938 317 234 404 327 642 022 833 952 812 676 242 780 019 363 813 310 213 \
 509 089 506 229 330 944  $q^{5112}$  -

133 245 093 584 420 009 372 354 840 823 624 787 238 277 203 822 931 025 647 461 733 325 137 807 009 \
 801 308 146 937 346 031 370 795 522 854 928 974 364 894 176 043 874 332 882 845 584 301 972 752 966 \
 458 192 211 003 801 600  $q^{5113}$  +

149 310 353 744 578 900 817 608 220 017 407 837 337 637 688 368 170 761 227 683 241 064 489 501 974 \
 056 489 136 959 810 753 396 148 247 182 367 541 649 582 870 687 689 756 993 120 786 410 627 171 663 \
 657 990 777 477 120 000  $q^{5116}$  -

155 083 744 109 352 927 254 691 667 991 971 841 787 285 075 644 490 576 505 837 648 235 394 360 994 \
 240 715 365 311 768 141 654 520 097 104 575 192 051 789 658 846 589 687 939 118 210 246 149 748 059 \
 493 932 125 929 023 301  $q^{5117}$  +

173 774 362 498 176 790 485 791 698 093 770 401 217 715 384 722 078 727 369 896 735 832 966 429 308 \
 528 440 514 561 071 289 474 751 888 354 677 528 067 658 197 111 928 155 250 478 144 318 122 971 638 \
 190 536 712 016 363 520  $q^{5120}$  -

180 491 035 622 494 749 592 856 217 405 167 986 288 452 764 393 556 101 889 692 323 531 904 550 785 \
 071 469 823 431 815 814 145 488 790 556 883 002 565 502 446 589 615 758 933 076 178 944 780 636 400 \
 769 757 783 146 496 000  $q^{5121}$  +

202 234 764 785 883 601 365 452 744 354 511 150 419 769 082 718 263 454 366 849 944 221 487 720 030 \
 130 824 099 380 632 314 237 830 621 976 958 421 194 306 882 713 823 815 474 707 262 011 788 819 316 \
 319 753 302 257 664 000  $q^{5124}$  -

210 048 379 095 124 233 771 146 082 197 747 423 781 154 452 693 424 714 948 431 918 648 321 345 607 \
 926 237 534 790 052 369 874 603 490 362 707 225 808 531 736 411 344 790 043 796 342 970 318 076 429 \
 758 663 275 651 189 000  $q^{5125}$  +

235 342 458 117 755 312 362 276 573 494 596 965 518 013 696 971 270 264 996 477 399 770 923 466 504 \
 681 911 053 065 357 827 886 890 457 727 444 108 890 270 132 909 213 506 213 038 465 613 520 472 506

735 336 707 341 677 568  $q^{5128}$  -  
 244 431 628 049 405 206 447 530 721 647 801 904 217 892 417 095 669 424 557 556 072 308 684 819 772  
 414 523 288 722 831 142 697 591 495 501 110 118 718 817 028 338 214 867 274 839 442 936 771 938 151  
 608 529 185 955 840 000  $q^{5129}$  +  
 273 854 036 728 763 362 632 123 946 814 547 803 055 051 279 131 899 424 025 059 527 469 907 366 904  
 660 693 969 345 097 271 375 626 308 511 524 615 102 998 643 189 806 412 409 248 603 389 733 877 305  
 289 692 002 358 119 936  $q^{5132}$  -  
 284 426 373 828 259 536 942 286 825 302 987 578 573 514 180 416 216 096 845 682 316 539 071 515 710  
 502 102 238 811 601 089 190 780 897 840 689 284 590 860 479 827 340 852 076 465 539 590 383 869 757  
 928 655 443 788 678 958  $q^{5133}$  +  
 318 648 904 172 314 192 343 513 206 251 559 557 384 446 998 722 494 452 590 381 615 710 387 465 799  
 442 312 310 418 014 182 457 471 279 321 816 996 539 101 412 388 283 674 675 504 737 729 124 237 204  
 484 901 264 343 040 000  $q^{5136}$  -  
 330 945 710 611 641 754 537 590 084 613 063 475 792 283 034 777 362 758 162 391 461 426 823 030 692  
 677 908 934 659 130 477 705 048 592 785 984 346 788 193 042 522 177 031 743 732 112 736 520 600 605  
 850 855 249 646 157 824  $q^{5137}$  +  
 370 749 148 248 817 701 339 657 598 388 050 791 404 455 073 247 608 757 946 934 265 446 887 549 209  
 944 318 513 636 743 433 632 435 904 988 853 069 872 714 177 071 224 518 997 728 078 816 369 786 621  
 591 094 967 391 744 000  $q^{5140}$  -  
 385 050 867 786 377 740 918 028 021 025 550 763 274 934 684 849 098 778 580 032 907 990 656 111 747  
 258 291 189 881 865 316 509 260 883 576 627 250 729 917 984 621 233 186 910 753 263 163 945 390 549  
 861 333 708 331 593 500  $q^{5141}$  +  
 431 342 622 843 167 661 628 264 284 784 731 208 603 530 422 021 636 430 516 533 592 761 311 064 107  
 384 177 263 145 785 353 592 367 093 326 104 028 631 195 069 694 492 738 240 565 069 787 707 702 492  
 784 414 262 633 664 000  $q^{5144}$  -  
 447 975 171 097 714 871 334 158 190 467 159 753 824 138 879 007 494 348 486 796 654 443 803 175 537  
 277 037 710 660 279 810 981 839 763 001 371 681 911 409 232 683 805 121 112 538 332 223 152 478 919  
 163 013 871 055 667 200  $q^{5145}$  +  
 501 809 752 582 745 317 810 016 940 928 806 095 891 446 892 146 293 038 433 751 288 129 097 388 759  
 457 637 277 604 331 857 870 687 338 857 438 372 341 917 531 745 511 735 840 259 500 053 246 372 992  
 698 483 715 799 848 960  $q^{5148}$  -  
 521 151 868 045 369 461 611 638 182 404 006 681 548 762 262 283 720 711 890 453 357 601 154 653 277  
 069 093 652 140 967 816 527 188 788 959 489 672 180 705 110 177 154 634 450 733 503 624 529 613 527  
 702 511 071 511 626 375  $q^{5149}$  +  
 583 754 658 978 405 390 949 231 987 975 934 580 870 843 885 117 742 165 178 923 414 654 537 361 971  
 487 530 573 566 621 157 042 231 420 792 554 330 438 160 314 351 961 488 664 278 111 127 792 972 718  
 210 729 062 352 142 336  $q^{5152}$  -  
 606 246 438 864 850 339 689 498 953 217 293 266 761 188 951 456 430 086 445 821 146 186 660 458 124  
 023 596 086 811 461 600 437 469 593 292 756 736 493 188 544 273 378 762 380 864 290 692 448 730 655  
 282 530 268 696 182 784  $q^{5153}$  +  
 679 041 302 695 379 772 173 115 798 193 833 435 009 026 138 361 653 950 023 564 624 665 908 375 414  
 813 330 583 447 995 479 961 106 567 575 868 378 291 844 957 256 377 514 173 881 190 749 289 447 798  
 259 491 326 183 424 000  $q^{5156}$  -  
 705 194 114 045 151 245 880 551 050 045 482 551 759 317 007 282 181 546 891 698 891 749 020 376 711  
 663 283 336 601 103 771 775 302 661 578 082 864 853 867 248 218 695 603 968 792 606 191 298 618 806  
 028 626 699 002 926 469  $q^{5157}$  +  
 789 835 447 929 202 094 295 562 743 089 819 818 960 913 171 730 723 836 918 422 586 555 134 367 728  
 207 024 141 015 442 794 340 408 001 635 554 651 486 881 563 861 172 602 594 585 789 877 407 775 801  
 012 907 785 732 710 400  $q^{5160}$  -  
 820 243 434 865 895 258 787 780 327 330 516 522 496 128 782 954 273 489 916 831 368 591 537 948 381  
 330 381 488 554 387 748 640 269 115 811 235 638 880 522 002 221 123 798 621 720 537 674 086 881 964  
 703 650 147 262 464 000  $q^{5161}$  +  
 918 653 383 979 126 343 268 216 129 844 452 893 806 600 505 892 175 887 947 772 900 132 845 817 498  
 210 787 641 007 657 239 677 117 296 977 573 690 467 624 941 384 460 857 020 148 488 288 457 132 294  
 458 780 070 210 880 000  $q^{5164}$  -

954 006 827 428 053 765 352 183 352 106 166 640 591 279 662 082 313 727 831 097 297 201 923 255 367 \
 658 380 399 352 476 968 110 582 821 892 159 176 415 449 288 680 813 293 806 276 454 552 249 140 504 \
 551 733 048 585 451 825  $q^{5165} +$

1 068 418 488 852 210 989 278 551 273 464 007 222 013 077 875 473 008 184 300 888 866 289 386 870 656 \
 344 457 186 306 310 215 032 216 668 668 372 121 898 315 800 558 869 874 399 060 897 686 111 568 196 \
 548 940 838 104 547 328  $q^{5168} -$

1 109 519 316 042 995 750 179 687 028 165 860 056 909 099 868 550 008 251 817 723 439 175 170 153 199 \
 889 975 125 464 314 308 106 980 082 141 654 829 786 644 995 174 099 305 093 455 042 105 617 604 975 \
 513 583 851 106 304 000  $q^{5169} +$

1 242 526 893 379 581 249 689 481 519 120 584 625 913 840 789 856 271 264 016 768 681 156 148 379 586 \
 271 263 337 336 367 318 218 080 071 758 820 671 845 403 284 374 787 063 868 218 785 761 125 170 600 \
 889 259 029 897 633 792  $q^{5172} -$

1 290 306 682 042 440 443 733 138 030 121 984 786 791 913 896 946 560 238 597 197 534 781 229 979 158 \
 464 962 599 950 409 564 394 953 786 032 220 018 225 079 056 324 811 165 350 138 999 230 831 355 599 \
 647 275 629 225 621 842  $q^{5173} +$

1 444 923 705 688 167 482 804 089 036 204 180 618 478 718 630 719 117 156 810 291 686 525 973 366 682 \
 633 832 592 714 581 747 880 716 687 076 284 529 284 830 535 591 216 101 534 171 751 902 135 971 650 \
 150 935 119 349 120 000  $q^{5176} -$

1 500 464 583 025 483 673 199 607 726 163 933 059 212 432 256 115 217 843 086 147 617 376 145 414 609 \
 175 103 145 432 659 161 020 569 118 749 041 428 899 974 005 024 064 904 309 755 228 865 047 261 153 \
 393 395 440 216 113 152  $q^{5177} +$

1 680 191 489 356 293 124 345 322 363 553 095 635 917 374 727 264 053 823 354 731 239 386 967 444 865 \
 982 191 231 302 346 642 121 138 792 188 964 289 542 597 072 175 509 313 420 434 350 724 153 241 619 \
 462 607 063 406 080 000  $q^{5180} -$

1 744 750 389 843 486 382 898 819 279 112 016 084 592 496 155 844 187 445 822 629 096 521 214 592 119 \
 829 309 910 278 796 727 942 653 891 479 856 596 849 157 362 828 151 949 361 464 239 661 069 059 492 \
 469 523 130 204 197 250  $q^{5181} +$

1 953 652 959 299 329 628 980 310 068 800 662 332 888 739 361 243 854 634 464 144 438 302 024 415 845 \
 163 248 570 942 505 654 361 263 503 272 971 208 612 410 940 950 395 018 849 135 819 050 350 117 683 \
 777 861 174 597 066 752  $q^{5184} -$

2 028 689 779 540 293 215 236 817 922 293 553 487 031 561 324 072 526 850 220 145 080 252 954 142 945 \
 592 301 407 291 253 729 876 151 029 555 323 701 044 395 384 123 111 670 888 736 519 598 416 677 844 \
 697 903 122 933 350 400  $q^{5185} +$

2 271 490 173 302 030 480 155 601 724 643 373 808 992 811 770 459 184 997 592 758 823 418 963 959 861 \
 380 297 899 300 584 092 410 874 579 931 014 915 532 438 053 161 988 078 110 518 738 438 565 494 823 \
 850 470 706 300 305 408  $q^{5188} -$

2 358 700 448 155 628 003 670 532 159 183 296 954 543 001 613 803 947 828 139 002 152 767 497 321 476 \
 081 310 680 201 931 466 344 626 776 473 052 266 865 704 489 322 868 948 936 998 660 657 610 074 209 \
 342 831 325 107 577 500  $q^{5189} +$

2 640 882 860 995 311 718 120 639 862 315 490 253 937 984 779 256 160 356 260 703 509 374 490 335 052 \
 967 485 942 545 499 831 450 996 731 771 977 261 469 796 120 712 020 459 567 284 739 141 571 454 112 \
 220 504 292 083 349 504  $q^{5192} -$

2 742 235 684 878 729 291 030 894 755 226 012 993 062 121 270 971 644 633 474 231 516 147 253 166 035 \
 049 506 125 120 598 527 124 856 528 749 266 746 537 186 412 574 603 852 261 929 417 377 567 580 302 \
 225 035 767 703 470 080  $q^{5193} +$

3 070 168 953 912 125 493 482 974 196 808 222 116 775 926 590 225 434 218 060 979 144 373 373 907 057 \
 443 029 204 178 590 987 115 491 735 259 829 374 079 360 615 229 108 040 529 399 863 994 015 952 279 \
 546 308 677 769 216 000  $q^{5196} -$

3 187 950 986 749 831 894 137 471 238 534 785 877 724 246 306 663 326 294 087 972 650 092 669 136 000 \
 755 178 486 168 550 544 486 184 568 931 784 693 685 066 209 995 707 318 716 026 859 411 658 895 355 \
 443 797 649 023 480 545  $q^{5197} +$

3 569 030 869 253 090 142 152 455 377 387 882 865 662 459 514 528 104 146 718 644 703 160 128 972 570 \
 958 184 917 461 125 575 157 343 782 831 636 608 595 850 431 194 059 026 518 503 729 748 470 887 120 \
 075 536 501 883 289 600  $q^{5200} -$

3 705 897 400 496 906 137 278 922 593 019 911 421 475 254 726 342 895 612 795 889 982 083 202 881 514 \

601 422 867 087 314 159 538 710 321 398 189 386 975 170 178 415 431 717 246 846 791 526 234 705 107 3  
 032 890 157 039 616 000  $q^{5201} +$   
 4 148 711 666 808 306 659 742 704 544 616 920 424 413 115 314 342 958 543 128 908 899 370 913 238 530 3  
 174 583 949 146 545 949 768 602 254 219 076 645 820 313 699 754 592 994 421 443 568 232 462 633 649 3  
 012 842 983 237 888 000  $q^{5204} -$   
 4 307 745 866 223 664 440 934 922 774 261 348 922 048 844 166 229 060 756 811 308 210 138 382 519 795 3  
 309 032 885 452 146 697 308 174 781 429 852 043 966 386 583 087 811 723 233 118 712 825 671 522 578 3  
 505 830 882 422 878 125  $q^{5205} +$   
 4 822 265 855 465 156 903 603 662 593 024 473 659 780 846 814 989 736 945 957 215 124 869 146 288 623 3  
 272 444 019 592 204 381 716 941 835 006 447 114 782 765 468 105 838 922 774 918 920 218 667 370 141 3  
 165 711 367 037 112 320  $q^{5208} -$   
 5 007 047 519 341 963 325 410 146 050 932 800 298 322 861 567 980 482 092 734 760 120 252 518 591 738 3  
 883 067 518 349 882 257 798 891 435 171 124 625 614 703 553 132 290 502 613 814 215 166 988 554 378 3  
 099 726 487 138 304 000  $q^{5209} +$   
 5 604 850 387 184 180 772 263 492 813 239 114 512 779 478 399 367 733 914 969 651 015 794 519 066 999 3  
 340 228 638 564 637 614 107 437 398 867 121 944 075 130 210 561 950 764 794 107 139 377 174 281 003 3  
 911 440 722 041 116 672  $q^{5212} -$   
 5 819 535 697 203 450 478 533 719 329 355 839 524 240 779 853 830 180 708 811 156 957 249 873 564 944 3  
 003 506 239 118 018 423 565 930 890 790 596 402 992 827 627 600 622 059 583 916 265 713 152 563 186 3  
 804 988 166 742 636 283  $q^{5213} +$   
 6 514 062 258 809 333 610 869 853 496 991 517 358 888 421 780 433 723 040 350 948 042 807 656 963 477 3  
 166 013 136 800 850 375 059 579 529 232 588 596 631 455 314 123 524 765 467 395 171 684 563 436 501 3  
 041 666 915 589 632 000  $q^{5216} -$   
 6 763 476 312 513 671 707 363 641 553 934 093 663 711 085 365 648 473 215 630 674 858 186 845 775 195 3  
 841 181 335 786 930 819 157 574 151 417 177 111 413 644 906 323 287 752 383 142 380 055 856 094 855 3  
 686 338 981 209 047 040  $q^{5217} +$   
 7 570 330 164 776 228 009 206 294 791 568 302 377 148 859 744 401 603 509 523 017 927 425 670 221 486 3  
 850 906 147 212 413 271 679 855 244 298 566 323 442 024 503 464 743 026 262 322 832 942 386 716 610 3  
 959 422 480 117 760 000  $q^{5220} -$   
 7 860 074 316 704 721 769 389 401 898 481 986 162 804 930 319 598 705 093 799 995 791 731 340 259 699 3  
 253 036 664 985 433 373 662 160 837 845 277 311 520 230 678 149 045 792 722 323 996 801 841 723 942 3  
 021 353 649 249 299 375  $q^{5221} +$   
 8 797 368 828 904 459 159 283 174 243 733 828 644 000 556 619 453 034 270 974 578 927 448 221 587 402 3  
 224 469 996 375 658 648 173 660 837 468 267 214 214 443 057 936 119 960 825 785 966 036 951 774 654 3  
 813 881 387 582 912 000  $q^{5224} -$   
 9 133 945 206 041 580 136 116 537 005 767 600 015 078 051 702 100 429 264 967 197 608 380 951 927 116 3  
 464 309 888 006 558 357 646 805 251 101 809 907 836 904 103 485 063 910 238 368 350 788 554 841 943 3  
 765 298 385 968 332 800  $q^{5225} +$   
 10 222 706 016 728 304 316 459 446 830 275 180 559 524 479 965 998 367 954 970 606 870 237 027 527 3  
 201 575 073 512 856 388 803 499 781 576 339 192 607 517 416 538 877 818 978 711 136 331 329 880 708 3  
 944 013 053 630 087 239 168  $q^{5228} -$   
 10 613 661 948 023 281 809 553 850 540 624 177 997 061 344 734 494 528 383 020 453 709 354 032 330 3  
 909 371 048 299 426 361 015 446 805 825 344 145 059 414 539 288 350 561 141 200 765 483 831 785 212 3  
 280 429 140 531 394 666 250  $q^{5229} +$   
 11 878 293 821 015 415 705 725 559 725 790 829 437 600 562 957 262 158 883 224 810 396 929 210 773 3  
 215 572 327 035 085 107 316 238 648 372 291 504 443 650 816 258 845 011 545 897 388 622 083 775 502 3  
 633 569 483 289 686 720 512  $q^{5232} -$   
 12 332 389 356 505 925 630 698 252 993 083 533 306 481 705 682 081 165 392 085 642 207 313 764 900 3  
 363 147 154 840 253 185 441 803 697 001 548 987 208 690 741 898 458 335 126 881 458 097 103 690 369 3  
 200 026 577 550 705 098 752  $q^{5233} +$   
 13 801 217 656 727 255 171 237 225 263 482 654 965 096 296 584 509 766 544 543 033 457 847 720 930 3  
 291 813 419 622 903 575 809 081 961 722 455 958 235 334 672 028 922 335 961 123 056 384 220 084 503 3  
 553 219 922 722 823 168 000  $q^{5236} -$   
 14 328 619 856 688 255 967 565 777 785 452 755 170 595 803 501 270 579 918 654 668 592 876 129 933 3  
 877 518 839 118 373 273 025 266 378 725 142 379 256 130 346 209 145 235 680 997 805 063 263 405 724 3

447 603 177 151 381 290 949  $q^{5237} +$   
 16 034 518 537 609 459 897 542 950 848 797 227 729 495 028 377 707 005 984 587 997 056 667 850 972 \ \backslash  
 099 041 234 460 256 856 839 583 587 134 095 025 471 781 240 074 153 595 127 489 463 940 110 411 924 \ \backslash  
 736 865 646 313 149 977 600  $q^{5240} -$   
 16 647 026 797 072 429 859 033 024 417 219 146 343 658 115 108 899 328 318 936 687 284 390 245 780 \ \backslash  
 243 940 906 498 774 004 325 542 152 779 386 726 662 536 505 361 427 051 685 094 905 363 351 930 401 \ \backslash  
 583 292 506 888 253 440 000  $q^{5241} +$   
 18 628 146 681 082 116 338 857 510 550 036 665 936 423 203 856 299 803 902 422 948 021 587 222 666 \ \backslash  
 433 046 633 686 343 303 069 329 737 307 392 601 425 461 106 482 345 836 990 858 363 056 403 669 080 \ \backslash  
 256 878 279 574 067 712 000  $q^{5244} -$   
 19 339 454 032 682 503 995 237 490 547 184 585 985 144 396 395 350 069 318 692 602 849 948 623 887 \ \backslash  
 640 380 117 683 962 746 678 712 260 497 348 532 049 980 209 191 231 244 851 054 599 381 980 108 343 \ \backslash  
 299 576 307 699 272 748 350  $q^{5245} +$   
 21 640 067 354 631 485 298 498 203 158 352 501 083 299 637 402 798 311 900 524 107 774 364 873 486 \ \backslash  
 668 743 279 410 778 158 874 319 467 624 350 545 268 458 969 912 729 848 509 568 563 281 584 612 816 \ \backslash  
 459 317 362 578 509 070 336  $q^{5248} -$   
 22 466 063 477 687 272 441 303 317 773 826 172 972 319 707 982 992 541 485 704 593 886 419 234 845 \ \backslash  
 358 651 675 413 284 044 232 215 250 031 260 218 567 257 887 382 131 960 913 965 121 202 561 410 816 \ \backslash  
 028 481 808 760 414 208 000  $q^{5249} +$   
 25 137 543 197 418 952 114 318 743 887 263 991 944 314 019 046 000 880 334 933 521 251 908 671 315 \ \backslash  
 904 115 151 021 853 994 591 186 609 093 233 060 741 072 655 429 316 001 360 870 534 968 482 839 122 \ \backslash  
 366 305 696 314 582 007 808  $q^{5252} -$   
 26 096 665 770 372 217 338 566 950 776 014 096 287 969 897 118 364 375 656 805 971 665 006 902 033 \ \backslash  
 422 907 311 014 518 999 320 942 064 104 299 029 063 988 661 282 958 077 183 961 343 996 704 053 269 \ \backslash  
 282 253 554 985 682 935 726  $q^{5253} +$   
 29 198 621 097 007 718 196 691 692 964 575 300 906 144 249 933 481 096 635 973 566 468 449 363 374 \ \backslash  
 504 918 264 258 519 984 429 547 356 587 171 621 570 846 513 155 620 379 166 139 409 485 449 708 061 \ \backslash  
 945 693 749 768 484 608 000  $q^{5256} -$   
 30 312 263 183 494 678 771 220 661 297 677 020 283 214 816 122 559 260 352 801 912 116 729 539 821 \ \backslash  
 925 435 537 346 152 907 542 491 399 704 214 773 551 558 967 173 679 289 365 593 559 458 719 037 192 \ \backslash  
 925 505 149 354 730 061 824  $q^{5257} +$   
 33 913 856 155 937 793 270 307 703 267 644 128 679 844 336 364 515 284 328 855 181 893 302 944 438 \ \backslash  
 730 482 626 951 479 049 501 879 853 578 373 526 556 021 283 702 321 004 886 493 402 254 402 586 984 \ \backslash  
 468 140 603 979 795 225 600  $q^{5260} -$   
 35 206 838 534 500 135 417 071 730 702 245 388 790 200 404 880 248 171 577 974 718 203 787 698 334 \ \backslash  
 453 450 326 325 595 444 650 937 556 985 981 610 242 640 468 452 696 915 059 516 847 579 840 829 478 \ \backslash  
 934 474 352 939 859 928 500  $q^{5261} +$   
 39 388 310 442 388 797 497 823 711 177 345 117 801 031 816 808 164 783 458 945 798 522 396 867 847 \ \backslash  
 720 139 745 771 145 715 003 561 043 698 363 649 219 719 616 044 975 592 900 364 990 834 138 292 854 \ \backslash  
 522 693 932 280 872 960 000  $q^{5264} -$   
 40 889 429 202 482 477 956 550 177 488 249 842 679 404 995 428 161 234 269 526 529 015 646 943 569 \ \backslash  
 315 935 073 669 993 573 866 825 962 676 432 831 951 284 139 643 220 431 635 258 135 674 586 012 089 \ \backslash  
 105 244 304 109 212 467 200  $q^{5265} +$   
 45 743 870 194 499 576 003 050 366 039 974 080 098 726 274 655 136 882 287 249 598 754 133 524 920 \ \backslash  
 402 890 840 383 181 714 969 559 286 847 935 626 005 056 654 324 629 033 037 060 463 718 661 892 380 \ \backslash  
 634 213 538 117 160 914 944  $q^{5268} -$   
 47 486 531 557 412 716 905 884 314 201 869 709 118 758 978 742 154 659 374 831 790 665 630 490 471 \ \backslash  
 146 576 802 994 232 743 828 478 679 735 325 360 818 421 064 214 703 997 114 080 144 555 064 969 999 \ \backslash  
 697 220 696 552 201 401 250  $q^{5269} +$   
 53 121 932 067 683 172 679 597 189 838 903 002 820 395 673 031 314 160 247 164 403 065 703 858 084 \ \backslash  
 660 177 926 494 323 859 599 603 702 112 735 237 491 444 304 407 882 860 005 771 302 629 750 473 365 \ \backslash  
 233 144 545 014 242 172 416  $q^{5272} -$   
 55 144 888 285 440 187 702 708 763 878 648 771 155 189 584 051 545 825 481 502 679 915 423 214 434 \ \backslash  
 921 590 219 244 432 735 852 255 257 420 722 991 473 302 172 882 278 951 998 912 139 456 349 286 933 \ \backslash  
 612 603 887 928 721 735 680  $q^{5273} +$

61 686 517 027 323 168 082 338 668 766 878 108 055 608 269 746 067 188 156 449 169 633 060 005 673 \
 496 599 224 707 442 873 141 232 324 178 475 183 701 539 609 033 535 853 509 726 830 357 580 625 932 \
 904 043 869 390 658 816 000  $q^{5276}$  -

64 034 719 406 357 465 822 547 876 923 351 848 913 300 132 930 329 407 801 590 226 563 614 715 581 \
 621 392 993 324 560 362 154 118 662 996 514 915 432 047 774 237 098 441 970 366 386 932 589 547 244 \
 112 801 002 401 751 148 677  $q^{5277}$  +

71 627 879 767 787 903 385 035 784 951 837 515 150 981 423 292 126 254 651 920 906 749 660 777 207 \
 407 071 668 305 473 805 924 605 273 872 020 277 999 171 320 318 434 529 279 426 621 376 261 923 672 \
 237 661 032 273 554 227 200  $q^{5280}$  -

74 353 467 404 238 420 430 426 996 523 786 055 956 465 970 659 621 709 486 824 091 296 996 020 811 \
 311 704 880 753 424 135 455 930 109 637 043 290 418 345 072 023 563 978 836 000 073 205 955 817 125 \
 496 721 361 892 659 200 000  $q^{5281}$  +

83 166 692 282 029 276 575 653 172 458 737 974 361 348 005 597 392 023 774 138 588 933 355 715 761 \
 088 560 111 519 340 439 522 945 339 473 677 197 959 294 680 359 253 415 256 505 724 944 060 828 832 \
 273 871 246 028 869 632 000  $q^{5284}$  -

86 330 138 036 485 307 955 159 731 858 312 960 319 472 174 879 942 019 484 913 327 811 551 747 843 \
 361 762 583 144 748 922 477 350 960 867 716 473 612 009 257 298 314 706 817 834 326 503 657 763 729 \
 565 874 599 007 082 860 200  $q^{5285}$  +

96 558 892 644 707 194 345 833 206 094 673 656 611 222 913 857 844 029 765 254 908 854 661 627 284 \
 763 634 976 923 993 711 155 556 487 314 862 294 055 661 562 451 516 682 206 732 530 196 808 141 239 \
 923 574 240 399 438 214 656  $q^{5288}$  -

100 230 331 289 179 462 131 813 723 807 375 439 963 396 259 615 031 124 063 015 795 079 650 065 510 \
 804 881 250 830 151 685 102 156 905 487 059 682 694 907 291 888 261 937 081 799 563 389 851 418 780 \
 371 498 018 174 836 736 000  $q^{5289}$  +

112 101 304 472 550 088 055 008 717 887 057 308 769 903 187 996 564 231 792 959 531 402 791 947 278 \
 578 506 890 543 681 116 268 539 933 792 100 111 958 474 561 059 803 293 069 369 724 730 417 767 741 \
 683 394 162 416 997 406 720  $q^{5292}$  -

116 362 071 884 370 640 382 054 462 027 857 410 906 115 532 952 031 882 950 189 295 397 917 639 995 \
 677 136 660 190 182 634 371 525 438 120 576 987 548 687 122 797 238 345 609 988 168 247 428 620 003 \
 501 759 186 666 226 405 499  $q^{5293}$  +

130 138 149 197 125 623 962 645 967 931 477 494 792 718 255 620 274 696 249 621 750 827 369 807 365 \
 512 453 486 240 396 609 296 092 114 657 471 806 509 882 058 681 244 131 361 291 306 984 175 575 017 \
 126 758 995 883 588 096 000  $q^{5296}$  -

135 082 566 037 809 566 242 217 714 178 292 293 139 265 956 446 360 381 389 629 895 526 794 122 078 \
 258 482 570 249 854 872 775 994 351 286 160 324 752 052 008 318 824 665 471 098 554 069 962 685 991 \
 781 637 448 107 507 646 464  $q^{5297}$  +

151 068 592 584 348 315 963 692 754 485 031 266 443 332 565 580 039 937 661 445 995 844 856 464 487 \
 866 688 495 295 451 057 723 322 272 300 189 372 535 787 749 656 226 183 794 852 202 061 735 153 940 \
 038 391 966 699 603 404 800  $q^{5300}$  -

156 806 031 183 859 054 356 371 339 067 216 792 169 894 301 482 512 448 271 468 393 599 635 922 507 \
 870 253 858 779 926 721 299 816 464 430 396 337 842 860 579 866 982 740 552 555 257 874 978 933 987 \
 194 720 798 263 855 797 500  $q^{5301}$  +

175 355 489 274 848 855 869 861 222 064 199 983 732 560 477 161 996 938 708 010 473 266 638 488 957 \
 688 718 771 213 204 401 580 490 536 580 709 585 325 250 296 491 556 173 790 838 223 423 232 578 310 \
 803 429 914 640 217 344 000  $q^{5304}$  -

182 012 768 556 175 353 788 985 767 404 990 663 829 605 532 571 623 917 703 476 057 548 203 403 200 \
 531 009 643 050 679 309 490 121 399 031 270 125 977 084 253 698 259 854 879 867 185 817 691 237 124 \
 250 287 151 842 641 510 400  $q^{5305}$  +

203 535 514 977 439 509 887 657 445 110 188 110 431 467 334 689 903 514 692 178 240 718 968 201 193 \
 589 647 525 026 618 905 891 581 059 173 898 184 185 544 646 881 748 366 340 521 769 550 728 637 483 \
 294 830 183 108 541 284 352  $q^{5308}$  -

211 259 675 333 598 252 590 486 739 188 009 419 847 657 861 370 197 107 644 901 857 899 179 038 241 \
 451 414 245 277 421 027 148 369 922 991 072 571 719 051 162 821 166 245 026 010 313 646 294 765 684 \
 311 566 225 176 743 712 875  $q^{5309}$  +

236 230 905 876 816 217 716 110 057 656 775 996 400 747 346 488 579 646 282 444 562 912 272 148 646 \

383 404 478 962 976 887 583 447 325 458 297 131 260 959 759 596 356 817 101 121 977 988 931 834 469 3  
 270 118 435 787 951 013 888  $q^{5312}$  -  
 245 192 424 103 475 425 238 265 059 538 479 739 490 426 355 653 610 888 305 221 884 256 983 800 179 3  
 649 301 139 147 476 778 820 029 160 174 384 103 385 715 840 777 660 738 825 364 000 200 584 280 658 3  
 671 218 315 116 225 101 824  $q^{5313}$  +  
 274 163 059 455 331 054 522 888 427 260 734 082 828 615 323 247 841 058 519 063 926 366 589 937 013 3  
 064 024 601 526 188 726 135 755 764 923 032 533 569 681 082 007 255 986 746 796 619 301 810 419 368 3  
 834 106 030 624 729 088 000  $q^{5316}$  -  
 284 559 573 322 022 785 780 299 922 283 885 786 511 531 399 976 477 561 000 044 762 701 511 312 443 3  
 340 626 678 253 698 215 428 950 361 407 555 449 304 038 265 232 233 660 075 631 572 833 501 496 991 3  
 939 319 311 186 028 613 490  $q^{5317}$  +  
 318 168 291 016 148 009 795 660 798 975 575 834 844 002 986 275 225 428 842 795 365 759 194 672 009 3  
 824 781 537 575 969 315 092 606 034 955 686 353 222 804 645 634 557 144 879 228 898 051 736 854 970 3  
 427 479 410 924 691 507 200  $q^{5320}$  -  
 330 228 914 029 639 842 118 651 271 566 391 185 088 417 470 192 279 366 631 037 849 699 651 275 570 3  
 358 047 835 146 612 231 343 178 470 789 188 728 310 333 673 635 292 034 429 826 057 819 576 042 430 3  
 982 531 563 191 230 464 000  $q^{5321}$  +  
 369 216 086 585 976 798 359 870 826 133 604 818 000 788 901 009 939 069 208 338 426 811 230 139 592 3  
 327 169 362 456 223 169 649 197 914 262 292 828 589 897 557 122 350 163 552 580 058 419 772 045 596 3  
 126 202 548 573 590 784 000  $q^{5324}$  -  
 383 206 406 194 592 935 624 330 667 656 698 265 036 663 455 977 791 874 582 316 006 433 201 219 467 3  
 601 665 855 273 599 498 301 748 008 459 349 574 633 449 755 193 560 444 468 621 098 686 793 060 302 3  
 037 187 983 628 167 583 750  $q^{5325}$  +  
 428 430 246 558 132 120 828 734 028 507 876 886 776 952 816 911 429 152 631 900 753 533 058 771 698 3  
 826 995 820 945 210 240 640 856 396 462 024 494 856 626 293 293 164 961 532 271 612 406 390 044 369 3  
 362 830 028 548 145 266 688  $q^{5328}$  -  
 444 658 113 735 969 069 304 168 859 134 283 098 585 773 874 187 443 204 277 308 672 983 238 034 000 3  
 810 178 628 904 010 455 502 243 425 069 514 035 212 749 925 445 374 387 838 336 163 854 051 307 600 3  
 541 067 530 700 292 096 248  $q^{5329}$  +  
 497 113 376 553 651 074 348 645 201 329 069 332 079 650 194 499 959 833 937 589 132 941 471 482 158 3  
 953 449 146 020 663 197 933 059 780 181 775 420 518 214 177 939 537 706 196 761 997 556 434 970 018 3  
 984 175 405 358 333 661 184  $q^{5332}$  -  
 515 935 611 701 299 348 069 826 025 208 398 052 192 093 126 401 113 391 894 170 665 331 470 696 579 3  
 701 422 313 394 872 716 235 561 061 317 803 419 018 928 913 052 967 078 941 215 470 691 522 708 028 3  
 402 637 145 671 906 149 962  $q^{5333}$  +  
 576 775 253 850 955 329 997 112 456 000 400 712 337 945 061 132 147 956 215 283 261 634 600 554 861 3  
 163 788 840 341 871 966 374 458 759 720 536 848 827 339 858 862 498 799 869 025 609 071 642 318 447 3  
 819 925 637 831 757 824 000  $q^{5336}$  -  
 598 605 413 615 922 720 180 612 424 172 155 530 185 565 921 282 884 945 020 960 208 137 521 767 705 3  
 909 756 501 718 948 690 592 769 468 373 711 344 952 464 018 744 462 930 398 562 027 351 789 890 429 3  
 255 647 727 226 077 642 752  $q^{5337}$  +  
 669 165 680 890 801 637 726 127 222 866 345 414 054 892 315 477 987 762 644 636 516 137 159 008 109 3  
 898 413 443 757 801 521 965 669 874 594 858 886 276 753 102 995 001 988 473 202 702 023 778 737 753 3  
 151 503 468 409 575 526 400  $q^{5340}$  -  
 694 483 053 264 181 789 740 958 088 503 724 608 879 155 000 012 081 597 072 604 638 699 783 703 962 3  
 694 355 797 096 509 707 628 109 206 093 910 530 019 479 171 132 928 699 327 378 144 146 164 820 199 3  
 857 023 783 404 779 496 500  $q^{5341}$  +  
 776 312 533 569 303 569 796 609 391 776 895 718 554 580 757 105 696 913 617 832 199 497 667 064 996 3  
 647 700 422 718 736 213 683 472 046 099 434 339 797 766 455 584 520 790 903 687 223 329 026 461 463 3  
 506 235 378 336 617 472 000  $q^{5344}$  -  
 805 672 554 938 420 407 809 028 057 713 632 185 299 985 271 917 151 234 836 746 059 305 437 941 832 3  
 960 455 992 073 608 679 666 242 850 665 160 213 102 907 126 817 008 660 842 555 948 960 857 316 311 3  
 456 296 368 460 732 825 600  $q^{5345}$  +  
 900 565 823 329 592 471 826 235 931 068 060 703 461 857 467 173 472 601 399 064 092 498 228 735 403 3  
 150 180 770 131 537 733 441 202 362 406 364 480 167 884 485 213 334 409 459 628 464 475 092 475 379 3

$036\ 220\ 915\ 932\ 926\ 803\ 968\ q^{5348} -$   
 $934\ 612\ 141\ 617\ 831\ 798\ 802\ 854\ 985\ 983\ 067\ 402\ 436\ 287\ 862\ 051\ 132\ 372\ 748\ 801\ 429\ 339\ 248\ 319\ 823\ 9$   
 $286\ 611\ 885\ 055\ 704\ 203\ 520\ 162\ 459\ 525\ 324\ 548\ 264\ 048\ 164\ 316\ 654\ 314\ 765\ 411\ 241\ 947\ 666\ 877\ 512\ 9$   
 $738\ 997\ 449\ 817\ 297\ 321\ 750\ q^{5349} +$   
 $1\ 044\ 648\ 720\ 812\ 767\ 894\ 585\ 012\ 590\ 852\ 503\ 338\ 667\ 859\ 659\ 578\ 588\ 578\ 435\ 161\ 970\ 522\ 469\ 096\ 906\ 9$   
 $474\ 013\ 767\ 470\ 942\ 799\ 219\ 870\ 321\ 367\ 120\ 402\ 233\ 603\ 349\ 153\ 755\ 135\ 603\ 863\ 138\ 967\ 939\ 204\ 836\ 9$   
 $864\ 517\ 920\ 363\ 034\ 672\ 128\ q^{5352} -$   
 $1\ 084\ 127\ 164\ 063\ 147\ 249\ 046\ 111\ 606\ 298\ 276\ 242\ 484\ 926\ 265\ 628\ 414\ 411\ 499\ 827\ 365\ 472\ 052\ 338\ 031\ 9$   
 $791\ 378\ 327\ 198\ 574\ 242\ 891\ 274\ 141\ 577\ 631\ 375\ 240\ 669\ 706\ 258\ 533\ 062\ 020\ 938\ 067\ 374\ 018\ 664\ 722\ 9$   
 $984\ 475\ 413\ 889\ 460\ 731\ 904\ q^{5353} +$   
 $1\ 211\ 716\ 637\ 759\ 869\ 178\ 786\ 424\ 148\ 119\ 666\ 085\ 155\ 493\ 733\ 995\ 667\ 400\ 537\ 493\ 071\ 167\ 570\ 385\ 084\ 9$   
 $612\ 296\ 159\ 349\ 208\ 720\ 376\ 653\ 906\ 885\ 921\ 041\ 544\ 628\ 279\ 525\ 251\ 627\ 538\ 767\ 547\ 739\ 762\ 246\ 151\ 9$   
 $742\ 116\ 377\ 550\ 299\ 648\ 000\ q^{5356} -$   
 $1\ 257\ 491\ 388\ 264\ 318\ 494\ 892\ 447\ 520\ 495\ 254\ 514\ 214\ 257\ 295\ 567\ 760\ 175\ 958\ 008\ 052\ 237\ 336\ 666\ 616\ 9$   
 $722\ 492\ 318\ 564\ 774\ 566\ 621\ 079\ 336\ 025\ 933\ 079\ 797\ 331\ 523\ 734\ 473\ 126\ 823\ 693\ 617\ 442\ 075\ 425\ 148\ 9$   
 $422\ 368\ 955\ 541\ 523\ 060\ 022\ q^{5357} +$   
 $1\ 405\ 425\ 636\ 122\ 782\ 502\ 096\ 582\ 177\ 474\ 764\ 965\ 440\ 501\ 233\ 627\ 068\ 027\ 093\ 761\ 256\ 913\ 197\ 704\ 620\ 9$   
 $360\ 608\ 094\ 569\ 824\ 643\ 606\ 284\ 947\ 491\ 988\ 280\ 556\ 858\ 013\ 226\ 702\ 759\ 973\ 325\ 863\ 867\ 325\ 538\ 104\ 9$   
 $440\ 516\ 003\ 324\ 829\ 286\ 400\ q^{5360} -$   
 $1\ 458\ 497\ 957\ 327\ 141\ 059\ 761\ 528\ 863\ 264\ 747\ 461\ 151\ 394\ 134\ 972\ 452\ 575\ 774\ 893\ 915\ 071\ 025\ 945\ 991\ 9$   
 $952\ 595\ 800\ 702\ 215\ 312\ 513\ 005\ 807\ 630\ 436\ 384\ 789\ 070\ 406\ 170\ 703\ 898\ 969\ 001\ 555\ 300\ 374\ 402\ 042\ 9$   
 $880\ 292\ 307\ 438\ 120\ 960\ 000\ q^{5361} +$   
 $1\ 630\ 011\ 632\ 588\ 910\ 962\ 733\ 538\ 659\ 702\ 964\ 432\ 156\ 226\ 433\ 816\ 821\ 126\ 496\ 436\ 291\ 945\ 589\ 788\ 587\ 9$   
 $964\ 921\ 311\ 002\ 664\ 178\ 141\ 799\ 925\ 858\ 992\ 740\ 380\ 710\ 127\ 215\ 363\ 686\ 124\ 917\ 944\ 690\ 961\ 743\ 072\ 9$   
 $585\ 771\ 751\ 705\ 800\ 960\ 000\ q^{5364} -$   
 $1\ 691\ 541\ 550\ 511\ 202\ 494\ 651\ 679\ 492\ 429\ 765\ 483\ 263\ 790\ 900\ 027\ 968\ 798\ 884\ 659\ 158\ 487\ 180\ 100\ 954\ 9$   
 $085\ 283\ 938\ 826\ 986\ 071\ 416\ 791\ 441\ 914\ 245\ 073\ 115\ 560\ 461\ 846\ 461\ 687\ 589\ 182\ 276\ 431\ 874\ 797\ 736\ 9$   
 $374\ 051\ 877\ 230\ 133\ 141\ 775\ q^{5365} +$   
 $1\ 890\ 382\ 097\ 165\ 612\ 175\ 010\ 506\ 270\ 862\ 137\ 086\ 600\ 859\ 926\ 014\ 682\ 004\ 805\ 377\ 139\ 512\ 950\ 073\ 822\ 9$   
 $247\ 362\ 926\ 707\ 124\ 241\ 404\ 047\ 841\ 593\ 220\ 649\ 440\ 371\ 312\ 740\ 686\ 412\ 689\ 180\ 237\ 940\ 283\ 540\ 095\ 9$   
 $227\ 228\ 443\ 258\ 444\ 366\ 848\ q^{5368} -$   
 $1\ 961\ 713\ 501\ 104\ 410\ 081\ 766\ 177\ 527\ 952\ 049\ 399\ 215\ 593\ 258\ 289\ 216\ 418\ 647\ 370\ 962\ 277\ 290\ 677\ 282\ 9$   
 $202\ 318\ 049\ 858\ 323\ 107\ 126\ 452\ 119\ 896\ 485\ 938\ 356\ 798\ 572\ 020\ 795\ 481\ 986\ 311\ 426\ 424\ 660\ 178\ 028\ 9$   
 $612\ 323\ 107\ 249\ 315\ 840\ 000\ q^{5369} +$   
 $2\ 192\ 222\ 210\ 975\ 494\ 818\ 498\ 999\ 029\ 944\ 742\ 770\ 170\ 833\ 981\ 097\ 673\ 698\ 803\ 400\ 704\ 167\ 645\ 644\ 764\ 9$   
 $147\ 964\ 681\ 573\ 574\ 657\ 256\ 581\ 897\ 671\ 346\ 953\ 221\ 067\ 333\ 798\ 793\ 587\ 568\ 031\ 934\ 978\ 051\ 837\ 092\ 9$   
 $327\ 349\ 060\ 636\ 017\ 836\ 032\ q^{5372} -$   
 $2\ 274\ 911\ 911\ 187\ 671\ 575\ 300\ 991\ 913\ 235\ 452\ 104\ 691\ 794\ 108\ 417\ 192\ 318\ 864\ 015\ 390\ 189\ 162\ 181\ 389\ 9$   
 $192\ 630\ 946\ 773\ 766\ 362\ 459\ 732\ 572\ 605\ 939\ 391\ 413\ 538\ 102\ 163\ 581\ 784\ 813\ 713\ 914\ 988\ 755\ 863\ 259\ 9$   
 $758\ 429\ 810\ 781\ 550\ 536\ 616\ q^{5373} +$   
 $2\ 542\ 117\ 756\ 610\ 293\ 821\ 152\ 409\ 153\ 007\ 132\ 350\ 527\ 872\ 009\ 238\ 011\ 244\ 743\ 123\ 577\ 584\ 341\ 058\ 628\ 9$   
 $206\ 674\ 444\ 326\ 939\ 207\ 852\ 626\ 294\ 217\ 068\ 586\ 772\ 979\ 580\ 231\ 297\ 991\ 603\ 499\ 162\ 942\ 061\ 950\ 880\ 9$   
 $525\ 968\ 005\ 652\ 021\ 248\ 000\ q^{5376} -$   
 $2\ 637\ 969\ 120\ 941\ 912\ 174\ 033\ 818\ 160\ 228\ 336\ 322\ 246\ 899\ 004\ 694\ 229\ 331\ 150\ 282\ 826\ 738\ 153\ 555\ 777\ 9$   
 $449\ 624\ 275\ 381\ 110\ 301\ 180\ 947\ 756\ 719\ 168\ 242\ 125\ 697\ 071\ 297\ 220\ 569\ 957\ 049\ 441\ 124\ 988\ 407\ 022\ 9$   
 $507\ 441\ 883\ 291\ 147\ 206\ 656\ q^{5377} +$   
 $2\ 947\ 697\ 370\ 782\ 471\ 979\ 482\ 991\ 541\ 801\ 946\ 398\ 523\ 600\ 602\ 237\ 744\ 416\ 438\ 697\ 141\ 973\ 834\ 009\ 930\ 9$   
 $621\ 488\ 411\ 091\ 863\ 167\ 204\ 180\ 221\ 395\ 471\ 510\ 354\ 974\ 280\ 631\ 389\ 225\ 230\ 060\ 321\ 444\ 489\ 363\ 965\ 9$   
 $120\ 975\ 249\ 156\ 033\ 740\ 800\ q^{5380} -$   
 $3\ 058\ 799\ 259\ 721\ 133\ 148\ 474\ 470\ 267\ 570\ 387\ 827\ 624\ 829\ 630\ 804\ 215\ 339\ 545\ 527\ 107\ 931\ 127\ 477\ 576\ 9$   
 $145\ 322\ 604\ 541\ 143\ 249\ 083\ 228\ 885\ 648\ 738\ 835\ 595\ 009\ 234\ 874\ 934\ 619\ 869\ 853\ 248\ 871\ 480\ 518\ 985\ 9$   
 $899\ 471\ 377\ 324\ 868\ 489\ 375\ q^{5381} +$   
 $3\ 417\ 797\ 201\ 114\ 658\ 318\ 695\ 986\ 487\ 971\ 935\ 839\ 223\ 402\ 869\ 639\ 501\ 057\ 888\ 095\ 268\ 247\ 653\ 789\ 199\ 9$   
 $858\ 893\ 138\ 124\ 246\ 653\ 672\ 964\ 776\ 345\ 035\ 519\ 123\ 230\ 638\ 152\ 866\ 409\ 468\ 555\ 723\ 681\ 425\ 475\ 074\ 9$   
 $724\ 644\ 930\ 855\ 106\ 176\ 000\ q^{5384} -$

3 546 569 033 450 877 242 162 844 952 276 110 690 816 097 615 336 768 979 348 728 201 722 423 339 312 \
 737 239 552 419 949 266 101 869 524 932 526 633 789 173 269 573 001 450 196 137 545 232 211 228 669 \
 558 482 530 012 230 451 200  $q^{5385} +$

3 962 651 485 400 604 384 558 845 424 359 982 510 409 978 605 149 359 449 434 544 620 294 693 360 727 \
 560 361 747 061 238 385 841 181 629 366 809 414 057 814 022 829 240 500 005 553 925 137 241 547 281 \
 009 583 279 341 266 693 120  $q^{5388} -$

4 111 895 397 013 696 506 286 492 483 186 961 922 940 051 254 931 181 125 145 930 445 376 959 100 555 \
 724 480 593 095 322 889 129 054 072 287 417 517 526 916 768 732 495 080 296 930 962 593 777 473 221 \
 696 686 087 007 999 145 250  $q^{5389} +$

4 594 113 122 590 052 826 700 724 239 316 963 411 460 804 711 325 474 405 071 413 992 184 737 361 785 \
 679 634 279 117 048 359 278 580 163 485 359 400 685 755 792 706 616 261 660 729 020 754 955 867 771 \
 245 285 739 167 249 858 560  $q^{5392} -$

4 767 074 331 553 409 358 376 831 357 535 869 689 247 435 185 112 697 380 617 879 534 036 282 249 484 \
 715 065 270 145 864 588 525 969 496 896 381 227 839 513 886 823 854 465 901 491 920 477 162 094 883 \
 316 858 279 886 511 210 496  $q^{5393} +$

5 325 908 941 684 879 050 228 825 752 206 477 969 727 018 722 270 267 809 301 967 001 923 479 578 097 \
 479 367 394 476 258 655 943 009 403 748 742 100 247 662 026 397 027 703 709 817 754 611 031 239 053 \
 118 086 807 000 413 184 000  $q^{5396} -$

5 526 345 607 085 197 856 430 662 134 595 943 548 906 653 172 854 090 093 760 832 366 410 691 888 123 \
 878 703 048 966 064 792 066 013 089 471 719 280 992 345 707 283 701 425 333 501 409 182 554 386 235 \
 570 346 835 995 469 863 476  $q^{5397} +$

6 173 935 111 076 203 618 981 260 184 474 532 843 925 895 284 380 380 334 616 607 085 416 411 732 498 \
 211 091 635 085 108 918 778 502 572 248 962 346 756 311 988 024 581 801 328 249 844 234 896 000 247 \
 578 586 856 605 108 684 800  $q^{5400} -$

6 406 199 174 322 025 675 946 965 860 985 819 073 216 899 746 614 821 240 062 973 953 701 415 588 312 \
 389 547 070 679 082 986 124 933 336 690 665 783 796 435 101 842 951 361 294 692 391 842 784 954 286 \
 966 483 792 009 695 232 000  $q^{5401} +$

7 156 598 982 071 723 492 522 210 351 440 452 911 599 383 475 083 184 898 841 037 762 687 742 416 582 \
 170 838 642 315 234 527 845 386 635 666 102 746 171 828 844 782 088 066 406 738 998 009 138 720 562 \
 096 226 626 523 559 936 000  $q^{5404} -$

7 425 729 712 257 431 155 938 376 871 250 489 574 207 343 751 037 736 466 941 271 438 105 366 810 597 \
 284 693 312 686 918 251 221 814 778 381 004 486 695 237 993 447 557 324 297 502 177 873 618 481 675 \
 254 562 264 362 849 728 075  $q^{5405} +$

8 295 214 644 329 595 749 142 462 901 232 734 032 931 259 779 063 823 476 010 832 228 301 375 468 040 \
 785 884 205 166 132 834 828 866 773 324 866 651 181 183 362 362 389 268 354 755 881 539 250 652 164 \
 455 401 162 469 930 248 192  $q^{5408} -$

8 607 046 878 306 843 152 375 685 527 166 896 008 672 588 581 483 272 048 876 754 451 083 265 823 118 \
 327 892 306 694 824 167 757 063 319 497 571 098 896 098 722 824 510 824 417 120 142 529 485 698 779 \
 339 472 298 819 932 160 000  $q^{5409} +$

9 614 460 608 272 039 944 187 433 189 862 680 765 416 488 483 432 059 522 076 152 803 160 058 634 929 \
 308 678 509 236 349 004 841 675 382 514 153 917 237 469 593 525 954 201 535 253 700 536 753 294 624 \
 307 858 779 337 617 113 088  $q^{5412} -$

9 975 749 987 103 928 559 576 987 321 341 425 826 212 830 011 566 310 617 520 122 929 886 901 988 679 \
 747 924 176 808 956 253 288 018 822 807 535 875 562 946 301 233 527 267 302 893 145 373 620 201 675 \
 123 896 661 259 471 850 799  $q^{5413} +$

11 142 909 344 141 218 467 767 876 045 424 246 046 839 862 354 679 088 843 196 951 399 178 077 103 \
 910 107 642 738 165 447 124 964 872 978 012 938 640 666 674 736 255 749 978 488 997 315 392 325 659 \
 668 486 622 608 390 565 440 000  $q^{5416} -$

11 561 477 207 092 595 480 488 568 883 646 650 923 160 631 280 731 377 985 787 853 852 464 819 467 \
 262 290 758 505 800 158 276 691 582 423 554 978 863 134 680 294 782 036 173 114 000 444 647 400 249 \
 224 897 319 656 012 618 858 496  $q^{5417} +$

12 913 639 926 720 151 281 749 193 326 354 820 300 439 416 396 418 005 901 305 582 062 934 919 033 \
 788 658 163 639 609 489 873 646 229 350 731 892 322 021 296 834 410 175 133 649 730 418 242 299 502 \
 133 043 897 785 301 213 952 000  $q^{5420} -$

13 398 540 939 397 256 904 428 869 187 354 727 027 745 539 307 104 816 862 779 905 994 853 038 323 \

120 314 757 732 144 551 868 593 758 607 567 999 737 028 755 128 847 593 073 230 724 902 316 453 299 \\  
 629 016 743 899 829 411 402 875  $q^{5421} +$

14 964 946 790 677 204 003 422 166 785 763 129 584 761 641 337 585 484 076 991 344 917 962 696 279 \\  
 964 369 253 516 346 138 143 962 667 290 474 116 978 310 320 514 798 224 729 557 305 307 082 333 805 \\  
 805 514 415 610 321 191 936 000  $q^{5424} -$

15 526 662 864 064 489 859 806 422 666 933 210 607 949 662 427 656 895 568 736 149 865 797 285 047 \\  
 171 282 691 670 653 095 249 280 145 471 047 296 653 780 346 516 061 328 255 609 526 049 531 526 337 \\  
 663 492 615 011 490 822 553 600  $q^{5425} +$

17 341 159 630 734 494 190 067 090 333 552 961 466 876 114 519 572 964 969 272 050 011 758 475 250 \\  
 466 769 349 566 723 144 158 248 078 009 138 355 733 914 924 373 093 282 335 886 937 289 041 040 603 \\  
 817 811 589 712 108 040 421 376  $q^{5428} -$

17 991 824 242 724 715 804 522 185 169 037 268 118 946 558 283 456 110 867 675 539 375 053 113 296 \\  
 411 293 884 229 154 624 843 814 916 543 123 022 243 290 347 807 663 418 784 727 558 120 574 423 306 \\  
 475 790 686 914 120 368 802 625  $q^{5429} +$

20 093 591 825 825 131 675 047 260 595 307 536 442 114 367 334 345 698 916 123 874 177 909 604 387 \\  
 170 008 253 958 150 046 347 841 256 764 404 662 745 879 955 796 989 017 035 332 330 234 864 863 515 \\  
 076 655 959 585 160 412 723 200  $q^{5432} -$

20 847 249 497 993 498 933 937 117 215 755 999 512 816 873 079 581 062 842 628 337 571 995 183 774 \\  
 997 070 647 727 454 992 708 839 566 468 597 095 939 727 063 242 840 959 253 056 309 706 938 657 042 \\  
 117 305 246 602 227 852 935 168  $q^{5433} +$

23 281 637 476 072 364 685 364 320 321 443 247 805 793 945 843 265 753 600 717 718 324 382 483 128 \\  
 339 441 243 562 794 591 229 509 044 682 118 696 581 825 696 769 165 424 564 491 970 629 154 479 232 \\  
 158 553 722 498 126 903 040 000  $q^{5436} -$

24 154 543 899 292 901 845 877 922 571 482 703 737 470 929 557 856 722 916 853 546 526 820 742 897 \\  
 782 488 523 292 199 020 668 869 621 936 663 300 549 371 675 367 438 608 906 574 784 753 775 766 557 \\  
 723 926 485 114 965 739 357 090  $q^{5437} +$

26 974 040 272 353 224 957 992 193 232 177 904 356 694 862 491 394 774 026 602 637 019 427 171 401 \\  
 668 310 850 219 605 491 422 087 633 681 322 062 340 304 014 356 085 166 198 861 332 398 062 611 909 \\  
 910 322 768 418 814 617 190 400  $q^{5440} -$

27 985 009 430 852 100 641 771 335 070 678 903 392 129 599 535 422 881 633 427 992 963 610 093 487 \\  
 173 098 653 705 101 782 512 639 430 023 516 603 613 222 988 494 678 904 805 898 896 240 224 357 756 \\  
 363 799 073 492 025 741 312 000  $q^{5441} +$

31 250 361 035 703 622 507 785 362 897 900 206 517 747 670 259 897 948 306 490 208 340 093 082 220 \\  
 804 632 352 590 266 117 447 914 697 706 241 882 992 448 258 170 073 580 763 430 292 353 896 529 685 \\  
 461 896 862 343 479 392 256 000  $q^{5444} -$

32 421 166 668 136 140 372 170 068 364 132 199 158 319 515 371 394 465 803 017 238 102 543 229 236 \\  
 945 827 915 141 870 799 226 817 656 050 476 887 767 009 724 857 479 644 586 143 181 093 513 395 773 \\  
 498 264 191 327 695 628 859 905  $q^{5445} +$

36 202 674 943 278 678 451 101 260 395 191 426 422 057 560 812 285 534 249 752 978 942 971 956 099 \\  
 361 570 657 275 010 528 405 059 333 254 689 036 933 519 920 254 828 180 815 875 992 066 872 895 400 \\  
 310 456 349 813 601 317 646 336  $q^{5448} -$

37 558 514 822 007 827 632 932 821 686 196 960 073 960 501 790 056 378 278 253 144 883 767 248 292 \\  
 232 761 563 911 713 138 952 187 734 532 664 464 506 592 365 088 794 633 492 926 185 419 449 951 767 \\  
 198 979 324 585 009 782 784 000  $q^{5449} +$

41 937 534 286 049 028 781 097 091 486 972 766 425 418 168 391 023 909 179 798 353 436 078 598 780 \\  
 768 151 051 125 968 431 403 879 658 509 054 946 553 688 235 584 962 315 690 049 131 887 478 066 008 \\  
 787 119 311 404 534 197 607 424  $q^{5452} -$

43 507 567 115 780 782 558 848 057 535 674 517 517 394 116 301 155 187 436 976 794 566 323 555 728 \\  
 701 803 340 569 724 039 470 166 352 562 102 226 540 973 042 817 240 121 545 379 282 568 885 697 983 \\  
 202 318 948 209 234 224 971 601  $q^{5453} +$

48 578 238 181 383 406 972 676 807 589 844 046 451 885 340 688 388 098 779 670 771 403 495 746 197 \\  
 394 906 227 547 369 335 694 926 410 068 615 639 747 899 967 289 325 198 421 828 111 541 388 907 269 \\  
 262 709 697 393 003 057 152 000  $q^{5456} -$

50 396 204 443 137 243 685 848 450 546 728 089 304 835 753 532 057 188 443 909 847 203 503 592 923 \\  
 376 727 734 274 549 514 809 972 999 822 401 556 434 189 485 632 077 977 534 723 084 115 359 022 709 \

351 707 452 077 978 721 714 176  $q^{5457} +$   
 56 267 457 107 148 104 566 808 035 975 907 843 164 130 372 120 174 837 355 256 616 820 004 519 694 \ \backslash  
 321 813 421 354 311 933 622 795 304 629 124 313 824 413 979 448 772 530 628 919 527 242 418 354 084 \ \backslash  
 368 425 412 659 572 395 622 400  $q^{5460} -$   
 58 372 396 934 909 101 945 420 861 060 329 079 425 914 351 037 118 333 301 569 478 160 714 722 585 \ \backslash  
 392 147 476 976 183 560 776 115 421 227 807 758 866 326 297 367 468 396 664 363 064 549 417 771 847 \ \backslash  
 269 863 113 548 787 864 317 375  $q^{5461} +$   
 65 170 267 566 857 219 866 118 774 985 336 087 577 257 599 948 794 976 749 192 709 136 568 683 467 \ \backslash  
 850 838 430 136 983 253 928 881 650 134 797 276 671 249 069 671 732 953 371 255 275 221 410 691 320 \ \backslash  
 355 876 464 944 395 506 880 000  $q^{5464} -$   
 67 607 350 778 758 218 853 483 914 283 937 875 560 742 691 051 917 068 082 847 681 168 323 100 418 \ \backslash  
 703 356 285 981 305 858 067 533 810 941 806 379 327 334 101 004 937 552 827 798 366 653 789 664 030 \ \backslash  
 559 032 777 579 121 549 312 000  $q^{5465} +$   
 75 477 660 792 305 796 728 736 674 305 567 276 447 478 102 830 388 257 006 992 065 919 939 464 583 \ \backslash  
 400 935 825 720 524 259 093 810 175 176 620 842 911 396 453 347 817 581 762 552 876 445 806 534 133 \ \backslash  
 876 557 891 442 705 710 389 248  $q^{5468} -$   
 78 299 146 548 057 829 162 450 657 228 470 904 412 724 526 429 566 178 520 015 789 652 439 996 155 \ \backslash  
 750 316 351 681 086 006 098 687 854 034 210 296 006 607 785 730 648 739 994 257 163 055 309 975 356 \ \backslash  
 382 814 925 319 054 343 035 000  $q^{5469} +$   
 87 410 599 319 420 600 522 750 886 735 862 293 816 031 220 249 618 912 544 895 409 515 490 931 879 \ \backslash  
 202 393 682 709 018 778 785 811 429 131 031 717 263 721 719 567 439 159 631 706 791 867 182 834 213 \ \backslash  
 353 905 927 142 848 698 306 560  $q^{5472} -$   
 90 676 945 589 691 899 849 369 240 659 513 082 943 521 815 441 051 294 738 735 998 826 584 229 802 \ \backslash  
 931 444 040 892 183 305 028 100 451 716 688 928 118 603 004 631 030 717 755 997 314 568 307 395 287 \ \backslash  
 625 463 042 829 551 259 287 552  $q^{5473} +$   
 101 224 706 740 683 322 758 918 902 168 464 070 996 521 388 583 983 800 544 255 264 530 622 464 960 \ \backslash  
 803 527 254 910 291 576 896 773 863 797 079 199 632 556 370 774 201 691 449 195 052 132 168 312 836 \ \backslash  
 942 832 845 152 535 289 882 752  $q^{5476} -$   
 105 005 852 908 479 338 939 789 911 623 156 367 927 625 731 556 844 577 741 791 924 157 892 703 296 \ \backslash  
 953 671 537 851 456 610 942 336 200 107 207 180 498 943 073 555 061 958 971 252 367 008 920 433 756 \ \backslash  
 277 310 585 535 724 752 940 115  $q^{5477} +$   
 117 215 689 181 062 508 359 601 784 045 735 167 644 512 401 097 004 441 469 209 974 988 435 682 844 \ \backslash  
 022 430 025 594 525 830 947 969 034 950 813 006 527 434 193 046 304 079 399 938 644 323 875 077 189 \ \backslash  
 204 832 218 739 693 677 593 600  $q^{5480} -$   
 121 592 538 714 806 211 902 349 184 967 360 936 937 924 552 687 333 876 471 924 829 585 565 943 265 \ \backslash  
 511 323 396 248 170 320 539 349 409 535 716 958 753 751 227 373 040 528 934 249 485 406 302 947 005 \ \backslash  
 083 345 811 654 409 519 104 000  $q^{5481} +$   
 135 725 602 338 184 385 178 917 644 254 152 471 323 087 986 968 201 639 179 685 242 487 867 280 383 \ \backslash  
 523 549 448 720 749 836 558 779 343 325 430 751 618 825 075 258 975 326 483 640 920 159 408 552 927 \ \backslash  
 208 199 657 655 413 424 896 000  $q^{5484} -$   
 140 791 736 656 061 271 691 634 882 341 209 322 525 866 998 045 847 449 290 612 982 065 591 889 347 \ \backslash  
 999 277 515 971 624 374 536 134 411 464 599 646 517 950 442 040 096 834 492 380 422 294 096 915 978 \ \backslash  
 560 359 915 163 341 102 264 075  $q^{5485} +$   
 157 150 095 587 959 647 677 501 898 868 850 586 003 174 015 753 086 877 099 268 566 437 604 553 112 \ \backslash  
 415 087 105 026 924 424 190 048 304 343 265 803 947 794 995 459 726 585 399 827 401 677 058 035 911 \ \backslash  
 721 725 503 455 600 559 915 008  $q^{5488} -$   
 163 013 755 059 632 903 511 374 341 336 941 137 157 434 943 554 888 195 339 494 156 374 706 719 396 \ \backslash  
 398 255 443 406 013 243 608 124 422 956 130 554 295 249 759 969 729 023 579 208 979 796 417 524 610 \ \backslash  
 133 989 044 560 168 521 728 000  $q^{5489} +$   
 181 946 785 049 257 392 085 604 501 769 523 212 612 818 332 125 764 295 656 625 838 420 954 054 185 \ \backslash  
 401 738 591 722 529 787 167 564 391 810 500 686 921 050 518 126 086 320 452 075 879 026 678 017 651 \ \backslash  
 338 182 173 797 108 019 087 360  $q^{5492} -$   
 188 733 158 654 038 030 097 359 491 605 038 651 695 490 112 216 940 845 513 689 919 287 021 697 506 \ \backslash  
 129 569 489 419 134 833 022 340 988 484 369 794 742 808 186 003 453 972 852 341 788 268 003 978 610 \ \backslash  
 524 041 023 550 409 399 829 208  $q^{5493} +$

210 644 931 046 863 510 766 285 374 453 830 396 004 192 058 245 729 233 417 355 507 882 983 659 406 3  
 033 309 408 683 495 008 801 363 288 880 382 634 329 352 024 144 482 984 894 603 967 054 689 682 081 3  
 168 084 095 778 166 945 664 000  $q^{5496}$  -  
 218 498 802 641 946 597 205 942 541 954 601 533 089 043 294 994 820 650 470 455 662 447 284 309 648 3  
 120 775 303 526 356 893 105 055 712 301 536 426 513 875 261 482 103 524 005 319 593 900 978 301 750 3  
 619 367 705 977 826 659 729 408  $q^{5497}$  +  
 243 856 622 597 075 018 675 819 652 914 832 728 131 951 389 174 822 052 188 233 985 130 740 069 596 3  
 765 510 685 804 775 352 896 474 884 520 879 602 300 980 458 181 292 197 242 880 949 539 362 991 596 3  
 563 746 526 034 897 752 576 000  $q^{5500}$  -  
 252 945 429 178 335 288 888 103 954 041 710 382 396 192 950 273 709 422 452 106 920 650 418 540 672 3  
 497 434 617 220 518 080 937 321 139 194 677 972 831 239 507 605 879 068 507 629 989 140 992 596 364 3  
 501 835 917 540 844 748 056 750  $q^{5501}$  +  
 282 289 702 925 811 380 151 562 548 941 657 312 528 170 623 908 431 904 877 446 450 276 809 693 460 3  
 185 684 157 241 248 104 128 178 212 284 893 342 735 188 376 788 720 265 114 396 277 166 171 604 075 3  
 063 913 811 914 749 931 520 000  $q^{5504}$  -  
 292 807 068 840 112 708 216 848 786 683 420 984 526 767 958 735 144 144 871 169 203 956 618 005 901 3  
 879 787 876 435 134 791 345 604 086 796 731 442 704 019 004 621 809 925 264 906 563 643 964 488 694 3  
 945 157 826 836 820 815 052 800  $q^{5505}$  +  
 326 762 706 262 227 569 635 269 201 480 021 998 611 922 402 102 672 461 221 992 918 858 523 484 240 3  
 304 619 958 173 150 811 823 710 791 619 130 032 126 856 787 040 517 593 015 755 815 782 028 872 055 3  
 170 521 740 972 556 464 898 048  $q^{5508}$  -  
 338 932 527 231 007 203 529 861 133 492 282 690 819 477 406 561 657 317 377 566 874 626 058 270 285 3  
 579 558 862 515 563 418 315 791 642 940 029 489 939 689 378 078 577 851 975 105 087 757 474 277 805 3  
 367 705 839 960 159 194 120 875  $q^{5509}$  +  
 378 222 117 978 073 112 501 119 679 424 710 336 961 426 931 143 607 400 094 359 099 216 385 521 637 3  
 911 004 928 740 870 396 364 085 801 367 633 135 461 761 098 660 980 828 029 853 499 660 868 902 196 3  
 419 043 347 760 207 347 446 784  $q^{5512}$  -  
 392 303 280 221 029 911 050 041 269 131 785 346 363 435 556 817 749 336 294 688 704 886 852 016 442 3  
 572 522 593 022 884 663 723 088 082 578 256 555 215 556 120 406 684 536 791 611 596 511 904 875 742 3  
 714 551 310 074 028 897 402 880  $q^{5513}$  +  
 437 762 318 425 692 441 712 342 731 259 823 207 804 020 243 435 978 480 857 832 319 848 407 818 676 3  
 730 618 869 842 922 194 669 589 247 798 294 004 327 048 350 833 760 504 909 234 587 043 517 615 340 3  
 710 166 889 918 858 506 240 000  $q^{5516}$  -  
 454 054 151 365 963 701 908 003 137 378 548 944 402 384 025 602 910 358 080 412 641 830 549 006 317 3  
 190 545 541 494 389 175 025 599 747 848 130 121 080 466 044 564 949 251 620 632 380 391 188 410 434 3  
 547 479 915 703 931 471 049 913  $q^{5517}$  +  
 506 648 626 559 051 653 850 735 550 555 482 550 945 552 846 839 959 390 710 483 963 959 512 608 242 3  
 566 474 233 713 746 036 464 221 827 189 676 578 290 668 695 195 274 940 166 634 439 735 180 199 697 3  
 778 209 337 003 438 342 144 000  $q^{5520}$  -  
 525 497 202 818 632 480 279 852 711 123 367 301 208 395 303 315 762 560 399 336 504 079 419 692 141 3  
 904 779 691 315 013 099 931 103 714 769 725 351 577 052 421 679 991 548 873 340 277 011 979 663 811 3  
 671 031 629 282 054 172 672 000  $q^{5521}$  +  
 586 343 923 748 401 953 478 233 562 865 877 237 696 999 800 165 485 381 490 766 245 418 111 249 006 3  
 507 624 796 867 569 093 168 282 528 689 138 165 176 355 713 177 410 611 049 134 833 774 713 964 238 3  
 801 954 197 064 531 379 456 000  $q^{5524}$  -  
 608 149 337 717 698 348 535 623 087 272 412 411 980 028 947 464 969 095 288 667 126 423 513 914 519 3  
 817 217 358 636 501 737 378 877 761 757 983 248 254 964 109 741 232 307 429 575 619 547 839 824 322 3  
 561 775 004 847 065 592 689 950  $q^{5525}$  +  
 678 539 412 441 824 800 010 712 125 925 863 328 123 807 038 751 260 428 176 519 524 383 662 789 274 3  
 737 400 368 114 144 480 121 931 977 457 244 620 014 602 515 340 392 727 203 518 580 882 538 412 477 3  
 136 937 902 004 550 338 679 296  $q^{5528}$  -  
 703 764 188 991 085 647 080 331 410 538 081 350 992 586 093 790 663 435 820 184 193 985 268 554 220 3  
 676 524 418 663 399 774 904 341 643 982 079 175 397 450 662 212 689 555 800 989 066 769 988 572 003 3  
 309 216 298 598 073 688 064 000  $q^{5529}$  +  
 785 190 150 010 286 253 026 377 544 935 321 132 045 001 229 116 415 173 310 564 858 281 966 678 627 3

268 581 983 333 457 699 809 482 232 970 084 238 760 878 293 206 078 631 499 999 243 114 027 682 124 9  
 643 706 572 464 693 892 306 944  $q^{5532}$  -  
 814 368 958 319 513 703 599 422 870 610 407 544 850 769 883 391 937 253 753 492 215 605 325 511 786 9  
 922 654 772 436 342 886 099 566 069 206 703 284 325 143 403 507 101 782 266 619 594 891 785 563 799 9  
 875 868 180 601 581 310 632 766  $q^{5533}$  +  
 908 556 096 994 948 489 815 330 184 034 564 108 528 022 325 867 207 569 194 064 118 559 038 543 571 9  
 931 400 402 273 310 977 547 191 866 694 288 271 681 190 292 515 582 029 870 979 118 252 528 798 285 9  
 624 220 556 682 740 638 208 000  $q^{5536}$  -  
 942 306 971 492 818 045 305 601 400 272 412 938 634 555 059 914 112 568 797 286 992 941 643 556 876 9  
 494 513 415 130 724 007 705 210 297 743 968 765 089 493 095 430 213 066 977 273 123 422 857 427 645 9  
 150 725 362 309 111 308 419 072  $q^{5537}$  +  
 1 051 249 533 083 699 641 993 901 529 019 171 980 283 174 371 094 202 831 582 519 773 795 381 453 981 9  
 276 521 815 511 565 247 333 506 214 740 970 375 924 092 964 716 887 880 126 196 762 623 908 839 321 9  
 347 124 885 295 713 953 382 400  $q^{5540}$  -  
 1 090 286 834 658 649 293 572 489 591 307 313 568 380 860 528 689 475 459 401 881 833 554 394 113 288 9  
 464 128 358 353 439 505 613 774 527 254 402 528 072 072 148 459 370 696 984 538 651 540 347 791 348 9  
 740 125 388 538 582 642 456 500  $q^{5541}$  +  
 1 216 289 825 816 043 511 282 802 964 962 405 572 467 399 914 006 288 778 531 691 284 772 235 035 132 9  
 134 751 725 423 289 064 343 785 519 615 369 075 003 797 611 748 510 156 763 514 203 518 810 031 000 9  
 500 102 398 143 523 406 080 000  $q^{5544}$  -  
 1 261 439 212 432 409 897 950 627 156 829 966 762 129 203 266 690 181 693 955 632 154 572 300 821 827 9  
 102 312 872 731 283 288 977 657 468 371 782 765 403 926 262 011 826 821 269 263 718 907 294 063 880 9  
 161 151 087 395 455 207 014 400  $q^{5545}$  +  
 1 407 166 688 947 458 284 346 585 707 396 162 837 342 772 115 747 174 361 778 291 532 640 626 130 398 9  
 370 601 094 035 654 695 420 760 477 269 689 308 133 120 279 975 738 637 804 063 541 978 327 552 950 9  
 260 155 048 883 213 584 906 240  $q^{5548}$  -  
 1 459 382 406 302 461 262 178 929 664 964 706 104 264 619 016 268 101 733 851 736 547 173 202 917 528 9  
 115 240 470 250 120 259 565 197 208 556 937 178 357 673 808 792 195 390 569 491 500 357 666 850 831 9  
 410 749 216 868 458 438 503 875  $q^{5549}$  +  
 1 627 913 242 704 501 539 057 264 364 887 124 011 748 548 043 389 966 467 676 135 073 267 545 816 504 9  
 406 603 881 752 162 010 112 274 835 446 781 224 907 023 491 678 878 138 820 750 597 134 195 996 755 9  
 537 168 978 778 948 200 624 128  $q^{5552}$  -  
 1 688 298 093 446 756 877 301 119 544 320 511 115 354 108 233 772 427 892 417 992 845 497 059 660 006 9  
 398 146 721 677 846 107 672 893 023 924 822 674 553 657 750 964 207 636 333 361 432 468 301 717 487 9  
 586 830 439 178 561 727 004 672  $q^{5553}$  +  
 1 883 190 390 414 282 384 584 782 294 024 804 764 356 427 834 651 168 463 486 216 997 627 339 278 238 9  
 826 033 453 932 742 155 346 945 639 728 361 203 996 846 854 521 539 559 743 891 660 164 390 816 401 9  
 914 248 761 123 529 704 960 000  $q^{5556}$  -  
 1 953 018 795 689 927 186 451 113 306 762 900 875 490 716 814 497 083 030 523 456 180 490 844 281 351 9  
 988 514 503 488 847 233 040 183 555 073 520 351 979 294 700 970 540 259 098 321 089 033 941 716 340 9  
 276 956 495 662 180 586 795 796  $q^{5557}$  +  
 2 178 384 259 328 526 803 195 991 572 481 352 148 845 283 965 093 540 603 637 296 303 864 046 086 894 9  
 978 438 391 667 183 014 805 113 319 046 487 584 120 825 889 069 924 056 321 870 923 789 054 299 231 9  
 984 134 686 059 839 464 576 000  $q^{5560}$  -  
 2 259 128 890 155 167 609 436 109 811 957 284 571 353 651 920 008 545 309 950 563 510 538 651 300 878 9  
 144 834 797 171 683 273 222 309 003 442 896 990 108 474 534 722 227 826 205 254 580 843 885 955 727 9  
 611 674 880 161 814 253 568 000  $q^{5561}$  +  
 2 519 718 722 647 113 858 059 516 558 352 615 977 910 509 858 000 709 625 346 974 808 815 036 800 808 9  
 263 944 682 098 844 075 495 630 027 011 371 738 759 182 671 183 001 823 514 620 510 858 678 170 392 9  
 024 807 556 329 055 718 656 000  $q^{5564}$  -  
 2 613 081 252 139 281 490 194 733 395 959 631 968 649 072 636 943 920 945 915 906 143 740 693 102 150 9  
 759 755 006 553 409 113 846 415 234 558 619 201 193 921 620 675 940 994 633 807 319 114 168 566 001 9  
 231 574 619 319 769 184 412 375  $q^{5565}$  +  
 2 914 385 330 270 439 160 011 850 415 820 233 703 692 263 159 196 954 939 484 059 591 615 984 379 559 9  
 088 082 735 519 136 918 967 114 559 742 603 735 235 404 618 901 059 316 537 324 620 180 506 482 715 9

422 894 642 115 431 444 643 840  $q^{5568}$  -  
 3 022 331 942 552 400 061 078 601 045 909 837 684 686 046 636 429 432 307 637 341 464 828 038 866 293  
 031 338 664 728 328 765 751 605 225 582 053 423 808 717 550 251 614 126 384 316 833 140 427 875 663  
 954 985 089 808 289 398 784 000  $q^{5569}$  +  
 3 370 693 334 004 980 558 252 009 516 456 910 282 018 518 375 084 456 265 475 733 543 577 010 984 910  
 682 506 005 451 344 044 811 684 280 711 903 842 607 869 855 805 673 122 779 264 767 711 411 831 158  
 813 268 710 942 987 491 147 776  $q^{5572}$  -  
 3 495 495 723 475 943 367 377 171 072 084 192 587 953 762 457 764 006 659 949 381 386 373 715 752 278  
 071 779 300 354 568 051 331 821 602 177 732 102 462 991 385 991 250 047 257 280 839 660 773 454 383  
 546 621 554 677 549 825 346 072  $q^{5573}$  +  
 3 898 242 906 109 437 044 699 137 127 084 787 270 050 102 524 102 983 802 215 631 303 773 766 304 389  
 062 085 126 819 813 662 607 170 494 474 358 974 942 125 428 763 349 158 439 044 912 172 442 990 319  
 021 791 017 174 441 957 376 000  $q^{5576}$  -  
 4 042 525 613 564 599 300 281 963 750 110 106 910 132 769 920 792 518 410 629 014 377 615 630 853 458  
 074 865 290 383 704 266 317 525 805 085 423 935 726 725 529 663 726 143 592 375 744 266 039 439 516  
 079 836 269 839 002 642 251 776  $q^{5577}$  +  
 4 508 125 126 611 152 087 050 370 512 510 278 768 812 336 451 396 365 674 824 120 392 656 512 981 984  
 097 236 699 660 819 317 028 955 519 236 972 812 727 619 161 014 634 500 114 236 715 149 208 483 757  
 175 848 174 273 322 195 507 200  $q^{5580}$  -  
 4 674 920 188 865 880 769 419 601 160 918 051 813 406 513 227 950 764 103 772 781 445 361 968 012 351  
 009 303 603 388 406 849 373 059 324 844 363 049 582 091 586 314 459 786 093 179 439 051 376 384 619  
 525 642 301 960 846 133 614 750  $q^{5581}$  +  
 5 213 152 864 439 068 603 716 920 397 963 678 587 003 421 698 592 994 854 685 086 492 408 488 041 799  
 376 832 010 074 311 147 233 938 619 051 987 792 142 437 040 744 004 256 104 919 952 681 777 861 015  
 305 861 931 381 189 789 696 000  $q^{5584}$  -  
 5 405 962 904 199 324 005 577 486 186 010 912 645 883 690 708 838 606 026 267 266 382 011 724 221 058  
 281 012 384 618 211 926 877 706 724 838 727 274 465 327 031 219 359 078 266 980 739 344 176 752 194  
 689 155 450 486 205 444 915 200  $q^{5585}$  +  
 6 028 127 311 283 822 321 702 071 664 333 120 967 182 736 810 440 953 328 309 280 134 623 814 562 909  
 486 292 589 989 770 896 005 398 597 417 565 542 715 220 645 140 742 737 238 741 155 852 132 632 156  
 456 303 671 555 344 589 512 704  $q^{5588}$  -  
 6 250 998 367 103 828 828 913 576 084 774 542 523 306 072 097 973 528 311 370 315 305 207 164 564 719  
 142 013 140 472 223 640 448 887 249 436 083 013 689 958 168 121 075 066 880 821 971 256 011 038 177  
 926 982 803 079 275 281 804 125  $q^{5589}$  +  
 6 970 145 658 085 089 474 989 667 455 707 417 883 637 653 229 592 345 815 282 598 337 413 497 036 697  
 425 728 753 036 405 855 411 632 724 638 284 817 944 202 793 136 624 196 299 377 441 401 321 884 723  
 795 043 785 499 083 786 869 760  $q^{5592}$  -  
 7 227 751 253 868 299 264 689 712 985 090 438 016 331 254 220 771 402 355 970 876 033 800 055 036 874  
 020 498 460 859 994 484 565 361 778 151 261 543 583 236 378 538 956 689 656 498 402 641 565 704 139  
 180 650 468 375 870 787 289 088  $q^{5593}$  +  
 8 058 956 247 001 024 407 017 340 922 151 008 657 175 157 462 357 274 976 048 669 504 392 279 683 821  
 718 604 916 979 785 688 454 397 479 620 882 675 092 620 782 106 180 661 906 488 072 613 539 911 464  
 666 483 565 880 366 692 096 000  $q^{5596}$  -  
 8 356 694 430 683 317 197 080 790 953 915 607 144 258 536 005 582 458 713 960 261 810 605 193 874 285  
 003 042 538 679 770 629 961 409 090 226 931 700 483 384 875 139 308 066 951 117 333 383 195 540 414  
 780 430 832 320 482 071 963 592  $q^{5597}$  +  
 9 317 368 503 735 657 364 949 809 267 923 027 572 581 745 295 381 237 409 921 688 160 068 195 439 743  
 160 015 805 077 173 290 091 890 313 089 140 181 263 564 482 807 937 479 390 302 683 623 989 901 489  
 460 222 301 409 794 268 160 000  $q^{5600}$  -  
 9 661 473 850 208 204 846 437 185 139 640 963 790 709 277 990 961 686 597 899 740 303 147 687 814 353  
 338 672 455 698 869 280 707 247 207 886 700 773 266 158 882 748 848 309 111 494 956 726 192 738 965  
 499 559 130 692 852 101 120 000  $q^{5601}$  +  
 10 771 726 075 893 141 737 625 829 242 326 908 287 934 601 202 247 592 446 747 102 197 695 939 038  
 588 011 630 548 099 381 817 517 388 703 219 537 291 058 046 983 781 675 170 179 204 469 353 676 738  
 981 768 867 119 197 646 059 520 000  $q^{5604}$  -

11 169 398 955 254 923 637 517 840 033 639 953 413 468 349 537 861 321 148 235 535 153 916 982 963 \
 452 809 940 265 387 538 024 974 829 889 148 125 539 005 704 808 855 201 612 755 433 773 438 786 462 \
 847 449 384 959 905 284 531 301 050  $q^{5605} +$

12 452 452 895 298 540 616 957 394 033 237 419 266 468 338 918 736 294 695 202 834 604 328 241 800 \
 135 330 354 079 654 379 622 294 077 112 894 818 316 288 667 274 111 987 461 370 035 844 698 137 537 \
 158 613 193 016 542 171 588 807 168  $q^{5608} -$

12 912 008 660 372 285 105 628 649 089 071 503 966 939 327 978 680 771 578 195 450 100 327 781 957 \
 005 764 326 125 111 409 511 291 022 890 573 611 593 154 436 178 443 316 405 864 926 740 553 924 785 \
 949 833 746 194 473 487 327 232 000  $q^{5609} +$

14 394 683 372 134 820 390 884 421 718 621 795 080 037 090 816 852 382 216 022 024 064 940 684 195 \
 364 924 250 514 965 388 757 239 413 216 650 430 118 523 587 863 270 715 522 979 208 620 908 432 710 \
 711 868 739 573 729 132 649 323 520  $q^{5612} -$

14 925 724 525 975 239 047 045 448 965 086 587 273 158 400 318 507 999 958 454 247 988 084 439 890 \
 833 108 946 881 778 932 044 776 955 921 183 673 523 776 169 049 395 937 289 854 109 249 920 915 506 \
 301 977 935 026 377 039 026 400 827  $q^{5613} +$

16 638 989 646 436 290 262 724 037 588 417 807 976 788 032 223 364 639 891 107 815 494 714 891 184 \
 677 950 180 570 710 794 269 123 818 065 890 067 428 361 932 926 201 882 564 358 212 041 896 909 635 \
 044 749 158 679 505 343 717 376 000  $q^{5616} -$

17 252 604 519 531 967 536 863 536 098 464 105 963 393 523 425 065 642 639 668 256 761 120 922 033 \
 729 516 239 501 040 152 911 409 331 399 083 901 669 621 739 751 116 634 501 349 449 521 226 897 740 \
 859 597 589 373 411 607 672 913 920  $q^{5617} +$

19 232 220 802 675 112 279 547 956 877 840 266 710 903 702 116 587 372 402 708 682 866 609 204 895 \
 875 428 682 175 621 528 243 137 106 490 072 825 553 784 295 579 425 789 200 622 947 748 232 138 704 \
 540 066 308 060 603 234 728 550 400  $q^{5620} -$

19 941 212 810 172 080 252 795 741 218 638 657 830 760 522 746 388 141 581 750 798 747 247 105 119 \
 954 403 133 766 175 981 751 748 581 912 921 815 259 458 152 798 358 080 994 889 538 873 403 111 847 \
 236 681 385 504 867 324 011 903 375  $q^{5621} +$

22 228 471 235 883 855 087 935 937 683 788 847 042 885 345 412 752 437 254 539 526 180 679 939 279 \
 700 372 812 329 486 717 647 607 789 199 567 362 729 531 272 012 385 196 077 674 242 247 527 599 078 \
 112 077 808 753 751 913 330 048 000  $q^{5624} -$

23 047 623 408 356 857 077 193 657 140 054 661 406 426 095 072 899 185 922 150 319 297 389 034 630 \
 458 860 343 251 250 967 899 817 593 711 282 758 281 926 176 252 040 674 678 402 878 404 982 306 603 \
 954 341 568 447 826 985 578 955 000  $q^{5625} +$

25 690 197 989 056 690 505 960 034 475 446 683 290 072 339 428 918 381 142 831 818 310 820 360 705 \
 260 329 538 189 365 244 849 433 717 350 730 908 100 419 945 862 896 209 708 511 515 616 850 978 842 \
 993 529 151 164 293 676 598 915 072  $q^{5628} -$

26 636 578 188 699 156 127 605 517 415 849 141 001 671 264 996 523 874 046 908 111 621 396 721 730 \
 948 099 171 126 762 549 181 672 693 171 728 853 442 833 198 982 863 907 812 706 321 438 443 366 652 \
 161 333 338 105 954 706 770 520 125  $q^{5629} +$

29 689 509 914 548 420 827 323 939 876 605 462 920 728 752 607 985 811 295 951 984 860 835 799 824 \
 318 523 803 262 441 135 242 035 603 662 367 376 316 668 400 796 734 507 549 378 978 395 254 657 792 \
 239 365 442 070 104 127 850 151 936  $q^{5632} -$

30 782 822 976 629 890 619 597 064 618 578 696 999 274 313 800 590 200 889 848 114 113 356 968 400 \
 167 751 515 747 834 817 664 466 639 628 726 257 790 516 194 361 272 611 940 273 424 774 180 969 919 \
 227 246 927 080 759 720 121 303 040  $q^{5633} +$

34 309 655 007 988 540 682 031 183 407 773 023 750 353 527 193 031 077 041 771 496 225 547 308 884 \
 902 561 078 814 033 030 260 324 807 852 196 181 173 143 315 798 248 349 977 418 470 161 186 597 876 \
 406 730 866 499 133 797 353 472 000  $q^{5636} -$

35 572 649 001 723 490 263 763 015 022 043 676 959 874 851 917 716 943 754 887 724 951 952 611 665 \
 040 485 316 809 817 433 130 395 726 607 761 496 815 932 078 501 407 954 054 717 113 818 506 418 638 \
 795 039 208 887 508 461 968 206 441  $q^{5637} +$

39 646 736 292 272 806 313 213 665 115 897 543 967 776 563 047 549 638 263 977 503 580 953 023 680 \
 758 465 501 802 004 945 042 149 764 936 699 478 157 569 964 389 347 649 031 007 890 099 208 343 658 \
 070 875 741 491 385 770 552 217 600  $q^{5640} -$

41 105 671 195 074 403 246 591 322 572 074 787 626 691 216 671 688 596 069 095 744 190 996 350 936 \

023 167 286 829 890 284 183 688 276 350 241 132 760 145 303 541 497 883 121 249 568 783 200 505 428 \
 854 114 785 022 147 966 427 136 000  $q^{5641} +$

45 811 691 272 599 382 191 989 770 512 902 503 330 681 401 766 644 346 028 559 979 891 997 181 443 \
 212 012 889 766 454 090 281 288 480 517 210 198 118 272 254 040 082 167 151 170 944 086 969 480 274 \
 753 675 066 242 679 882 683 136 000  $q^{5644} -$

47 496 879 619 187 797 229 706 480 110 876 772 906 134 710 646 542 899 038 321 187 802 352 288 044 \
 211 094 904 600 058 755 993 551 585 062 673 983 627 149 074 748 024 322 815 865 292 465 223 685 324 \
 689 666 236 759 793 714 552 438 650  $q^{5645} +$

52 932 575 334 695 824 880 385 654 679 252 201 777 186 857 512 624 188 827 547 670 353 149 304 073 \
 975 880 702 693 959 277 925 819 246 203 127 832 367 993 799 699 000 060 297 851 753 011 076 415 191 \
 019 728 755 762 270 612 255 932 416  $q^{5648} -$

54 879 005 863 181 715 202 977 366 845 997 227 629 705 128 120 692 071 159 073 939 787 899 867 858 \
 224 681 896 152 333 873 641 609 110 848 610 575 678 351 148 985 461 347 069 183 298 477 008 389 652 \
 629 664 864 208 229 500 772 352 000  $q^{5649} +$

61 157 195 624 916 314 731 481 981 490 062 887 339 919 706 117 167 479 482 091 241 578 539 056 980 \
 973 213 308 548 512 190 200 580 182 490 296 018 724 892 279 729 427 734 241 486 526 432 748 555 075 \
 178 365 292 518 670 630 227 924 992  $q^{5652} -$

63 405 252 625 138 205 737 005 743 365 383 981 278 223 455 602 736 087 056 216 652 120 070 558 578 \
 730 292 258 976 775 978 494 098 074 169 075 358 535 460 588 931 272 633 162 165 007 223 301 136 734 \
 058 782 838 895 757 144 691 895 795  $q^{5653} +$

70 656 149 056 660 720 706 646 583 630 566 812 620 730 999 334 607 013 322 371 339 959 299 699 301 \
 132 271 493 396 205 761 750 173 801 438 239 487 951 782 545 142 939 781 593 442 969 237 150 026 469 \
 514 009 339 150 414 296 126 592 000  $q^{5656} -$

73 252 442 065 520 313 293 290 473 599 440 740 518 830 733 038 926 125 753 049 720 194 723 804 844 \
 004 457 028 002 129 170 782 741 341 182 125 335 076 798 525 850 099 731 244 821 581 971 241 843 349 \
 978 204 130 972 124 975 953 674 240  $q^{5657} +$

81 626 326 275 233 529 375 962 668 467 362 794 178 286 912 870 886 136 081 952 031 338 506 752 877 \
 810 040 353 586 882 891 439 150 087 603 958 557 873 403 824 893 571 723 945 964 385 058 727 185 770 \
 207 421 456 794 764 210 827 315 200  $q^{5660} -$

84 624 646 998 465 514 147 447 139 730 229 299 414 417 120 477 761 538 897 877 128 744 812 738 931 \
 845 771 869 571 662 555 363 866 563 766 043 242 345 219 318 586 795 404 974 437 197 290 598 516 455 \
 628 585 296 911 688 485 619 227 500  $q^{5661} +$

94 294 952 847 082 747 943 133 467 179 564 518 343 147 200 227 738 975 703 395 581 275 964 695 667 \
 007 585 369 447 404 286 433 760 324 387 117 807 376 184 060 214 701 163 507 536 661 202 250 812 529 \
 683 132 191 497 012 794 222 592 000  $q^{5664} -$

97 757 378 761 628 951 324 173 422 974 418 289 418 445 174 933 586 314 999 999 821 245 165 389 079 \
 597 123 738 022 357 616 983 719 325 414 607 483 467 775 381 129 564 187 859 384 982 488 145 150 545 \
 667 580 635 128 173 538 549 760 000  $q^{5665} +$

108 924 249 808 467 279 398 967 756 653 297 219 095 627 377 079 363 417 366 516 974 968 192 823 095 \
 783 258 708 991 441 346 330 894 765 265 787 064 934 505 214 007 948 487 729 321 866 605 833 583 152 \
 688 798 059 088 422 073 902 563 328  $q^{5668} -$

112 922 416 865 995 588 807 401 095 237 636 837 409 823 770 614 140 801 212 951 789 095 155 088 275 \
 831 957 468 913 365 513 456 914 403 879 804 892 924 906 523 010 370 820 707 785 135 063 721 575 180 \
 697 315 905 568 255 984 729 552 625  $q^{5669} +$

125 816 808 230 750 618 012 669 401 418 709 705 916 735 272 877 051 956 604 390 352 510 400 637 450 \
 739 447 082 119 932 632 902 097 451 556 384 181 722 966 408 419 872 742 883 845 244 003 813 250 143 \
 683 574 074 321 789 516 798 950 912  $q^{5672} -$

130 433 378 500 270 952 879 405 560 776 432 732 959 425 536 067 287 302 670 161 254 180 570 104 285 \
 908 829 594 421 557 516 783 848 465 946 920 749 661 016 744 203 768 524 789 613 618 141 198 746 875 \
 866 301 670 156 981 392 220 422 144  $q^{5673} +$

145 321 786 885 407 586 169 278 192 257 313 041 032 349 087 073 743 380 908 543 076 384 223 510 117 \
 394 553 886 654 338 873 275 940 974 851 637 120 540 226 743 651 067 114 731 130 453 763 072 781 756 \
 566 724 442 727 874 548 992 256 000  $q^{5676} -$

150 652 140 909 779 133 274 625 387 209 016 919 539 144 079 565 295 205 348 617 599 274 658 287 819 \
 758 261 705 453 387 384 452 132 960 115 427 580 432 026 583 292 137 208 112 922 192 886 981 773 933 \

749 390 699 950 724 020 905 739 812  $q^{5677} +$   
 167 842 058 710 071 766 398 556 883 747 906 689 060 706 217 133 260 291 935 452 070 482 015 257 922  
 675 178 311 267 530 969 416 959 948 155 370 738 763 549 901 117 498 506 406 017 789 329 160 805 927  
 820 778 685 668 591 431 174 963 200  $q^{5680} -$   
 173 996 246 886 197 061 274 983 341 157 463 867 471 205 309 448 165 458 902 595 374 524 271 444 184  
 405 637 048 015 972 508 974 784 642 495 706 697 491 511 082 387 547 197 174 917 207 739 455 415 612  
 055 622 735 318 683 635 777 536 000  $q^{5681} +$   
 193 842 450 919 788 561 339 756 272 773 165 983 240 926 776 996 110 944 959 051 455 653 429 182 712  
 525 867 542 513 105 225 855 075 602 197 343 915 814 379 699 622 940 164 787 535 591 434 152 121 115  
 717 360 925 648 787 444 989 696 000  $q^{5684} -$   
 200 947 443 436 079 463 089 511 865 888 452 962 117 597 248 125 721 780 941 899 713 526 526 166 429  
 655 891 090 249 973 933 271 732 420 173 090 274 065 740 441 207 282 696 443 539 273 699 293 675 205  
 999 214 821 573 548 429 799 463 250  $q^{5685} +$   
 223 859 245 657 526 120 852 762 851 008 998 901 186 275 611 438 273 542 163 331 248 239 594 717 445  
 362 587 028 820 669 270 642 594 936 992 269 524 416 594 737 731 086 396 570 657 251 231 675 066 303  
 223 303 233 010 150 546 685 286 400  $q^{5688} -$   
 232 061 526 539 125 873 057 052 164 958 604 549 943 943 498 654 878 462 334 674 849 939 296 971 859  
 484 578 513 162 365 798 206 459 861 294 781 917 039 416 071 498 748 104 617 247 348 013 370 124 969  
 594 567 219 236 947 713 839 104 000  $q^{5689} +$   
 258 511 133 475 163 258 978 822 081 103 404 401 807 164 881 100 685 587 634 969 706 984 414 619 125  
 377 595 597 018 862 960 361 332 224 879 634 686 408 412 990 271 555 123 252 940 265 349 343 230 387  
 263 379 237 675 052 051 607 949 312  $q^{5692} -$   
 267 979 691 217 495 148 864 401 065 048 942 294 695 420 107 353 919 136 760 820 689 907 849 885 424  
 486 940 651 785 817 832 608 629 600 474 625 645 981 226 242 511 232 367 772 811 370 444 040 715 167  
 800 405 769 178 580 765 505 231 471  $q^{5693} +$   
 298 511 841 187 328 894 595 715 292 816 794 170 289 609 047 422 200 168 035 341 947 172 781 762 798  
 118 125 766 209 644 775 736 282 477 365 225 900 077 505 254 355 422 242 437 225 060 691 590 479 924  
 756 556 890 954 906 232 815 616 000  $q^{5696} -$   
 309 441 616 440 021 912 752 769 395 865 781 277 802 185 638 309 229 737 467 347 137 150 056 428 407  
 971 108 015 555 321 367 417 023 417 774 630 135 876 185 718 701 345 263 265 795 330 286 034 039 223  
 953 473 243 940 993 040 092 889 088  $q^{5697} +$   
 344 684 689 328 810 828 939 448 813 151 299 223 014 572 377 845 396 615 746 564 480 585 672 979 979  
 097 620 967 287 751 132 917 564 913 356 646 958 744 110 969 622 328 442 372 209 489 373 615 488 024  
 908 582 446 219 861 729 305 804 800  $q^{5700} -$   
 357 300 549 283 990 868 932 775 394 870 733 177 111 636 577 873 424 207 331 188 494 212 487 383 138  
 777 485 534 694 454 322 582 511 786 062 503 703 246 800 936 786 083 089 964 154 697 503 474 101 457  
 305 399 281 778 849 250 110 149 750  $q^{5701} +$   
 397 979 373 242 986 853 394 632 293 172 038 483 711 354 988 537 132 564 854 786 457 430 049 210 325  
 634 693 388 103 278 614 333 999 277 878 341 212 953 489 314 308 446 954 407 974 959 492 039 707 268  
 177 528 327 895 758 500 642 304 000  $q^{5704} -$   
 412 540 692 967 380 477 137 856 913 577 048 424 155 986 293 035 142 999 110 258 723 284 134 013 584  
 418 001 597 285 165 441 269 285 321 346 507 851 254 765 936 149 853 310 045 285 701 003 023 498 371  
 643 245 380 141 557 432 338 022 400  $q^{5705} +$   
 459 491 306 506 309 718 382 749 391 668 444 772 218 682 177 098 156 428 241 793 268 376 006 826 058  
 614 545 234 203 777 472 523 471 416 701 084 354 235 599 644 692 836 695 045 451 920 861 061 229 706  
 251 344 017 987 238 696 128 419 328  $q^{5708} -$   
 476 297 249 646 256 140 801 597 584 925 624 639 737 699 847 255 031 008 344 094 150 520 551 554 501  
 069 190 677 849 903 264 419 531 161 048 159 046 622 238 769 129 455 380 870 226 651 527 931 652 479  
 423 675 557 997 661 692 698 616 375  $q^{5709} +$   
 530 483 916 841 228 160 799 049 880 027 840 628 107 453 473 473 717 671 710 341 926 649 087 931 769  
 023 291 705 289 193 416 940 962 869 007 725 559 928 459 660 024 774 012 519 462 585 274 363 518 807  
 773 942 401 696 680 141 960 445 952  $q^{5712} -$   
 549 879 522 165 963 242 455 672 530 778 753 890 162 563 754 825 084 831 742 355 313 542 734 175 246  
 161 965 488 925 925 067 323 975 417 085 241 189 989 491 730 470 167 185 305 752 916 619 464 364 046  
 704 037 403 124 601 708 726 779 904  $q^{5713} +$

612 414 343 909 969 477 189 954 561 008 110 152 873 506 890 665 225 817 780 765 205 031 612 999 516  
 814 408 262 045 497 243 433 328 083 506 647 110 426 627 122 670 101 735 053 323 416 654 607 924 024  
 333 996 629 204 874 004 402 944 000  $q^{5716}$  -  
 634 797 540 320 396 634 556 052 804 922 991 718 558 093 407 200 570 679 455 949 604 793 636 976 795  
 381 329 690 931 542 264 373 900 608 167 921 659 812 756 266 983 840 883 608 876 132 605 792 100 648  
 351 528 387 733 490 280 856 521 620  $q^{5717}$  +  
 706 963 056 591 397 903 129 085 164 402 598 815 214 372 042 095 610 603 692 026 768 201 712 978 709  
 537 130 692 207 508 873 868 606 940 637 939 495 503 642 159 416 554 356 116 381 358 238 407 592 113  
 707 491 124 254 865 193 034 547 200  $q^{5720}$  -  
 732 792 747 829 982 849 726 650 812 421 910 413 429 147 631 030 545 086 448 611 238 216 177 710 151  
 869 502 665 982 759 322 385 865 328 869 009 189 914 609 238 006 589 057 503 129 295 770 980 124 059  
 123 682 161 256 331 806 044 160 000  $q^{5721}$  +  
 816 067 985 877 042 123 414 969 217 156 847 484 346 491 740 100 126 182 866 446 611 082 280 088 086  
 775 161 988 432 323 328 667 449 027 140 591 610 288 170 712 990 981 886 798 770 837 689 310 218 305  
 633 379 437 177 858 191 969 280 000  $q^{5724}$  -  
 845 873 367 598 786 635 208 233 882 113 435 938 361 130 957 316 670 302 813 291 453 616 732 251 943  
 046 620 880 707 268 778 484 712 297 627 241 420 167 956 075 927 314 850 108 318 601 919 896 892 178  
 336 896 016 042 951 024 102 087 325  $q^{5725}$  +  
 941 963 859 938 621 116 761 262 365 684 075 706 788 858 951 105 950 316 327 740 014 712 397 988 426  
 717 123 503 260 337 077 951 898 007 476 522 514 054 163 513 968 328 603 985 912 118 976 369 270 734  
 106 199 413 562 861 716 663 119 872  $q^{5728}$  -  
 976 355 156 468 207 271 713 439 849 455 364 130 607 731 191 670 458 334 272 756 557 370 193 288 199  
 884 121 647 447 750 602 480 873 029 307 869 402 194 863 559 329 551 845 416 699 144 755 841 350 755  
 286 052 455 716 524 544 401 408 000  $q^{5729}$  +  
 1 087 227 532 010 796 947 747 300 695 510 409 664 496 190 284 171 280 227 887 006 274 303 058 071 959  
 456 242 520 691 066 865 380 374 215 282 267 424 335 699 777 224 495 920 410 843 306 979 544 532 255  
 422 682 723 849 271 881 500 016 640  $q^{5732}$  -  
 1 126 908 368 505 811 344 145 452 501 944 507 770 153 466 447 904 171 493 134 258 815 994 521 495 168  
 395 746 442 460 026 811 899 235 051 800 179 962 507 172 173 955 748 641 418 215 907 372 202 644 718  
 144 559 563 597 308 730 695 593 702  $q^{5733}$  +  
 1 254 830 211 561 995 920 139 690 167 600 440 968 162 201 533 273 381 305 154 185 966 087 604 495 980  
 589 400 996 040 736 074 542 649 800 276 032 531 157 935 953 528 295 709 467 445 344 108 724 732 889  
 825 172 697 376 071 595 740 160 000  $q^{5736}$  -  
 1 300 611 869 989 044 325 556 368 233 157 082 143 187 455 716 168 631 149 148 406 175 594 788 884 152  
 933 996 310 132 835 660 070 953 237 744 485 951 977 753 887 420 673 386 704 349 595 160 999 898 776  
 953 939 897 408 120 159 980 912 640  $q^{5737}$  +  
 1 448 197 647 165 730 662 551 472 738 216 534 338 414 791 908 015 476 835 630 014 969 836 368 482 740  
 900 052 318 895 218 373 735 776 512 689 443 647 131 296 346 485 023 397 291 548 319 666 931 221 023  
 896 104 101 630 947 806 932 224 000  $q^{5740}$  -  
 1 501 015 492 122 206 735 631 230 050 337 028 312 230 603 784 625 825 715 057 956 229 883 279 217 028  
 807 344 252 391 280 441 457 822 120 513 959 995 034 957 172 646 930 098 663 941 013 659 369 696 912  
 586 133 694 479 440 988 350 615 125  $q^{5741}$  +  
 1 671 279 468 264 432 684 860 827 818 868 649 729 668 244 673 684 499 859 893 397 333 386 186 504 359  
 915 805 119 779 656 901 720 572 748 178 304 818 314 060 559 004 094 803 959 112 400 891 512 552 053  
 984 449 544 716 148 647 012 352 000  $q^{5744}$  -  
 1 732 211 871 987 928 529 836 367 968 299 201 747 185 674 509 159 514 885 340 585 907 334 075 256 791  
 671 874 039 760 508 612 155 915 487 977 700 516 437 673 876 253 110 517 442 620 937 643 711 753 262  
 326 188 878 263 886 804 849 459 200  $q^{5745}$  +  
 1 928 629 075 777 103 989 774 186 135 375 454 680 195 933 996 049 619 745 771 646 857 787 967 362 468  
 801 816 719 397 146 104 264 109 874 915 953 923 109 958 941 205 844 595 301 859 075 755 982 005 999  
 380 323 907 534 384 294 832 070 656  $q^{5748}$  -  
 1 998 919 221 532 990 684 603 386 526 368 728 913 129 783 132 333 990 374 791 134 723 860 497 174 510  
 209 191 570 209 798 114 456 323 986 200 515 013 063 994 344 811 239 644 240 539 203 005 665 396 034  
 714 031 997 301 074 588 246 653 875  $q^{5749}$  +  
 2 225 495 681 852 565 703 133 448 982 667 544 957 120 612 261 852 513 563 725 816 392 792 256 162 254

071 007 344 055 910 575 546 830 695 549 522 922 972 053 398 062 541 045 278 040 468 603 976 790 793 512 618 335 658 375 270 369 021 952  $q^{5752}$  -  
 2 306 576 682 262 756 892 285 231 361 213 504 732 139 630 372 071 010 907 522 431 591 022 966 090 976 050 638 559 721 412 217 954 135 469 013 956 372 437 749 849 190 470 721 944 945 006 530 890 756 531 725 990 756 181 180 420 694 835 200  $q^{5753}$  +  
 2 567 930 341 165 553 965 452 196 063 352 569 642 600 256 917 851 225 396 993 833 199 793 619 724 110 773 565 208 861 550 336 103 281 803 687 344 439 670 121 253 724 736 844 711 844 955 179 829 642 146 986 968 733 490 081 453 698 048 000  $q^{5756}$  -  
 2 661 454 174 070 366 530 824 998 879 278 443 379 602 801 610 887 004 507 320 517 269 704 639 060 826 229 057 787 428 511 627 152 451 364 204 295 909 005 955 054 025 205 871 260 663 146 297 251 642 469 288 306 048 595 623 435 103 274 083  $q^{5757}$  +  
 2 962 908 094 770 836 429 375 309 601 093 004 453 571 043 691 882 886 785 137 655 265 398 750 652 176 811 740 714 786 665 603 570 973 327 139 671 594 200 714 657 044 487 537 759 414 665 428 445 696 033 883 098 603 330 612 400 107 520 000  $q^{5760}$  -  
 3 070 778 935 203 630 674 249 632 072 577 115 183 845 969 489 068 150 509 506 635 629 191 139 433 228 379 706 170 827 262 041 029 079 468 561 627 368 671 914 654 132 896 680 855 434 419 822 342 918 577 110 314 382 772 884 580 491 264 000  $q^{5761}$  +  
 3 418 468 668 165 322 806 173 909 269 593 422 680 410 004 572 657 003 486 960 741 026 909 304 589 449 499 482 108 415 507 031 708 947 468 417 087 622 225 788 720 102 061 429 085 789 495 857 301 927 019 662 426 912 173 811 922 556 928 000  $q^{5764}$  -  
 3 542 881 282 464 114 612 005 160 986 050 371 274 482 737 116 788 062 404 704 075 636 542 299 141 738 827 961 344 043 545 216 676 073 716 466 904 998 567 230 610 742 391 376 773 418 004 374 313 930 610 272 364 990 803 751 243 343 730 225  $q^{5765}$  +  
 3 943 878 534 178 526 010 978 963 550 319 583 806 650 808 782 095 117 552 445 930 761 943 476 035 770 632 874 659 601 728 468 528 567 881 863 437 079 272 014 163 435 670 572 939 072 602 026 726 842 218 879 223 950 076 709 690 044 364 800  $q^{5768}$  -  
 4 087 362 502 882 551 803 877 859 489 369 991 570 094 123 141 686 569 700 356 057 891 518 671 410 596 893 821 611 713 556 191 524 388 170 880 484 876 925 394 611 139 344 423 287 823 866 691 680 747 023 738 508 858 477 823 047 634 944 000  $q^{5769}$  +  
 4 549 817 575 883 997 916 231 798 899 484 049 986 856 381 653 542 685 223 218 360 479 114 736 920 624 871 119 838 619 578 590 431 120 141 042 243 805 381 798 630 391 363 784 394 462 260 673 160 199 715 550 672 445 598 909 802 941 075 456  $q^{5772}$  -  
 4 715 288 227 847 082 346 938 810 721 655 324 414 180 678 169 407 423 337 253 858 697 329 455 231 510 462 020 460 586 660 774 649 261 340 794 039 346 261 577 407 710 562 548 038 907 088 254 719 026 779 286 204 305 091 309 986 348 425 503  $q^{5773}$  +  
 5 248 594 073 254 124 918 533 880 251 205 439 079 163 608 976 811 741 652 925 066 625 864 005 985 655 563 294 443 466 570 431 702 970 750 895 048 407 328 661 862 269 442 303 718 693 449 122 699 794 919 339 285 489 468 366 917 112 138 752  $q^{5776}$  -  
 5 439 411 146 628 333 839 375 956 983 673 920 896 429 526 084 182 039 421 054 766 929 599 427 433 235 394 466 479 905 283 501 668 549 005 437 688 509 046 711 072 817 106 669 484 698 692 742 111 242 052 420 257 731 512 774 395 010 220 032  $q^{5777}$  +  
 6 054 392 299 375 687 814 476 913 062 093 229 298 500 764 437 483 507 435 398 720 013 368 068 751 818 492 328 561 171 232 286 694 204 965 515 126 449 888 058 937 235 080 225 796 302 637 527 083 528 732 098 960 526 734 775 301 761 300 480  $q^{5780}$  -  
 6 274 427 498 397 081 480 955 143 609 381 242 674 235 249 947 938 409 050 269 116 757 731 104 872 391 971 662 766 522 964 767 391 470 024 813 417 579 817 739 153 968 135 169 079 696 955 820 807 952 531 830 282 282 738 694 921 532 139 500  $q^{5781}$  +  
 6 983 557 658 750 911 462 657 343 320 699 793 251 336 396 699 727 442 456 925 460 689 458 941 533 325 420 763 377 328 233 002 979 295 530 820 829 017 343 711 868 839 999 621 363 220 257 331 664 477 602 427 955 644 349 158 522 079 744 000  $q^{5784}$  -  
 7 237 272 451 605 420 244 027 097 152 666 127 175 676 527 820 644 522 556 551 031 495 673 828 703 753 586 676 462 643 370 804 042 674 201 398 889 922 482 931 789 196 187 365 373 646 649 543 912 461 434 191 507 110 208 370 859 180 032 000  $q^{5785}$  +  
 8 054 925 044 229 686 035 644 540 795 995 861 878 411 641 556 469 488 491 097 078 049 855 916 868 723 815 050 393 766 102 275 551 072 531 876 038 949 640 181 840 556 743 365 777 303 867 474 517 054 451

825 397 821 592 000 046 379 075 584  $q^{5788}$  -  
 8 347 460 250 153 210 733 314 917 940 178 904 198 166 074 142 730 126 269 278 038 272 359 366 896 265 \\  
 704 522 239 058 368 274 698 810 806 273 057 296 768 358 832 430 049 011 629 640 316 030 968 951 909 \\  
 841 009 552 393 685 320 270 717 625  $q^{5789}$  +  
 9 290 196 945 055 898 744 828 833 985 166 548 752 331 219 804 717 236 739 127 987 247 374 586 686 241 \\  
 778 723 479 766 552 235 025 220 406 431 940 925 868 456 809 706 437 073 878 497 932 915 551 946 926 \\  
 801 747 741 370 623 877 397 270 528  $q^{5792}$  -  
 9 627 475 892 208 817 579 886 417 685 912 326 506 697 526 593 930 296 406 999 331 499 475 535 419 750 \\  
 608 611 386 907 218 605 555 741 012 490 558 229 128 226 074 601 484 191 456 919 084 411 805 542 137 \\  
 941 385 504 822 774 981 936 381 952  $q^{5793}$  +  
 10 714 378 823 152 201 002 506 341 619 138 003 342 960 351 103 331 990 771 560 625 676 370 946 435 \\  
 748 109 655 862 054 946 578 254 108 787 238 496 563 010 096 826 094 785 187 852 079 294 497 055 254 \\  
 829 767 577 565 719 855 917 146 112 000  $q^{5796}$  -  
 11 103 226 127 280 132 828 529 362 764 615 202 704 325 238 779 220 399 657 134 120 036 520 233 658 \\  
 794 896 168 382 547 138 613 074 799 023 371 738 023 061 951 864 726 984 966 052 502 813 577 299 280 \\  
 337 840 494 398 705 966 978 672 337 186  $q^{5797}$  +  
 12 356 280 407 412 126 121 194 773 024 291 477 265 205 656 613 841 448 531 301 644 678 673 230 243 \\  
 834 355 928 594 163 587 624 204 732 645 031 551 336 027 708 068 050 926 536 960 030 387 303 718 217 \\  
 475 228 308 365 309 332 461 547 737 600  $q^{5800}$  -  
 12 804 558 730 121 940 179 888 602 877 506 246 119 405 260 122 599 080 011 070 156 889 132 687 093 \\  
 445 972 140 900 483 029 049 200 603 633 754 741 118 743 074 464 737 518 926 106 176 500 549 098 371 \\  
 632 238 901 161 232 233 561 128 960 000  $q^{5801}$  +  
 14 249 092 858 601 198 124 517 467 248 721 182 650 168 515 786 586 597 667 787 819 440 664 448 662 \\  
 971 149 343 078 321 345 887 644 971 036 784 835 700 692 815 810 362 482 172 355 763 873 275 024 643 \\  
 442 183 578 329 735 293 676 471 360 000  $q^{5804}$  -  
 14 765 860 359 290 114 844 993 461 358 347 945 384 617 171 009 009 881 595 042 375 642 944 555 499 \\  
 507 430 230 856 791 949 112 125 264 934 533 894 663 003 416 254 254 982 120 610 155 809 037 349 083 \\  
 362 027 638 209 623 269 271 564 757 225  $q^{5805}$  +  
 16 431 053 255 990 656 684 646 009 121 923 437 558 850 929 336 177 808 512 844 105 721 081 555 471 \\  
 720 858 858 748 147 104 566 192 326 929 981 203 340 344 247 737 325 210 683 685 036 180 241 017 422 \\  
 849 983 032 869 428 543 488 063 885 312  $q^{5808}$  -  
 17 026 744 860 016 680 738 304 634 910 172 401 297 881 413 208 012 322 882 854 034 128 886 642 972 \\  
 426 654 104 975 959 020 483 589 769 463 159 317 004 791 372 436 318 678 599 259 576 151 630 261 651 \\  
 975 842 541 806 745 736 706 613 248 000  $q^{5809}$  +  
 18 946 209 580 370 312 285 745 140 217 884 583 480 408 833 986 410 614 027 166 551 286 614 568 722 \\  
 684 774 218 878 999 049 815 947 470 298 641 218 495 807 170 687 073 266 574 728 918 287 881 799 172 \\  
 171 858 701 786 073 679 591 629 912 064  $q^{5812}$  -  
 19 632 845 655 932 260 583 365 777 512 656 026 847 291 749 164 253 440 811 080 550 204 959 991 131 \\  
 216 396 366 409 903 081 660 357 031 022 103 296 050 132 288 131 735 090 651 864 227 268 912 772 936 \\  
 937 691 565 909 581 635 963 586 833 561  $q^{5813}$  +  
 21 845 301 350 300 820 370 781 547 662 091 760 841 177 662 562 509 858 450 607 173 902 667 941 946 \\  
 156 442 693 608 482 431 718 577 047 962 340 977 740 755 923 717 258 745 010 399 473 052 700 068 611 \\  
 514 182 501 969 568 432 252 944 768 000  $q^{5816}$  -  
 22 636 727 926 886 867 275 478 060 770 880 481 651 962 131 241 102 457 901 374 194 913 384 676 218 \\  
 505 479 637 756 887 042 601 538 837 838 852 239 663 509 457 767 986 239 260 099 397 448 624 584 791 \\  
 211 825 308 932 586 403 138 349 563 904  $q^{5817}$  +  
 25 186 773 348 090 829 646 800 712 481 357 271 161 651 479 244 812 673 571 424 509 197 180 481 908 \\  
 399 007 288 945 441 035 374 485 160 671 791 280 900 087 032 176 478 952 857 706 701 467 658 543 520 \\  
 959 131 688 937 767 262 630 763 417 600  $q^{5820}$  -  
 26 098 938 630 807 391 852 536 369 899 452 581 572 676 896 747 939 126 837 701 972 686 540 152 469 \\  
 859 076 365 517 656 394 638 376 400 148 143 191 424 588 540 218 688 330 466 171 462 888 119 305 707 \\  
 411 010 253 136 884 638 260 922 884 875  $q^{5821}$  +  
 29 037 942 493 521 119 833 635 676 851 663 616 753 141 603 973 861 982 979 742 059 344 864 739 552 \\  
 508 915 950 600 751 653 839 046 987 278 163 457 155 254 491 257 584 029 118 753 175 463 904 284 115 \\  
 091 879 013 861 618 267 494 391 808 000  $q^{5824}$  -

30 089 215 142 255 278 406 408 129 852 297 054 264 076 351 560 158 770 773 515 062 166 211 408 918 \
 123 607 645 274 695 777 102 034 505 608 558 265 027 381 386 096 903 325 245 521 894 292 060 579 395 \
 026 041 808 580 251 260 293 019 238 400  $q^{5825} +$

33 476 340 937 925 998 060 116 961 930 140 418 436 750 561 379 371 767 261 548 016 684 798 308 694 \
 134 276 116 495 143 492 908 143 637 843 904 765 831 489 513 358 316 547 216 119 058 481 823 872 802 \
 214 566 254 067 585 334 175 987 367 936  $q^{5828} -$

34 687 876 402 059 706 144 427 427 791 763 412 887 320 835 268 392 153 533 831 016 378 212 905 065 \
 165 566 239 827 842 156 788 895 280 352 364 967 395 788 994 497 115 596 755 044 225 977 670 958 567 \
 494 781 953 399 242 261 547 272 416 125  $q^{5829} +$

38 591 261 917 649 775 087 501 995 722 556 049 483 614 120 881 808 472 417 827 256 064 322 111 692 \
 841 013 120 686 243 549 030 658 616 599 292 352 271 749 122 756 234 095 669 926 415 690 075 554 172 \
 435 592 485 182 088 424 188 782 322 432  $q^{5832} -$

39 987 424 061 946 106 748 899 200 583 876 518 452 805 476 359 540 315 761 434 033 030 206 294 589 \
 937 729 838 886 016 589 592 571 344 312 190 941 468 145 114 755 753 567 417 757 904 559 062 695 020 \
 022 384 003 208 736 385 078 066 511 872  $q^{5833} +$

44 485 538 891 653 514 378 853 549 832 259 581 391 763 115 240 928 151 727 703 890 436 202 691 583 \
 848 846 100 659 795 941 107 414 963 540 802 396 532 701 551 384 369 529 689 887 148 028 806 106 482 \
 449 044 310 043 067 074 464 699 584 000  $q^{5836} -$

46 094 385 235 374 568 073 368 878 631 528 916 671 519 654 110 710 126 974 242 425 576 783 270 542 \
 388 415 793 841 835 028 437 891 463 541 707 911 226 284 324 832 909 627 618 707 908 783 926 200 907 \
 600 983 063 703 892 619 053 484 937 245  $q^{5837} +$

51 277 593 070 750 293 627 536 046 626 174 120 868 549 023 933 715 943 719 566 943 730 478 944 383 \
 221 871 648 208 269 011 060 561 592 437 777 926 454 575 722 050 122 106 519 268 700 804 833 074 185 \
 265 570 728 065 139 129 404 715 008 000  $q^{5840} -$

53 131 433 211 185 449 825 667 433 945 524 691 190 811 882 283 511 570 760 670 493 933 560 126 475 \
 126 628 126 316 972 915 793 549 015 899 220 388 211 764 860 697 712 004 467 247 382 999 651 540 418 \
 397 249 898 620 651 215 347 896 320 000  $q^{5841} +$

59 103 789 714 753 341 375 742 874 044 672 234 494 205 998 971 665 019 999 298 982 828 879 330 905 \
 790 383 527 262 635 313 703 625 474 351 553 580 678 252 621 484 165 088 215 211 662 791 842 668 796 \
 591 093 436 348 662 895 044 937 216 000  $q^{5844} -$

61 239 827 942 427 222 188 073 492 427 654 393 122 391 406 701 791 223 951 563 717 244 793 403 054 \
 395 027 365 293 386 088 639 179 453 554 429 349 295 119 645 050 209 526 008 101 216 076 603 899 854 \
 084 568 351 271 804 822 387 927 123 225  $q^{5845} +$

68 121 149 631 167 439 752 005 423 924 067 678 497 061 253 543 495 068 263 221 522 691 386 185 255 \
 977 949 295 266 752 656 305 065 828 763 217 909 911 202 145 382 141 922 191 678 411 996 155 863 432 \
 601 758 710 607 947 102 681 894 608 896  $q^{5848} -$

70 582 224 394 968 282 293 127 334 481 035 442 085 938 224 322 473 700 542 728 900 857 803 680 601 \
 857 065 658 966 275 828 938 183 430 647 841 907 783 609 019 802 459 048 577 114 263 439 770 631 153 \
 468 646 152 644 167 559 987 453 952 000  $q^{5849} +$

78 510 469 272 628 603 239 737 073 916 269 410 592 819 997 903 794 281 886 450 254 047 179 851 725 \
 356 498 035 062 136 169 416 326 309 466 867 674 571 830 422 876 505 814 466 034 817 142 128 487 618 \
 843 963 065 972 730 922 225 646 505 984  $q^{5852} -$

81 345 904 051 013 482 595 376 045 532 204 899 810 397 126 272 415 330 857 622 609 924 173 982 371 \
 651 520 542 263 972 401 357 019 655 885 234 442 610 762 287 092 661 499 614 978 337 826 850 419 500 \
 435 534 352 797 309 709 462 431 159 487  $q^{5853} +$

90 479 910 835 305 385 137 290 696 990 220 272 728 789 042 175 627 616 205 934 679 724 689 657 917 \
 722 307 833 478 206 715 737 960 333 727 181 872 518 939 231 142 093 020 018 617 306 039 704 892 805 \
 664 007 732 507 244 026 841 166 848 000  $q^{5856} -$

93 746 493 151 433 665 827 337 711 121 996 969 743 569 824 813 012 256 330 238 206 977 020 616 846 \
 779 154 666 530 998 972 234 584 291 298 722 095 297 522 157 266 894 437 108 396 536 363 070 974 431 \
 871 855 122 110 666 040 021 667 708 928  $q^{5857} +$

104 269 132 962 238 717 754 211 389 972 555 449 128 605 431 077 147 287 905 519 710 609 971 444 379 \
 619 498 276 762 873 643 756 855 558 669 553 874 795 155 844 829 310 964 402 052 151 240 286 871 238 \
 825 840 475 678 529 035 977 926 246 400  $q^{5860} -$

108 032 240 788 673 368 226 848 358 452 932 370 131 521 005 750 780 193 391 471 694 236 490 662 885 \

261 425 959 519 187 293 700 959 991 051 946 211 287 334 884 830 104 953 032 625 900 894 074 211 137  
 390 760 571 535 471 166 663 713 108 250  $q^{5861} +$   
 120 154 043 232 538 549 721 071 140 600 095 277 398 980 826 509 373 506 670 983 205 605 235 227 038  
 822 772 581 440 695 256 288 647 452 100 345 370 719 486 626 663 065 805 652 472 236 138 987 362 120  
 847 559 341 328 359 488 714 152 640 000  $q^{5864} -$   
 124 488 940 913 642 649 377 583 781 769 083 526 280 516 862 732 862 955 340 867 093 489 474 593 326  
 515 832 576 372 717 763 295 942 988 677 089 660 156 817 709 553 789 788 308 172 120 039 246 121 071  
 525 267 950 420 031 462 897 156 096 000  $q^{5865} +$   
 138 452 265 774 424 776 407 264 561 873 410 835 111 839 271 829 319 136 301 475 130 798 949 150 981  
 549 604 506 504 783 558 390 620 699 499 218 884 431 735 309 660 404 625 439 033 089 097 184 078 301  
 249 946 979 570 844 146 141 544 933 888  $q^{5868} -$   
 143 445 594 907 598 876 231 812 233 548 935 495 066 396 342 588 138 847 846 338 496 021 151 670 978  
 866 341 866 018 164 517 917 367 426 682 270 906 310 429 119 278 478 959 718 664 423 690 610 092 111  
 249 799 017 012 910 130 096 540 928 375  $q^{5869} +$   
 159 529 431 312 707 808 767 979 446 440 339 915 835 736 830 245 062 858 280 211 712 935 317 716 286  
 540 638 495 035 856 952 970 510 872 570 985 132 242 549 833 003 198 601 716 691 953 779 464 948 138  
 124 289 243 593 389 423 516 638 806 016  $q^{5872} -$   
 165 280 925 837 290 058 394 067 578 877 220 689 990 939 786 423 261 592 402 796 652 173 005 447 026  
 605 379 394 638 243 923 283 861 584 848 398 163 127 833 223 033 416 815 088 248 169 167 470 856 564  
 289 827 438 691 001 457 900 468 961 280  $q^{5873} +$   
 183 806 413 019 836 751 898 527 613 578 833 440 934 555 205 394 511 493 891 161 333 830 946 377 421  
 514 436 027 839 096 810 616 196 122 642 577 123 560 589 287 300 251 461 100 363 577 390 338 564 109  
 947 224 000 932 593 095 312 825 344 000  $q^{5876} -$   
 190 430 872 138 474 589 706 866 279 600 351 296 212 283 146 316 244 750 324 179 358 271 371 578 202  
 047 959 623 216 833 613 818 775 432 299 085 280 559 781 802 153 516 483 381 900 956 027 987 453 731  
 484 484 355 947 932 745 348 951 746 244  $q^{5877} +$   
 211 767 649 994 644 210 801 329 414 372 364 288 510 772 218 958 745 284 321 230 981 785 395 289 917  
 524 837 675 267 170 295 621 526 155 213 302 069 158 426 804 438 010 187 250 024 010 563 130 228 086  
 229 186 937 279 513 171 157 156 582 400  $q^{5880} -$   
 219 397 207 580 833 078 430 048 685 863 669 959 995 877 343 131 947 237 442 697 761 621 366 083 684  
 012 409 550 291 466 982 042 661 139 655 106 840 715 372 362 804 620 486 470 799 916 256 760 680 443  
 773 195 345 780 405 693 720 350 720 000  $q^{5881} +$   
 243 970 721 401 035 079 158 769 997 945 439 482 638 101 372 209 389 786 563 214 016 172 599 341 584  
 152 288 405 766 189 749 968 913 379 795 529 440 392 604 840 104 559 726 561 922 390 426 316 216 785  
 669 058 346 430 833 161 256 807 936 000  $q^{5884} -$   
 252 757 456 325 451 101 940 270 300 916 581 088 240 924 881 671 312 319 141 936 611 823 558 686 903  
 938 493 908 006 093 143 251 131 605 091 151 649 645 493 627 271 282 588 628 334 342 753 839 839 429  
 198 766 795 933 064 006 543 055 098 650  $q^{5885} +$   
 281 057 358 669 682 643 293 603 580 821 937 582 939 599 097 355 049 931 621 274 314 617 471 484 191  
 161 339 281 417 095 833 233 510 224 224 722 020 048 338 110 081 069 478 786 069 549 561 345 741 133  
 007 440 831 036 465 022 926 781 939 712  $q^{5888} -$   
 291 176 297 118 472 027 271 637 314 695 479 855 720 674 799 886 402 427 846 176 554 906 755 088 349  
 362 475 294 066 756 953 466 368 177 566 524 434 786 903 285 728 003 580 014 465 775 108 609 669 673  
 938 626 858 587 766 114 893 209 600 000  $q^{5889} +$   
 323 766 111 169 654 917 175 782 965 369 718 886 430 581 319 684 960 677 994 305 605 895 967 151 269  
 113 914 491 426 650 309 439 501 981 535 828 545 983 696 279 507 347 836 461 585 150 613 244 713 083  
 117 671 622 204 098 942 134 580 133 888  $q^{5892} -$   
 335 418 679 658 089 902 420 221 802 989 545 567 962 606 926 482 702 440 526 093 115 883 628 507 204  
 518 205 881 802 179 227 530 122 696 398 752 264 749 946 591 222 529 802 921 000 008 202 602 545 049  
 380 494 639 049 572 502 430 709 179 037  $q^{5893} +$   
 372 946 912 933 899 368 605 915 348 924 709 877 851 428 880 467 720 266 988 203 399 409 571 487 093  
 840 520 861 434 521 085 560 261 100 902 986 214 767 947 082 680 462 573 469 746 678 771 738 421 943  
 389 358 122 197 880 875 478 226 688 000  $q^{5896} -$   
 386 364 909 485 871 047 664 378 011 949 309 546 590 174 736 795 999 445 875 531 755 267 699 329 653  
 825 490 414 997 147 684 248 758 691 875 661 006 064 039 891 823 869 422 860 037 581 028 849 546 197

011 094 549 785 484 226 671 846 359 040  $q^{5897} +$   
 429 577 834 992 840 213 936 076 819 312 584 133 637 406 902 738 579 651 464 884 939 913 796 920 503  
 159 763 928 757 986 645 003 709 182 122 031 524 688 140 090 901 278 399 417 729 674 454 855 725 552  
 727 477 394 716 826 852 894 007 744 000  $q^{5900} -$   
 445 027 996 029 438 408 579 371 178 011 853 697 174 343 759 347 604 295 883 633 341 908 121 238 298  
 817 088 533 645 963 169 300 915 212 049 545 490 572 432 536 830 143 643 017 683 918 127 592 362 777  
 326 894 424 515 216 928 748 854 476 625  $q^{5901} +$   
 494 784 350 346 076 095 046 104 025 361 323 294 233 980 916 387 894 047 873 854 159 177 442 396 374  
 087 736 601 929 567 466 618 289 742 534 663 398 692 125 509 159 086 792 339 310 476 700 530 236 801  
 028 931 319 458 192 061 277 634 560 000  $q^{5904} -$   
 512 573 602 398 938 731 363 446 248 327 091 565 919 472 315 058 369 573 277 589 040 737 469 813 745  
 972 435 810 673 105 457 955 054 580 835 389 789 534 301 094 036 799 871 241 740 509 143 496 641 470  
 339 242 587 857 614 025 045 799 731 200  $q^{5905} +$   
 569 861 487 400 889 989 371 303 605 164 895 461 715 701 617 257 119 575 837 024 746 903 432 856 000  
 552 214 036 177 899 295 851 640 672 921 633 798 830 447 739 535 521 296 622 175 196 290 187 823 529  
 548 502 876 972 601 385 804 059 869 184  $q^{5908} -$   
 590 342 986 060 746 959 408 767 788 411 634 149 856 332 984 076 162 722 006 511 661 910 114 455 931  
 182 524 284 687 369 980 478 896 337 765 493 338 777 406 202 683 818 513 278 409 013 185 218 559 098  
 692 939 583 371 652 114 170 133 234 625  $q^{5909} +$   
 656 299 303 766 662 746 685 282 667 575 425 853 712 034 786 634 355 138 291 032 903 438 299 973 202  
 479 307 850 591 677 205 229 495 855 309 398 760 663 969 142 915 017 593 973 288 029 859 177 066 632  
 141 071 632 241 434 263 464 366 492 160  $q^{5912} -$   
 679 879 377 550 178 048 090 216 574 382 566 136 294 777 993 563 928 385 336 837 208 312 460 337 772  
 719 701 951 136 761 235 502 824 695 887 745 966 949 643 262 498 767 116 756 760 834 261 113 318 329  
 748 536 356 343 202 760 719 290 761 216  $q^{5913} +$   
 755 812 176 693 946 993 257 422 598 392 689 457 743 987 403 055 642 409 219 991 405 457 069 478 579  
 063 494 094 162 537 659 337 262 435 272 848 881 986 451 907 292 754 960 550 229 043 371 006 652 059  
 220 711 924 280 641 180 315 194 368 000  $q^{5916} -$   
 782 958 311 056 040 017 263 546 376 372 277 420 236 727 955 891 748 854 208 953 722 631 495 829 148  
 457 483 328 748 366 673 645 350 091 108 196 319 256 616 418 082 389 673 691 056 996 873 009 290 784  
 815 896 498 432 859 281 500 672 887 985  $q^{5917} +$   
 870 372 480 423 021 571 169 785 080 949 185 527 978 894 867 442 781 165 735 206 082 540 792 076 582  
 230 594 585 483 317 939 916 274 077 951 727 268 341 941 788 264 598 118 328 371 382 363 618 062 343  
 450 723 533 063 104 459 908 697 497 600  $q^{5920} -$   
 901 622 497 294 206 748 230 582 894 053 448 929 998 738 458 242 333 990 937 651 545 837 451 813 670  
 541 150 072 739 930 219 913 250 910 344 246 059 088 408 003 148 681 263 167 513 727 720 291 150 443  
 810 234 655 605 723 264 827 039 744 000  $q^{5921} +$   
 1 002 249 305 679 340 021 876 157 424 273 257 866 696 165 207 882 113 652 002 396 599 894 958 723 550  
 455 357 972 023 546 357 685 116 825 238 247 077 213 989 672 971 872 522 980 915 578 026 473 501 094  
 770 216 067 639 163 654 936 651 776 000  $q^{5924} -$   
 1 038 221 917 054 974 595 710 566 205 749 521 187 808 351 227 279 268 831 324 713 816 803 414 279 123  
 401 276 567 544 915 021 926 655 685 381 992 276 445 993 654 999 939 693 535 602 475 610 110 342 717  
 232 935 200 291 502 713 275 686 678 375  $q^{5925} +$   
 1 154 052 974 152 563 194 020 890 663 850 042 572 137 635 933 733 828 797 543 757 662 218 293 999 758  
 275 222 974 496 198 315 708 710 418 845 128 770 653 200 854 297 913 000 414 374 332 589 999 145 057  
 430 871 553 177 029 322 685 573 306 368  $q^{5928} -$   
 1 195 459 914 847 124 436 455 576 706 370 314 432 193 634 159 089 374 411 153 403 385 834 148 095 858  
 097 663 764 245 737 011 030 727 248 830 247 849 076 272 960 719 246 338 947 236 781 472 393 454 616  
 611 713 458 270 280 853 903 331 328 248  $q^{5929} +$   
 1 328 786 212 892 975 420 606 908 501 009 949 159 139 981 337 308 213 120 666 037 566 480 441 749 159  
 072 742 720 158 572 520 085 483 650 920 401 500 718 537 251 086 824 128 789 427 823 141 705 381 100  
 697 514 830 056 310 799 895 658 475 008  $q^{5932} -$   
 1 376 446 188 107 098 650 955 048 888 039 807 133 916 489 941 452 843 907 186 943 661 726 903 417 777  
 503 226 257 322 579 423 936 025 895 212 373 114 932 206 692 385 177 805 171 292 904 202 338 427 433  
 083 856 274 929 853 982 821 767 346 332  $q^{5933} +$

1 529 902 982 301 702 226 772 606 112 588 246 968 558 709 893 849 110 743 944 785 493 071 379 603 046  
 982 330 957 880 438 142 412 354 244 772 528 813 437 292 699 700 169 172 200 677 393 677 671 246 427  
 669 718 660 808 557 263 146 397 696 000  $q^{5936}$  -  
 1 584 757 700 717 476 601 488 324 789 493 976 155 659 787 292 558 872 584 454 030 106 398 664 898 779  
 485 597 937 383 562 219 733 121 487 200 762 432 797 874 796 677 487 486 962 727 472 805 587 246 351  
 620 866 244 402 356 020 333 497 384 960  $q^{5937}$  +  
 1 761 376 099 244 232 897 857 383 040 549 325 383 451 600 166 087 312 613 942 145 201 459 983 321 521  
 452 594 071 116 897 389 882 460 069 205 272 585 563 646 875 780 623 141 832 602 612 186 717 573 510  
 346 322 659 080 385 261 096 249 753 600  $q^{5940}$  -  
 1 824 508 702 636 321 950 273 377 642 357 042 634 407 261 201 767 702 933 172 488 875 505 277 605 993  
 199 790 605 741 037 768 691 381 081 092 923 448 574 070 350 881 597 694 796 285 911 968 753 786 371  
 667 968 142 663 843 371 542 819 855 500  $q^{5941}$  +  
 2 027 774 966 609 287 042 679 672 170 868 176 401 214 093 068 725 692 876 722 144 023 732 874 483 605  
 817 688 239 575 147 958 929 157 285 736 076 866 127 205 635 042 276 653 062 204 052 998 733 679 461  
 993 188 795 064 538 617 453 321 344 000  $q^{5944}$  -  
 2 100 431 213 206 058 335 004 567 764 908 519 236 784 487 634 338 033 787 162 709 418 737 281 305 176  
 881 924 352 860 488 134 784 364 640 997 272 579 591 839 161 712 411 056 905 092 178 996 116 654 730  
 282 001 672 161 362 309 611 133 337 600  $q^{5945}$  +  
 2 334 354 915 613 672 509 190 043 137 596 933 177 648 027 294 984 463 828 650 873 200 416 968 110 285  
 507 509 124 556 279 231 772 821 898 395 899 591 976 577 341 252 832 909 651 444 419 653 201 398 921  
 292 566 004 324 099 124 440 215 977 984  $q^{5948}$  -  
 2 417 967 527 547 613 661 746 775 856 021 322 277 978 230 472 796 166 680 565 868 275 619 669 607 293  
 195 255 230 364 177 291 908 114 501 608 776 304 038 639 232 952 801 133 889 358 253 081 274 508 560  
 476 394 987 680 149 065 968 335 545 000  $q^{5949}$  +  
 2 687 159 891 044 209 834 902 212 679 662 565 677 933 177 641 038 483 703 384 565 968 226 368 674 497  
 050 389 835 884 604 702 109 379 170 166 852 192 195 058 499 614 201 963 122 676 599 610 050 683 321  
 959 190 692 076 719 483 618 817 474 560  $q^{5952}$  -  
 2 783 376 537 208 823 666 664 734 352 870 147 795 015 050 142 745 196 428 221 316 967 252 853 144 814  
 506 726 910 001 212 185 763 497 775 084 044 776 363 118 975 790 054 112 035 893 746 856 628 172 329  
 603 800 600 728 382 058 205 494 345 728  $q^{5953}$  +  
 3 093 140 466 705 432 716 601 685 466 048 536 905 577 875 401 750 587 871 420 992 776 555 298 848 273  
 402 373 993 903 260 406 816 945 406 750 830 120 208 848 692 674 419 129 991 779 405 338 207 685 621  
 586 051 036 688 041 621 051 025 408 000  $q^{5956}$  -  
 3 203 855 922 350 498 266 243 029 548 985 197 406 854 036 813 208 937 330 231 403 784 398 839 434 635  
 140 736 313 934 913 326 118 977 974 272 826 954 250 758 469 002 105 071 279 335 618 603 816 229 411  
 845 833 191 700 661 217 578 630 867 557  $q^{5957}$  +  
 3 560 289 473 512 505 329 298 304 646 548 162 585 925 725 432 525 775 213 419 870 181 976 139 142 496  
 577 208 616 610 230 336 212 075 717 762 492 194 310 698 282 553 039 057 156 262 630 900 006 575 561  
 550 088 253 087 743 212 035 009 152 000  $q^{5960}$  -  
 3 687 682 578 296 635 092 578 359 580 571 700 174 024 466 969 050 307 944 308 848 996 796 071 909 454  
 755 566 927 517 284 318 497 751 256 597 894 515 818 664 743 398 435 173 149 892 103 844 837 292 392  
 220 372 332 240 562 031 978 409 984 000  $q^{5961}$  +  
 4 097 797 861 561 748 371 304 794 162 441 090 840 573 802 610 343 947 521 415 544 088 074 768 121 916  
 223 815 256 630 593 728 323 696 929 462 927 914 949 906 204 437 939 186 338 038 948 169 682 203 437  
 050 777 606 764 830 371 100 794 624 000  $q^{5964}$  -  
 4 244 373 990 072 985 168 355 656 006 905 221 004 901 663 738 922 596 930 547 486 643 147 392 437 190  
 624 776 156 971 890 284 957 675 949 614 831 279 090 802 643 308 279 954 608 187 360 700 926 479 944  
 393 853 172 409 832 464 324 185 364 975  $q^{5965}$  +  
 4 716 233 806 585 020 003 420 243 427 651 999 458 256 394 131 113 429 003 761 322 870 528 608 825 753  
 933 831 579 082 336 129 034 285 425 043 271 216 951 370 013 133 688 292 260 417 046 357 209 501 387  
 224 559 222 022 942 023 836 014 657 536  $q^{5968}$  -  
 4 884 873 671 295 002 783 998 491 010 689 641 126 639 991 041 728 358 939 710 803 977 451 894 195 790  
 286 143 574 827 000 945 650 691 948 571 836 987 497 637 228 302 251 381 730 167 236 664 135 919 206  
 349 490 084 117 664 240 840 269 824 000  $q^{5969}$  +  
 5 427 748 517 859 118 319 618 321 885 852 457 446 185 129 768 498 051 067 188 905 594 110 240 200 022

575 009 319 939 791 700 311 784 027 802 510 683 283 568 396 696 469 114 284 930 407 842 240 278 569 073 383 224 928 355 433 671 990 081 536  $q^{5972}$  -  
 5 621 764 246 111 267 251 209 560 225 717 162 838 021 687 619 499 275 568 092 934 678 342 808 048 660 886 326 358 745 371 980 831 914 267 265 223 052 333 665 922 080 266 988 893 889 451 605 812 004 934 609 104 138 874 011 617 548 648 290 596  $q^{5973}$  +  
 6 246 312 717 398 788 683 288 348 689 710 295 115 570 744 207 331 985 289 076 288 447 959 096 339 041 631 997 090 019 411 109 670 636 132 569 561 085 239 653 909 245 277 693 694 175 903 973 980 606 068 304 544 285 086 241 443 650 482 880 000  $q^{5976}$  -  
 6 469 512 283 660 174 503 061 966 814 810 700 852 796 048 770 075 703 567 962 132 846 849 443 064 065 912 331 448 058 872 176 475 104 385 865 993 779 227 855 988 642 250 629 823 646 667 858 724 624 325 902 157 296 121 602 385 752 485 625 856  $q^{5977}$  +  
 7 187 988 348 864 798 190 884 388 790 763 792 672 924 992 393 055 687 101 837 406 547 423 531 786 890 045 057 794 986 220 973 142 090 275 455 831 964 454 772 073 292 241 509 918 249 543 281 109 047 233 305 815 331 443 503 574 084 396 134 400  $q^{5980}$  -  
 7 444 749 603 749 632 585 856 876 125 308 539 071 990 193 330 191 843 356 385 517 474 137 440 435 258 165 371 134 678 142 895 448 077 459 445 561 446 060 316 811 931 155 071 462 597 925 116 837 473 293 769 046 358 165 457 502 243 733 553 375  $q^{5981}$  +  
 8 271 240 750 255 125 235 972 739 373 998 024 088 882 758 156 582 710 322 062 594 863 758 467 570 547 262 586 340 351 319 206 886 660 913 115 139 734 415 988 343 742 251 540 925 651 907 653 569 012 017 579 533 518 840 388 756 845 587 456 000  $q^{5984}$  -  
 8 566 596 471 800 501 359 812 322 701 674 831 042 119 615 567 724 463 221 480 612 109 997 779 395 506 238 179 840 514 463 880 850 423 674 384 740 275 019 205 578 457 056 448 795 002 124 018 547 274 507 568 404 914 260 617 980 711 490 355 200  $q^{5985}$  +  
 9 517 297 299 951 772 808 092 685 461 358 688 049 109 412 740 763 484 214 836 658 350 073 352 008 699 011 175 414 454 105 821 303 017 607 801 787 866 712 893 159 717 848 699 322 050 557 519 093 377 280 860 323 481 971 653 757 707 204 575 232  $q^{5988}$  -  
 9 857 032 903 786 674 368 970 033 840 725 653 475 094 578 626 748 947 523 147 269 924 468 606 675 547 293 932 169 054 702 835 298 230 702 282 870 838 643 417 094 925 216 363 258 574 827 888 186 432 956 730 538 628 458 328 809 618 757 167 500  $q^{5989}$  +  
 10 950 559 435 789 617 271 974 634 215 441 527 570 502 546 084 516 824 126 523 041 110 682 832 666 031 847 911 116 264 763 047 226 509 279 834 004 734 733 455 481 046 001 803 655 249 974 631 522 122 501 057 505 388 193 498 010 057 175 867 392  $q^{5992}$  -  
 11 341 325 223 193 190 239 957 891 305 247 417 747 262 785 640 222 932 308 775 407 047 183 728 430 580 129 864 768 323 975 809 425 425 413 343 994 907 322 104 454 132 687 617 535 494 984 307 272 139 326 561 678 482 999 939 095 768 602 509 312  $q^{5993}$  +  
 12 599 075 968 382 823 326 764 327 952 405 878 589 009 911 925 015 469 147 995 579 956 592 196 623 011 235 435 017 974 158 794 163 921 672 475 485 679 347 117 450 424 100 754 456 741 847 743 465 905 341 546 841 420 616 315 966 454 047 808 000  $q^{5996}$  -  
 13 048 516 069 373 278 923 559 048 748 289 857 424 074 404 217 750 610 606 136 370 659 593 011 784 109 924 623 639 445 007 187 134 649 058 352 293 663 273 311 902 878 929 251 906 849 643 400 608 039 216 205 437 941 952 090 825 266 242 507 968  $q^{5997}$  +  
 14 495 086 782 355 962 611 214 131 246 136 072 736 191 784 069 170 332 187 078 012 879 980 058 178 309 928 948 056 259 714 885 960 723 915 384 438 940 402 808 588 783 752 257 470 382 969 861 621 748 900 620 889 980 033 924 909 818 474 496 000  $q^{6000}$  -  
 15 011 987 270 158 313 174 386 408 690 387 328 954 379 135 439 364 058 158 361 844 599 240 099 796 180 669 122 270 149 379 556 790 318 088 981 227 533 645 094 635 325 642 269 854 871 132 757 703 770 499 512 203 275 821 949 604 655 628 288 000  $q^{6001}$  +  
 16 675 647 364 593 522 808 899 924 900 383 206 013 025 985 960 406 634 196 871 546 899 949 163 499 188 894 461 097 079 512 170 217 032 022 531 878 313 291 896 697 164 058 820 872 810 909 944 126 105 450 246 946 087 724 013 220 801 248 256 000  $q^{6004}$  -  
 17 270 106 384 147 891 167 587 648 799 108 756 613 714 898 065 972 164 752 428 368 715 536 445 598 521 505 104 987 952 245 736 088 940 440 022 332 262 013 591 362 209 021 104 841 263 228 474 020 603 808 360 903 358 527 529 134 812 642 951 450  $q^{6005}$  +  
 19 183 346 142 617 464 128 892 524 871 298 831 706 466 889 878 998 398 973 448 241 486 024 657 945 220 159 829 111 715 399 419 215 949 720 532 726 885 895 677 282 645 941 115 867 741 409 233 424 364

$069\ 980\ 672\ 862\ 276\ 676\ 813\ 916\ 590\ 438\ 400\ q^{6008} -$   
 $19\ 866\ 969\ 316\ 142\ 788\ 726\ 464\ 866\ 194\ 886\ 191\ 572\ 812\ 156\ 649\ 936\ 590\ 712\ 530\ 429\ 393\ 315\ 678\ 358\ \backslash$   
 $317\ 616\ 698\ 874\ 725\ 550\ 984\ 354\ 855\ 891\ 231\ 518\ 123\ 804\ 808\ 983\ 562\ 972\ 967\ 680\ 829\ 309\ 665\ 037\ 315\ \backslash$   
 $885\ 451\ 536\ 768\ 320\ 278\ 647\ 612\ 616\ 704\ 000\ q^{6009} +$   
 $22\ 067\ 128\ 387\ 942\ 116\ 557\ 490\ 860\ 798\ 224\ 496\ 944\ 909\ 059\ 476\ 468\ 884\ 236\ 184\ 927\ 363\ 909\ 873\ 915\ \backslash$   
 $523\ 946\ 683\ 572\ 100\ 737\ 176\ 083\ 599\ 469\ 825\ 243\ 359\ 627\ 510\ 565\ 275\ 725\ 994\ 476\ 055\ 930\ 433\ 780\ 584\ \backslash$   
 $222\ 709\ 440\ 734\ 300\ 611\ 245\ 073\ 876\ 944\ 896\ q^{6012} -$   
 $22\ 853\ 253\ 242\ 913\ 089\ 238\ 883\ 023\ 655\ 458\ 302\ 373\ 267\ 634\ 489\ 976\ 307\ 605\ 795\ 738\ 378\ 512\ 572\ 115\ \backslash$   
 $216\ 275\ 650\ 129\ 840\ 944\ 225\ 065\ 842\ 862\ 991\ 553\ 884\ 812\ 501\ 240\ 784\ 441\ 575\ 867\ 546\ 781\ 338\ 994\ 089\ \backslash$   
 $126\ 587\ 041\ 023\ 553\ 389\ 955\ 667\ 074\ 839\ 336\ q^{6013} +$   
 $25\ 383\ 242\ 472\ 240\ 551\ 485\ 581\ 517\ 857\ 936\ 747\ 266\ 233\ 231\ 892\ 455\ 801\ 897\ 578\ 831\ 374\ 987\ 953\ 623\ \backslash$   
 $475\ 060\ 203\ 586\ 560\ 909\ 512\ 606\ 791\ 733\ 962\ 814\ 976\ 926\ 791\ 027\ 116\ 685\ 758\ 678\ 079\ 598\ 886\ 737\ 700\ \backslash$   
 $834\ 423\ 796\ 561\ 879\ 080\ 091\ 394\ 064\ 384\ 000\ q^{6016} -$   
 $26\ 287\ 196\ 190\ 585\ 461\ 275\ 603\ 298\ 089\ 440\ 812\ 313\ 522\ 205\ 823\ 995\ 488\ 962\ 286\ 147\ 370\ 441\ 672\ 693\ \backslash$   
 $660\ 125\ 807\ 082\ 902\ 874\ 343\ 996\ 622\ 399\ 999\ 308\ 789\ 567\ 312\ 232\ 416\ 408\ 008\ 498\ 745\ 415\ 845\ 833\ 711\ \backslash$   
 $247\ 511\ 492\ 767\ 662\ 271\ 467\ 261\ 749\ 854\ 208\ q^{6017} +$   
 $29\ 196\ 326\ 596\ 802\ 900\ 166\ 968\ 511\ 869\ 005\ 909\ 016\ 791\ 799\ 817\ 488\ 950\ 011\ 067\ 099\ 302\ 121\ 771\ 157\ \backslash$   
 $887\ 931\ 384\ 228\ 980\ 784\ 690\ 468\ 161\ 733\ 605\ 373\ 110\ 297\ 990\ 876\ 075\ 862\ 328\ 093\ 739\ 147\ 008\ 649\ 070\ \backslash$   
 $577\ 669\ 149\ 334\ 739\ 495\ 262\ 482\ 246\ 041\ 600\ q^{6020} -$   
 $30\ 235\ 722\ 019\ 140\ 787\ 718\ 601\ 548\ 361\ 057\ 918\ 622\ 506\ 755\ 056\ 655\ 328\ 447\ 701\ 432\ 607\ 230\ 294\ 201\ \backslash$   
 $505\ 373\ 770\ 086\ 961\ 822\ 794\ 863\ 114\ 998\ 807\ 086\ 081\ 547\ 687\ 911\ 159\ 385\ 028\ 611\ 305\ 240\ 004\ 138\ 144\ \backslash$   
 $050\ 133\ 928\ 094\ 200\ 198\ 606\ 633\ 024\ 810\ 125\ q^{6021} +$   
 $33\ 580\ 656\ 792\ 125\ 031\ 747\ 127\ 239\ 709\ 202\ 928\ 116\ 361\ 669\ 303\ 615\ 091\ 140\ 974\ 837\ 140\ 125\ 988\ 169\ \backslash$   
 $868\ 464\ 489\ 900\ 247\ 405\ 528\ 804\ 517\ 532\ 239\ 791\ 597\ 266\ 979\ 284\ 554\ 386\ 805\ 258\ 114\ 145\ 400\ 209\ 639\ \backslash$   
 $802\ 430\ 184\ 947\ 754\ 519\ 227\ 399\ 703\ 040\ 000\ q^{6024} -$   
 $34\ 775\ 732\ 339\ 419\ 037\ 428\ 531\ 079\ 119\ 499\ 772\ 123\ 289\ 278\ 668\ 914\ 379\ 803\ 850\ 065\ 605\ 369\ 355\ 581\ \backslash$   
 $572\ 406\ 836\ 927\ 909\ 769\ 361\ 709\ 798\ 279\ 554\ 799\ 345\ 831\ 448\ 408\ 533\ 873\ 787\ 478\ 897\ 136\ 910\ 070\ 856\ \backslash$   
 $028\ 544\ 071\ 688\ 722\ 473\ 614\ 839\ 302\ 553\ 600\ q^{6025} +$   
 $38\ 621\ 580\ 055\ 043\ 420\ 756\ 817\ 016\ 934\ 674\ 766\ 988\ 330\ 968\ 295\ 301\ 668\ 109\ 231\ 687\ 527\ 011\ 870\ 556\ \backslash$   
 $462\ 843\ 063\ 910\ 907\ 743\ 036\ 627\ 924\ 546\ 584\ 095\ 831\ 132\ 851\ 429\ 424\ 155\ 169\ 280\ 445\ 733\ 505\ 802\ 829\ \backslash$   
 $312\ 620\ 067\ 717\ 457\ 517\ 458\ 536\ 653\ 129\ 728\ q^{6028} -$   
 $39\ 995\ 590\ 065\ 897\ 192\ 128\ 589\ 395\ 625\ 567\ 078\ 793\ 618\ 232\ 878\ 359\ 284\ 851\ 114\ 606\ 096\ 252\ 925\ 687\ \backslash$   
 $147\ 345\ 203\ 455\ 187\ 316\ 121\ 292\ 370\ 960\ 644\ 984\ 677\ 002\ 386\ 894\ 215\ 499\ 596\ 945\ 922\ 389\ 385\ 026\ 605\ \backslash$   
 $755\ 490\ 553\ 487\ 826\ 939\ 267\ 572\ 371\ 615\ 000\ q^{6029} +$   
 $44\ 417\ 160\ 013\ 538\ 721\ 950\ 533\ 156\ 719\ 726\ 000\ 914\ 191\ 995\ 790\ 844\ 353\ 181\ 218\ 265\ 823\ 255\ 899\ 229\ \backslash$   
 $858\ 766\ 925\ 850\ 169\ 402\ 639\ 512\ 936\ 938\ 442\ 768\ 233\ 978\ 187\ 700\ 822\ 090\ 096\ 023\ 953\ 553\ 734\ 319\ 944\ \backslash$   
 $966\ 459\ 021\ 941\ 923\ 684\ 219\ 642\ 974\ 306\ 304\ q^{6032} -$   
 $45\ 996\ 822\ 954\ 261\ 707\ 108\ 531\ 462\ 758\ 627\ 136\ 401\ 990\ 163\ 012\ 281\ 675\ 253\ 078\ 520\ 108\ 239\ 777\ 911\ \backslash$   
 $810\ 533\ 471\ 654\ 510\ 104\ 317\ 291\ 867\ 509\ 048\ 489\ 475\ 304\ 047\ 843\ 995\ 427\ 746\ 375\ 952\ 568\ 906\ 317\ 074\ \backslash$   
 $380\ 977\ 621\ 991\ 360\ 323\ 741\ 343\ 689\ 900\ 032\ q^{6033} +$   
 $51\ 080\ 066\ 550\ 560\ 050\ 362\ 767\ 351\ 646\ 041\ 632\ 059\ 298\ 021\ 771\ 704\ 426\ 012\ 469\ 523\ 405\ 798\ 984\ 161\ \backslash$   
 $729\ 300\ 939\ 304\ 426\ 114\ 641\ 463\ 392\ 121\ 715\ 737\ 717\ 381\ 338\ 297\ 802\ 913\ 305\ 939\ 339\ 945\ 315\ 432\ 840\ \backslash$   
 $543\ 131\ 970\ 534\ 696\ 696\ 028\ 964\ 367\ 360\ 000\ q^{6036} -$   
 $52\ 896\ 079\ 655\ 140\ 878\ 695\ 034\ 708\ 619\ 313\ 932\ 313\ 929\ 633\ 205\ 994\ 036\ 555\ 887\ 196\ 162\ 645\ 095\ 733\ \backslash$   
 $130\ 914\ 681\ 845\ 083\ 446\ 319\ 653\ 103\ 659\ 721\ 282\ 363\ 011\ 538\ 438\ 234\ 984\ 784\ 646\ 395\ 418\ 646\ 232\ 121\ \backslash$   
 $837\ 170\ 331\ 588\ 036\ 395\ 685\ 745\ 638\ 092\ 964\ q^{6037} +$   
 $58\ 739\ 745\ 454\ 090\ 974\ 152\ 709\ 738\ 223\ 360\ 208\ 399\ 298\ 161\ 662\ 767\ 345\ 664\ 396\ 140\ 498\ 666\ 483\ 922\ \backslash$   
 $320\ 481\ 485\ 619\ 292\ 205\ 612\ 357\ 572\ 989\ 475\ 540\ 645\ 775\ 648\ 411\ 935\ 623\ 323\ 207\ 967\ 039\ 868\ 842\ 585\ \backslash$   
 $969\ 888\ 782\ 002\ 349\ 827\ 456\ 308\ 248\ 268\ 800\ q^{6040} -$   
 $60\ 827\ 375\ 613\ 056\ 441\ 252\ 204\ 879\ 943\ 187\ 485\ 439\ 717\ 817\ 810\ 937\ 296\ 704\ 876\ 451\ 651\ 370\ 223\ 575\ \backslash$   
 $025\ 443\ 530\ 266\ 536\ 789\ 573\ 805\ 879\ 266\ 040\ 593\ 501\ 931\ 486\ 434\ 064\ 162\ 654\ 762\ 900\ 844\ 659\ 983\ 252\ \backslash$   
 $526\ 102\ 793\ 939\ 695\ 256\ 889\ 007\ 595\ 520\ 000\ q^{6041} +$   
 $67\ 544\ 909\ 478\ 446\ 812\ 069\ 216\ 134\ 619\ 252\ 820\ 578\ 890\ 492\ 031\ 368\ 522\ 663\ 656\ 604\ 437\ 087\ 812\ 432\ \backslash$   
 $304\ 593\ 580\ 262\ 707\ 299\ 177\ 776\ 932\ 908\ 746\ 611\ 578\ 371\ 460\ 216\ 567\ 535\ 750\ 750\ 074\ 069\ 449\ 332\ 754\ \backslash$   
 $114\ 066\ 687\ 982\ 907\ 387\ 860\ 151\ 566\ 080\ 000\ q^{6044} -$

69 944 671 642 989 093 422 052 012 449 147 218 896 574 554 147 286 989 294 548 254 136 550 065 148 \
 996 993 305 749 146 666 165 669 847 997 733 777 614 432 805 389 919 059 976 019 630 636 749 981 843 \
 370 494 927 344 561 787 007 675 108 179 175  $q^{6045} +$

77 666 398 301 491 273 702 624 222 742 466 173 197 457 130 862 931 071 556 192 054 528 447 320 172 \
 739 881 238 124 552 012 668 749 842 444 044 052 135 451 575 958 294 899 360 689 721 607 385 546 016 \
 846 998 388 653 125 628 522 666 355 163 136  $q^{6048} -$

80 424 834 329 433 555 066 025 077 003 496 240 296 839 742 450 256 623 305 422 180 524 363 925 830 \
 815 228 358 179 868 347 847 067 580 359 709 677 940 088 368 880 298 408 120 146 434 020 265 843 058 \
 046 734 372 727 237 532 818 761 719 808 000  $q^{6049} +$

89 300 461 858 753 146 283 168 112 583 671 370 390 333 688 963 589 912 981 401 315 081 914 311 785 \
 164 806 416 841 379 499 204 022 124 799 716 452 716 529 496 072 285 631 284 260 366 877 252 140 986 \
 507 027 016 858 251 704 306 182 924 992 512  $q^{6052} -$

92 471 034 633 090 248 261 018 534 544 803 902 260 845 061 803 869 165 494 181 066 516 434 707 964 \
 721 538 935 685 294 910 309 035 568 199 227 685 921 338 978 768 688 440 821 267 645 111 320 628 716 \
 802 598 173 319 592 050 136 161 408 921 636  $q^{6053} +$

102 672 529 559 744 161 576 695 539 480 061 177 011 543 214 668 597 226 346 917 231 670 506 447 370 \
 063 665 727 752 476 163 812 199 796 736 252 127 731 775 585 179 951 876 744 717 913 616 442 261 471 \
 761 204 673 285 671 167 234 488 506 560 000  $q^{6056} -$

106 316 649 394 397 695 235 335 910 062 691 951 179 801 577 636 939 112 053 423 644 231 038 746 221 \
 740 366 028 953 783 156 906 201 279 912 616 008 894 029 698 856 284 359 487 593 439 586 439 208 948 \
 703 377 021 974 730 239 617 575 154 319 360  $q^{6057} +$

118 041 537 094 775 893 492 786 873 143 305 570 996 325 718 845 927 415 145 567 143 347 779 254 587 \
 777 652 174 471 894 703 316 115 358 383 636 018 557 773 470 256 137 251 855 621 952 052 613 914 527 \
 019 624 426 181 953 347 066 616 944 588 800  $q^{6060} -$

122 229 739 946 827 265 621 882 437 026 818 779 439 450 355 992 828 433 055 245 654 540 931 276 432 \
 598 698 843 533 702 582 155 158 578 825 337 827 429 701 622 163 670 792 931 828 711 683 600 819 390 \
 859 806 559 718 614 050 478 105 088 183 875  $q^{6061} +$

135 704 893 094 911 587 725 079 177 158 064 599 858 091 575 148 532 694 917 064 146 955 163 432 121 \
 345 528 762 794 521 876 737 439 281 010 622 665 476 002 368 064 290 105 374 302 911 861 883 144 771 \
 088 522 309 540 254 026 483 489 831 424 000  $q^{6064} -$

140 518 192 974 893 404 844 678 977 772 739 983 314 572 283 329 889 744 485 735 401 219 219 987 276 \
 203 166 230 582 452 030 517 191 415 222 841 886 315 226 626 216 643 168 590 320 860 575 283 489 084 \
 890 773 725 272 694 754 436 931 903 488 000  $q^{6065} +$

156 004 180 011 258 685 509 284 369 857 293 757 116 324 667 695 254 660 816 070 314 134 715 067 618 \
 161 940 014 331 120 892 333 026 968 882 692 610 553 308 018 886 372 777 089 881 893 167 451 237 777 \
 806 452 772 025 077 749 023 930 853 146 624  $q^{6068} -$

161 535 621 276 929 405 602 485 838 665 653 952 778 401 485 522 855 133 864 975 197 152 864 544 968 \
 003 332 403 877 227 205 225 818 344 724 703 540 458 432 602 526 367 981 577 559 459 762 141 544 840 \
 556 865 666 980 911 186 677 692 273 019 125  $q^{6069} +$

179 331 697 459 400 722 114 019 685 174 485 278 255 426 988 864 194 059 919 412 461 012 200 242 118 \
 834 350 792 431 625 330 236 001 195 355 256 641 910 131 909 509 384 029 912 411 243 890 292 011 248 \
 236 532 541 010 401 810 737 007 006 808 064  $q^{6072} -$

185 688 136 455 492 822 149 813 839 448 757 651 063 464 911 089 593 979 706 453 422 339 628 063 432 \
 451 529 943 307 210 240 685 834 039 885 349 633 608 345 167 477 591 871 993 475 198 950 307 199 043 \
 362 423 969 789 188 291 136 182 123 560 960  $q^{6073} +$

206 137 972 190 284 667 738 737 507 339 010 915 952 315 651 758 329 112 173 317 111 269 187 721 801 \
 188 900 057 423 121 799 843 156 373 620 601 949 142 440 301 697 131 760 318 914 681 544 617 274 075 \
 921 610 613 353 778 927 248 419 939 840 000  $q^{6076} -$

213 442 122 027 702 240 883 162 830 614 897 279 398 606 735 627 267 362 174 021 634 767 804 554 003 \
 987 198 661 329 611 154 842 977 610 362 837 128 125 217 753 264 282 406 372 847 718 591 603 223 632 \
 981 412 578 613 456 793 313 438 015 979 084  $q^{6077} +$

236 940 377 098 154 041 760 308 602 743 602 353 056 241 330 475 255 940 547 510 998 264 930 004 263 \
 014 232 626 052 620 959 582 026 091 513 403 635 550 629 248 962 727 346 948 653 976 748 162 349 101 \
 690 954 806 991 076 677 526 570 896 588 800  $q^{6080} -$

245 333 154 332 016 634 475 102 658 085 659 949 575 450 519 841 270 381 405 355 753 526 580 869 170 \

917 867 272 542 589 231 613 812 562 491 195 922 321 084 128 892 938 487 716 251 567 633 566 452 054  
 091 907 960 000 896 880 704 434 286 592 000  $q^{6081} +$   
 272 333 022 600 433 527 655 559 955 778 234 498 939 083 255 268 038 483 660 919 045 450 550 676 692  
 049 274 277 901 492 360 240 944 422 184 224 896 003 249 713 296 360 509 806 709 920 746 215 010 208  
 062 085 248 632 090 747 479 431 227 418 752  $q^{6084} -$   
 281 976 240 260 051 277 736 272 675 742 549 556 069 782 864 469 725 410 094 949 877 463 602 309 207  
 146 136 195 288 400 097 476 248 951 580 402 265 396 183 064 074 116 635 418 110 387 732 551 535 822  
 069 678 740 970 538 770 711 781 219 063 575  $q^{6085} +$   
 312 998 107 714 885 695 758 522 362 971 833 392 285 888 664 962 879 651 311 833 233 165 667 140 202  
 416 181 154 179 265 811 889 387 917 825 657 129 826 585 673 784 164 724 335 024 271 390 318 973 590  
 475 504 788 646 514 596 089 808 326 050 816  $q^{6088} -$   
 324 077 565 666 574 645 541 492 214 076 856 027 540 704 278 233 827 195 887 462 590 197 773 759 472  
 155 571 930 844 378 312 970 300 408 477 175 988 072 902 499 496 381 014 178 138 448 093 607 486 402  
 099 195 661 769 745 397 431 171 960 832 000  $q^{6089} +$   
 359 718 945 663 946 898 333 560 323 358 051 894 742 907 985 839 994 847 793 926 178 600 261 013 677  
 174 201 662 561 436 951 094 734 037 102 970 738 376 775 150 827 809 763 573 451 674 539 159 442 453  
 492 028 253 672 819 150 299 261 565 474 304  $q^{6092} -$   
 372 447 976 771 425 458 703 814 146 100 212 175 882 872 440 903 114 822 857 450 996 166 631 639 406  
 095 166 450 056 306 913 432 684 912 334 541 454 384 281 065 202 913 812 276 306 154 746 257 648 629  
 525 821 671 746 748 945 966 558 408 725 971  $q^{6093} +$   
 413 394 910 368 283 094 351 058 402 725 941 857 008 761 142 677 470 098 930 435 414 599 240 570 125  
 263 976 711 779 341 798 868 209 412 511 248 016 102 289 500 108 663 135 772 596 725 418 217 946 491  
 278 604 521 029 427 386 238 630 506 496 000  $q^{6096} -$   
 428 018 449 494 862 157 879 644 324 806 990 555 914 400 895 002 982 075 499 978 284 868 688 473 879  
 917 323 565 168 913 580 637 957 572 122 654 659 968 853 418 773 552 495 417 936 241 107 217 755 167  
 643 626 291 849 675 446 683 861 556 330 496  $q^{6097} +$   
 475 058 586 339 458 427 645 043 655 024 743 728 679 980 511 218 485 254 189 399 084 006 090 028 905  
 446 921 673 210 484 444 960 797 310 113 308 501 895 708 554 365 088 029 955 799 144 912 294 908 414  
 205 738 042 418 686 291 607 282 729 932 800  $q^{6100} -$   
 491 857 839 071 318 767 268 593 581 619 296 847 876 670 017 518 461 323 499 308 272 753 463 751 185  
 376 507 398 372 628 137 606 950 861 656 374 458 506 421 093 649 055 021 557 907 559 688 230 836 781  
 872 781 303 432 592 365 312 054 069 799 500  $q^{6101} +$   
 545 895 445 919 014 295 095 476 898 446 322 498 000 456 831 389 623 579 342 620 042 247 111 658 591  
 840 651 030 367 440 268 174 017 682 802 387 151 617 396 674 883 903 287 160 294 129 473 688 330 092  
 905 532 524 367 670 832 293 960 397 312 000  $q^{6104} -$   
 565 193 245 162 819 558 253 950 568 843 523 527 564 587 971 863 750 024 355 097 479 881 727 496 604  
 314 945 386 323 804 863 525 364 745 752 740 004 219 563 722 414 247 309 702 491 697 963 331 380 533  
 868 818 002 201 672 016 419 907 393 945 600  $q^{6105} +$   
 627 266 425 310 154 923 950 106 268 255 281 014 412 649 835 145 362 591 157 871 408 467 123 444 672  
 885 869 757 440 063 470 227 975 930 931 873 232 720 439 197 156 528 446 118 507 414 436 991 524 815  
 136 715 489 089 752 570 431 388 129 916 928  $q^{6108} -$   
 649 433 376 841 017 122 044 112 350 857 472 099 267 073 644 214 039 036 626 824 455 169 203 122 995  
 328 206 827 173 543 259 657 250 162 659 288 833 106 406 381 075 827 452 295 927 951 326 013 214 816  
 691 669 271 914 114 613 935 999 839 314 250  $q^{6109} +$   
 720 733 825 292 918 872 391 701 398 279 326 770 347 404 065 569 364 719 938 771 666 266 972 877 497  
 823 107 651 415 919 183 383 725 068 012 745 884 266 455 507 043 020 787 446 254 900 967 374 387 238  
 326 027 530 766 691 731 174 090 007 953 408  $q^{6112} -$   
 746 195 358 140 805 270 730 207 599 972 564 478 627 720 620 554 374 369 652 491 375 646 913 024 423  
 618 361 942 006 586 962 790 265 580 009 162 127 190 101 499 551 934 632 156 115 961 239 424 905 070  
 014 554 722 784 463 717 394 901 968 257 024  $q^{6113} +$   
 828 091 024 917 135 367 536 355 803 359 022 170 265 909 184 238 541 676 164 588 832 551 140 548 603  
 144 508 427 268 256 809 683 420 536 535 498 876 940 287 793 763 745 398 133 049 206 105 967 945 881  
 146 033 962 295 040 542 233 277 294 592 000  $q^{6116} -$   
 857 335 479 456 653 061 804 407 020 759 368 577 481 345 728 055 642 231 280 526 794 232 155 085 101  
 569 326 218 059 486 689 663 947 885 793 212 111 813 182 789 968 959 820 812 787 666 912 975 631 790

932 627 195 652 598 181 949 659 814 148 373  $q^{6117} +$   
 951 396 567 989 899 052 103 054 681 056 752 322 640 418 851 549 084 175 601 689 047 074 603 096 879  
 280 034 791 153 194 349 834 294 641 904 947 337 818 807 650 200 144 176 557 195 074 512 764 622 696  
 392 116 534 915 129 569 907 567 673 113 600  $q^{6120} -$   
 984 984 474 055 545 683 481 523 476 587 593 326 926 264 623 665 993 984 657 657 421 353 910 855 456  
 094 019 474 933 856 231 684 952 808 710 565 226 585 186 705 588 254 989 159 222 552 290 816 907 830  
 868 445 879 319 375 853 511 323 627 520 000  $q^{6121} +$   
 1 093 013 264 144 724 058 662 764 255 303 369 105 133 448 110 877 848 901 345 943 129 104 374 702 085  
 328 651 315 925 740 991 462 700 498 317 480 252 759 411 722 397 757 067 388 649 284 627 018 400 327  
 821 859 743 414 723 095 681 258 427 840 000  $q^{6124} -$   
 1 131 587 983 792 546 180 134 983 360 059 684 367 444 641 865 593 445 038 690 331 844 864 513 605 397  
 397 294 494 979 478 812 477 179 936 527 019 205 493 990 192 180 450 581 416 565 745 670 188 968 823  
 986 055 742 300 660 096 414 356 396 754 075  $q^{6125} +$   
 1 255 653 040 220 096 326 190 481 190 331 782 097 540 668 768 352 460 034 437 968 129 207 696 084 545  
 830 837 687 256 406 482 557 429 403 022 343 534 847 210 747 843 512 845 952 134 538 414 991 356 547  
 597 752 433 204 304 320 695 824 203 874 304  $q^{6128} -$   
 1 299 952 975 311 163 156 525 494 738 092 645 247 068 534 347 436 413 255 579 738 030 768 715 976 246  
 976 511 145 121 535 813 112 439 952 491 862 282 660 604 226 153 410 262 533 824 694 334 204 816 844  
 911 800 832 300 449 710 396 933 652 480 000  $q^{6129} +$   
 1 442 428 385 329 129 589 652 295 939 920 009 848 175 169 714 126 986 487 718 968 883 008 376 908 618  
 189 662 169 662 743 686 235 192 265 188 382 080 946 828 652 915 317 797 004 907 926 467 844 207 359  
 853 970 324 401 723 954 591 181 030 809 600  $q^{6132} -$   
 1 493 300 979 394 348 576 476 885 857 327 722 900 242 541 718 708 910 607 881 669 510 451 921 750 148  
 292 393 492 885 504 970 728 314 786 003 502 943 702 363 691 640 400 822 385 363 239 777 234 904 283  
 962 958 380 765 894 251 805 072 899 683 798  $q^{6133} +$   
 1 656 911 356 365 950 542 014 084 102 514 616 128 066 297 285 716 194 688 676 668 495 026 517 247 308  
 096 030 353 715 765 509 280 177 357 766 293 511 045 058 468 739 999 098 787 661 380 808 803 647 634  
 065 848 498 903 424 412 189 271 615 104 000  $q^{6136} -$   
 1 715 329 153 768 399 533 130 769 380 426 140 671 292 945 574 894 135 989 459 741 062 135 108 228 433  
 110 542 901 361 329 308 760 759 737 144 079 867 855 434 158 317 065 341 464 171 849 307 549 122 350  
 108 469 044 965 653 424 503 365 895 356 416  $q^{6137} +$   
 1 903 201 252 054 683 077 861 464 573 045 535 649 904 804 152 001 934 388 257 503 874 413 132 523 271  
 135 479 879 751 629 095 340 291 545 462 965 205 622 640 554 311 150 981 525 746 048 231 681 697 108  
 418 558 813 968 618 578 331 805 787 494 400  $q^{6140} -$   
 1 970 280 315 916 496 649 030 936 529 551 469 761 805 568 167 615 129 628 364 294 389 611 873 686 790  
 865 744 105 708 400 866 195 331 247 676 147 085 342 125 444 516 716 002 675 718 813 969 262 684 024  
 164 025 510 153 049 914 416 712 086 579 125  $q^{6141} +$   
 2 186 002 225 621 724 278 576 309 137 698 933 344 352 576 899 750 269 936 301 470 823 820 616 440 497  
 891 884 103 715 382 613 465 822 543 915 472 194 849 493 792 096 429 758 680 110 751 742 840 188 083  
 950 859 309 493 865 965 434 187 808 768 000  $q^{6144} -$   
 2 263 023 260 039 550 493 035 516 631 399 108 406 739 144 642 475 337 988 003 428 525 189 013 755 629  
 510 534 963 205 331 760 530 787 493 420 959 158 531 257 378 473 961 724 045 860 365 226 459 110 790  
 306 694 446 581 553 765 301 736 297 267 200  $q^{6145} +$   
 2 510 712 291 759 562 875 821 733 460 934 291 553 240 808 169 788 323 266 131 687 488 878 645 138 770  
 813 928 065 326 626 172 760 909 931 099 320 881 890 744 216 169 830 672 175 324 628 902 960 571 323  
 188 297 671 251 578 436 282 960 222 486 528  $q^{6148} -$   
 2 599 144 864 310 876 869 182 569 572 916 771 373 727 526 377 842 803 599 723 287 056 835 969 567 192  
 629 817 592 032 316 728 800 725 219 001 029 473 547 045 017 812 536 666 863 499 858 454 701 365 898  
 052 306 287 962 299 977 371 600 231 015 750  $q^{6149} +$   
 2 883 525 396 183 719 559 471 034 812 189 258 936 158 134 509 740 006 708 719 562 974 384 260 045 962  
 220 686 867 445 058 088 125 748 075 554 549 719 149 593 008 153 520 613 162 335 413 334 922 365 747  
 844 014 051 023 046 574 991 634 469 225 472  $q^{6152} -$   
 2 985 055 714 559 232 576 180 835 071 066 646 857 720 020 987 660 081 291 755 433 920 234 179 706 849  
 489 190 608 828 028 896 380 626 358 074 996 977 763 178 146 491 212 020 975 188 750 744 256 007 084  
 730 736 963 040 590 033 373 711 832 514 560  $q^{6153} +$

3 311 548 459 694 310 473 552 883 543 638 844 393 795 659 444 150 118 359 595 318 716 567 267 299 098 \
 822 897 368 605 183 958 644 321 092 514 515 221 818 192 489 617 351 438 862 454 501 600 894 520 554 \
 730 574 990 206 266 212 396 942 513 728 000  $q^{6156}$  -

3 428 111 222 548 050 784 421 272 725 964 359 746 727 423 792 705 202 751 165 404 450 011 483 658 093 \
 399 592 618 618 843 843 946 556 431 276 293 123 780 962 342 718 424 585 281 253 623 741 125 880 629 \
 889 494 507 690 477 718 574 633 761 536 284  $q^{6157}$  +

3 802 935 587 740 846 316 304 316 138 505 567 122 098 881 881 126 635 625 740 193 507 098 384 873 097 \
 175 822 231 261 839 930 425 126 755 909 269 063 626 603 310 073 069 830 078 108 067 736 825 912 708 \
 174 927 366 302 322 080 418 517 450 752 000  $q^{6160}$  -

3 936 750 505 752 791 603 226 775 697 788 947 787 670 510 977 976 629 217 386 465 689 949 643 526 196 \
 607 173 077 062 280 445 067 989 080 270 527 363 340 051 832 156 469 744 077 881 467 943 516 470 574 \
 596 412 513 626 555 782 537 414 311 936 000  $q^{6161}$  +

4 367 041 956 205 915 678 311 763 632 090 257 453 154 514 940 833 607 684 825 051 298 387 159 580 499 \
 447 974 050 209 523 898 849 738 592 171 928 677 009 570 196 803 920 413 370 298 226 736 057 360 370 \
 553 966 649 400 631 611 340 861 626 880 000  $q^{6164}$  -

4 520 655 626 303 165 623 315 226 986 109 499 382 017 585 389 812 589 205 197 314 137 385 628 446 188 \
 586 508 134 687 218 762 132 343 500 797 938 391 845 640 249 858 685 024 316 550 267 372 282 335 707 \
 863 374 624 419 353 557 858 873 333 831 500  $q^{6165}$  +

5 014 600 250 369 481 603 715 755 434 180 591 967 168 515 122 771 113 392 119 603 058 923 702 419 006 \
 699 171 093 114 024 250 730 900 301 143 925 677 378 633 633 614 651 286 196 376 345 237 093 144 205 \
 931 540 245 655 982 405 028 511 219 710 976  $q^{6168}$  -

5 190 934 165 654 587 209 930 793 033 589 917 736 523 312 509 406 797 453 008 954 659 162 450 929 505 \
 561 087 446 703 383 693 636 437 821 739 147 493 026 853 730 103 929 230 720 196 530 633 047 192 163 \
 542 745 328 619 297 094 002 264 809 472 000  $q^{6169}$  +

5 757 922 953 543 972 218 141 528 717 382 474 618 724 586 197 687 455 728 688 833 192 437 916 798 434 \
 599 839 048 794 194 191 924 091 521 232 768 344 048 520 068 036 570 872 626 592 194 895 259 653 051 \
 355 152 764 445 790 200 557 607 847 012 352  $q^{6172}$  -

5 960 328 545 569 071 082 700 508 722 778 334 460 938 989 479 676 178 821 981 237 901 184 978 284 098 \
 404 698 408 441 678 738 127 832 715 126 430 868 110 961 948 773 408 318 998 867 815 464 798 509 740 \
 769 293 062 891 738 464 222 521 343 352 682  $q^{6173}$  +

6 611 134 262 412 066 059 578 386 161 556 638 764 478 262 814 115 054 907 660 469 187 293 259 635 024 \
 158 245 680 141 675 660 495 111 349 572 933 802 008 294 668 001 634 510 384 532 861 200 460 696 088 \
 161 019 414 398 723 584 633 468 335 104 000  $q^{6176}$  -

6 843 456 003 116 492 733 523 323 469 408 332 712 616 541 288 754 523 631 754 786 296 863 448 189 589 \
 079 649 159 328 251 779 091 595 628 264 730 932 719 834 501 324 071 037 875 339 687 929 588 570 373 \
 467 720 345 597 293 843 658 305 832 878 080  $q^{6177}$  +

7 590 435 956 503 654 121 499 349 277 207 272 215 978 971 816 177 846 959 349 780 365 502 370 874 973 \
 845 914 893 269 970 607 886 152 620 120 191 760 578 017 189 498 772 988 456 881 635 228 262 481 945 \
 260 143 112 706 224 482 733 565 852 876 800  $q^{6180}$  -

7 857 083 696 806 329 852 165 580 902 581 272 149 329 183 663 708 386 442 533 121 075 422 517 295 326 \
 080 993 407 474 378 022 177 503 184 998 089 613 926 378 399 895 880 929 726 159 066 457 181 648 856 \
 797 623 545 272 195 302 892 943 342 828 750  $q^{6181}$  +

8 714 412 179 645 642 305 019 616 833 803 154 238 063 369 341 627 204 069 058 275 678 394 454 192 000 \
 457 316 870 311 103 059 568 790 064 034 479 087 882 039 367 395 024 560 062 714 511 483 689 204 917 \
 355 529 502 661 216 369 388 925 557 440 000  $q^{6184}$  -

9 020 444 073 105 342 687 694 588 952 592 399 668 705 973 951 384 716 042 630 273 480 661 376 901 841 \
 750 006 848 705 877 386 584 715 557 441 209 223 711 047 927 466 588 328 559 928 778 846 581 915 392 \
 957 169 831 319 147 508 743 193 934 233 600  $q^{6185}$  +

10 004 378 813 202 609 186 490 652 615 777 469 617 576 043 617 237 963 975 731 024 167 885 008 370 \
 757 388 888 769 804 545 475 875 481 484 460 008 596 132 040 482 642 948 304 976 822 359 500 893 541 \
 402 261 838 238 977 261 490 984 032 683 177 984  $q^{6188}$  -

10 355 596 369 480 804 292 737 312 104 125 430 351 221 405 739 125 628 099 592 597 896 298 062 052 \
 102 802 109 413 013 284 730 114 659 547 932 692 707 302 311 965 775 647 246 619 271 296 338 955 788 \
 214 955 262 357 869 597 944 534 332 991 063 625  $q^{6189}$  +

11 484 783 947 768 513 015 315 452 542 820 326 227 579 511 894 813 882 581 646 326 915 231 413 200 \

086 685 423 064 545 282 956 594 302 393 436 077 384 836 927 715 625 296 806 478 993 779 663 767 012 \
 598 629 155 981 658 573 325 459 244 024 246 272  $q^{6192}$  -

11 887 840 985 458 016 214 468 752 864 554 880 310 446 764 413 338 968 057 968 191 498 912 718 153 \
 833 319 993 086 991 246 979 324 939 057 921 708 827 404 397 434 561 720 567 981 265 651 403 553 317 \
 451 780 734 950 072 954 032 142 206 301 339 648  $q^{6193}$  +

13 183 666 906 858 041 054 991 316 244 494 330 497 810 599 977 485 522 668 310 157 556 080 030 174 \
 511 175 168 610 014 709 400 316 426 211 715 002 151 930 012 654 575 908 198 493 362 982 219 812 582 \
 822 114 566 786 759 965 287 327 430 786 304 000  $q^{6196}$  -

13 646 194 432 704 491 765 125 453 861 644 432 820 664 316 400 654 397 378 471 871 918 311 238 394 \
 479 318 617 248 811 254 729 852 290 400 835 680 519 809 795 298 376 873 806 709 295 676 712 151 332 \
 367 963 340 624 458 465 300 194 633 868 289 362  $q^{6197}$  +

15 133 184 360 463 330 747 903 342 878 156 790 754 951 589 032 529 112 647 039 876 081 924 661 982 \
 794 603 888 708 829 567 076 625 395 653 163 014 115 445 941 630 124 334 352 427 323 088 977 506 008 \
 048 888 055 941 937 031 999 609 280 769 382 400  $q^{6200}$  -

15 663 933 696 830 128 035 892 659 760 373 573 639 392 044 628 795 068 344 390 863 809 120 159 864 \
 763 176 301 532 890 822 408 607 505 553 789 607 682 065 062 105 086 017 521 423 243 938 707 572 485 \
 528 269 298 203 466 901 739 675 709 972 480 000  $q^{6201}$  +

17 370 213 307 980 425 804 258 405 356 603 224 998 666 139 406 953 976 479 110 670 476 502 871 221 \
 444 208 307 514 603 887 910 032 726 927 527 448 642 064 599 908 284 745 308 776 093 975 106 028 457 \
 321 753 602 696 142 288 460 228 542 728 704 000  $q^{6204}$  -

17 979 220 127 997 820 417 246 441 225 197 015 845 820 041 305 771 427 017 904 486 363 885 157 104 \
 621 131 900 993 971 414 381 551 677 489 161 000 092 094 444 739 143 333 198 365 327 442 058 308 477 \
 190 648 057 287 941 591 569 476 490 954 387 950  $q^{6205}$  +

19 937 042 131 734 506 161 021 125 404 828 899 165 829 421 266 579 322 869 004 932 491 046 615 687 \
 197 163 635 505 237 563 022 943 393 476 365 602 988 786 863 711 869 028 571 670 046 089 284 314 073 \
 192 272 234 891 494 666 248 556 072 320 106 496  $q^{6208}$  -

20 635 814 448 117 211 732 179 422 097 593 825 609 497 312 129 164 473 171 161 281 546 558 714 091 \
 346 263 178 343 185 639 473 726 458 773 201 633 725 402 327 773 978 880 599 326 581 157 306 800 155 \
 506 658 765 039 629 321 490 109 285 466 112 000  $q^{6209}$  +

22 882 162 550 193 453 245 410 816 245 515 318 733 042 981 706 364 683 691 661 868 479 102 570 342 \
 827 186 732 294 192 563 302 924 925 802 757 532 586 369 868 878 979 689 476 216 655 905 494 454 753 \
 307 857 688 530 452 174 999 688 860 803 039 232  $q^{6212}$  -

23 683 896 146 288 116 527 267 624 146 070 082 973 584 821 804 613 744 880 084 596 341 736 477 069 \
 466 210 729 198 486 023 379 418 392 244 041 294 940 901 562 406 519 630 066 743 813 868 210 091 648 \
 716 284 813 018 964 152 724 382 036 181 550 600  $q^{6213}$  +

26 261 177 163 763 592 163 067 300 088 340 638 748 633 628 781 251 664 831 931 627 129 475 308 906 \
 564 919 281 691 988 981 295 027 123 644 737 164 864 179 313 348 130 376 909 714 677 371 666 676 745 \
 021 299 164 285 476 551 622 942 122 155 776 000  $q^{6216}$  -

27 181 002 462 098 690 353 995 751 469 983 662 060 298 737 203 079 948 418 206 536 459 849 120 067 \
 736 957 437 976 286 187 252 582 813 107 509 974 940 635 593 456 732 524 296 463 805 725 623 476 736 \
 704 658 440 555 201 449 246 467 879 265 763 328  $q^{6217}$  +

30 137 839 419 916 230 696 012 428 193 877 700 643 621 574 456 818 560 354 373 811 826 805 398 187 \
 139 567 650 895 128 527 316 284 872 363 506 544 409 215 889 009 414 629 761 040 518 975 596 073 826 \
 527 121 409 590 404 936 865 514 674 336 204 800  $q^{6220}$  -

31 193 104 363 641 420 003 163 420 444 504 286 723 917 103 177 103 782 024 378 930 760 395 101 171 \
 068 684 336 189 227 508 271 314 502 978 141 807 857 325 008 857 669 224 409 079 311 598 986 420 376 \
 608 086 827 485 802 385 037 453 644 718 868 375  $q^{6221}$  +

34 585 245 267 322 776 577 911 142 165 195 849 304 359 420 900 886 707 772 376 141 922 453 859 836 \
 285 695 855 962 129 264 363 421 544 894 361 292 398 037 466 495 809 483 740 636 147 648 953 492 608 \
 608 638 906 635 025 637 590 344 828 880 896 000  $q^{6224}$  -

35 795 839 454 047 405 386 034 731 335 293 449 103 639 651 580 031 040 618 402 862 863 607 982 873 \
 915 725 015 760 697 846 962 893 305 354 601 859 185 466 782 502 524 581 890 044 034 568 223 661 658 \
 449 189 537 236 041 399 459 966 274 029 977 600  $q^{6225}$  +

39 687 198 565 327 802 668 020 259 394 962 888 112 755 678 430 437 215 641 145 156 557 794 422 021 \
 479 010 209 984 383 622 025 592 566 034 690 122 754 214 539 850 843 803 130 557 480 602 283 244 355 \

096 907 626 434 734 464 185 280 222 091 806 720  $q^{6228}$  -  
 41 075 924 633 132 318 324 570 067 902 036 534 252 960 111 473 848 848 214 199 997 162 033 803 156 \\  
 284 307 714 074 082 721 411 472 688 769 918 021 941 058 778 931 332 823 236 983 563 096 193 892 668 \\  
 976 231 150 221 708 168 619 593 827 939 282 500  $q^{6229}$  +  
 45 539 775 516 544 046 287 600 004 483 594 591 810 165 911 370 599 947 155 185 080 699 686 536 276 \\  
 071 455 010 780 409 609 117 094 707 636 647 755 769 425 676 226 870 333 516 318 703 089 751 472 105 \\  
 186 409 488 409 012 260 600 801 513 726 071 808  $q^{6232}$  -  
 47 132 774 652 224 145 736 828 308 323 778 393 906 535 958 626 161 486 496 081 723 358 654 985 433 \\  
 611 347 435 908 275 806 965 895 140 129 451 041 179 490 644 300 376 867 226 058 430 746 619 631 365 \\  
 257 932 458 967 925 262 932 713 423 260 876 800  $q^{6233}$  +  
 52 253 117 055 048 423 366 970 464 655 557 110 941 091 353 531 787 913 895 040 476 561 139 175 582 \\  
 541 214 467 093 577 472 276 978 554 122 621 705 484 595 850 871 774 660 520 176 543 229 951 576 408 \\  
 769 872 244 819 725 325 057 160 406 514 944 000  $q^{6236}$  -  
 54 080 356 490 839 561 592 684 525 146 374 057 889 058 315 852 456 254 710 289 415 096 937 627 860 \\  
 941 591 643 125 984 489 982 347 311 657 181 670 699 937 001 032 515 956 522 764 117 743 775 065 369 \\  
 900 944 822 369 520 426 680 706 418 375 334 623  $q^{6237}$  +  
 59 953 482 317 444 752 377 897 180 584 034 667 217 918 231 722 079 784 734 176 778 902 787 889 131 \\  
 294 472 632 294 615 306 864 201 019 269 567 472 305 102 145 351 006 008 516 251 358 531 484 046 145 \\  
 353 450 414 520 432 818 701 435 468 332 236 800  $q^{6240}$  -  
 62 049 313 822 729 368 339 621 167 094 381 216 882 362 667 918 066 140 262 045 605 662 414 840 475 \\  
 886 370 967 945 494 283 979 310 391 914 731 326 374 431 169 360 248 161 704 509 368 455 589 015 837 \\  
 321 967 918 974 089 926 795 316 118 568 960 248  $q^{6241}$  +  
 68 785 601 125 409 786 514 077 374 707 191 249 163 022 127 030 089 153 826 794 972 776 028 644 840 \\  
 904 094 172 070 094 784 590 512 052 038 110 828 790 477 927 247 592 203 426 446 677 560 066 617 161 \\  
 861 625 328 676 864 942 164 449 361 313 792 000  $q^{6244}$  -  
 71 189 400 805 010 634 235 595 320 227 260 146 360 897 926 515 946 574 048 398 213 946 180 777 143 \\  
 726 577 440 101 275 698 727 864 144 786 648 611 473 153 457 222 031 840 051 510 527 281 344 569 326 \\  
 784 834 774 861 905 697 498 455 230 102 350 825  $q^{6245}$  +  
 78 915 368 903 729 994 149 101 678 138 283 084 738 695 961 943 685 056 106 118 711 395 517 599 164 \\  
 090 846 383 080 993 994 266 968 804 322 150 111 959 282 295 456 569 985 232 446 137 319 274 369 567 \\  
 740 631 320 316 576 960 728 628 795 574 469 632  $q^{6248}$  -  
 81 672 270 108 108 682 426 032 760 031 278 015 643 389 714 552 971 636 613 453 103 892 623 158 194 \\  
 217 391 896 518 914 094 347 926 751 041 243 341 856 748 852 337 722 796 142 363 358 092 060 631 388 \\  
 032 888 966 574 465 144 807 396 323 094 528 000  $q^{6249}$  +  
 90 532 933 747 324 719 557 883 533 164 112 371 610 290 558 396 445 104 892 503 090 630 129 384 505 \\  
 411 141 360 278 566 903 377 673 847 282 192 634 962 681 372 680 299 138 770 672 983 958 710 047 229 \\  
 165 540 980 467 195 599 194 426 138 180 512 768  $q^{6252}$  -  
 93 694 666 609 521 319 015 540 895 174 868 203 238 053 267 528 295 580 187 001 290 141 469 843 262 \\  
 054 120 180 944 857 695 929 704 189 743 059 959 370 918 794 395 660 162 609 550 683 032 722 060 523 \\  
 337 054 844 449 500 343 076 829 006 487 537 443  $q^{6253}$  +  
 103 856 232 548 780 921 396 380 286 977 723 670 591 081 469 119 009 485 115 456 529 123 105 322 907 \\  
 117 433 799 799 869 510 697 733 057 396 337 400 878 390 317 131 512 232 501 195 455 003 261 212 475 \\  
 364 063 211 184 037 765 411 458 836 049 920 000  $q^{6256}$  -  
 107 482 085 619 342 792 211 557 285 029 566 117 100 878 781 526 087 312 128 355 491 029 772 995 025 \\  
 223 005 481 403 153 425 088 192 694 156 978 812 965 213 176 521 391 342 989 438 124 540 288 264 265 \\  
 522 471 946 850 443 302 215 172 376 161 386 496  $q^{6257}$  +  
 119 135 041 335 389 323 935 167 908 893 886 404 747 246 917 276 700 673 541 686 102 942 373 672 956 \\  
 783 623 685 379 912 280 011 214 665 968 062 776 785 357 419 190 217 468 026 959 577 296 785 843 152 \\  
 479 333 072 269 597 126 627 856 101 505 331 200  $q^{6260}$  -  
 123 292 963 025 408 119 947 160 834 617 105 299 924 682 347 377 902 067 817 471 315 724 581 937 241 \\  
 119 821 191 544 942 531 472 374 103 211 271 911 246 222 404 853 382 132 324 408 148 917 418 112 899 \\  
 416 120 230 474 800 432 823 245 096 701 962 750  $q^{6261}$  +  
 136 655 614 391 273 025 347 957 393 347 908 304 010 703 514 291 025 345 314 694 362 420 426 414 863 \\  
 347 975 315 502 975 355 502 323 729 823 543 022 031 467 585 144 161 374 093 494 923 885 005 042 774 \\  
 480 940 016 322 862 353 228 870 330 919 424 000  $q^{6264}$  -

141 423 474 495 650 019 370 117 891 441 103 202 754 267 604 169 210 421 912 536 412 106 998 294 795  
 663 803 062 857 337 149 620 293 874 750 986 956 081 361 301 700 062 726 158 352 584 449 088 003 228  
 849 954 744 223 177 849 743 966 996 481 638 400  $q^{6265} +$   
 156 745 997 527 141 965 501 319 266 141 198 139 041 082 913 641 360 346 151 849 440 810 933 144 071  
 681 984 746 972 800 307 412 996 616 672 249 865 548 368 176 901 154 940 349 754 924 379 878 793 486  
 117 180 091 904 770 491 186 499 600 949 981 184  $q^{6268} -$   
 162 213 032 031 846 194 841 049 744 182 412 144 360 142 484 571 902 456 264 409 974 515 032 475 134  
 608 225 228 990 510 525 575 376 678 023 408 376 526 686 290 730 687 379 121 869 336 283 902 265 193  
 238 797 314 569 589 379 414 487 535 609 550 000  $q^{6269} +$   
 179 782 113 203 278 318 216 226 745 166 805 798 103 646 505 769 325 547 572 201 771 972 403 221 819  
 917 110 119 654 658 059 802 282 361 919 127 234 417 157 437 314 496 559 013 411 121 936 322 500 473  
 005 607 947 723 406 486 456 534 857 587 834 880  $q^{6272} -$   
 186 050 578 934 839 835 099 560 343 944 181 427 453 870 873 624 884 675 022 545 344 646 757 521 793  
 033 731 241 669 029 571 772 188 548 595 899 767 799 230 293 286 349 662 365 419 810 270 502 450 387  
 527 748 378 513 964 480 755 595 683 286 548 480  $q^{6273} +$   
 206 194 729 334 451 213 472 704 750 675 822 438 528 953 946 221 032 322 698 652 375 565 763 603 500  
 373 999 770 191 464 234 658 610 241 459 052 170 458 196 784 459 815 912 407 054 232 132 125 934 168  
 585 601 090 928 819 821 837 577 792 313 344 000  $q^{6276} -$   
 213 381 798 848 066 791 310 525 754 040 841 725 529 224 099 952 734 694 481 288 116 422 360 523 549  
 873 766 417 064 343 260 339 531 660 799 823 510 027 367 331 665 237 047 543 383 517 075 567 413 489  
 911 868 189 687 979 407 572 280 730 757 347 609  $q^{6277} +$   
 236 477 439 764 594 302 756 973 334 132 771 533 794 075 589 039 396 905 082 918 091 324 823 992 986  
 310 556 455 733 754 184 013 578 306 463 212 117 814 933 687 112 346 816 020 090 448 372 174 418 394  
 291 752 305 976 845 268 865 075 917 872 768 000  $q^{6280} -$   
 244 717 371 258 565 355 062 252 802 421 092 100 404 419 349 762 433 722 660 138 607 142 428 280 296  
 241 364 205 050 002 592 301 101 639 907 706 798 370 661 083 813 442 219 258 791 094 121 655 215 215  
 242 684 658 886 691 414 392 098 523 459 584 000  $q^{6281} +$   
 271 195 802 887 002 349 930 126 775 106 502 898 378 789 924 773 419 787 587 042 207 252 671 627 956  
 764 533 155 276 440 940 135 591 260 421 880 247 398 928 408 497 028 772 477 285 574 354 737 326 874  
 559 189 455 690 362 800 887 152 758 184 000 000  $q^{6284} -$   
 280 642 424 955 299 438 778 488 122 661 461 014 351 782 321 410 282 337 300 921 467 036 111 450 186  
 014 612 329 747 286 677 021 751 732 693 387 713 720 930 591 290 641 666 663 818 993 312 229 543 609  
 529 740 284 352 394 660 975 349 906 612 970 675  $q^{6285} +$   
 310 997 806 037 239 051 969 478 334 770 893 449 672 429 143 966 896 694 608 410 690 272 358 677 759  
 893 177 511 399 498 558 532 109 831 111 995 305 305 729 038 087 193 728 117 079 785 485 366 381 851  
 875 195 208 800 631 849 927 905 857 978 892 288  $q^{6288} -$   
 321 827 362 819 720 678 624 809 566 001 309 560 630 584 538 998 347 870 738 123 326 106 492 778 811  
 611 912 603 329 432 264 877 917 003 064 573 287 843 718 419 366 890 641 637 727 919 083 096 999 366  
 841 413 392 751 037 325 347 170 840 932 352 000  $q^{6289} +$   
 356 625 847 483 607 482 788 957 949 567 004 822 669 042 562 981 582 779 541 472 690 318 893 293 540  
 887 652 458 828 574 769 249 402 440 212 787 135 098 431 926 342 004 910 922 147 582 110 864 887 807  
 544 234 580 332 786 445 189 025 740 041 107 456  $q^{6292} -$   
 369 040 256 348 771 291 248 773 202 615 711 234 012 262 798 804 408 382 405 108 770 255 669 237 316  
 492 056 832 630 250 584 061 992 530 667 491 458 921 702 401 165 580 275 506 652 537 372 530 875 975  
 694 666 009 548 731 127 453 617 109 727 150 565  $q^{6293} +$   
 408 930 455 521 471 201 225 841 625 100 464 280 886 222 773 726 895 106 869 452 134 388 981 223 366  
 178 153 320 110 325 143 165 641 265 943 555 000 584 144 577 360 158 090 324 020 766 865 982 153 103  
 692 233 548 537 344 274 314 803 140 446 528 000  $q^{6296} -$   
 423 161 036 938 436 504 987 076 119 972 396 997 941 713 539 361 525 301 029 612 303 718 672 140 100  
 835 533 509 379 055 777 674 144 398 713 925 005 130 551 715 346 809 352 940 666 712 835 713 833 599  
 702 423 751 148 217 828 821 854 416 913 989 632  $q^{6297} +$   
 468 885 995 843 165 666 536 769 634 017 437 575 525 253 702 403 544 760 683 164 503 586 164 858 358  
 731 459 760 783 034 204 930 577 547 430 917 315 117 110 261 252 701 094 922 327 627 595 222 503 475  
 328 543 855 377 477 057 296 549 671 183 104 000  $q^{6300} -$   
 485 197 743 703 753 767 681 048 379 649 837 405 859 700 922 738 575 516 902 555 093 263 845 277 179

869 875 752 188 327 519 391 028 489 471 026 295 514 654 483 654 431 821 895 278 528 432 488 559 496  
 887 777 554 796 962 892 564 262 313 605 145 000  $q^{6301} +$   
 537 608 654 576 582 982 924 082 606 654 588 592 789 234 619 016 375 226 297 424 503 339 400 879 358  
 495 200 852 702 574 025 203 605 775 471 672 535 500 625 499 211 044 547 276 311 423 687 818 663 062  
 099 017 299 144 277 974 652 148 534 553 088 000  $q^{6304} -$   
 556 305 125 070 207 516 240 562 713 663 511 373 205 511 577 168 510 369 104 290 087 011 233 384 379  
 846 116 966 359 519 217 112 593 316 972 652 513 882 914 890 147 790 533 007 077 398 752 792 660 015  
 521 216 555 219 121 002 752 528 939 712 512 000  $q^{6305} +$   
 616 377 025 816 496 679 541 660 431 780 232 468 127 982 847 350 146 618 363 734 881 832 948 252 515  
 542 223 147 657 791 177 978 175 053 182 120 919 567 704 997 616 211 043 208 005 750 623 066 779 999  
 809 243 773 593 885 080 784 964 986 461 011 968  $q^{6308} -$   
 637 805 934 217 664 825 311 456 774 173 870 924 420 348 203 868 867 644 859 486 330 091 971 341 743  
 121 041 483 845 265 435 244 602 834 230 753 276 239 966 074 438 252 905 836 099 556 603 208 190 478  
 758 653 053 013 374 126 589 299 735 338 266 500  $q^{6309} +$   
 706 655 679 860 627 495 675 222 792 170 685 727 023 926 551 817 945 102 147 344 746 906 357 461 639  
 345 496 265 166 324 224 663 331 166 592 924 698 802 563 680 986 808 766 428 566 565 200 431 868 460  
 814 923 639 913 518 770 363 524 991 739 625 472  $q^{6312} -$   
 731 215 307 464 156 142 406 495 003 985 028 464 581 630 343 771 742 212 084 531 031 347 357 811 481  
 482 136 431 055 297 500 986 589 974 566 191 214 813 662 628 310 451 534 342 127 126 330 539 210 357  
 177 805 490 315 106 464 231 504 702 895 456 256  $q^{6313} +$   
 810 122 142 561 562 774 492 853 501 795 064 549 266 329 123 495 251 904 837 595 394 948 578 438 718  
 639 249 315 277 625 734 912 489 277 323 301 595 337 883 526 902 750 637 849 431 352 174 917 838 467  
 169 247 852 128 622 056 828 103 896 133 440 000  $q^{6316} -$   
 838 268 670 726 136 312 533 930 189 281 905 426 797 254 693 227 330 677 419 507 730 573 768 492 668  
 222 175 157 300 189 610 083 958 780 731 102 232 351 241 836 447 780 280 905 657 592 529 232 760 011  
 330 131 553 098 861 960 737 885 146 299 024 896  $q^{6317} +$   
 928 697 778 192 330 360 523 212 660 714 239 086 550 715 993 525 397 550 066 473 167 035 171 852 623  
 427 060 168 682 676 515 671 027 270 184 657 232 089 413 642 716 737 326 753 546 262 887 073 022 452  
 931 420 307 927 582 167 272 225 449 231 155 200  $q^{6320} -$   
 960 953 683 293 948 328 297 891 716 805 800 140 040 469 176 905 617 737 082 483 538 123 063 801 314  
 020 691 076 452 748 660 368 317 402 406 481 013 096 286 607 637 247 153 920 938 396 027 471 688 376  
 775 074 104 616 485 740 890 812 862 894 080 000  $q^{6321} +$   
 1 064 583 139 113 691 739 833 895 471 224 737 409 815 508 610 400 337 061 181 493 368 469 725 292 445  
 848 509 099 743 248 037 201 542 071 200 443 605 940 678 810 471 696 955 558 612 285 747 376 485 302  
 673 315 353 754 253 036 264 182 523 474 944 000  $q^{6324} -$   
 1 101 546 801 469 960 666 689 749 179 342 036 695 759 007 588 367 685 171 875 118 529 186 212 641 899  
 694 593 113 088 469 319 871 945 929 565 127 566 541 892 805 060 891 582 384 908 364 279 446 021 457  
 285 882 983 897 290 532 438 532 228 610 486 625  $q^{6325} +$   
 1 220 298 426 600 563 472 441 036 905 716 795 105 271 471 865 041 101 386 934 576 885 540 673 739 379  
 800 331 450 849 891 681 145 452 111 712 088 439 361 240 544 245 556 655 424 983 584 628 737 910 204  
 921 368 606 403 963 398 939 633 600 479 760 384  $q^{6328} -$   
 1 262 655 128 451 073 844 413 799 963 062 480 686 815 130 118 530 009 075 542 413 710 427 898 345 350  
 574 345 073 722 749 914 288 364 269 332 096 087 977 707 372 197 326 417 906 636 158 515 307 894 124  
 717 061 785 681 621 755 117 344 477 626 368 000  $q^{6329} +$   
 1 398 729 799 891 149 189 656 843 160 770 999 825 173 635 612 893 719 156 861 467 133 676 642 115 471  
 984 109 028 671 106 531 395 870 150 808 377 711 089 832 015 117 852 392 555 176 724 840 016 136 108  
 804 519 854 598 970 195 927 580 856 470 069 248  $q^{6332} -$   
 1 447 264 312 704 224 229 777 079 219 995 462 332 522 307 953 942 414 096 939 586 523 803 637 374 325  
 790 949 137 241 988 049 057 137 948 731 426 729 265 696 769 681 678 743 364 363 832 132 467 642 622  
 519 945 030 142 871 307 060 629 913 587 129 341  $q^{6333} +$   
 1 603 182 376 531 328 726 285 512 165 876 186 417 505 034 727 182 715 730 685 494 608 963 024 252 609  
 915 860 766 178 962 801 067 180 060 550 452 001 020 113 753 718 973 402 683 811 259 208 838 207 896  
 120 089 607 920 291 062 253 351 905 767 424 000  $q^{6336} -$   
 1 658 793 366 705 648 207 205 254 825 457 053 658 116 967 943 130 621 106 357 266 957 709 858 676 404  
 451 321 420 825 806 705 039 489 875 051 462 678 616 125 757 125 358 304 104 928 488 321 072 662 673

548 664 034 821 744 417 345 816 782 697 758 720  $q^{6337} +$   
 1 837 440 888 302 443 453 482 909 538 557 138 658 913 569 448 809 253 074 596 337 701 131 988 703 757  
 630 641 954 803 649 195 796 394 835 606 628 763 016 769 821 101 153 206 555 193 802 301 983 113 849  
 616 754 022 819 874 865 908 138 984 319 385 600  $q^{6340} -$   
 1 901 157 403 260 429 285 030 584 083 317 397 906 665 779 950 662 906 360 462 108 711 689 794 035 193  
 195 754 745 748 369 782 443 988 508 798 215 543 405 421 926 784 177 971 573 647 764 608 176 170 049  
 532 430 341 752 072 641 258 335 606 543 177 375  $q^{6341} +$   
 2 105 839 095 618 425 189 112 383 638 984 608 812 992 997 609 570 574 607 820 665 972 834 319 272 614  
 139 568 205 144 190 056 834 471 171 828 642 911 615 152 402 517 042 681 843 969 984 713 792 596 004  
 270 232 767 214 517 663 490 160 970 562 944 000  $q^{6344} -$   
 2 178 839 429 937 602 522 861 780 756 309 158 403 527 292 949 868 800 424 976 097 159 248 052 909 023  
 324 379 001 097 682 459 800 099 720 622 352 657 413 597 911 854 843 651 310 872 487 834 450 135 099  
 759 757 248 351 185 185 427 044 476 760 883 200  $q^{6345} +$   
 2 413 339 221 744 265 295 372 312 895 707 724 185 130 736 208 389 865 408 986 662 606 582 149 242 601  
 253 754 406 891 559 616 445 425 400 046 412 014 993 446 735 490 001 799 431 231 801 573 666 322 241  
 694 912 946 892 127 004 933 418 674 448 920 064  $q^{6348} -$   
 2 496 972 506 018 141 474 609 137 643 538 773 043 519 290 274 111 971 269 982 818 369 996 754 108 780  
 891 077 552 981 731 948 380 113 349 696 616 701 760 207 224 258 596 341 184 554 058 301 304 712 008  
 077 081 948 188 179 661 498 532 141 684 961 750  $q^{6349} +$   
 2 765 622 849 362 753 386 483 604 708 718 193 524 191 181 043 861 520 832 143 054 151 153 785 897 375  
 380 584 910 712 705 199 020 881 458 202 559 183 064 275 990 548 138 400 634 480 283 107 009 605 456  
 670 790 332 515 480 341 481 055 606 203 498 496  $q^{6352} -$   
 2 861 433 753 695 419 154 655 387 809 930 340 538 303 519 269 350 372 867 685 208 769 549 844 245 630  
 509 368 758 620 026 270 924 790 466 846 817 601 725 665 981 801 087 436 510 296 517 598 397 727 816  
 659 090 219 990 356 237 646 423 646 610 980 864  $q^{6353} +$   
 3 169 194 929 145 942 687 178 133 007 920 873 184 756 090 689 635 587 462 923 135 423 295 736 272 693  
 404 702 089 918 141 303 229 097 528 412 035 722 513 678 672 622 649 812 717 057 740 392 433 588 473  
 962 545 644 215 733 975 345 300 721 324 544 000  $q^{6356} -$   
 3 278 951 929 445 895 360 568 170 781 049 694 288 968 396 092 807 246 309 091 163 992 214 602 495 747  
 949 971 606 877 042 556 744 289 158 787 340 373 792 256 302 420 922 678 140 160 242 389 590 855 895  
 741 194 067 814 652 584 146 434 233 093 176 075  $q^{6357} +$   
 3 631 502 786 780 311 029 620 514 781 029 316 398 161 702 160 816 175 766 458 676 487 272 230 906 200  
 171 786 213 125 665 068 150 281 411 881 233 786 371 151 554 662 679 009 477 226 513 027 054 761 099  
 558 144 520 365 918 085 372 789 826 866 790 400  $q^{6360} -$   
 3 757 230 506 335 832 058 057 331 229 311 287 037 165 324 487 829 570 263 421 898 517 824 761 146 503  
 388 927 391 947 498 380 017 793 457 623 019 652 198 785 540 334 013 470 321 491 260 933 745 659 235  
 381 568 968 331 588 528 626 419 651 596 288 000  $q^{6361} +$   
 4 161 072 285 586 932 135 003 533 005 288 977 996 607 291 760 930 760 792 867 302 343 483 451 000 307  
 305 301 764 207 431 437 760 976 196 621 298 004 626 956 547 960 015 713 882 888 068 897 218 565 209  
 983 620 231 508 060 082 491 017 938 617 088 000  $q^{6364} -$   
 4 305 088 497 928 084 644 401 170 382 005 774 710 465 858 373 837 695 610 154 208 606 556 968 083 228  
 302 676 199 597 330 549 836 238 474 028 491 552 176 023 815 218 614 822 018 028 909 858 107 812 226  
 352 335 410 105 071 928 140 784 701 860 750 275  $q^{6365} +$   
 4 767 663 611 310 569 934 780 782 885 620 716 435 087 627 897 429 901 787 036 751 877 136 908 419 295  
 411 166 914 061 155 514 963 653 858 466 947 200 845 762 246 899 184 012 995 345 604 968 122 836 092  
 775 394 251 806 888 124 201 757 808 729 448 448  $q^{6368} -$   
 4 932 621 574 405 722 866 091 498 024 728 983 435 691 757 851 193 755 605 031 000 322 291 339 991 311  
 166 269 797 565 587 313 348 547 315 880 055 263 726 385 130 041 727 286 164 688 751 970 246 523 262  
 831 415 779 366 621 118 296 849 355 448 320 000  $q^{6369} +$   
 5 462 449 499 354 204 014 280 345 112 984 092 020 180 206 896 336 438 846 765 356 227 246 315 493 716  
 708 845 493 217 416 538 628 528 394 551 668 114 256 894 416 635 368 452 304 531 239 388 885 440 057  
 080 642 534 061 911 126 325 349 582 926 184 448  $q^{6372} -$   
 5 651 386 387 253 264 864 176 450 250 687 493 281 673 954 717 288 199 720 927 380 726 987 825 051 104  
 979 764 997 172 630 237 986 586 348 248 686 679 911 618 372 477 008 317 198 346 710 432 117 630 106  
 836 074 072 720 247 468 271 006 150 347 140 010  $q^{6373} +$

6 258 219 129 025 066 790 473 745 559 239 952 854 782 382 641 881 158 400 375 645 565 939 656 779 292 \
 727 443 385 416 755 898 756 724 603 440 591 447 511 752 580 248 867 452 107 080 929 577 123 139 448 \
 414 753 530 734 360 663 969 688 122 643 392 000  $q^{6376}$  -

6 474 611 436 862 332 691 342 768 535 045 386 905 529 616 927 127 761 262 087 426 493 673 284 635 697 \
 330 788 795 986 764 767 280 186 203 536 051 080 558 891 122 118 489 636 421 071 867 550 562 115 783 \
 224 619 580 647 535 991 194 724 893 508 501 504  $q^{6377}$  +

7 169 611 371 450 817 250 729 936 390 634 483 223 338 147 731 515 771 500 328 839 858 042 305 734 986 \
 411 806 509 762 057 806 917 057 367 095 603 295 981 456 266 934 966 160 213 296 380 788 848 059 412 \
 024 277 867 013 633 700 176 562 329 504 563 200  $q^{6380}$  -

7 417 438 295 216 579 519 366 356 616 983 882 873 476 497 910 959 309 808 140 616 108 348 155 103 996 \
 232 327 206 416 165 018 013 557 781 042 825 418 578 158 258 143 434 739 486 440 113 634 272 110 321 \
 301 752 895 952 419 521 587 315 338 076 976 875  $q^{6381}$  +

8 213 381 605 962 610 085 610 087 932 849 303 087 695 736 798 610 912 497 401 754 075 944 960 816 282 \
 801 987 146 844 837 626 558 705 295 313 433 802 099 870 872 209 818 255 315 666 659 465 340 752 203 \
 712 746 992 744 695 531 292 725 656 199 168 000  $q^{6384}$  -

8 497 197 541 882 074 192 876 819 422 524 364 250 246 814 755 212 314 855 164 314 180 233 840 190 642 \
 066 268 864 349 361 240 224 787 328 978 217 543 065 618 307 582 301 523 278 811 494 804 645 874 831 \
 069 896 529 713 762 761 637 985 351 018 086 400  $q^{6385}$  +

9 408 706 923 340 459 404 327 914 626 937 134 416 011 489 405 549 154 973 375 025 446 066 123 605 871 \
 289 428 795 875 094 726 195 527 863 407 133 702 447 215 433 409 802 363 189 164 883 643 551 240 908 \
 792 736 578 730 525 982 426 321 415 777 957 888  $q^{6388}$  -

9 733 724 395 617 065 674 377 473 936 004 013 607 068 330 081 782 620 825 155 251 592 683 434 165 315 \
 542 557 606 305 438 795 821 876 306 834 601 176 980 528 145 707 497 692 277 247 938 357 588 589 016 \
 741 552 507 082 049 997 236 499 971 891 308 250  $q^{6389}$  +

10 777 535 224 128 949 351 237 661 509 719 341 727 685 486 187 248 611 064 868 481 324 065 108 647 \
 115 883 001 340 833 409 237 239 111 689 847 518 930 986 938 325 808 218 380 682 286 543 457 301 112 \
 751 597 486 853 401 898 960 332 682 966 482 722 816  $q^{6392}$  -

11 149 719 737 136 012 657 417 314 267 597 426 174 519 720 856 569 417 867 289 149 528 978 044 852 \
 234 358 802 367 411 708 063 003 280 150 342 860 714 291 315 719 093 580 109 548 665 014 211 551 380 \
 182 799 788 689 870 063 021 395 578 918 541 688 832  $q^{6393}$  +

12 344 984 508 539 924 233 816 442 810 252 368 668 142 208 179 102 287 656 246 531 448 517 792 714 \
 907 841 862 602 913 480 281 973 455 994 094 557 067 200 699 733 511 859 735 779 144 192 162 570 640 \
 789 484 092 033 716 560 613 035 016 766 092 288 000  $q^{6396}$  -

12 771 163 033 613 694 369 579 458 413 931 897 882 956 929 728 069 200 284 303 747 176 445 206 609 \
 550 597 050 215 387 805 753 510 075 119 549 923 004 558 759 397 471 729 517 428 665 132 082 757 576 \
 334 383 965 574 821 893 039 844 144 363 511 307 257  $q^{6397}$  +

14 139 799 555 290 285 154 883 845 259 460 163 674 540 491 763 421 270 608 583 576 445 420 196 773 \
 961 000 253 582 362 143 535 328 870 281 033 693 974 696 579 392 728 420 663 577 416 548 106 317 067 \
 477 637 810 446 965 395 290 278 539 408 944 332 800  $q^{6400}$  -

14 627 784 606 896 725 585 125 222 831 377 283 882 464 721 710 790 839 387 470 588 361 672 526 362 \
 145 410 473 820 348 987 370 818 625 443 885 963 887 443 023 394 361 255 730 693 359 124 779 254 091 \
 448 493 205 649 706 665 729 129 334 108 364 800 000  $q^{6401}$  +

16 194 874 216 096 786 155 204 372 911 592 007 964 563 489 803 352 150 177 326 900 528 178 786 739 \
 831 083 244 201 899 608 237 978 476 042 811 579 597 935 622 115 936 360 573 023 364 920 084 806 840 \
 792 976 360 216 460 864 201 941 913 518 993 408 000  $q^{6404}$  -

16 753 605 751 661 965 470 415 736 595 385 560 143 785 524 728 692 970 672 149 226 010 476 633 109 \
 885 419 768 185 866 151 881 881 453 375 715 836 632 592 623 957 460 418 861 982 184 830 866 022 365 \
 891 332 706 517 866 912 972 604 591 074 569 726 750  $q^{6405}$  +

18 547 848 728 759 740 064 864 751 145 062 826 691 181 468 015 503 618 557 012 338 234 892 759 758 \
 952 893 911 657 745 610 491 848 172 814 726 106 931 703 912 986 844 617 003 565 057 696 901 624 854 \
 490 120 734 180 336 377 885 521 214 065 358 311 424  $q^{6408}$  -

19 187 556 425 835 428 665 549 598 383 579 959 382 560 885 983 991 045 903 321 204 689 961 794 729 \
 839 441 714 564 993 981 926 840 687 503 571 266 268 775 592 114 467 114 654 081 201 250 627 941 148 \
 256 121 411 145 558 825 060 236 113 385 439 232 000  $q^{6409}$  +

21 241 792 795 704 546 294 189 820 534 990 695 395 268 835 754 873 800 742 080 447 898 064 282 603 \

669 923 211 621 513 608 123 219 456 861 417 326 268 920 979 261 729 701 254 986 589 236 482 710 099 \
 334 096 305 518 060 958 923 383 091 129 167 838 208  $q^{6412}$  -

21 974 181 625 056 831 096 446 782 710 294 115 574 698 861 465 062 364 245 092 572 438 436 904 442 \
 335 538 899 729 026 852 248 800 185 290 564 348 585 635 243 435 642 758 887 154 084 195 911 344 118 \
 267 263 430 413 895 291 179 328 620 097 336 943 604  $q^{6413}$  +

24 325 986 710 369 060 455 132 850 153 294 102 671 092 370 810 339 038 486 342 238 044 338 662 492 \
 765 101 104 935 464 583 108 903 782 940 799 197 893 791 599 530 385 026 515 767 900 831 240 037 469 \
 553 189 629 653 899 945 507 525 065 722 019 840 000  $q^{6416}$  -

25 164 449 140 503 422 753 681 593 552 897 535 383 812 867 137 208 429 203 783 126 773 346 422 976 \
 165 900 727 642 652 152 401 314 422 200 684 486 610 419 936 652 793 340 972 002 044 904 932 165 052 \
 500 891 319 762 742 650 138 931 401 880 255 397 888  $q^{6417}$  +

27 856 814 568 165 090 971 496 236 459 662 296 592 212 930 146 073 939 618 175 231 765 606 752 038 \
 432 641 654 296 933 744 066 240 497 919 914 278 939 475 800 457 963 789 122 501 881 696 053 761 480 \
 930 464 649 279 409 802 527 762 388 374 394 470 400  $q^{6420}$  -

28 816 673 213 129 628 934 223 164 418 622 768 204 640 164 425 690 838 567 778 449 640 248 855 386 \
 279 385 271 925 830 216 536 850 550 904 449 534 838 486 779 239 807 998 819 869 344 175 048 733 547 \
 547 454 893 932 843 313 711 932 824 318 458 579 250  $q^{6421}$  +

31 898 785 603 005 479 842 977 635 990 531 551 220 425 641 678 354 375 099 447 457 020 810 769 498 \
 424 336 570 464 542 886 973 222 350 092 239 940 961 238 327 913 031 081 991 529 948 884 118 236 814 \
 506 511 908 758 424 005 868 440 105 388 092 032 000  $q^{6424}$  -

32 997 570 669 486 188 692 616 803 400 276 401 007 816 616 351 058 575 042 505 760 343 148 777 615 \
 128 642 129 223 612 872 961 000 241 324 903 360 300 589 919 245 775 824 660 411 279 961 217 135 702 \
 083 297 686 732 569 898 243 274 009 571 180 544 000  $q^{6425}$  +

36 525 701 980 085 075 380 542 914 002 913 679 686 801 812 275 797 245 101 659 298 987 971 415 867 \
 211 850 028 338 375 618 788 685 863 933 666 387 025 525 555 811 469 052 863 363 377 121 364 912 316 \
 235 223 108 032 511 999 413 999 139 456 208 967 680  $q^{6428}$  -

37 783 468 491 461 139 646 580 919 957 571 989 526 872 538 507 916 313 545 388 327 751 622 594 925 \
 786 822 411 989 161 140 001 430 541 688 851 877 557 397 066 702 720 408 627 398 973 914 305 621 109 \
 937 501 374 261 288 775 505 334 964 863 851 393 250  $q^{6429}$  +

41 821 993 991 277 622 553 718 696 102 403 332 166 125 482 749 180 940 361 416 958 795 191 355 378 \
 137 345 624 120 698 083 618 806 560 441 878 457 825 958 089 322 710 745 140 711 477 762 925 602 091 \
 514 574 146 990 457 842 365 914 738 161 813 700 608  $q^{6432}$  -

43 261 684 476 443 892 782 671 938 479 689 044 514 824 788 579 627 859 955 537 786 671 922 565 981 \
 109 575 622 889 947 219 371 495 574 167 292 705 593 497 102 934 526 897 860 403 076 408 979 199 993 \
 708 996 281 439 272 836 065 392 571 968 355 237 888  $q^{6433}$  +

47 884 246 587 448 092 119 157 918 146 518 006 573 542 249 584 185 737 620 085 567 015 872 988 012 \
 490 295 936 150 887 700 623 960 798 571 600 645 798 462 356 029 820 550 652 211 549 337 409 857 862 \
 387 377 410 762 626 976 255 490 853 981 222 912 000  $q^{6436}$  -

49 532 105 733 398 207 664 278 287 668 413 507 564 392 185 315 024 402 801 037 311 668 112 782 282 \
 881 550 192 799 685 529 986 854 328 893 218 833 391 892 645 554 217 824 690 323 949 549 374 395 005 \
 041 912 650 510 375 170 390 076 016 084 528 524 558  $q^{6437}$  +

54 822 944 595 023 457 395 652 935 405 557 072 303 247 422 086 107 286 841 051 757 895 060 207 050 \
 658 525 465 353 678 947 572 048 047 539 093 569 788 284 601 751 548 280 698 560 817 321 576 164 185 \
 282 858 212 359 920 557 863 061 208 163 023 052 800  $q^{6440}$  -

56 708 993 288 761 034 072 315 761 517 866 278 749 614 533 606 442 300 635 788 043 782 880 653 551 \
 504 123 482 973 924 374 458 346 935 565 318 795 238 072 017 542 764 993 362 836 068 639 204 560 056 \
 728 343 113 964 306 952 602 808 403 071 401 984 000  $q^{6441}$  +

62 764 467 862 637 883 838 434 791 000 593 016 391 325 786 697 894 067 878 545 145 744 274 527 897 \
 995 695 492 830 993 139 483 090 267 284 240 666 944 962 007 473 040 585 360 377 805 682 640 597 203 \
 127 692 025 639 320 882 498 709 107 127 619 776 000  $q^{6444}$  -

64 923 045 106 315 306 735 816 871 383 869 403 502 724 159 458 525 421 899 168 041 727 502 662 554 \
 590 792 643 093 788 829 808 504 420 782 783 996 306 201 441 647 889 264 064 197 147 850 821 971 906 \
 064 981 100 909 860 122 159 560 008 266 486 455 250  $q^{6445}$  +

71 853 372 036 431 870 918 584 010 860 713 261 391 902 325 674 667 505 308 457 839 092 817 134 542 \
 623 756 480 602 993 806 553 510 205 145 205 849 277 515 268 152 741 948 630 857 584 783 664 019 795

150 691 077 042 208 514 408 646 921 319 987 077 120  $q^{6448}$  -  
 74 323 754 428 393 494 963 933 017 142 181 539 880 897 110 312 520 071 017 687 278 341 099 157 824 \ \backslash  
 556 368 717 351 164 403 822 286 927 932 981 362 297 013 194 119 993 372 109 959 686 181 305 045 609 \ \backslash  
 503 798 852 734 333 738 396 027 638 561 718 272 000  $q^{6449}$  +  
 82 254 995 748 243 095 721 618 941 191 857 271 053 850 069 415 151 483 528 410 596 879 614 409 175 \ \backslash  
 766 030 528 368 760 694 827 339 607 743 928 487 748 290 800 958 070 660 647 321 083 649 593 605 942 \ \backslash  
 274 613 394 267 388 052 647 000 899 294 219 429 888  $q^{6452}$  -  
 85 082 105 603 202 450 268 620 327 765 487 080 890 896 394 322 105 596 114 547 805 412 525 182 791 \ \backslash  
 351 502 602 664 403 758 228 985 255 203 033 112 686 296 736 049 386 592 198 290 548 675 581 265 976 \ \backslash  
 056 480 909 501 235 795 098 532 926 693 109 777 401  $q^{6453}$  +  
 94 158 440 809 201 317 403 558 719 819 969 175 386 322 008 732 698 922 981 707 151 781 446 940 829 \ \backslash  
 559 411 073 980 516 275 189 138 730 325 361 270 665 555 182 851 798 958 021 213 365 759 456 747 774 \ \backslash  
 602 278 627 619 937 599 425 140 046 727 744 896 000  $q^{6456}$  -  
 97 393 655 567 456 996 011 110 252 810 081 606 890 787 571 578 149 113 475 654 212 957 578 153 692 \ \backslash  
 924 875 307 582 816 849 077 984 760 235 214 992 504 335 283 079 615 261 309 407 177 395 390 419 435 \ \backslash  
 985 301 150 321 100 322 664 942 786 933 241 577 472  $q^{6457}$  +  
 107 779 978 634 538 612 846 544 520 177 963 595 324 042 375 672 124 430 387 027 676 286 304 012 156 \ \backslash  
 737 681 047 147 311 727 908 692 661 347 571 109 469 085 226 121 439 733 193 532 405 320 815 773 096 \ \backslash  
 766 583 193 150 289 391 333 836 097 893 178 675 200  $q^{6460}$  -  
 111 482 056 010 719 472 269 457 415 458 644 939 896 543 704 197 859 735 942 419 127 872 364 169 505 \ \backslash  
 281 445 370 707 577 328 920 746 725 519 957 054 262 837 543 793 395 494 874 715 086 724 566 632 775 \ \backslash  
 899 251 853 253 472 878 951 482 922 482 108 057 750  $q^{6461}$  +  
 123 366 943 700 632 533 578 811 223 558 616 967 611 578 199 134 465 193 182 749 131 394 236 095 017 \ \backslash  
 926 283 469 376 498 102 703 948 682 887 440 464 485 061 864 704 511 769 328 861 293 892 571 787 684 \ \backslash  
 585 576 432 467 698 620 517 268 343 572 905 984 000  $q^{6464}$  -  
 127 603 079 078 675 286 583 684 992 380 676 877 857 113 796 533 218 385 809 838 326 023 515 994 913 \ \backslash  
 671 948 765 182 491 518 607 258 790 764 612 379 134 181 739 732 098 152 435 441 932 303 785 469 188 \ \backslash  
 663 132 925 298 009 526 190 272 182 109 061 120 000  $q^{6465}$  +  
 141 202 183 485 812 529 045 999 029 888 306 600 751 579 470 118 359 778 794 026 295 074 235 879 555 \ \backslash  
 247 173 111 100 358 749 557 859 197 510 320 785 407 366 224 818 858 900 013 366 859 236 470 207 495 \ \backslash  
 865 605 683 100 362 856 378 387 025 237 116 567 552  $q^{6468}$  -  
 146 049 218 414 910 078 754 827 501 158 883 602 031 175 755 946 371 270 872 143 997 951 231 901 290 \ \backslash  
 331 121 550 368 446 113 812 421 369 562 424 108 719 205 557 985 016 044 181 776 747 568 916 917 750 \ \backslash  
 339 354 256 381 402 391 694 232 008 024 931 601 500  $q^{6469}$  +  
 161 609 144 224 521 782 736 441 902 408 881 869 368 686 914 165 774 475 366 812 595 349 503 750 212 \ \backslash  
 827 726 013 209 071 492 610 579 357 573 476 660 812 313 317 645 913 750 682 731 269 924 837 503 141 \ \backslash  
 530 057 179 080 481 781 650 996 734 797 901 097 984  $q^{6472}$  -  
 167 154 947 551 946 971 698 824 122 499 282 951 545 086 890 713 501 071 984 933 947 274 508 543 969 \ \backslash  
 167 886 089 993 339 854 147 676 099 293 830 717 023 567 701 749 807 253 029 284 552 873 087 505 261 \ \backslash  
 149 386 559 116 596 359 954 506 831 662 464 172 032  $q^{6473}$  +  
 184 957 683 083 778 509 396 448 358 355 224 350 155 598 987 286 018 018 439 665 637 102 522 425 750 \ \backslash  
 825 017 870 186 244 666 524 344 148 366 686 219 918 580 846 424 605 042 676 113 626 009 776 542 084 \ \backslash  
 142 985 979 770 580 406 550 263 541 109 117 888 000  $q^{6476}$  -  
 191 302 729 321 925 659 518 873 549 238 826 104 842 747 197 404 256 536 835 443 452 408 194 633 435 \ \backslash  
 785 842 041 177 767 534 703 333 574 948 156 665 604 211 380 794 008 762 400 303 436 227 354 003 624 \ \backslash  
 402 130 148 666 614 143 910 848 620 269 659 639 949  $q^{6477}$  +  
 211 670 710 249 790 185 925 626 212 841 576 973 735 162 726 824 343 509 706 586 402 842 370 986 161 \ \backslash  
 946 036 659 329 176 168 629 447 665 779 106 788 584 268 059 601 543 196 986 076 794 686 173 640 670 \ \backslash  
 141 610 807 306 865 940 759 108 523 005 527 572 480  $q^{6480}$  -  
 218 929 883 270 279 503 227 788 948 053 729 734 469 303 448 535 356 589 684 192 264 170 659 575 404 \ \backslash  
 183 126 415 805 414 652 296 108 079 616 608 660 739 507 129 364 552 999 630 300 228 323 820 581 350 \ \backslash  
 784 339 913 955 670 969 998 111 023 060 672 512 000  $q^{6481}$  +  
 242 231 779 117 288 206 606 085 284 399 698 548 317 029 515 983 258 749 638 010 261 223 679 947 707 \ \backslash  
 633 031 442 838 535 751 691 389 833 211 695 664 682 878 834 965 221 408 378 655 732 611 628 232 697 \ \backslash  
 867 655 607 060 324 995 971 063 800 136 861 952 000  $q^{6484}$  -

250 536 433 255 929 328 727 211 774 382 642 387 048 257 495 155 280 256 076 824 236 113 843 076 015 \
 961 268 661 834 805 715 237 175 682 088 256 483 999 321 709 399 309 081 825 579 070 773 382 739 329 \
 399 312 192 891 093 021 187 558 628 769 367 846 150  $q^{6485} +$

277 193 759 562 834 017 487 194 864 316 976 246 257 747 363 763 447 087 492 769 981 162 232 943 433 \
 799 310 643 909 816 009 585 305 573 918 584 168 257 753 966 820 714 227 540 953 865 674 119 942 049 \
 374 034 342 056 100 671 999 490 528 222 929 105 408  $q^{6488} -$

286 694 074 775 686 189 852 135 906 325 957 458 685 380 667 709 897 492 553 177 869 136 015 720 861 \
 904 283 335 446 955 352 320 863 807 615 032 834 833 245 171 446 004 231 952 943 691 993 518 105 617 \
 858 078 761 280 841 960 410 997 684 524 728 320 000  $q^{6489} +$

317 188 748 450 574 839 169 849 034 288 651 889 157 345 489 366 514 915 969 067 479 044 731 042 454 \
 930 409 347 995 129 634 813 342 612 182 063 578 458 628 232 232 669 945 260 973 112 340 500 250 299 \
 378 684 365 254 208 797 066 314 789 901 052 463 104  $q^{6492} -$

328 056 421 363 189 912 615 660 002 345 468 278 315 038 882 057 749 089 278 650 153 333 270 402 223 \
 269 411 984 165 334 022 310 247 399 253 779 657 311 705 894 143 898 421 797 594 491 169 875 359 712 \
 943 305 581 753 506 595 949 507 989 051 325 643 549  $q^{6493} +$

362 939 393 400 801 971 459 935 103 692 750 656 409 203 797 915 206 315 341 377 970 145 027 722 300 \
 393 437 414 006 877 479 621 341 482 184 394 994 915 945 834 161 477 133 592 056 690 499 965 497 824 \
 925 092 648 585 891 674 934 257 942 071 414 784 000  $q^{6496} -$

375 370 712 031 175 026 811 988 798 937 151 647 082 196 858 883 479 222 990 612 216 480 019 872 028 \
 557 330 097 669 340 411 510 075 410 298 128 139 077 599 787 733 960 956 125 226 303 351 160 203 993 \
 294 066 148 130 913 790 631 209 831 121 931 730 944  $q^{6497} +$

415 271 830 831 662 046 130 710 762 983 647 513 594 954 519 421 480 045 147 529 493 817 476 910 438 \
 647 891 296 288 261 386 234 418 923 292 700 038 581 020 330 063 710 957 504 503 713 655 409 947 898 \
 303 724 313 436 697 036 937 491 824 195 608 576 000  $q^{6500} -$

429 491 187 546 474 026 711 447 522 813 315 998 891 448 042 368 173 496 270 840 962 487 108 686 329 \
 188 632 893 149 108 968 114 223 786 207 401 308 607 281 127 586 115 522 396 368 882 916 664 660 643 \
 042 842 175 346 342 643 589 847 875 947 691 668 375  $q^{6501} +$

475 130 467 799 995 421 905 979 726 123 273 587 519 713 952 475 592 692 750 396 303 746 834 018 388 \
 556 983 581 511 466 643 659 996 102 971 841 959 857 023 675 328 365 115 456 843 268 916 562 482 984 \
 703 565 166 720 103 457 334 728 197 259 479 424 000  $q^{6504} -$

491 394 372 802 098 218 319 389 913 418 560 845 518 823 169 302 683 249 477 502 909 719 679 177 847 \
 265 553 639 511 061 378 865 289 525 009 916 548 403 402 393 356 259 814 598 341 778 296 713 614 330 \
 158 614 624 628 625 312 955 300 956 676 276 224 000  $q^{6505} +$

543 594 869 717 652 104 250 122 744 458 947 108 728 632 207 445 567 482 497 180 549 970 386 822 415 \
 676 890 285 283 299 581 878 587 932 993 653 371 352 812 417 232 906 946 981 908 390 788 499 263 900 \
 465 079 482 571 956 215 547 720 962 564 008 197 632  $q^{6508} -$

562 196 536 195 818 038 211 939 442 001 933 768 821 984 524 653 846 793 842 602 008 737 524 269 992 \
 605 363 167 206 807 103 956 871 685 475 571 288 606 780 649 499 546 342 445 215 792 170 438 964 560 \
 122 648 884 521 303 762 414 444 649 186 640 529 500  $q^{6509} +$

621 899 053 174 168 803 841 801 532 382 400 110 158 441 795 772 913 528 782 462 756 847 594 952 667 \
 760 662 483 396 463 139 566 202 226 341 726 426 090 761 093 839 404 894 510 458 732 186 695 709 618 \
 921 158 060 587 353 880 494 094 911 590 134 267 904  $q^{6512} -$

643 173 635 328 363 268 062 002 286 057 253 471 992 676 997 636 840 147 102 805 387 388 979 693 840 \
 654 689 950 542 099 470 656 025 882 181 977 545 126 319 274 260 735 604 774 460 107 631 942 889 713 \
 135 815 710 955 214 236 889 096 419 283 342 131 200  $q^{6513} +$

711 453 525 504 934 300 427 577 883 761 000 631 683 071 907 904 224 358 164 312 557 948 940 273 984 \
 414 025 092 228 051 180 617 026 210 378 072 029 391 884 452 830 012 408 450 613 980 742 778 583 831 \
 613 197 046 978 188 096 530 716 642 036 593 920 000  $q^{6516} -$

735 784 102 167 969 569 464 333 942 886 825 207 460 856 777 998 936 447 706 311 422 415 985 166 658 \
 120 037 952 437 398 528 428 887 100 043 106 578 544 457 968 928 143 797 157 402 570 185 794 337 527 \
 015 410 452 376 588 561 291 454 441 509 479 624 306  $q^{6517} +$

813 870 461 146 878 350 206 315 237 213 935 078 205 559 194 003 883 331 047 654 778 502 538 881 430 \
 258 751 418 086 250 749 866 277 707 968 055 044 291 286 082 082 398 212 652 718 291 134 671 366 808 \
 198 434 063 653 296 398 695 852 486 526 670 720 000  $q^{6520} -$

841 694 870 857 253 860 644 894 479 338 409 670 448 101 306 239 527 245 128 123 271 480 263 365 431 \

981 225 323 661 795 088 697 411 800 223 856 736 323 131 799 851 382 079 174 422 490 286 755 163 430  
 958 720 154 033 075 191 149 953 272 116 645 888 000  $q^{6521} +$   
 930 992 460 066 475 054 423 958 990 542 107 609 314 161 474 709 037 727 289 582 180 584 732 977 971  
 078 946 939 334 811 856 838 770 198 726 693 096 981 053 212 137 573 750 486 639 559 432 121 702 410  
 659 911 054 731 312 996 657 517 148 798 044 160 000  $q^{6524} -$   
 962 811 108 436 757 112 728 474 820 032 534 431 642 962 137 152 571 836 980 808 283 538 211 309 988  
 302 280 999 665 969 944 441 244 444 187 681 208 314 063 953 586 178 218 282 383 822 293 249 744 404  
 924 580 004 261 015 667 992 277 010 165 843 501 525  $q^{6525} +$   
 1 064 925 396 591 490 567 241 993 465 342 747 728 995 787 466 032 730 967 531 906 086 183 336 699 270  
 375 471 730 607 238 590 676 494 038 470 002 732 033 127 920 559 737 489 689 854 165 990 312 516 599  
 755 259 674 532 074 387 442 080 646 510 974 271 488  $q^{6528} -$   
 1 101 310 173 923 216 757 230 030 695 565 197 112 220 356 576 362 400 541 464 672 466 896 218 734 806  
 101 416 438 049 843 089 065 368 028 160 894 151 970 855 811 484 442 186 426 605 493 193 016 515 451  
 494 028 208 628 305 214 798 411 718 199 525 376 000  $q^{6529} +$   
 1 218 075 938 927 985 647 376 623 650 778 107 057 769 041 042 487 542 457 846 129 100 738 172 158 807  
 117 109 612 764 260 273 153 854 397 507 425 084 215 269 332 159 358 687 958 504 404 904 521 755 909  
 405 789 683 899 714 476 441 055 570 028 182 568 960  $q^{6532} -$   
 1 259 680 405 546 032 306 970 972 670 159 911 678 744 100 745 362 182 837 307 388 348 853 447 681 469  
 499 679 576 014 294 559 626 299 362 919 947 947 584 752 677 119 034 090 034 397 131 708 566 551 205  
 635 961 195 957 776 768 352 622 684 284 479 495 814  $q^{6533} +$   
 1 393 194 401 751 689 151 625 658 230 420 051 364 254 258 343 722 140 924 463 100 514 535 901 322 379  
 520 832 414 693 219 245 608 995 873 958 122 624 790 055 642 024 231 925 890 146 494 957 895 802 202  
 476 336 747 349 756 795 449 862 008 840 639 232 000  $q^{6536} -$   
 1 440 765 420 808 454 275 207 378 827 034 717 240 536 625 572 898 645 323 455 244 679 930 493 267 736  
 338 672 472 195 011 701 127 394 604 717 463 155 971 415 886 612 537 523 726 626 905 391 623 892 364  
 672 310 741 925 055 995 136 351 261 810 461 736 960  $q^{6537} +$   
 1 593 423 687 958 257 025 787 593 887 749 426 232 324 878 852 183 542 975 313 372 306 624 428 791 992  
 309 540 407 100 794 026 973 821 726 348 179 205 767 317 190 581 157 550 815 659 983 551 324 625 318  
 000 480 145 824 403 484 749 027 406 444 205 772 800  $q^{6540} -$   
 1 647 814 710 878 802 412 460 043 452 104 224 908 663 979 971 128 353 955 772 397 094 143 614 716 743  
 293 217 867 375 095 307 451 666 690 129 235 498 345 682 417 415 327 062 552 820 307 470 801 396 077  
 858 875 745 884 047 360 001 099 481 302 839 477 875  $q^{6541} +$   
 1 822 355 182 571 263 005 406 037 177 473 324 432 221 693 382 743 196 849 128 890 422 550 045 239 671  
 185 191 217 951 904 214 683 020 619 945 399 600 951 807 051 688 199 847 192 263 342 483 295 549 655  
 436 152 131 489 498 518 191 435 744 452 280 320 000  $q^{6544} -$   
 1 884 541 421 317 114 850 471 502 796 389 494 420 502 361 563 240 198 525 768 649 123 863 823 526 157  
 313 148 116 912 545 064 516 104 299 695 638 614 964 911 014 597 822 286 695 199 629 795 856 402 150  
 350 844 970 822 615 141 927 187 177 324 845 465 600  $q^{6545} +$   
 2 084 092 583 800 183 139 540 095 685 645 449 333 259 922 535 375 903 489 928 200 464 481 326 043 009  
 512 905 189 810 723 240 876 690 064 355 603 558 677 869 815 349 836 261 821 210 728 261 690 451 060  
 318 664 947 411 702 341 182 476 841 988 179 015 680  $q^{6548} -$   
 2 155 188 337 226 294 499 645 847 044 404 348 597 288 414 431 098 633 012 088 762 224 629 298 751 301  
 896 603 477 888 964 977 304 696 741 839 020 195 710 503 480 891 028 255 937 411 605 343 622 852 378  
 210 256 702 031 289 859 199 188 851 090 413 753 625  $q^{6549} +$   
 2 383 324 795 434 367 834 223 810 502 005 809 792 933 594 425 632 508 804 811 811 451 010 612 768 376  
 312 980 007 725 541 904 300 074 808 326 942 197 159 146 268 115 229 558 707 049 089 308 398 796 772  
 414 326 024 587 295 504 073 873 270 616 938 597 376  $q^{6552} -$   
 2 464 603 234 776 077 248 385 391 076 335 778 982 117 609 487 473 419 163 556 460 746 502 327 508 538  
 230 565 425 250 235 339 392 268 574 075 073 432 375 920 674 138 707 096 896 410 586 219 117 794 158  
 968 938 765 145 814 168 765 894 107 833 882 804 224  $q^{6553} +$   
 2 725 409 163 571 903 182 726 452 545 026 756 467 844 914 369 361 366 143 548 893 940 396 883 210 877  
 907 502 220 214 161 017 128 648 408 505 456 466 130 636 972 755 013 369 514 066 651 108 590 470 779  
 313 398 233 163 211 633 825 712 726 368 542 976 000  $q^{6556} -$   
 2 818 324 925 182 560 223 513 674 814 439 495 141 052 035 695 636 199 001 875 896 157 781 475 091 006  
 209 780 011 039 690 193 671 952 757 834 875 647 872 903 358 528 326 130 251 382 842 892 687 648 599

651 517 890 253 774 992 220 133 162 989 015 811 773  $q^{6557} +$   
 3 116 466 521 872 490 352 323 854 823 067 845 233 853 318 586 676 689 663 162 094 810 807 075 610 631  
 372 732 389 164 838 558 126 933 750 787 001 938 502 080 400 686 344 349 031 405 553 042 235 230 102  
 342 202 574 375 806 347 710 738 425 093 328 896 000  $q^{6560} -$   
 3 222 681 504 485 732 973 353 904 641 838 085 478 526 260 695 881 461 129 534 397 037 710 139 399 131  
 662 948 344 097 946 244 290 312 820 140 130 675 385 308 123 003 290 835 597 290 370 547 179 794 214  
 247 777 618 770 199 035 374 603 103 654 420 480 248  $q^{6561} +$   
 3 563 489 716 235 908 126 794 087 402 077 607 691 798 616 708 989 003 817 679 544 980 159 817 147 937  
 715 661 067 613 299 271 258 979 139 144 599 277 869 785 635 924 776 719 697 591 278 408 015 095 037  
 797 056 972 419 425 562 922 594 014 194 620 416 000  $q^{6564} -$   
 3 684 902 536 102 200 782 221 432 323 570 141 928 358 659 359 931 603 965 895 842 197 710 687 632 410  
 945 875 156 873 985 063 873 288 092 308 239 449 333 643 863 961 245 119 107 628 891 674 766 726 493  
 890 448 066 274 683 627 760 855 969 815 065 123 750  $q^{6565} +$   
 4 074 467 515 627 997 501 641 920 909 143 742 660 151 678 705 214 897 209 302 884 262 905 728 054 044  
 865 880 452 814 789 293 095 517 787 962 581 440 936 709 742 123 555 395 053 087 037 515 354 884 160  
 611 242 536 604 218 772 901 730 012 753 379 451 392  $q^{6568} -$   
 4 213 247 136 845 328 732 997 137 756 222 975 986 396 602 790 950 060 264 660 799 396 367 486 842 416  
 356 388 034 461 938 063 031 537 533 860 230 978 368 085 140 970 227 601 473 756 441 718 089 684 935  
 113 849 101 130 351 142 174 085 593 808 310 272 000  $q^{6569} +$   
 4 658 526 084 792 619 528 364 164 617 585 095 313 055 477 296 644 161 978 995 685 328 124 792 039 494  
 997 568 032 641 268 339 603 817 273 507 795 247 944 787 219 444 813 201 200 616 144 009 184 327 928  
 640 727 507 276 881 012 787 776 112 939 353 773 056  $q^{6572} -$   
 4 817 150 215 124 799 529 829 067 531 021 059 866 829 750 361 220 092 576 994 239 771 337 415 561 574  
 300 938 333 286 042 934 227 522 735 338 342 825 966 371 566 640 767 409 362 034 012 687 392 907 000  
 209 305 530 224 210 009 431 521 334 170 541 440 185  $q^{6573} +$   
 5 326 090 501 461 592 656 852 220 838 550 864 859 976 296 141 782 776 813 011 089 662 472 707 492 422  
 890 508 897 021 022 406 587 369 156 215 294 775 951 923 760 559 242 548 008 510 139 425 708 159 732  
 705 480 725 908 764 389 519 917 031 852 905 472 000  $q^{6576} -$   
 5 507 389 427 178 239 822 706 650 162 948 883 641 752 720 823 326 283 922 852 041 644 424 458 691 390  
 284 753 688 220 473 860 426 789 232 358 955 775 360 966 836 209 126 172 919 821 098 509 720 085 736  
 283 223 193 623 774 697 188 599 896 072 142 094 336  $q^{6577} +$   
 6 089 069 150 718 842 137 253 202 753 798 797 789 879 760 104 231 637 128 987 435 689 063 670 708 358  
 755 508 889 981 831 340 710 194 630 161 821 393 287 489 700 915 512 038 764 812 876 327 119 877 225  
 073 711 160 367 387 117 514 325 099 141 341 593 600  $q^{6580} -$   
 6 296 275 778 939 716 075 372 077 187 120 437 236 855 913 913 558 495 439 194 489 744 771 298 210 319  
 313 311 409 883 570 383 111 323 212 141 308 502 264 252 818 881 078 071 847 655 365 436 778 550 943  
 861 421 926 200 065 763 699 226 373 478 233 444 625  $q^{6581} +$   
 6 961 064 228 447 417 504 637 427 795 735 315 250 088 224 217 742 340 666 498 009 799 075 731 631 220  
 194 428 907 122 318 623 793 921 374 265 612 187 675 338 481 552 850 288 955 822 769 381 215 775 888  
 047 209 015 070 644 504 370 282 399 472 342 912 000  $q^{6584} -$   
 7 197 871 213 772 729 461 682 100 989 758 896 952 880 868 722 285 450 297 908 534 290 992 958 317 019  
 364 769 558 113 155 485 576 042 966 931 142 312 860 904 563 181 889 651 881 399 136 686 111 848 266  
 509 385 421 606 167 286 203 181 868 323 012 608 000  $q^{6585} +$   
 7 957 612 041 193 953 479 738 858 288 971 703 643 601 705 972 344 131 644 445 129 526 357 646 738 621  
 766 549 155 146 434 716 415 362 446 042 764 105 081 249 880 960 559 633 854 454 794 904 124 806 224  
 318 221 592 565 968 863 229 900 436 117 913 444 352  $q^{6588} -$   
 8 228 236 996 923 975 553 877 015 643 200 254 428 290 811 630 527 670 237 920 369 572 129 585 821 997  
 340 099 702 644 570 646 563 580 808 628 490 748 776 535 576 425 791 562 013 658 268 762 420 044 610  
 189 794 655 936 012 011 681 404 067 970 480 734 125  $q^{6589} +$   
 9 096 457 309 195 979 126 615 406 588 901 968 776 502 982 579 910 327 423 681 874 383 404 414 808 071  
 257 094 310 281 925 882 701 462 305 642 331 596 063 288 729 928 304 987 233 151 895 812 850 292 907  
 767 224 264 400 968 862 193 579 040 739 027 451 904  $q^{6592} -$   
 9 405 717 244 321 895 947 977 271 459 922 138 338 794 062 236 324 333 937 489 609 416 005 315 431 785  
 515 758 052 881 350 516 467 365 977 753 669 443 428 125 941 082 730 247 871 122 349 241 447 215 030  
 645 171 827 469 650 956 564 803 934 778 121 027 584  $q^{6593} +$

10 397 866 271 705 569 859 396 391 348 168 736 054 762 938 147 963 201 873 551 822 351 377 945 493 \
 028 822 193 222 064 766 154 488 407 643 453 707 886 184 090 100 608 370 554 102 321 318 912 654 808 \
 192 483 374 463 901 220 089 258 651 742 027 849 728 000  $q^{6596}$  -

10 751 262 555 521 729 502 845 375 646 451 201 241 364 315 925 760 204 300 437 728 879 419 700 737 \
 248 926 362 643 763 752 033 860 260 270 247 313 985 616 475 759 885 896 194 269 555 849 098 026 431 \
 887 370 204 339 062 402 778 229 281 126 093 338 418 492  $q^{6597}$  +

11 884 984 069 335 058 127 778 168 930 158 659 679 819 608 834 160 430 346 971 163 852 563 050 875 \
 912 073 822 830 067 387 697 760 054 546 851 545 601 875 829 585 954 606 802 278 335 995 847 303 091 \
 919 907 396 675 574 121 148 821 056 561 174 814 617 600  $q^{6600}$  -

12 288 799 408 753 312 002 870 659 539 140 414 729 186 209 103 048 438 440 667 313 487 225 046 536 \
 316 693 363 108 098 772 757 405 992 168 339 414 555 865 754 392 358 836 003 946 197 939 896 405 189 \
 457 275 154 084 767 333 881 161 555 507 552 567 296 000  $q^{6601}$  +

13 584 242 648 603 219 944 279 087 579 426 399 084 835 116 936 717 988 671 989 783 880 809 274 402 \
 243 715 175 319 360 225 835 335 421 719 659 744 446 495 448 612 600 129 243 930 027 168 952 326 501 \
 208 990 569 157 022 928 560 614 814 543 019 714 048 000  $q^{6604}$  -

14 045 651 772 203 110 782 740 902 046 004 822 104 940 631 706 567 398 745 497 686 017 828 782 469 \
 952 140 258 160 241 589 598 811 390 786 135 803 281 076 495 182 998 959 516 377 483 157 751 733 815 \
 715 309 114 392 437 398 328 627 402 148 141 320 907 125  $q^{6605}$  +

15 525 826 312 458 654 631 517 490 676 119 649 144 268 594 114 768 554 082 541 487 858 788 875 166 \
 524 144 677 168 450 099 814 275 702 280 013 517 922 607 955 986 349 960 529 765 316 862 381 151 595 \
 869 269 894 803 991 759 998 803 446 757 996 048 252 928  $q^{6608}$  -

16 053 022 293 584 533 036 320 030 309 491 753 861 904 955 444 772 124 997 648 388 108 099 332 612 \
 089 927 473 174 241 674 087 942 725 464 593 622 931 654 016 118 389 966 500 503 128 285 551 086 238 \
 004 874 460 473 433 236 018 399 727 213 286 682 624 000  $q^{6609}$  +

17 744 203 042 441 869 219 837 316 310 313 550 199 576 874 881 266 738 347 695 874 155 155 887 591 \
 935 494 179 468 121 482 689 156 129 108 238 269 359 840 493 274 590 164 179 040 885 309 502 659 061 \
 259 578 349 360 004 217 220 580 068 764 080 997 433 344  $q^{6612}$  -

18 346 541 465 364 328 175 766 373 989 933 873 053 327 203 452 065 456 910 343 396 468 994 568 365 \
 939 198 942 019 900 179 350 361 272 713 791 965 104 163 607 921 023 087 445 459 045 232 216 304 900 \
 601 595 294 113 236 101 572 849 208 532 838 380 912 050  $q^{6613}$  +

20 278 730 860 574 100 927 024 323 216 031 346 817 762 927 863 909 686 289 494 383 491 706 328 908 \
 718 672 697 687 776 165 740 656 021 000 651 128 137 050 170 663 071 216 051 371 224 633 627 267 462 \
 152 313 719 785 188 110 992 677 846 643 808 032 320 000  $q^{6616}$  -

20 966 894 343 546 241 473 413 345 465 722 445 570 445 389 638 422 783 419 810 767 554 439 339 924 \
 288 680 212 654 046 561 160 158 397 252 763 806 611 393 443 159 704 122 949 033 898 496 424 270 747 \
 003 726 263 973 817 525 568 426 523 516 184 188 747 776  $q^{6617}$  +

23 174 349 801 693 229 935 744 665 095 646 339 677 797 468 203 511 527 388 747 142 090 323 938 040 \
 880 681 893 144 044 045 983 082 033 418 658 620 692 509 497 193 053 111 127 324 235 717 046 097 766 \
 517 914 898 950 783 489 061 976 903 740 520 636 876 800  $q^{6620}$  -

23 960 535 743 982 936 380 020 230 174 738 702 318 165 197 927 109 213 026 040 017 465 785 884 831 \
 445 466 084 543 502 766 010 860 809 602 370 008 960 217 301 973 405 267 464 076 392 752 566 556 957 \
 628 706 942 548 715 123 107 127 496 205 704 863 232 750  $q^{6621}$  +

26 482 371 552 203 562 661 128 529 417 434 261 565 218 579 048 141 385 044 558 937 758 098 606 535 \
 756 959 621 002 252 747 147 868 277 598 527 043 908 433 696 977 048 964 627 565 662 043 637 145 083 \
 377 053 948 563 845 988 857 902 920 042 012 810 240 000  $q^{6624}$  -

27 380 506 374 945 690 875 004 659 959 155 929 689 438 305 310 844 821 545 584 258 497 969 373 963 \
 945 301 049 238 776 311 398 589 851 616 650 843 446 295 719 949 383 993 913 734 142 912 878 613 360 \
 356 224 839 031 354 682 948 588 901 439 906 201 600 000  $q^{6625}$  +

30 261 380 504 601 350 346 506 502 784 025 100 646 991 999 529 584 346 086 677 019 433 769 573 582 \
 417 853 971 464 314 457 002 646 886 410 398 601 092 425 403 674 403 078 157 988 780 855 663 756 596 \
 139 910 633 764 974 305 279 890 281 579 801 207 767 040  $q^{6628}$  -

31 287 364 114 510 342 446 863 713 504 947 510 852 852 211 601 107 227 488 027 272 726 718 281 705 \
 232 032 068 692 145 296 817 469 755 108 279 072 978 776 794 949 551 203 099 492 629 239 109 900 209 \
 448 549 388 344 628 895 654 102 866 236 047 928 190 375  $q^{6629}$  +

34 578 261 907 777 458 717 426 275 485 874 254 693 584 468 816 160 601 351 647 466 874 053 260 602 \

764 778 420 697 751 258 259 498 358 219 087 986 018 224 793 589 997 892 801 632 565 452 363 929 394 \
 268 146 778 554 808 123 171 014 859 862 267 944 377 856  $q^{6632}$  -

35 750 246 636 278 405 377 043 327 633 627 680 761 212 555 547 673 640 027 609 561 526 550 731 087 \
 245 223 138 556 588 047 090 049 264 529 243 118 286 509 088 778 214 503 151 441 888 093 870 799 028 \
 139 152 440 948 114 855 816 396 754 560 044 163 760 128  $q^{6633}$  +

39 509 374 994 135 100 346 338 398 859 606 284 159 634 539 455 421 322 405 265 412 919 644 305 235 \
 355 470 661 039 742 970 992 175 558 862 966 942 577 932 263 287 777 714 436 020 639 219 453 130 636 \
 825 377 470 967 010 718 335 064 371 097 701 961 216 000  $q^{6636}$  -

40 848 083 861 296 122 186 452 849 828 452 214 988 105 552 441 877 317 784 367 610 743 001 450 838 \
 562 437 595 540 834 923 264 682 765 165 332 179 913 158 524 667 959 704 065 566 426 412 789 696 263 \
 750 064 302 217 713 333 259 840 637 655 599 714 351 161  $q^{6637}$  +

45 141 891 473 767 276 492 643 644 260 998 369 747 993 497 402 158 195 453 887 013 120 671 274 014 \
 173 735 972 230 073 785 340 162 762 939 571 512 306 923 466 539 509 972 747 804 334 105 856 922 790 \
 820 060 395 671 883 535 667 680 867 004 038 583 500 800  $q^{6640}$  -

46 670 981 306 787 027 364 601 045 431 516 233 375 186 020 374 612 032 318 935 697 993 222 749 429 \
 711 009 912 285 548 848 892 009 563 520 933 966 216 532 725 578 357 511 310 424 312 961 340 919 802 \
 237 708 855 045 254 787 261 150 884 561 865 678 848 000  $q^{6641}$  +

51 575 322 646 352 057 504 219 242 353 550 761 947 389 706 909 276 397 927 570 955 621 254 969 448 \
 462 555 213 212 304 981 480 164 767 407 074 178 925 280 352 289 501 978 758 865 917 314 040 273 937 \
 205 817 415 064 420 740 492 345 603 643 857 129 472 000  $q^{6644}$  -

53 321 798 357 938 262 592 146 058 908 833 495 940 765 742 459 120 104 165 657 984 209 733 605 415 \
 894 646 124 145 910 864 125 814 327 226 958 930 735 263 557 427 891 041 723 115 739 564 960 395 484 \
 938 580 823 441 885 336 969 165 278 450 415 578 145 300  $q^{6645}$  +

58 923 261 642 075 259 538 634 416 874 301 565 047 716 423 574 685 502 556 873 569 724 904 489 637 \
 800 974 985 298 852 708 025 095 484 578 771 229 779 144 505 876 257 414 856 849 888 381 518 263 668 \
 634 933 367 417 898 061 687 865 166 951 241 371 853 824  $q^{6648}$  -

60 917 948 858 133 142 497 133 396 664 208 974 781 909 603 474 587 949 149 057 745 043 986 944 009 \
 791 817 077 606 832 402 510 237 947 025 214 097 823 247 687 102 203 177 373 411 539 092 526 215 304 \
 979 952 802 302 588 808 754 597 718 479 893 471 232 000  $q^{6649}$  +

67 315 371 019 638 217 196 785 749 523 062 924 415 294 411 739 371 108 759 478 686 250 387 787 403 \
 981 271 908 874 294 162 175 785 935 979 645 368 343 284 100 765 770 265 944 933 889 102 160 903 610 \
 324 742 542 074 452 894 234 888 630 707 431 675 715 584  $q^{6652}$  -

69 593 455 253 411 315 337 991 954 916 467 805 014 457 557 996 822 016 464 528 104 533 808 039 078 \
 994 156 234 016 901 841 825 218 576 465 585 979 893 163 823 757 895 450 525 883 161 450 289 898 330 \
 626 293 692 543 634 420 392 238 460 855 951 737 154 196  $q^{6653}$  +

76 899 650 185 887 837 159 085 358 417 185 425 935 517 891 765 779 351 876 274 716 997 167 233 423 \
 642 228 008 417 426 728 061 405 943 986 131 621 044 841 946 741 954 498 466 395 258 875 284 591 313 \
 186 904 935 981 367 314 994 793 522 731 056 332 800 000  $q^{6656}$  -

79 501 291 904 305 076 092 682 407 833 032 214 854 662 108 096 251 782 434 646 989 649 463 163 651 \
 541 168 859 178 963 486 783 689 057 556 818 988 317 476 596 360 452 840 645 171 978 153 612 036 274 \
 050 308 679 085 262 784 175 332 596 868 380 959 047 680  $q^{6657}$  +

87 845 021 930 307 110 501 324 696 571 738 993 204 350 845 255 532 197 162 977 506 470 882 721 940 \
 174 336 521 334 762 734 179 901 996 055 677 602 380 295 904 684 179 956 273 206 674 070 316 616 926 \
 377 973 561 313 404 233 118 560 025 668 477 888 102 400  $q^{6660}$  -

90 816 058 167 435 804 617 568 756 921 228 157 532 721 196 291 226 507 416 346 085 276 469 649 521 \
 088 813 918 077 713 974 049 009 768 037 342 287 301 376 602 797 931 303 797 571 707 493 208 274 704 \
 638 894 195 763 238 627 069 739 191 159 018 721 876 500  $q^{6661}$  +

100 344 282 871 101 653 143 522 623 855 449 104 731 964 285 148 473 952 836 606 913 461 697 674 753 \
 806 268 188 166 002 134 532 652 673 475 127 344 074 153 575 471 712 042 734 936 157 405 522 391 857 \
 969 390 909 748 711 157 676 765 490 477 085 961 856 000  $q^{6664}$  -

103 737 027 535 665 705 154 254 119 916 098 114 238 111 613 095 838 340 336 934 330 765 920 139 723 \
 635 959 549 080 849 122 731 273 914 274 588 569 100 356 419 278 944 665 464 101 468 551 877 192 633 \
 340 472 469 830 295 076 227 346 845 952 001 625 292 800  $q^{6665}$  +

114 617 468 881 970 633 184 475 813 287 445 700 293 935 023 959 587 119 460 814 874 721 789 711 206 \
 946 636 941 053 097 485 623 174 177 841 397 985 449 939 011 135 470 642 055 466 362 520 994 908 989

624 888 697 844 857 552 303 499 692 856 037 050 450 432  $q^{6668}$  –  
 118 491 625 606 357 829 522 731 078 687 340 688 743 126 119 777 327 058 826 043 759 621 513 821 011  $q^{6669}$  +  
 723 981 061 228 423 645 208 192 505 744 878 953 906 850 987 513 807 526 690 984 505 600 221 311 614  $q^{6670}$  –  
 353 093 734 020 076 228 835 425 992 810 658 191 397 500  $q^{6671}$  +  
 130 915 693 716 994 795 926 497 340 825 373 184 216 785 261 329 163 202 537 839 308 228 478 110 419  $q^{6672}$  –  
 535 445 152 231 778 191 541 906 414 908 907 149 810 320 543 905 738 341 289 501 298 771 050 380 541  $q^{6673}$  +  
 420 809 390 749 134 039 164 521 029 461 910 950 641 664  $q^{6674}$  –  
 135 339 397 033 081 340 070 685 342 210 458 183 931 309 942 373 372 006 492 306 065 420 411 729 026  $q^{6675}$  +  
 994 174 583 154 284 579 574 806 403 269 169 763 598 255 152 924 310 879 250 071 265 803 270 658 964  $q^{6676}$  –  
 969 776 335 089 297 581 056 718 673 216 259 936 059 392  $q^{6677}$  +  
 149 525 527 197 437 026 473 802 888 951 764 726 462 081 482 634 319 668 029 981 612 454 573 654 783  $q^{6678}$  –  
 038 493 611 219 283 042 700 267 157 035 067 125 735 053 866 602 491 687 566 135 874 330 175 179 181  $q^{6679}$  +  
 164 415 470 862 710 993 168 671 392 458 771 430 656 000  $q^{6680}$  –  
 154 576 530 032 970 612 542 351 842 977 358 271 479 557 153 323 292 833 337 906 232 711 211 409 110  $q^{6681}$  +  
 580 193 443 597 744 829 766 905 207 325 634 561 244 959 498 138 283 265 857 656 678 407 270 325 464  $q^{6682}$  –  
 841 852 623 295 240 802 293 246 974 721 713 532 010 392  $q^{6683}$  +  
 170 773 988 607 613 783 096 233 396 926 375 296 806 685 760 862 842 161 716 068 929 601 267 682 970  $q^{6684}$  –  
 357 673 412 023 936 137 746 635 817 424 627 802 523 322 734 279 705 546 739 574 044 296 394 580 267  $q^{6685}$  +  
 782 011 812 146 262 109 785 807 927 290 877 507 097 600  $q^{6686}$  –  
 176 541 016 613 481 799 782 347 960 791 346 649 032 901 213 004 356 801 367 255 410 158 515 951 158  $q^{6687}$  +  
 499 016 806 002 989 513 473 944 924 979 276 480 520 252 273 424 312 935 364 757 052 630 191 378 092  $q^{6688}$  –  
 287 279 302 930 721 955 696 076 053 543 741 407 232 000  $q^{6689}$  +  
 195 034 241 525 645 325 610 904 345 614 456 983 780 742 311 652 720 414 007 717 213 869 166 734 183  $q^{6690}$  –  
 180 599 213 406 639 305 980 168 238 708 107 246 348 299 356 977 471 644 820 999 763 938 535 160 873  $q^{6691}$  +  
 732 507 662 654 200 218 577 322 827 401 572 914 432 000  $q^{6692}$  –  
 201 618 537 612 005 872 131 579 760 024 914 884 541 184 819 188 345 269 296 260 026 182 431 590 490  $q^{6693}$  +  
 956 727 272 117 027 453 770 035 600 886 840 829 869 398 375 125 277 819 054 042 047 901 973 527 694  $q^{6694}$  –  
 786 679 966 199 123 158 407 240 870 042 457 042 423 100  $q^{6695}$  +  
 222 732 088 369 094 824 890 261 642 345 476 535 406 252 740 099 609 869 524 795 717 763 086 712 740  $q^{6696}$  –  
 132 031 361 660 197 842 883 387 973 446 062 395 474 535 620 246 314 032 760 394 282 216 183 998 130  $q^{6697}$  +  
 199 099 218 215 984 244 811 183 841 857 082 848 542 720  $q^{6698}$  –  
 230 249 174 095 913 777 145 586 390 570 546 146 872 777 889 175 328 447 470 816 634 615 243 171 091  $q^{6699}$  +  
 705 889 087 112 174 866 887 993 991 515 233 223 571 255 447 867 744 112 012 082 708 045 810 289 257  $q^{6700}$  –  
 154 435 447 573 595 465 640 338 221 462 316 949 504 000  $q^{6701}$  +  
 254 353 376 670 550 584 329 688 352 498 403 096 951 808 182 421 644 074 199 396 606 854 531 356 391  $q^{6702}$  –  
 612 810 103 125 056 443 387 126 939 393 298 383 986 544 410 266 330 863 968 506 845 508 188 855 075  $q^{6703}$  +  
 938 199 719 966 604 476 727 114 183 399 460 525 834 240  $q^{6704}$  –  
 262 935 060 861 196 240 687 443 116 276 960 566 820 621 352 247 730 910 049 653 672 104 397 604 206  $q^{6705}$  +  
 124 248 422 915 629 904 204 311 730 965 663 916 215 297 635 543 708 743 390 620 730 718 974 658 842  $q^{6706}$  –  
 389 006 756 399 148 725 558 053 645 430 334 248 538 320  $q^{6707}$  +  
 290 452 444 747 869 434 579 498 424 113 560 123 778 407 173 318 614 740 471 205 443 436 722 329 374  $q^{6708}$  –  
 258 601 921 541 731 392 962 470 631 284 296 723 365 165 871 739 085 277 034 326 039 011 970 864 229  $q^{6709}$  +  
 710 503 194 637 935 514 410 419 574 365 330 529 792 000  $q^{6710}$  –  
 300 249 113 936 413 698 321 803 842 507 333 944 639 089 025 353 432 099 445 216 928 685 154 958 235  $q^{6711}$  +  
 740 732 157 540 220 304 767 042 039 742 182 578 338 919 691 616 142 029 925 927 761 562 294 245 161  $q^{6712}$  –  
 817 994 019 382 743 803 886 638 395 679 563 895 930 880  $q^{6713}$  +  
 331 661 752 264 292 127 095 999 451 955 982 706 980 769 904 014 349 401 490 715 888 951 538 480 602  $q^{6714}$  –  
 641 162 389 721 817 012 760 293 584 881 909 255 715 544 406 088 899 208 138 280 597 920 452 589 102  $q^{6715}$  +  
 544 921 843 922 381 934 596 691 024 910 431 835 020 800  $q^{6716}$  –  
 342 844 982 420 186 394 261 568 312 108 483 465 287 762 215 438 950 348 937 366 146 994 119 500 400  $q^{6717}$  +  
 979 489 126 661 031 651 986 530 549 871 509 900 116 273 656 553 766 775 044 848 422 461 030 556 110  $q^{6718}$  –  
 669 188 898 458 653 624 069 720 072 114 025 702 737 375  $q^{6719}$  +  
 378 702 861 488 091 715 432 893 938 983 665 285 002 515 504 367 710 732 409 573 677 114 803 964 762  $q^{6720}$  –  
 080 543 932 600 817 928 787 383 467 500 272 422 780 170 757 315 066 420 513 957 186 200 140 669 752  $q^{6721}$  +  
 344 330 690 915 703 347 628 959 121 951 427 339 776 000  $q^{6722}$  –

391 468 395 968 061 079 251 206 218 031 103 472 694 276 127 654 459 632 191 772 550 471 608 439 966  
 785 031 114 538 941 633 934 429 594 040 664 096 314 338 314 118 668 944 288 647 959 676 501 656 243  
 764 268 106 171 455 633 567 475 280 577 547 665 408 000  $q^{6705} +$   
 432 398 958 204 978 220 365 853 082 897 118 193 469 115 689 735 871 394 269 045 453 728 946 078 492  
 468 990 579 011 984 927 414 060 991 848 019 440 652 980 662 943 384 408 576 578 284 300 869 626 967  
 023 078 353 683 979 254 730 603 413 489 036 554 764 288  $q^{6708} -$   
 446 970 103 154 828 814 532 627 060 627 246 218 541 700 812 939 003 807 989 129 385 327 705 216 758  
 705 355 212 499 187 886 607 811 175 314 333 040 923 321 905 156 499 044 775 518 757 971 702 310 856  
 649 118 833 364 124 719 691 988 273 988 687 071 918 125  $q^{6709} +$   
 493 689 127 602 150 072 069 078 428 078 924 340 567 566 265 893 026 404 955 116 060 663 610 176 115  
 840 204 843 994 491 835 390 671 247 356 677 795 867 891 819 501 272 296 960 264 965 485 996 651 867  
 592 978 176 818 050 357 208 266 064 164 551 453 512 704  $q^{6712} -$   
 510 320 623 177 190 102 811 858 188 776 973 818 276 715 849 843 886 161 177 066 631 737 291 068 389  
 759 291 099 827 999 534 413 875 664 106 064 161 655 770 997 395 457 066 803 015 419 769 791 288 854  
 016 879 615 116 875 655 134 671 449 918 989 392 084 992  $q^{6713} +$   
 563 644 630 478 099 018 647 078 571 254 868 419 558 950 086 483 825 843 448 259 766 081 224 227 843  
 127 408 620 932 155 918 930 559 804 027 664 629 776 727 919 376 782 856 380 363 617 827 435 587 586  
 216 627 178 509 921 449 486 755 401 661 958 690 816 000  $q^{6716} -$   
 582 627 064 391 263 441 925 678 263 084 394 086 311 626 510 209 076 067 266 295 808 373 537 120 299  
 652 098 581 155 383 581 841 494 732 084 860 754 044 454 282 779 961 531 727 367 769 301 212 312 026  
 818 036 046 322 557 024 628 833 314 456 874 081 204 823  $q^{6717} +$   
 643 487 459 346 461 149 892 031 637 288 883 144 296 215 902 623 705 072 973 110 725 887 926 823 058  
 516 093 135 307 980 290 680 977 805 456 387 607 422 298 771 357 542 617 433 963 407 946 408 799 499  
 424 866 319 434 056 537 536 236 575 890 767 662 284 800  $q^{6720} -$   
 665 152 298 526 020 761 150 708 197 419 234 738 814 822 209 784 766 622 391 277 036 666 200 345 405  
 248 840 574 354 754 149 833 000 255 968 316 914 981 234 091 061 945 266 872 095 079 509 593 790 394  
 551 178 651 802 818 914 289 108 182 577 297 858 560 000  $q^{6721} +$   
 734 611 492 975 322 479 785 882 377 354 843 233 144 471 407 086 591 123 891 932 021 492 953 437 517  
 970 126 309 582 948 835 230 598 656 022 435 100 259 576 664 308 175 961 729 185 604 131 182 333 816  
 728 421 754 846 870 720 600 107 189 232 342 630 426 752  $q^{6724} -$   
 759 336 819 676 375 744 139 786 229 253 860 475 628 745 785 434 645 931 537 019 355 202 927 570 143  
 513 578 426 178 406 932 964 768 962 613 417 196 524 676 529 166 297 581 974 853 884 875 509 376 118  
 989 930 438 408 498 268 025 048 528 881 065 797 638 225  $q^{6725} +$   
 838 606 612 295 675 185 159 759 739 075 875 029 903 245 162 121 281 708 005 275 447 776 819 847 968  
 487 108 112 511 787 938 594 172 911 329 598 680 602 444 244 473 907 857 534 307 654 808 464 913 196  
 836 394 315 074 914 604 087 561 136 641 361 956 663 040  $q^{6728} -$   
 866 823 663 040 336 985 508 928 380 340 562 928 803 625 836 888 907 943 191 898 772 616 933 609 530  
 891 916 199 447 477 215 227 517 099 266 893 590 694 660 666 985 304 173 369 088 932 908 388 406 412  
 873 475 105 968 556 531 413 790 666 133 751 877 632 000  $q^{6729} +$   
 957 286 191 175 788 924 366 738 220 688 486 788 556 536 796 044 337 446 306 869 519 867 244 474 756  
 143 158 596 474 581 103 313 308 664 821 386 325 523 265 035 981 552 883 201 243 945 001 789 699 967  
 183 725 825 942 664 628 322 607 520 886 975 766 025 216  $q^{6732} -$   
 989 486 810 599 724 288 063 871 867 132 502 986 726 538 912 490 168 074 055 395 741 029 957 179 143  
 736 232 432 738 959 382 419 192 798 000 868 520 015 061 396 294 469 814 545 943 955 467 058 065 914  
 185 449 931 958 676 171 774 514 537 838 551 401 030 416  $q^{6733} +$   
 1 092 718 433 147 697 724 264 053 224 763 917 826 743 282 190 904 881 913 062 193 577 451 665 100 437  
 131 778 309 715 681 425 167 026 117 818 047 657 590 801 962 888 148 866 875 169 914 193 753 608 173  
 110 822 300 332 493 992 053 317 225 340 422 240 256 000  $q^{6736} -$   
 1 129 463 570 437 183 828 742 438 543 843 956 817 859 988 025 858 003 594 348 503 953 998 265 858 634  
 468 228 693 021 230 211 966 303 083 334 752 326 061 811 274 348 401 569 895 346 360 410 139 224 175  
 920 218 528 378 211 167 448 204 313 678 368 187 056 128  $q^{6737} +$   
 1 247 262 090 761 719 847 979 522 021 410 396 813 523 336 988 056 342 988 909 863 046 626 076 187 050  
 253 735 668 347 305 282 214 793 849 865 913 444 195 703 909 096 892 445 801 759 241 737 832 861 411  
 926 117 149 639 565 200 801 789 181 745 897 791 590 400  $q^{6740} -$   
 1 289 191 484 139 588 616 407 136 779 469 560 410 592 523 867 507 069 390 500 937 071 376 189 521 587

552 303 317 956 008 575 210 603 059 719 624 345 575 367 300 374 092 992 531 424 527 135 300 324 723 536 396 064 162 781 224 735 978 951 611 203 909 572 625  $q^{6741} +$   
 1 423 607 178 943 487 613 409 849 866 408 997 273 096 555 188 657 294 630 835 421 619 010 527 634 138 822 230 411 243 459 548 806 406 953 775 932 790 584 039 889 646 526 848 686 168 413 444 824 560 180 569 358 325 806 056 599 069 683 853 470 023 016 064 000  $q^{6744} -$   
 1 471 450 393 904 405 700 384 701 176 308 817 257 431 622 757 008 529 583 826 103 073 139 074 493 544 900 155 560 174 066 445 807 450 269 725 831 865 738 930 768 684 600 251 475 757 638 961 740 271 760 141 259 585 809 043 909 829 568 510 558 338 632 908 800  $q^{6745} +$   
 1 624 821 378 797 145 248 472 497 025 269 487 808 107 128 904 520 662 471 526 401 491 970 410 618 819 339 953 207 876 930 321 198 798 981 289 027 062 811 511 683 470 007 546 103 642 926 068 928 881 974 985 059 941 069 278 507 219 391 904 454 959 663 280 128  $q^{6748} -$   
 1 679 410 388 844 527 467 428 815 868 978 846 279 859 614 739 930 654 448 367 416 903 228 323 115 947 869 325 617 691 881 885 381 843 769 862 736 131 304 505 847 341 768 289 610 550 611 461 782 398 138 303 870 500 121 142 294 736 403 873 787 938 389 160 375  $q^{6749} +$   
 1 854 402 925 174 294 263 890 152 268 190 770 540 122 375 183 916 266 240 349 261 739 638 939 619 536 263 440 496 342 628 543 088 819 936 079 167 484 140 972 302 357 771 133 320 774 289 376 094 496 449 841 835 242 250 916 395 225 585 994 147 916 831 215 616  $q^{6752} -$   
 1 916 686 450 061 737 189 554 726 876 292 680 728 811 509 800 731 280 541 663 399 688 525 350 835 795 242 459 896 509 790 247 924 482 409 133 771 735 680 255 908 129 420 171 144 461 952 960 310 189 433 850 295 285 607 001 986 617 511 659 577 988 969 365 504  $q^{6753} +$   
 2 116 340 881 645 413 233 955 366 319 546 718 445 270 856 166 463 996 652 247 236 822 660 468 498 493 550 475 511 704 822 783 338 676 428 511 852 968 454 158 289 512 209 599 253 925 604 788 096 609 152 690 909 133 236 456 939 613 844 233 886 211 999 744 000  $q^{6756} -$   
 2 187 400 728 017 618 063 804 195 330 718 893 109 798 233 761 106 535 565 742 618 501 279 265 276 997 285 523 195 494 432 556 161 501 477 276 948 664 763 503 642 479 111 569 405 825 670 894 995 350 392 797 830 888 155 344 859 965 904 442 797 268 798 272 203  $q^{6757} +$   
 2 415 183 832 129 035 246 096 991 979 261 000 082 173 635 738 797 698 965 405 836 315 512 228 444 026 710 534 191 740 134 824 222 224 629 335 737 985 652 522 065 522 591 957 544 403 557 502 092 902 627 202 144 305 161 295 985 489 242 916 501 461 588 160 000  $q^{6760} -$   
 2 496 253 515 494 627 246 824 917 429 259 624 718 539 410 801 049 017 170 231 151 402 705 993 144 037 619 662 353 840 650 770 631 073 270 522 037 735 611 752 094 522 484 851 949 418 585 209 340 745 593 499 062 407 595 231 260 358 836 254 128 052 572 160 000  $q^{6761} +$   
 2 756 118 161 470 897 830 766 499 539 902 847 047 437 019 120 606 843 380 403 930 348 524 036 952 629 934 184 027 838 458 752 101 617 253 488 135 912 525 045 775 747 516 630 932 959 000 102 591 143 666 338 542 314 642 894 021 650 392 473 194 401 578 112 000  $q^{6764} -$   
 2 848 604 127 195 749 262 109 384 847 374 541 455 408 347 458 773 887 311 361 845 155 928 090 439 157 586 823 148 293 128 277 077 624 310 671 671 028 406 943 707 662 119 487 035 697 802 414 189 306 412 521 322 769 288 469 787 728 695 914 749 793 391 262 675  $q^{6765} +$   
 3 145 057 260 129 693 184 587 188 324 426 906 402 963 279 284 299 504 122 924 757 081 726 503 462 127 726 511 223 439 413 189 039 406 605 952 529 094 416 206 293 432 064 287 100 955 674 661 190 106 339 129 995 331 412 746 938 587 482 434 482 854 171 475 968  $q^{6768} -$   
 3 250 563 065 266 837 523 242 920 993 456 143 787 103 579 118 481 625 680 945 833 693 939 680 369 499 627 743 057 185 326 679 399 636 798 521 377 604 560 878 786 276 000 524 112 980 356 861 466 074 310 335 696 407 585 776 948 941 849 494 761 651 060 736 000  $q^{6769} +$   
 3 588 743 173 559 399 998 175 294 294 463 935 840 076 670 751 434 410 970 847 465 335 218 416 274 554 671 987 706 496 243 027 691 439 162 645 179 597 262 516 625 314 286 228 900 158 940 954 113 300 982 160 471 457 310 143 469 287 548 554 543 335 380 113 408  $q^{6772} -$   
 3 709 097 041 572 910 198 041 921 921 466 874 073 852 056 642 929 808 145 078 522 613 537 529 013 814 854 500 611 482 232 594 394 619 420 033 647 929 736 114 721 210 870 185 141 384 418 090 848 787 980 510 288 878 650 395 269 893 060 367 508 537 961 063 480  $q^{6773} +$   
 4 094 862 428 000 017 920 413 812 453 691 531 896 661 360 679 686 966 434 064 157 606 542 110 098 759 044 633 096 027 624 705 298 731 670 385 880 565 101 921 956 913 159 919 451 284 974 049 539 464 015 882 555 122 355 255 999 145 946 910 886 849 731 200 000  $q^{6776} -$   
 4 232 148 645 640 218 141 047 931 318 671 010 257 228 285 785 924 014 499 977 304 089 166 777 267 639 006 236 096 227 008 715 119 438 505 209 520 853 248 716 028 528 366 912 312 149 436 464 547 041 407

$062\ 757\ 576\ 886\ 273\ 616\ 508\ 990\ 884\ 126\ 260\ 571\ 799\ 552\ q^{6777} +$   
 $4\ 672\ 178\ 004\ 748\ 495\ 246\ 524\ 532\ 481\ 944\ 801\ 604\ 576\ 661\ 794\ 855\ 754\ 173\ 936\ 084\ 817\ 500\ 902\ 809\ 056\ q^{6778} -$   
 $640\ 787\ 010\ 647\ 070\ 135\ 405\ 430\ 600\ 578\ 118\ 434\ 125\ 269\ 569\ 793\ 793\ 391\ 651\ 162\ 303\ 275\ 446\ 825\ 454\ q^{6779} -$   
 $532\ 755\ 808\ 553\ 929\ 325\ 652\ 655\ 399\ 622\ 207\ 812\ 812\ 800\ q^{6780} -$   
 $4\ 828\ 772\ 695\ 455\ 958\ 820\ 892\ 071\ 546\ 250\ 690\ 479\ 680\ 602\ 690\ 237\ 613\ 885\ 092\ 747\ 171\ 781\ 146\ 615\ 290\ q^{6781} +$   
 $165\ 803\ 107\ 762\ 267\ 033\ 145\ 680\ 330\ 595\ 649\ 290\ 001\ 368\ 331\ 102\ 901\ 391\ 436\ 079\ 731\ 008\ 760\ 089\ 438\ q^{6782} -$   
 $934\ 110\ 953\ 810\ 617\ 700\ 617\ 546\ 370\ 177\ 866\ 404\ 152\ 000\ q^{6783} +$   
 $5\ 330\ 679\ 708\ 618\ 629\ 246\ 432\ 537\ 679\ 234\ 123\ 861\ 890\ 662\ 692\ 889\ 188\ 261\ 423\ 729\ 825\ 514\ 271\ 005\ 706\ q^{6784} -$   
 $238\ 411\ 113\ 672\ 095\ 281\ 413\ 414\ 784\ 565\ 926\ 082\ 758\ 308\ 516\ 960\ 954\ 130\ 333\ 357\ 006\ 341\ 025\ 277\ 875\ q^{6785} -$   
 $829\ 333\ 853\ 281\ 756\ 155\ 881\ 138\ 108\ 322\ 799\ 915\ 008\ 000\ q^{6786} +$   
 $5\ 509\ 291\ 590\ 968\ 441\ 331\ 091\ 407\ 739\ 405\ 179\ 250\ 004\ 554\ 527\ 284\ 453\ 931\ 441\ 976\ 591\ 751\ 217\ 204\ 618\ q^{6787} -$   
 $056\ 094\ 998\ 141\ 116\ 503\ 271\ 674\ 074\ 054\ 232\ 892\ 434\ 907\ 575\ 466\ 636\ 501\ 419\ 252\ 226\ 550\ 535\ 509\ 674\ q^{6788} +$   
 $134\ 496\ 467\ 341\ 766\ 577\ 920\ 327\ 217\ 772\ 264\ 821\ 555\ 200\ q^{6789} -$   
 $6\ 081\ 755\ 487\ 808\ 123\ 363\ 100\ 540\ 885\ 470\ 584\ 036\ 794\ 985\ 686\ 735\ 082\ 874\ 245\ 938\ 110\ 228\ 251\ 975\ 344\ q^{6790} -$   
 $511\ 448\ 898\ 064\ 283\ 815\ 376\ 846\ 199\ 819\ 291\ 200\ 495\ 571\ 058\ 974\ 418\ 445\ 621\ 787\ 847\ 258\ 213\ 768\ 935\ q^{6791} -$   
 $834\ 435\ 640\ 948\ 115\ 394\ 514\ 144\ 059\ 667\ 079\ 496\ 515\ 584\ q^{6792} -$   
 $6\ 285\ 472\ 311\ 898\ 401\ 248\ 381\ 142\ 589\ 915\ 495\ 142\ 516\ 034\ 595\ 750\ 953\ 026\ 646\ 853\ 822\ 114\ 068\ 705\ 080\ q^{6793} +$   
 $922\ 060\ 052\ 932\ 884\ 167\ 005\ 942\ 618\ 840\ 740\ 280\ 732\ 548\ 905\ 336\ 276\ 308\ 491\ 345\ 787\ 176\ 422\ 951\ 144\ q^{6794} +$   
 $648\ 068\ 669\ 354\ 753\ 697\ 426\ 130\ 489\ 593\ 608\ 884\ 906\ 250\ q^{6795} +$   
 $6\ 938\ 386\ 617\ 001\ 195\ 381\ 597\ 615\ 127\ 537\ 663\ 632\ 800\ 148\ 115\ 061\ 248\ 089\ 101\ 825\ 767\ 704\ 984\ 151\ 721\ q^{6796} -$   
 $581\ 750\ 967\ 439\ 261\ 189\ 448\ 830\ 285\ 585\ 543\ 275\ 539\ 211\ 016\ 994\ 500\ 472\ 736\ 946\ 908\ 327\ 634\ 037\ 140\ q^{6797} -$   
 $305\ 060\ 717\ 644\ 248\ 094\ 012\ 247\ 642\ 060\ 098\ 552\ 014\ 848\ q^{6798} -$   
 $7\ 170\ 728\ 067\ 756\ 806\ 909\ 231\ 487\ 567\ 709\ 258\ 093\ 830\ 270\ 067\ 564\ 318\ 700\ 800\ 726\ 652\ 003\ 418\ 442\ 005\ q^{6799} -$   
 $232\ 351\ 814\ 847\ 257\ 443\ 560\ 497\ 504\ 548\ 046\ 148\ 374\ 117\ 221\ 496\ 988\ 560\ 647\ 020\ 716\ 223\ 933\ 874\ 226\ q^{6800} +$   
 $517\ 585\ 486\ 948\ 555\ 289\ 484\ 426\ 645\ 256\ 182\ 022\ 438\ 912\ q^{6801} +$   
 $7\ 915\ 370\ 059\ 194\ 497\ 415\ 452\ 441\ 708\ 519\ 389\ 894\ 168\ 212\ 428\ 253\ 904\ 815\ 889\ 159\ 036\ 400\ 432\ 610\ 695\ q^{6802} -$   
 $918\ 605\ 212\ 052\ 719\ 852\ 164\ 764\ 634\ 739\ 688\ 209\ 571\ 364\ 681\ 745\ 963\ 699\ 257\ 947\ 500\ 772\ 004\ 269\ 685\ q^{6803} -$   
 $322\ 827\ 749\ 493\ 576\ 244\ 376\ 927\ 878\ 497\ 684\ 378\ 304\ 000\ q^{6804} -$   
 $8\ 180\ 348\ 024\ 909\ 184\ 811\ 021\ 593\ 333\ 574\ 229\ 176\ 865\ 754\ 821\ 426\ 040\ 627\ 301\ 642\ 919\ 003\ 543\ 357\ 425\ q^{6805} -$   
 $748\ 614\ 534\ 284\ 242\ 836\ 172\ 417\ 631\ 065\ 756\ 369\ 519\ 857\ 637\ 587\ 884\ 251\ 232\ 968\ 147\ 907\ 130\ 090\ 727\ q^{6806} +$   
 $970\ 492\ 107\ 647\ 609\ 060\ 452\ 920\ 660\ 191\ 609\ 276\ 546\ 092\ q^{6807} +$   
 $9\ 029\ 571\ 781\ 209\ 836\ 183\ 494\ 993\ 722\ 811\ 303\ 769\ 228\ 873\ 482\ 085\ 112\ 773\ 416\ 561\ 955\ 703\ 047\ 766\ 408\ q^{6808} -$   
 $813\ 886\ 713\ 595\ 955\ 281\ 914\ 526\ 344\ 559\ 797\ 408\ 930\ 827\ 823\ 412\ 174\ 391\ 994\ 192\ 222\ 079\ 388\ 166\ 065\ q^{6809} -$   
 $749\ 539\ 664\ 522\ 358\ 086\ 713\ 082\ 478\ 839\ 218\ 978\ 816\ 000\ q^{6810} -$   
 $9\ 331\ 759\ 010\ 120\ 138\ 688\ 495\ 424\ 927\ 664\ 462\ 020\ 402\ 190\ 108\ 932\ 112\ 673\ 397\ 804\ 492\ 001\ 816\ 724\ 369\ q^{6811} +$   
 $541\ 018\ 584\ 618\ 574\ 631\ 576\ 810\ 815\ 806\ 572\ 626\ 796\ 222\ 514\ 919\ 834\ 902\ 460\ 803\ 518\ 865\ 192\ 683\ 263\ q^{6812} +$   
 $147\ 941\ 557\ 826\ 880\ 366\ 602\ 261\ 880\ 452\ 808\ 650\ 752\ 000\ q^{6813} +$   
 $10\ 300\ 215\ 320\ 847\ 764\ 606\ 867\ 226\ 014\ 969\ 606\ 463\ 182\ 606\ 054\ 173\ 797\ 660\ 816\ 695\ 817\ 586\ 950\ 323\ q^{6814} -$   
 $497\ 989\ 894\ 033\ 015\ 502\ 920\ 472\ 967\ 768\ 708\ 041\ 489\ 167\ 385\ 600\ 594\ 445\ 497\ 004\ 720\ 939\ 725\ 692\ 144\ q^{6815} -$   
 $750\ 062\ 081\ 936\ 444\ 602\ 668\ 228\ 299\ 098\ 348\ 463\ 337\ 984\ 000\ q^{6816} -$   
 $10\ 644\ 823\ 630\ 204\ 989\ 868\ 956\ 590\ 436\ 023\ 193\ 794\ 059\ 877\ 477\ 353\ 609\ 445\ 392\ 220\ 665\ 191\ 601\ 149\ q^{6817} -$   
 $078\ 724\ 744\ 027\ 640\ 409\ 594\ 218\ 673\ 615\ 169\ 426\ 296\ 335\ 446\ 997\ 900\ 504\ 110\ 997\ 425\ 626\ 050\ 372\ 287\ q^{6818} +$   
 $407\ 134\ 495\ 265\ 944\ 850\ 853\ 648\ 445\ 132\ 541\ 985\ 310\ 243\ 100\ q^{6819} +$   
 $11\ 749\ 210\ 498\ 899\ 175\ 101\ 701\ 915\ 565\ 577\ 310\ 284\ 042\ 473\ 542\ 429\ 257\ 374\ 377\ 943\ 462\ 916\ 458\ 217\ q^{6820} -$   
 $824\ 887\ 844\ 248\ 592\ 458\ 703\ 938\ 190\ 720\ 007\ 495\ 044\ 983\ 151\ 948\ 453\ 001\ 481\ 510\ 042\ 341\ 479\ 645\ 506\ q^{6821} -$   
 $412\ 850\ 616\ 838\ 307\ 779\ 737\ 160\ 731\ 735\ 420\ 506\ 198\ 023\ 168\ q^{6822} -$   
 $12\ 142\ 179\ 862\ 252\ 705\ 293\ 205\ 849\ 993\ 981\ 778\ 079\ 406\ 807\ 910\ 952\ 609\ 741\ 644\ 295\ 298\ 979\ 905\ 000\ q^{6823} +$   
 $192\ 545\ 582\ 780\ 892\ 921\ 081\ 728\ 324\ 366\ 038\ 149\ 161\ 502\ 971\ 865\ 892\ 555\ 499\ 613\ 175\ 911\ 415\ 057\ 414\ q^{6824} +$   
 $780\ 607\ 150\ 679\ 219\ 895\ 446\ 585\ 631\ 184\ 260\ 048\ 646\ 144\ 000\ q^{6825} +$   
 $13\ 401\ 527\ 846\ 729\ 652\ 321\ 987\ 705\ 358\ 343\ 644\ 976\ 986\ 724\ 311\ 862\ 899\ 176\ 860\ 347\ 084\ 672\ 798\ 314\ q^{6826} -$   
 $661\ 992\ 312\ 961\ 712\ 913\ 457\ 165\ 448\ 897\ 104\ 034\ 241\ 234\ 368\ 969\ 858\ 536\ 257\ 136\ 819\ 797\ 540\ 235\ 876\ q^{6827} -$   
 $802\ 076\ 508\ 239\ 239\ 656\ 289\ 511\ 683\ 462\ 166\ 058\ 208\ 090\ 112\ q^{6828} -$   
 $13\ 849\ 627\ 868\ 653\ 696\ 685\ 251\ 788\ 873\ 443\ 638\ 162\ 656\ 049\ 256\ 651\ 043\ 494\ 016\ 255\ 888\ 404\ 662\ 874\ q^{6829} -$   
 $180\ 765\ 728\ 236\ 988\ 456\ 869\ 095\ 582\ 042\ 131\ 618\ 786\ 848\ 116\ 005\ 783\ 589\ 667\ 919\ 467\ 295\ 165\ 799\ 611\ q^{6830} +$   
 $200\ 575\ 022\ 374\ 812\ 166\ 799\ 072\ 305\ 271\ 176\ 160\ 586\ 896\ 003\ q^{6831} +$

15 285 625 091 215 335 119 348 426 162 861 368 197 810 384 118 683 733 250 890 382 171 567 251 602 \\  
 080 220 197 129 352 277 071 318 812 905 858 567 486 911 335 689 484 951 926 304 131 606 927 380 636 \\  
 384 878 992 811 831 943 530 395 690 533 212 331 878 400 000  $q^{6816}$  -

15 796 570 587 570 295 740 747 112 529 929 397 200 890 157 721 357 891 838 593 681 812 475 522 948 \\  
 040 888 146 366 537 609 365 608 648 163 695 950 069 473 898 048 766 577 608 093 307 152 765 072 204 \\  
 348 282 596 999 967 324 554 705 006 952 383 943 284 883 456  $q^{6817}$  +

17 433 932 916 328 742 720 514 443 459 834 461 548 715 789 951 483 796 541 807 212 728 722 772 126 \\  
 011 995 112 325 644 580 193 525 356 118 209 306 272 763 811 423 052 251 154 443 591 081 914 884 247 \\  
 402 573 216 524 477 353 954 318 838 896 068 490 885 529 600  $q^{6820}$  -

18 016 515 555 837 761 266 456 941 440 343 820 914 903 858 155 012 254 480 097 807 185 718 995 703 \\  
 093 772 934 776 109 337 259 597 567 342 668 113 870 876 716 444 806 842 071 818 851 752 019 024 302 \\  
 733 411 186 160 639 037 631 594 692 949 267 803 300 757 125  $q^{6821}$  +

19 883 408 219 308 882 637 140 103 114 630 903 601 898 534 323 148 074 907 182 122 378 350 024 562 \\  
 396 929 046 507 263 534 856 359 950 180 052 271 527 098 621 968 186 693 777 668 922 810 700 016 170 \\  
 774 051 661 466 613 117 142 199 089 115 606 381 954 496 000  $q^{6824}$  -

20 547 646 452 719 477 682 723 368 520 505 143 322 188 965 321 273 786 853 161 007 871 652 968 229 \\  
 363 431 005 538 479 547 589 564 354 684 591 290 441 284 189 737 624 737 979 054 279 480 946 950 495 \\  
 793 781 199 533 361 953 547 539 860 993 913 392 370 483 200  $q^{6825}$  +

22 676 164 215 776 263 836 933 473 169 624 860 306 594 059 560 297 867 168 928 400 575 974 610 253 \\  
 040 248 054 660 230 875 871 096 220 318 148 464 537 937 509 827 702 559 706 996 389 311 646 240 653 \\  
 754 559 901 611 449 578 138 520 090 754 142 845 012 071 424  $q^{6828}$  -

23 433 474 026 681 030 229 282 075 406 036 567 297 617 830 516 366 192 307 383 572 399 512 177 090 \\  
 046 137 423 142 980 937 881 298 632 330 226 096 225 385 356 809 717 659 636 662 832 571 488 022 580 \\  
 665 360 390 295 131 630 165 813 162 562 421 569 180 452 750  $q^{6829}$  +

25 860 188 041 334 250 111 989 534 377 903 256 519 096 561 299 951 255 581 905 459 524 918 447 480 \\  
 546 005 066 400 406 176 024 919 011 880 365 060 645 881 497 082 085 876 501 165 215 875 118 561 271 \\  
 628 077 235 528 128 857 612 354 728 997 192 366 114 299 904  $q^{6832}$  -

26 723 577 402 978 022 538 600 368 342 840 014 290 884 798 686 961 415 428 655 006 585 819 955 786 \\  
 309 504 354 241 693 452 981 151 569 422 425 758 529 424 518 286 708 788 138 026 459 075 901 682 574 \\  
 569 487 698 089 672 398 832 190 289 991 509 885 962 846 208  $q^{6833}$  +

29 490 157 968 700 988 900 974 221 725 376 859 478 639 323 232 432 740 548 528 440 708 017 525 008 \\  
 930 441 527 635 466 641 173 981 023 228 304 747 012 808 233 121 173 998 081 971 617 774 546 082 601 \\  
 021 398 569 585 843 174 475 360 272 083 939 639 423 232 000  $q^{6836}$  -

30 474 448 289 644 082 408 531 977 665 151 341 396 568 826 548 614 422 801 421 387 352 513 096 945 \\  
 424 083 913 637 151 611 384 739 449 188 227 942 537 412 323 382 289 796 813 709 533 218 277 230 269 \\  
 698 499 568 236 415 075 981 792 947 809 264 769 041 469 750  $q^{6837}$  +

33 628 374 033 768 344 840 548 471 191 989 528 961 982 582 931 841 086 082 274 228 544 372 729 479 \\  
 000 063 230 840 199 625 587 999 777 184 385 820 627 580 287 383 409 229 272 169 395 510 072 336 251 \\  
 258 974 751 628 874 992 089 987 216 293 769 591 884 928 000  $q^{6840}$  -

34 750 452 328 747 136 874 873 098 648 053 116 075 752 909 115 106 941 248 487 859 640 970 641 106 \\  
 791 620 926 057 468 295 302 211 150 662 954 164 261 810 284 289 311 757 465 882 260 200 957 472 931 \\  
 207 561 285 361 904 685 203 643 826 149 277 438 234 624 000  $q^{6841}$  +

38 345 817 769 078 374 742 901 505 002 021 366 643 344 470 390 169 168 161 461 556 041 384 627 283 \\  
 128 387 461 030 016 550 745 607 027 506 773 403 423 301 237 354 150 966 761 091 177 253 202 433 916 \\  
 728 454 133 698 998 216 293 634 331 675 991 653 715 712 000  $q^{6844}$  -

39 624 923 807 357 163 619 299 452 130 284 441 970 805 687 907 745 788 697 872 145 671 253 599 798 \\  
 865 390 330 147 368 343 600 771 033 845 280 714 112 212 790 597 393 630 929 480 542 542 399 637 163 \\  
 663 651 217 554 633 517 928 147 698 181 388 284 266 770 855  $q^{6845}$  +

43 723 358 910 762 058 122 571 087 866 979 866 551 709 389 084 481 660 873 194 374 037 696 849 107 \\  
 479 671 062 437 504 793 376 897 425 385 677 822 461 234 450 389 544 129 640 616 680 892 206 230 128 \\  
 395 279 910 071 882 482 809 288 990 097 163 109 016 109 056  $q^{6848}$  -

45 181 412 181 290 951 978 128 208 159 763 201 003 362 584 687 759 810 893 403 096 291 338 179 228 \\  
 010 799 795 341 726 250 421 126 004 543 658 622 878 540 493 689 959 724 423 608 705 181 191 656 862 \\  
 166 115 795 697 215 273 638 353 042 313 942 901 071 872 000  $q^{6849}$  +

49 853 129 411 066 424 523 976 636 319 311 401 558 750 288 279 780 710 524 920 543 314 263 767 277 \

614 934 185 349 201 158 399 433 884 241 905 155 293 027 189 562 345 319 814 313 777 563 323 053 276 \
 430 425 704 328 264 111 601 486 360 362 840 124 399 042 560 q<sup>6852</sup> -

51 515 101 411 613 313 839 940 460 537 854 639 706 656 457 280 594 267 537 210 826 413 412 122 699 \
 515 685 688 103 860 517 762 034 407 694 859 374 991 534 694 237 420 733 113 863 259 462 075 608 268 \
 629 031 424 319 193 936 265 790 495 186 064 592 919 321 408 q<sup>6853</sup> +

56 840 087 894 215 908 670 683 585 335 121 533 049 753 080 719 932 507 725 750 232 067 115 498 936 \
 689 218 609 686 999 227 720 223 110 737 047 309 975 275 171 238 748 652 782 617 286 015 863 670 661 \
 744 054 374 970 049 799 157 059 376 785 021 425 342 592 000 q<sup>6856</sup> -

58 734 426 011 428 860 426 308 387 557 282 378 847 914 818 258 980 765 467 075 327 716 327 020 187 \
 586 970 771 380 656 061 444 987 973 850 820 116 520 104 084 094 950 974 968 842 423 063 395 863 879 \
 181 339 782 126 066 006 921 944 434 327 888 288 020 660 224 q<sup>6857</sup> +

64 803 800 885 142 519 448 752 526 307 651 856 440 485 049 353 315 305 198 706 752 745 659 200 885 \
 368 608 412 319 390 453 794 466 909 738 446 316 726 379 070 610 048 009 267 562 360 261 137 071 550 \
 101 167 719 811 284 152 085 437 066 436 093 891 617 382 400 q<sup>6860</sup> -

66 962 910 996 845 813 638 246 154 177 361 390 946 140 669 282 845 804 254 853 022 021 963 724 704 \
 616 356 884 939 400 718 397 799 707 664 848 579 849 595 266 946 737 993 257 756 222 696 825 066 693 \
 989 693 488 852 211 106 450 007 416 762 053 709 128 875 625 q<sup>6861</sup> +

73 880 470 771 595 966 197 782 574 784 378 496 014 227 245 062 879 446 527 476 233 169 444 536 268 \
 204 095 429 189 717 264 425 952 118 216 540 048 309 011 049 084 176 492 942 088 507 716 270 955 209 \
 587 006 608 318 524 381 029 783 457 066 672 516 595 712 000 q<sup>6864</sup> -

76 341 266 685 881 067 970 061 893 161 875 034 646 911 592 440 290 258 556 136 314 777 063 314 409 \
 061 782 340 496 445 973 301 324 277 913 145 421 994 097 548 618 039 771 853 362 961 348 017 617 249 \
 494 619 447 935 168 079 276 609 956 791 005 059 624 140 800 q<sup>6865</sup> +

84 225 244 590 588 792 522 443 179 274 263 647 735 870 569 206 192 410 466 447 128 304 229 831 015 \
 401 386 030 747 120 344 057 725 484 874 947 336 540 129 781 314 477 956 308 258 472 686 448 292 963 \
 570 721 957 037 426 264 621 612 017 319 753 062 456 557 568 q<sup>6868</sup> -

87 029 773 554 748 599 460 859 666 163 912 083 135 565 321 793 459 031 030 871 921 091 814 747 938 \
 059 498 755 512 911 512 538 831 330 662 726 394 911 707 545 402 723 917 277 849 647 217 176 554 536 \
 564 900 822 222 147 851 009 320 710 941 367 865 346 654 625 q<sup>6869</sup> +

96 014 842 428 575 028 016 016 024 554 262 534 451 565 233 525 665 166 620 193 516 472 671 774 099 \
 555 979 536 862 896 881 542 212 411 388 151 352 757 291 201 841 185 484 022 938 429 593 257 018 297 \
 070 135 997 051 720 963 460 102 452 350 359 999 560 532 480 q<sup>6872</sup> -

99 210 997 213 197 128 589 244 392 914 045 651 559 806 825 681 325 642 914 548 464 656 987 356 350 \
 569 579 354 347 785 498 723 320 454 110 526 321 157 348 109 796 079 493 192 329 041 482 397 838 199 \
 457 300 189 978 436 034 619 905 494 245 003 593 063 530 496 q<sup>6873</sup> +

109 450 549 569 115 739 298 803 060 850 047 505 509 270 139 957 239 825 773 889 406 430 262 122 920 \
 367 698 492 829 305 052 260 924 913 512 291 181 449 301 471 042 160 075 291 502 922 754 190 591 938 \
 592 871 455 895 518 628 847 604 967 422 699 380 252 160 000 q<sup>6876</sup> -

113 092 879 079 788 100 637 288 703 504 716 676 105 113 836 033 179 028 962 041 809 924 673 385 000 \
 204 596 020 609 604 957 791 553 338 734 699 333 046 195 076 148 433 227 972 474 696 763 968 118 276 \
 082 605 235 201 499 653 856 118 807 009 703 624 409 308 855 q<sup>6877</sup> +

124 761 622 600 623 166 979 503 778 942 458 487 318 355 044 163 801 691 389 564 392 577 205 910 335 \
 434 158 313 157 721 398 137 125 403 582 749 257 093 301 621 995 460 105 170 150 565 516 506 517 399 \
 653 949 816 278 766 551 158 344 557 921 168 363 725 004 800 q<sup>6880</sup> -

128 912 254 615 688 632 312 545 060 843 710 334 750 653 892 258 948 144 508 931 921 956 504 369 356 \
 464 732 707 429 023 112 493 639 404 750 444 007 858 348 227 898 092 436 878 790 948 105 852 714 645 \
 985 209 038 374 921 950 512 003 253 531 042 325 037 056 000 q<sup>6881</sup> +

142 209 166 610 783 952 574 643 062 098 453 835 989 824 112 037 719 884 312 819 783 626 921 197 804 \
 704 443 978 714 195 336 177 536 795 184 627 381 773 813 154 057 885 936 546 992 667 490 612 486 444 \
 734 465 974 219 064 199 209 092 784 032 865 668 065 280 000 q<sup>6884</sup> -

146 938 858 115 661 901 217 397 886 856 067 776 364 499 604 132 700 321 579 560 359 720 855 732 672 \
 793 167 187 115 341 181 553 493 726 387 540 063 578 187 142 497 125 651 949 727 720 857 413 968 209 \
 887 333 277 102 988 235 692 867 734 689 026 024 237 473 325 q<sup>6885</sup> +

162 090 548 457 896 372 628 735 658 384 854 062 941 866 140 859 506 474 250 191 529 410 360 600 675 \
 404 789 282 334 677 746 685 243 048 999 202 762 143 724 891 544 190 454 682 730 685 813 121 335 698

990 647 505 951 757 455 176 349 711 194 922 152 287 594 496  $q^{6888}$  -  
 167 479 881 175 650 604 786 902 252 445 364 191 057 235 986 494 809 571 435 692 656 070 467 321 077  
 351 216 079 766 745 807 711 380 206 419 125 985 728 782 335 406 967 510 104 096 279 535 678 025 440  
 183 581 806 037 745 158 339 225 747 578 868 479 184 896 248  $q^{6889}$  +  
 184 744 420 052 717 503 897 255 238 189 927 391 492 961 240 849 439 223 748 307 181 160 249 109 217  
 972 119 434 784 289 295 320 925 677 543 536 195 546 542 827 102 950 760 304 211 823 419 563 179 935  
 633 961 206 534 114 260 084 077 380 899 815 409 671 068 160  $q^{6892}$  -  
 190 885 161 192 002 700 040 192 828 966 014 964 633 077 330 376 282 586 843 351 512 278 325 831 696  
 042 441 464 393 201 494 358 384 665 359 547 218 205 844 781 969 566 155 756 415 017 365 729 529 646  
 543 802 732 656 798 843 308 998 301 193 141 442 031 113 731  $q^{6893}$  +  
 210 556 435 755 384 159 967 107 573 915 632 670 343 439 620 792 615 628 825 283 174 530 598 195 221  
 662 661 316 749 530 907 275 627 023 594 503 994 683 665 026 221 802 297 268 866 132 873 988 762 854  
 706 341 378 408 328 723 443 212 881 541 945 925 464 064 000  $q^{6896}$  -  
 217 553 086 750 674 323 496 138 614 838 202 559 180 000 520 535 525 404 804 437 435 918 818 514 519  
 697 353 972 119 677 174 667 626 782 733 506 922 004 280 052 534 280 629 766 386 461 718 964 887 543  
 106 843 128 976 504 655 628 489 652 227 885 832 085 274 624  $q^{6897}$  +  
 239 965 759 558 629 476 270 858 448 053 063 443 513 186 991 233 574 529 970 935 630 085 347 779 288  
 797 437 633 188 127 196 021 547 556 784 850 408 404 795 573 182 450 855 714 676 070 870 460 402 145  
 310 747 892 769 703 234 242 386 762 780 581 598 138 982 400  $q^{6900}$  -  
 247 937 318 709 212 878 505 519 483 312 527 718 402 134 060 378 420 701 918 756 530 796 525 513 643  
 337 935 888 246 272 157 505 116 323 985 121 989 604 561 516 481 963 364 965 456 421 995 310 031 277  
 555 145 656 231 717 638 994 777 012 690 312 355 364 403 375  $q^{6901}$  +  
 273 472 470 881 904 393 534 781 369 008 040 467 752 013 956 346 141 841 510 770 033 756 955 631 281  
 074 832 929 301 742 850 537 505 204 859 668 706 207 776 749 831 371 043 595 283 574 684 295 328 268  
 967 235 283 803 543 372 461 086 458 501 920 260 155 136 000  $q^{6904}$  -  
 282 554 439 357 224 947 110 067 397 907 471 356 409 752 318 626 593 955 706 952 522 635 872 780 542  
 067 571 321 360 004 996 274 049 652 268 356 154 756 944 577 940 541 397 575 432 708 637 595 141 891  
 628 097 894 432 628 642 099 808 345 258 798 901 621 555 200  $q^{6905}$  +  
 311 645 992 758 252 567 551 415 576 815 888 327 397 202 563 790 861 894 060 624 603 428 149 803 184  
 507 605 413 304 643 332 544 266 151 469 974 339 277 192 399 737 524 291 238 666 186 933 169 945 559  
 395 928 608 334 334 170 990 056 493 653 451 554 364 409 856  $q^{6908}$  -  
 321 992 657 486 549 581 802 556 347 380 903 704 172 258 348 935 770 053 691 805 702 504 157 025 352  
 211 760 028 336 831 716 657 740 662 352 287 830 308 828 325 495 056 984 637 789 471 504 672 061 679  
 416 870 922 185 542 196 284 641 446 993 492 698 017 654 875  $q^{6909}$  +  
 355 134 683 203 636 656 572 482 628 221 039 006 199 651 020 609 017 466 310 827 201 874 984 162 295  
 600 998 527 430 419 060 051 583 367 082 946 239 334 170 566 884 121 169 665 848 658 750 041 266 002  
 069 731 746 994 635 887 328 412 876 765 177 616 251 486 208  $q^{6912}$  -  
 366 921 714 765 265 047 794 209 246 081 359 587 770 092 640 958 804 914 882 186 256 774 283 342 128  
 216 149 082 122 595 357 880 764 127 217 308 682 261 788 534 911 493 734 971 342 995 664 388 214 547  
 245 104 310 901 215 272 433 836 426 670 677 748 133 330 944  $q^{6913}$  +  
 404 676 749 897 302 320 645 857 225 128 555 785 835 931 387 616 977 463 877 318 621 769 041 900 952  
 120 081 642 641 343 326 234 876 565 453 970 669 523 725 649 111 379 364 934 745 112 013 588 640 790  
 715 635 234 651 413 729 433 332 634 159 029 248 536 576 000  $q^{6916}$  -  
 418 104 158 779 495 786 500 027 239 539 397 385 287 396 735 568 620 579 221 781 243 986 405 841 662  
 449 481 706 736 588 577 144 459 599 404 860 658 695 964 889 257 756 706 503 493 572 457 383 532 709  
 873 837 288 929 926 026 076 110 925 461 916 964 520 963 449  $q^{6917}$  +  
 461 112 670 290 375 871 693 977 762 443 833 254 446 048 051 589 352 449 875 821 236 872 442 893 179  
 301 520 701 540 430 211 140 084 604 293 379 721 880 472 842 345 902 787 773 505 659 688 770 516 223  
 470 884 651 320 650 752 494 914 505 520 053 606 223 795 200  $q^{6920}$  -  
 476 408 170 812 789 099 652 011 938 270 428 489 655 331 472 061 800 534 858 263 328 760 389 037 812  
 588 529 299 112 779 451 673 183 459 434 352 835 825 779 662 962 246 569 859 407 616 778 761 354 053  
 250 009 059 000 730 556 326 198 079 402 262 282 424 320 000  $q^{6921}$  +  
 525 399 324 260 363 129 640 199 962 857 494 511 572 474 858 735 949 727 094 398 665 186 357 531 777  
 116 725 759 780 807 635 426 513 957 949 569 664 854 728 706 920 272 357 659 271 952 428 144 037 518  
 870 435 475 722 083 445 770 871 452 043 022 904 126 976 000  $q^{6924}$  -

542 822 162 248 497 308 921 211 585 036 374 497 947 479 122 933 205 791 071 579 467 425 853 693 728 \
 879 879 396 446 374 184 402 176 835 010 449 515 123 532 326 771 374 960 421 469 100 785 686 660 681 \
 567 595 739 557 476 667 803 962 075 820 458 549 204 475 550 q<sup>6925</sup> +

598 626 074 853 061 539 108 849 978 421 589 671 483 219 956 507 679 366 307 109 397 861 305 684 211 \
 803 126 974 434 126 463 186 279 627 100 735 077 129 831 081 940 906 877 193 347 018 197 067 360 253 \
 234 492 819 245 618 954 151 722 929 945 610 232 713 052 160 q<sup>6928</sup> -

618 471 382 830 999 717 651 297 453 050 045 069 997 958 507 407 448 209 388 747 174 637 281 421 054 \
 440 456 314 237 455 218 062 917 514 560 679 807 775 690 148 547 705 158 878 382 768 095 173 507 372 \
 873 285 837 400 364 345 868 638 383 637 990 458 662 912 000 q<sup>6929</sup> +

682 033 064 968 209 602 329 645 790 979 453 160 889 500 975 547 701 535 067 496 159 162 443 228 362 \
 820 607 053 584 756 571 488 899 741 180 838 714 037 744 165 028 529 853 799 240 497 401 758 720 342 \
 609 612 454 061 773 589 850 117 159 037 366 802 040 154 112 q<sup>6932</sup> -

704 636 817 389 498 289 720 128 156 235 009 103 950 104 244 174 314 952 379 774 221 033 774 018 265 \
 723 846 023 858 867 740 052 533 564 743 154 921 207 383 395 903 538 211 705 238 580 239 446 369 002 \
 458 221 750 241 530 417 435 028 168 048 811 672 288 221 435 q<sup>6933</sup> +

777 032 034 582 279 903 722 988 093 165 567 549 219 088 376 036 345 354 950 726 757 879 040 675 999 \
 385 194 638 107 209 368 287 823 477 687 995 485 755 859 022 831 220 662 499 709 042 377 328 864 353 \
 387 823 683 645 863 265 731 749 159 782 922 453 174 592 000 q<sup>6936</sup> -

802 776 685 562 060 835 654 691 339 469 604 898 598 410 502 852 673 199 259 210 778 207 809 604 431 \
 658 167 867 348 258 968 113 824 699 175 016 435 208 635 040 567 750 617 517 188 521 089 054 802 948 \
 358 564 802 406 405 986 039 165 508 850 603 956 034 928 640 q<sup>6937</sup> +

885 230 004 864 843 505 275 432 858 046 701 032 171 558 119 366 835 409 980 074 837 082 908 159 274 \
 123 464 083 487 789 991 578 753 974 607 027 559 516 151 961 050 025 211 525 271 393 153 214 407 023 \
 218 772 015 265 651 880 654 164 093 529 872 913 114 060 800 q<sup>6940</sup> -

914 550 902 180 813 378 450 342 981 792 051 471 892 707 930 962 648 456 388 763 625 139 377 718 204 \
 447 573 686 943 911 633 786 514 818 281 624 352 939 544 401 841 004 849 426 406 852 721 876 476 326 \
 270 009 176 285 029 589 186 032 834 864 229 383 482 303 000 q<sup>6941</sup> +

1 008 456 223 019 761 695 623 866 053 566 644 348 664 056 709 915 152 555 052 188 298 384 756 493 234 \
 091 591 680 993 919 665 487 868 992 429 121 886 857 695 194 445 542 465 641 054 009 935 443 854 220 \
 682 820 416 561 868 014 623 875 605 708 190 267 701 248 000 q<sup>6944</sup> -

1 041 848 904 999 804 883 171 990 844 038 124 843 977 495 060 396 557 413 640 763 230 166 968 601 351 \
 423 486 839 029 249 194 490 466 155 538 386 858 781 270 564 941 350 317 440 868 818 360 786 370 602 \
 235 026 414 508 545 282 609 107 230 343 067 210 932 224 000 q<sup>6945</sup> +

1 148 792 815 648 326 224 317 576 209 849 733 168 739 268 202 213 787 561 195 374 356 535 755 388 214 \
 999 054 009 421 920 147 360 131 153 766 266 947 701 972 724 990 120 229 871 583 975 858 527 714 771 \
 897 069 899 329 932 221 151 787 687 291 080 901 026 856 960 q<sup>6948</sup> -

1 186 821 312 169 571 042 826 663 581 543 029 108 159 691 573 481 985 251 366 000 391 625 215 723 175 \
 642 448 970 657 382 899 628 839 562 343 118 986 814 889 262 757 402 700 467 171 891 601 664 748 813 \
 622 539 883 377 062 616 328 934 115 913 628 820 661 945 625 q<sup>6949</sup> +

1 308 609 659 773 641 399 707 871 375 450 686 048 236 011 612 959 662 174 261 762 011 122 936 004 253 \
 030 859 291 190 106 470 655 787 607 848 315 192 745 510 734 689 996 620 620 402 359 539 495 823 455 \
 238 005 009 486 142 898 611 180 696 098 792 878 814 916 608 q<sup>6952</sup> -

1 351 915 935 200 766 586 309 248 966 066 351 965 027 794 261 282 474 003 224 494 383 939 374 742 415 \
 089 466 333 767 773 775 933 748 599 340 185 687 885 503 024 776 732 337 916 102 891 662 553 946 884 \
 668 300 481 368 771 339 454 885 736 126 908 827 429 765 120 q<sup>6953</sup> +

1 490 604 050 389 724 942 659 151 891 679 046 586 337 868 901 486 287 001 815 036 032 443 826 901 985 \
 499 895 655 659 672 148 715 695 145 729 823 204 399 300 565 337 013 992 894 216 258 396 267 641 360 \
 433 928 645 781 349 430 546 790 453 653 437 411 037 440 000 q<sup>6956</sup> -

1 539 918 745 151 702 235 094 943 949 982 197 256 486 926 811 804 673 884 409 829 283 964 205 507 360 \
 345 895 575 034 873 445 320 900 825 704 649 964 992 820 416 885 647 099 476 442 886 933 107 701 116 \
 295 972 374 155 483 222 556 781 304 757 077 395 115 317 745 q<sup>6957</sup> +

1 697 845 822 647 480 559 589 491 660 445 508 063 880 664 861 112 481 450 319 378 706 469 963 484 432 \
 374 025 920 855 986 967 272 581 873 179 727 249 895 861 746 955 567 678 315 418 890 684 148 593 866 \
 734 800 852 477 084 512 386 718 508 185 620 000 674 201 600 q<sup>6960</sup> -

1 754 000 471 600 695 141 270 018 708 610 390 078 181 185 909 248 013 078 895 793 735 180 591 860 141 \

630 736 145 785 049 995 934 422 811 530 471 170 752 650 931 490 063 598 802 177 643 222 650 329 900  
 661 945 326 961 543 496 474 668 994 311 163 943 047 168 000  $q^{6961} +$   
 1 933 828 676 860 677 591 262 708 471 289 380 406 000 289 537 733 140 578 128 433 803 260 023 841 967  
 261 127 885 739 941 238 600 707 185 466 686 520 226 294 209 329 289 743 272 288 710 655 125 440 710  
 067 210 618 855 518 950 427 555 202 453 730 387 407 104 000  $q^{6964} -$   
 1 997 769 606 963 653 681 628 970 824 133 929 410 039 441 761 449 641 602 985 580 870 130 828 804 397  
 805 163 830 945 609 781 994 970 365 887 487 151 443 749 421 045 696 108 257 258 805 533 298 874 600  
 293 737 553 283 420 372 075 230 502 470 489 739 060 619 875  $q^{6965} +$   
 2 202 528 556 882 574 345 387 045 252 552 238 093 796 549 599 967 179 442 947 456 203 731 365 428 964  
 095 481 402 096 313 487 697 791 032 032 251 398 905 548 065 554 035 341 223 305 685 202 954 991 160  
 303 386 153 205 192 935 656 679 189 759 098 189 722 864 640  $q^{6968} -$   
 2 275 332 694 412 198 596 914 171 774 645 342 025 406 429 634 822 554 066 082 005 971 052 997 024 375  
 943 991 150 459 616 605 127 601 362 237 142 765 416 887 870 830 273 552 030 276 877 577 933 729 784  
 404 485 600 037 202 332 894 602 569 552 774 122 651 648 000  $q^{6969} +$   
 2 508 470 048 742 369 328 600 178 835 411 597 338 560 926 158 114 207 066 877 810 632 186 223 655 824  
 824 814 343 897 289 601 390 006 999 304 786 694 531 293 856 605 009 931 666 622 223 915 002 350 605  
 633 326 634 839 387 467 166 376 389 391 928 459 506 868 224  $q^{6972} -$   
 2 591 362 897 766 585 669 798 784 609 619 503 017 938 438 196 044 227 184 721 789 218 125 754 829 926  
 004 773 469 545 380 201 338 753 073 219 622 765 827 281 536 272 275 303 448 186 129 461 085 138 932  
 000 698 988 083 805 919 672 972 589 905 701 704 710 675 912  $q^{6973} +$   
 2 856 801 898 642 251 663 066 564 876 248 860 174 540 625 775 136 118 504 531 953 496 788 036 353 095  
 572 548 219 483 637 046 904 717 681 296 576 967 754 105 150 801 918 389 914 204 305 814 071 135 567  
 826 141 840 280 171 832 221 197 496 237 961 429 106 688 000  $q^{6976} -$   
 2 951 177 988 244 262 004 613 233 484 480 613 516 225 081 978 604 855 322 419 214 545 383 711 703 768  
 116 857 736 403 385 952 932 379 825 190 290 777 996 751 785 797 285 176 065 795 941 323 359 510 878  
 904 387 441 805 233 980 123 633 466 191 062 140 725 002 240  $q^{6977} +$   
 3 253 382 899 660 728 672 461 132 064 010 564 867 944 027 528 060 184 037 427 602 035 138 843 919 201  
 042 690 591 038 563 574 037 579 341 086 721 651 686 844 021 921 616 574 313 326 458 514 011 131 605  
 147 723 955 560 233 881 027 551 578 384 279 366 617 497 600  $q^{6980} -$   
 3 360 829 038 069 202 684 632 991 562 246 107 465 732 014 962 398 702 139 963 068 203 327 877 948 982  
 336 200 951 035 631 063 151 526 618 358 981 932 779 166 581 289 545 400 744 473 899 198 229 148 177  
 548 026 976 813 465 137 036 073 577 755 244 161 079 005 500  $q^{6981} +$   
 3 704 879 567 239 689 495 566 363 537 765 842 875 424 810 810 092 069 805 887 668 396 046 857 926 521  
 883 434 381 698 315 957 966 167 813 767 058 675 132 079 128 872 199 503 058 882 662 456 947 451 321  
 749 018 211 609 965 327 149 440 855 963 252 271 335 552 000  $q^{6984} -$   
 3 827 201 287 222 117 671 378 225 037 053 876 578 307 647 793 224 072 906 352 992 914 865 875 874 095  
 701 818 510 627 353 128 872 629 280 205 928 013 225 286 997 130 649 425 237 680 362 736 143 483 474  
 017 737 648 719 351 190 615 331 256 806 847 269 049 139 200  $q^{6985} +$   
 4 218 877 217 537 862 387 803 601 908 467 309 322 380 255 080 138 314 403 712 616 754 378 056 287 575  
 609 998 520 597 613 914 080 681 311 787 562 989 250 409 965 250 726 224 032 679 245 178 501 532 596  
 997 783 787 334 886 571 657 317 162 899 167 041 397 862 912  $q^{6988} -$   
 4 358 128 849 913 800 273 603 505 578 955 031 600 304 983 198 380 243 282 713 663 983 761 303 673 230  
 988 440 551 782 034 225 523 987 223 672 909 483 666 828 266 686 901 744 479 086 431 802 623 746 047  
 459 802 558 070 605 527 945 382 245 625 016 255 302 814 250  $q^{6989} +$   
 4 804 006 283 176 552 615 224 225 774 392 090 490 163 716 890 636 702 868 308 275 560 854 492 741 180  
 815 726 017 142 027 755 842 501 704 319 822 506 303 807 643 416 649 575 881 865 694 896 787 817 481  
 770 591 613 349 259 686 746 504 045 506 579 191 330 734 080  $q^{6992} -$   
 4 962 525 154 960 177 902 593 690 872 791 089 612 720 602 725 597 183 057 030 613 329 747 869 462 592  
 968 483 536 407 497 295 943 276 615 480 631 967 074 761 356 909 356 406 436 512 232 235 432 455 781  
 054 981 975 596 280 770 083 424 001 642 076 157 543 710 720  $q^{6993} +$   
 5 470 085 951 378 655 928 497 833 711 520 874 003 233 130 458 651 402 266 556 997 545 890 540 741 378  
 034 169 872 729 867 056 834 097 585 071 005 537 288 179 780 356 298 378 632 344 063 303 861 177 807  
 281 026 361 802 967 149 004 254 668 535 808 145 091 584 000  $q^{6996} -$   
 5 650 531 272 837 965 326 630 769 455 295 337 851 445 321 147 187 934 252 653 320 513 695 199 938 077  
 224 129 955 076 591 451 171 344 039 676 898 654 253 408 791 070 990 644 430 653 886 660 538 364 094

606 438 023 360 095 972 044 872 804 873 231 824 594 005 445  $q^{6997} +$   
 6 228 287 494 090 088 528 848 126 150 736 752 103 490 186 504 100 130 022 550 549 715 808 988 762 895 \\  
 210 501 389 909 311 632 938 874 382 989 681 911 140 726 335 028 405 587 522 661 602 493 797 189 788 \\  
 042 254 550 296 533 176 776 419 645 269 358 816 325 888 000  $q^{7000} -$   
 6 433 684 576 017 167 405 881 486 338 111 776 358 296 729 010 572 215 007 861 669 574 018 441 122 973 \\  
 391 206 416 974 028 878 920 479 368 762 257 258 987 872 396 250 028 750 439 345 305 841 326 846 881 \\  
 274 133 065 840 594 625 116 760 176 664 258 113 413 120 000  $q^{7001} +$   
 7 091 319 983 008 340 339 841 364 858 228 636 251 815 207 289 038 010 126 300 881 114 449 657 385 018 \\  
 401 107 251 229 824 374 069 637 241 115 493 586 496 373 712 601 076 096 962 752 772 509 272 647 130 \\  
 837 740 440 703 880 963 151 278 569 154 792 675 303 424 000  $q^{7004} -$   
 7 325 110 512 985 036 092 564 578 084 338 517 390 842 026 806 045 578 744 352 962 337 327 609 995 646 \\  
 315 944 027 134 881 828 329 298 352 850 251 670 714 963 081 293 983 325 843 277 750 728 240 734 463 \\  
 241 650 443 243 788 227 732 086 255 766 628 808 256 763 050  $q^{7005} +$   
 8 073 641 449 788 255 041 135 247 791 058 531 571 100 438 055 725 584 412 531 390 094 779 194 114 837 \\  
 638 215 342 946 643 471 850 810 281 986 136 896 831 220 991 121 087 046 556 992 756 593 700 005 191 \\  
 734 313 601 386 241 323 284 826 505 000 227 286 398 517 248  $q^{7008} -$   
 8 339 740 655 627 715 491 039 998 932 522 078 732 308 478 257 311 722 825 659 410 638 647 904 099 672 \\  
 474 312 731 872 782 652 322 568 289 001 286 420 624 167 596 347 334 063 038 878 012 236 236 668 096 \\  
 337 355 311 842 337 765 362 663 820 018 574 303 039 488 000  $q^{7009} +$   
 9 191 698 969 025 702 407 570 758 940 723 695 515 261 738 826 094 407 665 994 344 927 424 253 008 377 \\  
 106 035 021 525 299 887 076 414 575 601 199 270 490 666 296 344 510 647 500 908 341 936 982 078 423 \\  
 689 517 152 824 375 409 496 118 404 314 188 656 923 918 336  $q^{7012} -$   
 9 494 560 610 488 848 724 808 848 341 967 207 029 811 146 151 978 119 879 351 824 686 586 220 216 117 \\  
 900 969 329 528 940 129 767 556 860 215 938 390 860 202 894 877 108 075 316 024 525 975 215 977 995 \\  
 271 945 952 810 685 205 258 729 951 308 263 640 351 205 783  $q^{7013} +$   
 10 464 201 615 720 137 349 190 127 908 739 299 808 685 588 336 509 631 493 348 266 308 587 553 269 \\  
 034 991 695 078 198 000 144 413 407 956 359 890 920 317 150 497 121 838 166 558 267 312 729 323 814 \\  
 025 191 853 797 856 961 448 543 204 151 367 764 933 874 496 000  $q^{7016} -$   
 10 808 891 873 882 328 019 875 749 788 329 698 208 942 099 638 636 777 708 016 470 331 594 219 582 \\  
 272 133 703 611 027 152 397 095 719 454 411 533 815 927 701 755 758 723 446 530 136 296 846 171 815 \\  
 900 420 222 474 646 839 331 831 303 547 819 417 615 951 822 848  $q^{7017} +$   
 11 912 430 787 490 333 359 900 572 689 911 583 807 973 073 738 451 396 511 237 521 094 026 140 720 \\  
 713 666 472 283 566 109 160 554 470 856 196 194 905 336 527 857 238 743 527 916 202 210 449 309 267 \\  
 806 271 444 291 948 987 713 371 999 884 103 707 401 559 040 000  $q^{7020} -$   
 12 304 712 266 850 759 328 553 362 743 565 746 708 954 822 146 048 986 424 241 688 123 937 188 056 \\  
 308 483 252 939 701 277 058 825 190 232 723 691 763 450 396 536 697 208 304 271 465 528 032 165 152 \\  
 486 339 388 995 230 985 948 696 452 240 112 590 551 101 938 750  $q^{7021} +$   
 13 560 592 993 609 693 088 504 078 129 308 576 258 249 629 670 669 656 961 246 622 786 400 129 465 \\  
 001 369 792 118 915 716 201 826 758 596 780 008 765 785 687 998 753 674 754 498 419 772 147 170 254 \\  
 574 627 049 685 538 136 152 070 619 630 475 913 301 751 808 000  $q^{7024} -$   
 14 007 020 217 559 903 468 921 039 758 021 144 569 907 586 417 558 520 009 570 749 779 178 498 218 \\  
 934 890 867 132 868 135 851 608 030 471 623 182 957 491 496 503 668 423 482 417 258 701 408 556 979 \\  
 610 405 335 132 816 730 479 903 732 735 102 198 966 800 384 000  $q^{7025} +$   
 15 436 220 907 867 769 337 889 206 978 469 989 277 690 365 486 803 852 243 576 720 935 381 893 577 \\  
 855 979 665 920 348 881 316 005 955 880 037 399 362 593 178 678 860 955 787 855 196 159 753 184 041 \\  
 314 835 784 549 111 258 710 984 672 274 828 136 208 659 329 024  $q^{7028} -$   
 15 944 248 876 151 665 014 923 240 484 272 681 028 608 018 826 923 446 668 150 317 389 324 786 936 \\  
 120 776 413 416 096 845 970 186 665 935 335 057 314 719 169 340 273 522 683 459 238 968 473 089 046 \\  
 524 775 770 438 072 963 561 966 995 391 055 711 335 270 865 625  $q^{7029} +$   
 17 570 629 271 625 443 729 504 166 091 469 268 443 714 847 630 722 832 142 715 304 028 746 829 980 \\  
 127 516 659 478 463 713 652 277 291 340 197 108 167 278 503 960 365 897 627 427 729 684 129 769 543 \\  
 548 623 314 207 116 442 480 565 000 606 457 550 946 364 613 632  $q^{7032} -$   
 18 148 736 861 979 807 920 686 812 754 079 299 189 658 527 259 327 170 126 187 607 637 776 779 737 \\  
 660 399 149 089 279 947 599 175 475 669 625 993 762 909 566 321 913 891 491 856 927 956 525 982 611 \\  
 276 210 006 556 691 898 719 504 208 764 654 035 267 273 228 288  $q^{7033} +$

19 999 433 130 009 493 667 419 963 610 071 051 886 256 098 948 299 920 819 341 272 370 563 723 174 \
 436 990 313 430 844 297 555 303 265 710 810 765 329 385 321 170 829 675 360 772 032 579 482 354 461 \
 464 587 207 121 225 103 262 159 050 036 629 618 162 930 688 000  $q^{7036}$  -

20 657 263 368 732 583 377 099 613 263 288 722 029 448 776 416 374 731 503 985 713 478 127 329 829 \
 946 149 880 461 005 413 886 462 205 128 006 672 148 037 176 283 190 699 892 535 653 619 182 698 281 \
 732 175 958 054 604 094 933 227 414 922 285 371 897 653 493 234  $q^{7037}$  +

22 763 136 902 514 976 009 737 759 657 149 672 896 928 192 155 672 128 445 871 663 474 546 196 819 \
 256 474 595 857 625 891 529 036 940 806 289 456 332 845 956 412 521 643 157 203 313 065 064 460 287 \
 203 123 460 257 845 586 122 746 272 234 610 103 505 077 862 400  $q^{7040}$  -

23 511 656 404 199 616 344 180 146 245 990 586 618 714 822 379 140 613 808 947 062 124 214 692 479 \
 205 415 798 928 666 000 151 922 424 758 273 240 199 169 225 257 073 773 728 189 725 425 221 414 301 \
 957 543 344 118 635 622 154 071 394 854 986 093 770 772 480 000  $q^{7041}$  +

25 907 803 945 841 283 589 983 122 040 659 897 655 238 584 870 028 905 376 813 354 801 416 740 633 \
 204 620 073 276 562 837 087 478 694 631 766 254 232 310 778 364 164 095 171 624 981 586 097 671 995 \
 998 351 667 956 972 442 195 525 347 549 556 973 756 270 592 000  $q^{7044}$  -

26 759 484 135 387 915 384 045 243 075 521 043 974 882 238 247 607 751 287 091 963 683 195 702 957 \
 565 703 174 269 298 451 699 650 491 884 643 813 880 312 897 073 442 563 295 107 190 770 525 586 016 \
 664 606 090 606 916 814 284 892 420 008 798 901 402 026 456 600  $q^{7045}$  +

29 485 817 580 298 272 355 309 942 178 341 141 756 320 442 788 020 839 412 953 923 128 880 975 368 \
 056 919 106 829 723 701 868 769 404 405 417 926 424 937 385 049 703 638 683 685 868 135 064 405 122 \
 928 050 191 950 750 546 265 160 972 477 268 890 098 729 519 104  $q^{7048}$  -

30 454 840 665 654 577 136 656 321 519 314 988 170 272 349 417 742 482 387 737 326 270 381 350 169 \
 847 569 298 630 532 833 671 518 354 334 909 199 764 098 994 842 857 425 410 649 053 150 869 490 447 \
 276 580 471 802 338 827 978 696 600 900 989 149 360 816 128 000  $q^{7049}$  +

33 556 746 042 829 259 739 395 911 425 060 282 302 867 230 593 034 411 376 080 346 542 832 403 982 \
 362 112 124 431 021 255 847 334 190 804 456 962 086 015 650 212 429 352 884 251 643 254 868 014 435 \
 908 195 837 794 384 642 668 740 091 781 174 746 546 199 336 960  $q^{7052}$  -

34 659 239 110 432 028 795 992 291 195 613 579 963 354 978 677 189 409 772 259 577 343 501 264 436 \
 201 964 883 528 179 773 415 366 425 181 931 415 852 266 822 366 745 193 130 822 779 448 548 041 977 \
 956 269 300 063 805 214 823 439 808 262 531 471 279 870 508 536  $q^{7053}$  +

38 188 325 523 723 737 552 492 999 401 812 838 577 719 498 143 057 028 960 573 717 569 520 265 535 \
 019 320 578 955 023 303 396 996 822 211 558 144 019 434 767 624 432 635 033 477 182 891 942 026 872 \
 673 322 025 838 383 454 631 097 542 053 395 180 496 294 218 752  $q^{7056}$  -

39 442 626 586 866 991 759 792 406 035 156 138 653 086 703 317 744 918 914 169 232 586 371 738 484 \
 129 582 224 548 774 361 563 424 555 166 179 916 978 339 147 670 899 833 299 401 957 057 793 864 264 \
 723 792 848 932 887 959 649 100 088 571 840 929 940 264 878 080  $q^{7057}$  +

43 457 577 367 805 589 994 332 739 316 247 472 321 207 408 189 383 045 049 270 264 178 092 558 013 \
 410 376 725 758 800 294 205 799 369 605 844 420 992 045 730 238 329 587 962 806 734 242 830 543 555 \
 978 410 348 163 557 693 778 524 913 260 406 371 724 459 315 200  $q^{7060}$  -

44 884 537 718 528 216 136 367 526 533 905 188 379 651 027 022 238 427 116 341 597 843 539 554 008 \
 802 260 569 673 792 654 686 878 106 627 927 266 151 037 757 228 985 370 941 788 246 419 812 193 878 \
 451 903 677 215 677 704 421 421 046 167 635 053 442 841 112 375  $q^{7061}$  +

49 452 077 705 347 591 383 615 921 178 239 228 435 329 347 717 916 883 570 853 301 254 502 288 593 \
 607 639 409 486 311 526 347 421 820 353 554 715 715 569 737 687 231 994 876 855 078 124 921 458 880 \
 095 110 165 939 591 356 967 716 863 031 797 426 186 376 128 000  $q^{7064}$  -

51 075 405 511 324 259 744 330 137 238 039 493 889 568 975 912 409 737 640 194 294 772 730 681 395 \
 328 724 085 100 518 886 738 687 474 505 030 958 122 233 588 649 881 388 514 905 333 358 360 974 325 \
 109 486 259 637 190 757 408 822 584 803 293 108 277 038 284 800  $q^{7065}$  +

56 271 400 258 436 244 519 746 230 977 883 173 701 980 778 401 588 071 393 316 312 226 361 180 704 \
 905 984 304 582 480 181 150 890 291 342 125 830 200 686 555 752 161 619 052 573 406 331 518 050 027 \
 876 443 583 320 037 120 394 755 957 019 121 561 951 589 330 944  $q^{7068}$  -

58 118 051 017 300 551 027 723 366 664 226 837 543 055 967 615 245 942 248 402 124 387 626 451 724 \
 634 631 074 982 941 461 336 116 072 159 285 047 066 516 624 196 882 340 705 835 076 539 529 389 448 \
 756 012 620 755 537 603 648 426 815 318 838 256 774 007 118 500  $q^{7069}$  +

64 028 755 885 004 050 896 561 518 752 181 441 317 214 434 100 722 903 478 768 072 802 102 549 675 \

655 919 793 881 586 871 774 749 911 555 219 031 326 161 562 038 480 425 727 900 147 127 429 301 484  
 435 409 287 310 914 566 943 355 465 071 202 374 683 331 313 664  $q^{7072} -$   
 66 129 376 110 351 710 716 190 865 910 830 786 160 563 548 956 590 475 769 065 230 755 092 288 446  
 087 974 616 214 932 574 079 797 727 901 953 955 698 649 313 006 844 438 637 182 189 175 050 840 655  
 744 234 723 655 453 130 392 902 564 875 502 488 130 997 616 640  $q^{7073} +$   
 72 852 855 620 665 458 855 377 180 559 903 599 949 266 673 121 621 240 556 697 963 738 426 024 659  
 001 451 471 373 497 027 148 594 546 273 038 785 640 620 311 624 471 894 962 117 634 554 607 613 961  
 738 964 520 446 615 242 781 753 871 897 252 507 063 951 360 000  $q^{7076} -$   
 75 242 286 998 955 510 727 599 470 238 546 680 625 668 642 666 929 432 907 839 648 814 544 737 632  
 846 400 927 735 726 995 521 119 121 661 810 423 303 990 337 262 842 870 648 592 672 040 819 247 201  
 273 089 693 968 626 290 487 426 053 906 129 306 020 438 271 983  $q^{7077} +$   
 82 890 027 609 364 958 344 063 280 139 794 663 527 086 693 060 742 488 591 614 225 677 920 095 300  
 491 454 730 627 257 007 125 983 775 412 573 669 389 586 402 481 519 871 361 199 129 178 921 834 966  
 746 506 094 136 190 946 015 725 494 145 959 881 352 737 433 600  $q^{7080} -$   
 85 607 879 848 990 518 360 657 773 071 750 899 327 609 596 856 078 790 099 329 770 183 965 208 075  
 931 157 043 284 643 560 099 094 137 241 716 733 871 016 151 657 442 632 140 314 225 137 493 939 241  
 969 530 990 050 078 443 908 115 441 486 090 445 551 927 296 000  $q^{7081} +$   
 94 306 622 436 141 565 842 662 112 232 673 123 253 105 775 665 936 673 716 217 431 309 175 127 800  
 685 673 113 698 949 090 576 668 808 743 192 378 562 960 841 185 236 447 233 254 008 848 340 464 906  
 462 167 001 863 208 754 544 783 663 957 345 380 052 519 424 000  $q^{7084} -$   
 97 397 924 144 887 995 177 990 652 545 100 466 611 167 826 981 768 047 753 202 947 581 117 618 769  
 155 026 498 436 077 537 780 428 651 123 596 842 120 405 575 619 142 703 855 892 789 586 341 095 926  
 015 721 193 914 684 744 718 255 997 015 531 795 125 919 276 700  $q^{7085} +$   
 107 291 746 055 380 660 017 882 801 868 594 140 169 308 505 958 353 411 077 338 935 069 058 428 624  
 887 023 070 944 872 499 380 921 013 783 327 774 927 032 370 646 547 820 821 132 790 676 559 992 645  
 734 784 940 621 576 619 199 889 424 506 700 977 668 958 875 648  $q^{7088} -$   
 110 807 684 248 266 762 160 733 209 172 119 549 375 419 203 975 928 617 394 489 775 609 192 373 393  
 142 104 670 728 909 546 313 612 231 380 479 181 409 672 929 488 157 921 537 179 965 157 839 709 737  
 218 040 200 615 088 747 174 417 085 399 050 638 547 419 136 000  $q^{7089} +$   
 122 060 364 821 044 600 456 436 032 259 921 727 420 675 082 182 868 249 820 488 921 860 146 444 422  
 342 039 304 535 009 128 162 155 732 101 965 025 531 374 327 267 344 831 979 078 107 880 138 017 189  
 594 669 512 664 109 352 348 893 073 380 585 001 551 748 691 968  $q^{7092} -$   
 126 059 125 097 505 797 190 770 250 009 473 758 196 595 045 034 838 695 673 827 513 269 084 209 405  
 799 580 229 799 387 455 794 668 936 078 359 727 277 505 459 132 515 571 426 580 281 005 996 446 975  
 416 632 822 746 449 564 429 527 342 574 344 963 678 289 738 772  $q^{7093} +$   
 138 856 833 156 966 435 884 521 340 236 483 715 925 340 495 026 742 152 035 465 710 109 935 977 112  
 183 562 247 997 840 080 630 087 805 451 309 996 194 964 450 174 501 488 178 196 643 630 709 262 300  
 136 374 055 924 325 687 962 039 063 261 848 269 099 696 256 000  $q^{7096} -$   
 143 404 554 217 581 868 246 111 462 109 960 291 511 767 157 955 533 473 186 981 839 932 422 344 033  
 637 865 572 935 588 193 489 952 569 811 797 396 910 026 120 983 160 016 826 112 392 197 617 506 107  
 628 251 472 616 688 187 078 948 915 704 472 664 911 963 029 504  $q^{7097} +$   
 157 958 901 252 272 046 922 034 932 252 560 627 250 120 107 938 973 331 446 660 408 734 552 434 897  
 252 238 835 529 080 139 098 299 911 866 938 978 214 954 610 082 866 600 344 378 453 287 919 437 514  
 128 422 646 807 927 256 202 286 321 259 601 175 832 392 140 800  $q^{7100} -$   
 163 130 759 276 962 126 761 615 187 342 557 127 708 582 074 016 209 885 641 170 549 826 621 448 897  
 947 999 779 089 694 665 496 794 530 730 588 965 460 271 670 829 837 157 234 926 336 461 400 780 292  
 643 951 669 754 269 751 583 435 639 147 661 611 450 297 366 125  $q^{7101} +$   
 179 682 267 939 321 801 673 632 853 962 952 195 057 464 064 146 462 553 849 339 662 080 168 859 806  
 267 970 606 608 241 470 757 361 489 385 199 527 995 710 701 922 042 385 872 490 623 808 311 168 823  
 755 089 615 035 104 799 091 134 360 362 993 021 448 568 832 000  $q^{7104} -$   
 185 563 708 450 875 855 872 254 428 640 002 290 411 418 510 721 491 569 234 772 275 658 080 388 085  
 226 116 826 529 723 433 816 270 475 959 338 171 500 538 255 323 756 261 039 710 727 110 726 265 017  
 612 858 195 812 684 632 313 288 072 636 432 480 043 199 692 800  $q^{7105} +$   
 204 385 752 733 980 926 209 463 198 738 215 002 425 258 261 120 933 651 011 370 802 522 535 701 296  
 089 191 637 125 735 140 887 403 298 214 952 385 582 300 406 744 369 154 830 969 515 774 284 416 375

492 186 118 160 490 440 012 192 232 740 969 075 380 869 103 616  $q^{7108}$  -  
 211 073 889 956 641 282 077 294 477 900 171 698 293 705 781 499 892 581 891 706 477 852 336 240 410  
 560 794 819 855 769 911 685 732 708 681 313 317 777 412 653 840 217 006 550 179 644 227 316 618 157  
 722 919 331 810 850 697 714 122 723 791 223 851 150 524 303 000  $q^{7109}$  +  
 232 477 171 032 061 932 869 390 559 512 928 913 273 105 357 616 475 357 991 651 853 229 443 435 079  
 657 839 494 432 001 257 067 389 926 765 914 726 777 334 002 293 313 088 592 447 896 653 787 835 753  
 458 878 654 231 330 047 531 855 972 271 277 844 774 683 199 488  $q^{7112}$  -  
 240 082 377 462 950 633 037 559 793 851 687 386 656 293 590 461 939 249 193 200 349 771 069 366 960  
 222 400 192 916 610 366 027 846 521 958 469 725 132 942 967 094 958 527 239 860 104 677 453 207 146  
 526 753 952 574 497 322 608 500 431 028 251 578 954 206 838 784  $q^{7113}$  +  
 264 420 007 821 982 599 012 734 708 858 736 002 767 027 476 165 454 605 617 350 403 999 674 583 974  
 940 137 169 221 818 913 691 471 083 106 309 446 727 879 702 558 687 819 853 116 500 309 811 651 842  
 224 994 396 311 914 451 904 482 773 690 584 893 580 488 320 000  $q^{7116}$  -  
 273 067 719 806 812 117 754 781 290 342 413 990 567 846 428 405 842 544 525 410 117 290 330 109 693  
 751 549 010 037 503 799 116 065 555 239 253 700 058 784 645 856 192 305 373 336 606 554 663 519 429  
 242 631 762 165 966 140 203 431 080 936 873 309 807 991 573 546  $q^{7117}$  +  
 300 740 998 174 177 080 948 501 257 533 175 227 674 347 820 897 420 426 820 694 616 239 428 274 711  
 974 787 492 527 706 753 781 994 796 893 164 379 201 983 939 778 456 605 521 316 570 050 516 859 704  
 116 600 915 423 224 067 437 687 606 019 841 188 260 913 152 000  $q^{7120}$  -  
 310 573 766 767 171 365 241 693 081 689 557 877 250 177 248 053 399 493 733 445 406 589 141 853 187  
 992 247 228 717 470 331 144 544 929 229 909 882 608 017 933 646 914 258 943 735 651 194 034 594 402  
 952 800 860 632 039 082 152 559 197 106 052 978 271 199 232 000  $q^{7121}$  +  
 342 038 737 409 184 575 402 999 276 888 781 301 805 550 883 545 112 653 755 613 922 601 092 299 721  
 535 031 077 654 249 981 316 745 081 234 290 691 041 927 910 828 920 192 236 157 569 791 478 220 853  
 784 641 929 248 952 570 638 726 487 165 664 483 039 535 616 000  $q^{7124}$  -  
 353 218 557 756 299 864 827 207 849 324 907 264 239 408 554 305 067 981 931 596 356 634 771 878 814  
 032 039 014 757 162 834 236 010 624 888 229 052 437 103 103 689 314 679 261 884 747 926 878 566 560  
 539 989 084 646 400 358 523 110 450 790 235 613 303 252 832 000  $q^{7125}$  +  
 388 993 460 462 968 965 341 565 987 824 833 653 492 551 174 412 026 428 823 491 296 558 429 683 070  
 171 562 416 840 456 040 145 829 667 761 559 739 966 916 819 887 829 601 780 099 940 107 729 371 590  
 701 626 739 576 589 341 591 533 126 039 382 205 836 521 156 096  $q^{7128}$  -  
 401 704 417 440 693 862 731 349 334 926 294 864 507 388 917 472 958 132 611 183 373 859 840 862 791  
 879 483 594 501 748 249 860 921 977 723 044 241 196 111 976 084 126 245 764 167 636 920 214 959 713  
 265 096 368 489 500 115 009 148 307 360 808 737 806 209 024 000  $q^{7129}$  +  
 442 378 148 825 712 552 053 626 641 935 618 309 245 659 414 462 380 657 601 083 101 166 360 715 096  
 021 574 689 978 467 958 129 112 036 668 496 942 349 901 592 800 277 980 696 802 620 620 587 910 396  
 909 329 571 579 368 288 313 539 430 087 496 019 355 098 073 088  $q^{7132}$  -  
 456 829 421 766 797 510 264 583 591 727 863 348 919 771 132 094 487 440 605 105 600 409 733 599 657  
 433 775 211 024 786 204 672 818 389 824 566 853 073 022 263 980 290 478 561 387 658 710 645 642 323  
 931 509 256 370 825 611 102 963 870 264 947 952 454 539 594 295  $q^{7133}$  +  
 503 071 144 830 580 009 993 309 649 426 810 649 611 469 928 492 804 190 081 422 457 688 947 508 210  
 949 170 049 932 266 824 373 259 870 425 270 954 701 498 415 911 952 724 506 387 457 393 085 029 511  
 577 042 701 443 112 755 109 375 763 779 139 034 826 997 760 000  $q^{7136}$  -  
 519 500 419 954 495 698 965 558 781 839 920 422 548 935 949 649 772 090 322 880 311 037 213 786 031  
 199 767 801 308 460 018 123 541 048 991 483 179 967 736 152 714 766 193 887 295 751 337 624 415 205  
 645 034 462 453 089 688 340 992 039 122 773 422 533 297 242 112  $q^{7137}$  +  
 572 070 477 353 730 673 340 641 197 650 722 027 866 593 532 002 308 904 288 990 847 527 726 808 611  
 962 208 826 355 880 826 405 447 532 289 984 934 353 082 963 607 423 633 586 021 982 808 023 837 571  
 160 178 311 368 452 044 139 977 027 061 686 085 515 762 073 600  $q^{7140}$  -  
 590 747 823 085 915 901 777 882 675 120 669 736 474 265 217 138 640 366 200 913 058 991 525 826 174  
 009 177 206 845 703 091 414 713 454 507 168 447 352 936 828 099 997 972 245 299 279 059 708 284 154  
 419 432 305 020 381 712 759 935 935 571 666 296 919 166 612 375  $q^{7141}$  +  
 650 510 130 544 013 464 566 423 620 962 113 035 442 667 661 358 813 987 725 834 111 316 672 454 565  
 515 811 964 834 771 630 481 243 216 385 616 712 731 364 490 264 611 556 227 015 340 802 540 791 318  
 674 416 654 316 024 381 181 707 136 680 005 749 012 641 152 000  $q^{7144}$  -

671 742 398 358 878 824 016 446 069 486 510 419 418 247 079 929 546 597 277 186 969 331 674 390 848  
 484 602 041 035 279 204 699 305 069 279 950 599 412 834 774 198 538 086 425 712 492 644 203 327 495  
 275 476 805 043 919 099 708 057 341 631 780 820 680 916 992 000  $q^{7145} +$   
 739 678 518 470 174 489 589 831 701 573 212 528 296 970 785 199 538 781 450 250 699 057 154 988 703  
 787 531 702 147 316 459 887 016 274 760 776 099 702 946 325 131 267 825 173 616 783 610 991 837 268  
 690 784 660 375 176 047 464 676 259 265 984 066 864 089 329 152  $q^{7148} -$   
 763 814 340 347 268 224 359 570 125 115 848 142 462 015 699 834 772 226 489 547 064 145 307 374 383  
 948 665 689 901 891 000 768 447 910 632 436 523 235 092 984 857 042 492 387 034 333 331 745 351 556  
 983 582 345 920 994 187 961 863 054 282 421 665 327 928 489 875  $q^{7149} +$   
 841 039 464 053 887 852 520 778 185 568 034 929 414 165 243 955 056 128 409 625 791 474 358 262 291  
 207 530 461 076 012 402 268 189 838 985 581 795 377 369 457 170 156 359 215 269 423 898 076 983 275  
 902 741 501 014 899 576 175 952 168 356 326 293 908 831 453 184  $q^{7152} -$   
 868 474 927 229 434 963 508 415 551 051 569 503 297 530 291 601 184 296 794 692 440 733 524 631 603  
 258 836 260 399 345 088 958 293 657 945 012 353 299 313 357 701 431 153 167 998 705 552 821 984 029  
 135 047 925 919 552 822 977 568 896 507 870 154 504 005 812 224  $q^{7153} +$   
 956 256 020 914 199 851 674 984 184 533 482 746 340 287 298 517 491 936 785 999 474 261 499 339 178  
 861 410 075 569 785 390 023 156 221 402 574 899 225 715 727 755 522 418 593 293 361 250 537 450 641  
 065 524 717 721 704 741 515 769 630 085 518 157 908 003 072 000  $q^{7156} -$   
 987 441 111 494 293 740 080 475 914 302 162 939 067 331 474 599 633 731 818 326 332 424 559 810 154  
 634 389 388 677 084 109 385 521 845 061 519 874 020 435 982 266 699 051 524 442 066 641 185 694 952  
 506 435 145 764 893 912 655 974 809 228 656 691 680 912 709 898  $q^{7157} +$   
 1 087 217 522 424 580 185 642 042 825 018 173 833 190 197 225 710 067 429 247 205 617 924 165 684 705  
 642 748 409 103 403 963 929 078 406 452 349 521 493 073 407 259 767 444 082 636 515 485 839 863 822  
 564 942 788 257 537 991 357 243 774 173 616 873 444 175 897 600  $q^{7160} -$   
 1 122 663 441 775 024 037 578 206 736 944 350 796 368 119 617 600 726 672 124 168 560 227 300 214 806  
 790 587 429 184 416 140 035 835 751 297 760 862 994 732 555 322 983 786 436 241 724 404 417 123 441  
 254 488 549 201 186 179 110 897 190 994 713 071 556 018 176 000  $q^{7161} +$   
 1 236 070 294 105 170 658 717 255 722 556 015 352 783 477 073 736 598 093 879 957 305 960 771 293 911  
 345 828 133 744 249 184 366 577 817 785 021 570 940 876 964 278 884 205 868 756 252 110 662 430 243  
 613 559 124 054 339 266 304 163 343 453 419 576 579 104 000 000  $q^{7164} -$   
 1 276 357 765 942 943 323 141 273 865 480 759 834 571 943 585 984 627 644 051 059 555 123 518 572 719  
 064 274 808 351 925 720 275 994 412 535 713 227 417 999 459 980 715 711 028 416 513 437 580 650 491  
 913 913 765 846 903 334 411 654 338 794 659 688 906 362 847 025  $q^{7165} +$   
 1 405 252 524 264 912 064 903 370 144 949 752 530 041 500 655 505 652 235 857 487 770 626 917 151 552  
 972 356 013 391 528 753 461 415 348 576 798 537 032 026 119 440 744 005 046 038 023 206 542 894 176  
 518 853 001 847 764 214 488 696 195 390 963 541 210 734 526 464  $q^{7168} -$   
 1 451 041 226 270 407 831 497 406 470 514 483 604 168 484 724 382 982 533 144 339 376 995 273 634 449  
 753 725 336 018 104 178 126 546 042 367 834 216 347 622 832 413 906 250 627 199 037 236 007 789 284  
 353 636 721 615 739 085 613 822 005 520 402 399 207 157 760 000  $q^{7169} +$   
 1 597 533 854 506 360 594 167 386 027 213 215 591 978 552 025 576 128 272 977 290 470 069 438 691 720  
 835 571 092 277 777 636 216 960 023 644 131 670 365 405 355 377 974 435 219 550 656 557 806 294 594  
 244 439 904 797 837 641 335 361 505 030 232 381 563 135 213 568  $q^{7172} -$   
 1 649 573 126 306 705 609 240 896 867 430 007 839 789 363 757 391 657 706 377 406 534 448 747 426 749  
 525 745 257 021 889 375 221 608 381 551 958 234 540 054 968 003 233 661 172 597 743 332 518 313 833  
 529 600 739 509 084 707 723 292 392 002 270 094 197 250 995 696  $q^{7173} +$   
 1 816 060 327 370 722 190 587 243 404 995 297 344 634 922 907 404 999 898 814 429 206 452 827 416 306  
 843 146 001 183 255 484 611 623 295 572 947 367 044 738 160 689 215 950 261 902 332 975 295 519 112  
 180 584 344 458 729 980 065 470 236 916 783 933 104 735 232 000  $q^{7176} -$   
 1 875 201 327 199 213 302 589 475 002 476 514 750 319 540 077 643 662 422 143 488 322 029 474 094 309  
 513 170 887 033 930 002 120 237 564 758 611 121 249 309 232 703 245 367 227 534 929 134 469 618 268  
 495 332 378 543 322 902 510 515 342 153 063 681 750 912 860 160  $q^{7177} +$   
 2 064 405 414 234 398 555 340 330 946 016 689 979 956 406 985 405 597 806 623 344 894 657 109 552 471  
 820 969 748 410 508 660 669 290 709 016 323 230 471 696 878 236 955 576 879 212 387 349 942 885 310  
 181 016 206 010 821 043 223 255 573 987 542 887 414 299 750 400  $q^{7180} -$   
 2 131 614 919 774 399 903 965 027 402 355 566 437 538 076 326 084 376 937 151 623 721 934 913 457 810

542 276 492 170 623 829 159 525 326 313 420 173 884 696 423 318 554 796 885 290 523 143 454 675 885  
 056 328 701 571 350 972 093 582 515 331 836 057 178 305 501 750  $q^{7181} +$   
 2 346 627 943 934 473 132 324 827 361 805 548 913 598 603 672 767 780 156 589 641 448 821 008 284 448  
 199 240 795 720 171 443 515 980 927 617 510 530 294 035 007 419 453 939 995 494 165 432 959 858 195  
 537 369 579 299 865 418 017 163 512 851 239 864 684 625 920 000  $q^{7184} -$   
 2 423 004 019 176 361 902 123 511 320 719 203 756 983 308 847 475 340 204 834 564 492 116 493 035 279  
 292 150 629 143 273 356 449 462 195 774 865 769 455 677 136 446 646 118 588 718 846 591 166 474 014  
 278 722 694 317 785 742 008 872 266 308 492 982 600 142 028 800  $q^{7185} +$   
 2 667 337 863 044 716 213 317 560 567 597 681 954 730 838 149 010 186 284 504 349 047 751 153 071 254  
 875 083 910 741 223 136 579 432 508 969 181 620 085 009 427 295 728 712 924 860 599 522 946 519 443  
 340 313 138 266 981 470 327 465 639 528 268 171 893 311 447 040  $q^{7188} -$   
 2 754 127 642 839 374 148 593 726 739 401 172 524 000 071 083 813 688 685 161 038 636 212 373 340 378  
 221 149 497 568 588 034 873 301 361 683 023 831 018 436 686 645 869 363 744 901 157 112 867 356 644  
 735 361 864 507 044 285 553 552 579 729 641 831 306 532 815 000  $q^{7189} +$   
 3 031 770 883 998 151 257 459 891 156 264 220 959 038 147 434 814 276 387 812 297 012 659 711 208 832  
 928 482 311 572 527 014 009 997 227 202 644 310 556 789 659 122 701 519 807 872 845 553 648 780 999  
 545 066 912 656 223 251 367 621 066 800 283 351 301 092 260 864  $q^{7192} -$   
 3 130 390 761 853 568 451 506 674 425 014 138 085 917 727 921 168 637 151 593 934 915 955 682 381 685  
 784 216 246 933 186 553 541 578 981 833 522 452 169 446 340 841 611 982 186 456 625 348 727 051 433  
 022 469 997 867 097 489 907 132 838 126 409 986 084 921 147 392  $q^{7193} +$   
 3 445 873 219 343 505 537 566 666 798 596 064 625 731 929 790 715 278 589 275 741 466 311 893 333 248  
 150 775 091 185 094 955 607 652 342 177 148 870 860 418 532 734 877 476 533 508 114 122 615 827 518  
 231 302 384 425 765 415 833 318 950 328 150 038 425 832 960 000  $q^{7196} -$   
 3 557 931 762 419 091 634 837 828 841 165 034 796 273 288 775 480 124 725 145 748 484 824 679 177 758  
 826 370 355 478 971 283 023 086 341 618 280 730 524 680 221 928 071 995 999 961 287 218 351 028 167  
 823 684 190 752 741 271 497 951 020 326 064 979 873 804 227 009  $q^{7197} +$   
 3 916 397 761 582 910 491 579 022 000 611 101 530 954 781 412 532 985 469 023 349 645 987 735 572 880  
 488 910 337 673 405 167 647 988 014 175 533 311 759 171 175 586 275 796 365 678 745 373 406 598 340  
 981 922 499 307 475 684 677 490 289 472 228 769 744 769 587 200  $q^{7200} -$   
 4 043 721 720 397 603 489 173 951 081 462 224 607 898 729 530 046 193 146 645 635 992 690 337 777 631  
 124 610 690 464 644 672 725 508 474 248 683 696 505 369 187 910 253 544 485 721 012 678 087 036 679  
 042 932 424 131 912 847 485 985 200 196 131 442 664 394 752 000  $q^{7201} +$   
 4 451 013 250 819 781 895 596 992 399 872 347 298 884 100 690 818 669 840 360 662 396 661 905 953 297  
 298 198 493 251 553 843 249 947 052 321 820 713 843 888 247 646 137 345 481 941 903 098 100 581 600  
 863 926 192 819 620 986 171 101 831 709 547 712 382 875 648 000  $q^{7204} -$   
 4 595 677 080 594 784 851 411 351 322 073 678 488 989 673 945 939 332 989 222 660 420 852 056 492 706  
 323 232 428 026 566 742 839 517 843 300 849 365 368 112 808 787 815 311 780 575 056 738 706 384 802  
 244 312 301 913 466 562 434 822 321 486 568 932 483 519 599 250  $q^{7205} +$   
 5 058 428 179 742 561 609 086 213 134 381 484 875 135 831 134 984 199 172 770 303 441 087 469 749 433  
 058 486 852 479 103 698 014 229 690 245 447 165 006 940 562 162 122 091 390 104 430 281 831 761 775  
 406 680 738 522 533 871 031 165 829 139 414 361 917 490 442 240  $q^{7208} -$   
 5 222 787 546 329 400 091 626 649 421 259 094 665 093 335 506 751 795 246 954 116 785 317 847 058 901  
 611 181 985 224 474 203 957 833 408 142 938 062 741 800 233 565 694 035 873 261 089 299 192 330 611  
 391 685 386 505 929 555 299 615 871 331 019 881 245 159 424 000  $q^{7209} +$   
 5 748 531 420 561 922 366 231 335 653 362 054 079 444 492 388 726 688 858 270 812 634 787 096 864 794  
 329 874 073 622 614 348 398 713 365 165 073 122 864 468 036 581 832 941 802 156 082 589 994 292 068  
 498 885 069 250 124 834 792 643 120 117 110 952 251 754 790 912  $q^{7212} -$   
 5 935 261 227 447 743 222 617 866 549 916 334 893 087 366 732 025 593 009 691 687 282 332 442 326 785  
 860 917 227 802 854 735 750 499 018 682 029 060 711 744 311 918 377 463 684 593 039 665 409 037 853  
 874 208 277 723 207 403 795 052 592 935 229 708 143 287 222 676  $q^{7213} +$   
 6 532 551 825 123 871 392 555 620 792 186 917 457 842 493 170 468 766 190 267 283 026 259 137 460 210  
 586 368 892 632 333 298 292 359 382 516 934 901 120 085 404 548 325 941 025 297 725 327 502 472 192  
 698 664 023 987 042 011 282 613 515 311 516 881 463 985 152 000  $q^{7216} -$   
 6 744 689 370 063 001 270 980 374 047 290 631 259 110 189 699 758 056 671 465 075 944 408 691 074 308  
 744 197 615 630 308 474 186 110 802 286 952 432 418 647 294 218 588 814 115 669 419 328 341 678 828

265 409 138 846 536 392 666 094 051 801 977 086 996 155 138 048  $q^{7217} +$   
 7 423 239 351 752 732 809 365 509 819 688 035 790 139 468 082 975 113 293 648 315 120 761 770 140 097 \ \backslash  
 214 565 621 391 891 056 263 966 099 733 161 659 460 542 047 987 399 684 438 081 693 718 895 487 632 \ \backslash  
 206 201 830 825 574 589 820 853 795 402 216 244 384 760 145 920  $q^{7220} -$   
 7 664 233 303 284 992 325 383 605 467 428 694 426 898 770 109 708 189 339 130 507 642 895 263 653 844 \ \backslash  
 820 584 602 416 098 585 094 363 736 050 761 996 853 340 920 840 097 633 539 534 442 259 675 293 377 \ \backslash  
 915 945 775 349 045 342 904 649 184 495 646 165 506 366 791 875  $q^{7221} +$   
 8 435 070 615 212 111 237 535 429 840 400 702 566 625 988 701 704 949 677 458 927 944 725 996 473 594 \ \backslash  
 665 361 708 611 027 190 682 446 127 788 567 453 000 925 850 530 409 339 288 784 651 288 232 239 039 \ \backslash  
 769 863 929 416 792 159 192 536 673 051 448 095 997 883 648 000  $q^{7224} -$   
 8 708 836 591 984 584 668 706 824 128 760 908 982 525 351 331 134 760 685 515 921 545 134 469 353 239 \ \backslash  
 804 045 044 430 800 276 203 364 693 453 039 617 671 662 203 564 346 045 400 363 847 427 421 711 539 \ \backslash  
 255 511 878 424 602 676 744 045 944 756 818 574 040 955 748 600  $q^{7225} +$   
 9 584 482 144 921 371 829 459 124 729 918 183 080 538 188 338 660 488 682 491 321 367 948 545 919 238 \ \backslash  
 564 694 227 768 749 135 604 822 627 589 368 780 925 235 130 358 247 667 226 079 616 570 031 125 171 \ \backslash  
 207 678 151 621 979 866 671 511 932 755 415 944 878 707 894 272  $q^{7228} -$   
 9 895 465 785 793 647 420 752 912 289 378 099 146 458 323 202 513 822 160 680 301 822 361 470 198 960 \ \backslash  
 285 075 212 278 488 448 477 442 277 148 733 581 219 335 974 693 930 693 142 405 430 223 412 886 751 \ \backslash  
 359 240 745 879 660 801 974 738 816 818 092 132 073 009 454 375  $q^{7229} +$   
 10 890 135 077 364 229 022 023 323 127 982 269 929 921 006 149 167 344 857 415 060 533 046 673 541 \ \backslash  
 271 567 805 677 759 392 541 581 867 209 066 769 045 384 321 605 349 076 275 383 145 223 722 235 952 \ \backslash  
 846 764 690 801 876 799 200 491 059 660 917 030 772 577 226 719 232  $q^{7232} -$   
 11 243 383 609 404 854 829 223 780 822 142 036 871 861 683 847 971 653 595 010 191 960 630 192 215 \ \backslash  
 642 924 153 512 809 316 934 077 790 552 379 127 332 511 938 989 792 402 250 760 744 440 263 558 579 \ \backslash  
 970 245 288 668 348 528 551 480 713 779 590 066 855 277 860 257 792  $q^{7233} +$   
 12 373 215 508 426 573 270 252 961 773 222 243 492 850 221 602 266 556 818 979 421 196 522 906 011 \ \backslash  
 697 395 426 656 334 155 221 286 745 294 959 147 399 431 368 967 123 685 038 459 218 509 124 111 807 \ \backslash  
 194 946 094 947 787 035 806 890 551 588 576 611 782 371 909 632 000  $q^{7236} -$   
 12 774 458 954 978 757 003 202 932 727 357 711 383 401 327 173 771 820 875 862 956 557 516 390 438 \ \backslash  
 533 216 209 472 085 906 135 511 693 325 278 834 969 848 537 335 271 242 854 194 227 823 059 846 032 \ \backslash  
 353 598 088 072 178 962 384 056 762 467 009 424 874 790 042 958 317  $q^{7237} +$   
 14 057 775 298 080 769 406 481 799 245 310 081 740 467 116 692 218 875 383 827 761 977 514 927 548 \ \backslash  
 618 142 234 209 907 122 657 126 333 104 041 722 108 774 594 089 384 535 707 221 418 598 335 060 762 \ \backslash  
 282 007 724 900 744 153 830 363 274 423 897 587 180 848 282 035 200  $q^{7240} -$   
 14 513 518 622 216 516 940 723 467 945 137 802 638 847 461 802 799 130 711 424 100 024 852 126 632 \ \backslash  
 373 863 509 027 082 110 569 367 236 151 201 964 791 773 762 380 782 029 380 854 911 162 930 761 536 \ \backslash  
 780 533 271 653 021 795 402 181 161 075 216 255 613 959 684 096 000  $q^{7241} +$   
 15 971 118 762 320 756 256 629 210 953 489 411 040 647 151 529 614 013 745 188 232 688 566 951 640 \ \backslash  
 119 632 585 374 805 597 547 763 372 822 754 508 015 802 122 043 210 685 479 401 788 236 885 291 190 \ \backslash  
 589 365 103 932 077 816 174 497 885 165 731 992 913 607 048 128 000  $q^{7244} -$   
 16 488 746 414 626 457 977 303 680 213 910 183 949 060 584 742 549 535 269 286 936 624 071 078 186 \ \backslash  
 913 119 999 013 908 584 418 864 640 411 962 436 111 150 668 780 753 337 147 291 250 848 268 922 520 \ \backslash  
 899 974 696 804 787 339 200 171 376 225 694 542 779 649 655 043 875  $q^{7245} +$   
 18 144 241 415 662 552 158 188 045 624 093 930 691 733 252 099 301 280 625 828 757 416 848 745 234 \ \backslash  
 641 460 060 312 154 750 360 641 679 980 771 318 827 718 932 702 515 341 397 024 164 196 200 866 576 \ \backslash  
 717 935 772 486 750 168 936 518 327 049 650 551 484 722 716 377 088  $q^{7248} -$   
 18 732 135 952 138 345 243 117 185 847 732 845 222 991 998 461 301 444 075 441 923 655 506 069 210 \ \backslash  
 537 112 283 693 380 547 921 611 217 926 071 504 259 029 398 154 754 978 670 763 375 994 526 009 438 \ \backslash  
 316 903 499 412 392 674 963 252 356 438 031 902 013 878 333 440 000  $q^{7249} +$   
 20 612 327 753 321 082 792 520 499 972 483 534 267 201 316 874 067 338 454 378 531 269 859 558 508 \ \backslash  
 810 212 758 894 325 670 197 953 286 032 504 588 737 944 005 532 781 958 869 258 625 691 275 552 420 \ \backslash  
 208 373 892 145 594 766 965 544 078 397 275 696 328 828 576 622 592  $q^{7252} -$   
 21 280 004 412 327 731 553 960 222 301 822 079 484 099 716 890 228 029 613 822 646 320 717 627 787 \ \backslash  
 146 635 917 051 918 279 343 855 818 320 794 736 417 849 983 637 956 700 701 540 393 947 701 803 766 \ \backslash  
 420 013 477 975 785 337 508 669 947 524 324 868 984 439 715 560 009  $q^{7253} +$

23 415 315 998 344 955 387 316 731 875 194 858 733 448 492 367 185 784 010 310 603 375 637 995 269 \
 380 313 367 667 557 436 698 964 315 319 168 981 505 447 511 034 283 205 784 772 569 170 820 922 496 \
 481 870 985 000 019 084 808 781 596 518 291 020 461 963 837 248 000  $q^{7256}$  -

24 173 575 378 504 119 565 510 181 030 453 315 706 956 177 484 303 188 161 561 046 962 215 917 319 \
 476 852 097 540 356 644 785 512 472 279 477 476 787 135 731 883 854 125 330 655 724 898 394 374 778 \
 809 716 535 229 106 020 039 267 845 016 812 658 390 944 510 181 376  $q^{7257}$  +

26 598 538 800 252 288 328 046 841 592 563 529 380 411 369 224 005 421 811 493 506 883 250 061 901 \
 127 532 143 244 357 230 808 418 252 615 675 743 140 178 523 283 876 414 985 285 234 389 330 325 595 \
 807 023 523 919 854 851 980 486 941 973 318 064 017 449 138 534 400  $q^{7260}$  -

27 459 640 067 974 227 492 657 581 260 033 269 673 742 906 386 492 609 514 606 142 554 061 286 594 \
 083 264 144 658 840 505 630 022 431 519 882 926 748 948 813 639 331 751 023 781 921 042 337 387 095 \
 937 057 283 492 750 054 078 808 484 265 885 985 066 832 925 254 625  $q^{7261}$  +

30 213 450 074 736 712 714 749 344 566 426 776 989 708 305 393 607 116 277 077 838 686 946 373 457 \
 910 783 504 450 302 761 334 682 233 520 305 630 683 167 737 707 348 027 279 840 376 249 679 989 444 \
 077 845 937 522 105 788 175 223 994 301 466 625 740 959 610 368 000  $q^{7264}$  -

31 191 307 455 117 689 886 556 631 470 823 015 538 180 028 587 599 869 911 647 882 171 177 406 091 \
 132 833 754 577 396 053 596 131 501 286 597 243 531 426 136 684 388 184 369 964 576 326 291 808 539 \
 867 281 920 268 057 424 979 736 560 339 878 881 716 312 812 748 800  $q^{7265}$  +

34 318 449 537 694 006 310 161 022 505 443 533 300 560 725 604 785 674 187 362 166 275 861 761 948 \
 764 989 028 262 107 583 889 988 421 719 039 528 119 447 833 857 832 057 164 317 243 988 265 344 123 \
 447 316 066 347 049 897 172 866 019 467 372 622 528 807 990 099 968  $q^{7268}$  -

35 428 855 210 996 670 656 272 243 672 525 146 289 722 578 800 346 538 882 362 285 271 047 201 680 \
 384 387 525 492 195 816 817 921 675 798 795 683 846 583 923 587 329 732 281 871 283 766 955 435 316 \
 973 067 209 654 834 471 529 856 889 278 854 737 361 604 889 194 000  $q^{7269}$  +

38 979 818 032 558 462 111 437 091 433 704 393 390 570 502 583 872 993 038 201 373 779 835 724 279 \
 531 586 955 356 947 137 377 273 204 226 253 564 632 021 446 489 188 825 648 472 442 477 020 707 045 \
 747 020 371 148 782 997 230 098 784 483 149 286 578 353 556 134 400  $q^{7272}$  -

40 240 694 976 143 262 987 179 930 159 528 239 488 460 667 948 645 805 208 154 345 851 790 762 393 \
 236 662 437 059 394 054 586 828 852 536 757 597 028 065 088 929 315 413 293 056 399 181 990 628 109 \
 895 661 165 283 480 195 992 718 127 402 814 658 157 718 519 218 176  $q^{7273}$  +

44 272 778 501 980 133 674 013 514 762 374 962 673 984 217 344 671 412 631 229 713 685 314 918 596 \
 161 912 032 584 205 076 864 563 615 189 005 253 478 875 244 728 659 645 687 887 481 689 412 313 095 \
 877 478 048 236 364 845 065 757 313 989 559 033 246 062 105 216 000  $q^{7276}$  -

45 704 467 290 943 404 633 031 383 885 315 217 619 995 993 124 802 786 716 568 335 687 866 928 244 \
 876 460 542 332 274 559 561 689 327 445 967 587 904 205 916 481 994 174 201 538 876 142 293 794 296 \
 760 480 509 752 271 269 548 930 202 964 375 636 902 499 550 152 454  $q^{7277}$  +

50 282 699 440 686 816 192 461 960 434 534 177 329 964 412 655 581 800 123 851 072 681 126 052 285 \
 314 581 874 750 231 140 061 768 392 636 130 166 200 540 189 728 216 604 510 261 900 242 443 603 776 \
 265 665 329 897 526 661 229 609 023 246 074 231 345 801 422 438 400  $q^{7280}$  -

51 908 283 557 000 538 122 880 822 937 186 132 783 885 546 008 456 588 615 864 231 577 860 357 493 \
 901 012 868 819 710 758 469 161 412 919 120 907 322 858 538 166 371 288 515 116 430 159 116 815 166 \
 264 238 324 201 861 166 818 762 139 479 323 647 340 608 798 720 000  $q^{7281}$  +

57 106 459 917 073 374 869 125 217 192 693 078 452 807 328 794 145 170 402 322 079 489 409 567 807 \
 523 813 663 077 751 737 790 438 253 192 801 176 538 255 462 106 234 953 813 686 766 306 304 778 076 \
 541 641 911 129 449 070 231 909 340 909 594 269 372 954 491 392 000  $q^{7284}$  -

58 952 134 725 116 933 165 428 523 904 909 559 677 419 376 106 132 638 210 961 819 232 393 759 810 \
 045 864 398 352 522 664 427 247 971 081 368 994 372 922 946 549 186 515 037 478 243 248 311 077 218 \
 665 422 051 278 679 932 136 846 423 044 383 169 096 154 680 311 025  $q^{7285}$  +

64 853 997 801 892 598 997 609 307 501 580 161 744 390 011 559 545 047 965 535 651 772 743 281 328 \
 784 498 846 014 175 086 300 121 763 332 621 011 220 240 076 240 629 820 172 288 690 021 623 348 272 \
 603 814 375 827 466 827 358 612 938 010 110 999 123 610 927 362 048  $q^{7288}$  -

66 949 489 037 437 927 803 564 723 885 568 054 405 362 087 755 194 443 605 245 479 290 868 950 407 \
 006 282 970 894 074 167 209 726 456 625 485 350 755 369 878 275 530 645 934 861 729 302 143 850 358 \
 064 951 620 218 730 220 141 316 447 213 676 998 434 575 982 592 000  $q^{7289}$  +

73 650 065 733 311 562 998 912 913 243 486 939 899 351 617 157 347 168 901 916 585 516 666 262 473 \

819 670 916 186 916 283 209 467 490 649 759 128 816 319 357 009 973 217 907 997 532 508 919 285 574 \
 186 981 888 982 726 338 592 626 226 962 411 099 334 454 726 811 648  $q^{7292}$  -

76 029 104 134 053 194 433 638 479 209 461 724 294 345 028 905 923 384 851 226 137 415 343 367 624 \
 896 591 811 515 453 138 101 344 501 755 313 141 553 810 512 741 331 313 016 934 270 002 007 639 222 \
 580 105 158 989 622 851 679 494 305 977 843 799 795 889 289 189 388  $q^{7293}$  +

83 636 222 623 769 106 748 363 287 954 652 653 463 165 312 970 047 897 791 278 557 392 177 089 800 \
 523 230 497 966 001 953 851 975 937 797 682 861 452 095 937 552 389 284 833 489 881 725 004 150 903 \
 420 178 310 203 731 594 486 339 811 990 294 942 234 000 621 568 000  $q^{7296}$  -

86 337 082 214 593 796 462 011 716 850 614 360 862 564 050 723 532 097 483 171 005 511 669 779 830 \
 149 228 790 973 675 242 868 871 366 037 903 520 781 996 231 291 322 414 326 123 747 300 896 592 227 \
 203 434 264 047 031 172 133 226 677 389 030 442 085 829 465 833 472  $q^{7297}$  +

94 973 092 226 746 633 891 861 847 574 370 513 380 969 485 404 662 514 997 953 707 789 315 877 228 \
 943 827 595 298 801 309 782 395 102 568 343 562 326 096 158 709 751 537 223 259 892 031 681 018 941 \
 819 820 057 889 252 091 670 608 262 931 902 241 254 522 384 793 600  $q^{7300}$  -

98 039 200 775 947 467 217 943 541 845 713 627 562 797 361 788 716 191 754 920 695 209 580 946 197 \
 572 040 804 343 020 760 752 533 750 801 155 281 112 563 535 974 050 877 913 723 730 299 308 392 961 \
 524 245 410 319 422 321 849 120 370 849 246 963 787 054 092 116 875  $q^{7301}$  +

107 842 924 488 762 613 231 991 920 994 469 593 906 328 767 920 948 677 555 244 131 696 087 824 820 \
 434 906 253 108 307 732 880 218 743 913 016 160 603 808 925 994 783 536 709 193 788 429 855 135 675 \
 472 235 781 891 711 177 987 720 936 561 345 801 310 398 165 504 000  $q^{7304}$  -

111 323 555 787 988 292 369 676 524 800 713 282 105 541 965 020 406 147 661 503 124 043 468 519 754 \
 958 934 044 538 854 262 364 371 954 279 635 883 860 184 452 164 054 818 538 542 290 159 308 547 785 \
 407 959 162 275 383 148 476 468 926 819 631 718 006 189 268 992 000  $q^{7305}$  +

122 452 500 179 329 921 059 219 163 813 274 554 916 583 709 499 647 007 623 465 763 762 023 094 341 \
 149 938 724 153 899 999 799 050 114 903 066 978 178 953 283 986 258 290 741 977 144 387 588 900 979 \
 720 179 257 233 188 442 126 965 848 720 768 168 251 588 633 982 976  $q^{7308}$  -

126 403 559 087 966 868 511 287 081 761 970 785 658 849 760 734 890 901 660 085 409 883 631 060 170 \
 159 291 863 338 524 563 176 391 430 702 486 337 369 269 445 031 018 803 513 793 275 063 226 472 401 \
 470 361 083 721 114 713 268 590 279 620 914 567 513 963 970 039 750  $q^{7309}$  +

139 036 424 693 693 198 633 223 178 691 726 197 761 211 486 622 634 170 320 275 892 749 358 267 934 \
 858 907 852 781 256 395 203 854 188 836 718 144 456 271 210 929 725 330 786 824 991 297 596 473 136 \
 643 267 693 933 995 637 023 110 835 119 779 641 671 355 806 777 344  $q^{7312}$  -

143 521 337 347 703 532 158 642 083 548 068 513 095 326 335 898 475 008 818 664 644 428 250 574 617 \
 951 551 586 565 953 531 791 119 528 870 359 131 357 633 901 040 085 085 536 597 490 200 946 936 216 \
 588 640 573 740 414 024 565 569 050 156 287 697 918 376 591 425 536  $q^{7313}$  +

157 860 863 044 170 859 344 400 133 913 387 537 474 913 243 410 777 911 097 465 650 896 956 686 027 \
 527 164 009 790 532 693 633 809 316 569 872 071 372 208 204 214 954 004 394 235 155 609 910 048 599 \
 264 150 607 594 429 958 180 710 014 529 775 169 636 876 579 840 000  $q^{7316}$  -

162 951 586 282 913 232 385 028 218 086 037 084 141 891 272 593 541 920 264 615 686 523 690 035 543 \
 468 243 153 024 308 794 940 505 302 234 197 568 928 868 390 105 032 652 305 263 362 796 748 972 936 \
 995 515 058 861 119 284 946 056 305 455 320 631 033 351 087 708 988  $q^{7317}$  +

179 227 774 991 308 413 855 568 768 961 417 072 875 601 218 705 850 370 804 291 089 143 345 374 670 \
 377 658 536 897 731 875 440 786 343 579 789 881 346 950 765 253 457 105 956 648 341 314 675 808 416 \
 060 533 359 881 055 477 790 113 403 242 368 693 556 191 550 720 000  $q^{7320}$  -

185 005 940 929 325 813 199 920 204 840 024 299 608 208 161 076 429 279 360 160 378 453 720 101 045 \
 029 779 672 487 225 796 882 081 471 389 723 750 239 572 466 651 460 933 639 126 372 001 463 959 324 \
 576 315 303 452 305 142 761 214 155 443 053 099 540 148 494 336 000  $q^{7321}$  +

203 479 717 123 892 035 487 723 738 255 780 925 776 395 247 694 894 597 101 108 898 450 653 399 415 \
 249 710 529 046 114 046 402 807 422 215 346 080 917 513 128 923 695 038 331 287 316 719 730 886 874 \
 349 375 097 253 054 619 818 070 147 646 207 055 116 245 620 992 000  $q^{7324}$  -

210 037 930 917 248 451 796 799 963 602 846 852 906 410 171 994 819 098 928 084 213 941 738 166 090 \
 249 238 298 347 290 948 577 753 958 428 272 613 471 672 733 203 840 342 934 922 023 709 156 348 547 \
 409 714 197 476 000 720 223 112 185 735 035 506 910 432 968 220 125  $q^{7325}$  +

231 005 287 599 569 910 857 378 386 685 575 697 228 490 005 037 856 945 089 512 195 223 125 102 302 \
 451 413 765 553 747 253 434 998 448 986 516 184 160 891 967 169 171 527 791 623 384 735 215 631 868

070 412 459 459 938 975 185 154 308 089 850 829 426 539 669 786 624  $q^{7328} -$   
 238 448 598 861 107 662 605 961 833 041 326 123 020 356 438 392 511 680 118 162 360 003 876 979 637  
 052 721 995 221 331 798 738 781 755 574 426 245 309 785 784 606 272 474 500 696 405 723 690 658 963  
 142 566 120 568 610 794 530 464 514 492 430 745 385 190 842 368 000  $q^{7329} +$   
 262 245 299 343 980 664 620 890 212 842 901 700 493 225 709 116 941 730 032 312 505 684 010 450 499  
 116 265 428 460 335 148 177 385 210 209 335 074 770 992 045 343 724 515 634 828 807 338 477 166 076  
 391 080 363 929 782 997 259 738 234 670 385 341 490 844 491 808 768  $q^{7332} -$   
 270 692 870 386 277 352 039 235 597 668 233 305 751 124 491 744 058 105 213 374 048 123 247 070 105  
 925 761 803 609 843 740 395 811 885 082 113 818 041 684 622 226 965 411 457 629 520 141 224 840 304  
 788 459 191 995 821 483 616 616 529 844 654 771 802 171 074 748 747  $q^{7333} +$   
 297 699 778 932 829 504 640 904 782 935 074 636 465 918 612 251 916 694 781 187 355 987 018 204 385  
 414 466 622 161 385 750 500 122 036 251 573 381 733 473 832 186 112 223 079 303 797 989 732 329 357  
 619 420 677 498 810 592 304 416 139 039 706 911 594 866 848 640 000  $q^{7336} -$   
 307 286 776 104 034 803 807 928 270 647 734 740 444 237 046 390 609 535 463 445 628 584 188 253 304  
 240 529 084 916 115 707 809 543 903 593 460 784 180 019 541 501 907 385 980 510 212 607 646 206 738  
 561 201 069 368 506 456 044 922 977 156 566 854 667 058 969 051 136  $q^{7337} +$   
 337 935 901 325 980 841 091 043 255 985 804 269 881 099 103 531 176 830 326 263 110 719 321 105 346  
 926 771 208 280 709 081 047 349 682 518 806 509 708 596 572 719 985 371 700 915 727 395 296 192 241  
 478 481 512 226 547 558 798 155 680 367 971 367 948 788 317 926 400  $q^{7340} -$   
 348 815 639 200 090 230 961 633 939 737 086 872 106 791 911 075 382 443 098 118 704 998 273 060 422  
 208 750 685 050 713 198 728 422 583 666 350 523 137 136 263 451 798 269 315 040 828 300 202 720 038  
 634 675 973 261 657 412 023 849 675 078 888 509 856 718 590 151 750  $q^{7341} +$   
 383 596 985 286 548 464 416 945 599 795 803 021 510 416 745 420 577 431 100 027 392 159 844 074 943  
 247 609 112 195 394 429 159 984 567 687 358 088 932 518 056 497 261 936 014 154 683 783 235 509 185  
 630 432 993 551 906 842 795 095 120 040 895 402 965 566 181 376 000  $q^{7344} -$   
 395 943 357 430 349 554 849 999 607 187 990 730 941 768 297 321 112 414 918 359 123 018 928 655 535  
 097 145 805 018 528 036 738 372 113 585 772 639 266 770 616 919 988 675 842 455 378 928 529 261 617  
 007 553 015 802 599 135 423 571 669 781 140 657 743 401 608 806 400  $q^{7345} +$   
 435 412 690 928 959 098 924 796 282 496 565 678 551 531 880 058 550 086 040 382 867 342 689 577 014  
 166 222 576 123 336 116 522 768 574 292 702 022 498 067 068 689 550 512 511 984 439 816 352 295 614  
 010 914 204 274 398 493 806 007 171 597 903 916 063 012 841 955 328  $q^{7348} -$   
 449 422 925 454 373 836 880 300 864 590 404 286 135 763 129 628 723 834 085 230 475 606 810 141 835  
 318 839 740 185 898 364 457 022 932 036 962 031 110 918 978 969 617 004 934 976 165 820 521 570 714  
 734 911 396 571 218 128 872 350 063 764 863 677 603 019 905 913 125  $q^{7349} +$   
 494 210 579 655 949 556 630 475 832 267 516 678 531 052 670 525 809 234 603 772 641 062 853 420 721  
 463 512 597 863 419 296 570 198 335 494 656 699 872 124 552 696 179 356 552 044 931 081 636 568 931  
 559 494 138 210 579 419 313 077 190 149 820 839 249 845 391 219 712  $q^{7352} -$   
 510 108 362 848 427 854 357 010 658 346 629 206 320 556 582 567 083 019 491 645 379 862 316 267 595  
 842 974 448 682 007 095 829 419 522 170 924 121 466 001 560 179 172 023 409 783 460 322 854 564 296  
 093 538 007 373 663 015 038 009 128 429 238 877 714 315 261 345 792  $q^{7353} +$   
 560 929 218 057 418 176 855 948 615 590 790 767 150 394 678 343 391 914 660 486 087 194 804 089 206  
 005 037 966 665 713 691 149 810 152 090 819 555 722 860 267 973 379 988 511 061 091 937 413 541 011  
 044 734 453 417 041 767 744 922 666 653 076 604 104 400 831 744 000  $q^{7356} -$   
 578 968 235 127 250 895 869 338 332 655 303 297 612 457 764 058 332 758 440 915 127 916 928 688 792  
 954 120 844 269 307 958 097 279 016 076 500 108 102 273 110 713 269 519 761 817 358 068 625 559 871  
 885 417 080 426 044 861 346 481 020 510 942 434 189 458 801 373 629  $q^{7357} +$   
 636 633 031 484 545 422 768 044 509 147 036 020 540 664 567 545 333 179 791 268 831 283 594 061 932  
 296 845 429 332 286 773 831 072 278 735 273 372 504 908 569 765 683 504 844 044 835 981 907 637 392  
 027 945 729 670 484 135 785 813 560 439 982 236 410 849 979 596 800  $q^{7360} -$   
 657 100 980 007 704 950 379 698 116 459 849 881 801 381 536 251 073 647 495 712 193 742 135 448 982  
 561 142 997 300 792 866 377 716 061 422 355 800 873 100 800 644 520 928 462 929 376 270 774 752 986  
 603 557 621 261 350 002 306 972 737 731 513 499 525 073 551 360 000  $q^{7361} +$   
 722 529 140 354 838 287 796 412 173 506 030 474 426 776 437 749 257 152 897 005 509 557 226 875 901  
 772 152 254 822 973 045 512 220 204 810 817 166 155 798 559 141 644 059 097 902 043 541 962 620 846  
 724 264 478 919 099 854 192 679 075 560 996 607 049 140 310 016 000  $q^{7364} -$

745 752 279 354 255 164 624 873 636 626 189 684 164 757 578 817 089 497 985 975 161 869 716 614 194  
 683 148 172 892 697 942 235 150 947 732 891 121 602 716 286 634 942 972 824 007 882 601 031 868 664  
 966 779 297 171 797 844 862 404 171 822 171 202 194 544 338 921 925  $q^{7365} +$   
 819 986 443 211 355 717 250 075 835 718 249 628 591 101 515 134 769 166 409 840 448 220 728 574 121  
 139 633 738 077 342 742 551 491 508 651 761 428 981 707 246 211 544 112 576 646 834 172 244 414 588  
 791 096 032 848 998 381 154 396 134 750 661 643 631 648 946 268 160  $q^{7368} -$   
 846 334 749 192 768 346 584 487 548 056 438 368 608 314 832 867 009 701 973 118 666 309 717 448 511  
 123 523 894 142 842 627 238 645 915 716 310 129 743 301 517 826 652 065 481 222 260 596 440 077 583  
 796 178 611 711 240 396 803 583 441 062 598 838 570 538 901 504 000  $q^{7369} +$   
 930 557 245 631 866 984 276 921 891 500 583 017 342 071 871 174 133 068 998 527 408 169 796 838 764  
 668 311 560 687 332 232 313 504 689 971 518 459 905 531 051 126 101 869 989 901 340 858 941 467 418  
 210 524 325 133 767 097 366 488 868 629 523 210 066 656 854 174 720  $q^{7372} -$   
 960 450 256 359 999 407 088 474 848 423 455 717 938 150 157 365 525 594 214 996 359 732 123 904 824  
 435 361 822 140 100 463 211 678 138 829 752 894 993 904 987 783 605 765 901 571 083 465 156 625 710  
 909 913 477 399 753 973 488 642 520 035 291 506 169 286 552 529 482  $q^{7373} +$   
 1 056 001 773 803 885 375 962 180 313 097 927 820 501 404 120 044 751 739 798 948 138 891 441 818 589  
 229 558 982 290 718 240 179 395 702 390 549 999 958 651 008 791 134 491 814 703 904 050 937 279 994  
 716 866 163 479 975 405 007 549 643 357 572 815 328 749 668 352 000  $q^{7376} -$   
 1 089 915 211 331 255 924 482 419 800 657 983 431 258 989 170 374 304 148 077 186 846 012 038 143 334  
 156 920 279 955 129 894 255 225 837 219 775 510 393 453 270 205 251 811 314 421 689 541 953 787 683  
 988 706 342 558 455 135 703 099 899 785 545 634 832 903 301 726 208  $q^{7377} +$   
 1 198 315 956 563 812 065 964 306 043 196 778 289 267 511 182 019 220 756 890 091 632 104 150 899 608  
 819 896 326 465 062 478 714 832 584 296 099 988 223 836 729 768 925 390 558 441 195 223 889 580 818  
 942 373 036 038 143 407 147 819 685 462 602 040 170 336 252 928 000  $q^{7380} -$   
 1 236 789 233 171 821 172 758 941 323 908 116 219 489 853 220 264 202 632 563 204 959 593 765 025 024  
 611 296 099 204 401 067 840 635 091 480 587 161 173 103 676 808 483 588 547 281 250 345 329 357 678  
 775 869 342 933 951 317 937 283 680 644 338 575 270 985 185 688 625  $q^{7381} +$   
 1 359 762 910 638 251 523 654 500 192 742 256 677 269 210 477 354 714 738 915 627 852 998 692 158 941  
 505 540 394 869 769 777 111 149 249 016 699 630 365 685 690 130 711 092 955 828 156 645 366 357 878  
 378 356 367 858 782 157 346 758 353 905 565 835 799 879 608 960 000  $q^{7384} -$   
 1 403 407 635 106 077 993 458 882 786 362 479 002 274 549 910 629 562 118 027 248 433 594 010 643 623  
 613 725 137 540 389 584 895 729 934 476 014 284 800 723 758 768 932 752 029 991 233 133 129 606 885  
 730 044 519 216 180 132 567 238 955 889 593 141 828 064 006 963 200  $q^{7385} +$   
 1 542 908 621 510 036 966 653 918 880 917 081 697 379 612 014 312 177 499 669 521 876 320 664 291 266  
 380 802 880 130 819 756 085 442 619 155 554 555 696 660 568 982 371 482 013 358 550 200 140 003 500  
 948 155 593 503 570 051 500 086 812 093 064 048 858 109 819 979 776  $q^{7388} -$   
 1 592 418 238 703 773 393 190 074 675 505 544 421 364 072 742 360 809 947 484 057 565 942 397 789 330  
 992 393 648 942 146 732 152 951 580 954 803 022 739 278 509 847 431 282 469 625 239 144 641 194 338  
 664 961 683 293 559 531 506 386 754 144 094 508 883 256 715 814 625  $q^{7389} +$   
 1 750 662 377 651 492 202 678 536 235 675 911 753 122 241 095 556 918 459 673 208 695 270 991 528 836  
 582 581 643 188 264 164 318 791 110 951 189 238 901 775 218 634 129 554 436 970 414 904 525 940 977  
 039 770 926 716 998 162 747 610 969 027 496 182 096 202 484 006 912  $q^{7392} -$   
 1 806 823 092 064 357 697 462 784 634 517 521 414 260 335 990 694 062 738 348 129 593 327 590 464 042  
 669 464 810 991 821 022 401 677 463 708 981 183 471 370 994 112 006 061 688 192 005 874 038 650 970  
 889 638 053 573 235 516 735 551 466 676 927 125 329 233 451 155 456  $q^{7393} +$   
 1 986 322 589 831 198 465 723 791 482 870 907 962 111 223 641 441 406 703 931 662 365 265 203 581 177  
 608 574 494 772 931 372 070 676 234 072 067 621 838 742 925 032 666 882 208 519 572 719 771 612 868  
 427 190 863 447 117 970 384 748 654 874 897 759 679 595 190 298 752  $q^{7396} -$   
 2 050 025 743 677 748 228 640 320 994 309 499 567 650 801 333 706 577 411 613 790 871 674 901 892 116  
 843 217 356 043 229 096 991 361 573 765 466 447 123 205 365 516 512 046 695 990 386 180 584 775 031  
 277 477 162 233 248 927 922 114 957 947 577 888 684 061 110 081 370  $q^{7397} +$   
 2 253 628 710 949 088 634 075 687 232 029 682 761 383 308 493 702 013 092 746 457 940 673 487 361 963  
 192 516 784 827 690 284 105 190 433 694 621 245 406 029 411 215 426 455 350 192 414 582 378 516 705  
 823 364 967 391 652 902 267 754 015 865 855 237 217 095 024 473 600  $q^{7400} -$   
 2 325 884 810 030 108 661 211 821 384 170 335 058 048 186 337 253 044 856 062 414 617 838 279 594 820

597 584 667 661 400 775 601 354 265 780 717 536 491 594 249 601 482 220 227 358 170 391 251 547 968  
 614 633 443 103 775 198 553 416 754 676 525 510 234 917 572 608 000  $q^{7401} +$   
 2 556 820 066 679 379 880 706 838 688 607 990 516 788 487 419 397 646 522 465 781 458 995 102 617 781  
 095 660 609 860 582 505 857 508 908 879 955 779 987 901 043 503 207 296 031 288 092 069 498 327 329  
 908 136 279 805 932 751 385 497 329 523 799 837 941 223 148 416 000  $q^{7404} -$   
 2 638 774 672 838 180 201 862 900 724 194 374 325 142 901 137 490 447 423 030 084 085 774 775 996 677  
 770 928 359 204 592 379 838 397 873 561 669 226 639 226 246 508 979 235 062 273 011 655 419 961 535  
 921 971 981 461 261 863 908 971 023 484 906 686 040 337 943 412 525  $q^{7405} +$   
 2 900 702 514 563 009 780 084 251 469 487 708 324 280 237 158 419 213 188 188 217 223 328 773 093 875  
 363 407 726 747 516 396 728 143 227 476 090 865 715 551 318 151 224 906 112 731 119 403 904 631 348  
 102 062 175 791 218 380 209 241 570 474 764 485 012 329 361 801 216  $q^{7408} -$   
 2 993 654 252 542 562 313 849 104 169 257 824 732 173 415 297 137 338 080 859 631 907 739 916 566 667  
 747 099 113 744 178 255 816 415 582 540 059 859 678 400 613 541 827 599 210 210 936 377 364 268 158  
 344 880 029 516 536 724 195 565 959 187 531 299 250 425 110 528 000  $q^{7409} +$   
 3 290 723 970 744 525 634 178 649 799 841 055 598 229 370 659 971 149 845 662 914 014 602 932 205 676  
 088 066 501 385 859 909 738 960 990 430 660 580 115 150 040 243 489 628 185 403 684 203 693 802 781  
 826 656 775 929 456 639 557 792 001 517 216 157 277 995 811 426 304  $q^{7412} -$   
 3 396 144 930 074 691 586 590 279 668 704 268 761 196 555 988 280 304 662 804 252 621 134 219 774 202  
 219 987 738 388 364 498 434 438 790 579 189 287 891 496 879 589 063 230 938 944 595 088 573 719 173  
 141 729 279 882 552 001 529 429 145 923 610 790 479 761 229 764 381  $q^{7413} +$   
 3 733 059 981 164 046 090 105 828 748 051 854 065 281 636 770 939 907 846 515 650 318 216 957 129 592  
 607 053 944 299 701 641 436 744 901 174 074 535 834 248 750 665 536 314 952 934 258 890 531 864 367  
 867 480 788 190 979 769 692 757 118 578 766 894 038 865 073 024 000  $q^{7416} -$   
 3 852 618 830 864 082 804 086 251 749 475 922 916 088 012 180 472 134 202 471 853 063 049 385 940 444  
 368 193 425 336 782 189 309 611 829 117 865 015 496 957 823 677 215 910 837 074 833 968 337 823 687  
 315 745 055 135 081 055 342 680 816 921 916 839 889 020 108 210 176  $q^{7417} +$   
 4 234 710 669 810 371 210 120 297 608 198 043 912 558 519 550 505 542 639 405 705 773 663 565 229 756  
 195 305 753 203 234 140 286 531 376 753 821 250 853 782 729 966 478 861 145 844 839 356 207 858 260  
 440 184 606 566 246 441 583 856 335 141 838 035 146 560 092 057 600  $q^{7420} -$   
 4 370 298 845 755 507 513 379 157 935 819 061 218 722 594 712 205 184 236 514 611 452 211 682 693 565  
 380 458 729 121 660 819 536 658 010 578 855 222 036 664 569 324 088 525 155 770 898 409 168 250 737  
 604 605 409 687 760 684 097 079 585 070 331 706 488 181 302 658 375  $q^{7421} +$   
 4 803 610 573 012 415 615 927 388 716 327 873 787 386 671 258 209 409 059 003 058 189 050 943 946 731  
 184 997 444 706 830 007 890 621 225 474 930 358 751 639 770 883 909 556 608 009 594 936 835 986 770  
 185 433 031 936 344 928 729 382 964 745 138 174 510 842 380 288 000  $q^{7424} -$   
 4 957 371 945 431 189 570 306 378 491 555 064 157 792 140 949 736 583 596 145 471 547 192 008 622 442  
 474 550 275 088 844 728 203 443 449 914 814 094 342 615 144 684 329 281 383 671 421 383 364 108 646  
 961 158 125 367 388 576 094 486 051 928 034 418 401 058 884 812 800  $q^{7425} +$   
 5 448 753 068 403 712 606 961 768 375 100 627 853 396 841 848 102 263 348 580 155 311 789 195 598 801  
 654 404 963 065 133 573 040 684 869 784 700 865 302 036 284 167 415 240 575 361 059 061 372 874 677  
 747 161 777 575 560 567 014 907 198 949 562 096 387 510 535 536 640  $q^{7428} -$   
 5 623 117 550 876 627 491 503 917 232 759 071 492 207 413 818 548 304 901 112 896 062 989 422 870 279  
 989 566 971 824 374 397 195 708 977 062 738 784 869 312 752 874 020 920 796 790 438 743 368 914 279  
 521 691 692 835 430 083 169 942 228 827 201 791 712 246 117 808 250  $q^{7429} +$   
 6 180 331 333 205 908 690 052 802 870 297 227 305 070 615 211 754 782 514 707 206 216 981 506 615 048  
 352 225 588 667 085 155 071 505 541 180 550 877 860 339 383 747 420 608 204 671 289 293 354 479 352  
 716 674 700 235 114 204 434 926 318 919 512 731 907 501 151 005 696  $q^{7432} -$   
 6 378 052 955 553 579 170 067 836 710 986 504 145 961 267 775 366 017 085 250 987 790 016 743 194 306  
 097 072 514 558 035 568 881 218 473 686 413 046 312 573 907 629 231 885 865 138 950 959 219 497 357  
 884 525 579 319 120 185 157 358 226 921 641 075 112 623 170 060 288  $q^{7433} +$   
 7 009 898 022 312 066 190 106 742 849 633 769 820 852 244 706 836 474 255 620 668 431 613 743 529 742  
 141 867 242 004 379 017 604 536 292 769 357 476 746 034 151 144 216 620 294 693 507 127 828 082 770  
 006 767 797 947 122 775 116 279 196 457 288 264 698 482 875 328 000  $q^{7436} -$   
 7 234 098 058 828 943 800 380 914 186 143 313 786 489 111 804 956 422 371 019 318 738 924 040 548 516  
 412 633 064 134 412 009 120 919 500 985 303 331 337 448 332 910 904 276 897 237 815 605 981 052 599

749 189 937 364 398 298 985 208 928 087 606 544 926 544 685 168 793  $q^{7437} +$   
 7 950 546 146 235 175 235 174 210 857 175 151 302 571 188 447 521 096 590 546 285 789 453 853 711 474 \ \backslash  
 102 740 428 288 748 748 528 890 327 992 295 239 757 757 933 542 604 514 911 881 660 056 350 872 459 \ \backslash  
 546 292 707 802 696 429 738 692 272 598 859 109 948 362 915 840 000  $q^{7440} -$   
 8 204 761 968 902 709 451 009 249 669 493 395 040 394 951 177 355 327 503 863 852 368 153 908 148 472 \ \backslash  
 475 372 557 709 762 307 433 621 112 196 960 268 670 343 498 608 530 989 997 066 082 987 875 312 626 \ \backslash  
 745 413 888 114 813 008 751 042 433 564 736 046 374 372 581 376 000  $q^{7441} +$   
 9 017 113 956 763 067 232 890 546 121 495 060 306 508 637 018 743 625 886 354 327 442 456 901 036 805 \ \backslash  
 966 565 839 012 239 470 623 072 574 600 747 146 026 039 680 835 044 716 782 361 383 044 374 870 608 \ \backslash  
 466 954 426 288 034 730 822 969 809 083 541 424 697 417 345 792 000  $q^{7444} -$   
 9 305 354 371 562 442 130 335 856 018 441 569 970 757 243 738 306 286 803 194 347 613 280 909 888 579 \ \backslash  
 036 583 391 333 179 403 615 724 698 037 667 458 197 924 969 864 432 563 112 528 561 343 413 023 123 \ \backslash  
 390 680 522 752 436 598 290 380 862 394 768 882 112 758 044 960 550  $q^{7445} +$   
 10 226 417 019 152 546 402 206 675 268 811 286 872 535 892 587 226 933 601 718 403 284 950 618 902 \ \backslash  
 647 575 747 955 857 504 029 633 718 780 226 596 618 053 884 820 208 430 414 852 849 363 123 537 974 \ \backslash  
 341 268 589 062 207 842 033 719 386 155 635 094 991 048 553 694 805 504  $q^{7448} -$   
 10 553 224 943 747 939 558 782 567 916 621 299 787 849 342 239 944 744 322 148 872 824 553 000 301 \ \backslash  
 204 029 552 620 280 889 325 877 729 684 410 170 777 797 553 908 570 233 448 994 277 442 047 022 678 \ \backslash  
 979 904 168 580 799 143 666 101 638 796 326 359 870 700 065 849 344 000  $q^{7449} +$   
 11 597 511 069 587 113 532 030 934 253 298 655 058 264 677 114 861 010 969 234 645 299 063 138 714 \ \backslash  
 933 277 805 119 213 522 250 425 981 642 495 304 956 650 804 495 337 768 865 350 839 082 458 858 751 \ \backslash  
 254 833 117 466 004 941 267 238 725 418 404 052 611 939 595 474 470 912  $q^{7452} -$   
 11 968 034 523 999 702 516 282 409 362 895 829 623 879 401 452 440 664 912 704 306 469 536 411 978 \ \backslash  
 123 525 803 434 159 934 448 736 353 336 779 871 373 329 697 149 274 908 282 509 028 871 064 539 776 \ \backslash  
 674 595 996 509 248 166 386 285 821 044 543 525 521 889 588 682 349 673  $q^{7453} +$   
 13 151 989 731 844 065 876 197 515 004 827 991 968 183 737 657 513 853 902 608 378 916 297 730 982 \ \backslash  
 512 961 613 737 133 659 822 980 446 106 248 536 206 054 333 531 826 555 387 824 926 107 489 973 522 \ \backslash  
 130 696 581 943 558 776 592 634 635 130 097 928 076 867 200 315 392 000  $q^{7456} -$   
 13 572 062 242 019 944 788 179 156 296 099 544 724 244 113 218 827 532 252 137 511 815 789 067 592 \ \backslash  
 830 779 557 992 906 027 547 347 274 087 760 917 522 433 826 739 424 192 747 924 251 963 728 457 348 \ \backslash  
 061 341 233 811 229 201 927 576 126 483 925 005 049 103 417 318 998 016  $q^{7457} +$   
 14 914 321 704 941 382 002 042 610 784 474 719 194 675 251 287 267 413 422 850 717 693 508 517 681 \ \backslash  
 705 144 550 433 653 650 929 532 306 352 871 087 636 274 908 854 876 976 244 203 374 975 899 342 864 \ \backslash  
 135 466 614 954 461 341 244 636 601 788 552 707 501 659 935 218 073 600  $q^{7460} -$   
 15 390 553 364 295 906 270 347 377 690 565 157 132 764 105 764 960 656 335 262 931 750 827 276 705 \ \backslash  
 110 851 512 578 740 115 802 048 100 274 709 391 606 742 988 054 591 438 373 768 504 899 461 468 586 \ \backslash  
 672 992 344 590 504 900 820 063 577 588 896 911 904 864 720 010 088 750  $q^{7461} +$   
 16 912 232 642 189 820 159 323 408 152 339 556 432 074 329 714 625 912 173 986 976 304 396 598 923 \ \backslash  
 068 457 245 289 578 704 384 300 302 734 843 923 961 375 968 706 011 008 318 796 045 257 812 943 011 \ \backslash  
 406 936 017 673 719 803 523 817 244 458 409 203 983 460 265 412 096 000  $q^{7464} -$   
 17 452 113 240 506 781 300 029 804 685 553 734 991 038 464 232 805 682 870 005 739 901 613 449 338 \ \backslash  
 437 455 199 968 395 833 639 982 537 384 990 663 361 915 666 899 404 433 460 879 784 908 324 830 872 \ \backslash  
 188 778 983 405 940 961 321 718 685 341 243 364 916 988 561 334 272 000  $q^{7465} +$   
 19 177 137 630 866 850 747 829 260 096 384 662 108 170 729 291 933 181 135 619 962 866 538 057 938 \ \backslash  
 109 091 755 389 842 337 078 559 631 433 546 581 883 123 260 901 009 883 054 328 304 040 580 449 399 \ \backslash  
 179 142 385 404 897 936 321 157 840 496 242 972 849 483 859 197 528 576  $q^{7468} -$   
 19 789 153 445 854 413 471 404 657 140 018 699 042 678 574 475 861 524 940 630 630 242 306 958 080 \ \backslash  
 103 240 689 989 685 893 775 419 399 194 329 759 275 990 258 506 666 611 468 921 688 575 118 319 057 \ \backslash  
 884 766 718 438 533 408 629 058 097 231 749 474 769 441 190 080 341 125  $q^{7469} +$   
 21 744 630 961 181 849 020 330 659 472 046 015 077 509 311 653 358 866 646 306 642 829 278 145 683 \ \backslash  
 527 414 365 542 281 835 507 642 962 409 936 830 642 306 143 755 991 713 817 858 275 446 765 645 861 \ \backslash  
 318 101 679 817 331 652 642 138 348 347 919 580 969 900 467 411 095 552  $q^{7472} -$   
 22 438 397 018 378 544 388 642 228 375 849 743 927 932 772 761 000 511 618 321 076 764 784 508 096 \ \backslash  
 355 312 298 668 961 629 569 059 954 103 863 843 061 218 506 956 957 845 313 282 906 522 636 275 047 \ \backslash  
 768 524 367 848 167 297 569 123 582 181 452 228 152 300 799 095 734 272  $q^{7473} +$

24 655 040 755 220 969 747 752 714 550 066 703 910 306 447 483 908 513 704 162 860 085 712 211 275 \
 169 306 997 928 872 901 449 421 195 192 021 046 565 225 031 239 264 237 768 019 672 114 967 422 613 \
 612 432 130 077 367 961 887 366 865 116 358 503 487 898 003 538 944 000  $q^{7476}$  -

25 441 450 600 016 495 362 193 345 516 198 114 060 019 811 337 138 611 124 831 578 448 755 786 813 \
 970 523 456 302 215 274 511 249 837 140 821 861 111 628 614 683 785 228 440 173 628 780 583 321 553 \
 551 336 884 039 176 694 581 157 073 443 092 789 873 413 653 398 871 383  $q^{7477}$  +

27 954 057 024 609 295 044 484 624 342 354 164 807 981 348 619 180 801 436 426 284 805 254 938 329 \
 368 478 138 556 847 294 822 850 095 267 827 204 566 901 083 825 018 865 458 364 260 115 323 748 267 \
 492 586 659 927 720 870 924 535 984 906 368 537 145 992 013 485 158 400  $q^{7480}$  -

28 845 452 319 529 401 655 270 642 528 246 875 377 949 955 581 782 569 573 600 302 506 311 870 967 \
 187 575 987 593 794 059 660 670 896 442 130 123 107 447 536 495 617 113 889 929 664 730 254 741 020 \
 332 776 854 985 551 897 742 883 234 557 813 504 108 108 428 201 984 000  $q^{7481}$  +

31 693 442 854 934 360 769 733 052 102 991 584 844 339 176 860 506 697 258 573 401 161 762 107 366 \
 923 219 679 449 283 179 846 594 012 825 432 965 730 136 545 867 740 677 604 062 196 009 192 387 145 \
 522 696 547 660 834 104 187 215 801 260 783 197 613 694 249 497 088 000  $q^{7484}$  -

32 703 805 420 145 357 217 064 680 082 523 367 918 501 330 210 198 247 807 043 853 756 652 908 723 \
 579 559 664 752 186 743 021 693 836 496 574 333 717 496 600 146 695 298 638 128 139 730 270 030 981 \
 251 656 022 444 288 818 938 016 144 916 120 433 226 807 065 074 977 650  $q^{7485}$  +

35 931 839 692 759 728 932 894 052 696 429 890 779 966 358 646 801 769 898 170 270 677 486 312 213 \
 838 525 979 247 945 678 580 916 341 666 701 981 892 424 016 955 352 329 556 289 761 564 662 975 812 \
 870 362 665 116 115 750 309 138 823 195 661 220 733 996 104 114 372 608  $q^{7488}$  -

37 077 008 952 622 577 350 521 036 161 238 603 486 422 220 430 529 814 825 526 869 607 281 314 041 \
 761 421 825 227 126 645 017 536 601 579 076 330 512 354 515 908 783 845 370 569 211 725 714 973 067 \
 575 791 574 363 155 172 168 724 075 741 119 635 846 824 281 415 680 000  $q^{7489}$  +

40 735 679 156 794 484 111 308 656 638 861 642 905 224 646 695 619 293 768 905 602 424 858 803 815 \
 095 337 632 010 007 279 430 156 749 232 194 027 826 190 852 940 024 803 769 641 490 847 789 924 082 \
 145 017 411 675 458 202 725 105 491 679 291 677 195 525 859 990 814 720  $q^{7492}$  -

42 033 598 345 495 587 454 765 956 143 063 779 431 540 989 908 377 042 917 382 731 857 825 884 168 \
 165 207 418 114 412 788 184 907 525 444 033 311 142 038 361 625 786 772 163 261 362 652 400 187 746 \
 671 935 156 808 094 024 987 934 671 044 542 010 201 536 071 756 832 112  $q^{7493}$  +

46 180 215 430 497 178 572 928 925 911 307 257 254 844 898 729 820 343 591 444 292 233 236 588 919 \
 098 354 096 461 506 112 605 866 609 805 736 101 278 737 230 511 319 443 257 279 355 957 441 409 713 \
 533 797 209 181 580 647 610 443 975 793 376 755 570 147 871 172 096 000  $q^{7496}$  -

47 651 210 351 244 702 114 715 790 991 336 402 279 460 330 866 665 308 546 570 258 540 017 995 583 \
 375 264 587 563 053 499 684 265 792 463 539 486 853 726 388 666 686 649 933 908 378 143 376 746 848 \
 361 983 094 005 089 632 904 210 864 100 195 170 124 441 747 192 184 832  $q^{7497}$  +

52 350 694 143 984 429 754 011 921 679 177 971 803 749 450 331 759 438 219 658 746 554 014 420 828 \
 344 360 210 010 168 457 095 090 103 873 937 232 942 156 804 182 089 454 473 384 785 391 579 595 281 \
 014 345 810 196 091 848 269 681 262 465 295 815 991 017 994 068 416 000  $q^{7500}$  -

54 017 788 775 704 398 392 329 923 144 616 212 240 489 274 598 333 290 973 014 982 999 569 376 485 \
 583 274 746 632 761 364 026 563 925 864 208 157 181 277 233 745 864 510 867 253 586 493 657 557 531 \
 230 262 859 658 994 456 522 237 887 675 974 895 917 408 376 940 697 875  $q^{7501}$  +

59 343 675 746 745 425 590 558 631 363 526 470 510 623 185 317 772 739 822 399 295 414 650 791 609 \
 961 428 506 066 534 822 682 723 942 257 119 527 168 323 372 422 190 743 617 612 208 805 809 039 510 \
 165 704 540 131 425 877 136 534 130 469 631 626 484 288 359 301 120 000  $q^{7504}$  -

61 232 949 557 238 478 473 433 998 564 435 330 260 867 046 012 979 906 434 266 893 879 248 395 114 \
 011 325 973 285 789 626 163 097 860 002 592 396 924 082 583 485 023 708 124 754 507 046 090 503 875 \
 149 060 291 231 886 019 533 226 883 006 202 925 315 884 037 573 836 800  $q^{7505}$  +

67 268 533 741 175 979 573 956 863 607 083 960 331 233 984 291 348 554 288 451 242 706 003 790 971 \
 557 724 833 078 368 662 788 117 590 151 374 948 064 507 749 468 232 397 946 978 931 494 575 144 728 \
 406 868 667 962 864 134 040 311 525 316 539 699 954 567 523 114 821 632  $q^{7508}$  -

69 409 526 204 894 242 783 846 431 459 750 051 016 103 667 251 598 689 704 210 255 961 133 476 714 \
 486 523 428 798 295 518 646 361 601 441 290 787 800 523 348 962 554 637 470 318 799 055 883 998 485 \
 875 477 908 496 789 206 296 039 549 864 344 394 735 117 659 918 441 375  $q^{7509}$  +

76 249 150 826 343 254 289 423 217 862 976 699 165 936 877 162 742 500 379 592 169 652 290 367 267 \

111 810 294 241 959 258 795 278 165 678 776 774 859 383 286 163 263 436 730 848 312 110 890 531 966  
 496 351 111 438 248 186 093 161 497 339 540 499 472 376 476 147 353 600  $q^{7512}$  -  
 78 675 319 368 030 637 860 985 703 585 200 890 266 722 999 507 619 896 932 599 062 737 303 596 724  
 660 886 093 470 007 414 405 610 385 808 517 307 855 639 575 485 074 002 116 917 097 141 490 754 728  
 868 714 993 343 565 224 887 463 397 344 979 719 022 230 767 434 366 976  $q^{7513}$  +  
 86 425 839 032 383 039 600 392 430 463 597 077 245 865 953 891 658 300 860 721 671 952 023 592 105  
 772 751 161 940 688 569 615 470 725 497 851 745 476 869 618 809 820 489 976 742 559 065 495 925 431  
 046 374 885 061 308 387 506 486 225 271 439 324 560 337 077 275 904 000  $q^{7516}$  -  
 89 175 077 435 773 682 782 666 506 094 572 050 761 155 115 755 265 658 232 273 734 446 756 375 032  
 660 435 075 597 235 599 626 458 327 579 521 244 919 243 735 471 905 400 994 300 554 664 823 352 328  
 238 416 163 868 378 632 556 477 098 673 461 587 477 230 064 992 371 596  $q^{7517}$  +  
 97 957 513 354 541 408 962 721 113 302 654 438 978 617 738 040 867 151 544 730 050 689 287 863 283  
 831 288 085 930 274 462 934 566 209 825 430 644 475 705 788 258 397 539 114 885 438 567 414 395 944  
 919 140 129 979 234 063 893 179 827 267 500 472 543 332 843 777 433 600  $q^{7520}$  -  
 101 072 738 600 546 658 656 923 956 408 046 713 813 992 021 508 994 347 478 308 859 542 870 821 052  
 271 148 919 424 654 643 657 983 511 532 310 663 361 991 809 088 140 850 277 857 742 875 919 067 592  
 071 941 757 988 062 691 824 320 704 441 891 170 889 693 079 379 968 000  $q^{7521}$  +  
 111 024 152 274 138 224 067 512 854 404 508 225 672 870 757 660 791 756 062 565 217 574 871 441 099  
 332 319 990 072 939 816 950 953 584 678 520 618 322 135 273 373 319 432 412 216 293 933 053 333 609  
 942 957 334 029 116 251 538 990 497 829 331 171 884 651 381 209 088 000  $q^{7524}$  -  
 114 553 968 819 510 362 032 495 858 573 365 572 833 794 017 976 002 672 574 527 670 511 279 162 820  
 277 820 665 767 639 753 914 769 435 424 030 519 362 983 562 507 547 631 958 380 985 342 262 009 417  
 742 225 344 538 340 911 593 965 272 868 767 500 218 186 966 095 117 950  $q^{7525}$  +  
 125 829 582 940 481 584 920 100 924 357 836 392 169 834 736 898 216 706 422 123 415 193 067 763 063  
 794 218 126 630 585 681 821 239 078 626 214 340 921 372 681 642 527 866 197 593 627 609 684 468 863  
 888 260 534 759 914 887 591 078 711 710 973 931 670 328 882 251 437 568  $q^{7528}$  -  
 129 829 034 631 692 882 786 561 114 145 882 100 498 368 289 175 063 351 967 519 162 703 641 921 500  
 761 258 057 788 485 380 847 493 605 105 738 065 855 747 428 175 057 063 411 637 570 889 197 047 078  
 571 010 110 239 898 526 027 589 407 400 055 230 914 328 153 092 096 000  $q^{7529}$  +  
 142 604 633 749 508 777 645 800 530 584 091 210 526 477 993 553 108 829 345 559 263 432 501 382 898  
 553 156 132 803 662 258 483 967 516 177 510 728 411 838 192 144 487 923 828 557 702 134 045 633 084  
 763 487 059 911 348 070 259 965 943 786 895 810 817 865 237 244 484 608  $q^{7532}$  -  
 147 136 054 905 468 779 331 117 089 188 485 869 187 334 597 241 350 797 157 598 104 987 008 582 644  
 695 281 804 251 858 895 890 700 243 266 780 943 352 744 286 646 993 504 774 577 287 351 585 737 298  
 597 967 878 571 084 877 417 163 385 708 065 594 150 173 285 025 796 527  $q^{7533}$  +  
 161 610 702 666 857 797 692 933 234 095 517 970 995 018 122 710 990 781 554 336 500 828 490 428 563  
 494 547 631 119 598 818 037 925 853 555 358 338 392 962 186 479 032 911 166 455 166 957 393 455 368  
 683 815 481 872 855 725 702 913 354 267 548 583 135 088 986 654 720 000  $q^{7536}$  -  
 166 744 681 378 392 116 115 155 945 433 205 614 957 358 824 342 367 264 932 053 293 755 850 410 265  
 080 502 848 886 499 903 432 308 991 210 013 107 506 265 480 909 331 925 078 302 951 279 085 155 390  
 962 009 712 662 581 712 374 045 362 002 493 674 818 314 352 568 008 704  $q^{7537}$  +  
 183 143 795 990 179 447 351 258 382 551 241 440 678 303 195 496 150 438 173 612 000 099 883 425 170  
 372 397 784 497 414 789 676 855 350 390 938 174 792 920 344 710 865 530 852 575 142 955 157 903 046  
 726 634 774 175 308 767 428 393 602 236 891 005 367 078 932 377 190 400  $q^{7540}$  -  
 188 960 264 396 837 253 066 213 481 911 138 689 622 492 516 277 435 442 299 036 197 983 545 679 392  
 122 844 958 794 864 574 921 115 109 172 124 708 384 475 954 095 967 993 086 474 567 292 007 400 768  
 494 947 380 064 830 279 663 401 074 273 894 883 875 105 543 540 961 250  $q^{7541}$  +  
 207 539 099 423 863 126 144 989 001 274 814 451 151 034 387 065 793 528 608 412 907 310 566 302 325  
 776 223 605 591 367 048 063 099 985 797 365 893 056 337 934 364 465 835 313 727 596 384 850 834 068  
 099 053 010 127 296 920 606 718 476 181 212 859 031 969 745 455 104 000  $q^{7544}$  -  
 214 128 567 665 524 859 542 281 309 506 246 301 988 921 781 358 213 853 566 398 214 205 762 327 498  
 301 315 804 800 406 518 071 843 815 233 578 258 144 292 259 658 753 107 938 307 759 849 558 778 995  
 248 321 873 145 503 578 074 225 966 384 751 009 990 690 272 727 859 200  $q^{7545}$  +  
 235 176 151 457 576 131 948 455 415 550 741 931 757 304 642 986 889 841 002 120 139 730 467 528 334  
 049 241 642 073 008 315 587 266 597 031 468 876 531 507 088 358 320 417 945 351 417 305 004 881 249

668 052 827 125 050 053 083 883 530 687 511 545 243 369 159 096 827 904  $q^{7548}$  -  
 242 641 104 188 793 145 206 893 460 200 177 646 433 286 655 802 890 171 813 064 277 147 002 356 367 -  
 638 657 436 252 186 419 370 621 579 648 747 604 027 912 227 335 894 742 984 252 541 922 391 561 824 -  
 451 215 503 993 232 592 982 728 685 813 512 604 872 068 418 165 302 375  $q^{7549}$  +  
 266 484 698 220 868 802 114 211 840 210 905 302 864 004 568 381 567 185 210 046 368 566 333 120 763 -  
 023 367 433 369 464 174 945 243 817 926 086 412 395 565 508 817 149 530 566 115 346 512 935 551 359 -  
 792 910 407 621 941 596 277 036 267 245 890 449 056 004 894 325 637 120  $q^{7552}$  -  
 274 941 175 052 995 724 617 920 134 756 345 405 429 768 915 446 214 653 864 543 728 551 308 709 334 -  
 404 436 864 589 591 265 635 883 004 217 820 598 745 799 700 550 640 063 731 297 315 913 529 942 180 -  
 401 172 142 853 445 225 874 240 363 748 057 656 713 534 266 504 183 808  $q^{7553}$  +  
 301 951 319 368 334 909 315 264 140 755 669 750 848 664 172 323 409 288 706 583 855 547 564 197 442 -  
 251 646 857 891 565 500 246 296 632 579 049 309 303 777 275 717 736 304 615 050 480 048 754 151 367 -  
 347 203 882 533 855 599 446 577 208 698 840 389 556 422 739 021 824 000  $q^{7556}$  -  
 311 530 703 405 740 692 334 920 421 169 096 507 022 708 987 051 737 251 617 329 514 661 256 270 973 -  
 490 715 763 323 883 264 560 490 504 429 365 607 423 324 391 988 423 404 141 593 720 859 467 192 018 -  
 952 855 250 383 338 691 767 705 657 577 903 752 021 531 478 708 744 715  $q^{7557}$  +  
 342 126 926 290 273 126 256 379 076 462 795 365 011 321 990 634 774 476 917 655 976 127 303 927 618 -  
 104 438 308 187 942 165 948 501 041 077 176 882 000 011 268 022 185 250 648 373 117 025 633 957 633 -  
 308 743 939 590 941 481 522 394 285 673 455 537 511 582 624 388 096 000  $q^{7560}$  -  
 352 977 968 094 539 897 621 324 524 071 202 034 117 449 550 145 477 069 698 046 516 524 693 046 924 -  
 074 235 197 666 112 620 071 455 838 761 076 919 828 636 867 648 246 362 917 916 725 138 057 317 324 -  
 882 409 490 554 736 370 956 974 454 260 962 589 422 701 935 845 376 000  $q^{7561}$  +  
 387 635 247 219 730 924 237 273 568 878 894 304 979 861 544 973 147 317 184 085 588 443 314 200 438 -  
 522 796 679 411 572 092 199 782 673 152 309 310 782 433 467 714 416 988 782 892 183 264 797 673 205 -  
 985 572 803 607 656 862 071 358 589 649 593 934 392 158 676 416 128 000  $q^{7564}$  -  
 399 926 355 117 581 095 673 002 838 837 381 152 684 037 517 921 603 265 445 094 061 356 977 565 738 -  
 137 277 231 640 936 480 602 555 327 914 587 877 032 036 679 710 682 026 327 055 331 990 730 502 415 -  
 367 559 748 906 867 144 545 650 055 698 504 827 399 671 145 956 710 950  $q^{7565}$  +  
 439 182 428 818 565 584 712 809 293 269 707 969 494 378 428 959 918 374 277 040 449 465 122 189 614 -  
 007 904 235 164 632 637 540 305 709 777 463 410 061 277 546 020 322 024 409 479 158 457 609 591 019 -  
 876 605 722 050 568 831 135 935 697 193 220 825 529 944 238 579 122 176  $q^{7568}$  -  
 453 104 260 519 330 929 508 703 586 557 553 233 672 745 241 994 308 670 553 327 454 413 600 016 077 -  
 829 178 764 828 836 820 548 230 655 311 913 238 397 986 796 867 748 050 074 856 810 236 303 716 006 -  
 553 495 292 453 468 838 875 481 151 309 919 808 974 139 466 141 696 248  $q^{7569}$  +  
 497 567 900 799 143 093 963 104 750 817 804 503 631 576 399 733 298 202 130 748 657 633 121 729 051 -  
 574 389 772 483 797 117 458 668 972 704 159 294 185 340 371 569 563 996 035 666 925 398 235 656 445 -  
 235 311 773 494 757 568 722 089 695 836 610 982 196 859 541 927 677 952  $q^{7572}$  -  
 513 336 295 866 970 518 404 580 871 383 260 564 687 666 441 896 534 521 588 685 056 457 144 212 990 -  
 306 960 676 539 173 819 337 768 527 353 475 186 254 913 738 157 535 073 283 213 693 815 883 964 417 -  
 898 179 579 885 641 150 688 353 392 389 190 458 890 063 030 937 567 992  $q^{7573}$  +  
 563 696 669 330 392 023 959 426 360 498 401 735 869 663 629 649 751 874 846 062 661 346 953 987 414 -  
 596 008 879 259 747 868 963 629 331 188 262 154 628 800 840 603 610 011 387 079 331 492 692 309 573 -  
 418 047 927 170 726 389 934 127 481 114 434 429 047 900 758 477 376 000  $q^{7576}$  -  
 581 555 967 234 080 153 513 245 505 585 266 332 584 730 476 627 723 577 051 916 957 355 814 452 908 -  
 251 587 859 551 819 776 908 180 197 482 854 957 072 735 610 737 831 312 124 278 794 833 894 387 389 -  
 805 966 197 332 900 612 639 862 264 103 507 130 706 866 851 477 094 400  $q^{7577}$  +  
 638 593 226 676 300 678 687 800 537 637 101 760 291 489 553 188 728 675 236 503 996 138 626 568 467 -  
 540 640 327 994 814 074 431 571 077 371 822 295 452 896 812 756 219 031 190 477 562 074 634 849 976 -  
 058 232 378 213 980 023 607 086 579 697 511 440 631 864 111 421 900 800  $q^{7580}$  -  
 658 820 020 993 665 920 310 026 686 374 887 671 910 639 249 049 054 570 164 211 362 313 463 721 107 -  
 868 926 621 031 812 382 869 557 010 619 992 703 200 570 729 462 702 592 791 789 929 424 281 316 098 -  
 131 108 795 874 436 257 540 306 508 354 618 632 763 910 819 746 958 625  $q^{7581}$  +  
 723 417 289 048 363 545 981 375 724 947 758 044 259 784 943 880 424 006 500 829 205 838 465 190 808 -  
 131 096 263 563 835 557 396 594 658 526 136 080 902 827 929 371 125 532 505 131 716 734 431 761 713 -  
 901 811 133 573 058 145 325 587 756 966 202 321 560 613 899 404 288 000  $q^{7584}$  -

746 324 675 020 471 532 777 656 845 072 809 777 215 833 251 419 547 396 971 861 182 498 082 620 810  
 155 696 300 110 498 801 974 050 380 027 863 880 325 883 908 221 417 664 505 935 297 985 104 997 773  
 921 422 970 025 738 246 416 545 844 864 858 069 064 576 124 393 881 600  $q^{7585} +$   
 819 481 602 390 205 640 209 763 926 873 239 550 721 968 536 909 176 353 902 385 525 630 022 895 553  
 718 374 083 688 669 405 923 558 751 832 255 660 770 654 519 519 694 222 638 758 206 441 276 898 439  
 470 040 876 351 648 811 432 230 306 889 862 770 287 668 455 094 681 600  $q^{7588} -$   
 845 423 982 503 257 778 726 134 955 070 483 473 281 144 774 407 871 679 422 263 756 756 510 077 981  
 916 719 466 001 558 802 498 997 907 316 051 468 555 807 515 669 042 688 204 539 753 217 557 308 725  
 412 255 457 457 864 395 523 064 314 145 811 202 114 241 638 986 671 750  $q^{7589} +$   
 928 272 087 169 896 183 999 644 926 754 011 454 300 310 335 091 394 867 819 804 073 013 647 277 591  
 071 872 262 736 290 892 703 060 839 360 574 621 897 390 459 880 359 890 981 255 457 350 390 344 952  
 789 203 460 144 797 590 802 522 502 932 828 664 981 585 392 544 420 864  $q^{7592} -$   
 957 650 607 901 557 310 512 793 534 579 077 491 461 845 700 993 496 188 587 336 059 995 542 530 638  
 967 394 999 176 319 151 479 936 121 974 552 291 275 037 418 320 378 556 209 285 335 692 536 461 815  
 149 869 522 556 241 361 553 469 900 138 966 367 728 246 219 679 236 096  $q^{7593} +$   
 1 051 470 628 704 783 105 746 443 136 573 475 914 899 405 916 414 005 074 208 666 293 391 419 558 214  
 522 303 131 063 608 006 619 240 985 446 698 449 384 904 250 388 822 150 008 775 602 552 354 476 254  
 969 952 480 819 713 003 833 737 298 912 326 022 679 404 306 889 920 000  $q^{7596} -$   
 1 084 739 331 134 420 914 054 312 654 659 614 336 912 187 727 909 754 873 459 885 835 517 551 142 297  
 167 568 197 648 068 438 645 034 703 566 305 198 673 863 328 406 868 049 826 389 566 912 491 188 667  
 023 424 661 657 256 909 424 548 646 274 188 469 927 834 500 545 092 418  $q^{7597} +$   
 1 190 980 859 617 764 333 462 013 382 720 608 292 073 518 524 180 924 560 616 837 788 868 277 574 156  
 332 201 954 344 739 374 053 963 374 453 922 975 588 800 282 122 823 732 473 154 780 990 275 981 405  
 869 032 588 042 054 131 917 657 890 676 827 300 411 807 172 350 668 800  $q^{7600} -$   
 1 228 653 637 410 105 145 060 141 593 986 217 617 943 046 112 688 515 065 526 448 234 603 231 882 734  
 361 891 613 353 064 146 277 390 329 867 755 698 217 930 335 660 877 833 892 120 960 341 924 748 489  
 591 869 596 669 479 711 010 876 484 112 054 761 439 719 593 406 464 000  $q^{7601} +$   
 1 348 957 326 324 676 837 002 440 895 776 561 164 105 310 226 509 188 395 817 234 055 249 532 963 105  
 486 783 712 716 654 032 818 651 976 885 286 958 546 823 131 911 848 818 925 386 323 614 259 589 592  
 320 662 517 124 708 172 445 658 809 201 821 907 580 417 250 849 024 000  $q^{7604} -$   
 1 391 615 796 816 081 337 521 602 794 535 822 263 207 698 898 944 673 964 403 546 712 925 361 618 920  
 792 107 880 087 100 381 879 076 006 491 252 747 645 180 839 330 831 435 444 173 288 202 078 914 741  
 584 266 067 281 691 874 191 813 380 340 773 872 081 207 294 640 681 670  $q^{7605} +$   
 1 527 838 482 659 999 073 854 818 884 959 952 998 118 495 445 626 549 350 997 291 455 820 327 057 410  
 488 475 822 287 277 724 997 829 386 207 510 017 088 177 624 609 101 067 275 046 875 602 442 262 313  
 945 858 235 245 572 791 559 222 372 292 020 799 298 358 027 463 451 648  $q^{7608} -$   
 1 576 140 890 589 313 412 324 365 759 192 504 594 160 031 771 826 340 368 174 785 442 748 368 928 698  
 898 689 850 747 592 221 035 614 505 800 038 222 612 104 399 982 868 356 672 868 311 056 326 291 980  
 879 596 009 182 805 831 095 690 700 549 172 331 795 570 341 855 232 000  $q^{7609} +$   
 1 730 384 011 630 672 806 222 195 713 337 825 530 214 820 556 003 054 441 157 696 249 773 489 265 497  
 024 095 323 998 566 468 892 380 037 493 520 638 989 831 920 925 849 736 792 617 588 597 754 629 364  
 964 545 038 088 400 582 684 973 891 317 605 821 472 952 396 214 384 640  $q^{7612} -$   
 1 785 075 300 669 603 200 995 234 668 574 826 198 758 876 113 857 601 671 631 729 510 619 188 363 539  
 881 410 447 960 893 848 090 200 485 770 757 986 910 337 227 390 780 086 794 010 691 721 425 283 926  
 715 532 192 651 859 688 004 419 610 305 332 764 624 673 715 687 661 452  $q^{7613} +$   
 1 959 717 041 713 610 190 697 086 632 837 614 792 597 067 291 336 284 188 494 931 627 872 719 239 801  
 360 807 716 434 114 775 918 775 032 168 362 845 021 101 182 725 985 453 446 733 009 068 943 976 549  
 170 789 467 584 241 376 849 243 673 871 174 337 681 758 509 039 616 000  $q^{7616} -$   
 2 021 640 246 598 873 431 946 908 274 082 465 371 601 412 784 346 242 162 940 602 881 291 895 347 527  
 276 155 055 529 510 450 859 795 561 241 696 145 378 315 182 528 320 912 816 062 950 994 880 647 722  
 330 547 479 625 030 030 529 425 378 363 144 189 677 156 707 413 295 104  $q^{7617} +$   
 2 219 371 898 062 032 084 963 395 433 966 340 163 534 165 776 743 058 588 245 699 618 588 501 644 809  
 374 613 023 921 390 429 968 217 700 025 687 881 507 828 433 068 755 911 043 098 318 168 188 751 697  
 185 724 544 759 548 386 391 482 961 073 669 615 774 639 099 136 409 600  $q^{7620} -$   
 2 289 481 030 077 582 491 589 370 840 601 057 837 159 925 397 657 197 393 948 284 281 276 523 665 905

110 745 734 929 966 409 105 238 217 105 748 867 888 799 407 187 430 200 645 712 834 797 631 477 307 3  
 293 727 252 032 137 937 885 946 212 832 976 604 642 651 750 338 050 250  $q^{7621} +$   
 2 513 348 112 567 046 136 523 030 187 300 367 619 605 915 493 493 454 122 299 395 084 810 864 601 853 3  
 424 571 571 924 651 556 192 569 601 329 973 181 256 744 372 694 619 955 070 150 201 861 048 107 531 3  
 095 401 907 467 687 105 609 133 111 883 272 456 676 164 994 048 128 000  $q^{7624} -$   
 2 592 722 733 668 194 897 946 567 559 789 928 019 236 631 300 749 273 091 892 736 496 644 904 299 194 3  
 104 751 378 804 341 313 143 747 708 570 716 631 070 457 434 547 880 797 687 388 863 869 042 647 765 3  
 550 185 905 607 413 617 123 612 590 306 412 025 235 177 244 721 152 000  $q^{7625} +$   
 2 846 171 511 185 330 332 505 875 457 978 983 260 594 573 055 529 229 128 221 038 876 484 129 269 571 3  
 647 151 623 181 580 177 494 125 933 692 703 360 603 730 058 126 292 731 961 310 661 193 462 707 331 3  
 883 876 442 011 195 595 622 712 783 223 306 550 309 292 761 929 974 272  $q^{7628} -$   
 2 936 033 217 535 006 063 538 179 123 931 997 489 911 711 631 147 531 686 641 526 153 252 387 729 827 3  
 416 496 558 075 565 967 296 990 277 797 116 767 747 880 838 624 916 197 618 652 434 292 778 463 481 3  
 135 836 797 345 577 284 609 196 705 371 367 397 354 813 457 362 774 125  $q^{7629} +$   
 3 222 963 303 705 182 517 235 407 176 223 086 325 626 825 126 997 439 700 995 573 428 225 100 228 771 3  
 489 533 574 940 534 489 808 687 778 741 279 033 248 076 439 494 527 451 803 514 731 551 366 604 673 3  
 719 581 868 363 916 320 702 537 923 386 098 625 698 603 256 895 422 464  $q^{7632} -$   
 3 324 694 368 187 118 353 815 155 048 636 434 357 484 682 902 455 817 106 856 774 852 414 667 132 300 3  
 095 442 385 132 661 198 750 957 777 769 321 663 462 209 629 186 774 594 780 997 511 826 361 266 006 3  
 419 276 324 811 914 913 743 859 756 231 766 829 879 771 171 826 302 976  $q^{7633} +$   
 3 649 518 221 778 483 263 634 688 052 038 506 688 640 970 796 487 933 470 941 474 602 886 924 233 968 3  
 079 902 278 637 713 349 702 682 490 675 093 159 530 087 671 218 331 069 083 856 562 500 838 739 935 3  
 534 158 297 448 714 487 089 437 048 907 518 501 139 576 249 144 832 000  $q^{7636} -$   
 3 764 682 677 593 332 740 338 156 791 996 567 196 147 175 231 164 614 911 661 674 863 754 498 418 897 3  
 245 611 915 627 105 418 863 298 754 685 076 538 791 768 721 557 436 523 658 657 945 723 414 618 272 3  
 026 751 128 919 963 565 921 584 568 587 850 742 182 599 869 580 419 891  $q^{7637} +$   
 4 132 392 887 399 150 363 274 604 380 741 255 892 098 799 576 402 924 693 627 776 125 370 307 411 308 3  
 393 656 003 491 332 261 511 716 453 175 893 855 072 822 193 351 076 128 249 505 973 181 833 482 895 3  
 271 799 154 187 222 735 464 940 339 873 102 007 849 761 752 771 840 000  $q^{7640} -$   
 4 262 760 371 623 783 610 664 940 090 082 193 446 714 399 065 199 565 575 223 925 393 665 537 536 206 3  
 284 390 283 481 327 180 936 761 483 506 152 785 872 899 516 914 542 406 563 741 034 017 091 624 831 3  
 104 194 183 735 265 345 470 478 785 970 070 376 907 523 090 169 856 000  $q^{7641} +$   
 4 679 005 748 096 929 171 441 420 459 150 318 828 713 382 278 504 086 179 438 209 588 976 366 753 211 3  
 418 596 191 796 793 361 073 880 989 437 099 956 639 042 711 096 442 776 377 735 513 883 522 852 536 3  
 598 971 158 613 829 423 519 114 198 616 990 761 874 970 299 655 424 000  $q^{7644} -$   
 4 826 578 465 643 777 521 845 539 477 263 096 377 605 777 421 684 527 634 670 792 247 331 796 332 194 3  
 454 654 790 521 854 178 438 295 321 703 358 075 732 842 539 559 846 733 172 691 533 746 484 519 418 3  
 008 661 584 395 113 744 576 468 019 432 465 916 563 193 151 613 283 500  $q^{7645} +$   
 5 297 750 089 240 184 030 355 121 844 477 791 789 693 190 607 094 967 736 512 208 580 399 318 055 537 3  
 412 236 216 015 433 702 744 209 974 466 716 810 566 151 530 129 116 147 846 236 505 116 676 390 151 3  
 422 108 612 277 321 596 139 289 999 535 936 578 583 692 762 898 350 080  $q^{7648} -$   
 5 464 793 304 612 939 668 111 193 096 977 184 478 151 324 615 551 883 013 858 302 976 691 234 260 169 3  
 631 254 703 733 244 429 371 060 499 773 988 222 380 168 480 768 695 569 569 084 786 658 076 760 032 3  
 207 961 450 811 368 395 147 017 153 529 091 258 071 363 700 412 416 000  $q^{7649} +$   
 5 998 121 830 601 962 136 772 111 224 047 029 982 602 098 517 688 917 854 803 613 118 128 310 907 139 3  
 798 002 701 650 256 775 893 904 806 827 095 957 722 069 183 126 795 874 367 755 080 066 852 955 733 3  
 488 600 696 181 126 355 560 654 694 395 013 048 562 705 378 339 405 824  $q^{7652} -$   
 6 187 198 347 906 960 317 445 437 919 525 714 148 841 591 903 222 186 218 606 396 719 663 828 300 794 3  
 879 146 126 528 288 581 293 715 315 051 241 039 066 257 858 716 657 790 577 589 353 633 196 881 840 3  
 590 158 487 477 418 720 946 839 985 342 773 537 734 374 825 960 399 565  $q^{7653} +$   
 6 790 864 036 675 606 461 994 457 872 700 346 585 169 860 285 871 000 386 346 033 526 046 690 127 795 3  
 348 480 787 365 909 939 553 639 761 867 074 295 680 276 809 134 933 086 803 313 745 700 773 545 802 3  
 405 078 270 687 640 202 697 793 398 732 422 776 863 313 230 525 440 000  $q^{7656} -$   
 7 004 873 188 306 256 325 918 210 540 083 019 541 027 798 022 032 640 689 900 154 889 022 942 153 866 3  
 828 643 882 349 747 963 634 652 799 633 746 781 398 671 219 399 188 157 415 824 146 982 405 161 639 3

342 628 111 579 098 544 711 058 062 632 247 469 503 674 246 324 355 072  $q^{7657} +$   
 7 688 130 321 445 026 887 031 496 289 746 909 120 218 606 738 436 482 046 807 752 934 676 750 942 954 \ \backslash  
 764 721 088 308 316 607 882 379 757 917 255 503 253 264 199 108 219 224 898 338 301 223 128 587 463 \ \backslash  
 570 580 915 799 051 242 196 140 088 022 722 114 873 208 127 961 779 200  $q^{7660} -$   
 7 930 352 053 603 528 280 097 041 613 156 793 352 965 054 341 588 116 287 051 681 755 489 823 683 084 \ \backslash  
 957 144 204 402 502 176 539 993 978 545 322 709 844 570 632 023 651 717 794 370 433 723 894 529 395 \ \backslash  
 130 225 163 627 649 790 499 711 076 110 360 349 223 799 728 064 251 500  $q^{7661} +$   
 8 703 669 612 164 665 554 772 184 432 923 686 168 738 546 535 346 909 734 996 416 660 862 985 651 892 \ \backslash  
 307 085 810 244 546 873 842 552 460 129 057 874 225 895 553 640 908 622 180 937 212 822 026 641 052 \ \backslash  
 992 639 994 834 904 598 241 470 793 692 608 967 512 738 550 415 360 000  $q^{7664} -$   
 8 977 814 331 930 361 305 096 265 993 078 769 273 959 740 862 750 838 508 299 998 723 345 605 081 738 \ \backslash  
 532 239 784 743 922 724 359 495 448 265 615 092 729 608 346 675 258 946 041 574 266 710 135 851 500 \ \backslash  
 792 192 162 061 417 547 927 186 889 541 893 354 603 184 069 774 540 800  $q^{7665} +$   
 9 853 035 057 413 656 617 279 539 499 428 623 285 213 972 298 673 639 441 046 014 859 449 836 253 915 \ \backslash  
 944 212 897 592 383 285 235 082 742 575 433 046 654 457 048 999 081 621 694 266 813 592 659 745 887 \ \backslash  
 181 215 305 956 546 519 877 543 263 265 000 131 975 526 013 781 180 416  $q^{7668} -$   
 10 163 299 992 550 636 209 694 179 015 749 798 864 963 675 487 867 165 943 440 618 633 118 123 594 \ \backslash  
 703 313 400 112 513 691 730 104 515 757 652 568 588 504 736 287 361 406 126 126 235 484 583 166 263 \ \backslash  
 789 103 732 843 432 016 289 662 315 062 798 294 223 745 850 561 054 840 625  $q^{7669} +$   
 11 153 820 227 032 762 340 256 886 876 856 187 718 328 845 529 019 390 985 882 269 799 152 270 108 \ \backslash  
 147 752 476 042 303 803 414 794 122 174 835 028 143 930 196 342 541 423 742 878 170 287 538 977 410 \ \backslash  
 922 789 950 091 837 052 947 025 893 341 248 241 758 911 647 917 459 197 952  $q^{7672} -$   
 11 504 953 147 438 006 867 862 906 056 817 887 880 115 130 274 297 474 454 960 854 405 187 796 218 \ \backslash  
 799 750 374 340 966 473 484 336 725 421 197 960 270 096 403 039 646 204 952 052 033 697 313 562 912 \ \backslash  
 033 881 137 781 792 716 546 753 996 662 735 204 283 487 842 098 099 322 880  $q^{7673} +$   
 12 625 926 160 923 584 263 675 662 010 660 089 221 536 811 075 904 699 442 507 312 358 104 891 827 \ \backslash  
 024 022 318 805 229 038 895 344 901 791 859 944 105 344 446 126 029 665 915 293 271 345 491 957 182 \ \backslash  
 386 537 597 834 626 150 869 377 028 268 346 827 755 193 546 061 930 752 000  $q^{7676} -$   
 13 023 297 421 004 615 265 291 443 419 250 403 740 917 991 428 412 014 458 386 082 043 163 402 504 \ \backslash  
 247 205 921 985 948 261 679 655 915 840 480 727 043 345 843 189 882 042 434 761 880 173 484 804 419 \ \backslash  
 409 416 229 238 261 727 034 955 241 453 027 774 931 090 092 396 155 056 196  $q^{7677} +$   
 14 291 863 286 176 224 936 319 427 538 743 409 027 904 344 947 710 563 269 263 024 792 453 045 009 \ \backslash  
 777 522 607 130 576 820 834 347 658 116 142 260 821 006 884 476 692 257 695 610 892 219 318 428 639 \ \backslash  
 088 219 091 796 390 790 714 014 535 562 198 836 971 511 155 694 174 208 000  $q^{7680} -$   
 14 741 547 272 155 264 266 801 611 520 988 500 761 190 000 549 156 658 990 980 105 976 603 778 925 \ \backslash  
 885 036 458 612 169 120 407 269 282 007 375 889 820 526 629 904 041 201 142 475 023 988 627 620 715 \ \backslash  
 466 739 563 754 320 078 519 875 317 213 642 867 154 221 614 527 688 704 000  $q^{7681} +$   
 16 177 092 744 469 451 453 676 938 763 197 202 320 213 733 229 218 518 694 683 191 547 170 182 114 \ \backslash  
 381 459 318 536 925 184 910 038 542 532 683 022 793 591 600 760 237 964 582 141 551 297 936 759 903 \ \backslash  
 637 961 140 631 013 233 368 226 503 949 444 214 603 991 687 402 082 304 000  $q^{7684} -$   
 16 685 959 951 492 871 468 267 036 856 470 112 295 011 453 145 209 047 771 864 974 494 814 776 864 \ \backslash  
 047 874 232 611 618 719 510 852 410 995 163 955 384 192 291 915 073 006 484 071 442 049 538 560 337 \ \backslash  
 328 635 880 867 957 837 862 141 528 577 317 128 552 548 540 500 338 547 925  $q^{7685} +$   
 18 310 412 261 919 793 655 101 813 858 301 378 304 695 703 958 615 427 145 016 601 713 037 027 349 \ \backslash  
 660 831 033 916 600 517 583 029 346 277 695 485 406 723 707 587 751 876 142 931 943 907 707 444 030 \ \backslash  
 867 885 030 584 654 636 263 750 563 292 257 755 943 805 717 850 388 040 960  $q^{7688} -$   
 18 886 233 384 999 788 016 615 190 506 433 421 453 730 702 112 784 559 944 769 899 600 726 532 466 \ \backslash  
 783 500 117 270 149 567 669 574 745 851 858 592 636 668 960 867 760 962 261 978 891 466 421 531 268 \ \backslash  
 102 418 799 461 308 681 021 852 246 343 082 510 723 241 983 886 802 944 000  $q^{7689} +$   
 20 724 392 360 308 457 358 065 199 603 302 117 126 441 529 045 728 012 971 919 144 274 897 613 101 \ \backslash  
 570 304 979 859 896 662 225 949 098 992 328 067 171 827 426 734 945 943 162 963 757 889 988 898 185 \ \backslash  
 523 968 153 657 497 712 580 192 440 193 097 781 621 369 202 894 761 825 280  $q^{7692} -$   
 21 375 955 962 901 163 008 489 948 300 962 559 479 335 448 060 481 316 887 644 321 093 294 583 323 \ \backslash  
 563 510 376 258 477 041 723 149 657 208 979 724 837 603 099 604 008 911 033 677 550 584 317 323 841 \ \backslash  
 214 931 214 808 427 942 976 760 686 325 662 425 333 358 052 582 493 419 373  $q^{7693} +$

23 455 869 461 784 345 546 826 398 592 359 568 196 763 642 717 532 008 088 337 690 219 021 569 415 \
 656 792 777 646 853 855 119 804 684 161 876 290 878 240 560 124 286 073 643 130 973 225 017 764 168 \
 826 101 040 842 645 264 100 021 315 623 316 280 777 967 924 072 939 520 000  $q^{7696}$  -

24 193 114 988 882 769 623 507 341 369 020 074 134 374 904 097 764 786 517 989 464 383 987 582 879 \
 185 494 627 871 794 009 655 166 043 992 366 862 041 573 753 732 887 745 947 772 595 894 074 781 716 \
 888 804 857 041 940 213 382 880 179 778 295 147 205 776 283 269 535 465 472  $q^{7697}$  +

26 546 503 289 901 768 925 369 327 386 075 022 242 822 595 710 964 332 704 158 313 084 540 121 561 \
 290 154 808 558 899 637 863 506 732 785 319 667 087 151 284 149 628 608 913 478 329 834 336 970 953 \
 459 152 867 673 666 721 807 518 391 686 928 556 352 011 017 632 585 523 200  $q^{7700}$  -

27 380 671 421 904 651 183 638 049 582 731 811 950 176 629 941 520 650 107 860 577 808 169 633 113 \
 376 505 015 727 392 813 976 375 231 320 769 858 858 905 174 148 156 573 795 011 798 506 256 393 944 \
 873 194 152 504 719 042 355 939 543 124 341 504 778 199 889 527 762 196 500  $q^{7701}$  +

30 043 406 930 817 899 788 617 765 895 075 106 029 675 389 182 149 899 016 722 953 351 051 696 325 \
 200 103 795 493 985 151 666 503 229 009 945 277 200 403 069 528 122 978 236 635 711 573 942 637 503 \
 009 108 902 041 427 398 592 641 356 647 918 461 571 119 586 331 414 080 000  $q^{7704}$  -

30 987 209 533 527 353 459 200 588 112 634 363 223 703 765 445 455 149 534 391 696 994 331 815 069 \
 540 960 150 723 556 464 149 884 830 430 318 441 741 940 225 094 921 657 010 763 285 806 307 868 700 \
 404 388 945 338 205 866 757 491 038 559 805 019 611 061 138 352 896 409 600  $q^{7705}$  +

33 999 859 003 889 881 149 356 416 280 483 664 873 153 925 659 312 974 545 733 378 431 750 857 382 \
 016 750 519 003 200 493 295 054 305 810 027 678 584 984 283 742 120 435 551 662 713 650 248 384 467 \
 085 102 776 845 637 797 822 886 826 516 636 737 969 183 654 536 205 078 528  $q^{7708}$  -

35 067 671 222 630 018 927 640 072 471 918 440 200 900 569 650 761 500 264 342 580 514 716 938 619 \
 168 262 834 765 346 508 339 887 499 821 188 622 661 463 390 398 212 367 087 010 102 684 071 797 042 \
 298 999 607 569 279 602 221 176 795 012 654 371 105 341 281 208 027 049 000  $q^{7709}$  +

38 476 108 616 853 152 756 357 346 292 596 659 762 467 158 656 782 647 576 966 580 453 192 176 760 \
 907 621 566 551 033 500 547 458 283 365 326 913 734 251 560 529 722 551 839 321 803 023 299 852 400 \
 346 019 627 100 374 027 779 429 399 378 700 174 518 937 196 077 840 113 664  $q^{7712}$  -

39 684 185 993 222 467 717 949 309 785 082 363 923 338 838 983 169 477 144 422 844 937 968 100 252 \
 130 607 380 804 321 874 963 794 204 713 899 522 220 249 109 890 168 589 539 524 322 263 485 332 900 \
 008 579 682 454 038 611 874 420 472 171 082 123 898 210 846 390 151 413 760  $q^{7713}$  +

43 540 285 165 381 785 690 088 344 447 301 638 715 130 851 595 359 132 965 328 884 359 827 393 989 \
 637 818 285 802 276 243 314 598 080 391 057 460 411 928 622 661 004 041 300 870 775 496 920 548 047 \
 932 781 510 413 020 530 980 416 981 335 997 775 065 797 664 733 935 616 000  $q^{7716}$  -

44 907 009 028 445 835 448 313 537 328 563 868 754 011 877 102 594 166 645 512 401 920 828 066 612 \
 341 595 401 430 526 061 748 836 371 514 952 650 818 198 321 052 538 705 232 219 752 135 342 680 006 \
 276 553 649 738 071 839 850 962 119 751 389 651 876 926 317 674 370 343 727  $q^{7717}$  +

49 269 426 600 618 082 169 935 213 575 033 124 144 901 510 708 681 653 862 592 508 412 901 663 547 \
 391 090 831 605 586 104 299 741 400 515 870 099 771 648 672 665 255 770 806 026 398 790 716 492 933 \
 023 086 372 983 251 759 307 687 703 702 154 983 819 002 163 651 356 646 400  $q^{7720}$  -

50 815 581 405 938 303 229 782 643 961 273 527 924 741 230 459 584 435 110 180 101 822 592 320 463 \
 838 645 201 674 872 788 222 215 538 300 097 486 290 041 029 306 690 685 776 180 949 823 001 975 873 \
 025 299 369 669 056 861 782 412 739 456 567 703 094 659 957 790 162 944 000  $q^{7721}$  +

55 750 641 554 341 586 783 339 241 412 687 483 527 214 771 027 137 537 102 469 269 572 769 504 853 \
 189 453 535 263 582 671 735 016 810 369 666 862 914 271 607 878 139 345 217 907 031 279 684 578 089 \
 359 130 025 599 719 392 122 016 346 769 821 062 368 919 120 090 246 208 000  $q^{7724}$  -

57 499 728 320 354 407 895 011 535 228 662 022 214 906 836 505 563 424 838 465 173 529 399 887 034 \
 655 443 782 937 160 441 564 490 447 784 860 325 265 268 303 775 404 575 224 031 308 023 708 651 384 \
 579 707 734 342 375 630 173 429 833 710 606 158 254 871 458 227 789 943 475  $q^{7725}$  +

63 082 422 705 934 924 657 269 746 283 534 250 385 915 784 236 775 401 881 677 664 254 005 585 380 \
 876 524 888 718 408 553 765 294 987 885 321 473 145 524 506 027 612 038 259 217 565 553 223 190 094 \
 110 072 300 587 321 850 419 106 911 456 739 158 460 630 714 800 666 296 320  $q^{7728}$  -

65 061 013 234 878 992 131 151 854 950 087 877 191 394 636 474 503 355 208 090 432 400 574 926 189 \
 232 246 443 725 351 595 042 975 684 426 661 912 778 700 540 110 073 725 906 097 288 899 581 358 366 \
 123 222 730 933 311 226 472 809 980 460 017 876 330 565 575 177 367 552 000  $q^{7729}$  +

71 376 131 027 664 976 482 566 901 468 147 154 246 223 677 946 182 061 057 536 623 938 021 782 673 \

328 130 272 576 822 223 771 515 731 262 772 313 330 885 589 615 529 859 009 314 568 677 979 276 511 \
 133 541 635 809 986 746 601 656 222 943 843 388 295 205 035 170 541 111 296 q<sup>7732</sup> -

73 614 268 205 445 280 303 692 446 334 668 439 206 691 511 978 666 637 196 462 375 247 238 341 608 \
 052 267 124 535 408 948 384 549 446 184 160 121 271 202 872 450 715 613 891 430 417 983 473 250 495 \
 601 729 545 735 517 679 878 706 500 489 006 586 347 463 306 309 088 040 039 q<sup>7733</sup> +

80 757 673 088 295 538 478 752 304 959 810 822 227 971 137 914 299 893 417 325 914 821 367 303 644 \
 716 207 939 085 712 536 228 390 199 946 144 620 728 246 284 218 149 721 593 679 751 468 306 943 945 \
 424 914 323 869 131 887 987 833 476 904 198 983 957 294 973 568 039 040 000 q<sup>7736</sup> -

83 289 323 243 335 684 833 836 004 439 598 435 505 281 336 947 481 149 060 943 446 328 363 290 278 \
 761 022 337 952 383 478 417 657 998 363 583 368 235 996 769 519 697 728 223 654 926 885 670 600 051 \
 372 183 365 738 469 903 233 688 363 084 131 993 631 589 483 437 030 539 264 q<sup>7737</sup> +

91 369 396 467 224 904 327 744 555 173 037 327 332 731 647 149 328 229 132 549 835 897 690 511 626 \
 355 744 840 790 724 264 457 064 575 410 242 366 438 361 996 410 924 950 346 042 836 459 021 066 351 \
 671 550 449 399 643 410 066 578 853 495 887 318 318 648 623 158 698 444 800 q<sup>7740</sup> -

94 232 960 542 610 221 090 123 939 275 930 715 130 260 094 119 379 618 860 123 654 515 874 184 045 \
 062 109 842 250 111 496 706 505 346 654 945 893 424 943 192 540 803 055 805 628 399 229 533 257 332 \
 719 950 533 626 249 612 993 257 541 604 680 986 265 409 729 013 092 189 875 q<sup>7741</sup> +

103 372 231 574 571 761 667 387 614 753 276 905 643 324 160 930 744 629 807 687 037 816 612 660 944 \
 128 659 606 777 680 091 813 923 014 683 700 518 644 318 708 194 808 758 971 451 227 064 048 983 690 \
 838 918 914 664 296 234 237 354 964 116 664 467 623 661 251 563 263 434 752 q<sup>7744</sup> -

106 611 122 742 045 250 152 730 446 623 393 147 036 638 527 123 148 858 264 980 994 181 012 097 822 \
 933 235 522 958 690 455 936 614 906 787 753 056 505 143 820 247 209 314 041 993 444 833 451 614 749 \
 921 564 115 259 514 088 491 879 036 918 259 661 380 884 698 096 866 099 200 q<sup>7745</sup> +

116 948 111 834 738 245 117 974 841 759 137 252 435 005 575 879 114 178 230 704 669 606 445 098 624 \
 449 288 739 783 392 716 525 889 703 794 098 113 097 904 597 666 714 219 451 040 253 175 935 615 058 \
 494 325 751 283 624 179 195 259 749 090 609 382 588 017 938 364 262 252 544 q<sup>7748</sup> -

120 611 408 166 265 906 661 828 150 921 940 487 055 467 761 116 148 992 772 324 281 397 581 101 878 \
 265 960 027 879 697 071 210 549 432 758 141 699 490 450 437 266 771 683 927 504 392 464 226 552 606 \
 237 985 879 693 930 622 234 567 124 614 793 621 254 268 207 872 475 048 750 q<sup>7749</sup> +

132 302 708 325 931 847 051 098 870 341 430 833 228 996 751 393 178 829 937 110 035 915 685 333 764 \
 763 781 232 675 305 904 619 565 298 238 058 166 121 077 629 943 439 144 852 849 572 906 878 482 348 \
 116 002 100 050 781 075 126 683 957 162 979 223 838 789 431 877 443 342 336 q<sup>7752</sup> -

136 445 890 253 147 703 021 049 576 103 165 624 044 690 165 898 113 708 410 738 409 502 665 998 479 \
 428 647 202 955 214 677 639 080 604 514 061 758 931 165 871 013 112 076 697 487 937 791 963 961 311 \
 830 558 186 347 910 265 990 343 549 226 042 921 587 846 618 166 540 730 368 q<sup>7753</sup> +

149 668 519 636 837 953 409 261 769 824 857 780 079 132 612 250 653 656 837 418 958 252 649 336 091 \
 912 933 774 877 264 880 452 724 631 873 409 130 499 215 866 426 589 905 689 962 608 069 421 568 402 \
 979 501 000 387 499 232 380 516 943 265 443 909 220 769 766 444 134 912 000 q<sup>7756</sup> -

154 354 303 187 125 505 927 232 177 677 143 548 971 757 506 912 892 439 758 277 840 400 670 741 594 \
 021 821 702 093 613 719 703 943 151 127 759 196 215 884 293 948 810 505 535 646 119 582 295 571 268 \
 571 362 788 475 714 893 233 511 744 186 963 901 005 777 195 852 109 919 617 q<sup>7757</sup> +

169 308 362 972 839 461 437 701 025 672 782 536 886 169 261 964 776 881 326 867 756 176 418 029 565 \
 238 863 441 066 011 044 644 894 358 380 296 563 925 104 764 785 816 750 734 018 130 970 027 092 390 \
 257 598 916 797 830 628 176 218 265 532 729 130 892 107 445 327 500 902 400 q<sup>7760</sup> -

174 607 641 191 627 733 889 021 064 831 014 983 744 400 518 391 489 111 438 953 568 206 145 255 224 \
 193 128 216 791 175 192 374 984 321 018 622 453 143 860 160 898 991 133 150 657 150 630 966 670 015 \
 487 080 502 375 861 221 464 463 171 633 829 833 165 629 529 119 391 744 000 q<sup>7761</sup> +

191 519 318 495 447 858 781 450 579 608 865 927 034 984 751 993 745 374 505 192 697 626 492 981 660 \
 363 838 819 833 002 510 215 065 804 720 285 759 655 497 332 318 672 232 959 402 612 250 749 234 317 \
 045 839 399 501 317 173 246 012 625 901 325 230 544 522 630 309 012 480 000 q<sup>7764</sup> -

197 512 225 068 398 139 251 993 268 401 282 660 424 252 893 862 681 393 179 861 575 988 614 166 644 \
 565 344 518 031 040 926 296 782 432 681 570 072 076 189 028 262 582 802 371 996 058 863 212 055 303 \
 079 825 208 106 807 950 607 805 816 930 366 169 995 443 647 066 223 494 425 q<sup>7765</sup> +

216 637 185 597 473 039 812 064 360 494 536 824 198 167 041 667 097 467 622 535 978 225 224 836 257 \
 690 818 145 218 952 541 920 947 842 425 378 426 373 998 942 429 189 608 326 403 171 892 092 579 351 \

255 456 411 568 430 817 057 071 794 032 751 967 693 951 711 755 264 625 152  $q^{7768} -$   
 223 414 296 497 192 877 851 599 480 755 531 188 835 239 402 426 083 762 014 217 978 933 677 187 768  $q^{7769} -$   
 499 756 103 430 230 960 213 264 260 953 863 181 829 198 630 471 937 264 956 352 302 214 331 045 586  $q^{7770} -$   
 461 820 140 913 391 028 866 147 030 736 480 380 023 654 726 162 153 472 000  $q^{7771} +$   
 245 041 517 401 688 560 500 531 475 750 945 362 242 220 146 329 205 901 013 201 639 373 992 581 267  $q^{7772} -$   
 135 102 074 053 467 215 757 179 281 157 759 392 365 511 209 447 846 278 359 894 273 026 686 340 801  $q^{7773} -$   
 900 921 523 856 979 473 147 298 051 237 179 901 878 917 176 857 964 029 952  $q^{7774} -$   
 252 705 208 428 046 412 479 612 528 497 145 971 721 841 174 655 958 655 226 172 892 161 693 700 385  $q^{7775} -$   
 049 006 305 523 391 894 982 934 315 008 971 936 603 086 219 587 540 643 645 632 286 900 551 069 312  $q^{7776} +$   
 325 165 718 148 812 684 531 647 853 097 520 037 129 847 490 890 399 329 512  $q^{7777} -$   
 277 161 308 333 796 251 160 440 813 874 707 460 410 661 398 203 049 748 725 507 576 664 392 677 006  $q^{7778} -$   
 961 169 613 961 536 724 451 394 613 476 654 041 480 238 539 523 497 939 220 567 754 289 589 368 681  $q^{7779} -$   
 350 448 042 272 877 587 719 587 235 935 887 437 925 831 839 834 907 136 000  $q^{7780} -$   
 285 827 288 724 853 388 596 554 779 486 941 316 305 302 172 062 848 308 598 964 890 697 952 560 543  $q^{7781} -$   
 512 648 250 638 136 552 008 597 130 502 520 632 001 032 228 175 144 596 663 458 279 961 041 568 429  $q^{7782} -$   
 302 545 206 735 256 192 984 863 485 492 920 517 518 495 227 935 270 961 152  $q^{7783} +$   
 313 481 419 287 114 008 970 400 387 564 958 866 801 372 014 642 902 916 044 872 152 869 659 792 745  $q^{7784} -$   
 107 218 511 022 815 498 074 963 441 930 653 300 867 199 638 641 301 712 467 795 086 530 337 249 919  $q^{7785} -$   
 690 921 216 801 358 233 070 949 523 013 030 854 159 852 627 691 464 294 400  $q^{7786} -$   
 323 280 464 183 023 257 450 100 871 682 712 905 704 551 844 582 065 601 270 688 864 670 413 823 899  $q^{7787} -$   
 323 774 164 688 601 154 760 172 898 062 105 018 602 059 511 439 537 495 176 483 484 453 186 806 636  $q^{7788} +$   
 051 420 009 823 925 599 578 639 183 652 865 864 544 682 227 804 685 052 500  $q^{7789} -$   
 354 549 835 808 493 110 784 798 706 146 163 633 021 837 113 719 689 675 555 193 428 258 474 910 874  $q^{7790} -$   
 752 430 704 127 242 904 759 847 812 024 038 040 120 521 085 014 908 004 808 329 183 132 355 198 187  $q^{7791} -$   
 008 475 088 954 629 736 738 629 339 561 238 805 205 860 252 883 249 536 000  $q^{7792} -$   
 365 629 743 291 666 739 534 834 881 832 412 293 089 506 910 323 066 469 399 973 574 020 084 740 116  $q^{7793} -$   
 176 615 230 646 904 585 191 479 784 669 350 046 625 850 959 341 580 805 625 810 126 324 328 288 055  $q^{7794} +$   
 419 302 121 291 940 402 466 536 531 634 022 184 071 006 123 589 599 232 000  $q^{7795} +$   
 400 985 867 052 606 842 953 115 064 686 233 048 202 557 908 731 324 607 352 623 692 511 562 904 038  $q^{7796} -$   
 830 880 909 839 270 089 214 589 156 145 359 586 523 874 950 133 631 050 329 760 921 643 587 425 257  $q^{7797} -$   
 151 632 388 600 400 363 125 146 114 360 196 796 782 414 207 251 716 325 376  $q^{7798} -$   
 413 513 668 807 161 551 554 238 364 443 677 801 446 619 953 528 242 819 779 728 111 598 403 265 924  $q^{7799} -$   
 833 574 345 815 039 330 874 920 785 857 580 575 620 561 683 058 715 833 938 710 182 129 223 923 359  $q^{7800} +$   
 486 518 485 631 379 932 022 537 289 420 384 943 504 728 063 306 854 790 625  $q^{7801} -$   
 453 489 407 155 560 453 756 081 319 317 143 898 935 062 140 801 196 825 398 154 532 189 343 141 494  $q^{7802} -$   
 020 495 888 955 264 565 870 860 713 705 690 312 064 937 601 919 770 449 364 638 358 082 859 951 268  $q^{7803} -$   
 492 395 514 131 096 818 321 199 874 127 327 326 642 056 760 304 003 432 448  $q^{7804} -$   
 467 653 865 536 169 322 713 135 886 693 090 905 354 289 211 107 186 642 449 466 458 667 186 527 576  $q^{7805} -$   
 314 804 655 956 991 153 108 466 263 380 460 225 201 723 308 519 128 920 896 949 400 375 905 184 209  $q^{7806} +$   
 039 295 497 760 320 459 171 869 437 564 776 129 245 079 784 111 704 506 368  $q^{7807} +$   
 512 851 396 372 529 163 133 698 135 802 104 797 336 767 194 576 504 819 520 788 920 763 314 088 898  $q^{7808} -$   
 464 886 653 193 754 986 049 716 684 731 551 840 901 937 658 965 015 948 544 061 038 722 215 523 805  $q^{7809} -$   
 727 280 328 834 120 995 154 036 909 388 899 734 513 859 674 099 418 880 000  $q^{7810} -$   
 528 865 824 902 249 827 339 801 527 684 633 439 549 810 452 159 356 675 808 776 318 797 980 460 940  $q^{7811} -$   
 720 388 921 446 607 454 068 649 992 439 257 834 624 448 040 619 830 871 064 056 784 070 654 252 468  $q^{7812} +$   
 343 623 560 852 270 415 848 252 286 108 385 156 463 762 677 650 339 760 411  $q^{7813} +$   
 579 965 637 037 729 622 385 025 309 723 420 515 545 189 513 744 896 290 509 853 866 821 217 092 675  $q^{7814} -$   
 808 572 012 494 919 681 466 112 932 454 215 546 316 558 790 363 199 420 272 814 591 193 947 078 634  $q^{7815} -$   
 651 737 042 316 582 758 538 518 046 390 042 864 018 500 398 767 935 155 200  $q^{7816} -$   
 598 071 086 128 071 417 920 479 106 565 434 086 952 996 431 804 824 123 023 113 592 979 289 451 369  $q^{7817} -$   
 985 152 479 511 921 642 788 534 390 572 598 587 698 575 247 267 698 213 863 579 185 406 848 207 484  $q^{7818} -$   
 539 887 825 146 072 164 846 645 746 797 300 985 593 520 010 226 622 464 000  $q^{7819} +$   
 655 842 139 397 821 459 087 934 449 825 979 999 374 176 956 923 595 413 192 531 368 384 194 153 223  $q^{7820} -$   
 530 873 575 526 994 859 779 787 254 369 020 196 434 032 342 979 230 895 904 833 938 445 962 407 503  $q^{7821} -$   
 365 896 782 514 030 009 116 474 217 020 888 606 681 381 242 837 853 184 000  $q^{7822} -$

676 310 994 472 133 420 038 665 200 947 346 073 703 272 446 766 269 905 872 980 374 563 355 340 304  
 203 555 665 162 654 660 412 893 053 068 679 299 798 963 270 561 207 292 877 262 160 411 977 322 249  
 959 002 180 722 088 528 878 373 167 957 820 984 450 755 176 466 390 924 450  $q^{7805} +$   
 741 622 194 934 392 904 282 455 857 996 372 118 902 487 441 437 368 255 328 900 921 202 292 678 966  
 402 725 720 733 595 425 591 055 263 021 767 393 551 057 594 372 625 844 378 359 386 923 817 001 588  
 155 301 392 310 947 194 759 721 425 482 039 115 228 507 514 976 273 924 096  $q^{7808} -$   
 764 762 240 216 419 875 566 152 605 917 534 760 215 943 066 887 462 088 930 244 947 834 867 637 691  
 185 571 807 840 111 102 643 488 883 628 693 064 602 984 894 037 359 222 767 058 704 874 344 524 744  
 974 107 929 261 128 829 334 133 122 166 448 090 910 585 927 613 440 000 000  $q^{7809} +$   
 838 595 400 257 550 272 349 939 207 563 294 548 913 286 991 788 332 981 204 762 350 816 693 887 877  
 646 669 938 579 862 966 855 617 314 187 237 430 449 216 690 523 206 516 617 380 812 135 545 797 561  
 246 473 482 212 031 907 807 719 782 162 981 799 901 205 488 409 583 058 944  $q^{7812} -$   
 864 754 408 349 629 283 125 088 053 350 673 270 494 566 846 833 675 959 406 491 086 313 350 241 039  
 023 723 991 666 134 504 691 552 783 313 252 721 090 830 610 345 473 847 183 433 283 112 439 126 365  
 329 725 547 326 630 211 956 982 394 270 205 584 573 162 956 028 633 588 694  $q^{7813} +$   
 948 218 883 393 103 528 488 840 089 712 751 169 255 249 801 791 942 992 248 276 278 996 069 627 211  
 124 220 332 831 942 750 691 044 215 175 515 734 098 369 045 224 709 800 458 150 423 126 578 584 935  
 150 500 159 007 923 641 224 505 233 796 812 868 921 043 455 034 284 160 000  $q^{7816} -$   
 977 789 798 513 252 041 878 282 141 676 341 916 239 976 734 092 872 420 246 406 894 755 996 445 819  
 953 496 673 608 707 831 922 705 807 276 681 668 344 904 076 382 170 526 144 342 486 803 957 429 176  
 078 928 178 502 018 833 203 420 553 041 049 161 723 703 386 356 078 313 472  $q^{7817} +$   
 1 072 139 016 720 371 041 685 713 977 634 522 652 718 240 027 366 665 788 726 173 419 265 589 277 694  
 725 142 258 024 056 247 232 922 654 349 217 307 129 950 941 880 686 088 929 817 406 390 193 884 585  
 763 156 911 626 207 819 557 302 389 848 889 489 389 287 887 520 349 542 400  $q^{7820} -$   
 1 105 565 808 207 583 332 778 559 372 278 915 783 492 418 875 538 660 167 656 442 093 326 008 598 438  
 464 183 010 161 406 403 995 788 379 130 671 971 972 563 004 014 040 082 272 446 798 302 112 530 516  
 237 091 566 732 404 037 261 831 744 358 138 652 670 687 466 012 054 607 250  $q^{7821} +$   
 1 212 215 937 419 906 269 622 794 324 673 008 300 894 978 450 050 281 747 920 594 325 017 177 764 414  
 278 337 868 154 340 645 248 216 811 411 972 251 147 764 078 629 374 764 571 782 144 492 217 188 620  
 519 085 222 641 933 624 828 709 956 049 885 783 480 002 884 604 641 280 000  $q^{7824} -$   
 1 250 000 209 979 928 823 981 125 696 007 305 817 594 329 590 131 744 503 557 577 496 619 227 257 990  
 385 468 023 697 182 048 914 793 850 982 042 942 969 080 226 770 072 448 425 016 109 668 423 491 425  
 416 114 236 847 334 600 940 996 814 148 955 956 792 222 686 939 258 880 000  $q^{7825} +$   
 1 370 551 237 594 767 129 388 368 018 760 275 466 083 101 223 486 957 172 483 802 490 807 713 489 548  
 936 142 834 361 545 461 509 345 892 687 848 832 999 470 808 391 399 256 959 795 178 026 716 168 713  
 063 334 120 680 235 878 543 558 998 124 536 625 057 009 799 584 420 495 360  $q^{7828} -$   
 1 413 259 695 888 395 248 378 527 058 857 989 108 187 189 797 593 521 043 345 090 637 262 135 812 234  
 011 906 868 897 805 043 247 746 773 456 027 038 064 406 736 361 225 038 827 646 498 313 624 151 429  
 592 644 411 043 848 396 755 249 998 828 974 774 293 692 547 985 945 224 000  $q^{7829} +$   
 1 549 519 232 837 928 231 280 551 382 924 932 115 795 914 700 962 129 401 414 449 012 433 037 400 135  
 388 954 551 294 754 734 718 751 133 184 508 541 533 316 600 144 804 949 365 308 218 162 674 967 325  
 299 182 535 027 306 668 850 705 469 752 968 356 735 589 303 416 997 736 448  $q^{7832} -$   
 1 597 792 110 572 785 258 309 357 716 295 458 860 462 308 571 924 798 517 325 729 075 805 072 894 640  
 115 998 891 867 531 400 374 917 490 504 513 611 746 497 437 000 476 266 701 071 518 915 719 682 490  
 439 288 058 191 479 047 806 041 705 150 168 244 709 496 550 791 395 803 136  $q^{7833} +$   
 1 751 802 270 611 752 651 680 796 754 882 207 373 534 230 728 974 073 076 506 113 231 247 026 343 670  
 019 433 306 325 604 730 153 505 381 941 288 912 309 336 725 895 362 449 461 384 198 758 442 154 809  
 991 301 902 139 822 135 818 175 095 933 258 460 891 759 745 574 062 848 000  $q^{7836} -$   
 1 806 362 848 469 664 289 571 254 931 983 700 360 948 830 370 838 562 086 814 963 067 521 797 380 842  
 762 353 312 861 973 810 697 298 437 415 281 517 672 087 799 611 679 405 187 843 008 773 919 504 448  
 162 643 574 284 591 963 907 033 442 383 416 509 539 750 119 378 838 662 132  $q^{7837} +$   
 1 980 430 599 149 650 801 097 538 682 944 217 349 707 334 726 748 464 540 471 134 592 025 110 547 047  
 170 923 291 147 614 609 046 612 831 026 865 356 525 121 073 924 265 916 356 131 333 995 661 970 855  
 766 541 476 775 084 274 884 072 273 832 719 571 319 262 886 464 504 934 400  $q^{7840} -$   
 2 042 095 951 871 593 215 044 498 291 373 852 830 358 674 477 210 646 571 266 548 073 503 875 327 842

257 582 879 303 682 874 653 123 151 858 920 856 709 120 124 089 384 393 204 248 006 892 103 318 856  
 022 786 957 934 861 486 781 873 178 153 523 849 928 963 860 348 469 248 000  $q^{7841} +$   
 2 238 827 384 549 678 090 273 983 769 565 329 725 401 333 978 883 671 665 938 721 515 805 435 789 881  
 178 463 337 373 766 139 557 475 048 604 322 996 573 544 280 878 205 928 735 750 685 290 397 437 200  
 379 487 126 768 254 689 028 491 624 241 116 316 926 097 991 738 957 824 000  $q^{7844} -$   
 2 308 520 515 541 726 290 161 185 798 449 572 092 723 310 825 792 576 575 622 678 832 785 275 940 946  
 515 948 724 794 494 368 131 858 723 479 757 470 597 448 963 927 532 001 927 404 681 632 801 406 600  
 441 283 465 730 423 624 756 163 570 296 715 079 502 213 385 360 921 251 450  $q^{7845} +$   
 2 530 859 539 279 830 615 699 561 525 866 974 014 157 199 074 553 582 766 478 398 741 893 336 977 214  
 036 471 859 208 390 311 471 021 543 518 012 550 375 744 141 959 601 244 458 922 262 837 357 729 700  
 766 929 232 341 659 287 588 741 846 162 543 553 254 901 079 343 705 575 936  $q^{7848} -$   
 2 609 623 081 459 175 630 022 979 365 089 033 861 998 041 000 865 523 430 634 262 242 319 381 009 734  
 471 158 823 026 978 390 382 777 967 063 407 940 820 364 995 562 276 442 304 814 772 067 896 918 862  
 387 312 976 246 634 366 754 650 814 690 799 207 539 856 874 816 987 136 000  $q^{7849} +$   
 2 860 895 110 554 688 589 033 968 323 965 506 397 417 945 079 863 670 372 201 388 347 402 573 480 955  
 543 317 778 871 239 952 486 790 627 034 575 018 371 050 275 055 969 741 130 504 350 674 151 428 882  
 547 704 262 242 458 896 472 126 513 850 061 145 615 176 927 502 216 014 848  $q^{7852} -$   
 2 949 906 795 120 777 946 994 868 622 378 407 864 611 687 045 523 135 870 865 712 035 827 729 719 355  
 878 101 275 227 089 502 753 344 127 569 157 061 542 832 832 915 941 113 194 625 092 335 553 844 004  
 415 163 172 783 324 431 536 390 090 824 889 168 708 325 096 745 215 494 956  $q^{7853} +$   
 3 233 868 073 212 728 379 345 141 639 995 297 996 509 464 261 165 587 474 927 462 220 534 718 267 835  
 048 820 134 771 484 828 568 552 788 837 664 783 899 269 869 647 059 767 386 963 287 018 116 494 569  
 677 789 596 252 325 710 719 147 181 602 470 733 343 820 090 770 415 104 000  $q^{7856} -$   
 3 334 458 193 938 874 167 938 017 918 103 386 192 851 901 297 245 714 745 979 994 728 580 987 776 151  
 327 966 988 420 069 697 104 517 247 275 579 987 731 973 250 083 011 531 023 851 908 757 726 157 023  
 117 222 291 478 805 078 696 814 381 235 050 071 159 663 565 745 961 205 760  $q^{7857} +$   
 3 655 351 480 221 257 427 496 767 032 633 589 910 332 330 832 608 408 362 564 660 481 089 846 993 096  
 488 448 572 529 877 902 470 923 495 587 719 304 181 660 157 288 854 803 087 742 504 322 377 560 783  
 962 928 047 178 622 494 255 943 469 203 863 726 941 999 231 007 466 086 400  $q^{7860} -$   
 3 769 022 610 093 235 433 317 408 316 198 154 523 245 403 476 532 693 366 255 195 180 434 801 428 029  
 667 626 808 552 767 274 207 024 254 942 596 086 871 378 745 311 538 861 173 387 228 594 813 007 895  
 220 023 041 606 774 968 288 453 763 349 913 549 439 175 047 458 633 285 750  $q^{7861} +$   
 4 131 640 046 338 146 625 621 118 216 080 891 284 323 175 432 969 132 537 975 467 178 365 689 793 144  
 365 426 594 613 813 204 362 619 583 047 491 487 590 584 353 920 772 788 129 143 702 980 171 278 358  
 572 530 967 870 340 364 277 325 237 249 545 997 138 892 072 846 682 752 000  $q^{7864} -$   
 4 260 089 296 343 018 530 716 379 814 291 768 436 080 233 668 795 969 312 184 361 156 764 305 388 547  
 110 688 806 778 900 282 074 680 373 417 643 696 196 967 646 155 181 247 327 872 063 901 777 581 619  
 790 695 125 195 330 982 350 490 581 857 818 788 578 207 377 233 721 753 600  $q^{7865} +$   
 4 669 843 378 544 130 450 428 773 411 278 324 766 247 123 830 956 776 779 972 433 703 299 754 969 651  
 395 948 512 692 358 453 151 832 772 125 862 028 452 774 396 556 504 362 162 732 465 288 768 418 839  
 639 304 566 475 433 154 187 173 554 175 323 892 416 056 423 947 803 328 512  $q^{7868} -$   
 4 814 987 525 613 570 006 168 864 743 762 935 817 304 927 332 174 699 965 851 294 797 677 001 582 772  
 409 101 528 137 322 630 182 401 451 194 005 548 611 279 190 525 194 040 751 688 760 705 047 945 027  
 459 876 182 938 899 923 037 044 536 104 828 387 125 884 280 895 224 288 750  $q^{7869} +$   
 5 277 991 222 630 975 164 249 581 684 640 051 973 773 913 316 560 821 722 093 363 606 313 101 605 230  
 233 996 889 784 823 159 536 371 529 183 041 597 198 262 842 389 269 113 736 024 105 568 962 706 803  
 322 181 967 433 340 686 132 196 829 791 403 975 671 399 330 390 973 415 424  $q^{7872} -$   
 5 441 995 075 708 646 115 120 196 570 882 512 439 201 756 822 595 032 485 522 549 446 443 196 318 903  
 483 878 541 856 909 492 588 691 738 169 776 753 308 530 386 952 330 798 241 874 550 362 326 994 876  
 998 528 698 832 901 342 985 220 941 673 235 769 951 798 081 618 580 307 968  $q^{7873} +$   
 5 965 152 271 049 468 067 338 957 970 193 241 600 738 241 804 022 647 083 538 604 050 325 180 199 575  
 600 865 282 976 314 536 005 718 060 222 625 855 965 575 986 177 678 269 895 076 760 450 665 688 349  
 536 809 640 672 623 032 717 671 943 013 423 767 339 543 207 427 508 224 000  $q^{7876} -$   
 6 150 460 691 590 199 864 290 532 045 920 933 242 494 128 302 938 721 820 331 403 616 493 976 387 453  
 453 728 273 606 222 706 308 923 342 707 278 123 811 568 726 445 125 693 809 932 963 250 735 692 020

943 121 301 975 426 767 695 498 685 776 041 483 991 958 194 251 619 196 810  $q^{7877} +$   
 6 741 568 275 335 296 561 609 404 269 991 885 935 773 784 953 840 991 684 217 566 235 451 747 268 317  
 671 111 097 809 454 472 738 910 161 959 058 633 940 310 236 023 062 652 994 702 544 290 069 833 746  
 550 113 753 153 901 280 631 556 368 013 349 851 508 938 961 180 678 988 800  $q^{7880} -$   
 6 950 942 321 941 239 599 478 030 788 924 273 205 980 847 521 985 983 353 439 163 950 252 711 853 865  
 165 245 446 901 770 302 567 204 877 008 101 757 438 868 922 253 415 897 235 424 247 935 231 524 226  
 744 706 463 654 705 454 174 001 530 624 110 578 654 015 226 539 114 496 000  $q^{7881} +$   
 7 618 805 430 013 608 185 227 215 204 728 628 723 421 415 631 773 700 153 299 921 518 060 100 147 780  
 931 854 284 754 628 036 569 198 883 834 823 917 062 572 198 948 273 513 695 072 629 083 047 345 273  
 983 649 042 528 310 432 839 305 034 132 464 249 045 084 848 122 356 736 000  $q^{7884} -$   
 7 855 363 157 142 989 521 950 764 180 337 167 411 376 184 387 337 193 111 926 739 204 845 630 405 812  
 442 736 318 903 486 049 422 747 008 804 769 442 478 918 050 970 633 977 299 219 251 237 220 243 232  
 821 556 382 715 603 039 581 220 054 270 492 945 424 277 660 147 575 635 375  $q^{7885} +$   
 8 609 925 247 073 620 138 068 603 506 257 491 352 278 494 640 545 626 017 538 063 992 640 872 584 343  
 821 518 978 379 760 551 829 752 960 878 593 617 588 436 228 561 147 606 701 044 222 750 722 386 803  
 761 263 293 826 592 801 644 325 163 773 248 218 207 963 219 895 830 609 920  $q^{7888} -$   
 8 877 187 755 693 509 174 262 573 353 042 549 203 092 977 152 528 020 213 044 998 016 348 813 017 095  
 997 011 675 322 985 841 179 273 257 508 757 404 142 503 793 571 833 672 045 748 209 204 689 769 365  
 261 575 652 519 897 590 237 211 806 337 799 058 321 162 898 452 905 984 000  $q^{7889} +$   
 9 729 677 424 554 973 736 834 878 075 774 302 533 180 429 590 574 677 896 151 327 880 889 346 998 318  
 693 315 477 433 253 526 381 409 040 119 887 306 880 266 174 413 486 767 740 380 720 231 105 359 067  
 587 492 021 099 808 218 359 533 133 551 976 009 334 620 222 214 148 294 656  $q^{7892} -$   
 10 031 620 839 234 060 598 839 991 672 449 228 104 429 319 853 440 957 271 438 787 269 033 146 751  
 785 621 173 079 011 282 898 060 809 379 064 464 069 542 020 430 223 384 462 273 273 668 047 331 307  
 543 491 552 781 726 191 313 134 055 448 350 781 997 336 001 208 497 442 143 960  $q^{7893} +$   
 10 994 717 533 614 590 842 693 216 771 411 051 115 906 206 105 682 665 037 310 046 775 526 851 038  
 073 553 676 460 310 718 092 821 582 435 481 005 660 043 262 265 014 090 512 986 368 312 130 918 479  
 598 716 655 889 316 385 758 152 478 385 397 667 935 891 209 864 678 227 968 000  $q^{7896} -$   
 11 335 831 666 974 062 272 616 697 764 560 691 653 549 930 459 668 928 092 945 622 935 428 998 034  
 576 173 339 222 130 149 838 067 755 372 675 092 497 650 404 283 687 598 154 426 664 176 012 761 236  
 796 610 919 705 610 201 547 516 407 241 983 072 125 375 611 200 141 372 358 656  $q^{7897} +$   
 12 423 852 710 287 755 269 521 971 702 158 503 749 602 071 199 635 270 841 949 475 426 505 022 916  
 481 253 519 799 611 597 420 731 267 732 892 813 223 795 064 829 396 808 661 393 029 664 264 332 320  
 846 065 306 673 802 015 039 898 893 938 106 056 742 090 366 603 041 006 489 600  $q^{7900} -$   
 12 809 207 273 197 745 210 730 143 255 673 066 986 922 271 589 881 453 302 229 850 951 976 270 175  
 599 431 356 772 304 890 351 962 634 312 265 425 459 902 551 737 420 451 785 896 019 206 581 989 339  
 065 521 199 497 455 221 294 375 405 398 166 974 102 683 175 600 375 149 657 250  $q^{7901} +$   
 14 038 318 946 251 951 698 581 018 166 769 887 907 454 165 183 735 610 170 324 952 151 187 455 169  
 232 023 997 275 110 709 057 071 014 960 922 882 565 936 873 796 664 575 843 681 798 714 599 006 843  
 100 958 635 356 148 680 890 906 008 730 109 488 157 091 912 787 288 998 912 000  $q^{7904} -$   
 14 473 638 272 086 630 684 425 806 794 256 198 177 349 951 217 697 453 224 780 362 845 867 559 504  
 781 242 095 651 154 485 351 491 324 780 796 903 642 779 080 745 991 085 042 296 612 870 630 329 697  
 092 437 677 159 005 963 948 374 703 968 055 529 562 826 177 370 524 650 700 800  $q^{7905} +$   
 15 862 094 033 144 379 682 740 237 261 989 978 929 808 031 484 316 850 868 530 497 652 428 203 971  
 105 277 077 374 185 813 130 972 642 822 430 350 507 289 336 909 591 301 570 683 029 457 282 164 873  
 614 125 553 140 933 674 965 406 321 729 226 233 713 402 755 601 626 449 264 640  $q^{7908} -$   
 16 353 841 408 378 671 980 922 742 828 217 793 895 828 430 547 848 777 964 471 831 080 134 132 801  
 481 534 162 658 588 555 570 397 215 717 498 568 229 851 655 244 768 840 621 371 593 049 514 557 627  
 557 846 392 365 267 303 848 605 437 293 367 074 540 235 336 804 919 395 172 000  $q^{7909} +$   
 17 922 250 734 022 074 195 112 732 954 445 610 650 850 728 186 670 418 890 049 496 503 404 677 091  
 611 195 906 408 259 469 742 341 949 383 958 766 850 437 726 423 645 570 415 414 628 381 518 730 813  
 757 197 683 596 266 449 951 515 120 759 422 014 102 453 597 278 164 554 552 320  $q^{7912} -$   
 18 477 723 567 257 411 922 037 675 222 632 643 977 444 745 867 638 909 968 661 376 776 962 305 410  
 175 368 664 107 645 772 898 138 268 666 255 979 676 369 411 485 133 856 395 018 583 253 793 683 656  
 309 083 968 339 019 658 032 059 868 083 768 704 138 163 257 630 900 223 279 104  $q^{7913} +$

20 249 355 340 880 816 607 711 098 150 944 991 876 263 005 370 144 801 526 625 370 614 188 952 132 \
 660 884 558 137 072 740 165 860 181 470 336 192 994 241 668 181 245 190 029 557 313 523 263 997 658 \
 865 404 961 352 065 707 878 126 139 047 710 139 120 573 656 041 948 802 240 000  $q^{7916}$  -

20 876 792 560 044 063 977 447 698 469 883 777 570 470 189 491 166 583 254 219 996 386 957 612 153 \
 102 779 396 650 917 691 818 578 541 317 504 769 749 654 532 574 341 462 376 328 970 502 862 828 761 \
 112 983 440 423 477 651 035 431 869 234 232 390 607 273 864 223 722 058 917 736  $q^{7917}$  +

22 877 917 437 211 972 055 941 411 029 136 610 186 359 114 402 475 500 323 968 716 221 839 836 073 \
 405 421 256 917 251 825 938 565 057 451 406 343 676 669 730 976 405 662 725 714 923 563 424 371 147 \
 864 885 778 868 373 134 555 300 817 207 999 217 584 738 465 349 921 187 840 000  $q^{7920}$  -

23 586 620 682 455 022 158 860 840 644 528 988 027 704 113 173 043 681 099 386 433 454 513 956 054 \
 550 519 285 860 861 530 920 256 234 298 766 954 016 711 954 568 068 855 844 029 805 867 064 845 656 \
 686 463 972 925 173 524 281 622 441 581 355 556 107 913 018 160 700 948 480 248  $q^{7921}$  +

25 846 897 428 895 231 393 058 539 792 326 381 065 706 181 166 355 744 256 311 130 118 959 065 207 \
 689 309 429 214 589 143 399 997 207 646 212 371 206 814 283 674 868 513 218 345 982 556 903 004 593 \
 765 274 732 953 295 659 364 052 035 030 432 884 892 728 432 594 033 293 824 000  $q^{7924}$  -

26 647 367 809 196 205 732 563 493 457 714 976 884 710 970 865 195 390 004 542 409 829 634 467 814 \
 819 833 397 760 260 397 406 471 104 512 730 629 821 747 611 079 259 542 080 957 809 463 606 836 902 \
 913 914 257 373 079 939 778 420 672 311 457 814 665 975 877 830 788 633 318 100  $q^{7925}$  +

29 200 279 246 030 065 349 110 493 395 650 307 742 474 031 270 915 585 249 527 641 188 482 225 394 \
 528 003 118 654 156 720 253 467 054 780 288 865 222 262 291 784 100 635 604 549 915 119 912 248 183 \
 733 997 747 864 293 442 369 980 510 365 018 689 446 362 503 223 839 657 162 752  $q^{7928}$  -

30 104 371 653 549 673 805 904 063 487 392 940 293 618 522 077 078 303 131 040 945 324 716 397 039 \
 545 424 390 460 972 279 578 815 026 056 122 158 973 140 229 523 491 654 367 750 547 413 366 812 318 \
 341 764 552 830 604 545 926 141 480 932 418 566 314 926 425 698 090 475 520 000  $q^{7929}$  +

32 987 716 564 692 926 152 658 946 101 963 817 513 384 277 265 385 441 536 691 545 827 692 537 769 \
 064 261 473 203 876 798 391 351 893 938 710 191 227 526 106 123 857 343 716 772 956 124 977 674 735 \
 479 811 042 903 941 093 915 038 969 381 484 868 411 001 417 419 807 815 084 032  $q^{7932}$  -

34 008 813 795 827 534 113 624 401 262 044 537 219 446 213 867 596 099 870 486 149 598 089 292 961 \
 409 916 724 913 859 440 296 846 705 230 737 246 503 528 925 438 131 856 065 804 191 530 260 853 230 \
 416 579 152 249 391 409 811 056 252 036 877 645 613 512 813 190 445 184 866 148  $q^{7933}$  +

37 265 261 964 700 396 357 726 001 046 398 171 080 871 644 471 228 371 765 214 879 972 859 704 690 \
 486 989 181 093 099 126 897 514 200 974 182 671 635 824 451 490 552 484 479 701 466 412 247 255 127 \
 331 639 297 100 206 777 123 542 547 846 916 316 266 551 461 126 805 913 600 000  $q^{7936}$  -

38 418 471 184 166 395 503 078 346 908 325 920 985 685 106 710 481 317 906 681 324 161 028 960 792 \
 033 205 243 155 665 424 939 489 961 060 180 202 343 712 679 331 547 321 717 593 403 413 246 543 196 \
 551 621 479 878 538 947 683 483 134 851 991 848 381 363 253 076 598 287 597 568  $q^{7937}$  +

42 096 189 642 620 920 439 889 113 810 785 519 026 657 198 056 201 448 516 656 165 365 638 873 833 \
 583 148 715 287 342 120 394 786 592 163 191 147 942 932 503 043 147 869 799 453 927 049 613 767 471 \
 304 377 486 556 333 630 192 325 469 516 041 252 259 621 442 277 642 249 011 200  $q^{7940}$  -

43 398 564 050 938 743 982 338 340 536 030 543 769 868 785 054 670 248 030 783 299 668 680 553 395 \
 113 831 521 790 412 191 256 780 811 531 447 159 078 910 324 313 978 203 136 670 659 799 690 797 566 \
 338 049 321 117 156 794 104 118 370 462 208 748 357 729 107 360 420 079 395 500  $q^{7941}$  +

47 551 923 655 819 872 999 126 927 762 759 657 928 655 663 295 828 881 217 051 289 321 334 231 740 \
 135 225 804 192 806 890 147 544 650 768 493 549 323 320 030 798 879 354 514 748 591 692 024 297 776 \
 618 524 312 650 079 908 340 684 339 417 603 782 419 095 069 408 674 925 824 000  $q^{7944}$  -

49 022 712 585 901 025 114 169 919 609 442 411 059 952 175 162 223 229 259 230 074 615 696 504 008 \
 744 343 402 081 279 928 991 489 772 682 766 044 246 963 620 987 534 528 018 875 267 275 560 138 889 \
 133 780 834 800 291 013 257 678 169 194 025 717 037 119 746 919 390 427 545 600  $q^{7945}$  +

53 713 085 202 752 003 543 120 085 595 682 048 459 635 789 831 260 857 968 487 579 380 635 567 305 \
 347 457 068 865 276 920 554 625 922 065 738 683 731 553 500 070 205 972 993 527 777 471 854 925 708 \
 284 847 582 209 798 562 452 481 678 710 318 404 403 709 514 193 888 170 833 408  $q^{7948}$  -

55 374 016 283 180 813 203 491 393 695 612 883 343 599 468 758 819 912 979 083 252 552 871 162 353 \
 439 671 257 935 296 014 917 200 156 562 466 458 026 097 873 109 996 033 253 781 611 730 510 004 818 \
 583 995 875 626 686 359 121 548 431 380 477 328 312 512 911 787 761 243 929 875  $q^{7949}$  +

60 670 674 169 014 521 428 912 498 134 259 144 732 875 384 547 629 768 443 328 220 080 638 971 910 \

627 558 859 940 549 441 258 773 309 114 986 520 246 808 314 362 963 202 202 328 616 684 116 672 273 \
 680 411 576 841 263 454 286 650 027 610 198 352 946 816 780 249 375 839 617 024  $q^{7952} -$

62 546 271 655 976 326 620 637 482 728 176 811 766 371 439 242 138 708 406 888 109 261 608 390 486 \
 405 714 437 822 913 051 211 684 460 334 679 851 691 489 548 010 530 481 918 286 369 207 896 831 535 \
 635 395 563 333 436 321 645 342 430 962 895 178 289 416 366 610 832 369 975 296  $q^{7953} +$

68 527 402 112 614 656 563 317 207 886 775 759 456 445 014 742 699 265 273 634 351 208 525 780 356 \
 302 876 492 888 051 071 193 711 930 929 091 598 299 716 310 168 012 068 703 713 082 323 471 225 886 \
 158 649 984 642 171 687 807 939 310 715 294 419 787 154 614 825 509 359 616 000  $q^{7956} -$

70 645 346 015 922 775 007 643 728 593 259 698 244 095 625 271 919 748 548 663 620 436 888 996 164 \
 221 858 653 452 493 828 020 675 650 508 900 333 369 264 290 866 865 534 982 181 969 660 000 162 240 \
 285 140 015 973 146 671 159 351 507 730 734 578 209 594 463 375 080 449 655 798  $q^{7957} +$

77 399 196 053 400 438 572 640 537 428 392 305 524 335 112 212 888 520 433 239 761 065 775 819 066 \
 469 500 745 196 218 519 633 262 899 416 735 888 124 445 979 625 407 484 684 617 279 055 148 235 976 \
 879 946 754 936 714 811 401 558 139 781 126 538 948 117 495 180 438 317 926 400  $q^{7960} -$

79 790 727 272 230 228 779 533 618 902 500 036 290 621 224 749 112 502 034 811 658 443 818 548 386 \
 988 263 089 693 738 816 531 875 703 781 102 127 158 786 245 755 870 754 877 011 215 183 051 069 760 \
 296 801 016 449 188 720 727 573 688 547 786 599 887 079 904 226 730 258 432 000  $q^{7961} +$

87 416 894 902 104 740 378 052 011 278 085 822 033 963 123 039 711 175 813 578 792 424 186 081 122 \
 247 630 472 517 948 140 021 253 840 421 404 100 903 051 415 384 240 492 163 251 933 835 304 027 324 \
 043 332 500 352 976 679 752 224 867 217 174 821 044 110 743 379 189 540 608 000  $q^{7964} -$

90 117 272 251 321 570 220 874 115 292 790 361 626 224 070 300 056 604 103 180 003 446 507 336 980 \
 646 932 813 121 551 312 197 905 192 714 531 725 905 535 476 240 307 649 991 746 335 484 423 246 953 \
 583 996 940 026 032 734 417 464 580 801 495 051 165 220 694 816 378 826 389 075  $q^{7965} +$

98 728 163 149 399 143 731 770 433 317 539 139 709 504 908 922 639 209 229 463 720 573 518 193 759 \
 970 662 895 969 455 134 211 490 153 932 737 409 988 698 171 230 755 639 165 751 995 169 328 993 487 \
 166 057 203 666 698 428 850 582 435 199 081 255 439 348 123 959 253 699 493 888  $q^{7968} -$

101 777 178 907 308 539 229 273 251 518 895 877 066 420 733 745 088 306 126 815 980 189 145 126 177 \
 469 699 412 930 489 486 899 318 564 197 080 005 696 648 115 000 553 415 626 071 670 726 569 073 701 \
 354 663 342 060 452 212 684 516 446 789 672 454 088 830 665 681 657 184 256 000  $q^{7969} +$

111 499 649 574 675 642 523 103 242 943 795 759 751 537 658 637 498 796 783 669 635 319 232 545 274 \
 273 582 929 283 755 149 720 088 087 858 534 255 735 972 606 202 364 514 177 393 462 425 320 411 838 \
 769 710 615 516 281 437 466 888 356 015 229 802 208 567 522 281 948 188 016 640  $q^{7972} -$

114 942 211 028 377 458 248 318 606 067 952 389 996 713 458 506 969 383 157 564 104 484 414 890 918 \
 908 524 048 537 786 624 999 934 518 056 868 343 047 047 008 267 941 125 170 817 950 736 004 297 727 \
 426 249 017 999 565 603 609 008 635 923 498 953 741 883 980 397 094 700 536 790  $q^{7973} +$

125 919 422 272 959 054 926 520 007 666 763 633 896 163 065 621 362 328 945 789 504 783 355 587 285 \
 775 050 222 689 652 294 761 291 660 629 525 847 244 786 416 492 623 919 228 469 419 990 250 215 374 \
 306 381 352 449 472 019 753 880 063 184 730 451 480 877 841 516 627 028 544 000  $q^{7976} -$

129 806 207 690 363 958 171 544 789 630 194 551 481 711 161 776 228 663 292 561 755 905 314 841 742 \
 117 025 361 515 746 532 703 511 302 002 476 339 986 886 671 516 932 160 724 516 303 296 048 548 344 \
 844 057 409 853 274 396 414 798 677 333 545 346 375 734 555 623 474 265 489 408  $q^{7977} +$

142 199 715 287 087 835 094 872 061 369 488 500 839 816 724 171 416 366 648 524 448 621 117 568 010 \
 871 418 476 697 788 509 987 101 588 170 298 978 181 065 003 790 147 994 191 065 526 700 009 713 713 \
 760 211 480 175 482 113 990 923 640 748 660 658 771 355 040 983 754 811 699 200  $q^{7980} -$

146 587 913 818 698 168 969 736 503 292 551 695 267 996 803 361 134 152 759 432 425 850 840 920 416 \
 013 048 499 197 634 485 328 281 465 962 883 396 889 263 686 041 108 359 422 561 781 113 789 529 380 \
 144 943 162 744 273 447 300 171 761 329 096 763 004 988 537 998 487 555 605 250  $q^{7981} +$

160 580 026 628 190 479 803 034 607 108 969 293 597 972 263 488 788 441 744 273 114 978 160 401 997 \
 400 517 447 916 462 398 255 353 464 974 848 967 246 433 351 467 977 597 033 811 695 621 825 330 578 \
 448 479 085 065 079 356 379 441 830 798 175 369 310 993 009 758 542 144 000 000  $q^{7984} -$

165 534 172 852 330 547 568 397 399 787 351 345 926 546 432 738 599 195 386 147 960 874 672 999 379 \
 484 089 683 928 065 430 298 272 285 398 770 211 480 451 286 109 220 833 352 279 135 468 015 084 426 \
 755 420 612 050 913 687 947 621 872 405 213 679 193 178 457 074 599 518 208 000  $q^{7985} +$

181 330 612 534 862 601 552 937 749 015 550 756 206 134 476 268 257 125 692 963 294 316 051 076 445 \
 848 132 459 676 971 051 421 510 010 514 818 524 351 534 958 926 952 261 870 231 426 719 644 867 792 \

938 305 168 413 067 294 992 476 929 309 991 415 620 445 212 659 099 734 124 544  $q^{7988}$  -  
 186 923 527 724 483 113 431 299 341 816 636 839 928 695 429 628 431 764 389 172 441 639 790 245 619  
 641 959 600 916 542 254 381 874 322 917 308 165 742 710 884 100 254 785 377 562 368 970 085 791 828  
 027 949 349 907 153 679 950 187 743 221 924 445 594 448 516 799 684 523 825 375  $q^{7989}$  +  
 204 756 428 532 791 645 078 817 771 065 799 548 171 347 690 137 147 984 657 024 102 938 964 289 954  
 235 197 825 357 587 241 853 579 291 088 469 026 716 019 272 516 319 708 064 901 284 713 801 929 271  
 107 088 391 646 236 005 516 836 375 286 924 088 215 482 071 502 913 527 205 888  $q^{7992}$  -  
 211 070 282 259 778 334 545 786 307 661 843 977 598 193 784 352 621 960 367 859 432 334 589 266 582  
 011 153 792 391 343 225 276 142 667 436 353 869 856 603 903 011 927 387 020 929 251 935 473 757 692  
 238 620 307 652 701 644 749 242 544 032 653 703 493 401 749 109 312 506 003 456  $q^{7993}$  +  
 231 201 574 293 527 838 624 433 355 183 863 816 975 528 456 886 940 781 552 261 943 942 649 711 189  
 612 447 541 626 962 641 099 872 359 703 284 396 787 486 530 614 491 529 978 606 309 923 366 817 217  
 397 350 929 781 137 210 239 231 717 887 332 011 385 250 491 709 509 516 800 000  $q^{7996}$  -  
 238 329 081 719 591 904 825 201 590 581 078 325 698 894 903 384 307 073 303 622 218 198 909 357 916  
 722 563 080 603 700 856 074 038 502 492 278 255 280 668 389 037 583 851 782 949 649 021 380 549 446  
 580 753 529 608 526 926 863 528 201 305 504 009 102 155 938 619 699 977 367 515  $q^{7997}$  +  
 261 054 306 545 634 553 374 123 157 694 652 834 549 796 669 589 795 377 234 309 742 123 627 382 698  
 921 069 802 839 477 256 894 874 597 487 283 998 588 370 814 543 560 031 289 675 565 214 980 818 221  
 710 186 321 880 559 522 617 841 793 105 753 256 119 194 947 736 773 872 844 800  $q^{8000}$  -  
 269 100 078 702 108 898 182 143 992 267 726 511 112 014 953 545 626 187 619 595 344 563 545 489 531  
 493 499 548 921 342 174 847 993 506 211 210 183 426 669 676 248 619 712 090 716 560 600 742 564 041  
 479 889 673 399 601 141 328 212 141 360 909 803 838 766 965 983 862 374 400 000  $q^{8001}$  +  
 294 752 692 467 172 972 237 898 271 939 827 230 823 455 871 630 744 409 567 574 145 665 176 117 483  
 689 354 859 884 046 619 487 740 906 511 665 821 441 268 334 143 228 157 046 398 974 444 307 525 008  
 867 712 552 693 670 466 674 620 096 809 070 836 478 061 266 532 376 535 040 000  $q^{8004}$  -  
 303 834 759 027 269 626 302 634 352 422 788 946 601 095 037 971 512 567 710 449 047 405 631 385 950  
 437 879 271 752 983 087 816 128 459 231 021 191 613 608 973 657 408 544 867 410 602 058 092 458 769  
 372 387 070 767 533 214 783 743 038 374 711 176 058 675 277 803 272 038 165 575  $q^{8005}$  +  
 332 790 985 202 087 382 777 818 818 249 344 303 800 517 433 415 388 452 398 603 960 153 581 362 564  
 308 464 317 122 264 233 266 929 921 732 561 682 187 681 574 938 686 464 676 342 997 056 252 598 110  
 701 909 755 448 588 085 371 864 255 567 918 450 701 669 778 699 336 076 107 776  $q^{8008}$  -  
 343 042 511 729 799 542 442 328 449 113 883 605 148 309 611 657 453 086 014 483 642 741 587 849 913  
 998 688 370 346 826 043 636 521 433 123 578 054 592 578 717 404 506 595 820 072 888 157 999 222 261  
 846 192 051 274 917 448 565 655 103 128 768 027 356 843 248 181 619 654 656 000  $q^{8009}$  +  
 375 726 813 526 011 567 425 084 428 956 360 773 399 109 151 503 559 040 609 287 264 751 253 348 509  
 362 035 268 559 790 191 472 636 315 135 114 621 832 013 139 013 859 871 834 845 085 035 464 968 663  
 062 856 300 545 543 123 724 139 563 213 036 653 732 775 522 861 509 439 269 376  $q^{8012}$  -  
 387 298 037 981 249 375 709 298 506 162 452 802 935 391 098 152 914 672 955 478 373 306 601 259 152  
 480 642 336 602 494 392 430 811 563 867 983 226 332 442 956 721 098 673 053 351 648 188 324 151 073  
 573 176 596 838 066 079 208 413 572 020 561 981 736 574 633 171 438 269 561 911  $q^{8013}$  +  
 424 189 289 387 377 315 315 837 892 508 993 142 438 197 097 469 723 866 556 014 413 401 676 410 632  
 280 581 646 794 196 378 388 951 547 852 833 355 865 026 434 442 906 485 490 667 642 521 342 642 591  
 957 618 239 517 145 070 402 580 172 159 947 441 733 368 404 620 694 323 200 000  $q^{8016}$  -  
 437 249 705 816 961 085 701 353 436 529 840 878 212 884 637 974 968 650 925 748 013 636 178 392 253  
 049 512 418 650 627 825 216 109 374 730 879 473 853 585 372 694 324 435 906 070 165 394 810 733 949  
 949 011 390 658 482 597 254 424 724 503 934 256 455 100 077 960 435 319 537 664  $q^{8017}$  +  
 478 888 150 234 241 347 749 545 025 880 889 296 151 321 113 591 087 501 832 149 833 067 340 733 563  
 109 658 233 904 713 221 446 784 667 133 492 321 669 402 723 918 210 218 695 424 351 402 005 483 094  
 806 064 031 778 239 937 399 624 387 452 164 025 314 729 257 622 941 165 568 000  $q^{8020}$  -  
 493 628 971 127 924 059 583 924 113 960 639 928 748 776 739 218 753 772 589 184 254 253 021 453 809  
 588 492 666 736 060 064 943 322 663 462 998 126 145 610 890 718 677 100 736 129 251 031 618 524 905  
 456 618 956 267 055 630 315 485 338 075 462 880 372 257 576 319 226 675 789 625  $q^{8021}$  +  
 540 624 067 893 787 409 776 856 656 849 937 633 802 882 732 874 820 119 202 832 301 933 899 755 472  
 618 056 211 568 744 012 784 425 942 241 214 131 032 652 576 462 917 699 691 365 615 164 240 834 816  
 878 152 282 420 774 910 464 503 680 999 393 902 006 559 826 931 475 364 864 000  $q^{8024}$  -

557 261 000 684 092 559 085 068 109 494 064 744 287 394 582 747 662 283 872 825 394 815 530 072 417 \
 525 759 912 417 800 711 881 727 192 327 356 180 020 809 902 031 653 029 321 695 578 675 339 663 904 \
 198 689 429 554 379 251 591 015 737 985 329 836 355 682 242 736 950 736 486 400  $q^{8025} +$

610 300 272 511 552 482 425 482 220 200 999 648 555 959 645 378 572 742 234 093 355 397 664 028 211 \
 502 607 613 074 663 587 114 410 386 893 216 926 444 008 582 083 083 149 049 228 545 135 846 087 472 \
 086 858 845 743 228 306 202 428 040 136 113 634 486 501 242 807 786 173 865 984  $q^{8028} -$

629 076 650 202 828 221 433 630 073 465 119 574 603 682 821 384 903 175 496 457 593 528 239 000 484 \
 177 530 380 731 009 419 372 456 173 885 660 566 515 097 257 007 654 080 849 505 391 255 188 046 282 \
 681 797 560 530 745 618 863 744 016 924 267 553 071 421 909 777 384 259 151 625  $q^{8029} +$

688 935 658 919 320 187 325 489 171 096 731 667 507 772 757 540 489 347 544 909 282 363 900 086 492 \
 283 819 369 294 889 818 245 237 176 677 015 061 100 015 433 851 596 295 094 924 357 213 047 036 857 \
 144 276 782 088 789 144 448 704 196 235 226 606 920 229 160 223 637 143 138 304  $q^{8032} -$

710 125 969 909 146 320 844 985 504 261 627 271 555 051 885 513 108 196 379 569 061 606 843 172 081 \
 633 042 867 991 207 876 297 623 143 755 001 098 242 469 833 794 858 799 720 111 545 151 446 712 234 \
 756 841 245 141 976 733 901 117 410 037 232 793 163 368 172 525 275 152 777 216  $q^{8033} +$

777 679 564 052 637 317 955 668 048 458 353 514 862 465 811 911 346 921 126 045 101 301 266 585 392 \
 518 821 288 543 641 915 089 193 190 254 691 210 059 027 954 506 939 521 222 969 872 828 071 331 544 \
 246 104 068 000 747 391 534 189 674 331 783 468 114 720 820 148 255 903 744 000  $q^{8036} -$

801 593 431 929 788 876 425 136 453 743 634 117 269 498 377 052 083 593 692 962 163 957 801 146 970 \
 810 041 128 317 555 875 887 071 540 112 407 045 149 401 173 590 895 403 813 491 120 765 151 544 751 \
 500 114 558 950 666 979 289 322 261 843 061 941 947 596 048 470 784 740 231 313  $q^{8037} +$

877 828 427 983 210 116 671 102 736 021 951 552 168 691 658 240 518 795 479 075 717 973 429 489 979 \
 968 393 117 618 472 983 458 780 889 857 121 310 153 279 828 273 512 202 377 825 536 178 039 995 598 \
 427 480 961 409 058 113 321 070 183 006 694 819 114 863 871 116 208 137 932 800  $q^{8040} -$

904 815 098 532 099 657 123 379 183 428 303 641 153 275 147 263 644 945 240 390 751 946 633 833 610 \
 401 797 360 719 697 606 794 100 665 038 344 301 899 610 184 897 753 688 555 285 316 048 491 831 556 \
 851 276 308 399 528 480 573 328 680 498 259 619 017 064 960 497 248 002 048 000  $q^{8041} +$

990 844 578 108 307 871 378 965 065 330 177 817 951 582 335 448 986 237 741 311 108 125 092 879 835 \
 788 508 314 997 096 553 792 286 587 148 752 153 504 024 524 177 291 504 309 472 010 936 712 463 483 \
 906 604 954 757 088 176 479 890 304 692 371 045 274 403 243 577 914 608 832 000  $q^{8044} -$

1 021 297 978 011 773 572 952 200 411 102 696 552 638 752 122 887 046 150 906 114 438 903 821 964 771 \
 189 443 926 470 942 050 931 227 313 309 636 299 406 624 546 886 445 367 341 250 466 958 853 772 295 \
 427 551 484 913 752 105 616 405 296 451 703 096 323 796 177 710 301 290 984 400  $q^{8045} +$

1 118 377 406 431 934 698 562 575 430 636 310 999 109 329 240 469 296 230 836 344 761 522 761 896 570 \
 973 281 938 819 128 518 226 191 511 228 848 677 730 727 957 273 783 934 709 710 965 677 334 181 901 \
 011 911 085 551 152 924 609 021 950 054 587 882 546 196 818 534 253 779 599 360  $q^{8048} -$

1 152 741 846 345 533 720 783 166 455 591 969 687 194 178 496 818 096 852 544 653 438 407 832 963 351 \
 747 151 604 353 516 914 140 401 628 550 842 688 334 655 002 973 086 915 973 230 241 256 541 891 172 \
 830 091 952 605 359 722 952 147 438 991 088 643 209 324 889 962 511 323 136 000  $q^{8049} +$

1 262 287 244 112 426 127 726 700 235 909 899 368 660 250 757 613 522 165 944 548 886 163 296 088 409 \
 429 870 850 396 224 257 993 150 057 225 604 766 834 240 186 492 182 191 411 304 737 995 717 760 535 \
 312 669 846 747 500 617 679 152 660 803 851 133 841 071 022 708 674 685 894 656  $q^{8052} -$

1 301 063 848 000 151 726 376 057 131 824 477 179 463 067 013 005 143 549 071 781 911 045 024 997 290 \
 380 286 364 487 021 361 761 337 709 650 726 433 481 890 214 792 859 653 035 119 049 414 610 578 778 \
 716 058 919 549 099 737 377 776 002 068 238 551 733 397 823 925 329 750 183 800  $q^{8053} +$

1 424 672 276 024 169 507 703 526 676 055 779 187 096 927 429 383 819 446 414 397 310 956 506 235 506 \
 023 912 387 000 139 150 723 894 343 892 378 561 054 110 995 968 626 274 198 194 437 635 682 859 838 \
 905 234 908 980 732 324 457 301 311 411 647 447 174 979 417 414 711 056 512 000  $q^{8056} -$

1 468 426 229 028 487 935 363 645 506 867 874 967 103 312 302 962 505 998 855 037 136 702 615 212 961 \
 134 497 635 748 340 423 054 092 567 718 967 641 886 436 535 648 908 481 866 763 122 528 095 845 727 \
 724 885 574 463 287 667 156 802 474 234 220 025 407 348 031 115 332 778 393 600  $q^{8057} +$

1 607 898 881 534 443 101 925 157 507 034 981 144 928 008 275 665 387 179 784 096 221 973 886 689 594 \
 707 829 348 860 397 141 335 982 379 414 898 145 943 941 741 057 706 157 091 861 777 049 743 887 929 \
 207 473 327 362 776 125 035 689 448 487 013 216 499 098 215 305 453 871 411 200  $q^{8060} -$

1 657 267 600 349 966 676 105 248 120 619 279 487 831 671 450 416 976 989 573 592 184 851 457 717 881 \

522 750 427 091 820 969 567 894 495 083 410 175 433 924 982 882 848 593 221 232 254 522 205 642 880  
 930 489 848 061 507 212 876 902 344 186 011 654 674 428 352 034 233 161 052 750  $q^{8061} +$   
 1 814 635 836 645 943 816 534 747 719 523 829 900 046 434 425 294 923 506 291 530 038 860 565 269 963  
 511 414 399 059 906 921 957 050 434 784 771 816 136 723 715 541 834 257 930 198 216 993 125 191 870  
 383 803 777 840 151 370 788 599 217 343 301 856 102 386 893 032 088 166 400 000  $q^{8064} -$   
 1 870 338 179 541 686 929 825 561 460 220 179 394 660 288 778 432 544 608 357 626 653 761 708 331 605  
 135 567 422 114 258 624 850 793 081 561 577 143 722 646 077 714 620 698 120 234 378 964 326 036 451  
 067 513 396 406 587 075 572 471 421 945 975 761 007 128 705 090 136 404 787 200  $q^{8065} +$   
 2 047 892 867 795 034 332 605 777 008 419 720 659 156 296 704 683 495 202 054 561 642 904 202 888 395  
 269 595 682 433 944 635 233 773 914 007 955 407 115 065 832 192 243 759 369 304 924 596 497 317 987  
 184 918 633 723 627 667 517 550 978 098 479 962 583 927 539 432 391 372 685 312  $q^{8068} -$   
 2 110 739 516 271 679 811 686 703 338 010 475 381 262 298 908 950 786 242 058 212 225 836 667 766 323  
 134 070 989 301 821 828 532 260 974 180 579 008 789 682 371 078 947 612 316 971 883 818 815 093 142  
 914 925 239 933 615 823 201 583 350 572 608 987 328 657 710 910 067 219 557 750  $q^{8069} +$   
 2 311 064 109 706 022 069 373 025 846 827 697 078 362 359 267 120 407 139 842 734 217 278 304 653 153  
 043 648 165 779 201 665 414 744 795 352 769 247 171 913 836 739 970 228 173 113 348 463 424 310 402  
 359 371 020 335 485 222 073 867 684 321 674 687 417 126 015 874 219 264 275 456  $q^{8072} -$   
 2 381 969 270 492 091 585 411 556 963 903 199 673 732 958 701 078 270 044 220 701 177 285 935 147 774  
 305 343 313 136 899 547 070 538 168 513 109 843 001 638 600 671 570 020 267 773 247 164 038 971 834  
 965 799 449 746 510 217 916 369 621 196 147 717 818 002 639 445 552 774 250 496  $q^{8073} +$   
 2 607 977 089 662 118 320 354 612 093 826 325 958 787 588 665 237 359 977 657 794 380 049 484 143 469  
 191 210 227 375 242 779 630 396 928 398 276 391 570 975 435 837 798 592 718 624 060 000 260 125 695  
 382 193 524 866 455 571 162 143 733 021 301 708 117 947 136 847 614 843 392 000  $q^{8076} -$   
 2 687 971 684 582 974 042 615 357 816 726 408 658 855 429 854 771 493 133 266 427 214 643 918 694 604  
 852 217 841 000 523 078 048 291 595 100 610 242 797 927 309 972 324 882 718 060 188 562 553 751 549  
 711 313 698 938 188 807 168 877 938 387 967 594 863 779 868 316 165 984 974 694  $q^{8077} +$   
 2 942 947 939 353 992 462 524 866 133 409 914 821 846 234 997 661 560 619 018 905 973 621 952 196 809  
 375 264 392 281 375 476 157 190 385 404 096 227 962 643 850 701 915 400 949 290 661 304 155 947 572  
 324 348 572 635 094 594 070 851 862 524 902 031 399 834 353 801 369 518 080 000  $q^{8080} -$   
 3 033 194 471 816 546 123 656 437 293 895 511 824 826 524 064 479 815 129 301 556 489 273 771 806 375  
 350 571 703 636 783 912 693 013 803 179 546 395 563 191 350 378 749 892 178 595 210 430 887 311 134  
 993 956 653 819 497 394 788 985 878 758 822 611 409 581 617 274 348 158 976 000  $q^{8081} +$   
 3 320 843 624 221 443 981 964 082 433 285 034 685 186 781 537 197 121 398 049 420 879 280 054 325 789  
 990 928 386 327 138 078 147 481 431 912 218 965 563 205 240 848 106 543 760 164 941 499 483 594 825  
 082 099 085 556 215 638 762 810 060 621 932 759 265 674 107 611 148 296 704 000  $q^{8084} -$   
 3 422 652 934 945 165 693 705 294 612 744 307 741 002 584 203 441 725 187 353 035 951 439 030 326 084  
 572 949 118 271 815 560 439 900 939 741 167 492 898 820 250 161 633 239 698 151 045 609 304 645 612  
 825 008 778 208 475 197 524 736 258 597 341 890 272 350 975 657 003 050 464 525  $q^{8085} +$   
 3 747 152 080 167 240 444 929 362 744 478 015 891 929 006 164 756 718 462 200 548 638 087 449 134 264  
 626 052 190 520 744 788 220 330 552 123 538 452 830 322 259 626 487 432 170 443 854 575 644 763 778  
 868 229 640 365 898 837 664 463 469 583 768 620 076 613 592 154 087 375 087 616  $q^{8088} -$   
 3 862 002 231 696 102 720 858 882 938 161 130 600 707 570 930 966 105 950 588 862 613 593 962 704 834  
 716 532 057 454 239 131 492 261 109 819 635 475 852 786 580 072 809 083 169 809 406 688 740 173 934  
 275 756 313 691 658 659 751 506 903 021 176 560 200 611 178 970 158 292 992 000  $q^{8089} +$   
 4 228 061 260 106 943 216 344 519 965 743 774 682 167 703 557 239 282 872 081 671 388 679 410 877 790  
 637 174 336 447 036 954 515 603 625 481 825 366 402 186 798 503 992 822 596 892 990 829 949 441 236  
 761 662 872 681 933 651 949 707 899 272 776 725 258 570 497 210 440 491 202 560  $q^{8092} -$   
 4 357 618 819 937 304 624 255 734 285 275 061 665 557 742 611 083 967 726 067 039 411 167 012 512 185  
 839 492 570 248 660 646 852 722 222 356 322 192 144 805 834 144 305 006 744 867 628 980 450 363 429  
 774 010 487 993 375 103 782 103 432 528 250 190 315 193 703 105 375 584 779 401  $q^{8093} +$   
 4 770 548 219 614 440 884 777 634 873 240 814 910 757 204 484 086 353 470 656 765 507 515 193 075 859  
 190 200 013 078 785 176 277 993 143 207 876 805 534 088 711 817 426 047 571 553 921 694 511 026 180  
 901 814 729 983 662 802 834 154 673 888 468 765 627 158 821 587 541 359 616 000  $q^{8096} -$   
 4 916 692 245 898 329 941 578 801 471 257 694 108 579 186 894 692 580 335 010 748 164 657 033 802 196  
 303 152 936 786 111 194 698 394 303 189 201 825 107 724 852 687 822 608 631 301 372 393 903 667 092

469 978 688 246 695 493 001 736 016 325 650 775 745 492 787 857 205 735 882 752  $q^{8097} +$   
 5 382 479 513 719 622 759 546 590 379 279 936 848 309 799 265 433 188 933 898 248 919 540 271 680 321 \ \backslash  
 751 961 942 700 707 641 953 127 576 853 003 029 638 962 489 422 283 991 553 146 150 018 712 367 498 \ \backslash  
 896 069 636 669 576 171 220 766 447 135 058 060 487 456 279 324 765 165 955 200  $q^{8100} -$   
 5 547 328 585 932 939 472 417 915 152 815 097 208 150 408 205 581 929 910 156 698 614 294 671 452 296 \ \backslash  
 784 640 350 718 129 020 334 283 862 132 649 381 733 641 770 930 076 170 342 353 767 162 537 400 531 \ \backslash  
 089 748 360 424 293 558 413 748 250 701 679 990 766 264 124 558 430 544 631 250  $q^{8101} +$   
 6 072 724 337 726 709 411 882 926 953 168 373 781 983 427 148 648 766 785 574 848 923 703 430 260 715 \ \backslash  
 650 371 971 270 325 275 213 570 096 255 009 610 925 078 219 409 608 046 422 601 883 752 285 747 169 \ \backslash  
 102 508 792 580 730 858 480 835 278 138 020 705 210 144 374 745 777 395 392 000  $q^{8104} -$   
 6 258 667 017 969 523 535 859 701 555 972 429 335 296 468 811 097 061 684 365 861 757 109 178 047 371 \ \backslash  
 126 740 961 291 156 899 224 564 601 212 840 300 286 980 129 793 738 213 477 321 990 733 582 723 034 \ \backslash  
 244 676 856 533 606 492 192 600 464 564 457 428 372 446 872 608 657 104 896 000  $q^{8105} +$   
 6 851 282 026 016 829 171 634 031 452 708 006 818 408 730 592 216 851 176 251 592 478 581 937 127 256 \ \backslash  
 795 749 250 163 952 852 982 034 778 172 233 449 847 517 752 498 114 135 496 658 869 654 731 759 119 \ \backslash  
 392 802 316 477 811 534 559 086 482 883 456 642 569 471 173 223 314 855 233 024  $q^{8108} -$   
 7 061 011 185 348 297 786 244 621 453 655 697 116 629 601 439 720 475 760 878 087 522 145 773 486 926 \ \backslash  
 734 996 413 426 762 104 901 922 638 386 138 028 409 129 260 196 852 360 915 048 247 657 630 026 588 \ \backslash  
 108 005 120 608 994 419 574 206 182 767 266 050 865 331 950 364 358 672 814 375  $q^{8109} +$   
 7 729 425 726 728 875 679 637 587 551 508 631 011 925 546 940 339 837 989 281 367 416 481 701 811 809 \ \backslash  
 622 438 949 068 727 570 461 965 435 826 645 037 480 414 580 276 342 770 496 342 226 286 626 905 255 \ \backslash  
 773 971 906 914 919 802 186 851 021 165 364 463 787 151 482 020 319 007 789 056  $q^{8112} -$   
 7 965 977 225 819 007 717 240 022 030 520 934 006 286 800 161 679 615 264 304 449 560 705 438 517 638 \ \backslash  
 632 531 442 144 324 899 996 165 872 336 537 836 931 052 396 908 931 610 174 443 873 665 477 990 201 \ \backslash  
 627 142 357 991 289 390 432 148 538 843 441 663 109 707 771 140 418 096 529 408  $q^{8113} +$   
 8 719 864 299 851 340 866 422 070 530 645 968 421 993 490 404 859 800 923 516 247 781 607 628 125 725 \ \backslash  
 302 915 740 908 884 363 069 719 725 172 519 974 429 515 637 376 732 138 826 619 989 246 756 688 291 \ \backslash  
 699 375 786 659 898 687 139 117 445 996 369 343 755 432 687 769 951 950 080 000  $q^{8116} -$   
 8 986 660 575 028 781 349 767 809 419 889 455 661 925 646 302 357 883 927 789 810 543 084 572 318 590 \ \backslash  
 104 733 890 758 703 673 974 986 337 820 732 738 445 183 253 298 704 413 305 987 300 280 462 156 221 \ \backslash  
 517 836 036 993 912 876 535 861 105 271 510 284 229 818 384 569 320 214 330 584  $q^{8117} +$   
 9 836 924 744 838 121 205 997 455 291 923 197 091 304 774 920 211 648 665 399 043 582 134 329 680 751 \ \backslash  
 967 806 853 304 004 907 488 356 734 786 186 895 998 393 991 819 652 904 144 830 833 435 796 983 745 \ \backslash  
 190 401 160 809 148 310 402 085 655 377 010 178 149 061 068 069 126 981 478 400  $q^{8120} -$   
 10 137 823 920 197 186 472 760 364 868 501 598 335 311 851 782 119 962 430 397 156 573 680 823 959 \ \backslash  
 859 758 937 796 296 119 002 702 845 081 772 911 879 411 318 386 858 512 380 545 533 957 131 933 951 \ \backslash  
 505 092 660 501 683 506 397 162 259 823 381 348 414 132 985 372 576 873 115 648 000  $q^{8121} +$   
 11 096 757 755 022 423 094 840 424 068 444 995 469 084 940 335 722 656 820 909 229 689 371 021 127 \ \backslash  
 615 803 846 168 381 665 851 322 914 116 420 326 077 277 324 038 655 710 366 930 660 581 922 472 832 \ \backslash  
 283 125 021 073 142 000 150 865 432 763 226 551 347 371 172 926 841 073 924 352 000  $q^{8124} -$   
 11 436 108 979 602 802 922 865 144 066 827 291 588 306 620 409 160 973 548 231 157 281 743 234 372 \ \backslash  
 196 105 188 542 028 162 732 531 193 799 397 054 103 332 593 299 147 232 017 418 263 494 866 046 580 \ \backslash  
 908 755 726 921 611 577 660 770 695 143 300 414 442 716 663 841 575 389 210 707 250  $q^{8125} +$   
 12 517 569 323 940 574 153 526 339 994 970 360 553 283 529 649 550 174 837 752 196 777 261 891 325 \ \backslash  
 451 324 921 931 107 635 447 646 599 715 412 992 297 512 324 521 347 172 456 126 658 245 131 452 052 \ \backslash  
 267 488 093 355 593 067 130 972 009 126 114 148 780 628 688 877 552 436 502 331 392  $q^{8128} -$   
 12 900 275 121 211 241 464 373 566 206 072 126 001 788 894 508 393 799 901 082 760 964 943 527 567 \ \backslash  
 695 666 489 107 786 225 058 283 179 176 154 344 551 607 022 683 613 478 266 661 398 343 527 318 599 \ \backslash  
 305 265 546 424 659 754 882 947 238 925 986 452 806 565 859 846 765 621 563 392 000  $q^{8129} +$   
 14 119 881 697 801 201 922 036 785 776 460 569 323 403 112 647 875 748 001 105 639 769 832 622 705 \ \backslash  
 539 242 516 355 117 103 475 818 500 244 648 785 807 892 581 859 855 931 460 220 187 926 102 642 265 \ \backslash  
 430 162 276 727 304 333 981 620 232 966 853 057 409 706 260 545 750 038 859 595 776  $q^{8132} -$   
 14 551 468 214 006 119 054 791 072 378 032 860 051 925 839 944 360 860 403 286 474 517 880 244 006 \ \backslash  
 544 605 503 726 990 535 246 074 514 823 447 640 790 771 490 563 036 429 679 357 247 061 065 587 225 \ \backslash  
 631 421 284 584 446 160 053 465 152 268 410 701 992 746 647 285 728 886 684 863 712  $q^{8133} +$

15 926 827 383 932 263 324 849 059 263 696 602 897 578 848 587 590 237 443 851 411 627 835 885 269 \
 942 551 865 679 402 299 315 842 733 731 476 446 261 611 729 307 782 808 949 139 835 392 076 564 491 \
 539 504 587 831 041 939 039 268 267 813 302 601 001 583 225 474 152 480 382 720 000  $q^{8136}$  -

16 413 523 533 684 885 544 705 411 248 194 632 102 193 333 460 598 616 935 607 615 962 980 969 854 \
 991 510 053 993 996 421 621 365 263 987 566 459 883 323 058 621 268 933 226 345 471 686 190 246 596 \
 527 896 371 124 261 902 269 606 845 652 970 251 119 147 356 736 856 117 049 622 528  $q^{8137}$  +

17 964 480 392 946 469 243 333 099 427 456 530 874 857 374 539 753 113 907 561 523 018 223 283 077 \
 687 533 361 044 382 974 684 304 363 586 235 618 092 182 138 437 590 210 601 635 804 848 959 595 201 \
 695 957 915 320 224 954 689 510 551 093 012 605 841 898 370 560 493 892 227 584 000  $q^{8140}$  -

18 513 307 026 363 162 239 900 434 140 815 882 641 878 372 876 147 717 440 645 703 556 124 112 133 \
 302 434 748 334 966 992 606 585 175 477 337 892 705 424 017 309 596 914 871 717 540 671 985 554 149 \
 283 742 526 015 027 612 921 538 964 103 846 396 697 439 836 205 236 462 334 039 625  $q^{8141}$  +

20 262 229 419 154 029 149 242 409 301 713 441 280 248 712 734 270 500 006 721 496 338 316 391 956 \
 820 247 640 965 024 497 491 899 263 286 384 828 382 469 598 539 233 547 652 373 249 293 556 240 760 \
 730 832 053 862 273 458 196 902 744 717 470 165 700 698 137 869 692 288 419 840 000  $q^{8144}$  -

20 881 099 776 560 451 608 061 478 083 860 391 679 986 614 478 862 295 454 802 960 736 606 536 159 \
 939 585 441 132 251 709 335 503 605 660 085 346 011 676 965 548 245 737 559 599 645 654 886 446 112 \
 631 821 459 105 023 366 717 956 733 458 078 358 506 487 520 566 587 040 351 846 400  $q^{8145}$  +

22 853 198 256 812 709 573 161 819 090 863 101 845 067 173 776 424 721 324 969 005 748 707 908 053 \
 305 542 729 915 198 582 461 698 329 277 203 348 408 530 461 878 265 963 793 964 198 384 765 254 818 \
 004 009 495 313 889 872 543 823 026 467 547 588 533 535 101 167 280 795 789 090 816  $q^{8148}$  -

23 551 031 136 630 451 342 825 711 036 691 167 624 300 397 627 386 066 032 454 415 555 979 659 543 \
 566 365 002 043 290 832 996 738 007 493 340 199 666 973 389 923 291 195 585 448 755 342 517 951 529 \
 442 075 753 891 730 956 646 943 436 503 682 812 403 299 412 496 614 881 739 999 375  $q^{8149}$  +

25 774 719 417 457 305 101 816 390 879 167 577 496 934 489 385 152 721 479 908 351 176 033 390 676 \
 124 373 009 383 517 287 685 696 035 836 649 089 699 042 607 817 204 879 787 732 552 579 974 044 297 \
 201 450 306 457 664 392 426 791 681 716 260 212 997 239 028 014 730 836 860 784 128  $q^{8152}$  -

26 561 566 662 518 144 702 118 981 294 481 672 128 041 874 531 479 560 611 471 389 438 010 430 511 \
 308 428 145 928 955 204 917 473 259 834 618 545 241 207 774 643 649 250 932 256 536 757 269 845 685 \
 761 840 012 738 415 822 468 083 101 753 991 705 061 800 451 212 252 799 253 348 352  $q^{8153}$  +

29 068 867 665 153 812 918 369 289 161 769 440 216 169 659 089 927 985 566 760 426 969 041 206 055 \
 077 220 696 491 725 251 087 760 574 135 379 253 451 883 297 351 050 355 192 892 711 789 819 058 656 \
 020 658 769 746 627 202 970 658 006 238 968 648 865 798 948 490 186 462 652 160 000  $q^{8156}$  -

29 956 057 774 913 554 686 584 219 191 524 306 214 618 496 125 479 723 328 528 803 084 687 807 506 \
 434 018 302 916 262 161 916 141 939 858 687 904 355 053 650 430 997 349 163 428 086 985 716 489 716 \
 196 616 366 278 281 621 888 494 145 095 643 707 393 142 947 298 582 087 835 649 784  $q^{8157}$  +

32 783 061 032 609 789 874 851 843 336 070 556 180 773 153 396 548 605 140 439 163 524 420 451 195 \
 017 432 901 353 394 088 481 535 918 171 776 724 137 780 294 885 271 971 788 044 849 606 565 318 074 \
 777 003 986 115 975 174 417 190 684 404 442 870 328 461 074 346 369 654 830 694 400  $q^{8160}$  -

33 783 360 936 375 610 005 025 973 808 767 102 763 507 947 775 444 539 111 063 788 316 619 182 875 \
 005 934 215 320 134 337 790 142 716 207 058 278 977 702 542 551 989 624 844 850 418 195 404 383 555 \
 203 447 539 563 191 022 580 684 080 508 617 030 017 617 116 814 141 726 089 216 000  $q^{8161}$  +

36 970 737 833 491 698 049 371 187 914 478 513 534 818 382 648 987 867 402 610 517 364 129 763 124 \
 924 082 929 408 384 517 005 688 152 573 989 314 322 535 070 222 627 763 689 402 026 135 906 452 679 \
 460 873 489 915 328 506 264 561 948 285 902 186 121 017 697 439 987 927 457 792 000  $q^{8164}$  -

38 098 535 116 023 639 569 534 914 418 587 490 024 621 129 787 462 604 004 553 453 442 692 005 296 \
 763 080 368 577 555 120 598 108 866 720 289 495 809 243 532 512 250 512 358 155 580 063 184 392 556 \
 898 714 654 237 039 486 057 866 041 275 566 344 934 556 595 435 079 141 698 228 625  $q^{8165}$  +

41 692 119 258 385 509 689 468 898 961 015 444 491 681 518 703 174 070 482 870 237 298 673 786 382 \
 957 919 270 337 817 122 449 178 487 766 914 200 173 438 022 910 925 542 897 795 515 415 643 873 323 \
 099 206 202 608 825 847 308 221 509 595 940 368 955 494 096 503 446 231 655 728 640  $q^{8168}$  -

42 963 627 417 670 374 233 654 284 904 494 138 837 710 632 521 795 690 180 935 326 877 056 679 429 \
 706 238 211 712 796 317 947 112 326 993 933 093 256 841 934 072 237 725 670 180 147 355 520 920 176 \
 338 703 693 069 025 719 954 414 324 382 089 727 951 604 328 638 046 498 373 632 000  $q^{8169}$  +

47 015 068 348 589 431 359 887 540 415 110 779 567 850 501 080 126 560 398 470 446 396 325 168 520 \

134 609 617 105 591 284 005 627 329 637 105 610 355 072 379 873 501 509 812 224 074 802 558 261 542 \
 320 222 393 928 034 708 119 413 158 270 839 040 216 642 285 850 439 616 824 663 552  $q^{8172}$  -

48 448 557 990 248 541 139 615 510 151 587 202 370 928 505 370 543 432 802 602 174 908 509 428 219 \
 934 070 945 594 193 936 157 778 889 859 628 125 872 915 726 686 227 180 446 039 510 718 836 352 550 \
 710 024 754 280 984 700 679 331 838 281 826 104 453 171 107 514 198 273 879 934 392  $q^{8173}$  +

53 016 057 500 224 484 704 428 991 796 520 460 160 510 433 656 083 540 196 216 328 372 713 415 734 \
 347 416 223 744 392 630 051 657 379 274 191 084 496 182 496 739 992 355 640 856 429 506 371 828 936 \
 093 151 381 969 574 478 564 087 444 473 062 311 316 654 532 008 384 009 519 104 000  $q^{8176}$  -

54 632 116 738 444 897 089 395 960 008 939 803 521 004 536 476 110 193 657 707 338 749 775 519 841 \
 488 911 288 081 056 189 683 945 371 663 581 834 311 169 587 383 480 297 107 359 519 725 226 056 207 \
 936 205 077 864 759 452 985 689 784 263 887 633 331 934 770 852 427 426 033 827 840  $q^{8177}$  +

59 781 258 179 977 308 977 909 852 516 040 486 444 172 039 234 124 047 084 723 784 416 365 445 388 \
 080 773 488 450 105 683 352 866 462 979 398 020 271 646 727 771 508 136 555 998 841 561 192 283 819 \
 287 940 564 672 848 552 660 402 270 512 303 485 180 642 470 184 427 444 370 227 200  $q^{8180}$  -

61 603 085 926 155 818 862 536 783 775 848 529 311 464 734 809 297 615 721 554 523 401 953 571 022 \
 505 300 050 460 919 201 336 428 364 816 648 484 051 621 606 704 206 995 514 676 163 182 049 195 045 \
 236 166 021 916 708 236 787 682 069 323 065 193 662 822 331 574 804 973 598 029 000  $q^{8181}$  +

67 407 768 254 510 952 277 027 212 699 864 510 122 979 759 948 846 432 283 183 310 791 858 637 514 \
 624 178 792 891 691 691 515 036 357 687 786 745 227 510 442 822 330 754 090 669 104 378 090 118 099 \
 611 260 430 067 130 402 190 365 914 636 556 309 907 505 022 339 217 802 380 288 000  $q^{8184}$  -

69 461 504 537 716 654 367 862 390 099 161 640 950 731 001 660 213 290 414 776 560 144 061 064 260 \
 352 654 367 259 631 593 376 309 930 148 356 248 992 668 251 803 794 844 579 490 590 223 946 545 467 \
 283 039 148 707 789 702 630 957 045 746 856 448 703 624 111 696 087 446 339 584 000  $q^{8185}$  +

76 004 994 272 224 214 214 334 180 666 285 944 317 099 528 684 181 777 235 404 814 135 649 586 199 \
 301 088 287 691 163 218 382 197 748 683 178 730 677 456 112 880 432 119 225 423 803 947 662 439 662 \
 936 655 812 648 276 762 533 473 410 866 708 344 778 545 088 095 445 671 971 536 896  $q^{8188}$  -

78 320 092 256 581 433 780 532 937 441 824 147 638 124 710 374 668 542 541 007 158 673 430 277 107 \
 896 160 395 000 109 089 388 139 734 687 703 342 768 130 774 690 602 370 636 860 775 628 607 928 760 \
 485 234 361 801 047 851 341 521 344 487 514 244 040 689 533 014 434 868 636 507 500  $q^{8189}$  +

85 696 208 215 641 379 959 522 957 426 566 599 734 242 359 603 926 453 261 690 796 990 089 753 860 \
 200 678 500 394 391 800 981 389 063 786 719 717 715 716 155 007 419 069 618 092 198 499 566 019 922 \
 204 828 090 346 680 799 078 842 278 711 403 846 859 791 136 330 720 307 876 724 736  $q^{8192}$  -

88 305 853 166 080 704 179 732 731 619 501 779 031 586 142 666 673 284 065 354 062 922 835 670 084 \
 387 383 565 572 054 725 610 697 029 436 693 773 820 646 605 011 226 144 685 698 882 950 744 304 283 \
 568 656 540 080 213 882 381 948 618 661 556 266 990 919 657 814 311 214 208 417 792  $q^{8193}$  +

96 620 300 695 681 780 771 246 302 716 517 791 907 042 596 583 184 507 046 410 311 816 039 450 240 \
 246 565 366 999 404 590 846 950 552 665 048 867 957 161 073 247 955 721 367 797 340 676 271 264 518 \
 865 854 315 584 313 383 179 115 396 613 891 142 612 467 577 653 785 153 857 536 000  $q^{8196}$  -

99 561 881 803 381 023 678 485 015 089 224 123 983 634 154 155 563 340 825 666 279 459 618 746 081 \
 199 171 528 955 460 319 744 568 855 870 971 897 272 456 278 885 613 881 540 314 039 490 060 043 240 \
 384 198 712 079 591 437 610 925 532 407 531 502 347 048 691 278 180 042 407 561 749  $q^{8197}$  +

108 933 755 319 599 948 206 672 406 925 277 633 175 800 008 740 899 697 804 888 497 397 446 650 117 \
 366 311 431 761 085 202 074 925 634 478 587 887 587 769 430 880 858 119 989 312 456 869 811 295 397 \
 686 620 260 195 654 102 416 255 009 975 957 038 856 293 969 461 083 773 539 507 200  $q^{8200}$  -

112 249 397 041 038 596 473 963 431 776 642 942 532 956 128 018 455 944 717 436 631 976 294 990 455 \
 429 417 306 904 123 575 751 152 905 908 542 519 079 913 005 774 233 939 488 289 079 352 041 117 018 \
 204 178 361 146 672 550 615 077 477 485 507 629 655 647 870 506 813 273 280 512 000  $q^{8201}$  +

122 812 872 070 980 359 345 692 182 889 302 536 127 399 848 582 061 300 888 111 900 565 583 039 340 \
 023 305 240 502 920 406 670 685 959 162 265 622 675 049 924 532 937 028 892 674 579 809 202 208 592 \
 918 024 236 075 145 384 906 041 777 917 944 817 685 411 420 058 766 833 278 080 000  $q^{8204}$  -

126 550 032 470 208 165 866 877 719 267 278 669 167 397 335 393 923 606 446 287 860 914 682 835 382 \
 595 790 605 191 301 082 256 730 097 978 675 821 268 190 300 552 680 303 475 410 746 409 817 659 092 \
 322 711 959 893 197 811 670 722 667 654 326 711 713 119 847 459 385 178 982 717 625  $q^{8205}$  +

138 456 271 036 096 781 367 866 937 515 074 454 434 313 225 154 745 722 890 909 673 707 546 226 635 \
 320 338 469 882 313 350 191 204 896 007 421 571 910 071 941 128 814 830 270 178 541 633 047 371 764

795 361 928 116 714 464 339 255 741 012 551 149 360 540 935 549 741 196 510 756 864  $q^{8208}$  -  
 142 668 415 560 208 868 007 940 843 916 909 008 894 081 980 741 922 679 853 622 937 891 455 654 071  $q^{8209}$  +  
 881 189 857 705 478 953 704 435 340 035 553 157 056 094 030 456 782 834 710 039 466 203 088 268 738  $q^{8210}$  -  
 826 516 517 269 705 187 400 312 223 973 499 721 226 129 615 489 430 384 173 056 000  $q^{8211}$  +  
 156 087 711 744 886 713 313 537 494 413 206 254 081 091 555 529 788 023 591 112 440 601 772 556 079  $q^{8212}$  -  
 095 859 350 456 269 621 646 836 323 072 673 269 226 907 882 937 028 430 529 549 781 868 232 378 288  $q^{8213}$  +  
 577 602 840 671 687 278 572 283 969 802 873 114 183 809 322 417 359 433 191 368 704  $q^{8214}$  -  
 160 835 071 920 895 152 699 317 964 555 102 237 328 681 422 102 969 587 251 564 923 376 628 362 650  $q^{8215}$  +  
 399 470 035 841 636 374 200 089 602 494 457 243 586 108 690 816 043 382 568 114 517 653 670 746 201  $q^{8216}$  -  
 589 889 819 428 848 769 160 554 865 072 991 922 739 339 045 616 164 663 980 180 513  $q^{8217}$  +  
 175 959 267 821 501 308 766 503 683 152 734 977 916 526 738 041 209 682 628 166 944 635 482 874 037  $q^{8218}$  -  
 909 942 778 285 747 760 954 303 825 808 424 645 802 833 568 490 850 036 004 610 878 157 010 492 481  $q^{8219}$  +  
 689 007 334 031 848 624 035 418 685 727 928 685 954 216 851 233 883 913 268 992 000  $q^{8220}$  -  
 181 309 695 553 520 955 206 095 357 037 786 621 670 971 068 277 915 607 774 479 789 768 293 916 553  $q^{8221}$  +  
 095 272 493 799 562 734 845 394 949 925 911 584 848 855 691 009 737 041 206 739 431 277 567 756 273  $q^{8222}$  -  
 741 823 527 255 430 908 265 726 253 988 769 866 867 631 270 721 120 083 212 075 008  $q^{8223}$  +  
 198 354 901 620 454 513 303 783 752 598 269 683 103 461 830 147 370 507 205 702 510 605 369 444 021  $q^{8224}$  -  
 526 471 028 702 741 035 086 295 156 106 388 448 353 951 798 701 211 309 410 141 564 507 694 564 313  $q^{8225}$  +  
 785 575 747 023 082 233 187 700 344 974 690 476 358 608 833 640 606 008 234 598 400  $q^{8226}$  -  
 204 384 831 105 939 279 924 793 377 929 267 009 972 605 052 537 137 517 685 697 735 424 899 013 544  $q^{8227}$  +  
 390 710 502 988 512 788 779 699 125 496 172 849 031 025 554 499 000 823 122 365 172 876 693 915 379  $q^{8228}$  -  
 434 714 929 903 688 295 242 628 452 176 344 677 996 637 045 311 871 725 122 905 250  $q^{8229}$  +  
 223 594 489 129 074 987 790 074 923 390 504 276 201 375 790 721 985 795 509 307 186 067 210 540 902  $q^{8230}$  -  
 407 981 793 875 314 560 696 665 882 286 336 442 256 142 997 288 929 975 744 327 357 887 314 112 598  $q^{8231}$  +  
 123 403 271 106 396 049 246 654 951 416 115 785 189 887 675 994 796 942 864 384 000  $q^{8232}$  -  
 230 390 019 920 374 865 403 129 722 572 098 010 639 291 202 318 977 473 842 228 556 272 637 081 364  $q^{8233}$  +  
 358 448 273 229 653 201 579 937 585 805 219 504 595 746 322 602 834 277 735 020 395 192 573 127 510  $q^{8234}$  -  
 520 521 372 041 009 551 390 742 773 569 646 511 161 623 204 572 969 855 515 033 600  $q^{8235}$  +  
 252 038 351 723 158 003 413 403 763 599 566 465 211 879 327 972 176 357 342 002 786 019 714 750 119  $q^{8236}$  -  
 201 120 151 236 789 008 075 588 541 335 384 096 509 856 835 558 813 731 629 950 339 627 190 850 022  $q^{8237}$  +  
 424 665 953 086 048 906 535 440 514 821 828 018 055 947 593 382 082 409 151 381 504  $q^{8238}$  -  
 259 696 468 156 863 351 757 822 006 839 333 671 402 687 166 523 388 325 368 829 348 964 940 998 448  $q^{8239}$  +  
 038 179 545 237 312 793 804 494 473 739 534 716 294 504 892 021 962 106 844 679 968 584 659 126 130  $q^{8240}$  -  
 802 794 062 348 074 852 207 977 045 435 710 740 759 817 271 883 923 434 080 049 500  $q^{8241}$  +  
 284 092 358 458 027 333 684 276 953 344 302 481 126 142 227 342 001 416 320 981 628 279 102 104 769  $q^{8242}$  -  
 368 988 910 577 886 469 496 076 059 672 863 665 220 423 513 344 467 149 824 510 289 482 424 789 122  $q^{8243}$  +  
 257 061 015 538 873 170 181 893 242 094 756 592 118 222 132 765 747 134 122 205 184  $q^{8244}$  -  
 292 722 302 582 981 916 025 189 552 046 940 406 196 570 692 547 138 951 906 952 929 839 626 130 162  $q^{8245}$  +  
 812 134 842 286 842 563 351 395 453 259 025 408 790 913 394 594 326 203 709 944 332 562 114 173 683  $q^{8246}$  -  
 191 142 277 567 239 555 226 190 417 014 901 937 545 536 846 067 085 336 053 121 024  $q^{8247}$  +  
 320 213 670 560 169 985 860 847 043 529 873 422 726 345 875 488 502 558 862 462 433 206 308 013 516  $q^{8248}$  -  
 754 209 522 145 654 899 445 708 993 291 865 659 853 655 778 078 735 560 263 836 874 838 713 070 496  $q^{8249}$  +  
 464 338 835 494 889 099 393 318 325 944 087 964 900 395 751 933 180 960 102 912 000  $q^{8250}$  -  
 329 938 487 842 159 035 002 435 704 488 645 413 279 873 498 649 495 445 797 208 244 606 339 067 381  $q^{8251}$  +  
 967 559 003 449 862 867 182 388 658 013 264 059 307 198 020 238 206 511 000 104 586 757 887 372 256  $q^{8252}$  -  
 192 841 910 376 695 936 255 036 693 699 327 004 332 210 346 521 475 884 150 522 521  $q^{8253}$  +  
 360 917 208 765 992 379 474 967 029 141 803 830 819 100 670 678 330 835 303 587 951 986 110 373 131  $q^{8254}$  -  
 380 075 167 414 752 171 405 827 987 160 989 326 554 321 467 240 609 918 364 296 560 483 270 211 438  $q^{8255}$  +  
 278 807 863 523 032 362 081 171 226 368 266 631 633 953 272 653 986 658 409 881 600  $q^{8256}$  -  
 371 875 488 262 737 203 578 349 354 376 243 977 258 480 942 602 739 298 544 171 837 255 565 584 981  $q^{8257}$  +  
 778 539 207 139 756 576 744 826 962 968 302 180 447 284 317 350 950 201 153 087 022 440 920 266 652  $q^{8258}$  -  
 966 790 450 132 704 640 245 222 492 627 708 655 582 528 788 027 731 042 729 984 000  $q^{8259}$  +  
 406 782 934 258 655 686 935 981 616 191 987 580 599 986 475 365 991 402 242 678 903 921 339 554 745  $q^{8260}$  -  
 987 535 142 355 481 782 041 767 949 243 119 628 759 850 650 646 074 933 664 482 214 897 487 625 406  $q^{8261}$  +  
 367 142 292 961 561 196 339 005 553 254 618 932 252 090 528 621 750 899 088 640 000  $q^{8262}$  -

419 130 767 676 371 813 050 813 046 395 119 818 115 249 971 277 686 625 187 379 566 264 126 148 487 \
 301 779 622 409 919 244 125 398 086 407 408 519 766 045 893 086 845 779 988 860 357 970 993 020 415 \
 404 708 334 036 498 121 034 538 870 177 071 608 715 520 311 070 272 037 689 070 425  $q^{8245} +$  \
 458 464 045 321 482 649 808 345 626 057 869 753 313 269 045 175 321 106 375 335 801 232 954 822 001 \
 424 065 376 793 051 498 475 409 091 004 359 746 692 962 414 763 461 110 501 059 623 506 093 993 977 \
 929 857 451 379 622 808 565 439 760 996 694 285 178 292 475 937 775 820 810 218 496  $q^{8248} -$  \
 472 377 232 421 554 281 622 313 387 129 791 018 617 574 180 442 715 751 174 445 570 539 939 017 656 \
 187 892 233 505 036 610 495 461 239 495 259 359 387 223 487 219 803 147 044 902 020 933 212 770 400 \
 203 157 180 699 941 956 768 527 052 863 650 943 250 182 692 299 639 246 577 664 000  $q^{8249} +$  \
 516 696 204 614 629 031 079 578 100 052 264 552 045 658 873 163 075 841 559 237 480 892 449 223 614 \
 222 398 775 483 550 114 454 438 295 505 695 442 677 911 597 876 750 973 231 236 312 503 020 317 671 \
 262 116 554 575 520 676 250 198 949 867 636 079 279 223 289 430 957 360 913 661 952  $q^{8252} -$  \
 532 372 735 878 276 770 436 292 888 558 831 331 991 891 208 311 222 043 419 830 892 311 052 115 295 \
 431 019 881 897 467 565 560 025 120 256 127 061 949 711 900 383 699 629 691 396 836 397 113 852 577 \
 786 804 396 827 243 118 670 406 772 805 632 698 693 195 581 504 067 691 526 386 152  $q^{8253} +$  \
 582 307 926 367 724 982 607 279 133 454 997 803 509 628 752 048 929 218 204 735 828 990 514 748 082 \
 686 142 711 446 899 818 489 745 386 067 733 493 547 812 227 711 429 128 269 252 909 618 194 220 777 \
 747 445 685 075 992 815 880 975 363 074 340 390 547 802 196 518 760 535 162 880 000  $q^{8256} -$  \
 599 970 777 695 524 635 002 829 213 457 303 926 518 735 710 271 689 490 748 386 521 331 140 268 408 \
 483 833 918 062 942 477 225 652 735 501 942 981 101 084 233 513 303 068 895 066 302 076 450 727 133 \
 231 713 780 237 505 448 193 005 143 694 833 719 244 735 149 128 675 790 945 779 712  $q^{8257} +$  \
 656 232 268 964 198 285 919 609 431 108 890 408 372 318 145 328 560 272 204 789 303 267 563 885 292 \
 847 575 007 229 803 365 478 066 408 096 644 777 724 816 824 506 904 239 450 008 673 360 097 583 853 \
 232 954 524 808 241 719 382 105 189 044 529 858 985 752 688 876 887 021 747 404 800  $q^{8260} -$  \
 676 132 547 539 498 867 424 097 241 239 441 926 621 075 939 597 832 621 634 915 111 979 075 109 045 \
 198 569 241 336 989 900 253 115 159 316 347 425 482 177 895 583 125 402 142 723 980 327 606 856 562 \
 946 377 788 079 950 353 292 159 167 405 977 103 875 323 714 345 445 521 836 291 375  $q^{8261} +$  \
 739 519 996 596 949 721 954 861 351 737 712 000 752 975 152 324 535 946 526 048 966 158 408 714 694 \
 016 249 398 787 991 558 377 565 707 367 772 690 424 760 198 679 988 388 608 828 871 562 644 554 454 \
 740 636 736 111 690 022 794 561 200 252 246 731 612 344 729 747 860 375 145 472 000  $q^{8264} -$  \
 761 940 481 937 850 921 180 875 029 073 817 690 492 878 159 221 951 862 265 651 431 587 421 501 295 \
 456 584 046 819 388 405 653 811 725 722 766 236 858 046 952 334 737 392 867 026 062 514 394 538 981 \
 408 710 128 868 963 869 048 878 826 941 317 682 665 909 453 851 641 277 851 238 400  $q^{8265} +$  \
 833 354 394 151 765 850 567 111 955 386 741 315 001 700 656 206 619 167 883 819 676 587 177 674 248 \
 134 821 453 985 454 422 445 457 306 598 097 049 424 749 372 452 157 924 670 600 405 856 514 858 455 \
 910 571 882 197 112 908 579 057 215 895 038 407 297 659 886 523 640 305 046 646 784  $q^{8268} -$  \
 858 613 523 883 047 570 521 225 274 525 097 993 806 850 846 716 822 461 736 672 546 228 571 734 202 \
 502 696 575 129 752 612 714 223 750 365 245 878 692 984 516 955 653 784 713 319 657 524 325 741 662 \
 904 459 630 807 695 495 859 365 874 006 675 456 016 648 868 184 947 703 788 818 125  $q^{8269} +$  \
 939 067 942 507 434 308 923 008 216 004 024 731 671 262 643 744 186 671 476 948 715 771 679 645 121 \
 816 806 744 576 747 231 924 364 662 281 891 712 847 587 565 277 518 776 227 786 848 231 581 442 245 \
 463 560 631 186 946 390 285 022 620 886 735 208 448 048 432 504 574 948 558 405 632  $q^{8272} -$  \
 967 524 298 577 796 490 441 821 847 460 542 087 164 981 874 542 071 884 442 565 541 922 257 037 652 \
 788 523 224 457 131 650 426 559 231 530 334 446 663 667 584 280 716 738 603 508 646 048 195 594 973 \
 187 385 724 433 821 744 864 355 682 216 321 018 125 421 196 839 729 434 046 234 624  $q^{8273} +$  \
 1 058 161 087 348 264 979 253 965 296 956 133 655 064 280 173 163 204 867 061 793 936 333 530 287 425 \
 267 159 876 996 819 069 242 911 749 901 926 803 620 282 999 302 243 003 877 295 700 638 008 982 324 \
 732 436 242 118 791 518 413 296 147 576 748 135 398 655 090 805 191 099 286 272 000  $q^{8276} -$  \
 1 090 218 445 385 005 750 722 155 403 960 597 028 709 216 466 468 247 203 402 408 903 158 074 377 079 \
 719 465 168 474 446 567 409 735 481 132 123 523 622 537 425 384 299 145 729 354 209 746 542 475 811 \
 850 320 997 089 006 022 821 440 567 391 892 629 902 120 201 378 574 369 184 215 901  $q^{8277} +$  \
 1 192 323 363 723 459 214 202 371 714 618 319 098 740 887 347 740 102 368 914 734 567 309 024 789 565 \
 595 428 525 715 144 674 160 574 471 680 528 379 384 003 263 921 055 803 276 688 498 554 311 674 646 \
 848 434 696 967 458 204 394 921 097 982 160 661 566 764 507 901 649 142 288 409 600  $q^{8280} -$  \
 1 228 436 376 052 495 302 712 021 805 218 623 464 790 656 355 871 245 398 799 249 068 076 711 367 106

141 785 225 762 438 047 305 832 223 197 973 318 601 500 003 116 532 909 226 470 045 457 351 185 766  
 227 295 506 710 506 692 607 243 479 695 335 563 585 120 954 859 746 888 114 176 248  $q^{8281} +$   
 1 343 457 171 360 802 330 835 237 740 165 092 998 708 603 203 169 805 373 652 498 114 544 888 857 378  
 100 290 465 280 902 193 497 711 609 512 134 939 238 568 815 342 794 699 569 987 055 566 012 273 924  
 997 050 056 185 179 526 010 135 612 739 600 432 301 109 481 690 463 281 872 128 000  $q^{8284} -$   
 1 384 137 763 032 867 796 113 569 339 615 775 806 249 349 053 481 420 863 238 876 874 957 895 469 687  
 701 009 092 992 370 920 085 812 146 081 025 069 634 901 118 904 530 280 946 137 168 655 358 453 409  
 105 837 287 531 479 165 818 339 106 909 517 131 150 731 801 090 358 823 041 709 150  $q^{8285} +$   
 1 513 704 532 601 736 042 637 580 681 528 835 042 914 410 576 730 359 539 234 226 058 090 118 706 699  
 102 253 864 524 142 213 640 415 467 642 844 893 858 675 270 378 506 355 648 763 517 384 323 380 109  
 969 447 979 296 441 867 155 709 642 605 292 588 011 764 583 892 944 917 466 415 104  $q^{8288} -$   
 1 559 529 099 677 262 995 891 314 247 138 384 111 456 515 917 460 482 257 010 717 210 509 406 475 715  
 167 236 849 310 042 305 487 525 924 733 946 408 741 388 092 103 516 782 765 350 310 069 700 187 440  
 558 106 428 851 109 915 895 209 760 600 944 318 419 072 526 848 893 506 928 640 000  $q^{8289} +$   
 1 705 477 206 279 402 823 420 247 167 291 333 449 013 240 076 135 069 617 836 888 748 864 936 752 564  
 315 755 943 139 560 475 522 283 246 619 083 905 187 112 447 331 268 790 849 516 725 399 776 830 371  
 686 509 890 880 815 243 764 798 337 831 086 780 180 823 658 080 149 907 568 869 376  $q^{8292} -$   
 1 757 094 716 771 662 867 165 203 176 221 043 948 852 446 912 820 476 949 913 188 410 437 510 908 234  
 525 434 581 915 372 457 162 422 039 952 315 993 485 048 803 207 983 138 882 472 338 772 065 272 678  
 617 306 072 747 319 640 951 513 833 030 526 463 597 004 894 630 315 093 827 362 236  $q^{8293} +$   
 1 921 490 577 482 255 833 474 958 805 098 289 316 910 148 423 190 794 709 896 993 635 036 937 615 272  
 975 521 797 739 192 009 691 359 033 552 958 426 420 340 672 252 190 459 157 434 123 248 318 748 804  
 277 867 014 512 157 115 365 621 686 726 005 389 331 806 344 386 207 861 399 424 000  $q^{8296} -$   
 1 979 631 687 894 457 619 795 412 310 000 633 168 555 146 225 885 371 946 175 684 230 195 662 669 046  
 017 180 131 217 307 670 283 923 538 878 064 260 585 608 515 710 274 167 308 951 076 274 871 481 538  
 327 316 903 569 217 563 113 170 426 623 962 024 927 551 778 184 701 159 257 341 952  $q^{8297} +$   
 2 164 801 795 575 730 994 026 373 024 011 169 095 743 197 538 041 414 633 187 533 599 614 283 179 093  
 272 055 985 514 100 500 225 618 435 917 789 273 767 932 277 876 587 020 272 365 823 591 680 653 788  
 539 496 036 728 147 463 959 498 495 289 642 946 795 650 001 132 314 208 541 145 600  $q^{8300} -$   
 2 230 289 110 065 624 143 917 479 519 835 602 309 823 092 647 003 189 467 841 314 704 084 389 814 768  
 417 775 792 573 791 378 664 574 724 731 632 057 023 403 784 421 683 935 149 388 857 055 741 477 081  
 776 007 791 893 825 292 088 589 696 777 369 065 921 675 439 230 096 294 686 337 125  $q^{8301} +$   
 2 438 852 691 815 420 919 010 764 598 689 474 283 040 701 900 430 328 066 810 313 252 770 300 346 762  
 765 148 668 304 976 918 607 694 844 860 712 627 250 230 298 983 364 429 909 427 275 882 135 606 243  
 217 042 850 205 107 282 106 957 060 143 275 743 984 916 691 445 865 853 282 304 000  $q^{8304} -$   
 2 512 612 306 874 668 511 553 427 052 122 208 022 779 652 129 085 971 870 912 054 221 432 773 152 195  
 250 315 492 713 042 943 082 658 112 467 443 425 559 696 200 923 008 912 618 639 433 990 982 731 719  
 031 533 723 046 215 653 968 246 798 321 415 842 477 485 894 773 068 969 905 356 800  $q^{8305} +$   
 2 747 518 074 188 882 461 043 932 317 029 204 669 485 359 388 268 392 182 979 182 748 709 261 072 718  
 056 443 405 322 963 283 691 911 348 690 479 591 802 399 921 504 909 067 564 811 984 398 168 145 420  
 629 348 464 359 386 336 619 924 921 447 466 280 351 283 096 844 150 325 204 107 264  $q^{8308} -$   
 2 830 592 569 552 226 003 825 238 073 854 322 646 405 475 976 514 559 937 338 007 371 945 285 552 322  
 424 901 715 334 847 124 982 326 456 422 099 561 687 470 773 520 142 834 349 543 954 340 688 177 346  
 902 284 372 199 731 062 580 272 546 753 479 622 314 963 280 382 514 102 783 555 000  $q^{8309} +$   
 3 095 160 071 682 013 834 278 587 503 031 028 316 337 816 819 972 057 374 223 338 410 217 898 904 765  
 760 420 722 405 029 384 140 395 231 848 942 418 196 524 593 231 787 088 894 409 460 510 191 526 755  
 058 085 759 152 640 859 586 458 554 655 600 946 821 003 064 022 136 607 463 188 480  $q^{8312} -$   
 3 188 723 128 228 311 097 969 678 789 374 343 285 099 713 734 197 216 618 490 614 020 299 354 402 707  
 335 148 244 139 718 071 488 931 530 173 052 657 661 441 506 853 809 150 496 458 616 084 516 850 375  
 213 233 718 460 721 066 105 935 468 610 902 996 256 974 143 358 748 936 271 167 488  $q^{8313} +$   
 3 486 689 284 005 324 560 222 375 205 223 157 626 527 081 065 404 754 651 071 118 709 020 151 278 614  
 275 441 516 675 242 665 658 202 921 291 281 560 805 380 941 428 784 055 218 634 756 333 484 591 525  
 229 474 016 409 837 240 245 766 489 115 608 344 303 350 465 977 148 353 968 128 000  $q^{8316} -$   
 3 592 062 131 954 535 824 808 223 212 311 014 972 124 808 506 042 143 849 523 266 091 675 859 615 611  
 154 789 258 721 845 687 287 020 057 859 441 900 626 201 991 798 931 862 111 633 740 092 007 835 102

454 645 237 478 236 544 261 982 101 322 281 172 162 920 063 975 203 361 098 185 425  $q^{8317} +$   
 3 927 633 587 087 960 913 369 627 131 492 196 650 004 122 050 153 339 697 861 563 248 249 791 150 154  $\dots$   
 894 542 990 048 152 361 578 531 496 619 954 807 052 823 249 303 856 446 367 201 087 867 396 694 301  $\dots$   
 884 592 264 244 276 044 456 365 634 602 079 004 683 951 433 630 362 055 686 553 600  $q^{8320} -$   
 4 046 303 513 144 895 356 214 239 670 425 303 759 771 937 594 190 679 681 522 005 542 542 320 322 482  $\dots$   
 982 004 071 003 287 094 533 004 928 857 698 385 004 203 749 865 266 221 134 271 123 864 956 096 716  $\dots$   
 410 662 465 115 577 820 281 981 863 870 960 880 915 241 922 778 669 616 922 624 000  $q^{8321} +$   
 4 424 215 550 648 425 391 764 369 304 613 689 982 018 881 388 071 428 563 446 111 052 974 261 089 621  $\dots$   
 717 435 682 721 993 739 043 687 713 311 780 155 180 546 812 086 087 284 838 591 080 086 957 995 774  $\dots$   
 397 590 283 597 175 014 569 483 227 858 422 692 397 181 091 551 388 462 692 352 000  $q^{8324} -$   
 4 557 856 721 243 720 679 137 550 149 742 929 024 759 613 599 017 291 859 194 641 915 238 249 338 541  $\dots$   
 725 156 559 963 695 840 104 237 947 892 308 479 201 049 195 478 550 708 573 230 215 511 950 111 635  $\dots$   
 432 857 727 158 102 284 007 180 946 530 795 214 974 166 253 589 098 075 216 661 250  $q^{8325} +$   
 4 983 439 543 336 396 708 102 521 559 595 383 560 180 865 661 753 264 748 926 338 561 492 238 446 767  $\dots$   
 660 347 594 688 040 854 350 142 747 422 627 055 476 823 235 640 663 198 494 377 661 928 208 519 111  $\dots$   
 425 570 684 070 558 622 979 963 057 981 291 554 662 245 073 056 706 439 917 993 984  $q^{8328} -$   
 5 133 936 433 159 101 681 110 265 659 677 200 409 052 462 688 797 998 784 903 275 486 208 491 410 682  $\dots$   
 224 382 210 291 991 444 047 446 616 057 091 230 202 728 707 221 635 147 656 953 022 745 534 719 170  $\dots$   
 892 430 914 939 964 460 989 762 881 932 398 738 911 798 009 189 423 523 528 704 000  $q^{8329} +$   
 5 613 189 734 946 078 165 604 780 889 262 793 294 822 772 286 671 294 609 666 918 464 963 127 298 945  $\dots$   
 732 131 237 810 728 174 127 451 336 959 566 443 873 433 420 028 255 259 627 099 648 285 373 149 317  $\dots$   
 209 198 069 515 121 503 950 923 983 637 218 052 755 828 836 429 602 956 732 937 728  $q^{8332} -$   
 5 782 663 485 990 106 954 395 438 827 745 299 275 426 823 797 870 029 107 403 100 101 395 029 552 948  $\dots$   
 171 698 365 457 435 809 816 008 285 282 832 362 814 158 119 777 085 559 289 554 514 783 539 049 643  $\dots$   
 364 368 560 857 375 403 293 697 024 635 897 408 949 281 487 139 671 600 579 058 563  $q^{8333} +$   
 6 322 340 355 866 823 972 745 255 572 688 317 675 265 998 578 093 641 639 094 017 577 352 856 395 793  $\dots$   
 035 702 477 303 478 156 406 685 134 139 797 236 361 266 418 223 782 885 200 943 519 470 475 483 727  $\dots$   
 972 144 727 035 706 063 699 466 391 536 849 887 530 594 618 268 114 254 888 960 000  $q^{8336} -$   
 6 513 178 432 719 658 497 670 213 836 808 969 773 557 773 789 231 806 975 178 871 190 829 701 705 689  $\dots$   
 527 051 881 081 093 170 154 823 067 649 587 583 940 454 496 135 802 638 086 140 667 273 112 824 039  $\dots$   
 901 197 792 300 973 050 908 205 222 267 800 396 836 121 773 678 242 890 617 913 344  $q^{8337} +$   
 7 120 879 743 327 774 598 585 981 670 414 069 330 791 353 156 476 349 712 224 555 556 620 449 301 362  $\dots$   
 220 319 118 903 761 938 338 825 310 906 967 954 215 242 227 657 586 475 582 617 567 074 623 301 848  $\dots$   
 650 499 625 682 588 795 209 339 574 979 959 940 185 018 897 659 569 745 620 582 400  $q^{8340} -$   
 7 335 769 295 969 486 910 641 267 992 132 375 755 431 702 246 162 656 472 436 823 751 860 162 860 247  $\dots$   
 218 814 918 428 281 765 540 499 079 335 696 158 238 091 268 916 550 358 233 300 402 522 613 740 124  $\dots$   
 052 559 842 319 055 077 093 944 823 588 001 926 764 615 749 873 110 028 904 606 750  $q^{8341} +$   
 8 020 049 894 431 957 578 913 225 785 722 153 741 995 966 369 129 937 463 751 496 682 036 033 108 980  $\dots$   
 139 215 155 705 569 657 453 632 993 487 562 859 724 906 787 791 689 835 472 403 815 026 708 789 065  $\dots$   
 054 481 217 508 631 084 831 405 510 690 353 959 311 675 661 552 097 512 251 648 000  $q^{8344} -$   
 8 262 015 291 010 000 071 888 383 778 572 686 082 572 669 521 096 167 514 189 830 652 286 821 224 153  $\dots$   
 290 683 751 395 955 252 471 480 968 098 124 628 074 310 046 617 561 933 322 458 913 865 296 337 121  $\dots$   
 965 721 390 660 970 712 080 157 961 972 071 043 735 903 707 491 906 531 804 774 400  $q^{8345} +$   
 9 032 503 460 071 163 428 720 585 437 203 498 375 885 834 858 732 090 118 840 174 628 512 170 740 344  $\dots$   
 935 623 008 997 303 947 590 296 124 577 455 537 631 908 989 793 187 883 493 089 396 765 706 449 499  $\dots$   
 855 516 764 023 330 370 169 594 570 602 737 638 391 651 821 754 120 619 731 793 920  $q^{8348} -$   
 9 304 948 509 672 734 431 680 862 198 108 536 262 463 079 455 254 795 044 707 564 179 196 651 718 516  $\dots$   
 601 847 077 171 722 400 823 393 407 456 439 311 648 202 925 188 525 594 575 160 797 572 633 450 471  $\dots$   
 394 767 450 424 913 505 523 514 876 152 209 231 521 616 843 191 871 803 708 285 500  $q^{8349} +$   
 10 172 480 354 498 037 925 253 389 840 264 149 233 591 057 247 124 426 053 942 965 395 357 119 452  $\dots$   
 855 607 339 589 155 948 820 633 245 747 644 055 361 393 199 895 106 714 038 506 838 516 747 696 678  $\dots$   
 521 388 290 263 157 029 669 106 953 940 495 541 057 873 364 392 480 096 551 164 416 000  $q^{8352} -$   
 10 479 235 804 645 207 074 401 235 611 630 842 794 012 824 334 763 287 774 305 054 773 311 214 479  $\dots$   
 220 974 167 903 735 197 948 844 584 782 332 776 639 826 739 930 146 640 598 771 810 174 154 936 202  $\dots$   
 797 751 891 957 913 892 069 911 281 941 147 564 786 149 131 801 696 122 511 249 211 392  $q^{8353} +$

11 456 006 425 900 992 886 630 086 059 775 932 339 259 013 411 415 499 065 956 045 525 293 948 864 \
 524 492 760 524 550 869 864 977 672 905 980 555 606 272 033 114 960 149 458 502 985 785 789 311 134 \
 975 822 459 015 587 228 185 323 781 963 547 207 307 783 958 869 403 565 946 214 400 000  $q^{8356} -$

11 801 383 392 229 635 816 154 959 896 872 549 628 875 218 283 181 023 341 671 254 205 835 138 106 \
 963 910 975 287 906 535 580 363 581 157 743 177 141 251 455 311 499 608 096 373 945 454 739 216 177 \
 346 606 722 781 165 785 155 016 212 629 441 179 833 184 051 588 414 739 246 849 454 377  $q^{8357} +$

12 901 116 937 482 818 289 824 789 174 716 719 019 931 922 957 572 726 185 533 082 606 978 644 059 \
 004 732 888 174 272 335 935 675 585 734 479 555 949 834 528 274 593 213 567 291 070 180 825 707 124 \
 748 834 073 458 616 986 048 422 486 619 763 004 058 634 790 742 467 049 465 390 694 400  $q^{8360} -$

13 289 967 004 829 691 015 311 622 897 956 189 709 682 251 723 690 906 992 279 797 863 601 742 511 \
 205 796 720 356 704 628 614 129 762 439 980 108 506 264 136 011 347 660 291 421 358 123 437 001 378 \
 914 568 719 092 866 802 798 539 061 525 481 319 523 395 963 801 985 801 998 692 352 000  $q^{8361} +$

14 528 107 950 444 956 394 970 060 924 851 883 751 780 029 398 142 138 330 753 661 427 812 513 214 \
 084 445 891 847 783 385 708 686 386 782 646 382 105 790 625 193 085 096 254 363 151 961 238 833 898 \
 900 394 709 967 478 116 933 107 849 227 833 320 300 330 986 597 003 269 095 665 408 000  $q^{8364} -$

14 965 890 776 475 820 174 280 863 566 151 235 765 518 433 344 555 361 788 615 637 885 322 024 193 \
 476 242 529 837 351 663 593 410 557 630 383 519 568 783 266 808 240 146 109 608 284 185 428 298 521 \
 330 995 207 392 106 205 615 420 855 220 587 182 023 086 233 106 166 792 280 743 114 525  $q^{8365} +$

16 359 819 084 599 968 447 312 227 871 374 730 564 021 904 922 730 611 838 297 881 974 655 298 499 \
 558 279 157 599 798 905 118 335 391 034 724 330 876 992 096 805 043 687 040 275 577 784 726 390 587 \
 253 701 298 542 054 189 666 143 950 990 453 207 894 973 757 313 552 497 807 303 438 336  $q^{8368} -$

16 852 678 440 421 557 296 692 229 672 326 389 412 369 288 222 410 996 554 442 009 665 786 631 078 \
 010 721 077 252 889 291 884 992 675 149 418 704 369 673 398 358 215 383 991 075 395 669 981 939 253 \
 855 729 965 185 090 346 418 906 183 452 659 131 520 269 781 369 837 711 585 312 768 000  $q^{8369} +$

18 421 951 564 325 873 879 582 111 660 641 944 130 366 272 816 361 253 562 354 237 142 391 330 573 \
 787 524 878 259 088 156 493 804 701 156 680 916 779 397 155 561 243 448 307 675 763 380 560 731 852 \
 371 020 736 691 897 690 042 983 520 923 358 747 775 038 236 817 752 506 992 776 323 072  $q^{8372} -$

18 976 800 862 646 824 513 283 068 151 801 737 145 883 791 269 317 769 012 853 161 448 810 646 686 \
 811 271 879 255 392 058 553 635 283 322 308 835 571 366 167 720 763 269 422 029 234 414 358 937 007 \
 867 518 982 717 448 434 713 251 036 873 927 780 876 244 530 583 388 139 480 679 731 052  $q^{8373} +$

20 743 425 943 137 421 164 282 624 571 287 841 241 952 294 401 663 826 945 029 344 299 811 811 898 \
 402 302 423 768 867 190 723 139 500 389 739 215 875 399 001 058 338 389 057 147 895 391 400 611 568 \
 307 715 462 131 806 969 740 684 386 393 680 406 516 888 255 688 591 386 662 111 616 000  $q^{8376} -$

21 368 044 435 063 468 400 108 014 892 296 506 303 214 201 951 387 440 466 720 471 764 710 233 489 \
 442 700 204 139 183 624 922 078 996 661 911 335 841 805 820 868 730 297 449 426 306 004 166 020 529 \
 404 272 153 092 155 701 345 541 544 103 666 093 463 629 997 908 174 591 032 817 614 848  $q^{8377} +$

23 356 784 445 909 095 608 537 966 036 267 364 664 793 995 677 998 729 476 743 408 371 890 242 289 \
 400 621 587 402 040 525 759 704 127 929 787 160 677 505 223 209 718 062 817 071 959 957 207 337 672 \
 766 640 662 485 191 044 653 996 181 440 052 944 770 519 719 730 686 133 070 108 006 400  $q^{8380} -$

24 059 925 414 157 020 611 470 363 879 831 746 936 090 757 423 047 354 925 334 049 554 895 325 180 \
 950 645 912 202 051 070 727 051 862 452 924 129 378 561 365 416 286 055 957 758 007 915 004 747 417 \
 699 469 201 356 927 236 465 327 823 747 094 930 281 508 755 151 184 588 130 041 063 000  $q^{8381} +$

26 298 643 481 189 156 565 921 237 645 092 687 443 496 566 552 015 661 352 821 871 622 904 351 820 \
 806 308 371 378 721 352 058 560 247 733 023 312 378 712 199 474 629 376 347 947 580 360 059 381 367 \
 924 334 691 766 141 052 392 074 621 123 658 161 350 938 566 842 891 806 801 416 192 000  $q^{8384} -$

27 090 155 922 383 153 181 500 522 519 812 778 297 420 506 403 589 946 348 763 407 248 553 015 164 \
 444 124 393 152 901 530 314 280 851 521 154 853 395 412 524 283 824 782 621 093 966 574 146 178 715 \
 082 206 641 842 850 543 041 059 485 971 766 371 884 494 236 633 796 073 282 548 531 200  $q^{8385} +$

29 610 202 565 458 618 885 831 726 620 851 552 997 904 131 013 860 876 651 410 527 588 725 898 636 \
 081 572 327 004 332 570 564 761 871 363 706 281 357 906 403 935 202 224 333 699 738 542 839 308 351 \
 390 318 028 058 528 233 622 593 095 584 848 427 352 150 965 721 575 727 351 232 610 304  $q^{8388} -$

30 501 168 039 479 828 986 815 358 745 179 586 676 735 421 657 033 273 807 333 606 110 015 487 214 \
 215 037 757 093 073 043 150 495 429 884 266 160 659 828 584 646 293 958 250 285 488 394 304 818 693 \
 388 425 954 880 094 127 183 066 567 794 811 572 058 456 378 509 498 134 911 122 040 875  $q^{8389} +$

33 337 816 676 011 433 532 076 492 344 004 196 188 720 467 696 383 934 368 416 629 463 664 800 969 \

309 341 807 856 457 649 767 362 718 383 497 558 521 118 612 644 824 600 760 976 037 426 250 924 041 \
 357 947 368 568 957 063 298 167 872 517 626 256 605 211 772 592 814 560 297 723 019 264  $q^{8392}$  - \
 34 340 703 208 631 633 169 481 102 564 825 672 729 018 678 596 036 680 678 695 170 369 588 788 548 \
 641 162 930 434 857 753 636 697 412 439 617 286 977 765 419 444 565 476 079 097 120 340 822 331 459 \
 353 274 486 344 247 731 578 201 134 093 465 914 150 542 034 247 998 603 458 633 531 392  $q^{8393}$  + \
 37 533 639 919 919 023 947 570 645 239 707 581 376 729 831 507 020 393 057 932 234 027 283 762 806 \
 691 805 266 233 897 345 977 266 176 302 770 665 218 256 717 236 904 191 404 243 315 050 155 208 457 \
 552 668 248 007 783 851 426 431 609 142 612 231 942 779 050 523 734 201 641 055 424 000  $q^{8396}$  - \
 38 662 475 078 999 514 779 979 651 501 416 685 988 507 287 611 031 869 181 011 931 486 902 716 255 \
 550 685 989 363 801 211 518 443 465 655 329 469 280 123 154 201 243 082 379 022 117 781 354 256 267 \
 758 181 424 636 356 810 722 463 244 904 934 505 203 395 776 225 817 682 889 473 314 883  $q^{8397}$  + \
 42 256 349 385 152 584 245 240 608 589 933 230 511 778 883 394 681 969 343 046 122 386 419 075 156 \
 939 683 579 046 016 969 977 949 236 611 407 526 252 057 764 672 838 464 238 331 085 609 908 671 977 \
 038 091 183 101 190 332 877 694 227 156 337 158 230 881 047 448 962 764 205 020 774 400  $q^{8400}$  - \
 43 526 914 913 715 743 499 821 231 060 663 213 470 840 883 569 159 977 107 616 347 714 222 268 241 \
 587 594 612 332 112 347 278 771 848 604 421 675 967 760 903 155 179 655 477 103 651 040 462 438 111 \
 546 896 051 444 322 147 547 541 332 560 756 670 937 406 867 798 795 483 819 139 072 000  $q^{8401}$  + \
 47 571 959 139 691 074 566 046 296 120 121 327 206 064 299 017 426 125 426 540 091 447 753 441 163 \
 926 572 997 249 880 960 010 624 790 195 225 986 641 034 623 442 661 000 641 118 060 480 911 969 609 \
 796 814 426 289 872 575 875 696 660 389 148 341 812 306 667 107 124 152 986 143 232 000  $q^{8404}$  - \
 49 002 009 824 754 048 167 214 530 670 365 884 910 203 260 446 120 548 112 533 221 294 296 629 057 \
 554 802 906 670 713 627 557 121 601 017 032 062 597 660 745 116 792 062 584 652 063 800 417 634 295 \
 574 311 166 463 202 504 039 322 355 795 622 422 936 528 261 116 727 181 872 210 441 995  $q^{8405}$  + \
 53 554 735 580 304 606 956 380 667 386 260 112 750 675 866 702 696 895 324 324 603 012 404 106 475 \
 319 055 487 900 094 902 255 543 887 736 330 780 251 197 927 382 004 281 022 528 979 921 279 622 708 \
 366 419 103 287 063 272 287 408 702 749 913 183 526 259 270 587 114 635 119 541 679 616  $q^{8408}$  - \
 55 164 245 368 522 740 388 976 613 334 850 167 473 109 041 393 604 631 008 562 096 257 142 297 472 \
 166 016 189 274 551 275 061 054 407 134 208 249 240 927 710 691 389 214 503 636 511 106 180 176 229 \
 781 920 362 593 526 167 416 907 475 940 511 735 985 677 979 013 084 501 822 853 120 000  $q^{8409}$  + \
 60 288 226 721 478 817 292 329 729 924 897 340 593 483 507 373 916 691 600 362 795 884 473 581 196 \
 378 708 138 967 913 182 129 592 306 777 659 244 675 045 881 571 201 845 207 670 018 166 262 887 069 \
 037 747 113 884 092 670 708 923 565 858 293 067 637 715 693 326 000 390 443 591 419 904  $q^{8412}$  - \
 62 099 665 465 896 439 503 893 594 799 714 312 108 709 080 010 311 370 760 828 150 501 660 701 330 \
 252 516 705 028 083 619 863 709 148 156 747 046 231 116 835 830 307 680 011 341 347 396 333 781 114 \
 872 611 461 396 348 056 907 790 188 600 193 114 469 537 467 705 230 567 381 116 019 356  $q^{8413}$  + \
 67 866 419 575 513 477 871 994 974 146 916 151 120 309 462 413 639 493 096 620 431 630 975 902 496 \
 324 745 750 908 099 475 239 785 622 997 873 645 707 365 285 166 281 624 765 983 512 994 324 012 825 \
 628 305 920 741 493 112 008 493 617 424 708 869 629 369 636 716 795 488 529 478 656 000  $q^{8416}$  - \
 69 905 064 217 133 706 239 274 720 053 853 477 689 290 456 488 170 432 729 784 694 082 581 031 810 \
 624 316 704 009 027 530 784 051 809 823 821 217 105 593 453 846 196 105 454 301 548 080 743 737 145 \
 442 353 573 989 627 689 654 718 093 898 194 810 653 510 849 396 208 306 874 582 597 632  $q^{8417}$  + \
 76 395 041 528 390 878 079 478 242 874 798 293 431 545 578 972 650 683 612 754 476 644 720 923 432 \
 020 665 935 155 899 309 286 017 386 429 870 706 471 560 279 390 715 387 472 037 216 235 158 319 578 \
 524 878 184 280 685 746 698 180 159 130 938 456 075 682 449 725 562 813 072 487 219 200  $q^{8420}$  - \
 78 689 325 987 550 980 375 582 497 623 858 736 113 399 546 567 105 612 495 856 085 425 014 909 664 \
 111 411 447 767 451 408 809 296 161 659 259 526 703 542 149 921 554 010 768 572 985 374 711 504 883 \
 827 352 684 002 968 701 518 203 163 482 406 007 574 416 636 037 508 481 273 896 986 125  $q^{8421}$  + \
 85 993 023 586 380 255 024 956 298 063 094 084 431 185 770 467 037 302 039 249 039 091 088 079 743 \
 349 617 692 319 303 570 281 583 642 060 502 260 458 149 939 133 412 251 867 016 894 279 525 334 906 \
 353 247 197 885 804 244 358 723 578 617 618 011 130 502 961 904 603 723 678 825 280 000  $q^{8424}$  - \
 88 574 932 168 452 990 586 660 672 643 364 976 338 120 685 541 366 047 976 472 958 381 346 613 984 \
 652 071 316 354 009 099 900 962 347 120 432 630 261 925 212 534 468 376 650 923 170 531 038 470 580 \
 562 491 835 906 911 242 341 740 196 076 687 165 025 624 757 012 450 405 937 097 932 800  $q^{8425}$  + \
 96 794 145 582 269 480 037 197 188 929 409 975 134 823 579 319 147 549 912 790 401 687 763 321 862 \
 852 063 909 605 636 680 561 635 299 818 767 973 214 692 773 908 914 223 672 505 610 564 744 830 615 \

928 077 257 203 283 708 057 540 809 670 023 255 262 175 035 948 216 578 989 424 583 168  $q^{8428} -$   
 99 699 655 297 189 538 733 831 259 564 262 275 133 745 842 825 742 771 514 466 531 416 832 473 028  $q^{8429} -$   
 381 037 818 549 868 151 640 835 381 182 869 314 499 535 448 736 378 806 055 710 545 516 636 728 865  $q^{8430} -$   
 068 432 871 775 750 808 951 616 165 930 709 967 654 546 641 606 294 378 195 550 634 625  $q^{8431} +$   
 108 948 885 917 631 944 641 672 867 847 865 307 258 248 028 492 171 880 954 843 135 224 378 367 643  $q^{8432} -$   
 242 991 102 973 556 073 645 110 258 126 712 580 028 966 278 597 990 726 369 292 947 229 490 900 841  $q^{8433} -$   
 811 135 650 240 971 341 671 721 726 189 148 059 500 179 929 336 511 271 195 261 992 960  $q^{8434} -$   
 112 218 463 781 240 219 819 931 091 754 779 401 597 838 119 693 785 923 101 058 758 051 948 353 240  $q^{8435} -$   
 858 155 879 853 149 942 084 524 533 332 098 385 906 117 720 767 412 410 679 761 287 879 878 107 126  $q^{8436} -$   
 300 554 551 572 868 855 967 143 968 404 207 717 166 659 295 944 653 779 365 207 506 944  $q^{8437} +$   
 122 626 501 212 379 017 781 301 285 842 987 568 161 428 352 907 113 710 965 288 552 201 794 408 431  $q^{8438} -$   
 053 783 166 528 626 847 713 984 165 168 840 402 508 379 144 682 943 855 306 292 966 440 241 830 781  $q^{8439} -$   
 966 492 132 142 309 200 390 430 411 127 344 616 782 473 239 686 567 232 072 035 328 000  $q^{8440} -$   
 126 305 663 348 649 002 648 775 973 464 518 433 351 823 823 529 125 577 883 814 099 788 878 453 125  $q^{8441} -$   
 475 712 074 071 914 205 821 398 496 951 422 501 029 007 576 960 279 243 418 968 190 713 266 030 589  $q^{8442} -$   
 273 332 641 971 952 626 657 320 491 510 958 142 262 922 089 244 485 045 521 076 538 646  $q^{8443} +$   
 138 017 364 372 900 485 529 181 479 870 373 026 892 751 693 877 267 964 774 476 078 611 186 510 477  $q^{8444} -$   
 071 281 099 114 370 344 748 423 856 251 481 249 049 977 740 005 748 691 882 266 707 263 696 865 234  $q^{8445} -$   
 614 506 401 686 035 794 390 493 533 548 353 231 324 757 413 748 750 495 008 308 096 000  $q^{8446} -$   
 142 157 304 579 938 376 734 629 695 145 684 047 682 005 960 984 921 241 820 316 390 888 701 408 051  $q^{8447} -$   
 617 400 154 832 956 540 236 050 700 239 151 448 559 125 220 847 671 261 795 360 181 199 883 205 026  $q^{8448} +$   
 802 799 205 879 237 000 540 395 821 254 345 211 276 826 590 471 710 428 315 672 576 000  $q^{8449} +$   
 155 335 593 117 900 405 559 989 635 049 801 574 926 481 716 790 541 207 942 419 018 035 398 471 102  $q^{8450} -$   
 715 930 853 747 775 654 648 936 166 892 596 656 222 112 524 021 260 151 585 385 166 017 762 845 748  $q^{8451} -$   
 387 023 032 086 219 717 603 484 348 914 258 243 405 068 998 273 766 184 286 874 112 000  $q^{8452} -$   
 159 993 889 508 622 945 396 092 691 594 010 195 154 685 236 776 622 983 787 233 645 545 372 555 388  $q^{8453} -$   
 841 473 959 412 323 376 216 017 559 853 147 341 196 813 234 903 620 735 410 398 382 224 387 108 405  $q^{8454} +$   
 289 192 110 566 787 099 612 476 778 440 862 417 747 610 345 685 427 440 112 363 407 575  $q^{8455} +$   
 174 822 004 964 368 422 703 724 332 636 272 449 244 078 656 783 330 380 107 091 695 124 535 322 935  $q^{8456} -$   
 965 287 390 879 313 942 135 844 988 446 040 056 785 795 348 927 595 175 517 212 659 130 236 305 587  $q^{8457} -$   
 326 850 682 234 755 577 980 163 856 418 550 726 150 521 586 431 353 143 693 217 366 016  $q^{8458} -$   
 180 063 414 357 794 701 714 933 595 544 862 610 059 641 492 849 331 811 255 498 069 284 352 951 233  $q^{8459} -$   
 085 929 857 051 510 643 939 487 462 164 808 309 388 133 703 337 632 690 685 839 637 963 542 348 037  $q^{8460} +$   
 906 107 079 597 444 235 621 078 190 541 585 456 060 006 878 793 498 523 375 484 928 000  $q^{8461} +$   
 196 747 439 128 634 455 078 231 026 608 190 024 254 826 859 465 837 735 187 544 634 388 817 535 335  $q^{8462} -$   
 473 755 699 124 018 966 169 836 115 810 541 642 431 656 801 609 766 829 912 715 851 837 762 796 697  $q^{8463} -$   
 692 142 406 602 036 466 536 594 362 981 623 633 242 827 024 335 380 332 010 876 370 944  $q^{8464} -$   
 202 644 790 064 191 966 511 830 333 598 374 901 381 632 650 931 264 013 790 299 968 990 308 322 983  $q^{8465} -$   
 237 795 598 601 479 855 850 061 946 943 431 044 556 250 751 110 706 323 958 186 181 441 051 507 111  $q^{8466} +$   
 174 680 031 729 469 182 058 462 414 243 498 484 248 853 903 984 038 595 915 146 308 698  $q^{8467} +$   
 221 416 490 799 378 840 438 795 708 060 724 139 577 872 632 584 541 049 006 174 237 216 296 717 956  $q^{8468} -$   
 935 010 811 601 797 664 128 116 488 993 412 505 119 579 019 149 655 352 702 359 006 957 003 944 456  $q^{8469} -$   
 106 911 336 958 433 898 026 585 341 773 323 161 372 240 467 697 132 399 924 184 832 000  $q^{8470} -$   
 228 051 687 390 703 178 088 123 999 611 397 754 878 466 298 494 108 811 955 868 190 864 659 601 606  $q^{8471} -$   
 831 563 557 080 366 697 111 758 858 871 333 991 092 121 681 135 827 532 469 696 429 149 939 126 284  $q^{8472} +$   
 857 856 340 491 126 656 688 335 803 920 755 313 668 987 055 149 170 195 729 465 638 912  $q^{8473} +$   
 249 171 708 858 453 535 917 933 700 612 372 189 941 486 002 563 053 585 957 579 471 958 819 807 028  $q^{8474} -$   
 849 370 981 156 036 775 368 904 226 936 326 530 320 710 300 510 946 071 147 255 292 193 565 465 975  $q^{8475} -$   
 822 233 743 118 572 718 399 555 313 489 138 940 314 284 544 153 762 038 582 220 416 000  $q^{8476} -$   
 256 636 859 213 026 563 665 643 278 145 912 259 134 903 640 792 572 413 841 144 133 359 665 713 162  $q^{8477} -$   
 041 589 893 372 245 779 216 528 120 824 328 228 141 206 967 454 878 661 505 198 700 512 375 564 144  $q^{8478} -$   
 087 121 257 866 510 789 061 071 190 309 396 014 836 301 446 859 809 483 459 031 743 125  $q^{8479} +$   
 280 398 314 437 365 187 529 909 338 281 695 446 102 639 180 549 375 322 359 324 404 318 657 504 470  $q^{8480} -$   
 250 782 804 638 047 257 764 674 871 080 496 269 511 585 554 392 960 149 413 729 129 171 818 589 897  $q^{8481} -$   
 214 730 318 271 233 234 055 822 937 867 136 101 032 101 974 978 452 259 710 783 818 752  $q^{8482} -$

288 796 999 064 391 447 495 563 389 225 813 554 373 551 322 293 039 436 113 795 697 958 243 958 363 \
 705 249 268 521 926 308 219 865 772 085 275 601 446 448 973 794 800 072 221 182 781 240 482 860 031 \
 287 067 057 167 914 908 632 034 664 165 535 499 517 757 628 209 692 061 043 595 673 600 q<sup>8465</sup> + \
 315 529 504 787 558 067 006 807 710 607 143 405 892 832 296 717 705 959 948 737 754 618 245 208 816 \
 913 419 506 517 501 462 556 650 776 065 874 656 886 626 253 371 903 184 385 380 927 456 361 962 590 \
 157 389 937 724 112 114 021 081 732 103 658 459 153 755 380 414 776 490 545 238 478 848 q<sup>8468</sup> - \
 324 978 202 321 632 167 564 397 613 234 759 601 970 747 434 214 720 552 710 949 988 444 830 942 354 \
 521 968 439 881 689 832 794 916 340 457 761 561 095 199 076 819 354 008 004 455 891 805 389 029 067 \
 574 535 825 278 059 513 764 188 520 594 127 117 974 817 941 036 121 687 353 156 968 000 q<sup>8469</sup> + \
 355 052 414 906 965 093 605 369 953 134 402 826 880 409 595 334 182 770 299 241 234 769 886 469 373 \
 663 456 859 278 017 657 531 007 094 618 371 736 072 699 517 921 913 424 066 505 238 612 233 308 990 \
 839 838 736 139 543 315 384 823 327 549 804 042 491 764 078 082 337 549 924 083 407 872 q<sup>8472</sup> - \
 365 682 104 615 054 684 027 236 251 834 135 812 208 700 259 122 117 367 910 699 005 002 790 411 105 \
 900 800 588 092 089 311 555 106 482 945 127 734 378 438 769 928 658 416 066 016 165 773 399 216 505 \
 241 072 496 941 761 500 320 785 456 783 196 062 189 589 751 306 056 665 372 010 938 368 q<sup>8473</sup> + \
 399 514 818 311 173 086 872 480 298 851 416 561 131 275 294 233 690 231 054 120 331 492 311 287 296 \
 865 219 204 419 528 586 071 131 798 138 692 726 512 176 931 433 317 628 333 520 631 619 410 899 233 \
 582 238 438 541 535 605 064 621 199 019 121 038 350 427 296 758 729 891 018 557 184 000 q<sup>8476</sup> - \
 411 472 781 254 110 434 461 195 113 561 670 610 827 474 009 587 281 363 862 548 992 238 944 506 573 \
 735 134 346 533 830 568 998 692 887 676 257 882 038 515 826 335 979 844 461 357 987 244 935 266 931 \
 022 803 465 566 918 302 520 967 247 076 071 777 499 329 428 739 013 290 262 084 668 034 q<sup>8477</sup> + \
 449 532 658 385 671 829 536 603 715 584 363 863 233 989 341 624 686 994 018 964 483 928 302 390 518 \
 503 896 461 400 367 501 746 985 443 305 263 047 878 848 034 023 107 745 269 449 257 429 044 542 175 \
 238 540 219 904 189 657 134 722 889 624 870 866 742 711 668 776 076 672 556 302 540 800 q<sup>8480</sup> - \
 462 984 501 805 132 992 766 772 529 943 523 913 221 090 872 186 172 211 267 716 145 752 904 535 432 \
 017 542 489 423 749 390 687 436 613 465 770 100 223 253 630 757 789 654 098 003 163 771 436 204 566 \
 036 348 037 984 929 004 223 295 781 520 751 528 522 240 713 883 140 182 766 739 456 000 q<sup>8481</sup> + \
 505 798 513 041 531 834 968 103 856 973 508 049 206 164 145 038 393 616 244 781 870 740 533 078 921 \
 124 666 650 900 247 075 705 463 718 705 467 561 315 215 115 027 496 181 747 583 856 296 520 467 725 \
 061 668 923 382 914 863 558 858 277 134 438 672 094 222 980 447 819 589 054 926 848 000 q<sup>8484</sup> - \
 520 930 445 575 784 178 402 979 301 791 525 551 344 698 952 365 623 185 797 195 584 483 107 482 158 \
 064 309 906 420 691 148 234 670 763 021 019 968 921 536 681 541 545 075 647 863 770 853 694 610 091 \
 133 172 053 410 665 374 333 088 825 789 336 528 989 512 677 562 958 204 354 937 893 825 q<sup>8485</sup> + \
 569 091 108 072 610 686 539 602 871 287 892 060 942 201 122 494 838 938 515 589 349 745 263 091 799 \
 533 492 673 492 177 259 624 471 951 412 007 318 765 322 349 604 162 409 459 236 750 458 956 148 360 \
 003 022 876 679 672 357 724 071 767 516 359 432 037 670 283 939 388 267 933 443 010 048 q<sup>8488</sup> - \
 586 112 496 809 989 197 382 153 263 493 768 792 437 161 189 013 554 264 494 141 677 349 756 302 761 \
 066 392 344 006 683 601 113 691 167 900 695 821 075 591 303 461 650 509 742 031 710 025 588 992 810 \
 686 165 947 507 859 961 900 398 977 796 288 732 518 508 906 842 856 612 803 051 520 000 q<sup>8489</sup> + \
 640 286 008 848 805 860 507 456 473 053 571 857 582 611 247 712 422 650 245 105 248 182 574 428 189 \
 305 101 871 847 721 809 963 615 076 381 248 248 014 680 079 757 275 483 825 721 943 939 953 309 190 \
 331 475 384 941 575 849 325 541 913 087 886 287 053 571 033 616 578 290 400 212 143 104 q<sup>8492</sup> - \
 659 432 253 052 808 821 438 863 553 777 189 763 532 513 134 044 449 921 421 622 903 176 626 089 208 \
 231 855 120 549 580 767 353 686 201 588 363 359 130 105 223 071 958 694 195 987 424 678 468 287 027 \
 604 454 628 612 545 458 761 330 858 778 750 530 826 194 429 454 623 507 564 005 842 171 q<sup>8493</sup> + \
 720 367 635 968 674 758 936 920 402 670 843 987 813 814 682 400 940 239 121 888 694 821 662 959 125 \
 045 639 106 920 486 882 497 351 313 442 249 843 974 597 994 227 100 590 078 305 452 369 952 030 682 \
 290 570 905 824 921 571 584 228 447 651 791 451 433 467 785 931 379 035 272 721 920 000 q<sup>8496</sup> - \
 741 903 396 604 245 402 404 980 346 084 077 066 683 545 111 604 218 659 198 991 852 225 347 179 336 \
 754 164 754 147 358 168 799 709 757 750 585 014 807 199 174 952 802 890 336 069 168 838 034 114 061 \
 483 816 496 872 011 887 336 750 778 425 870 158 993 966 195 952 586 433 044 964 311 040 q<sup>8497</sup> + \
 810 442 768 451 151 569 507 266 114 499 025 098 718 395 111 259 693 327 378 141 461 202 257 156 999 \
 683 745 808 715 113 747 898 859 056 722 897 720 523 895 990 891 655 437 931 473 319 184 382 173 258 \
 481 422 596 695 028 141 143 126 859 834 309 821 426 372 051 168 803 177 508 269 056 000 q<sup>8500</sup> - \
 834 665 597 465 940 919 697 513 244 623 706 979 163 628 810 370 810 842 364 474 347 140 574 504 302 \

101 264 293 282 173 958 455 735 126 515 005 430 355 138 178 417 392 669 088 962 248 781 187 510 897 348 730 584 618 130 027 031 555 583 668 535 752 897 151 895 060 305 576 967 284 778 875  $q^{8501} +$   
 911 755 718 211 700 383 586 533 691 017 560 984 525 346 178 087 756 790 557 268 454 824 612 824 517 428 574 988 577 060 118 402 310 884 017 743 288 618 845 455 787 515 471 427 632 320 056 907 637 145 573 788 162 938 473 693 441 368 117 558 119 707 048 831 586 458 376 654 889 368 960 000  $q^{8504} -$   
 939 000 136 943 776 753 700 947 924 653 562 819 833 527 320 437 511 805 121 810 415 809 944 321 588 951 068 778 272 104 831 374 022 173 918 178 224 172 763 052 233 287 227 620 339 808 993 748 077 786 079 323 038 944 191 199 478 921 507 799 487 224 970 579 810 625 799 887 081 473 638 400  $q^{8505} +$   
 1 025 705 382 214 247 763 200 009 109 991 668 719 019 572 091 000 180 661 057 769 636 704 486 801 398 779 417 070 381 493 277 269 897 725 623 896 947 411 944 223 598 006 344 418 255 914 281 716 681 674 802 542 329 421 534 771 963 287 891 706 105 688 279 152 639 947 907 429 526 452 750 336  $q^{8508} -$   
 1 056 347 464 381 667 968 285 239 170 067 764 259 807 299 218 509 062 378 674 256 268 651 481 108 813 384 373 987 452 969 653 975 367 955 569 682 784 696 833 163 824 634 670 656 207 321 430 472 667 892 064 137 880 430 263 706 680 037 965 328 980 403 727 080 521 752 407 654 219 683 079 000  $q^{8509} +$   
 1 153 864 404 121 044 857 048 840 374 131 973 529 471 400 622 714 218 136 090 775 064 733 953 115 214 932 939 263 674 738 044 096 505 271 585 234 918 889 585 072 688 836 413 169 816 635 176 896 089 918 568 086 392 095 406 893 903 485 452 923 260 068 829 210 137 793 460 197 011 996 540 928  $q^{8512} -$   
 1 188 326 925 680 688 717 168 937 652 825 677 582 546 648 715 163 012 194 448 181 378 851 918 025 643 132 131 919 665 968 808 932 820 436 862 859 967 958 692 665 606 192 164 443 680 618 556 651 535 049 547 566 604 921 404 710 391 072 337 386 750 303 883 025 995 072 070 912 511 589 842 944  $q^{8513} +$   
 1 298 000 705 819 903 899 498 255 099 827 783 976 002 355 378 799 363 870 187 528 530 132 379 622 337 976 599 172 857 594 708 104 787 730 296 783 742 537 068 662 190 223 361 442 595 191 778 384 768 567 585 616 663 177 893 524 918 653 501 454 925 587 213 669 477 210 154 075 184 558 080 000  $q^{8516} -$   
 1 336 758 931 654 764 499 562 779 781 344 763 286 003 591 878 318 406 597 608 567 335 570 665 924 984 771 056 561 466 760 268 583 316 987 039 143 272 444 622 457 804 007 912 269 074 157 050 446 451 419 505 362 972 784 506 645 699 305 869 765 857 213 300 351 440 212 623 066 094 152 716 815  $q^{8517} +$   
 1 460 101 681 275 550 878 474 320 864 515 978 465 463 372 556 101 724 003 755 886 224 657 001 231 957 658 935 161 689 367 120 995 128 365 688 487 378 693 106 205 873 956 989 786 211 111 032 297 927 846 509 875 289 722 958 604 301 149 073 135 341 400 236 245 838 505 436 958 021 211 136 000  $q^{8520} -$   
 1 503 689 867 284 268 443 421 047 062 868 598 938 523 012 300 834 285 393 102 044 449 155 596 229 314 471 159 484 610 096 966 711 123 647 653 991 472 020 899 418 896 902 696 999 077 090 594 774 647 295 804 997 609 867 954 805 686 620 215 096 995 839 418 206 634 477 881 169 018 789 888 000  $q^{8521} +$   
 1 642 401 381 159 588 882 241 858 832 067 255 428 290 135 812 926 158 352 971 227 268 471 722 132 648 107 755 298 227 976 843 260 236 840 644 124 809 084 870 010 150 872 508 844 007 393 958 632 709 467 541 457 178 841 784 422 632 091 476 779 266 414 682 175 632 068 992 328 433 984 320 000  $q^{8524} -$   
 1 691 420 079 995 020 661 088 894 279 571 818 175 778 537 799 794 083 995 758 802 103 647 823 564 404 784 352 034 832 532 186 798 768 710 599 848 862 067 293 939 128 776 082 397 163 097 013 793 963 036 266 997 198 689 420 181 277 550 188 324 584 115 155 930 127 373 658 109 652 460 366 650  $q^{8525} +$   
 1 847 411 057 144 900 001 381 070 514 006 842 945 593 571 824 300 546 787 176 242 649 361 866 849 796 175 833 552 336 536 083 095 692 352 555 337 333 868 058 924 972 025 351 220 875 898 923 641 016 729 269 712 628 535 097 012 091 551 428 561 734 171 749 514 979 469 755 179 079 169 114 112  $q^{8528} -$   
 1 902 535 326 709 680 409 090 448 268 050 263 079 350 487 612 531 881 912 539 657 409 732 199 418 720 957 925 426 682 435 815 494 678 309 169 647 149 649 829 390 510 257 171 555 390 496 130 836 784 096 307 050 999 629 574 761 322 103 463 916 773 443 351 188 361 250 894 393 829 584 896 000  $q^{8529} +$   
 2 077 953 480 147 454 456 534 955 070 429 066 040 472 781 147 375 163 281 599 678 088 944 021 728 512 352 088 519 546 725 594 486 281 836 058 469 719 596 130 646 411 054 081 219 191 448 105 986 332 178 250 477 062 571 522 957 093 041 693 527 223 150 061 417 885 788 997 765 849 789 513 728  $q^{8532} -$   
 2 139 942 106 149 437 128 198 084 980 507 576 723 498 346 484 882 957 031 424 440 218 981 374 192 298 892 866 850 773 857 429 861 382 321 258 903 194 987 273 901 968 927 885 309 848 648 626 174 228 034 701 818 385 756 576 711 134 734 436 667 383 644 647 932 739 244 146 586 384 072 508 863  $q^{8533} +$   
 2 337 201 497 769 986 498 946 388 456 896 963 581 552 078 383 737 749 404 530 229 837 643 554 003 321 268 556 955 790 882 082 225 881 145 635 456 913 275 811 116 421 432 968 046 083 405 872 956 127 803 808 005 755 205 736 222 894 948 003 847 545 475 047 140 344 943 954 402 385 264 128 000  $q^{8536} -$   
 2 406 907 355 332 597 949 118 421 029 854 376 612 976 513 187 638 423 946 728 863 297 529 060 172 742 718 695 360 564 337 010 319 455 450 635 006 497 589 716 087 372 190 887 277 664 934 033 179 743 143

946 443 272 594 920 135 709 038 542 582 629 490 633 658 217 808 230 275 792 081 354 752  $q^{8537} +$   
 2 628 721 353 430 788 633 264 475 529 330 387 836 692 127 588 316 536 334 220 971 478 626 405 023 196  
 047 587 701 323 220 082 177 253 329 225 137 789 818 990 735 801 546 717 790 211 378 682 670 499 120  
 572 875 493 348 201 301 329 427 938 317 286 890 712 197 324 143 962 590 930 246 656 000  $q^{8540} -$   
 2 707 103 048 126 066 464 308 404 588 051 067 162 017 768 380 204 720 788 582 831 711 701 681 683 793  
 576 531 182 111 652 455 642 767 912 258 690 055 643 573 912 122 342 437 393 996 409 402 341 529 930  
 629 656 736 180 367 298 302 114 111 648 844 545 467 086 048 387 475 638 086 149 956 250  $q^{8541} +$   
 2 956 521 353 913 406 121 954 438 308 161 125 023 799 187 611 219 579 247 388 502 998 736 289 950 838  
 993 551 794 478 595 663 957 809 710 811 035 798 982 071 816 993 143 057 136 510 757 715 838 557 342  
 696 332 898 003 620 934 118 375 633 413 858 293 523 208 542 260 516 534 585 582 592 000  $q^{8544} -$   
 3 044 656 299 844 664 407 466 496 365 720 139 112 346 006 128 964 444 994 165 560 149 552 585 318 100  
 160 054 758 622 920 985 447 868 913 328 164 395 849 298 081 587 902 877 448 957 535 170 168 808 315  
 648 592 059 546 081 625 806 729 220 123 668 558 333 283 841 641 076 002 565 146 214 400  $q^{8545} +$   
 3 325 106 544 209 388 945 764 126 896 476 224 386 377 852 279 102 718 296 593 519 547 275 870 760 557  
 758 263 842 935 800 519 319 133 555 907 395 666 578 333 412 472 729 581 595 610 331 776 999 501 189  
 300 427 826 546 765 850 741 605 560 778 759 706 320 109 238 137 589 634 119 055 310 848  $q^{8548} -$   
 3 424 205 656 147 021 151 428 485 161 067 864 468 893 394 462 464 796 525 154 717 185 310 201 814 487  
 068 642 341 044 661 167 201 255 812 647 044 700 441 619 123 064 854 925 421 662 169 698 650 562 064  
 912 960 583 309 061 993 745 835 779 619 536 113 432 877 873 172 906 722 046 971 003 500  $q^{8549} +$   
 3 739 540 129 511 676 052 992 623 357 873 442 566 085 805 467 763 873 075 551 709 313 866 905 260 967  
 720 811 146 964 116 715 440 348 776 610 997 050 674 093 653 041 218 974 470 097 550 816 265 958 909  
 957 551 947 175 740 650 992 169 600 122 588 274 916 125 889 415 788 436 028 283 727 360  $q^{8552} -$   
 3 850 964 327 838 760 087 412 893 513 537 862 510 099 168 812 681 030 022 712 722 394 426 551 987 630  
 078 918 401 927 717 055 289 431 196 656 142 474 974 194 183 848 832 219 741 300 150 387 190 242 086  
 686 405 114 981 090 564 253 011 847 553 913 128 160 778 043 281 316 261 281 164 918 784  $q^{8553} +$   
 4 205 512 475 133 747 556 461 424 376 998 082 897 350 464 800 914 100 549 657 984 641 071 238 280 971  
 656 659 797 102 460 109 935 932 589 493 934 627 098 850 073 646 115 321 240 903 336 804 551 395 245  
 667 454 811 859 737 139 250 826 244 522 778 404 522 933 833 103 672 887 889 604 096 000  $q^{8556} -$   
 4 330 791 226 778 702 971 102 158 195 402 207 460 500 875 257 266 019 394 493 081 597 117 494 736 685  
 035 480 865 403 515 203 514 576 100 995 284 194 847 143 954 131 504 574 550 956 086 444 539 338 126  
 704 372 164 205 887 497 988 240 276 142 349 004 041 932 891 688 799 661 004 014 722 327  $q^{8557} +$   
 4 729 418 617 194 758 622 643 724 586 695 486 769 734 612 839 542 788 281 347 046 851 868 324 648 622  
 301 756 690 124 917 193 241 033 927 303 120 966 161 748 016 527 048 104 131 319 561 191 673 691 122  
 288 702 258 936 417 935 201 906 121 620 377 817 905 135 032 642 108 294 840 104 960 000  $q^{8560} -$   
 4 870 270 763 142 681 325 676 304 753 980 657 030 567 578 188 756 950 539 537 384 830 941 906 129 602  
 786 410 688 021 347 203 332 240 969 110 759 532 952 642 755 266 237 075 829 781 487 925 746 905 087  
 923 220 627 631 483 318 055 620 254 612 372 758 432 701 300 137 912 798 237 614 080 000  $q^{8561} +$   
 5 318 445 331 487 229 459 809 418 378 442 439 857 994 802 619 609 725 884 376 580 309 603 014 457 403  
 472 999 125 565 311 827 551 483 055 591 252 196 610 793 872 292 775 177 425 799 223 617 829 808 876  
 999 298 626 884 597 598 388 894 352 433 979 266 119 120 162 219 064 403 557 393 152 000  $q^{8564} -$   
 5 476 802 482 235 894 148 526 815 238 587 123 712 186 384 954 194 203 905 883 231 914 637 678 762 213  
 324 749 823 937 468 921 691 428 311 679 720 687 262 925 762 670 631 898 333 334 694 420 317 963 961  
 440 812 032 291 537 137 586 521 170 451 725 719 431 267 810 515 788 201 771 132 163 500  $q^{8565} +$   
 5 980 668 936 561 743 083 701 845 537 394 371 000 957 061 983 412 745 145 579 141 840 556 121 872 278  
 796 269 431 754 997 455 112 168 245 207 935 254 502 385 388 824 322 528 477 394 006 725 069 492 099  
 113 331 610 917 182 020 245 196 098 472 047 883 412 595 285 653 391 886 928 382 978 048  $q^{8568} -$   
 6 158 701 751 433 511 177 640 774 352 158 983 064 379 694 759 280 200 066 952 290 547 771 597 633 268  
 388 653 291 044 522 181 101 774 627 740 548 993 506 215 240 945 435 364 667 311 079 254 138 230 213  
 470 400 498 615 925 342 111 911 021 995 470 546 111 710 282 197 342 871 225 810 944 000  $q^{8569} +$   
 6 725 165 151 439 474 010 563 076 525 911 822 447 908 166 019 934 960 687 647 774 549 936 621 320 466  
 131 608 175 541 031 919 057 245 395 672 278 645 658 992 321 550 183 389 829 075 957 189 991 223 248  
 089 157 534 415 157 265 402 051 709 284 472 836 904 901 527 282 166 626 322 695 446 528  $q^{8572} -$   
 6 925 312 856 437 504 691 567 469 952 890 135 829 050 918 630 227 847 735 852 129 242 947 616 093 888  
 113 254 207 958 429 379 151 507 011 549 591 074 078 478 775 769 530 961 470 943 105 719 761 777 564  
 546 223 475 549 307 917 482 959 109 131 478 680 048 802 642 690 603 841 098 654 322 263  $q^{8573} +$

7 562 132 490 424 696 541 856 823 771 154 180 847 703 277 351 393 083 110 103 907 347 154 146 002 756 \
 281 808 476 356 369 645 097 474 345 266 055 100 897 241 724 455 181 758 196 198 188 542 804 709 602 \
 808 771 360 868 502 323 306 524 311 640 184 021 702 433 215 887 075 495 621 988 352 000  $q^{8576} -$

7 787 136 032 848 200 250 525 461 039 190 332 579 342 298 254 717 453 499 338 193 672 403 663 962 546 \
 807 997 662 198 520 972 750 363 000 374 723 323 098 767 074 555 172 051 073 539 232 185 855 255 966 \
 794 420 249 375 016 174 873 809 126 663 452 546 090 965 843 522 511 248 241 963 433 984  $q^{8577} +$

8 503 030 859 397 144 254 673 498 387 549 027 217 916 852 185 559 222 483 564 378 111 849 218 259 925 \
 496 041 744 579 931 834 513 647 340 525 627 737 212 328 607 155 839 414 567 892 074 813 976 216 391 \
 640 729 384 583 128 580 588 724 129 064 571 597 893 639 298 960 893 125 586 573 721 600  $q^{8580} -$

8 755 970 146 286 296 861 563 749 853 358 243 988 532 981 687 258 350 981 794 896 062 656 542 098 621 \
 050 273 110 388 780 126 777 935 935 769 394 509 172 148 749 563 981 209 379 932 060 404 947 671 335 \
 163 892 057 871 942 830 853 709 587 175 288 092 942 968 400 069 197 588 444 251 125 875  $q^{8581} +$

9 560 737 222 143 238 422 534 215 381 608 359 236 793 930 420 389 231 459 553 197 360 310 583 738 697 \
 541 785 149 291 586 477 739 648 948 760 541 574 901 354 698 769 382 220 185 775 975 317 530 002 263 \
 998 258 871 963 614 022 332 104 673 853 933 325 118 247 437 174 451 985 194 060 160 000  $q^{8584} -$

9 845 072 944 460 907 741 604 042 968 794 070 586 862 323 152 659 024 469 715 359 035 377 502 844 018 \
 461 708 565 566 337 356 944 975 369 289 103 150 621 770 977 223 418 647 218 129 455 352 316 755 628 \
 791 467 330 206 467 818 594 238 602 285 520 297 665 807 730 859 342 558 229 823 488 000  $q^{8585} +$

10 749 720 434 456 452 097 014 025 495 362 097 628 134 952 837 619 318 025 228 720 007 115 327 648 \
 436 661 375 628 859 118 025 645 696 453 165 033 916 512 545 107 814 563 941 334 753 030 681 132 982 \
 952 533 064 544 777 632 151 953 330 343 392 458 978 049 163 493 037 060 353 368 334 855 168  $q^{8588} -$

11 069 341 040 461 564 936 073 374 832 545 334 508 889 613 880 088 945 551 446 941 088 590 377 615 \
 542 983 130 250 074 739 651 349 508 017 630 111 677 222 380 518 955 601 629 185 329 077 569 878 000 \
 553 093 617 146 108 415 867 109 644 970 207 323 845 634 021 201 230 831 075 911 392 091 125  $q^{8589} +$

12 086 237 600 952 727 576 609 089 169 576 010 721 996 222 600 596 027 790 577 757 524 921 142 024 \
 223 352 536 657 723 300 080 223 480 340 123 004 626 173 193 626 218 493 212 525 133 375 138 593 759 \
 455 467 727 317 572 670 035 443 787 554 381 723 082 251 996 685 210 409 797 439 836 520 448  $q^{8592} -$

12 445 512 051 298 438 463 023 891 793 709 317 148 171 879 312 751 039 470 642 322 593 381 495 515 \
 809 656 799 761 689 512 342 434 322 893 051 928 857 408 195 252 138 091 480 553 599 904 330 481 989 \
 650 570 337 422 113 075 099 302 633 747 045 103 754 678 243 694 503 810 655 010 774 515 712  $q^{8593} +$

13 588 554 598 231 167 129 532 605 938 241 081 734 294 093 299 181 391 378 373 760 592 989 552 626 \
 675 953 668 070 906 613 963 702 060 138 331 346 966 551 293 748 147 214 454 253 524 877 573 330 834 \
 231 760 153 251 378 295 297 372 079 916 144 909 708 585 951 224 193 451 279 907 358 208 000  $q^{8596} -$

13 992 391 612 849 342 752 565 396 019 040 822 747 098 242 532 234 683 242 120 897 200 127 306 965 \
 608 643 996 297 359 288 881 820 915 381 129 635 397 301 728 097 370 694 104 265 394 843 767 897 737 \
 645 826 306 299 892 198 276 271 461 059 130 446 304 150 443 151 582 260 726 155 707 557 498  $q^{8597} +$

15 277 193 732 004 594 047 167 727 424 714 205 688 188 749 489 783 378 735 554 319 879 696 463 811 \
 822 400 723 276 805 914 572 226 477 329 130 417 021 784 210 128 235 687 119 766 693 230 502 317 705 \
 231 502 038 988 657 179 624 269 261 855 117 434 832 299 064 065 179 963 073 853 948 352 000  $q^{8600} -$

15 731 108 325 847 852 868 428 497 769 885 945 503 824 490 601 849 994 286 083 408 101 776 255 123 \
 078 196 553 955 444 463 583 841 535 821 529 883 921 235 800 379 616 714 567 521 820 872 742 495 952 \
 154 320 906 635 651 558 513 300 414 116 145 731 505 440 514 446 425 788 499 892 142 080 000  $q^{8601} +$

17 175 211 859 438 343 366 260 202 690 378 412 595 900 691 872 008 285 463 354 279 998 456 116 394 \
 823 604 231 800 134 017 492 656 033 057 907 464 686 182 345 857 270 228 059 474 546 029 488 735 148 \
 282 624 784 656 899 236 408 173 323 441 366 351 566 450 860 720 483 759 903 990 185 472 000  $q^{8604} -$

17 685 400 061 798 940 552 806 140 472 744 032 889 556 828 064 487 150 763 737 582 339 077 146 621 \
 658 599 856 136 676 766 375 351 565 543 137 853 720 971 920 538 727 971 484 758 001 277 982 143 735 \
 274 395 744 672 264 551 857 676 597 446 334 384 077 634 765 105 935 341 299 223 542 623 650  $q^{8605} +$

19 308 512 716 002 846 945 647 763 277 977 459 883 468 517 484 691 673 608 417 273 497 685 371 948 \
 901 992 961 235 066 426 380 318 240 839 165 786 825 740 752 084 348 001 355 889 137 531 955 297 136 \
 405 730 046 604 517 495 290 986 864 645 355 931 015 865 850 391 504 286 669 833 450 835 968  $q^{8608} -$

19 881 935 477 711 885 682 693 572 726 202 599 226 773 449 812 623 824 719 103 882 325 975 936 999 \
 959 703 543 461 628 318 717 763 695 281 516 637 219 772 465 630 764 522 853 537 783 718 823 280 085 \
 750 217 640 671 116 933 348 519 459 988 437 102 879 366 463 060 872 730 349 992 116 224 000  $q^{8609} +$

21 706 197 644 088 789 173 118 577 315 414 800 735 259 626 362 535 761 997 684 914 451 253 134 225 \

809 773 466 035 158 385 758 578 123 288 943 927 833 843 942 594 876 273 817 211 429 776 327 667 926 \
 206 548 080 452 978 295 129 897 409 980 535 513 084 086 661 698 726 714 187 515 394 326 528  $q^{8612} -$

22 350 675 059 875 359 801 132 730 383 312 591 487 687 086 113 657 877 090 679 830 563 616 970 999 \
 472 937 860 269 763 934 391 104 629 247 753 840 536 585 209 275 685 185 320 211 329 740 832 946 175 \
 844 746 133 391 321 623 706 781 156 863 423 282 290 716 842 718 316 710 258 428 094 007 145  $q^{8613} +$

24 400 959 434 535 382 061 353 025 723 775 556 284 749 625 816 190 407 507 766 341 082 826 597 242 \
 065 567 974 736 738 446 553 150 062 782 221 495 817 400 815 222 515 855 719 455 376 610 180 579 741 \
 395 932 306 777 147 105 163 441 874 155 482 932 055 901 643 871 512 627 862 086 527 232 000  $q^{8616} -$

25 125 276 545 826 230 503 368 291 478 518 746 391 871 107 599 404 193 489 107 696 508 709 586 619 \
 855 395 108 674 748 527 546 712 262 194 220 139 273 851 112 715 114 060 773 948 703 187 412 934 631 \
 500 853 169 302 522 555 290 515 906 763 979 944 816 767 858 889 368 790 130 878 910 889 984  $q^{8617} +$

27 429 524 568 905 338 648 425 286 802 006 771 424 073 237 063 390 062 760 374 030 291 093 316 076 \
 462 336 105 038 969 547 565 057 018 745 202 959 936 097 344 719 765 988 502 832 738 002 517 469 940 \
 792 825 022 906 868 816 078 457 181 871 040 472 665 308 008 936 497 513 453 273 059 276 800  $q^{8620} -$

28 243 550 167 203 167 826 661 083 086 941 812 299 707 383 988 231 865 677 508 789 175 721 797 032 \
 867 427 476 666 580 892 053 672 446 225 231 125 891 101 479 802 671 866 549 202 905 067 787 071 670 \
 266 410 631 460 327 362 852 293 291 379 062 501 990 497 709 893 450 728 012 683 590 226 125  $q^{8621} +$

30 833 149 797 457 113 036 718 532 296 968 422 864 071 032 804 212 431 064 045 083 224 154 610 184 \
 065 184 056 708 398 526 895 089 989 146 949 008 482 188 343 017 755 734 338 142 345 567 792 278 680 \
 990 447 971 405 311 335 949 863 006 752 950 959 799 444 217 176 510 283 316 285 881 856 000  $q^{8624} -$

31 747 969 822 204 038 227 104 916 622 914 650 431 386 507 647 285 507 031 111 847 550 406 520 637 \
 527 302 145 753 773 626 375 780 772 216 145 152 988 495 813 650 099 915 649 880 446 675 439 772 217 \
 319 885 642 349 717 721 394 054 143 275 414 855 822 217 458 950 570 061 153 373 634 560 000  $q^{8625} +$

34 658 179 713 899 379 434 339 282 020 850 598 606 346 331 141 213 212 870 501 740 005 539 683 991 \
 233 737 628 094 798 789 701 200 780 472 643 184 264 245 860 753 527 652 025 729 320 623 197 393 558 \
 755 152 301 153 482 511 503 695 843 757 941 307 525 130 384 249 410 993 177 143 797 440 512  $q^{8628} -$

35 686 247 033 715 632 876 526 185 397 876 250 677 845 199 108 416 814 753 036 496 823 880 901 321 \
 322 422 954 429 582 670 786 812 423 852 256 051 541 302 939 972 389 812 998 275 309 929 694 742 966 \
 300 698 467 127 291 596 470 944 730 825 209 760 458 321 209 211 801 448 459 745 721 098 000  $q^{8629} +$

38 956 672 802 791 701 415 575 874 647 924 679 995 754 445 423 432 397 402 240 221 965 238 332 865 \
 429 736 662 169 703 038 015 895 073 909 794 751 571 132 102 983 279 711 103 266 628 348 471 580 722 \
 010 933 199 335 622 733 050 779 319 870 391 444 907 268 782 995 357 741 408 665 919 943 680  $q^{8632} -$

40 111 975 387 762 797 798 751 662 286 054 314 019 087 375 543 399 164 691 224 117 424 303 699 961 \
 793 843 157 439 052 063 214 655 063 790 082 448 586 733 374 499 520 346 663 754 533 571 406 302 860 \
 500 468 778 936 871 079 137 968 451 077 311 476 910 957 934 889 359 897 670 132 414 808 064  $q^{8633} +$

43 787 104 349 676 389 187 605 648 686 042 730 468 549 077 582 960 847 141 208 798 493 136 734 302 \
 890 651 296 507 901 804 752 073 719 182 724 662 139 408 914 530 312 887 839 577 286 829 368 167 377 \
 076 708 386 043 277 342 186 421 105 461 524 687 901 546 000 697 454 065 165 720 883 200 000  $q^{8636} -$

45 085 354 087 843 132 775 265 791 779 926 641 288 640 839 779 597 113 710 437 106 557 845 745 678 \
 908 925 995 350 251 259 304 389 138 550 847 470 341 251 196 028 761 686 545 423 186 085 358 470 281 \
 553 576 195 741 356 953 440 654 493 035 402 064 407 587 296 477 709 292 273 796 873 599 466  $q^{8637} +$

49 215 155 629 799 439 453 733 748 519 146 508 120 453 247 512 311 418 693 985 009 086 714 740 201 \
 985 324 272 604 002 024 457 570 586 635 620 812 359 476 033 367 839 010 044 386 249 515 356 556 103 \
 740 117 076 596 280 179 596 710 418 904 415 824 794 093 612 328 145 605 015 131 088 486 400  $q^{8640} -$

50 674 000 316 435 109 271 901 945 456 598 822 802 924 451 640 692 960 657 848 206 722 581 577 979 \
 428 107 651 236 283 402 140 667 289 796 249 202 016 562 513 829 760 482 496 728 133 525 740 589 050 \
 193 581 089 276 724 896 230 703 514 603 384 394 305 301 925 356 395 230 026 460 573 696 000  $q^{8641} +$

55 314 599 942 184 409 246 252 719 815 685 263 548 040 556 400 242 638 060 260 624 096 027 107 453 \
 405 762 648 937 839 304 339 306 362 127 313 696 523 854 057 279 474 730 667 222 224 973 777 125 698 \
 984 973 330 712 303 491 780 420 671 492 166 561 851 626 062 041 723 275 730 842 306 560 000  $q^{8644} -$

56 953 861 279 467 864 133 923 493 901 782 114 067 898 435 710 472 614 790 623 806 070 152 144 540 \
 746 041 372 028 234 270 184 002 128 325 685 760 384 955 399 719 179 727 508 370 673 023 422 221 453 \
 533 659 467 342 017 995 927 656 777 043 352 970 255 256 509 373 977 413 520 458 079 384 400  $q^{8645} +$

62 168 297 347 093 121 869 755 455 602 878 724 122 556 292 080 411 611 921 255 637 657 555 242 904 \
 100 311 103 197 798 867 901 207 754 114 250 015 309 795 514 317 792 856 150 316 364 630 243 073 455 \

842 816 715 778 058 779 644 279 925 561 251 438 886 784 979 900 794 173 477 825 952 258 048  $q^{8648} -$   
 64 010 238 138 493 888 421 586 901 953 903 444 915 675 993 796 265 950 207 128 084 211 169 213 213  $\setminus$   
 367 158 530 814 557 129 998 899 019 021 832 842 028 313 995 415 460 118 101 508 365 483 244 372 232  $\setminus$   
 548 329 789 496 530 308 987 405 576 323 962 404 756 184 256 247 514 378 458 959 876 096 248  $q^{8649} +$   
 69 869 311 413 622 063 262 053 475 566 633 502 883 071 232 999 538 616 660 445 189 325 771 993 483  $\setminus$   
 201 711 101 235 944 076 422 812 153 168 407 171 499 049 735 932 150 377 916 956 826 275 200 326 149  $\setminus$   
 023 294 920 791 048 504 437 722 920 792 459 158 902 615 352 454 602 888 190 095 556 251 648  $q^{8652} -$   
 71 938 935 526 288 639 684 872 395 310 458 096 115 788 824 389 727 241 939 598 427 504 249 417 768  $\setminus$   
 630 949 999 432 030 082 210 491 255 107 566 388 290 337 192 386 513 335 653 508 948 977 719 155 508  $\setminus$   
 083 684 696 071 078 429 427 258 601 613 241 490 190 586 945 420 334 005 299 726 170 251 025  $q^{8653} +$   
 78 522 162 909 497 975 501 684 830 581 691 083 159 400 658 717 816 114 496 476 341 690 573 359 028  $\setminus$   
 062 066 372 237 115 119 244 293 983 795 933 973 341 376 412 479 109 861 187 440 361 769 612 055 916  $\setminus$   
 343 928 802 383 503 777 241 568 336 986 622 647 090 467 473 072 109 304 324 435 482 624 000  $q^{8656} -$   
 80 847 552 014 325 155 811 476 065 549 197 431 462 675 236 379 804 109 630 031 077 185 642 622 108  $\setminus$   
 716 080 534 642 155 701 074 204 968 915 321 414 895 910 487 866 656 653 174 515 281 609 051 263 988  $\setminus$   
 447 789 734 552 377 065 456 831 159 363 022 458 109 109 215 118 607 272 973 735 242 989 568  $q^{8657} +$   
 88 244 237 188 530 478 549 495 570 347 774 430 388 334 727 349 817 338 199 898 026 702 421 694 201  $\setminus$   
 604 117 942 348 692 905 133 073 666 240 287 034 939 678 263 878 895 926 995 748 931 247 505 134 552  $\setminus$   
 924 861 596 728 641 969 016 871 151 210 847 124 850 639 168 980 091 987 351 087 982 080 000  $q^{8660} -$   
 90 856 928 777 141 071 883 544 740 062 028 212 848 071 575 253 067 758 145 680 968 477 423 873 770  $\setminus$   
 578 184 662 153 446 091 794 374 028 203 524 857 582 884 795 630 206 324 279 581 697 155 813 380 352  $\setminus$   
 645 635 284 573 591 696 417 763 122 921 966 197 537 604 174 380 590 872 235 070 921 754 625  $q^{8661} +$   
 99 167 364 076 740 386 701 228 917 304 688 666 729 418 727 158 856 467 700 249 634 669 468 370 188  $\setminus$   
 401 384 048 576 049 988 453 751 461 758 144 890 564 129 004 663 857 841 602 659 160 246 194 697 481  $\setminus$   
 066 551 292 736 347 283 714 307 882 994 967 027 992 272 003 226 866 785 085 703 992 768 000  $q^{8664} -$   
 102 102 775 803 816 492 689 749 997 997 580 443 849 886 091 694 097 572 095 160 290 939 036 371 612  $\setminus$   
 952 944 684 418 643 712 028 557 523 203 156 913 139 479 349 067 605 629 108 201 950 552 905 066 530  $\setminus$   
 857 185 925 261 943 110 378 819 165 030 410 404 258 428 736 400 754 048 647 338 301 849 600  $q^{8665} +$   
 111 439 591 352 919 086 432 052 442 873 260 440 576 299 772 474 980 587 022 620 788 610 338 340 182  $\setminus$   
 235 518 205 782 257 433 880 876 700 737 969 499 959 928 243 630 193 513 606 785 846 935 200 191 068  $\setminus$   
 571 393 287 543 918 542 362 705 549 883 427 168 666 900 172 168 353 552 817 040 088 176 640  $q^{8668} -$   
 114 737 497 368 407 632 407 470 672 081 989 905 250 054 993 948 797 268 215 070 696 496 417 247 771  $\setminus$   
 441 418 212 343 996 464 801 413 924 374 662 035 954 406 839 531 117 873 875 222 678 947 092 014 311  $\setminus$   
 364 437 688 618 708 945 174 758 416 791 713 082 311 341 780 354 399 921 471 295 589 682 250  $q^{8669} +$   
 125 227 175 493 572 592 143 330 359 557 528 701 034 369 324 009 908 904 450 861 210 715 272 983 900  $\setminus$   
 055 874 484 250 007 329 016 863 833 741 532 880 881 278 785 968 270 257 519 132 600 123 493 056 427  $\setminus$   
 099 250 563 617 058 201 651 513 851 503 076 230 369 064 331 480 002 228 188 160 211 959 808  $q^{8672} -$   
 128 932 241 120 397 950 078 739 006 580 018 061 175 894 480 160 111 345 430 253 588 783 937 951 467  $\setminus$   
 942 210 712 935 092 547 676 145 265 413 694 983 290 104 228 368 020 687 850 129 500 192 623 646 503  $\setminus$   
 723 229 645 088 571 421 545 902 653 006 355 841 287 420 804 075 900 413 022 389 028 290 560  $q^{8673} +$   
 140 716 816 239 822 263 228 012 687 777 189 200 542 223 896 474 327 256 419 664 014 332 626 025 761  $\setminus$   
 506 310 953 495 562 591 978 634 777 343 543 181 412 934 234 411 194 489 378 553 335 753 601 103 245  $\setminus$   
 302 448 245 449 013 910 945 892 176 725 861 181 460 795 020 395 895 792 789 978 224 640 000  $q^{8676} -$   
 144 879 198 127 979 924 594 877 950 600 842 694 857 182 749 921 830 364 210 728 534 575 842 119 056  $\setminus$   
 962 622 315 016 826 187 719 639 075 592 932 075 220 526 727 705 596 785 296 627 013 012 639 374 061  $\setminus$   
 971 147 409 551 856 958 339 255 050 611 766 715 420 801 800 531 498 301 992 385 610 536 494  $q^{8677} +$   
 158 118 164 782 948 542 174 237 256 707 458 796 697 374 031 230 959 119 496 961 432 663 900 608 455  $\setminus$   
 120 458 707 419 719 433 566 174 486 508 692 585 833 802 006 922 246 460 605 756 962 940 893 159 525  $\setminus$   
 493 911 124 981 730 937 825 743 046 400 332 677 831 640 026 279 771 373 756 278 217 216 000  $q^{8680} -$   
 162 794 184 540 447 445 688 577 886 811 066 901 541 288 832 374 849 644 064 058 551 117 227 541 571  $\setminus$   
 815 885 271 534 166 485 216 347 536 738 886 157 476 091 005 314 327 067 178 255 509 490 350 940 911  $\setminus$   
 301 576 248 270 966 308 929 618 249 195 480 920 417 861 439 428 583 283 116 193 177 600 000  $q^{8681} +$   
 177 666 638 998 565 780 017 151 494 541 949 951 393 365 342 406 125 194 363 541 460 065 377 467 973  $\setminus$   
 075 934 114 643 824 634 046 295 188 911 469 659 472 310 367 832 840 237 843 450 623 477 598 892 059  $\setminus$   
 177 645 345 632 048 064 144 727 794 906 665 605 176 431 032 480 649 844 167 690 900 864 000  $q^{8684} -$

182 919 539 275 090 947 906 738 316 688 690 043 362 650 545 442 096 945 147 505 793 114 031 028 054 \
 141 482 084 887 161 908 204 374 925 454 042 245 482 265 296 064 673 686 117 909 240 195 612 087 824 \
 754 146 658 761 177 676 101 957 003 410 501 156 037 090 880 121 032 770 298 595 968 073 700  $q^{8685} +$  \
 199 626 583 234 770 231 670 912 579 419 872 178 192 509 617 520 758 678 068 289 412 684 172 735 052 \
 350 122 250 634 569 456 531 228 422 219 642 723 199 231 202 846 495 607 873 388 459 622 241 715 383 \
 877 685 592 658 270 416 317 254 569 250 027 675 329 208 267 490 278 153 761 379 920 363 520  $q^{8688} -$  \
 205 527 376 327 998 223 630 745 061 522 208 121 907 352 175 909 977 994 002 980 307 756 871 260 885 \
 541 461 670 527 314 907 323 775 178 085 164 352 799 140 809 464 416 120 763 013 781 379 069 167 790 \
 561 165 372 944 406 129 509 410 049 824 236 279 987 916 462 818 266 411 117 499 822 080 000  $q^{8689} +$  \
 224 294 814 730 673 865 204 583 705 190 426 081 593 152 545 151 059 733 627 910 725 111 941 569 247 \
 007 012 781 025 352 704 976 831 125 644 953 567 118 786 810 270 655 871 499 830 524 318 583 592 974 \
 054 451 694 697 124 356 545 076 659 855 837 890 723 012 811 430 059 887 591 806 574 448 640  $q^{8692} -$  \
 230 923 235 012 293 771 978 648 598 248 293 210 227 809 471 341 090 180 954 479 042 274 340 634 043 \
 861 833 061 207 761 029 193 256 094 234 059 401 711 771 119 662 028 064 724 741 501 967 737 350 421 \
 507 128 486 171 956 402 222 010 490 631 386 838 316 914 433 511 975 440 358 314 889 476 574  $q^{8693} +$  \
 252 004 603 868 688 305 967 635 097 333 118 027 034 824 290 647 201 833 675 356 872 047 667 559 498 \
 554 644 783 405 579 320 878 616 651 183 878 181 112 162 053 153 620 260 019 478 941 713 383 364 163 \
 108 572 854 826 721 323 314 096 828 360 408 466 505 185 742 631 607 597 677 020 276 736 000  $q^{8696} -$  \
 259 450 176 703 507 465 335 417 731 962 149 616 465 312 623 426 607 236 220 448 663 301 441 874 972 \
 385 431 799 968 214 431 748 635 768 163 775 724 665 237 350 636 220 960 205 571 186 029 858 219 695 \
 070 641 487 536 680 154 802 129 027 981 614 342 752 603 507 114 095 843 302 664 970 895 360  $q^{8697} +$  \
 283 130 141 214 206 577 819 847 594 368 256 867 285 375 013 205 908 187 495 551 256 633 676 234 211 \
 283 330 907 063 613 635 960 956 021 440 125 891 553 237 369 308 039 366 220 029 831 381 402 421 781 \
 482 957 310 665 075 573 437 885 126 847 894 726 509 171 712 578 545 480 443 689 135 769 600  $q^{8700} -$  \
 291 493 382 589 354 907 752 002 276 542 762 555 638 317 938 295 159 539 036 879 240 324 002 289 093 \
 997 883 744 142 273 431 720 536 287 534 630 420 960 480 283 009 924 550 890 978 637 488 818 219 339 \
 937 040 899 945 812 488 946 013 043 160 283 545 420 298 202 189 406 871 515 172 511 528 375  $q^{8701} +$  \
 318 091 550 745 562 228 017 761 854 121 878 633 933 213 460 360 643 369 853 971 340 545 577 758 550 \
 022 175 311 289 569 840 769 071 837 808 656 158 844 746 979 379 964 227 615 026 276 726 918 834 996 \
 252 333 399 786 616 305 631 455 135 443 764 553 126 310 476 360 956 311 867 848 458 240 000  $q^{8704} -$  \
 327 485 313 558 045 360 790 112 525 744 428 427 345 834 761 521 388 758 405 913 943 529 581 494 784 \
 313 109 047 637 149 006 967 356 330 968 570 206 578 293 362 483 715 569 621 183 728 914 352 896 799 \
 474 434 540 726 434 838 791 950 751 726 286 740 348 668 408 197 692 785 413 988 458 496 000  $q^{8705} +$  \
 357 360 515 910 095 753 083 681 190 943 152 219 329 335 808 627 016 903 559 493 368 199 390 401 429 \
 277 851 869 534 852 793 692 402 148 465 590 245 036 262 892 233 663 836 468 758 934 962 443 004 694 \
 244 517 827 651 310 434 642 111 348 849 041 592 250 021 476 910 693 602 272 638 115 676 160  $q^{8708} -$  \
 367 911 500 802 534 352 231 142 821 338 557 380 619 482 575 956 720 730 317 185 541 061 558 661 218 \
 111 519 949 101 909 386 589 630 211 339 894 126 444 724 928 883 084 045 451 429 149 036 644 994 794 \
 286 758 221 171 322 271 415 510 131 636 625 320 297 425 870 893 834 270 139 791 435 617 750  $q^{8709} +$  \
 401 466 593 253 855 159 911 195 661 550 169 915 372 223 888 546 913 541 119 900 995 772 728 231 577 \
 261 796 005 544 417 285 002 856 929 892 946 350 585 052 397 151 659 905 524 837 909 273 851 931 406 \
 936 021 616 961 625 775 138 595 590 216 233 613 615 297 395 164 620 944 920 217 246 608 640  $q^{8712} -$  \
 413 317 044 065 687 830 322 276 946 146 939 614 880 631 644 753 094 824 783 814 605 062 416 244 634 \
 334 397 405 531 240 184 019 638 589 431 179 806 055 282 158 040 302 082 933 635 631 996 951 864 872 \
 135 859 500 209 684 743 990 873 834 314 090 793 200 972 695 269 535 519 666 485 518 630 912  $q^{8713} +$  \
 451 004 297 469 426 203 760 651 927 033 750 982 888 469 098 217 071 449 944 204 566 270 376 645 714 \
 465 339 699 530 596 513 171 287 046 347 028 369 212 192 591 126 632 964 218 546 674 323 976 275 790 \
 683 128 219 671 363 277 223 919 403 802 371 869 659 902 069 441 254 517 154 938 989 504 000  $q^{8716} -$  \
 464 313 903 812 733 093 420 095 197 047 579 060 472 659 128 065 442 561 819 490 006 252 254 042 530 \
 639 020 612 807 530 710 780 436 777 467 165 191 439 357 904 516 411 406 314 507 880 812 009 598 302 \
 548 553 556 229 532 310 188 643 158 832 530 242 901 541 615 451 042 383 084 405 529 482 594  $q^{8717} +$  \
 506 641 051 908 038 476 121 443 667 799 229 377 100 508 819 598 058 628 822 352 755 054 661 242 780 \
 360 092 502 107 504 566 302 096 634 090 511 970 452 954 210 823 816 676 442 634 374 825 298 674 065 \
 715 444 333 452 503 112 911 489 681 353 858 892 927 753 282 419 718 078 103 432 658 944 000  $q^{8720} -$  \
 521 589 084 115 506 104 908 950 217 265 461 003 973 645 022 491 904 698 177 114 741 879 843 407 462 \

376 141 847 401 607 889 765 585 756 902 508 315 828 963 895 372 696 863 114 546 767 620 172 097 938 \
 007 500 220 250 224 617 007 540 679 760 298 949 879 770 592 991 518 517 174 595 387 392 000  $q^{8721} +$  \
 569 126 110 042 276 214 219 487 132 161 154 929 003 075 297 695 750 553 742 222 461 477 514 694 928 \
 256 081 875 948 525 966 248 253 566 488 473 445 138 062 530 690 146 385 811 417 833 566 949 782 716 \
 312 082 275 842 679 929 624 774 501 475 938 024 959 246 801 872 836 324 465 754 196 480 000  $q^{8724} -$  \
 585 913 814 805 589 794 423 389 588 758 918 547 010 185 106 483 406 675 482 577 978 786 994 819 141 \
 689 300 337 338 790 414 087 482 852 323 336 508 694 870 899 982 394 875 344 309 570 419 759 198 697 \
 706 569 047 636 937 550 789 694 052 711 011 976 997 222 896 821 051 773 588 690 924 272 950  $q^{8725} +$  \
 639 300 566 194 469 973 755 556 780 351 967 037 055 901 769 949 490 041 235 041 770 948 528 155 141 \
 793 722 145 670 710 586 499 784 779 825 727 014 495 648 188 787 084 209 385 450 174 179 784 271 861 \
 739 022 250 554 691 401 554 792 391 801 638 911 670 550 277 618 330 132 291 476 108 816 896  $q^{8728} -$  \
 658 153 854 654 847 935 228 987 099 714 251 168 633 084 949 607 200 819 214 139 473 891 249 891 345 \
 517 275 915 246 455 094 908 582 042 089 881 620 364 639 100 915 739 395 352 986 362 329 885 561 121 \
 695 072 979 205 844 169 773 060 960 986 132 175 727 545 104 241 656 679 082 901 569 536 000  $q^{8729} +$  \
 718 108 588 231 324 131 516 464 271 138 027 969 488 713 809 741 961 190 956 800 009 710 129 134 950 \
 805 053 701 279 811 809 655 817 194 411 542 725 727 383 229 303 882 152 533 628 593 964 556 601 608 \
 087 230 756 514 912 536 894 133 405 933 033 341 670 409 055 361 364 326 168 185 280 366 592  $q^{8732} -$  \
 739 281 052 145 126 737 619 293 657 029 415 586 892 683 919 429 359 386 594 583 108 185 461 212 187 \
 950 967 981 360 579 266 910 824 657 778 612 467 669 711 614 183 322 876 454 696 808 081 992 098 042 \
 642 531 692 346 674 725 816 001 108 632 581 998 925 576 486 200 168 499 017 773 777 841 470  $q^{8733} +$  \
 806 610 021 056 034 121 188 829 447 154 915 494 909 475 580 063 053 533 711 028 169 791 857 704 024 \
 787 179 073 091 142 140 362 932 277 568 775 039 709 976 931 334 524 369 874 972 254 851 129 012 485 \
 543 434 204 141 284 784 019 858 356 663 210 348 946 788 108 747 326 839 257 761 273 856 000  $q^{8736} -$  \
 830 386 316 987 962 267 758 005 283 798 920 696 143 935 619 882 231 862 463 723 303 755 266 076 385 \
 427 852 932 051 657 874 390 688 925 547 722 172 612 534 640 899 759 734 468 392 511 568 792 944 118 \
 103 195 488 536 398 494 153 916 076 948 345 169 012 249 640 004 282 989 814 977 674 248 192  $q^{8737} +$  \
 905 994 527 816 326 765 057 668 174 916 281 480 230 581 386 580 632 299 568 156 843 703 000 823 881 \
 866 884 807 148 488 922 812 173 193 965 240 205 115 070 931 461 568 415 575 179 009 641 414 271 438 \
 950 451 060 827 219 112 180 716 974 024 627 672 853 520 666 415 063 941 674 085 301 452 800  $q^{8740} -$  \
 932 694 174 167 366 221 309 497 718 188 471 792 378 983 757 133 109 095 302 516 176 698 145 600 798 \
 537 854 963 441 368 616 565 385 994 587 451 773 398 352 324 823 671 109 507 214 911 189 700 899 941 \
 986 534 200 052 689 284 733 354 106 753 989 857 436 911 827 285 807 888 479 742 222 415 000  $q^{8741} +$  \
 1 017 597 456 027 294 387 838 970 767 847 996 293 162 146 894 070 786 552 154 246 929 747 342 982 322 \
 584 830 213 980 649 349 338 206 578 795 804 543 751 361 538 108 355 150 968 027 997 785 649 654 527 \
 645 462 341 537 848 431 136 181 773 007 531 443 308 685 709 803 796 611 721 921 985 472 000  $q^{8744} -$  \
 1 047 579 093 147 788 800 824 297 639 063 010 534 183 897 295 990 561 219 143 542 281 978 308 227 270 \
 376 777 059 249 833 086 203 336 660 836 201 227 427 435 522 794 428 732 510 284 399 839 587 920 814 \
 799 595 160 335 145 331 709 028 863 074 404 651 969 359 263 890 138 667 497 468 759 244 800  $q^{8745} +$  \
 1 142 917 638 546 958 116 472 642 384 640 603 357 187 835 351 028 937 501 394 058 418 062 722 122 051 \
 432 169 710 121 539 453 180 805 472 729 406 554 554 204 021 217 895 589 234 302 460 588 998 741 754 \
 389 117 064 025 221 695 877 890 706 638 006 873 356 044 837 810 345 938 869 320 213 106 688  $q^{8748} -$  \
 1 176 583 808 288 215 951 839 528 475 090 464 214 640 619 818 369 146 310 886 834 293 077 843 101 101 \
 080 096 796 608 608 531 042 922 162 310 005 045 358 972 079 518 181 244 398 542 890 723 617 583 805 \
 803 284 468 181 333 891 933 909 452 674 390 149 973 739 623 964 766 952 882 739 718 862 250  $q^{8749} +$  \
 1 283 637 364 837 594 666 306 270 898 898 929 031 773 170 728 472 517 717 109 738 121 003 942 362 429 \
 689 814 379 432 482 900 560 611 738 078 880 626 948 665 069 501 696 858 274 276 121 018 942 708 578 \
 009 289 436 395 351 718 142 481 871 511 667 212 577 938 889 385 934 845 574 039 406 628 864  $q^{8752} -$  \
 1 321 439 872 738 050 884 183 373 074 677 230 991 338 817 008 010 609 902 505 642 742 448 715 331 846 \
 755 276 030 539 809 242 484 902 183 149 076 348 795 357 021 385 905 454 230 963 363 107 102 499 738 \
 732 576 433 521 878 360 772 001 973 082 207 066 322 220 859 935 274 600 978 016 145 801 216  $q^{8753} +$  \
 1 441 644 786 530 297 279 062 233 116 710 979 541 532 193 662 860 934 970 805 840 442 557 536 761 907 \
 973 021 555 019 988 187 421 483 539 936 670 393 028 676 937 328 954 664 885 580 795 864 195 500 147 \
 688 217 982 039 338 227 002 633 868 318 861 976 662 681 419 983 816 157 269 199 060 480 000  $q^{8756} -$  \
 1 484 090 717 503 890 250 761 180 325 904 064 534 364 320 046 629 280 479 755 371 165 293 609 451 851 \
 542 202 605 733 093 243 242 682 646 736 284 086 946 133 213 535 579 964 488 774 061 609 762 222 106

728 605 282 992 982 540 343 162 679 862 394 267 822 466 895 643 045 197 542 292 762 883 689  $q^{8757} +$   
 1 619 059 053 357 538 221 560 091 526 222 181 287 740 083 137 832 250 456 793 139 643 953 649 850 009  $q^{8758} -$   
 400 879 374 341 000 716 148 419 740 173 932 193 331 872 951 240 398 917 117 048 951 435 806 548 534  $q^{8759} +$   
 063 583 091 149 871 881 983 861 471 790 298 727 276 719 204 276 514 330 819 689 920 460 800  $q^{8760} -$   
 1 666 717 520 352 846 443 214 453 070 757 686 386 663 614 443 780 915 021 103 468 100 235 591 932 421  $q^{8761} +$   
 836 657 612 511 619 951 740 556 654 578 460 462 930 289 897 557 937 524 068 379 132 859 529 071 332  $q^{8762} -$   
 279 024 114 457 287 304 856 745 396 957 555 418 889 391 993 854 609 406 210 799 783 936 000  $q^{8763} +$   
 1 818 258 511 447 242 524 258 265 171 004 085 606 475 310 211 696 734 845 151 533 506 985 289 347 463  $q^{8764} -$   
 570 673 166 523 441 273 098 893 582 478 053 313 961 833 340 077 832 596 803 819 871 741 094 535 782  $q^{8765} +$   
 208 906 135 310 367 152 920 508 982 967 632 351 896 432 326 211 979 657 218 527 290 368 000  $q^{8766} -$   
 1 871 768 226 188 363 265 405 216 113 801 955 883 590 797 345 247 172 172 728 229 769 520 057 674 191  $q^{8767} +$   
 349 143 677 681 116 325 203 818 382 219 625 697 117 797 999 521 077 381 664 027 534 644 765 136 639  $q^{8768} -$   
 049 845 505 435 234 835 541 580 568 376 784 964 939 899 071 334 494 448 524 473 857 132 050  $q^{8769} +$   
 2 041 912 336 251 142 227 650 872 779 036 845 591 793 949 765 202 446 651 043 178 285 815 217 975 079  $q^{8770} -$   
 534 988 576 345 540 773 817 259 538 642 599 998 791 717 344 166 524 214 398 904 417 750 607 546 052  $q^{8771} +$   
 176 176 845 397 656 634 471 628 745 276 642 181 645 522 665 349 164 767 814 808 479 203 328  $q^{8772} -$   
 2 101 990 101 981 138 482 607 068 579 084 185 816 457 275 471 321 364 197 119 977 347 412 850 203 492  $q^{8773} +$   
 428 548 188 967 341 442 497 404 794 746 707 519 829 165 036 852 901 535 894 123 526 848 599 019 689  $q^{8774} -$   
 986 540 354 201 178 472 196 267 563 267 277 635 528 888 252 039 054 272 953 965 633 536 000  $q^{8775} +$   
 2 293 016 017 535 591 688 648 250 993 878 674 879 210 555 195 187 035 680 463 319 338 008 936 442 439  $q^{8776} -$   
 090 662 143 076 183 200 613 177 321 433 205 938 305 808 111 921 479 226 909 055 170 476 273 367 428  $q^{8777} +$   
 611 019 081 211 133 264 147 349 920 879 781 104 825 026 406 793 273 246 530 409 181 970 432  $q^{8778} -$   
 2 360 466 255 801 611 461 668 698 117 210 718 877 048 886 697 840 148 207 289 898 524 991 158 220 253  $q^{8779} +$   
 335 092 336 786 668 890 624 679 417 282 401 178 075 270 312 511 279 752 354 961 165 552 822 541 151  $q^{8780} -$   
 732 912 456 697 174 711 417 589 601 330 082 824 548 817 694 762 861 566 749 128 916 455 079  $q^{8781} +$   
 2 574 931 164 483 589 994 849 572 040 210 665 974 109 942 941 375 401 051 943 095 605 953 684 712 412  $q^{8782} -$   
 097 608 051 475 778 170 207 013 276 051 318 978 830 178 228 349 262 118 106 386 833 577 716 771 239  $q^{8783} +$   
 632 706 351 177 378 090 734 459 563 370 425 000 753 916 309 928 602 693 118 728 953 600 000  $q^{8784} -$   
 2 650 656 601 587 498 916 672 561 401 843 882 986 011 626 589 256 564 683 444 043 543 951 092 072 103  $q^{8785} +$   
 718 722 768 618 131 672 003 532 822 615 872 000 262 447 542 057 329 121 624 675 600 929 712 641 000  $q^{8786} -$   
 336 600 850 275 644 096 369 349 807 311 158 861 322 751 805 756 784 180 508 421 203 197 952  $q^{8787} +$   
 2 891 430 155 702 469 494 634 695 767 283 549 993 181 651 589 266 579 838 345 978 200 720 306 703 118  $q^{8788} -$   
 552 950 213 967 603 735 322 335 789 555 853 162 830 045 937 687 237 898 383 266 755 717 607 714 532  $q^{8789} +$   
 237 865 121 653 512 558 791 289 578 571 697 165 212 812 528 471 622 558 802 117 914 624 000  $q^{8790} -$   
 2 976 443 809 669 103 527 172 241 449 281 802 639 653 474 673 566 583 536 504 571 869 472 631 366 121  $q^{8791} +$   
 185 086 519 918 732 833 734 619 855 345 822 241 667 777 835 701 994 731 045 663 397 841 626 317 750  $q^{8792} -$   
 077 077 464 164 202 824 704 594 870 828 871 103 562 485 458 354 588 101 345 485 492 141 875  $q^{8793} +$   
 3 246 746 222 542 091 372 674 098 910 810 048 444 624 872 488 917 943 213 508 625 609 581 366 130 303  $q^{8794} -$   
 000 546 779 594 171 839 069 453 264 498 037 395 137 494 398 002 876 690 561 038 221 577 895 434 074  $q^{8795} +$   
 496 357 836 309 568 203 862 759 435 630 744 850 478 081 565 449 172 797 749 590 435 840 000  $q^{8796} -$   
 3 342 184 848 527 433 914 894 946 630 021 680 263 529 216 147 516 088 872 234 927 030 692 019 809 899  $q^{8797} +$   
 050 093 877 647 801 457 997 495 849 608 351 195 306 940 787 708 331 604 289 331 891 166 220 603 380  $q^{8798} -$   
 640 398 896 001 541 244 015 426 394 841 318 709 617 627 339 765 439 907 730 799 412 838 400  $q^{8799} +$   
 3 645 629 625 432 051 820 863 709 737 475 125 364 498 171 701 643 975 224 972 071 019 055 336 201 462  $q^{8800} -$   
 567 551 884 749 837 854 566 950 218 460 763 274 942 518 319 207 899 056 351 536 315 564 884 677 605  $q^{8801} +$   
 222 315 464 903 043 979 931 271 618 557 710 989 403 551 120 565 640 617 094 578 568 048 640  $q^{8802} -$   
 3 752 768 796 628 070 042 807 327 656 323 942 803 006 927 391 609 618 875 223 185 412 647 092 874 631  $q^{8803} +$   
 237 752 179 281 376 232 269 075 222 245 725 959 198 230 514 293 743 412 501 450 577 209 665 819 031  $q^{8804} -$   
 110 590 493 676 606 822 664 897 298 852 138 405 978 192 187 901 431 044 893 642 580 268 750  $q^{8805} +$   
 4 093 410 662 871 756 797 985 054 221 900 672 791 374 405 801 104 176 702 897 245 908 689 425 074 971  $q^{8806} -$   
 211 375 734 698 201 777 683 639 048 827 151 982 054 575 620 113 209 202 107 884 861 641 609 290 020  $q^{8807} +$   
 159 344 968 510 659 581 194 827 265 918 636 545 393 348 536 464 801 059 014 669 720 861 696  $q^{8808} -$   
 4 213 681 685 412 367 093 409 739 689 192 048 788 603 921 573 955 555 841 216 459 384 477 679 693 870  $q^{8809} +$   
 620 888 702 494 551 736 882 198 457 037 464 859 956 083 903 880 071 336 547 779 705 255 931 850 233  $q^{8810} -$   
 979 783 687 514 272 512 115 122 904 256 584 615 954 246 874 594 956 807 458 951 813 365 760  $q^{8811} +$

4 596 070 342 294 473 770 684 485 622 746 885 645 030 118 257 641 417 940 829 546 508 461 487 065 864 \
 442 602 543 370 458 735 416 060 098 712 757 538 911 267 533 294 696 666 733 372 110 935 850 757 502 \
 770 292 807 483 864 165 843 723 360 640 026 071 983 288 131 161 199 256 117 655 071 488 000  $q^{8796}$  -

4 731 079 226 707 204 587 533 279 112 662 369 575 591 470 381 743 781 840 184 404 504 000 899 197 455 \
 081 805 884 533 916 325 434 518 734 309 192 193 341 977 604 629 457 588 634 922 293 170 853 032 883 \
 495 272 716 120 077 368 857 242 208 620 710 798 808 844 666 181 653 267 637 387 648 162 026  $q^{8797}$  +

5 160 319 642 441 044 146 352 647 262 756 771 679 154 170 364 194 565 322 477 719 206 655 685 116 178 \
 790 924 460 179 799 476 535 822 564 577 102 116 683 549 882 998 221 434 012 384 671 130 049 609 594 \
 745 379 577 778 671 613 476 866 812 431 049 170 228 541 233 539 244 158 417 214 997 196 800  $q^{8800}$  -

5 311 868 381 134 074 452 762 220 207 348 254 969 545 426 426 681 266 937 708 168 976 283 297 686 660 \
 746 708 609 798 525 714 133 674 667 578 083 870 112 104 821 279 125 291 348 922 913 486 888 205 619 \
 742 791 073 434 721 115 838 021 083 781 321 743 226 584 611 474 798 740 840 849 203 200 000  $q^{8801}$  +

5 793 688 409 426 536 238 154 075 195 434 429 522 802 391 248 037 049 521 217 558 355 417 289 837 079 \
 642 100 001 898 673 799 920 490 082 240 475 445 992 336 476 177 456 739 491 065 723 093 710 478 168 \
 846 360 395 632 166 694 578 092 798 931 650 120 196 136 396 980 688 160 571 717 746 688 000  $q^{8804}$  -

5 963 798 839 901 181 623 758 280 080 573 367 727 366 246 677 687 744 366 995 386 150 477 832 564 867 \
 982 439 409 451 946 182 761 011 368 198 907 046 002 485 047 903 442 299 158 782 362 599 541 901 848 \
 057 341 492 529 602 185 844 970 727 991 318 328 551 623 321 636 999 838 561 091 252 287 750  $q^{8805}$  +

6 504 625 054 826 543 373 786 078 435 736 416 433 464 712 814 393 180 934 624 665 310 852 924 824 405 \
 987 444 879 611 925 174 277 370 162 112 500 891 324 616 199 976 018 504 729 313 285 805 658 018 311 \
 330 963 469 964 611 692 236 022 968 432 352 339 433 626 299 009 040 962 158 828 567 444 480  $q^{8808}$  -

6 695 565 622 153 352 854 518 809 997 304 583 250 030 131 760 519 731 313 777 530 295 320 704 793 691 \
 186 325 189 368 779 478 968 663 714 348 345 687 010 166 134 269 652 134 299 181 444 276 542 691 897 \
 935 360 057 091 499 744 142 182 035 063 898 189 324 947 160 148 554 498 988 577 193 984 000  $q^{8809}$  +

7 302 608 365 487 868 469 982 710 299 034 195 030 682 157 122 902 474 402 327 539 956 349 464 300 889 \
 174 845 256 341 838 218 439 243 639 581 660 921 521 650 217 078 837 616 547 281 915 639 131 578 421 \
 493 024 922 894 827 837 315 566 468 416 118 436 820 788 595 264 231 114 384 733 541 140 992  $q^{8812}$  -

7 516 924 135 519 897 463 983 030 713 812 912 922 955 517 496 452 630 277 664 307 734 566 877 311 869 \
 032 083 390 977 610 598 967 514 834 272 788 273 161 483 157 873 750 197 038 057 021 426 322 817 996 \
 039 628 203 227 559 502 275 789 618 295 681 568 786 059 564 911 033 757 692 752 300 364 263  $q^{8813}$  +

8 198 272 893 216 867 211 499 526 617 557 444 187 925 836 127 348 461 215 458 336 522 498 022 559 575 \
 679 705 853 943 969 647 325 191 733 450 241 321 420 558 546 032 251 719 768 634 422 819 669 380 604 \
 160 244 590 166 667 449 777 166 661 106 894 963 525 590 904 700 503 538 422 312 556 544 000  $q^{8816}$  -

8 438 819 210 528 885 242 939 495 727 811 368 076 339 723 632 459 428 415 513 040 629 769 780 384 541 \
 836 253 277 299 029 626 645 181 170 701 337 995 405 213 919 833 048 729 035 959 925 570 588 855 744 \
 424 815 131 341 830 958 008 159 398 085 156 114 031 662 082 027 655 027 951 071 473 598 464  $q^{8817}$  +

9 203 549 570 074 381 349 216 562 457 780 259 169 276 030 927 662 716 710 004 540 722 374 808 209 949 \
 398 860 628 325 038 777 632 793 691 175 362 240 475 788 497 650 860 337 450 426 687 645 964 967 681 \
 903 655 425 856 359 298 749 142 613 656 820 929 554 443 526 749 017 209 041 928 183 736 320  $q^{8820}$  -

9 473 529 802 263 444 870 065 545 561 870 613 402 200 647 652 147 764 340 935 895 786 894 004 464 327 \
 230 901 056 026 005 838 858 196 069 210 099 004 152 238 522 584 380 857 490 250 124 396 508 827 658 \
 041 019 255 562 198 073 957 337 119 578 058 808 838 535 468 475 422 802 950 492 341 940 125  $q^{8821}$  +

10 331 823 394 012 854 099 047 699 032 056 482 493 657 041 966 209 685 569 124 844 170 644 553 809 \
 339 996 779 202 666 827 452 868 928 930 899 595 500 859 945 249 453 990 733 397 487 759 389 605 188 \
 632 719 891 829 423 278 545 177 840 112 421 934 133 140 890 247 984 066 714 822 399 064 064 000 \
  $q^{8824}$  -

10 634 831 257 391 824 959 802 129 498 625 117 671 954 403 000 715 050 205 399 164 462 898 495 222 \
 768 513 180 977 676 709 645 330 504 606 473 336 029 319 769 758 742 549 255 105 921 279 939 248 478 \
 512 395 491 130 779 694 485 911 943 672 194 495 545 142 417 443 108 546 987 451 605 650 636 800 \
  $q^{8825}$  +

11 598 110 252 609 648 383 449 434 675 252 825 197 546 302 010 945 650 729 997 829 826 963 641 244 \
 162 892 592 184 389 892 592 680 670 864 469 971 889 568 575 597 160 073 595 415 158 812 993 575 347 \
 036 001 226 383 623 900 049 817 763 543 796 652 265 706 583 196 544 534 071 767 125 101 961 216 \
  $q^{8828}$  -

11 938 177 274 163 131 025 011 527 316 959 921 719 192 766 043 262 157 187 408 815 824 352 260 179 \

458 753 778 871 080 054 669 206 828 254 580 338 687 312 080 901 639 699 674 730 678 137 657 040 468 \\  
 390 442 626 292 269 767 761 723 936 019 900 819 210 280 441 834 884 297 127 191 722 363 910 250  
 $q^{8829} +$   
 13 019 255 202 571 653 737 740 172 952 653 600 952 675 123 686 183 853 837 669 285 125 576 863 539 \\  
 887 489 818 366 881 688 418 163 287 216 421 034 015 850 341 581 387 033 203 715 172 228 394 333 209 \\  
 131 318 670 981 811 710 126 758 286 278 454 704 788 341 155 573 736 857 468 351 798 631 858 176  
 $q^{8832} -$   
 13 400 903 940 098 892 508 256 321 315 712 608 393 877 706 467 733 771 753 699 896 989 170 849 863 \\  
 475 759 770 490 360 052 160 873 185 016 671 381 147 216 294 228 702 919 798 747 565 696 773 664 076 \\  
 633 526 907 350 171 211 675 787 603 237 503 550 683 360 256 789 457 763 420 674 955 625 201 664  
 $q^{8833} +$   
 14 614 154 802 748 117 590 295 294 252 812 558 437 314 544 575 483 121 628 078 490 526 575 116 409 \\  
 225 204 266 682 971 631 903 765 999 054 952 572 046 905 103 218 465 744 890 097 686 573 763 847 534 \\  
 885 988 873 665 800 271 065 382 579 557 692 804 862 382 909 815 018 043 259 020 980 248 602 752  
 $q^{8836} -$   
 15 042 458 520 258 212 569 828 065 675 111 527 956 305 151 897 869 705 377 720 070 191 909 503 551 \\  
 297 531 934 769 087 396 692 214 556 194 887 194 565 495 860 517 062 715 023 617 032 377 691 274 527 \\  
 823 779 805 765 822 754 758 875 872 076 769 501 269 108 481 165 855 703 984 705 123 473 143 338  
 $q^{8837} +$   
 16 404 006 412 218 327 805 028 923 806 379 974 831 781 486 871 404 804 897 462 550 429 630 851 677 \\  
 456 240 539 260 432 679 863 253 427 969 424 491 216 057 275 643 212 144 930 139 656 264 994 458 170 \\  
 039 704 147 117 877 225 275 304 526 322 440 269 815 777 231 825 177 594 912 095 886 411 110 400  
 $q^{8840} -$   
 16 884 655 991 842 568 228 045 499 605 825 059 426 373 847 679 902 782 568 469 965 279 149 380 198 \\  
 763 286 675 661 720 508 886 224 078 975 579 300 327 478 549 838 654 544 739 886 801 909 135 593 789 \\  
 555 256 819 884 002 275 231 386 399 611 701 940 049 527 105 256 657 045 064 325 649 727 488 000  
 $q^{8841} +$   
 18 412 587 716 680 876 733 007 068 297 356 631 549 306 510 338 436 886 984 137 128 782 694 182 988 \\  
 864 191 478 834 171 309 652 603 617 751 638 805 385 182 087 879 147 733 396 792 525 417 309 038 856 \\  
 943 334 872 058 807 950 086 778 812 639 517 986 445 851 939 425 058 765 363 217 624 553 984 000  
 $q^{8844} -$   
 18 951 966 682 714 730 523 723 309 315 638 703 932 596 383 455 512 520 067 242 117 165 104 718 933 \\  
 947 159 327 007 653 000 307 741 290 547 985 466 968 924 342 950 529 202 269 440 016 744 219 603 757 \\  
 861 924 967 571 532 255 870 516 090 025 774 148 080 243 410 032 876 317 888 020 511 333 787 525  
 $q^{8845} +$   
 20 666 570 140 412 017 298 586 654 438 071 621 347 294 608 459 624 701 432 740 252 076 797 118 426 \\  
 091 647 522 505 218 146 936 495 615 315 304 675 067 356 191 263 517 553 824 932 246 795 148 975 998 \\  
 789 336 181 704 745 066 914 673 124 959 814 651 235 968 024 381 773 455 524 073 367 473 487 872  
 $q^{8848} -$   
 21 271 838 776 815 820 182 634 894 059 830 705 017 682 539 390 829 213 323 504 467 459 100 136 512 \\  
 506 616 415 083 323 275 817 851 773 138 524 702 686 746 489 386 569 870 685 866 307 659 539 094 883 \\  
 199 947 090 543 193 942 309 498 423 145 501 532 507 088 675 011 936 161 263 772 663 009 280 000  
 $q^{8849} +$   
 23 195 870 242 578 454 898 544 779 559 722 167 009 214 866 234 791 039 774 436 809 703 299 334 547 \\  
 212 926 738 203 419 955 646 666 750 455 614 725 045 603 117 987 909 017 911 797 173 552 196 529 573 \\  
 311 598 066 469 909 878 959 663 358 982 752 209 754 862 565 995 698 087 021 476 590 442 694 656  
 $q^{8852} -$   
 23 875 059 903 718 036 032 113 375 316 173 893 002 373 874 496 183 716 975 464 342 376 813 962 461 \\  
 327 708 615 632 066 470 006 461 634 181 989 462 005 067 220 728 328 517 345 591 106 511 560 902 129 \\  
 176 557 978 083 722 964 328 533 797 568 239 449 549 654 563 456 962 350 173 741 281 281 078 624  
 $q^{8853} +$   
 26 034 043 691 392 692 069 456 948 200 275 416 909 071 068 809 987 938 676 598 615 202 639 209 861 \\  
 571 845 456 277 733 671 388 026 928 654 453 186 830 829 785 677 210 751 688 222 381 340 013 301 513 \\  
 694 510 647 767 704 035 639 072 240 379 852 231 727 889 067 833 163 309 459 940 965 737 984 000  
 $q^{8856} -$

26 796 162 538 519 970 681 482 386 897 345 673 112 830 445 083 260 370 419 481 362 871 378 062 062 \\  
 309 926 149 152 043 822 079 483 633 765 304 145 593 805 677 038 207 602 803 717 154 499 306 661 908 \\  
 116 843 187 426 507 525 743 582 918 375 344 597 519 972 080 367 189 078 182 785 766 467 895 296 \\  
 $q^{8857} +$   
 29 218 726 963 879 368 214 547 030 186 808 019 599 473 597 982 112 074 844 283 393 588 168 495 301 \\  
 060 539 699 143 907 226 694 105 675 744 406 383 684 052 090 029 223 951 915 692 813 874 378 324 797 \\  
 244 042 171 852 366 967 319 668 969 788 271 337 121 258 785 105 702 214 174 888 255 761 766 400 \\  
 $q^{8860} -$   
 30 073 878 508 552 896 992 628 166 346 303 043 867 417 483 207 866 563 127 738 737 763 879 600 466 \\  
 737 937 414 576 440 715 736 304 206 698 071 378 516 987 189 705 279 781 040 276 312 108 442 706 980 \\  
 717 883 472 666 323 053 135 700 846 772 443 715 283 566 786 105 471 663 042 898 997 678 279 375 \\  
 $q^{8861} +$   
 32 792 132 540 038 212 676 354 573 357 965 574 625 649 031 542 350 731 539 860 975 986 778 059 286 \\  
 456 421 927 927 889 159 489 624 562 828 186 393 644 867 674 154 394 460 878 461 821 462 916 467 822 \\  
 012 839 714 454 973 055 384 753 655 839 211 867 985 100 519 792 963 003 275 013 283 755 520 000 \\  
 $q^{8864} -$   
 33 751 648 542 284 868 667 792 129 013 920 479 750 482 702 907 447 182 175 788 406 498 903 656 909 \\  
 385 928 031 634 488 703 494 858 087 238 204 618 904 598 884 060 575 711 621 405 249 870 934 138 984 \\  
 798 298 856 585 269 188 329 706 434 570 332 613 210 972 112 823 219 671 397 494 133 366 784 000 \\  
 $q^{8865} +$   
 36 801 604 055 960 991 057 540 411 933 889 495 687 766 212 034 831 652 466 682 529 685 188 470 201 \\  
 056 402 113 459 383 766 674 904 140 661 669 663 506 262 949 043 060 468 406 589 567 298 727 825 161 \\  
 847 978 283 289 111 648 604 973 001 595 847 491 296 666 953 328 143 706 873 049 581 342 343 168 \\  
 $q^{8868} -$   
 37 878 193 511 632 865 252 322 394 977 218 719 728 604 809 448 605 175 047 274 101 062 289 896 388 \\  
 141 483 226 285 332 661 995 334 411 146 076 103 465 304 721 519 650 837 361 115 017 740 703 624 021 \\  
 694 571 299 578 565 050 474 140 285 183 657 704 845 975 829 019 523 800 890 316 781 346 106 750 \\  
 $q^{8869} +$   
 41 300 238 659 965 049 415 355 734 334 891 774 205 972 472 039 294 236 548 644 878 719 404 529 939 \\  
 987 952 901 022 349 822 486 735 564 619 703 893 827 834 446 363 280 162 767 602 979 938 483 364 362 \\  
 986 925 853 780 233 084 431 963 222 058 196 214 585 721 329 040 252 615 557 873 798 694 471 168 \\  
 $q^{8872} -$   
 42 508 154 820 858 142 969 473 955 426 894 406 675 870 744 669 781 663 434 754 523 731 225 834 631 \\  
 000 598 142 438 793 837 216 633 077 905 625 835 160 128 144 852 168 233 228 954 117 078 843 387 073 \\  
 346 752 356 020 802 410 920 956 515 378 659 931 346 562 171 740 134 737 809 957 558 102 884 352 \\  
 $q^{8873} +$   
 46 347 584 689 099 736 106 190 616 588 517 077 277 495 592 742 026 611 595 189 098 337 302 789 156 \\  
 979 542 614 404 135 352 942 106 129 383 256 577 975 050 727 559 788 707 691 812 322 551 263 331 329 \\  
 587 349 064 639 285 792 577 715 124 862 641 339 739 095 795 635 845 421 818 552 092 049 920 000 \\  
 $q^{8876} -$   
 47 702 812 293 669 980 029 297 479 966 337 840 918 916 605 743 198 026 362 807 703 479 647 093 537 \\  
 634 186 264 139 487 723 611 595 475 496 315 114 666 033 491 215 240 167 927 814 216 728 108 561 561 \\  
 586 836 314 665 169 815 615 956 506 146 738 688 126 381 050 016 419 572 358 176 547 774 871 683 \\  
 $q^{8877} +$   
 52 010 423 761 723 892 921 511 359 274 243 874 820 807 216 758 390 316 555 685 531 802 808 162 213 \\  
 491 015 141 090 088 333 238 242 756 289 570 860 056 116 655 745 630 930 302 575 562 048 701 797 405 \\  
 884 049 496 426 590 836 569 714 930 592 478 842 127 325 735 469 206 134 882 722 178 437 529 600 \\  
 $q^{8880} -$   
 53 530 888 916 680 983 031 419 837 339 929 843 324 549 892 122 082 430 956 565 061 875 751 864 477 \\  
 668 069 927 649 091 463 262 149 761 747 133 993 783 144 316 698 353 480 420 544 786 512 133 691 025 \\  
 720 943 084 557 403 049 609 428 740 715 017 296 115 314 139 077 920 364 790 527 976 517 632 000 \\  
 $q^{8881} +$   
 58 363 647 477 851 386 123 805 732 427 595 459 955 758 944 587 574 825 142 157 037 995 351 833 517 \\  
 486 064 833 853 980 437 927 081 112 764 558 854 325 618 590 991 483 500 465 140 946 725 976 773 742 \\  
 159 959 515 298 789 800 768 370 040 056 580 540 034 120 197 359 135 169 295 739 680 062 720 000

$q^{8884} -$   
60 069 452 924 913 368 899 213 545 183 545 105 998 213 617 314 050 275 419 195 561 611 147 429 506 \ \backslash  
449 497 836 479 733 151 941 269 110 246 414 302 416 446 640 281 838 829 550 621 806 756 577 162 210 \ \backslash  
778 917 449 464 631 832 647 225 599 973 562 715 511 084 223 707 322 890 460 012 878 743 995 500  
 $q^{8885} +$   
65 491 240 146 735 998 070 368 415 339 791 941 689 551 644 813 102 766 532 034 922 813 553 601 304 \ \backslash  
258 406 108 220 533 544 785 513 329 411 284 030 983 246 071 492 995 871 614 924 883 204 804 090 222 \ \backslash  
576 794 752 103 051 785 407 417 993 195 677 366 472 576 428 350 399 617 151 000 728 227 083 264  
 $q^{8888} -$   
67 404 928 978 173 774 178 489 932 387 428 587 593 833 006 030 516 263 454 724 262 217 765 752 922 \ \backslash  
142 099 669 547 953 027 975 658 433 774 174 423 200 466 324 314 618 303 985 344 778 674 952 464 579 \ \backslash  
136 805 026 972 040 659 515 166 182 254 447 511 955 363 658 734 769 326 052 971 098 476 544 000  
 $q^{8889} +$   
73 487 380 336 526 158 437 371 263 079 236 941 807 948 907 192 978 123 197 907 908 656 901 879 201 \ \backslash  
730 897 091 389 391 654 356 085 754 474 618 134 522 897 474 820 717 189 894 981 473 294 480 433 085 \ \backslash  
321 753 072 056 350 473 159 383 661 691 653 879 044 812 071 800 286 602 454 872 053 974 087 680  
 $q^{8892} -$   
75 634 231 592 056 705 386 094 807 142 944 427 111 566 383 728 752 053 081 572 654 091 893 308 027 \ \backslash  
460 093 169 771 603 578 579 778 078 629 144 261 262 958 602 133 090 791 428 015 110 002 348 280 982 \ \backslash  
741 078 414 554 619 032 158 101 587 106 796 285 990 745 547 917 293 677 454 402 920 565 029 880  
 $q^{8893} +$   
82 457 675 581 465 708 946 462 424 743 142 497 045 852 622 473 873 669 908 701 613 928 258 671 354 \ \backslash  
401 871 658 971 705 456 663 885 035 722 084 635 755 550 155 125 048 219 227 850 241 156 437 528 669 \ \backslash  
194 284 272 753 733 650 169 250 182 720 469 102 585 251 297 927 455 307 893 359 131 881 472 000  
 $q^{8896} -$   
84 866 035 572 312 926 882 399 144 366 960 675 128 634 760 095 176 916 631 695 662 256 242 373 469 \ \backslash  
248 855 510 685 670 598 480 320 210 700 960 713 117 613 454 531 630 629 096 993 576 566 271 477 733 \ \backslash  
225 533 091 809 287 997 010 014 745 640 355 485 564 900 004 423 694 456 356 995 461 831 720 960  
 $q^{8897} +$   
92 520 546 307 869 483 425 676 915 137 410 867 408 605 390 675 194 810 641 824 178 558 740 626 231 \ \backslash  
982 315 746 866 627 481 200 072 290 632 283 600 351 756 952 559 091 551 376 257 538 549 087 262 513 \ \backslash  
398 334 434 267 685 111 064 379 778 670 270 991 427 542 141 864 607 472 126 160 747 101 798 400  
 $q^{8900} -$   
95 222 199 976 717 256 158 559 640 003 403 990 226 282 087 675 149 261 379 409 574 938 427 354 402 \ \backslash  
720 602 444 787 152 339 619 538 286 527 449 737 559 923 182 960 581 368 557 234 137 509 637 366 458 \ \backslash  
178 544 759 608 497 455 976 978 221 654 818 603 790 740 831 569 150 264 796 092 951 184 693 875  
 $q^{8901} +$   
103 808 776 973 153 830 830 903 753 607 155 626 839 969 491 960 242 616 902 588 114 143 391 479 055 \ \backslash  
995 532 756 146 060 696 174 021 383 600 578 299 532 146 166 039 353 229 083 425 978 222 017 932 158 \ \backslash  
294 552 036 776 385 008 032 851 366 572 564 725 512 927 780 572 403 227 629 058 176 698 624 000  
 $q^{8904} -$   
106 839 364 117 218 165 923 441 811 649 670 548 449 791 403 329 461 947 181 074 388 057 584 443 640 \ \backslash  
205 864 113 200 186 863 952 832 323 617 669 167 812 853 373 593 386 360 376 543 290 811 664 864 312 \ \backslash  
245 340 867 505 167 590 602 688 725 460 875 537 893 703 045 467 984 908 138 853 053 048 422 400  
 $q^{8905} +$   
116 471 254 577 398 913 418 606 105 788 680 573 824 142 997 505 152 492 601 980 168 397 505 388 070 \ \backslash  
914 753 874 866 746 247 322 238 050 758 061 867 067 689 726 710 437 752 732 804 870 577 214 202 972 \ \backslash  
581 978 443 601 318 803 304 542 670 380 087 752 882 905 082 177 452 816 562 295 540 740 713 472  
 $q^{8908} -$   
119 870 736 342 607 668 047 749 760 603 941 306 707 899 815 988 489 612 341 926 680 538 340 095 341 \ \backslash  
385 883 764 385 795 380 593 261 671 044 485 027 632 921 056 346 356 501 828 007 485 726 822 109 246 \ \backslash  
031 605 400 879 767 169 652 444 151 204 102 352 329 948 920 068 186 717 223 059 629 899 401 250  
 $q^{8909} +$   
130 674 917 132 079 872 400 364 067 065 763 838 466 775 585 756 633 662 274 197 548 389 002 701 800 \ \backslash  
093 375 718 738 060 225 095 673 416 152 712 429 221 029 786 349 982 884 702 118 010 856 122 919 039 \ \backslash

882 215 965 473 344 952 557 732 416 831 952 570 012 462 702 064 230 842 520 415 724 329 943 040  
 $q^{8912} -$   
 134 488 098 836 829 112 733 201 398 444 890 351 837 625 264 287 376 834 270 578 939 179 809 932 620  
 897 137 236 860 927 556 679 667 992 711 995 535 742 540 104 153 305 911 317 265 197 928 979 214 445  
 341 532 191 553 968 473 033 838 615 477 467 636 021 788 313 590 169 749 214 167 761 372 348 416  
 $q^{8913} +$   
 146 606 937 386 872 183 578 249 415 813 713 359 246 993 361 149 686 076 383 921 089 951 633 715 152  
 541 806 996 980 522 639 718 564 929 188 665 486 520 170 374 951 107 444 266 910 430 594 356 530 832  
 865 936 490 111 817 211 374 318 276 785 482 381 573 297 457 379 439 486 662 665 301 032 960 000  
 $q^{8916} -$   
 150 884 054 462 378 998 353 678 347 841 412 846 435 924 650 708 841 763 800 536 363 257 679 097 363  
 675 119 881 195 417 746 149 450 079 545 219 200 079 440 551 196 748 468 147 846 506 148 905 021 868  
 462 890 334 735 905 217 102 181 858 328 340 054 171 634 247 340 692 007 427 841 639 139 736 377  
 $q^{8917} +$   
 164 477 170 157 680 206 891 285 271 582 469 833 570 899 884 175 869 284 993 508 748 418 310 143 329  
 119 167 070 226 458 143 155 416 679 432 614 673 859 739 988 379 639 689 795 787 786 293 131 371 714  
 823 746 528 086 292 169 476 603 060 276 749 539 140 601 264 409 669 890 970 587 732 839 910 400  
 $q^{8920} -$   
 169 274 544 807 922 326 904 581 452 465 280 571 657 986 930 459 727 417 096 101 654 122 296 481 562  
 034 613 323 983 776 620 158 544 608 290 534 840 187 319 789 463 649 667 653 530 745 907 758 244 038  
 070 327 840 087 869 495 317 076 594 905 721 619 855 009 458 856 678 747 796 860 808 663 040 000  
 $q^{8921} +$   
 184 520 895 006 291 708 407 745 199 624 791 741 586 258 954 616 423 539 556 747 924 481 629 264 200  
 815 029 199 699 288 988 949 888 983 105 032 091 913 517 994 071 755 971 289 842 421 066 477 765 163  
 382 233 086 630 573 286 216 196 947 798 102 254 343 304 392 731 249 578 966 023 900 925 440 000  
 $q^{8924} -$   
 189 901 672 104 381 340 322 568 441 055 148 439 375 329 263 133 829 172 911 159 924 364 345 592 476  
 074 121 432 329 800 857 144 724 871 706 460 026 947 433 541 663 658 289 334 952 575 397 111 518 614  
 453 845 593 724 718 026 313 772 580 803 357 082 942 222 548 307 722 267 680 294 186 369 202 700  
 $q^{8925} +$   
 207 001 889 838 023 754 552 645 135 800 466 474 960 402 190 350 877 271 025 071 099 934 995 838 293  
 397 929 913 230 455 810 652 386 199 330 418 057 959 782 192 691 818 776 577 212 401 261 202 075 531  
 032 316 390 251 956 435 967 168 603 124 659 038 695 394 002 995 936 655 998 485 288 805 154 816  
 $q^{8928} -$   
 213 036 861 599 323 845 657 919 305 215 758 370 837 001 950 782 522 529 791 324 193 925 218 424 791  
 851 868 852 770 449 324 593 855 381 835 902 197 989 764 304 725 701 903 378 224 382 719 287 309 850  
 587 268 577 939 026 660 411 103 913 274 963 718 070 190 989 982 005 695 333 137 445 908 480 000  
 $q^{8929} +$   
 232 215 875 257 315 796 656 439 251 232 688 854 779 425 678 752 058 365 692 941 367 118 471 820 858  
 931 715 481 443 002 174 582 327 133 785 192 485 958 693 736 670 560 458 417 002 856 241 662 575 055  
 453 741 662 463 374 710 303 483 935 528 914 505 191 237 345 583 227 166 995 367 615 478 956 032  
 $q^{8932} -$   
 238 984 405 375 788 257 021 429 931 754 844 061 229 334 429 114 624 781 232 653 852 912 425 847 452  
 159 300 264 620 549 917 452 370 288 027 957 301 738 597 437 510 977 265 374 441 772 756 729 423 609  
 486 801 901 259 675 908 344 849 965 095 318 504 767 346 279 331 956 603 771 527 326 036 290 335  
 $q^{8933} +$   
 260 494 374 307 205 367 737 504 005 708 720 257 069 811 070 937 598 498 843 324 117 926 070 127 445  
 753 121 874 708 446 368 262 910 686 537 453 104 381 326 301 738 205 360 608 413 096 834 018 614 041  
 974 998 793 149 411 048 081 191 555 599 686 480 512 510 411 422 068 358 547 688 592 137 152 000  
 $q^{8936} -$   
 268 085 433 525 065 660 117 985 607 331 638 319 160 266 419 724 090 488 548 019 050 090 119 368 927  
 793 940 994 970 511 129 748 305 776 540 014 399 612 229 956 450 384 557 352 257 395 134 666 524 305  
 395 536 984 356 449 974 355 760 935 197 411 194 421 168 944 809 354 751 504 618 449 864 359 936  
 $q^{8937} +$   
 292 209 037 578 290 679 632 740 738 569 342 824 295 640 922 723 137 718 889 774 265 452 083 396 830

620 873 293 310 022 468 448 247 924 152 125 507 215 425 533 770 433 917 367 956 471 889 865 645 868  
 988 624 374 238 463 853 111 131 991 667 474 958 952 523 903 411 278 357 622 357 160 128 665 600  
 $q^{8940} -$   
 300 722 364 096 467 673 947 140 696 580 904 269 373 181 512 553 986 666 485 892 701 677 070 512 605  
 697 266 163 965 175 904 518 478 096 744 759 835 104 264 829 196 214 348 974 220 851 009 761 639 141  
 544 611 113 371 731 074 734 106 484 578 557 848 680 428 910 076 664 466 436 648 035 875 847 625  
 $q^{8941} +$   
 327 776 489 674 760 345 180 715 703 717 848 966 655 185 334 609 891 673 167 599 836 889 170 721 877  
 372 170 187 841 753 643 632 142 255 826 197 089 259 393 940 662 041 038 670 279 369 861 887 793 083  
 431 922 200 079 242 835 729 781 087 127 243 794 237 964 551 541 601 893 469 361 332 807 680 000  
 $q^{8944} -$   
 337 323 889 421 322 231 684 876 107 498 833 973 760 259 970 420 574 433 863 250 700 402 196 376 607  
 722 066 138 284 468 666 788 011 109 015 930 074 015 444 984 404 389 800 809 893 611 402 494 612 580  
 103 768 766 540 039 503 967 901 153 100 256 949 225 271 739 361 908 296 903 055 007 545 753 600  
 $q^{8945} +$   
 367 663 759 746 160 655 313 979 040 357 763 056 821 611 794 367 263 745 604 511 776 205 241 696 147  
 016 373 820 476 511 805 769 002 742 498 282 705 144 773 278 226 629 861 329 375 670 338 054 911 953  
 547 933 992 801 981 476 022 013 501 849 944 950 875 828 137 243 803 208 340 478 789 772 834 816  
 $q^{8948} -$   
 378 370 563 322 360 252 886 506 542 870 696 501 595 156 331 119 641 105 428 966 123 041 805 602 888  
 225 302 916 460 099 125 982 057 149 665 267 800 661 517 021 235 120 340 029 371 612 916 612 469 101  
 093 231 360 370 761 828 421 774 551 990 373 127 463 961 762 914 921 267 425 029 050 992 313 625  
 $q^{8949} +$   
 412 394 366 319 747 164 850 891 742 102 833 956 421 167 211 903 129 456 924 680 738 856 239 619 801  
 542 950 203 382 395 045 495 894 400 297 171 994 874 934 348 723 621 647 036 885 273 187 786 371 584  
 476 256 736 725 946 772 883 114 795 322 873 637 068 466 771 585 780 046 329 238 518 403 468 288  
 $q^{8952} -$   
 424 401 061 461 713 220 671 943 127 913 990 850 207 351 354 264 764 189 937 622 759 375 715 924 881  
 547 204 177 857 788 325 320 840 740 793 650 520 038 027 406 143 169 419 920 705 935 362 675 139 048  
 723 435 783 690 634 376 552 736 674 695 927 027 293 007 689 341 625 290 054 959 570 374 426 624  
 $q^{8953} +$   
 462 555 135 095 757 437 725 584 707 523 592 426 460 163 493 251 096 126 341 944 110 847 000 915 301  
 628 672 504 927 999 579 898 696 124 731 290 403 658 051 901 013 941 974 663 706 939 474 814 756 046  
 289 522 078 665 222 307 160 739 361 147 208 445 332 869 504 910 029 932 049 418 052 588 544 000  
 $q^{8956} -$   
 476 019 195 749 911 874 989 825 354 229 339 602 124 248 503 136 578 052 814 242 927 607 563 097 659  
 835 158 607 592 608 421 045 883 472 126 334 277 806 605 222 741 640 556 127 548 177 462 301 201 139  
 444 115 009 021 209 466 415 084 206 560 446 583 859 739 651 112 689 660 779 218 085 872 792 633  
 $q^{8957} +$   
 518 803 837 804 449 913 930 293 126 699 603 955 027 789 160 932 896 596 658 217 313 813 423 080 753  
 640 908 376 444 570 755 533 674 121 723 964 766 648 257 452 065 592 224 226 608 798 204 951 907 099  
 878 574 232 432 293 516 063 660 940 864 753 069 688 434 876 343 643 894 456 025 977 913 344 000  
 $q^{8960} -$   
 533 901 773 445 340 351 449 145 299 499 637 027 720 926 062 693 115 815 165 029 762 994 730 990 403  
 489 670 907 711 383 641 272 424 191 800 970 135 372 587 696 034 976 781 965 008 134 786 760 813 345  
 012 104 735 423 274 097 164 800 486 417 372 375 307 232 289 828 988 695 721 132 532 891 648 000  
 $q^{8961} +$   
 581 877 750 789 826 597 224 545 753 260 738 572 873 871 503 463 024 337 720 689 450 888 692 587 342  
 208 220 186 198 027 571 096 246 531 964 647 262 163 552 338 604 292 444 505 436 189 646 445 826 805  
 897 233 543 734 965 103 017 178 355 125 856 337 309 547 151 549 668 062 524 508 092 243 968 000  
 $q^{8964} -$   
 598 807 402 442 547 341 060 747 242 945 361 505 207 813 431 090 967 395 670 560 799 643 006 740 122  
 177 943 997 840 721 755 103 001 452 701 395 880 887 916 865 260 426 278 323 914 040 838 200 253 101  
 643 762 193 228 444 783 081 355 773 730 253 268 468 019 541 100 052 435 972 381 419 083 855 825  
 $q^{8965} +$

652 603 243 815 511 569 382 292 965 415 483 482 590 582 616 079 516 358 620 450 124 317 761 222 595  
 982 292 585 168 997 978 828 085 263 269 906 931 836 136 757 389 891 415 178 444 257 057 957 363 078  
 512 279 940 591 197 674 136 723 482 087 257 803 773 459 028 260 076 726 944 710 734 872 160 256  
 $q^{8968} -$

671 586 356 417 415 296 480 816 490 520 487 605 577 862 328 845 800 526 428 151 428 315 238 201 535  
 113 032 341 873 947 047 203 566 386 440 484 989 260 982 682 679 031 508 604 496 666 852 524 398 185  
 350 436 295 071 709 480 234 540 965 157 984 045 851 587 763 918 032 132 186 085 024 911 360 000  
 $q^{8969} +$

731 906 522 834 289 857 338 154 728 110 857 834 055 891 953 241 841 103 264 790 397 966 233 179 381  
 396 914 223 643 685 928 939 189 601 096 957 090 545 982 973 149 666 166 887 111 402 123 093 102 936  
 928 929 470 314 510 091 354 241 647 977 601 739 383 176 591 558 305 338 849 190 090 869 736 960  
 $q^{8972} -$

753 191 627 122 747 290 899 702 395 153 176 422 195 970 865 084 161 143 136 446 373 427 224 989 504  
 738 263 032 254 541 624 824 929 333 679 902 466 694 853 701 470 442 661 593 047 691 465 612 615 537  
 250 002 843 897 457 115 490 295 167 218 085 427 144 811 041 352 796 633 684 155 213 098 223 745  
 $q^{8973} +$

820 825 665 293 310 511 853 395 394 261 115 512 593 206 522 294 394 970 322 763 904 418 005 195 843  
 048 411 185 441 838 213 971 119 151 589 466 554 907 103 647 813 269 649 293 803 092 533 068 044 664  
 288 262 435 754 193 494 851 178 953 595 157 058 705 398 440 393 600 180 250 698 821 468 160 000  
 $q^{8976} -$

844 691 306 383 160 247 437 809 326 838 581 759 536 778 365 756 965 341 704 590 331 065 215 028 269  
 532 854 360 285 887 723 465 868 202 444 398 048 321 217 327 205 872 731 983 649 035 308 427 616 479  
 770 214 117 958 560 947 302 507 390 203 285 893 268 430 970 797 965 736 025 039 838 935 842 816  
 $q^{8977} +$

920 524 103 151 043 625 200 207 977 079 319 388 390 756 325 876 085 141 287 989 859 575 140 395 624  
 836 894 899 066 003 567 044 663 001 170 052 055 041 897 026 774 852 906 821 169 773 141 709 302 593  
 998 755 803 490 172 477 983 063 232 272 010 700 909 744 245 060 575 685 665 117 980 089 958 400  
 $q^{8980} -$

947 282 457 417 788 758 873 792 841 480 238 949 367 436 172 750 847 697 636 402 204 588 325 609 927  
 768 182 515 257 407 014 321 135 648 964 742 131 903 485 539 532 533 751 143 312 962 501 763 391 431  
 569 148 423 220 898 007 594 891 679 360 850 922 621 695 165 958 700 788 749 001 908 712 057 500  
 $q^{8981} +$

1 032 305 727 371 397 233 962 052 557 476 374 744 871 609 506 371 789 509 066 189 461 221 717 695 704  
 533 318 561 656 364 878 286 915 949 580 022 422 411 022 256 100 303 776 160 321 951 962 671 675 791  
 406 285 392 086 564 899 548 478 174 917 811 513 408 146 225 661 379 192 964 362 661 205 056 000  
 $q^{8984} -$

1 062 306 654 240 886 897 363 389 032 028 234 447 521 864 761 604 562 190 106 831 925 715 690 473 436  
 068 804 778 915 087 691 943 434 248 806 325 032 364 471 509 780 324 710 619 413 473 881 875 490 723  
 525 635 887 176 170 584 862 005 786 344 606 908 544 226 247 530 054 822 641 743 134 310 400 000  
 $q^{8985} +$

1 157 631 808 471 791 314 968 202 384 426 189 516 557 703 194 864 942 617 495 918 058 508 616 577 159  
 428 955 055 995 618 737 107 397 465 223 001 432 619 879 780 427 381 700 684 019 297 717 358 170 967  
 006 726 560 777 151 972 725 426 282 748 994 295 601 497 405 878 614 527 115 886 555 942 834 176  
 $q^{8988} -$

1 191 267 389 297 565 839 232 613 206 493 325 211 880 996 304 718 179 966 610 639 218 288 005 432 523  
 473 038 167 290 226 099 932 034 034 232 836 619 462 488 340 919 783 326 307 570 777 057 534 473 135  
 672 084 666 880 707 503 325 813 011 042 327 775 818 858 143 549 937 973 328 176 040 788 189 500  
 $q^{8989} +$

1 298 139 951 000 492 177 933 563 802 481 142 666 412 416 162 831 593 679 263 292 412 577 817 151 268  
 136 309 618 739 895 926 280 369 493 114 634 319 894 448 140 314 247 218 965 234 256 672 952 085 886  
 396 063 018 672 381 320 868 248 211 105 883 268 411 709 643 760 360 560 874 702 347 631 788 032  
 $q^{8992} -$

1 335 849 573 457 219 924 815 265 029 865 292 072 754 496 075 244 294 592 862 234 514 719 522 593 669  
 188 958 466 467 084 215 650 624 155 540 789 869 073 465 885 200 722 215 212 250 401 648 858 231 985  
 749 263 265 149 861 928 903 184 782 173 100 479 472 082 506 576 746 264 586 255 601 513 627 648

$q^{8993} +$   
 1 455 665 325 900 715 574 381 182 198 162 160 796 674 721 962 523 222 455 985 418 012 691 685 757 386 474 228 778 852 943 832 697 790 042 173 697 524 452 014 949 765 203 729 810 652 126 055 700 722 029 958 535 169 719 099 080 771 725 655 647 346 063 848 058 096 766 427 037 200 991 414 972 416 000

$q^{8996} -$   
 1 497 941 379 315 711 940 724 487 035 027 675 706 816 733 769 963 968 088 287 519 820 258 160 170 790 214 214 004 271 771 729 537 199 803 342 516 571 396 248 071 938 735 219 600 602 328 353 815 339 421 586 183 102 961 714 809 804 055 384 951 809 325 687 025 655 625 518 262 676 003 343 973 427 838

$q^{8997} +$   
 1 632 264 453 916 785 340 002 356 157 435 083 478 770 800 219 918 110 182 735 810 036 321 024 937 192 849 922 337 601 368 489 398 963 717 698 012 968 386 882 162 170 882 850 714 506 710 490 347 729 410 081 493 228 799 547 784 858 740 775 222 461 063 564 166 917 904 914 251 219 903 883 520 640 000

$q^{9000} -$   
 1 679 658 708 790 443 386 677 233 014 685 187 897 872 230 648 007 678 986 682 001 863 768 205 211 591 065 397 262 228 440 209 695 432 571 386 014 478 568 797 215 955 903 096 380 406 427 928 861 954 770 441 349 319 979 958 694 216 832 758 131 555 717 864 849 327 793 304 276 145 110 609 293 312 000

$q^{9001} +$   
 1 830 241 845 882 341 509 512 711 925 643 212 768 856 155 388 376 929 633 661 103 052 189 942 544 404 937 835 000 770 871 596 445 251 705 763 317 294 050 858 678 879 728 177 010 042 167 394 028 719 276 559 736 327 917 384 923 342 798 524 996 546 481 098 564 915 891 053 817 200 645 613 209 792 000

$q^{9004} -$   
 1 883 372 599 611 964 198 982 379 479 532 352 129 447 908 554 885 604 767 577 857 213 217 209 545 326 912 749 070 055 305 901 378 157 666 859 136 599 001 282 567 084 073 554 928 911 373 766 327 145 011 683 030 336 145 223 297 111 650 666 368 960 515 321 859 850 709 193 306 791 033 202 029 643 025

$q^{9005} +$   
 2 052 179 842 317 749 843 195 059 559 599 431 115 531 322 344 928 404 635 696 818 701 168 798 839 523 889 491 371 464 033 864 171 629 932 234 269 430 692 925 239 765 504 231 932 040 380 684 247 553 930 944 998 085 233 074 325 560 690 337 991 539 030 606 675 619 417 807 173 179 571 826 395 901 952

$q^{9008} -$   
 2 111 739 922 949 138 816 627 287 416 375 161 068 974 597 328 731 606 885 403 276 122 852 335 579 234 018 432 455 341 812 422 653 142 048 218 797 769 489 101 300 410 329 133 132 847 255 686 915 905 797 660 562 648 431 489 138 852 740 488 480 551 600 867 276 867 423 878 737 025 347 655 458 816 000

$q^{9009} +$   
 2 300 972 035 718 404 585 606 604 701 384 386 514 788 393 035 588 318 936 093 088 341 694 821 067 245 877 709 609 812 150 901 594 754 493 798 245 426 534 909 192 787 468 707 271 487 541 689 614 487 375 000 249 898 600 650 803 085 693 094 726 808 783 888 600 570 968 206 192 083 213 379 027 341 312

$q^{9012} -$   
 2 367 737 766 530 254 981 477 102 270 932 649 132 724 757 163 035 436 191 904 306 135 567 960 402 771 555 542 228 295 650 776 702 325 299 048 892 101 093 999 787 232 529 288 746 238 071 604 830 420 890 109 335 037 984 682 594 837 914 740 526 355 049 275 009 064 234 029 370 191 480 199 907 057 002

$q^{9013} +$   
 2 579 860 704 757 740 146 512 099 773 840 207 038 010 189 834 021 828 049 134 011 199 083 619 662 484 275 760 684 144 126 221 431 687 564 517 763 001 681 346 793 763 960 547 417 144 344 385 314 997 232 916 787 380 948 838 239 038 454 693 001 978 804 322 612 508 561 613 428 796 771 804 322 432 000

$q^{9016} -$   
 2 654 701 944 774 853 742 165 382 069 910 220 545 005 810 399 809 389 950 622 449 748 250 728 931 995 439 905 224 581 470 594 871 949 413 838 740 840 371 376 228 277 771 698 123 429 496 787 321 184 466 188 347 735 190 766 127 617 671 525 891 460 741 167 052 782 237 245 714 632 812 182 937 468 928

$q^{9017} +$   
 2 892 478 740 940 504 882 451 703 710 967 406 850 081 022 186 272 558 602 665 714 185 996 228 137 941 335 706 839 025 080 202 746 484 463 103 425 985 011 619 963 186 196 699 179 489 305 459 166 391 160 344 280 407 694 384 845 984 480 848 057 493 402 464 270 872 883 010 566 262 970 288 032 460 800

$q^{9020} -$   
 2 976 370 130 229 073 742 802 030 314 900 958 919 715 011 399 245 359 983 030 727 589 288 730 441 419 874 494 413 927 775 616 939 584 638 366 600 246 927 291 384 815 024 178 850 066 317 030 927 769 443

466 407 853 311 370 061 745 609 304 394 684 111 079 166 109 531 396 818 268 949 898 980 675 250  
 $q^{9021} +$   
 3 242 896 605 674 390 896 050 268 931 868 287 353 040 522 389 796 658 262 007 798 513 579 362 696 479  
 957 044 265 464 388 322 888 354 835 905 732 620 838 967 656 151 535 392 476 849 327 531 378 489 254  
 349 691 580 329 349 374 735 347 538 999 569 054 157 108 416 819 786 639 691 873 964 589 056 000  
 $q^{9024} -$   
 3 336 930 159 670 664 876 769 728 166 018 659 632 868 525 606 415 348 636 320 260 261 244 903 052 450  
 968 999 906 165 011 228 351 427 824 377 215 465 328 526 728 096 648 995 703 730 644 543 986 887 700  
 414 458 855 248 888 618 315 686 482 342 346 363 074 762 067 754 434 329 066 354 647 000 318 200  
 $q^{9025} +$   
 3 635 674 920 010 007 588 897 230 325 921 376 599 935 719 972 686 482 463 601 684 860 339 325 573 784  
 566 027 705 322 662 791 828 508 487 255 631 665 689 271 782 754 825 333 614 159 580 896 697 631 705  
 760 889 120 008 630 452 728 794 142 116 601 641 716 500 019 550 758 511 662 035 866 828 963 840  
 $q^{9028} -$   
 3 741 074 134 367 818 207 667 315 960 460 955 720 210 829 436 137 696 530 540 962 455 665 415 539 819  
 901 603 638 677 447 674 143 769 552 644 614 821 510 152 207 866 368 805 096 604 490 330 080 290 651  
 792 300 107 923 191 666 317 176 009 020 632 727 971 165 941 135 948 373 243 972 765 207 711 625  
 $q^{9029} +$   
 4 075 923 361 245 514 009 569 115 402 460 171 314 011 876 558 017 367 905 571 456 721 391 505 175 077  
 394 970 681 472 150 873 573 139 730 317 886 990 599 878 383 839 300 338 612 936 243 862 554 496 253  
 324 450 438 388 570 087 085 413 624 124 213 381 986 505 083 146 770 874 952 179 344 856 472 576  
 $q^{9032} -$   
 4 194 059 007 976 851 039 359 833 705 632 544 855 452 654 925 831 909 099 854 842 100 828 278 818 077  
 768 800 040 657 966 011 360 999 848 655 143 399 431 812 436 621 690 448 862 197 915 393 738 465 892  
 251 235 065 871 603 682 348 109 739 832 961 630 144 836 082 167 048 783 550 693 062 344 278 016  
 $q^{9033} +$   
 4 569 366 621 114 851 913 086 238 612 123 015 713 313 331 051 380 823 427 472 488 327 295 636 801 865  
 196 204 809 051 307 786 452 313 763 506 662 373 583 190 756 457 155 038 321 022 171 217 182 001 798  
 584 990 559 059 905 078 397 660 478 455 346 227 663 956 499 925 111 779 202 013 853 983 552 000  
 $q^{9036} -$   
 4 701 774 438 385 382 112 180 420 198 780 338 382 000 526 571 702 464 479 405 280 954 340 050 019 348  
 498 699 431 640 029 981 313 186 780 622 552 607 120 998 901 224 614 083 716 347 158 919 039 890 842  
 057 557 835 704 898 105 430 815 821 528 467 417 040 529 972 882 473 368 904 447 528 850 386 637  
 $q^{9037} +$   
 5 122 418 270 397 567 493 371 634 518 162 554 425 930 793 438 820 512 076 925 027 778 313 236 669 608  
 840 469 876 360 657 913 633 444 824 432 232 073 261 259 942 152 546 145 577 011 745 431 778 640 517  
 584 863 602 176 373 788 497 817 468 926 228 015 874 385 245 144 553 743 564 279 931 316 633 600  
 $q^{9040} -$   
 5 270 818 772 499 062 456 751 493 373 799 220 601 618 446 075 628 940 506 112 463 598 825 959 291 872  
 320 859 447 051 594 215 130 432 540 646 338 206 211 766 053 848 682 875 357 522 050 452 021 235 196  
 612 184 378 529 069 143 736 159 534 128 061 712 333 801 939 552 632 548 275 059 535 400 960 000  
 $q^{9041} +$   
 5 742 263 475 644 871 786 119 904 410 187 567 552 929 538 521 483 854 544 827 588 441 522 780 055 938  
 909 717 892 782 638 606 936 552 590 762 866 725 151 390 833 186 848 814 765 235 351 679 124 635 733  
 403 529 179 819 506 844 875 475 914 504 001 769 768 234 632 210 182 445 526 962 858 484 736 000  
 $q^{9044} -$   
 5 908 584 136 704 836 137 572 118 195 169 473 290 377 952 836 922 291 840 649 130 920 939 690 739 470  
 153 608 879 298 918 737 414 589 628 761 701 651 579 095 216 032 385 515 401 557 029 217 730 130 918  
 291 940 190 060 778 858 246 041 321 117 979 939 569 066 525 566 462 465 065 529 751 911 804 925  
 $q^{9045} +$   
 6 436 951 626 587 481 314 887 203 341 160 787 819 056 316 803 886 773 176 411 684 533 977 030 504 283  
 697 977 832 638 110 203 330 025 521 245 857 519 768 051 712 640 489 410 108 612 727 911 257 990 193  
 092 175 553 976 450 148 740 335 244 044 708 243 130 063 277 805 342 102 917 915 228 772 050 944  
 $q^{9048} -$   
 6 623 351 721 834 994 612 004 925 832 572 470 910 176 124 451 451 112 913 292 417 460 621 656 565 203

844 113 215 322 053 547 480 538 851 108 338 135 765 918 087 683 075 295 926 881 455 220 875 611 013  
 959 980 269 848 896 125 931 156 850 169 252 883 967 906 987 464 697 901 471 440 714 227 712 000  
 $q^{9049} +$   
 7 215 500 059 103 966 056 478 461 865 597 741 280 474 792 588 298 090 993 371 019 847 423 947 354 933  
 632 993 112 447 861 606 688 913 695 744 147 014 421 203 788 005 251 287 519 315 774 887 400 982 587  
 393 872 626 333 910 406 686 925 970 349 145 109 317 551 842 137 331 052 170 160 002 149 199 872  
 $q^{9052} -$   
 7 424 398 481 372 608 432 330 775 986 192 347 953 587 197 665 551 817 462 235 706 746 895 238 537 409  
 095 547 080 604 056 464 897 976 282 372 927 406 797 806 194 221 341 243 068 004 041 006 761 474 908  
 640 198 170 220 576 985 758 101 684 096 010 021 713 555 672 848 622 782 312 455 637 988 158 060  
 $q^{9053} +$   
 8 088 010 199 981 255 000 705 684 173 979 681 645 740 166 471 208 978 772 404 538 761 882 945 218 537  
 896 094 985 655 236 625 723 665 345 813 084 752 124 275 170 565 020 616 919 820 517 842 031 136 989  
 966 361 825 651 155 861 849 915 709 483 775 324 258 795 474 611 517 155 252 369 842 253 312 000  
 $q^{9056} -$   
 8 322 116 607 023 103 382 488 600 485 174 686 520 036 166 941 210 600 042 562 191 733 110 042 193 126  
 862 379 005 481 037 438 396 325 427 825 990 512 883 220 816 403 379 465 144 820 464 647 132 434 142  
 981 522 347 058 033 590 845 572 568 871 172 787 511 241 544 768 390 581 562 657 785 659 555 840  
 $q^{9057} +$   
 9 065 797 617 878 479 935 744 812 542 698 090 049 386 319 802 696 162 594 984 656 299 303 560 123 852  
 737 554 771 871 987 940 973 697 345 892 079 628 114 046 158 369 942 119 079 827 191 126 783 376 698  
 009 153 676 305 150 939 028 723 540 561 366 750 076 648 087 081 156 053 948 767 433 621 504 000  
 $q^{9060} -$   
 9 328 147 308 466 424 526 717 408 542 166 914 310 246 406 077 745 785 115 553 885 838 758 895 954 946  
 898 467 485 419 229 990 325 791 890 715 364 635 998 722 799 496 566 747 850 007 523 270 610 672 490  
 896 409 492 551 557 894 955 210 312 813 508 545 500 877 154 554 808 668 556 574 786 174 624 250  
 $q^{9061} +$   
 10 161 537 641 910 184 464 283 550 540 774 266 770 775 842 637 641 820 749 252 955 595 626 114 209  
 912 001 652 922 811 615 285 344 944 292 185 995 666 130 792 226 180 739 378 274 567 774 695 746 407  
 197 690 623 525 426 920 465 178 466 001 298 089 158 450 975 198 650 612 391 800 665 930 732 928 000  
 $q^{9064} -$   
 10 455 530 606 154 875 444 785 323 737 438 428 469 995 548 419 240 600 746 810 928 871 564 761 693  
 547 507 733 265 767 042 268 486 374 596 749 965 339 314 090 564 533 737 865 210 268 707 456 078 269  
 134 331 316 456 008 873 480 185 113 494 406 101 283 030 264 607 000 457 541 624 353 587 049 267 200  
 $q^{9065} +$   
 11 389 428 407 330 695 981 238 698 889 536 896 507 303 282 826 777 136 516 355 023 969 327 202 976  
 449 186 750 659 421 305 605 352 342 045 024 387 511 893 793 202 484 859 046 062 817 228 850 401 726  
 729 360 537 579 133 335 136 455 570 874 517 073 941 638 500 667 182 846 465 279 245 206 034 458 112  
 $q^{9068} -$   
 11 718 873 049 732 419 277 536 990 529 495 803 707 826 188 542 168 398 443 858 458 224 839 948 010  
 359 376 318 867 003 023 445 434 238 772 153 745 963 102 219 177 554 095 896 894 531 588 394 295 409  
 631 570 050 932 197 445 281 290 030 373 788 996 056 424 740 798 606 589 758 311 565 007 970 720 750  
 $q^{9069} +$   
 12 765 373 409 428 679 450 753 245 103 172 735 866 232 763 492 991 299 327 082 455 759 309 819 717  
 762 560 381 181 576 745 885 772 071 868 556 024 805 914 023 993 969 100 817 463 088 755 862 631 076  
 391 064 068 436 138 711 526 489 547 148 947 984 477 469 392 248 234 382 027 384 150 540 453 527 552  
 $q^{9072} -$   
 13 134 535 502 593 495 676 488 116 404 637 268 366 687 204 531 823 241 288 878 085 576 726 535 717  
 525 771 247 493 905 554 443 119 414 488 857 077 886 822 290 352 643 766 329 313 129 587 541 778 678  
 567 570 366 438 722 165 834 607 929 439 553 295 225 994 969 822 101 936 057 684 595 024 072 572 928  
 $q^{9073} +$   
 14 307 185 894 726 331 839 369 921 959 364 431 491 424 490 788 388 501 117 251 287 379 286 306 611  
 368 976 007 286 931 076 088 882 724 500 043 880 129 986 705 853 016 999 091 629 703 786 985 185 966  
 154 326 355 806 128 978 643 049 628 895 332 799 722 132 688 017 180 150 617 196 540 591 459 072 000  
 $q^{9076} -$

14 720 843 388 149 390 932 559 591 771 791 582 330 785 620 715 647 506 282 514 437 242 000 700 227 \\  
 645 220 478 024 827 028 897 690 092 256 707 388 695 359 506 607 217 327 815 540 862 702 320 541 765 \\  
 003 885 809 904 928 203 220 182 511 745 798 552 408 901 067 759 169 327 564 253 132 674 074 258 205 \\  
 $q^{9077} +$

16 034 817 696 049 366 800 013 402 883 000 159 670 171 348 954 175 209 356 709 067 346 486 897 025 \\  
 115 572 484 687 994 650 998 825 861 918 409 118 567 815 021 704 657 111 529 670 924 780 324 572 848 \\  
 200 371 900 027 868 345 019 370 861 174 488 991 626 625 506 905 354 676 841 133 858 675 497 651 200 \\  
 $q^{9080} -$

16 498 322 078 744 690 919 988 491 592 736 516 817 246 055 527 120 099 853 992 001 360 963 454 617 \\  
 379 212 789 996 560 818 343 022 069 868 848 508 280 705 622 049 682 676 315 239 052 657 936 963 106 \\  
 603 364 888 155 739 840 878 012 555 229 814 115 142 851 796 948 766 703 759 170 275 086 192 640 000 \\  
 $q^{9081} +$

17 970 615 428 490 327 624 629 313 840 599 614 040 873 769 745 187 087 484 625 183 779 757 405 849 \\  
 229 902 169 856 699 787 269 371 946 994 782 255 425 637 503 152 855 245 132 553 253 605 481 342 741 \\  
 015 486 256 150 147 989 781 002 786 484 584 665 445 175 450 241 812 952 353 439 875 615 632 640 000 \\  
 $q^{9084} -$

18 489 960 427 463 045 896 121 374 513 467 727 641 953 993 318 993 256 227 920 598 296 036 636 740 \\  
 486 047 913 778 980 042 182 932 102 536 564 130 489 636 706 493 575 485 219 498 551 563 052 744 815 \\  
 640 594 794 748 088 080 273 698 520 838 422 031 133 044 443 389 602 885 401 812 835 879 633 092 625 \\  
 $q^{9085} +$

20 139 607 310 641 483 978 768 913 990 151 078 669 168 585 724 798 051 187 005 830 983 769 394 680 \\  
 250 018 329 849 185 374 174 782 901 519 280 219 534 667 965 838 771 492 700 368 426 392 145 193 805 \\  
 862 720 972 536 101 787 877 886 846 227 179 954 574 994 866 971 177 736 906 167 293 706 603 397 120 \\  
 $q^{9088} -$

20 721 505 800 303 991 039 111 478 856 972 133 926 565 538 497 390 644 862 757 898 882 811 506 993 \\  
 422 369 885 151 260 426 204 825 685 902 562 145 653 954 974 308 219 821 360 157 788 843 088 542 253 \\  
 500 919 321 159 464 986 969 214 082 970 570 307 876 669 041 296 001 817 733 245 724 618 432 512 000 \\  
 $q^{9089} +$

22 569 824 264 100 360 315 104 875 781 216 300 104 774 873 477 340 925 894 703 388 482 477 991 641 \\  
 455 971 906 713 431 517 233 920 959 905 799 186 470 721 185 183 133 103 415 459 605 247 117 751 600 \\  
 441 654 820 053 753 744 846 782 267 468 708 335 875 777 580 109 710 727 829 863 763 226 100 301 824 \\  
 $q^{9092} -$

23 221 794 365 900 728 224 339 864 110 162 297 748 219 957 447 881 179 930 657 113 025 571 175 698 \\  
 107 170 737 029 021 648 183 864 593 786 673 428 001 301 717 752 324 109 467 895 165 394 056 109 439 \\  
 670 749 089 988 640 648 352 539 618 201 380 048 594 807 449 835 155 185 533 667 603 827 577 233 512 \\  
 $q^{9093} +$

25 292 659 379 044 369 323 555 861 486 564 162 042 670 275 495 896 172 612 281 185 606 174 544 282 \\  
 801 112 450 630 055 405 608 548 898 069 859 956 160 500 505 362 984 127 096 564 525 566 165 235 852 \\  
 057 338 272 532 976 739 260 186 014 148 658 517 933 852 617 410 727 980 322 160 857 139 369 984 000 \\  
 $q^{9096} -$

26 023 120 847 114 880 201 975 979 917 656 870 576 163 044 027 993 505 323 113 994 565 022 726 627 \\  
 120 446 147 835 252 548 372 614 035 977 368 257 099 268 076 857 972 205 196 780 299 015 925 141 273 \\  
 166 877 718 621 730 768 726 652 092 936 993 223 465 207 312 533 877 288 081 512 193 622 629 580 800 \\  
 $q^{9097} +$

28 343 270 320 103 597 219 711 342 222 595 666 871 438 637 083 099 423 880 085 883 451 737 371 846 \\  
 730 071 094 277 131 096 553 608 632 518 110 147 770 134 539 290 442 743 262 759 812 466 112 985 845 \\  
 566 344 638 560 818 922 325 004 496 933 193 047 819 816 372 283 428 284 985 445 287 551 216 460 800 \\  
 $q^{9100} -$

29 161 652 439 115 912 323 277 574 526 235 868 935 397 046 026 270 681 282 389 725 169 021 309 222 \\  
 201 750 858 404 063 597 848 455 949 911 433 314 646 653 443 673 027 716 222 356 471 698 725 103 852 \\  
 210 284 208 131 826 412 449 309 713 106 788 643 150 651 851 332 871 043 754 681 776 219 708 639 125 \\  
 $q^{9101} +$

31 761 029 790 952 329 572 972 974 788 360 448 546 919 920 838 781 434 760 299 811 774 815 733 036 \\  
 014 756 745 347 480 943 687 447 330 920 827 476 564 509 319 054 829 747 897 682 558 774 331 941 437 \\  
 069 368 092 329 655 877 970 831 383 024 468 842 709 060 810 027 330 140 656 791 026 037 227 520 000

$q^{9104} -$   
 32 677 892 158 223 429 201 296 428 242 223 613 981 573 817 249 495 459 456 508 145 807 662 268 654 \ \backslash  
 463 404 216 059 395 740 451 706 236 910 911 762 193 485 669 091 602 036 697 601 246 999 925 996 355 \ \backslash  
 907 722 400 029 617 646 570 818 314 084 359 938 243 608 646 427 209 368 415 759 696 893 557 145 600  
 $q^{9105} +$   
 35 590 029 784 833 943 185 521 735 677 309 869 509 758 289 227 373 653 981 793 701 033 698 269 010 \ \backslash  
 246 792 165 424 433 202 203 916 311 878 728 985 989 786 812 879 141 061 243 523 882 582 347 834 845 \ \backslash  
 903 242 963 499 265 294 339 644 421 333 855 692 696 225 200 201 805 315 759 761 823 145 406 451 712  
 $q^{9108} -$   
 36 617 197 511 897 316 821 959 896 420 692 798 496 739 642 953 379 654 883 645 066 508 084 817 320 \ \backslash  
 048 281 658 481 206 160 878 002 596 401 673 364 170 364 865 024 635 318 056 582 931 369 040 312 505 \ \backslash  
 739 686 041 028 353 225 995 591 854 637 350 507 598 153 244 122 775 613 561 582 470 217 912 911 750  
 $q^{9109} +$   
 39 879 646 029 282 952 114 424 716 232 100 332 776 973 579 364 628 590 647 634 811 000 267 699 578 \ \backslash  
 236 209 071 746 019 346 506 755 364 905 320 163 640 509 226 887 234 935 020 728 334 292 997 790 833 \ \backslash  
 757 544 281 597 419 667 536 388 814 356 903 218 034 192 497 991 030 284 208 046 753 952 290 535 424  
 $q^{9112} -$   
 41 030 361 080 673 118 537 776 126 558 808 708 166 862 358 607 809 367 594 315 652 158 470 394 923 \ \backslash  
 205 412 583 094 011 408 454 575 934 836 026 914 098 249 688 538 618 288 273 397 676 706 956 326 397 \ \backslash  
 264 698 537 875 240 678 457 957 893 959 864 265 907 823 611 290 246 549 427 312 349 164 212 191 232  
 $q^{9113} +$   
 44 685 169 795 169 473 440 776 347 465 502 655 298 303 270 063 746 676 883 468 197 962 896 683 855 \ \backslash  
 817 057 895 922 589 864 127 585 926 478 897 708 688 463 361 958 707 024 850 604 682 775 980 801 573 \ \backslash  
 858 257 217 226 515 208 870 865 431 218 496 373 234 175 704 283 172 389 659 773 219 072 683 264 000  
 $q^{9116} -$   
 45 974 260 386 357 638 435 793 416 432 458 093 010 413 851 262 880 881 364 783 649 961 173 600 362 \ \backslash  
 862 749 034 012 155 637 165 981 196 441 714 907 406 984 839 243 574 191 997 617 946 267 959 018 893 \ \backslash  
 847 759 387 742 833 832 359 980 321 005 052 739 683 404 069 591 688 048 683 802 687 629 237 699 567  
 $q^{9117} +$   
 50 068 515 092 433 609 103 473 197 802 131 607 246 042 608 507 010 841 525 431 025 031 884 471 362 \ \backslash  
 547 245 438 619 048 767 989 663 647 268 167 962 080 173 494 113 254 516 101 736 566 053 796 580 958 \ \backslash  
 261 590 782 216 459 101 650 837 757 278 502 097 539 888 812 952 405 621 169 173 764 526 039 040 000  
 $q^{9120} -$   
 51 512 585 297 261 919 134 832 621 251 503 234 014 241 072 227 245 379 110 294 618 685 150 047 055 \ \backslash  
 102 739 340 155 651 417 959 149 432 942 263 308 790 819 192 892 119 758 424 755 193 676 137 755 991 \ \backslash  
 912 025 993 273 809 870 604 634 257 890 523 477 701 838 761 952 281 165 762 797 213 472 800 768 000  
 $q^{9121} +$   
 56 099 010 228 199 159 134 303 094 521 735 796 631 213 183 486 559 723 376 963 722 208 851 191 835 \ \backslash  
 256 882 044 051 987 986 935 241 182 258 085 005 707 656 608 679 763 374 273 049 086 566 520 912 637 \ \backslash  
 913 291 342 663 134 467 851 060 895 655 015 481 831 943 228 487 716 038 764 549 068 955 740 160 000  
 $q^{9124} -$   
 57 716 652 201 657 244 439 191 671 674 385 307 196 119 283 854 593 447 534 726 279 091 270 340 319 \ \backslash  
 140 516 804 160 568 564 793 406 253 827 998 080 173 112 165 893 530 685 319 022 244 679 445 522 253 \ \backslash  
 271 378 985 240 145 437 758 057 966 740 395 956 449 256 773 132 356 563 200 893 291 486 404 473 750  
 $q^{9125} +$   
 62 854 283 769 320 400 211 119 943 953 501 818 513 028 252 283 165 830 055 625 779 356 212 007 594 \ \backslash  
 547 974 298 139 661 705 995 261 536 559 000 787 213 518 417 290 822 988 780 588 259 423 821 671 876 \ \backslash  
 115 288 628 846 035 970 899 561 365 982 722 640 160 336 407 943 913 060 198 483 097 419 685 062 656  
 $q^{9128} -$   
 64 666 315 277 295 949 174 187 188 829 772 335 783 782 884 375 035 449 182 544 722 061 904 762 307 \ \backslash  
 104 864 341 842 490 858 546 506 770 288 622 987 225 809 883 871 021 625 105 496 718 795 473 018 906 \ \backslash  
 048 475 593 663 593 885 407 981 929 772 913 396 246 520 127 610 399 392 352 126 699 294 416 896 000  
 $q^{9129} +$   
 70 421 256 144 197 827 435 738 602 238 963 734 874 573 672 799 327 032 607 635 217 545 474 178 628 \ \backslash  
 869 796 616 211 226 585 550 026 321 969 646 236 352 056 465 201 528 981 216 482 349 541 356 623 798 \ \backslash

687 797 013 314 455 817 466 412 969 528 545 030 126 655 870 328 700 605 548 291 395 761 176 316 928  
 $q^{9132} -$   
 72 450 986 411 496 492 871 771 364 516 535 328 287 535 700 335 304 238 456 555 926 557 295 376 423  
 373 180 266 357 554 709 427 118 848 850 438 521 778 659 229 995 516 701 092 020 485 190 940 985 324  
 960 413 805 071 385 555 227 251 326 513 340 635 565 524 072 369 157 857 774 708 000 426 624 349 089  
 $q^{9133} +$   
 78 897 249 452 853 425 190 338 282 939 016 112 040 392 700 045 892 062 594 014 560 007 817 864 662  
 352 351 273 905 023 814 119 041 774 952 412 527 551 742 829 480 154 091 885 665 942 268 597 017 586  
 876 081 671 275 061 937 797 978 989 543 058 815 157 528 676 281 675 007 236 322 736 052 307 456 000  
 $q^{9136} -$   
 81 170 776 698 329 190 222 016 038 102 568 837 210 957 384 720 077 539 968 336 566 039 783 764 582  
 075 883 257 990 591 171 955 734 724 604 214 713 256 709 632 526 764 323 145 748 930 184 799 844 701  
 577 927 100 810 239 165 126 571 382 166 174 877 416 290 621 646 187 195 805 836 199 269 299 585 024  
 $q^{9137} +$   
 88 391 229 546 503 129 986 729 342 973 555 364 164 998 558 691 560 007 065 401 825 660 534 021 653  
 161 229 419 871 480 636 817 204 167 630 415 410 159 851 987 820 739 742 044 836 301 773 842 819 836  
 271 390 529 538 518 906 242 816 509 948 123 909 453 085 847 544 190 292 239 828 689 812 952 576 000  
 $q^{9140} -$   
 90 937 773 974 048 011 116 125 242 879 107 054 593 517 718 776 173 069 573 348 990 114 461 521 488  
 276 609 167 256 722 442 351 316 480 171 706 313 077 065 842 240 219 842 502 894 235 759 960 892 718  
 493 522 951 484 211 841 050 377 065 382 671 101 075 974 895 931 493 873 779 744 715 983 622 150 750  
 $q^{9141} +$   
 99 025 196 106 896 792 809 001 266 919 359 463 656 240 582 669 984 186 359 280 612 132 690 476 132  
 743 900 885 271 640 596 446 666 924 535 350 456 359 227 660 970 233 558 004 907 012 194 646 849 835  
 437 009 933 143 111 196 881 658 959 496 133 672 266 498 183 773 211 719 582 568 699 997 614 592 000  
 $q^{9144} -$   
 101 877 472 568 316 675 313 768 655 376 301 428 992 865 481 696 996 768 673 574 716 447 299 656 408  
 875 687 764 269 152 723 671 446 794 575 810 492 425 703 492 293 617 185 042 641 167 624 479 394 601  
 312 667 275 165 049 916 132 833 070 853 328 839 808 048 171 391 212 685 190 075 238 150 619 136 000  
 $q^{9145} +$   
 110 935 738 322 412 817 481 392 196 070 268 251 345 113 511 190 988 255 498 020 491 579 172 146 270  
 581 916 462 699 032 518 746 405 679 273 057 517 932 455 844 552 121 267 280 315 912 668 947 945 998  
 252 915 050 720 468 042 096 922 985 772 255 641 195 533 791 385 915 024 868 519 307 476 855 259 136  
 $q^{9148} -$   
 114 130 373 368 463 377 059 659 662 483 807 742 722 490 609 529 913 918 131 174 500 843 351 404 159  
 920 049 436 748 307 209 427 585 132 095 743 053 161 153 030 543 680 225 334 277 926 717 089 959 427  
 091 251 344 412 377 288 111 479 697 854 728 725 783 731 674 882 059 739 517 841 985 546 968 130 250  
 $q^{9149} +$   
 124 275 775 845 659 650 570 912 026 498 412 421 135 705 227 483 655 803 443 179 114 655 362 375 540  
 393 482 007 665 382 722 643 719 879 488 855 394 336 011 816 844 486 783 204 682 903 237 939 118 714  
 698 960 827 981 146 211 167 107 556 881 959 793 649 667 961 336 940 096 607 888 486 576 771 694 592  
 $q^{9152} -$   
 127 853 774 440 992 168 900 221 343 830 352 354 290 782 952 999 493 015 803 370 104 074 762 493 193  
 033 690 732 359 185 362 197 646 597 355 506 793 645 515 417 394 165 179 341 005 284 990 920 809 560  
 239 777 308 948 145 949 555 651 568 124 197 870 357 416 740 204 616 583 731 834 234 871 009 050 624  
 $q^{9153} +$   
 139 216 507 052 268 737 893 351 889 066 722 402 392 122 845 977 662 819 956 989 932 683 995 790 592  
 829 508 866 508 242 957 041 772 930 906 102 040 748 837 700 994 249 037 528 094 365 613 497 628 307  
 240 044 388 245 924 245 054 964 199 520 056 416 553 334 115 834 288 139 331 869 717 542 371 328 000  
 $q^{9156} -$   
 143 223 774 855 737 723 226 558 963 971 707 345 710 263 934 732 742 241 391 362 912 131 241 858 422  
 281 676 793 497 638 920 808 155 687 723 379 403 511 637 644 654 153 755 513 492 550 648 124 317 862  
 850 948 914 509 351 834 916 885 737 739 331 344 365 136 503 265 601 028 256 021 359 645 096 679 312  
 $q^{9157} +$   
 155 949 589 231 862 417 893 738 856 466 386 449 576 029 258 495 147 114 473 653 509 963 072 282 303

414 630 548 192 071 371 677 284 138 637 961 828 900 937 050 260 819 446 605 899 944 148 453 837 872 3  
 105 444 298 659 103 083 070 139 892 512 923 892 042 191 703 870 071 788 953 525 605 829 783 782 400  
 $q^{9160} -$   
 160 437 517 043 397 799 340 035 944 050 399 915 417 207 142 679 355 246 826 557 662 554 719 119 281 3  
 559 293 314 069 403 846 360 336 373 503 354 029 500 570 880 878 674 841 475 139 114 625 348 192 294 3  
 235 468 869 338 683 274 284 687 142 889 508 937 454 899 540 518 971 274 230 400 444 162 408 448 000  
 $q^{9161} +$   
 174 689 578 262 486 469 148 500 221 882 837 826 060 926 087 807 288 917 623 625 170 318 526 098 813 3  
 575 577 798 986 498 995 235 229 146 920 967 570 508 268 944 764 884 545 674 647 941 806 744 499 937 3  
 374 844 536 894 416 804 472 550 281 036 221 953 310 563 534 904 847 243 524 027 553 103 894 656 000  
 $q^{9164} -$   
 179 715 696 020 277 244 408 378 826 544 131 812 295 663 778 703 866 545 740 512 583 981 239 995 961 3  
 443 624 819 437 691 130 682 659 269 214 164 214 613 641 468 474 364 041 641 500 492 812 209 302 205 3  
 575 788 664 508 315 721 391 001 203 992 704 343 313 086 997 982 022 113 894 671 682 324 564 846 550  
 $q^{9165} +$   
 195 676 658 585 598 520 960 726 381 144 596 788 829 205 320 055 683 881 224 368 813 256 551 294 825 3  
 586 079 398 768 747 919 501 741 186 998 687 513 350 962 906 759 422 839 724 162 294 604 752 242 910 3  
 563 284 921 533 823 390 349 458 830 662 172 597 829 959 371 444 408 402 313 705 892 953 963 495 424  
 $q^{9168} -$   
 201 305 367 172 447 034 084 977 199 777 224 851 977 337 269 445 463 870 593 434 257 150 973 313 262 3  
 167 381 465 617 715 204 699 640 389 820 044 795 032 176 239 012 262 658 644 189 663 603 474 604 600 3  
 812 009 657 467 026 278 464 061 487 758 743 510 366 401 796 759 271 229 260 347 035 651 014 656 000  
 $q^{9169} +$   
 219 179 697 950 787 400 700 569 922 583 927 804 263 425 029 198 311 561 429 686 796 194 359 971 696 3  
 820 260 509 829 394 630 167 372 100 973 063 301 407 001 420 213 507 122 389 062 187 215 470 906 504 3  
 455 501 476 782 209 346 572 625 809 096 877 849 416 491 000 079 756 547 037 041 860 752 053 819 392  
 $q^{9172} -$   
 225 483 088 047 100 437 106 055 456 521 552 222 632 942 752 659 503 011 637 273 599 196 110 368 067 3  
 004 483 414 735 465 540 955 326 726 237 587 258 110 972 559 122 922 023 241 493 583 928 526 366 076 3  
 003 766 461 826 663 380 231 838 812 549 062 974 866 507 306 900 121 364 506 969 762 920 643 587 122  
 $q^{9173} +$   
 245 499 665 483 356 619 677 997 917 541 812 836 372 229 249 328 154 847 802 334 051 944 362 508 459 3  
 527 947 078 283 773 504 992 098 263 191 229 891 841 701 448 014 072 689 291 970 393 220 701 852 321 3  
 271 042 261 909 429 551 053 713 025 066 521 564 620 551 321 458 802 788 517 694 770 995 916 928 000  
 $q^{9176} -$   
 252 558 433 798 554 734 483 076 673 192 814 479 709 397 896 012 362 997 489 959 149 976 612 265 468 3  
 885 424 163 560 591 485 779 336 063 029 481 774 624 381 167 788 746 270 806 939 800 802 711 103 255 3  
 279 323 925 836 381 903 774 501 479 057 429 983 551 527 137 718 669 842 194 971 241 833 224 863 744  
 $q^{9177} +$   
 274 973 456 194 699 036 002 034 143 262 253 241 257 402 079 899 812 229 444 948 907 926 852 616 738 3  
 714 405 741 363 770 090 005 673 492 114 109 056 414 012 090 482 544 931 411 707 931 814 323 302 594 3  
 661 247 585 917 353 733 063 043 840 579 080 933 683 079 774 596 721 614 068 815 953 640 824 832 000  
 $q^{9180} -$   
 282 877 930 632 500 720 186 039 797 800 774 168 532 947 835 852 211 001 488 026 438 541 650 165 473 3  
 580 361 823 993 867 479 125 288 011 230 001 142 586 594 179 065 598 978 212 474 646 932 231 241 468 3  
 269 545 166 365 098 609 493 700 328 367 000 007 812 052 246 528 535 716 897 726 360 577 277 075 250  
 $q^{9181} +$   
 307 978 170 161 981 318 219 051 643 903 729 573 798 333 222 400 527 225 918 615 837 324 961 971 809 3  
 853 516 390 935 503 720 194 693 244 717 699 140 609 083 623 456 364 970 980 488 012 690 231 966 042 3  
 787 719 006 202 080 759 374 346 813 747 096 646 781 091 048 346 707 719 865 165 289 405 214 720 000  
 $q^{9184} -$   
 316 829 456 843 312 734 694 365 202 561 065 628 597 890 119 548 873 666 881 909 636 232 461 218 425 3  
 262 848 621 743 689 748 926 254 881 267 140 428 777 755 880 376 725 620 424 578 090 984 312 048 424 3  
 282 402 190 039 970 047 695 085 563 592 678 767 403 240 729 533 184 143 868 606 922 163 567 001 600  
 $q^{9185} +$

344 935 900 313 713 845 453 047 107 647 360 191 687 315 695 776 441 897 212 903 037 842 965 890 315 \
 877 452 042 520 336 423 860 896 060 322 433 467 045 977 485 151 986 437 795 827 744 582 734 141 085 \
 314 118 798 774 678 796 265 441 493 788 213 567 794 571 709 283 888 220 830 999 162 408 038 793 216 \
  $q^{9188}$  -

354 847 166 910 962 968 460 047 527 121 558 289 870 259 190 160 323 917 004 537 463 994 694 127 440 \
 477 651 938 710 510 332 417 334 038 006 137 493 453 345 676 078 675 430 715 175 881 141 594 019 630 \
 278 444 577 022 166 200 963 834 258 440 155 594 821 143 941 119 672 514 832 823 220 761 317 364 375 \
  $q^{9189}$  +

386 319 089 142 465 138 619 463 017 920 225 444 316 134 145 855 251 300 902 138 693 727 655 525 877 \
 555 463 130 765 717 321 515 835 641 743 615 359 107 184 693 680 591 448 447 132 901 497 535 895 245 \
 677 992 788 166 889 229 687 190 959 277 042 854 093 507 027 987 932 801 107 813 733 298 889 056 256 \
  $q^{9192}$  -

397 417 000 689 503 246 108 370 261 012 567 664 955 803 360 155 664 274 799 435 858 318 431 470 270 \
 096 811 139 678 521 786 353 588 008 940 353 445 112 968 902 087 950 879 313 226 068 870 772 852 439 \
 704 978 439 425 760 136 534 308 047 233 220 381 128 329 155 703 899 483 297 385 037 813 004 763 136 \
  $q^{9193}$  +

432 656 521 804 824 223 165 377 009 758 147 731 497 921 079 360 127 515 849 072 505 405 959 481 157 \
 502 188 545 241 107 940 918 213 531 448 809 977 897 153 386 190 289 317 670 210 135 920 569 877 397 \
 591 657 865 741 023 892 635 459 580 440 768 110 574 593 755 543 399 263 710 035 140 065 078 208 000 \
  $q^{9196}$  -

445 082 847 059 962 546 129 958 124 093 304 756 153 281 403 616 898 392 473 358 137 910 743 598 321 \
 085 744 673 902 309 953 752 155 956 470 980 609 032 303 463 560 528 068 361 484 720 593 020 334 453 \
 815 797 386 966 004 895 387 668 036 497 890 690 058 762 563 346 832 464 398 610 500 539 185 888 205 \
  $q^{9197}$  +

484 540 031 050 610 426 592 934 346 602 313 726 808 576 377 421 248 834 558 090 326 490 454 849 638 \
 905 560 614 438 315 829 936 727 166 773 624 819 824 663 377 739 505 199 735 410 568 656 978 505 858 \
 447 829 475 626 157 142 386 377 756 121 748 275 636 778 778 977 889 853 219 558 041 261 877 248 000 \
  $q^{9200}$  -

498 453 439 628 256 047 270 548 485 703 636 238 943 566 172 815 102 327 646 997 987 963 395 715 246 \
 687 414 662 901 962 068 031 549 421 815 987 998 165 344 035 922 742 202 136 470 287 997 023 625 349 \
 584 454 454 768 136 522 859 548 725 722 020 421 222 613 414 267 609 166 327 749 409 665 617 920 000 \
  $q^{9201}$  +

542 631 998 347 623 876 376 697 830 550 364 737 336 267 324 662 343 217 703 706 143 668 310 148 676 \
 487 046 035 953 914 046 187 439 056 853 238 424 873 053 703 240 376 618 042 159 535 594 809 994 378 \
 312 389 877 318 069 634 977 795 201 954 135 988 363 382 640 597 366 162 671 074 469 392 490 496 000 \
  $q^{9204}$  -

558 210 071 225 457 491 615 117 996 194 065 288 778 340 385 382 846 161 858 074 718 469 007 647 159 \
 223 823 883 693 149 275 708 382 429 961 045 009 971 001 847 948 965 920 103 389 706 803 269 553 437 \
 802 626 306 432 790 855 606 889 223 175 275 919 629 091 930 399 339 459 282 912 307 832 985 384 075 \
  $q^{9205}$  +

607 673 745 545 949 184 781 774 325 198 983 916 662 327 904 794 056 004 862 362 177 677 979 425 164 \
 557 328 706 719 041 649 271 111 468 503 598 188 858 967 036 751 264 960 265 467 362 335 321 690 953 \
 661 518 783 117 527 999 885 653 399 824 835 208 160 243 553 949 918 535 424 248 356 856 620 142 592 \
  $q^{9208}$  -

625 115 224 227 707 606 125 900 267 992 856 540 539 587 832 098 081 721 589 519 831 001 080 081 146 \
 630 880 667 367 518 192 837 881 014 519 939 651 877 227 681 383 925 146 740 196 854 729 731 730 332 \
 324 795 066 347 203 349 908 562 337 644 365 934 615 326 319 677 016 141 362 237 590 451 826 688 000 \
  $q^{9209}$  +

680 494 922 581 049 945 075 985 364 975 489 987 068 867 448 996 409 264 959 178 732 562 219 939 681 \
 794 888 155 921 188 223 971 947 323 400 386 290 833 690 888 693 910 853 590 714 801 520 612 756 901 \
 990 130 766 743 555 793 629 986 152 460 686 905 372 933 871 274 117 835 656 376 765 939 399 118 848 \
  $q^{9212}$  -

700 022 225 183 693 439 739 293 389 800 206 342 000 607 731 493 999 147 253 688 360 976 999 004 191 \
 545 564 728 986 110 074 567 930 114 175 916 481 440 238 061 409 652 530 797 639 292 832 535 686 670 \
 929 334 865 720 365 844 087 825 256 922 684 107 140 265 793 313 981 708 594 733 319 290 413 127 163

$q^{9213} +$   
 762 024 009 186 287 052 559 815 640 814 204 957 318 999 692 134 196 222 377 611 376 782 715 378 809  
 425 943 538 689 187 654 854 823 844 966 459 790 268 311 520 297 388 433 763 058 559 991 905 084 009  
 399 180 688 098 845 712 720 496 397 247 496 500 366 279 533 546 606 680 016 207 186 200 535 498 752

$q^{9216} -$   
 783 886 045 061 606 870 107 835 542 805 815 571 967 860 386 129 825 719 477 909 592 185 698 974 758  
 030 751 583 537 985 300 518 564 966 189 301 446 445 377 140 825 053 585 602 143 527 753 745 074 449  
 241 100 669 782 519 615 760 421 486 566 291 367 433 915 665 184 845 157 705 548 881 023 372 165 120

$q^{9217} +$   
 853 300 062 528 018 172 452 056 635 048 483 535 070 500 948 803 956 991 246 682 435 522 029 736 885  
 013 095 813 680 725 030 706 437 805 620 055 851 603 788 855 740 270 896 795 869 878 782 581 695 353  
 490 047 193 223 845 096 987 449 517 101 157 794 425 282 235 150 320 753 006 030 028 129 806 745 600

$q^{9220} -$   
 877 775 380 764 097 689 424 679 937 173 662 266 777 161 107 554 057 554 353 876 043 080 227 671 043  
 519 503 561 353 503 218 808 773 841 780 158 461 118 616 153 424 613 176 401 912 686 572 215 200 599  
 048 394 214 341 557 279 386 134 670 419 668 276 915 082 563 862 244 534 795 764 143 548 873 502 500

$q^{9221} +$   
 955 485 858 263 252 549 405 597 547 211 539 645 347 836 331 045 819 993 927 018 414 311 467 861 816  
 870 461 537 001 397 858 636 527 168 513 967 474 458 748 029 630 345 397 517 887 754 129 711 421 432  
 945 386 271 048 591 520 289 293 462 343 123 188 896 943 679 294 508 458 691 579 836 873 902 080 000

$q^{9224} -$   
 982 886 169 587 016 665 491 489 563 548 196 966 337 647 063 907 595 106 459 628 241 319 184 362 165  
 337 705 056 481 444 750 158 173 934 848 271 535 914 100 782 487 033 815 709 060 292 596 401 574 592  
 713 377 948 442 685 589 876 356 784 802 692 734 860 983 647 568 445 018 384 552 197 490 227 609 600

$q^{9225} +$   
 1 069 882 589 944 447 610 340 314 917 362 381 824 866 418 106 355 629 413 866 024 118 718 892 666 718  
 505 116 356 111 041 318 590 669 232 093 571 996 550 425 087 972 251 919 470 098 445 758 883 229 815  
 527 068 440 218 838 300 191 600 635 415 192 078 432 073 298 400 975 490 273 406 533 178 031 702 016

$q^{9228} -$   
 1 100 556 706 214 646 516 603 946 722 246 891 974 477 681 020 786 506 688 647 241 793 356 145 781 611  
 855 494 036 875 623 846 021 852 391 674 090 237 142 141 963 119 447 826 790 602 087 390 816 542 394  
 389 278 169 368 762 494 408 111 599 954 692 584 540 758 720 305 671 355 309 565 011 185 797 278 500

$q^{9229} +$   
 1 197 946 311 174 667 310 243 968 113 067 164 194 923 310 886 752 326 056 712 265 927 411 206 034 345  
 957 512 340 585 772 715 249 762 946 083 035 125 266 360 810 374 352 513 083 425 749 337 355 929 496  
 153 408 754 283 567 793 525 125 555 018 193 222 961 039 847 038 158 890 500 382 956 192 373 932 032

$q^{9232} -$   
 1 232 284 551 872 954 916 473 478 601 036 171 896 628 801 910 732 810 468 740 666 843 423 419 513 964  
 189 032 468 247 965 260 793 706 460 420 782 548 643 311 407 173 926 911 359 994 294 507 227 967 047  
 788 014 297 012 306 941 050 466 560 671 631 498 914 581 998 973 761 576 307 439 303 239 378 599 936

$q^{9233} +$   
 1 341 306 326 690 588 469 107 249 040 116 415 698 575 810 698 304 298 993 389 092 526 558 123 137 690  
 078 716 624 892 751 171 622 638 783 423 551 848 646 995 989 495 677 919 112 417 036 248 971 426 391  
 556 964 915 358 566 068 789 286 585 971 410 097 627 998 575 381 500 028 157 959 204 335 218 944 000

$q^{9236} -$   
 1 379 745 447 651 583 203 115 164 144 374 006 650 253 278 618 703 791 653 629 627 012 436 205 643 549  
 991 288 129 983 308 974 756 391 688 461 839 986 151 386 459 409 354 137 580 529 077 709 255 651 993  
 062 807 616 896 013 593 795 788 133 405 055 295 827 585 128 043 333 755 134 258 302 502 833 724 373

$q^{9237} +$   
 1 501 785 762 890 711 717 727 551 246 240 922 514 984 549 908 195 390 069 926 921 977 775 391 565 125  
 304 185 146 211 448 470 989 746 595 240 484 827 712 610 671 039 457 830 895 186 938 635 753 811 227  
 787 772 875 119 226 184 501 002 697 415 710 297 263 081 649 727 320 861 339 210 278 274 664 857 600

$q^{9240} -$   
 1 544 814 469 032 373 176 371 672 275 972 238 772 831 277 370 157 426 240 356 921 727 975 317 565 836  
 131 693 381 240 791 703 396 087 761 572 168 919 342 728 781 880 990 546 183 080 770 661 646 450 183

326 132 308 458 967 647 688 824 876 459 009 286 645 520 602 466 092 641 141 066 120 022 790 144 000  
 $q^{9241} +$   
 1 681 424 575 533 260 770 424 534 578 478 364 034 029 904 286 402 602 304 896 944 540 662 513 939 779 \ \backslash  
 582 409 575 668 435 889 762 610 426 407 470 845 227 511 012 663 329 974 640 840 107 093 875 587 388 \ \backslash  
 891 136 797 509 450 743 854 193 194 179 383 018 862 557 371 947 112 667 636 755 546 276 249 856 000  
 $q^{9244} -$   
 1 729 589 686 637 368 790 636 721 617 402 217 271 799 803 593 277 202 043 308 281 614 959 574 075 403 \ \backslash  
 678 272 649 685 071 643 917 496 673 313 091 344 896 506 486 696 435 033 454 188 016 982 799 336 974 \ \backslash  
 574 239 928 379 584 649 632 638 342 802 175 949 775 943 587 553 364 470 337 698 626 246 104 425 255  
 $q^{9245} +$   
 1 882 505 282 739 681 527 439 836 148 257 796 197 663 731 025 383 394 006 053 215 033 200 450 121 840 \ \backslash  
 515 173 365 669 953 441 853 776 297 134 917 524 240 799 137 734 881 305 199 014 229 302 864 407 868 \ \backslash  
 479 618 460 550 156 870 185 497 132 997 203 232 162 637 745 196 899 218 792 182 183 272 843 081 728  
 $q^{9248} -$   
 1 936 418 629 478 930 865 802 743 303 162 092 264 673 250 684 518 213 567 680 089 345 024 751 272 051 \ \backslash  
 557 730 147 563 360 933 719 365 105 056 156 625 770 911 445 534 791 377 753 425 327 507 488 644 824 \ \backslash  
 590 606 298 257 519 808 232 778 652 260 505 580 359 413 256 720 970 549 956 696 080 061 599 744 000  
 $q^{9249} +$   
 2 107 581 745 431 959 635 865 352 873 214 168 042 523 587 503 892 258 963 217 694 551 018 574 861 583 \ \backslash  
 551 584 022 906 885 163 642 706 545 011 697 066 805 632 116 601 708 703 283 396 359 838 638 863 877 \ \backslash  
 362 772 130 429 864 807 048 481 184 186 657 634 323 113 701 052 814 072 851 035 260 757 875 687 424  
 $q^{9252} -$   
 2 167 927 881 946 036 423 780 200 922 904 785 425 187 993 865 632 803 542 061 593 232 353 408 307 928 \ \backslash  
 908 281 241 021 439 294 560 172 886 517 961 223 872 730 400 449 731 909 684 210 949 561 035 608 415 \ \backslash  
 921 825 581 255 941 362 347 654 041 828 229 001 880 054 877 061 304 741 573 309 032 604 221 235 943  
 $q^{9253} +$   
 2 359 511 355 325 902 426 387 481 801 426 862 574 204 519 651 090 063 304 601 274 539 455 208 053 127 \ \backslash  
 264 937 395 630 935 573 711 115 705 670 603 512 772 594 131 696 402 904 042 213 120 715 235 348 803 \ \backslash  
 564 404 228 570 313 370 852 067 684 429 320 941 382 756 551 555 691 816 179 661 818 975 393 920 000  
 $q^{9256} -$   
 2 427 056 184 826 566 319 848 940 688 542 128 214 794 091 312 108 334 045 862 413 367 550 449 332 611 \ \backslash  
 994 028 052 813 597 953 869 624 362 822 005 525 787 871 671 139 358 083 614 473 198 621 306 181 209 \ \backslash  
 194 709 585 218 531 186 751 090 259 364 050 509 308 580 532 571 645 474 208 101 026 677 799 845 888  
 $q^{9257} +$   
 2 641 491 033 068 149 520 041 110 694 017 221 536 471 130 080 763 131 291 397 759 977 542 386 879 460 \ \backslash  
 033 767 898 468 061 046 886 923 498 563 762 511 223 229 097 531 499 888 151 226 469 978 003 181 440 \ \backslash  
 041 687 945 840 135 429 509 130 628 850 579 028 861 555 097 132 775 271 100 056 012 048 161 612 800  
 $q^{9260} -$   
 2 717 091 454 328 695 654 837 756 480 953 472 358 286 757 709 489 702 806 644 550 969 826 119 282 316 \ \backslash  
 875 881 766 887 525 819 647 702 880 466 134 987 369 696 864 632 630 005 087 492 889 792 850 705 555 \ \backslash  
 094 104 970 168 569 913 181 034 294 349 195 130 526 024 797 105 621 633 793 605 500 202 615 073 375  
 $q^{9261} +$   
 2 957 097 486 567 158 309 367 451 693 233 695 106 830 536 958 891 637 305 883 727 897 936 601 729 975 \ \backslash  
 124 111 253 074 857 428 730 349 247 012 575 356 891 962 878 155 885 038 362 480 216 809 180 841 636 \ \backslash  
 307 220 248 853 353 009 732 187 154 551 608 927 431 995 260 589 061 336 702 462 999 076 847 616 000  
 $q^{9264} -$   
 3 041 712 181 865 317 935 438 834 030 373 014 574 591 346 002 194 732 434 025 931 015 616 472 998 738 \ \backslash  
 971 369 451 287 377 946 330 441 815 491 456 193 957 499 171 887 280 976 869 510 745 647 826 899 117 \ \backslash  
 976 566 408 124 758 200 734 224 247 006 478 540 218 461 677 197 056 477 625 349 424 536 010 752 000  
 $q^{9265} +$   
 3 310 332 232 614 475 130 545 361 430 658 273 600 032 731 353 387 615 386 730 071 615 219 327 179 346 \ \backslash  
 767 339 752 992 971 044 871 300 726 328 457 822 457 835 016 402 914 071 135 863 650 254 510 628 231 \ \backslash  
 201 410 175 905 896 546 546 323 387 987 595 637 396 105 155 867 868 421 277 669 909 067 262 664 704  
 $q^{9268} -$   
 3 405 033 731 906 955 316 513 535 893 361 756 540 798 294 198 808 055 420 886 774 148 649 876 253 301 \ \backslash

430 432 213 516 044 091 813 213 624 553 000 304 061 210 442 829 316 571 586 992 860 619 352 473 968  
 836 301 648 430 704 672 645 821 011 636 280 896 650 468 970 164 201 794 240 064 051 065 723 298 125  
 $q^{9269} +$   
 3 705 671 944 177 713 641 347 124 212 166 858 808 667 352 673 951 360 965 591 619 439 388 865 565 021  
 516 206 888 986 811 124 192 360 658 667 529 303 730 008 206 278 415 027 934 317 275 209 175 380 688  
 521 197 124 685 784 460 275 052 185 976 438 310 335 988 816 916 153 209 704 695 889 908 943 881 216  
 $q^{9272} -$   
 3 811 660 116 164 703 917 655 800 618 589 582 702 071 131 628 573 177 955 789 650 426 179 130 821 845  
 427 749 641 627 255 530 023 036 384 619 035 927 166 882 738 585 860 806 465 034 431 434 703 000 119  
 538 394 002 197 528 036 334 455 844 109 774 142 445 901 337 831 226 775 536 086 653 768 218 443 776  
 $q^{9273} +$   
 4 148 124 752 003 063 701 864 758 993 032 551 636 202 745 806 504 267 205 720 911 528 752 738 867 429  
 867 080 203 043 028 269 882 840 040 461 225 278 246 574 229 034 307 091 395 248 507 603 000 022 932  
 579 232 328 111 814 925 900 451 895 717 943 871 180 126 598 860 135 395 112 925 687 220 705 024 000  
 $q^{9276} -$   
 4 266 741 890 488 238 982 947 494 597 088 521 872 458 911 821 003 121 533 361 588 740 832 813 255 217  
 338 546 379 825 411 385 782 823 686 907 910 394 835 200 232 600 114 458 595 342 503 194 347 280 059  
 713 413 011 769 214 598 516 770 021 647 283 821 835 534 870 700 719 371 334 399 322 314 613 155 688  
 $q^{9277} +$   
 4 643 293 203 210 848 640 365 633 153 842 038 897 885 756 379 744 005 198 031 343 560 444 761 138 489  
 398 571 251 622 564 048 077 816 032 763 367 676 706 508 386 175 926 880 573 727 439 569 578 581 934  
 224 117 063 117 137 388 807 910 518 255 130 119 677 663 250 512 883 978 047 051 647 200 840 908 800  
 $q^{9280} -$   
 4 776 040 896 995 722 915 434 015 596 225 365 605 789 199 199 936 800 873 638 786 329 213 339 820 779  
 365 056 997 346 993 398 969 039 165 465 046 076 282 014 995 235 538 425 382 063 683 283 613 772 696  
 660 002 262 640 397 989 729 832 139 346 557 657 230 350 527 286 989 093 737 564 093 949 902 848 000  
 $q^{9281} +$   
 5 197 444 662 316 416 603 095 623 918 779 601 711 389 699 739 993 465 583 257 684 948 910 137 571 673  
 689 415 563 718 249 751 186 982 407 380 104 134 424 660 422 147 280 437 815 435 886 210 440 380 690  
 937 409 847 058 265 673 360 708 949 157 445 249 626 413 647 702 989 020 587 429 155 639 646 208 000  
 $q^{9284} -$   
 5 346 002 659 032 045 093 950 333 426 998 719 908 107 793 081 456 655 506 939 599 967 019 295 941 537  
 241 013 682 683 633 147 366 064 529 089 884 489 471 316 042 184 468 210 192 170 744 630 620 339 290  
 818 702 806 464 004 324 046 630 081 727 702 445 455 445 733 505 348 400 274 456 566 825 182 537 425  
 $q^{9285} +$   
 5 817 590 032 581 242 585 355 968 119 909 598 477 096 075 859 060 503 361 919 836 534 569 985 953 875  
 814 320 676 681 303 161 778 476 317 224 262 689 704 936 626 537 303 248 985 779 651 061 152 435 158  
 760 493 801 445 044 164 651 366 141 928 777 158 071 740 380 641 198 922 292 153 137 508 068 130 816  
 $q^{9288} -$   
 5 983 837 331 628 566 317 200 855 203 759 018 218 458 717 357 349 372 041 294 969 407 716 869 083 273  
 072 315 781 302 719 057 442 348 025 415 791 091 849 448 600 585 217 912 373 161 921 386 661 038 524  
 198 379 964 987 281 101 393 287 020 977 778 360 406 648 944 411 224 070 343 212 801 803 395 072 000  
 $q^{9289} +$   
 6 511 571 778 935 746 442 562 438 215 748 670 666 167 854 608 161 133 633 303 094 427 278 119 862 132  
 262 592 477 916 599 219 379 637 710 488 265 768 524 847 860 830 199 842 101 475 350 971 054 610 776  
 580 746 123 274 791 960 583 959 800 218 959 706 039 097 353 616 875 687 497 776 013 927 463 792 640  
 $q^{9292} -$   
 6 697 610 216 383 643 178 113 528 743 128 615 186 938 950 863 971 502 215 777 571 560 471 562 212 081  
 943 065 530 435 874 658 635 042 057 283 531 344 549 939 845 914 455 436 478 075 529 324 997 482 807  
 372 233 381 697 029 411 448 286 329 599 007 660 120 601 028 518 618 148 348 481 089 203 008 707 914  
 $q^{9293} +$   
 7 288 162 349 189 630 248 586 432 536 500 864 928 549 308 007 479 155 726 541 161 353 931 989 622 460  
 938 989 640 643 352 979 806 371 947 378 828 425 400 775 108 576 081 681 521 082 211 768 516 940 924  
 942 088 611 250 888 115 981 183 545 116 285 950 386 097 631 053 733 034 919 635 584 357 928 960 000  
 $q^{9296} -$

7 496 342 968 408 020 967 690 578 180 659 431 848 811 536 642 493 026 493 783 464 326 178 882 803 385 \\  
 458 643 606 051 530 148 427 786 600 038 761 557 552 865 815 026 017 992 555 834 804 625 304 024 779 \\  
 673 633 388 993 346 748 859 913 101 417 753 696 729 412 344 697 581 145 748 132 671 283 862 142 976 \\  
 $q^{9297} +$

8 157 174 219 280 132 131 463 203 839 176 783 665 494 205 017 673 641 524 368 787 246 677 178 444 400 \\  
 348 981 395 595 177 770 864 159 537 006 237 871 469 569 132 664 726 267 529 487 418 873 316 901 160 \\  
 133 227 889 119 217 720 111 927 262 796 550 792 116 980 369 672 515 878 883 540 282 025 619 763 200 \\  
 $q^{9300} -$

8 390 126 755 645 225 150 083 825 855 755 798 737 901 080 980 864 378 733 689 682 191 606 854 728 196 \\  
 770 315 987 090 670 301 069 111 805 503 427 267 326 884 191 212 623 956 976 296 155 303 513 949 122 \\  
 881 243 543 183 619 063 447 063 731 727 468 189 890 264 607 709 660 803 007 797 915 717 783 246 000 \\  
 $q^{9301} +$

9 129 582 932 492 497 210 366 521 484 111 925 627 295 378 453 435 192 118 520 552 771 638 067 939 526 \\  
 396 690 064 672 572 501 669 769 677 399 044 402 025 607 388 357 466 604 125 209 569 583 534 604 089 \\  
 039 340 069 213 154 311 453 736 398 588 543 242 768 357 123 106 642 442 620 029 913 766 066 752 000 \\  
 $q^{9304} -$

9 390 248 779 117 912 104 614 805 133 584 449 971 621 965 372 978 260 969 340 603 089 935 020 874 889 \\  
 377 151 521 064 601 891 076 773 889 298 891 143 236 959 018 427 091 469 083 479 386 878 496 807 140 \\  
 149 510 790 153 710 586 380 677 036 562 054 136 113 995 835 713 980 796 294 792 256 447 356 928 000 \\  
 $q^{9305} +$

10 217 664 663 695 000 228 930 031 266 674 830 297 961 945 354 617 591 229 374 050 341 410 480 100 \\  
 402 576 219 348 586 486 657 931 030 635 599 208 958 129 539 487 371 642 841 411 791 603 589 464 360 \\  
 862 008 224 763 334 253 949 403 240 221 637 151 892 315 372 677 863 033 271 931 251 290 479 343 679 \\  
 488  $q^{9308} -$

10 509 333 728 291 325 812 594 091 584 353 301 125 471 430 715 979 996 652 797 926 869 814 350 680 \\  
 292 124 227 558 000 719 337 226 480 323 994 315 802 724 636 622 015 875 810 524 394 495 071 376 312 \\  
 701 095 717 931 311 122 294 495 973 573 745 864 330 720 575 448 390 210 323 490 209 612 030 651 581 \\  
 625  $q^{9309} +$

11 435 150 019 645 326 943 536 077 840 600 121 859 833 485 358 973 132 449 225 341 179 718 224 976 \\  
 466 971 999 812 650 959 060 917 146 814 584 054 251 669 739 589 729 413 618 717 699 239 107 725 381 \\  
 107 893 708 910 213 544 184 850 671 489 444 603 206 516 399 669 476 948 391 380 301 503 610 398 507 \\  
 008  $q^{9312} -$

11 761 501 930 822 405 526 600 406 383 101 404 958 823 393 817 111 310 091 716 449 080 183 501 404 \\  
 200 731 923 076 116 389 088 009 616 341 644 273 571 352 328 781 142 837 615 831 080 519 037 819 755 \\  
 628 649 354 285 271 300 087 255 060 888 675 613 280 488 959 903 568 649 663 216 224 472 420 316 250 \\  
 112  $q^{9313} +$

12 797 395 987 560 032 507 417 482 662 287 984 654 947 106 388 350 183 243 758 961 718 318 460 492 \\  
 060 029 225 103 173 264 498 105 001 936 980 229 750 590 353 909 276 502 813 450 191 566 232 186 133 \\  
 857 394 369 875 689 027 151 454 602 726 008 183 340 242 314 748 265 089 984 987 896 747 365 253 120 \\  
 000  $q^{9316} -$

13 162 546 162 753 728 781 795 281 490 595 138 606 565 492 060 783 151 052 635 973 521 382 140 502 \\  
 072 542 269 054 296 093 975 109 322 844 308 400 902 699 297 983 446 574 995 709 300 946 188 947 772 \\  
 900 621 651 884 758 028 727 593 059 324 344 668 331 743 361 389 590 691 924 688 932 465 209 690 181 \\  
 997  $q^{9317} +$

14 321 578 168 866 860 059 063 309 589 055 729 397 164 146 146 720 305 810 781 504 588 236 062 458 \\  
 975 758 893 037 996 509 263 601 404 172 833 548 457 811 455 880 638 686 102 172 182 035 720 278 592 \\  
 314 583 425 471 642 077 252 752 381 156 018 559 275 562 746 422 978 365 609 210 977 709 881 032 320 \\  
 000  $q^{9320} -$

14 730 129 316 257 331 293 406 137 837 093 503 872 529 357 062 507 240 328 702 507 486 852 971 313 \\  
 869 981 343 313 988 248 868 035 303 555 143 397 240 619 705 704 158 411 623 787 489 753 744 184 462 \\  
 866 778 843 281 547 580 810 815 284 206 843 190 142 921 633 729 047 622 337 054 059 785 779 208 192 \\  
 000  $q^{9321} +$

16 026 905 686 142 519 007 850 313 591 325 956 377 242 565 461 697 599 637 092 345 582 210 009 902 \\  
 765 380 783 666 445 174 113 255 629 130 148 131 996 794 149 703 862 603 755 435 131 517 930 662 027 \\  
 094 057 565 780 097 034 499 516 474 094 707 899 218 723 351 467 228 915 069 364 609 461 551 678 720 \

$000 q^{9324} -$   
 16 484 005 380 173 454 916 714 782 612 106 568 933 345 404 427 104 238 509 578 657 423 526 671 935 \\  
 718 886 187 390 496 628 360 397 457 564 543 488 516 353 065 815 681 114 245 010 217 452 054 891 271 \\  
 142 683 532 667 069 233 277 435 602 055 864 519 967 444 042 923 878 538 171 452 884 417 050 946 162 \\  
 $525 q^{9325} +$   
 17 934 861 431 760 247 975 281 272 890 923 979 429 431 567 061 361 963 395 385 088 157 337 418 391 \\  
 139 842 557 830 857 575 781 385 183 021 012 340 783 038 231 791 514 723 635 650 245 734 053 467 873 \\  
 361 915 336 794 271 332 977 194 286 098 763 098 896 464 137 939 550 369 839 464 516 431 512 629 329 \\  
 $920 q^{9328} -$   
 18 446 266 476 993 946 551 581 969 648 278 293 396 011 606 647 165 946 298 466 244 502 007 003 808 \\  
 444 680 333 696 709 998 266 610 558 122 645 938 752 164 265 349 580 477 124 700 126 310 856 945 163 \\  
 207 951 512 913 399 992 440 838 610 339 239 874 724 889 096 016 001 879 897 208 371 194 939 658 240 \\  
 $000 q^{9329} +$   
 20 069 470 640 176 435 883 694 107 882 478 586 167 903 987 159 623 223 186 369 846 506 961 298 863 \\  
 859 342 435 094 362 735 694 929 502 014 269 535 493 338 687 392 402 502 912 323 386 158 403 524 758 \\  
 906 488 804 786 522 158 933 107 627 137 143 602 805 722 181 963 276 706 665 513 184 492 796 908 193 \\  
 $792 q^{9332} -$   
 20 641 619 022 150 093 567 341 314 968 102 970 457 685 670 149 631 939 175 557 890 407 239 555 061 \\  
 425 542 453 365 035 047 513 961 637 263 545 465 019 398 577 145 948 213 433 381 180 135 909 813 900 \\  
 337 467 915 139 855 755 405 496 586 287 276 923 800 184 811 713 182 246 945 042 209 377 901 309 048 \\  
 $242 q^{9333} +$   
 22 457 601 115 920 184 508 373 407 291 455 641 939 007 842 877 745 200 937 590 575 532 643 433 579 \\  
 208 005 593 362 464 761 420 213 815 786 223 679 093 712 353 670 525 670 571 497 752 904 555 999 169 \\  
 283 891 910 022 585 715 310 971 468 457 166 465 054 006 364 408 165 366 180 808 401 546 739 279 232 \\  
 $000 q^{9336} -$   
 23 097 692 431 434 221 785 656 708 212 480 650 574 551 494 890 422 394 373 027 653 833 347 418 249 \\  
 921 067 181 928 131 560 294 310 249 803 392 732 531 495 875 658 288 288 245 761 038 438 225 134 604 \\  
 997 298 327 385 860 115 471 319 543 679 085 173 705 340 476 083 243 672 170 481 117 446 689 331 642 \\  
 $368 q^{9337} +$   
 25 129 298 840 509 377 902 550 264 670 208 195 441 709 788 689 492 015 421 811 756 944 796 703 738 \\  
 523 149 388 779 088 292 705 164 662 499 676 165 927 520 128 611 290 591 469 725 732 770 823 071 648 \\  
 532 260 766 186 895 702 330 903 471 008 440 948 236 159 219 057 751 849 130 488 267 814 726 791 936 \\  
 $000 q^{9340} -$   
 25 845 384 204 528 999 420 034 487 051 706 068 320 757 949 962 859 407 171 505 811 353 135 085 802 \\  
 196 841 850 606 991 663 032 494 147 696 378 824 451 953 791 079 002 387 059 737 508 561 167 776 351 \\  
 358 553 269 827 284 664 260 916 031 280 695 532 739 043 183 214 721 063 100 767 694 260 298 067 480 \\  
 $125 q^{9341} +$   
 28 118 163 118 498 256 990 353 097 050 245 302 646 630 933 900 869 969 741 160 866 533 813 186 089 \\  
 709 673 848 900 599 429 013 144 194 722 592 728 405 110 682 159 637 434 117 358 475 870 737 391 299 \\  
 234 207 255 619 825 617 188 841 175 660 695 971 536 619 785 368 156 687 331 793 504 375 893 671 936 \\  
 $000 q^{9344} -$   
 28 919 245 661 868 948 494 276 987 003 963 894 198 052 229 455 050 595 306 117 913 590 832 526 623 \\  
 455 375 881 199 576 271 987 574 516 377 319 268 184 262 684 137 378 063 611 514 614 224 941 864 568 \\  
 270 113 818 395 769 853 920 508 605 183 017 244 829 577 122 022 611 096 259 710 214 766 597 360 844 \\  
 $800 q^{9345} +$   
 31 461 765 911 021 000 344 810 622 253 237 370 376 198 188 361 971 783 009 951 211 926 481 589 828 \\  
 150 816 520 182 739 286 095 322 300 240 162 109 871 213 813 954 137 011 182 606 339 908 758 125 750 \\  
 472 316 867 450 066 034 697 598 052 036 806 238 248 733 213 510 211 763 364 207 701 316 306 590 105 \\  
 $600 q^{9348} -$   
 32 357 913 113 921 292 384 527 806 469 368 352 890 070 434 606 964 638 585 381 285 953 052 532 968 \\  
 968 072 464 849 732 405 483 173 440 570 384 972 277 168 333 184 719 179 220 865 193 294 119 061 268 \\  
 634 806 263 236 790 224 268 217 746 017 000 025 622 478 822 885 197 763 640 153 939 463 138 465 150 \\  
 $875 q^{9349} +$   
 35 202 120 550 514 500 428 069 238 853 692 406 584 560 073 690 612 485 436 612 437 311 265 991 304 \\  
 193 574 414 629 371 375 702 649 914 746 609 331 557 620 473 795 749 836 428 049 655 428 434 625 305 \

967 670 873 090 297 958 603 456 330 095 912 905 014 043 847 985 806 570 405 835 707 895 817 945 053 \\  
 184  $q^{9352}$  -  
 36 204 589 802 596 328 297 746 364 689 237 072 990 981 459 156 508 354 561 082 217 001 752 607 169 \\  
 280 647 854 199 831 895 743 521 203 042 113 898 669 218 917 681 705 752 338 283 740 046 334 233 804 \\  
 701 460 249 372 635 842 944 910 860 088 760 069 987 629 974 634 185 943 055 995 100 180 291 236 069 \\  
 376  $q^{9353}$  +  
 39 386 205 639 460 036 576 508 372 272 999 593 438 209 077 059 720 077 161 993 031 872 771 931 491 \\  
 848 042 868 386 582 661 174 614 453 502 097 755 722 686 988 493 770 643 332 468 098 581 093 975 198 \\  
 029 042 210 939 676 289 407 898 689 596 637 405 797 838 453 335 835 837 524 071 771 833 864 545 984 \\  
 000  $q^{9356}$  -  
 40 507 584 580 746 358 191 507 127 039 659 401 434 590 283 754 308 624 539 127 996 718 862 063 514 \\  
 166 013 711 493 012 504 673 314 545 237 369 123 904 663 573 777 353 365 572 451 314 308 825 592 424 \\  
 214 808 347 482 035 774 259 181 170 566 613 014 368 586 051 452 980 038 584 473 695 613 453 536 128 \\  
 237  $q^{9357}$  +  
 44 066 550 616 435 215 610 261 433 973 149 402 660 878 758 015 227 738 910 674 223 013 885 840 392 \\  
 689 648 497 375 873 333 756 494 966 316 259 087 643 263 918 019 185 260 917 475 570 766 279 428 433 \\  
 005 022 661 995 961 579 445 228 820 776 496 129 166 268 470 623 357 718 493 190 092 750 647 558 144 \\  
 000  $q^{9360}$  -  
 45 320 913 995 252 613 488 343 646 693 112 271 042 704 449 438 784 112 958 816 999 881 564 874 595 \\  
 754 873 965 915 904 408 648 256 151 230 480 090 555 238 976 537 333 479 747 227 061 818 167 209 590 \\  
 395 359 834 284 092 698 005 140 132 400 849 431 461 469 922 933 599 495 337 050 510 359 481 606 144 \\  
 000  $q^{9361}$  +  
 49 301 890 232 841 007 128 219 789 350 154 201 780 195 961 615 753 329 084 533 778 604 618 985 712 \\  
 870 319 637 817 618 498 793 419 538 526 040 356 747 312 864 882 907 827 339 082 318 078 870 462 220 \\  
 641 989 831 553 272 496 212 552 676 185 373 517 011 229 582 355 258 363 423 624 180 958 196 504 320 \\  
 000  $q^{9364}$  -  
 50 704 975 220 590 883 810 251 968 241 489 005 321 154 515 328 832 099 772 098 384 532 676 405 963 \\  
 476 711 731 403 278 863 981 190 162 279 167 905 952 765 392 963 418 379 230 997 301 089 860 266 250 \\  
 555 099 641 418 965 434 047 416 774 377 935 743 038 710 008 310 445 271 054 302 805 809 628 794 784 \\  
 300  $q^{9365}$  +  
 55 157 896 032 660 985 678 251 384 515 418 613 691 895 578 056 718 403 351 481 631 789 284 367 474 \\  
 815 016 101 426 665 945 112 506 368 041 377 614 641 321 005 308 387 976 496 221 284 490 959 059 071 \\  
 003 937 040 426 634 476 932 097 021 723 639 834 914 454 105 675 467 211 942 252 295 225 076 920 749 \\  
 568  $q^{9368}$  -  
 56 727 298 162 565 500 029 628 462 946 679 567 308 927 649 031 140 217 353 591 453 050 122 503 102 \\  
 878 189 076 637 509 778 508 291 629 377 461 052 224 647 984 720 603 397 937 335 514 700 504 173 038 \\  
 869 183 799 915 140 785 012 286 767 392 269 049 209 155 950 612 743 435 638 840 006 484 116 750 336 \\  
 000  $q^{9369}$  +  
 61 707 993 875 901 317 380 672 278 930 271 848 624 910 280 955 034 758 704 630 214 478 611 621 638 \\  
 851 372 715 771 272 539 695 524 070 973 086 505 597 702 395 398 516 491 521 485 038 924 683 682 476 \\  
 656 206 313 426 563 824 626 741 625 064 413 746 133 925 083 499 192 222 277 360 592 430 774 387 634 \\  
 176  $q^{9372}$  -  
 63 463 386 026 778 192 184 343 353 447 874 700 191 424 605 999 560 855 437 454 591 013 028 230 933 \\  
 798 595 002 081 177 723 203 413 598 842 411 357 433 902 220 329 703 343 586 071 622 736 142 772 584 \\  
 437 617 014 121 773 737 661 352 511 281 882 728 578 605 892 495 102 975 469 070 097 539 916 295 986 \\  
 491  $q^{9373}$  +  
 69 034 277 605 540 126 970 832 007 931 292 405 231 476 024 479 886 537 489 789 406 473 120 245 113 \\  
 050 499 172 483 439 840 709 367 236 500 279 856 086 197 227 119 492 180 408 680 293 965 768 451 178 \\  
 413 700 844 512 234 116 417 295 922 074 292 300 936 961 662 120 797 051 824 027 973 303 822 078 464 \\  
 000  $q^{9376}$  -  
 70 997 654 735 266 338 188 094 208 323 384 309 054 054 324 489 817 411 800 030 180 819 835 820 939 \\  
 324 787 732 687 972 699 771 188 521 084 468 065 153 305 644 046 161 741 896 386 551 157 552 128 057 \\  
 704 741 936 264 666 327 720 883 707 459 470 872 341 275 494 221 896 664 428 918 696 270 963 618 611 \\  
 200  $q^{9377}$  +  
 77 228 530 140 822 972 830 966 640 262 488 597 472 574 236 969 373 360 032 431 742 685 340 115 842 \

777 888 969 110 802 664 583 849 638 677 658 144 795 153 401 591 939 934 315 917 711 834 548 302 354 3  
 794 108 083 298 524 204 334 462 302 771 673 531 616 579 696 377 216 609 034 471 207 620 628 456 243 3  
 200  $q^{9380}$  -  
 79 424 482 790 904 841 238 297 411 455 822 479 820 427 319 169 548 498 356 529 602 832 606 978 224 3  
 074 029 024 235 683 166 333 134 898 817 525 460 112 522 493 334 946 861 417 954 589 415 943 572 119 3  
 384 534 960 517 209 888 560 226 872 605 138 394 088 715 917 825 524 245 519 460 212 561 370 678 984 3  
 125  $q^{9381}$  +  
 86 393 364 601 023 221 661 757 436 473 586 522 142 474 304 693 896 882 800 836 766 134 461 345 019 3  
 434 255 631 577 438 962 119 394 244 698 236 990 356 324 793 006 175 577 799 117 922 530 229 766 746 3  
 710 087 291 588 485 935 487 582 968 162 737 620 012 719 486 813 355 590 709 335 989 237 449 965 824 3  
 000  $q^{9384}$  -  
 88 849 384 547 466 565 084 290 897 290 013 729 214 648 755 479 105 284 598 900 835 302 171 697 495 3  
 868 192 246 555 223 412 335 480 049 261 654 736 609 600 217 193 963 423 022 997 647 510 343 276 669 3  
 110 595 703 567 849 325 983 301 486 451 536 906 081 634 830 254 165 923 729 027 690 757 232 425 369 3  
 600  $q^{9385}$  +  
 96 643 499 539 469 853 803 204 862 251 415 132 666 857 686 745 853 024 411 024 502 219 425 927 242 3  
 674 464 138 209 827 070 191 556 253 903 054 300 812 513 762 538 153 768 294 482 079 657 796 422 516 3  
 038 371 896 458 055 885 041 659 328 421 104 697 387 119 762 336 745 394 459 135 563 153 741 161 667 3  
 072  $q^{9388}$  -  
 99 390 321 360 255 733 477 691 798 676 406 739 451 689 532 676 706 506 127 208 654 546 452 732 535 3  
 182 657 422 420 322 558 424 241 729 613 466 688 153 920 586 936 451 228 786 251 460 020 615 770 123 3  
 156 730 704 833 885 112 861 124 213 225 207 786 099 121 905 980 527 568 800 134 347 653 905 415 510 3  
 625  $q^{9389}$  +  
 108 107 184 015 735 434 067 653 065 866 074 807 653 694 818 882 665 502 566 471 449 493 055 940 139 3  
 467 981 185 325 907 785 079 407 608 817 305 825 310 193 806 994 451 476 793 459 120 020 896 968 809 3  
 515 394 623 796 621 266 863 576 913 173 360 107 005 556 816 200 579 249 914 116 320 229 076 643 106 3  
 816  $q^{9392}$  -  
 111 179 166 786 474 148 036 852 817 571 718 738 153 826 994 751 045 804 772 928 919 211 433 677 607 3  
 489 595 854 364 556 596 230 324 301 396 866 807 688 806 936 308 823 079 002 757 415 815 592 268 559 3  
 877 972 555 011 911 486 324 416 464 305 350 826 376 149 178 828 411 743 600 441 626 312 752 460 201 3  
 984  $q^{9393}$  +  
 120 927 790 074 473 536 734 458 515 060 019 782 792 064 039 806 326 490 853 498 096 536 090 576 214 3  
 097 125 567 428 543 163 323 892 973 051 820 852 573 966 119 459 971 021 270 552 293 006 690 083 581 3  
 826 189 033 821 619 802 048 811 784 723 327 263 497 760 644 112 823 760 762 503 698 292 183 512 832 3  
 000  $q^{9396}$  -  
 124 363 343 896 612 120 143 388 587 553 882 492 805 709 278 463 215 272 901 870 591 798 264 597 151 3  
 214 551 684 685 617 472 374 901 611 427 104 798 881 991 214 312 069 779 507 333 509 978 431 189 178 3  
 784 423 280 550 098 670 905 391 439 335 881 941 350 273 881 662 909 132 027 614 697 356 264 164 924 3  
 596  $q^{9397}$  +  
 135 265 592 254 936 075 231 147 290 301 297 683 103 197 133 937 954 793 324 377 194 507 846 970 423 3  
 559 446 550 847 201 778 377 796 807 156 158 880 244 625 925 095 064 042 756 505 583 603 636 981 473 3  
 615 729 945 029 109 452 242 769 820 853 939 114 117 800 531 593 456 354 266 243 177 117 707 819 878 3  
 400  $q^{9400}$  -  
 139 107 654 871 238 745 145 237 116 957 472 389 277 843 806 408 378 678 908 713 032 447 946 622 331 3  
 669 801 943 113 038 029 986 152 867 721 715 197 091 337 297 527 165 711 857 210 378 783 563 429 138 3  
 008 112 592 338 684 946 946 743 516 932 061 701 312 031 455 801 035 521 702 816 904 350 500 782 080 3  
 000  $q^{9401}$  +  
 151 299 756 050 734 853 172 438 434 026 389 192 967 973 908 347 131 841 418 124 327 637 870 401 690 3  
 889 372 165 339 269 772 905 700 557 831 414 295 562 586 923 855 861 130 324 641 954 401 725 219 109 3  
 517 334 272 647 995 450 095 113 298 260 020 417 337 784 413 181 075 535 546 385 696 388 158 237 696 3  
 000  $q^{9404}$  -  
 155 596 325 417 346 151 731 700 106 707 311 635 503 956 972 668 397 440 067 211 647 005 022 948 344 3  
 816 695 957 565 379 335 217 204 675 410 061 344 439 664 501 262 478 387 805 798 095 086 426 969 602 3  
 722 759 192 192 106 712 365 632 804 032 108 964 538 812 242 965 699 111 211 455 523 628 315 921 325 3  
 875  $q^{9405}$  +

169 230 559 802 899 071 563 706 660 524 821 881 216 002 586 338 851 474 895 428 231 710 589 281 949 \\  
 100 397 224 251 384 976 960 716 465 663 579 919 701 195 353 800 773 340 681 193 463 029 973 782 240 \\  
 351 567 751 695 271 057 358 899 751 640 712 092 508 402 162 646 816 333 248 678 106 923 593 285 009 \\  
 408  $q^{9408}$  -

174 035 289 173 620 027 395 468 756 270 670 551 081 691 349 386 893 418 936 610 582 644 564 393 971 \\  
 992 156 170 205 401 182 052 659 004 796 477 851 915 912 026 348 490 142 782 705 893 132 491 078 748 \\  
 669 534 943 590 509 102 979 080 212 812 015 520 810 860 866 717 531 806 318 556 618 230 050 029 568 \\  
 248  $q^{9409}$  +

189 281 877 371 933 093 506 838 821 849 741 657 085 633 605 673 705 809 978 226 612 484 156 857 307 \\  
 270 211 135 945 140 820 045 215 369 128 436 249 479 448 494 099 658 522 694 539 134 844 463 266 922 \\  
 427 149 675 090 909 284 520 801 640 089 481 478 422 979 060 910 896 098 728 352 215 266 296 034 361 \\  
 344  $q^{9412}$  -

194 654 740 216 745 639 020 313 309 042 810 919 747 091 634 212 743 259 388 290 126 249 126 817 615 \\  
 161 037 391 893 756 361 149 342 836 988 383 944 999 860 447 339 133 347 488 421 648 649 495 802 959 \\  
 198 328 992 022 286 064 353 840 150 868 176 625 257 863 615 186 288 463 348 132 963 174 903 663 493 \\  
 258  $q^{9413}$  +

211 703 952 131 235 963 399 562 747 423 237 046 742 700 266 743 057 504 245 473 861 408 411 983 122 \\  
 509 075 405 456 448 551 520 741 569 436 729 692 188 785 288 153 314 671 251 919 563 277 970 919 240 \\  
 379 606 640 167 152 823 385 215 148 241 458 840 462 437 000 873 475 287 605 764 618 675 124 608 000 \\  
 000  $q^{9416}$  -

217 711 985 066 925 125 015 957 759 210 805 753 260 400 364 903 257 433 676 737 502 870 568 230 502 \\  
 805 946 032 095 449 430 047 304 098 927 638 205 605 165 250 184 362 120 540 095 585 934 156 607 671 \\  
 026 567 203 268 735 483 775 978 521 613 019 095 622 666 118 211 686 789 029 688 612 791 557 072 683 \\  
 008  $q^{9417}$  +

236 776 496 393 794 164 014 805 813 319 628 528 824 844 251 436 284 542 290 062 457 839 965 229 022 \\  
 902 728 750 736 660 369 594 343 983 997 808 673 012 083 753 793 417 687 104 832 664 173 022 116 403 \\  
 258 237 099 423 556 331 378 359 282 182 455 679 602 166 832 284 873 272 306 419 431 631 364 916 377 \\  
 600  $q^{9420}$  -

243 494 629 260 149 702 111 333 697 549 896 036 148 344 245 697 096 316 520 759 713 528 869 564 817 \\  
 032 169 425 427 182 619 608 710 228 616 659 171 633 178 437 734 183 505 737 929 098 661 068 652 113 \\  
 213 629 629 138 575 882 383 557 198 601 857 483 379 593 903 543 056 785 778 816 559 282 842 042 782 \\  
 375  $q^{9421}$  +

264 812 154 369 908 215 973 778 215 661 179 209 612 204 172 310 197 334 129 496 280 364 833 480 942 \\  
 710 318 130 255 289 311 252 457 870 851 810 567 117 998 006 995 822 172 529 080 390 831 605 634 948 \\  
 071 126 395 660 053 867 818 031 858 728 690 439 559 560 790 402 139 353 837 862 772 557 328 564 224 \\  
 000  $q^{9424}$  -

272 324 137 652 055 089 366 564 240 205 902 808 855 507 937 173 316 216 995 732 078 073 954 712 035 \\  
 097 193 616 771 563 854 156 032 713 745 672 008 893 495 747 419 812 981 444 119 609 798 459 961 829 \\  
 946 877 324 553 569 119 015 362 812 786 202 097 391 392 025 650 088 186 657 077 335 557 094 716 211 \\  
 200  $q^{9425}$  +

296 160 371 204 310 338 134 849 254 907 577 475 598 467 719 471 218 942 048 071 009 955 756 884 942 \\  
 232 119 457 405 634 487 868 542 392 766 700 335 672 806 255 452 482 631 370 931 450 361 773 820 210 \\  
 636 362 643 697 626 734 341 572 529 393 900 375 989 211 354 525 272 933 639 916 116 505 455 861 401 \\  
 600  $q^{9428}$  -

304 559 812 193 187 568 777 836 952 331 811 245 161 618 872 691 634 669 153 209 051 865 171 959 860 \\  
 118 815 528 835 341 071 146 292 223 207 170 760 295 649 375 628 566 969 226 196 357 538 994 219 475 \\  
 453 057 040 873 587 574 999 223 657 876 884 630 453 092 540 422 067 095 244 562 633 132 094 018 630 \\  
 000  $q^{9429}$  +

331 211 715 610 449 302 515 978 667 662 652 856 218 453 003 562 894 995 511 300 129 557 928 667 638 \\  
 715 062 998 526 926 672 180 930 805 352 348 907 129 044 667 062 297 903 475 962 726 297 574 895 213 \\  
 992 367 239 803 039 243 397 199 688 754 269 351 423 984 646 914 477 119 745 582 709 296 381 556 101 \\  
 632  $q^{9432}$  -

340 603 236 023 802 171 949 252 623 028 856 130 094 081 120 475 964 745 998 059 324 024 114 276 435 \\  
 833 114 692 169 161 750 299 732 726 476 662 296 195 170 495 657 367 764 996 725 463 515 988 460 354 \\  
 935 749 745 066 693 358 927 123 635 430 396 648 683 526 593 856 536 735 543 248 566 906 670 427 275 \

$264 q^{9433} +$   
 370 402 709 168 313 128 537 618 288 422 296 753 650 172 770 316 381 342 205 289 200 059 886 425 656 \ \backslash  
 269 426 103 660 096 321 091 316 674 476 130 747 642 954 139 069 002 140 262 661 542 935 169 508 930 \ \backslash  
 748 088 734 355 885 912 372 589 973 851 793 606 749 887 946 210 140 307 788 440 116 732 732 606 464 \ \backslash  
 $000 q^{9436} -$   
 380 903 238 439 936 955 600 141 726 592 227 021 447 532 392 230 498 426 609 221 292 896 202 703 357 \ \backslash  
 390 318 453 438 428 150 931 911 021 781 052 698 954 397 541 480 005 486 482 103 648 487 415 723 285 \ \backslash  
 396 959 863 951 145 291 479 836 071 205 086 080 353 522 270 090 076 466 084 436 283 811 186 352 279 \ \backslash  
 $451 q^{9437} +$   
 414 221 221 547 289 590 720 302 636 011 409 792 720 914 199 883 932 975 765 183 670 367 615 526 882 \ \backslash  
 991 474 263 005 578 769 914 039 649 256 862 681 202 744 753 054 299 526 087 774 571 798 234 579 619 \ \backslash  
 585 014 278 002 664 210 087 850 316 143 742 496 580 444 624 236 310 635 759 517 462 106 710 138 675 \ \backslash  
 $200 q^{9440} -$   
 425 961 441 650 692 222 625 376 046 481 540 321 699 844 524 144 771 922 829 620 315 420 454 297 187 \ \backslash  
 186 852 909 984 126 710 952 895 002 299 269 801 861 375 460 874 999 089 100 443 202 403 612 978 206 \ \backslash  
 343 314 311 525 681 858 665 281 954 431 239 334 202 485 876 772 241 154 235 154 779 742 413 377 536 \ \backslash  
 $000 q^{9441} +$   
 463 212 497 832 405 356 193 653 675 506 165 463 478 694 353 759 701 697 810 505 165 482 958 085 681 \ \backslash  
 183 470 554 150 879 190 739 862 905 562 704 566 501 884 417 868 218 868 151 802 171 880 579 477 121 \ \backslash  
 848 497 916 413 926 109 087 471 093 397 065 151 937 344 672 030 544 052 762 482 090 957 027 690 496 \ \backslash  
 $000 q^{9444} -$   
 476 338 457 356 659 491 404 015 848 345 259 129 450 058 560 905 606 622 330 880 641 439 182 091 399 \ \backslash  
 719 864 519 332 132 793 283 045 580 374 793 968 159 002 300 955 609 271 199 403 707 855 012 767 721 \ \backslash  
 181 109 385 758 352 703 250 475 769 221 353 580 201 930 165 224 771 309 665 598 436 738 625 545 214 \ \backslash  
 $700 q^{9445} +$   
 517 985 891 854 736 444 921 519 038 557 104 108 726 041 276 723 951 058 312 273 131 545 674 324 320 \ \backslash  
 128 712 839 337 060 015 781 942 291 169 928 004 542 992 576 618 496 816 236 889 594 912 354 686 320 \ \backslash  
 009 244 296 257 565 847 373 817 192 543 053 984 398 441 630 823 093 503 376 295 533 459 885 094 002 \ \backslash  
 $176 q^{9448} -$   
 532 660 809 117 525 710 065 614 524 046 207 751 861 195 826 337 252 186 508 015 257 952 056 401 141 \ \backslash  
 252 723 694 824 025 384 880 026 444 885 388 094 980 526 078 576 653 486 393 279 626 659 864 840 527 \ \backslash  
 687 217 445 285 443 870 230 087 098 029 495 680 279 611 700 589 296 771 709 510 637 771 086 450 688 \ \backslash  
 $000 q^{9449} +$   
 579 222 388 048 477 948 202 588 166 487 214 019 579 328 398 965 336 096 570 363 094 940 906 487 026 \ \backslash  
 500 088 071 893 733 285 457 358 432 223 453 962 219 699 700 958 182 543 475 038 669 616 752 395 384 \ \backslash  
 336 523 971 404 800 600 644 551 214 878 793 028 272 589 577 171 080 309 568 202 548 194 562 383 356 \ \backslash  
 $928 q^{9452} -$   
 595 628 665 339 260 389 721 847 639 113 850 135 581 793 097 230 861 086 657 568 248 946 688 285 359 \ \backslash  
 284 585 414 912 720 252 460 551 519 290 419 933 990 737 048 014 426 700 706 898 680 282 823 381 758 \ \backslash  
 977 291 940 434 723 732 659 414 713 962 454 700 852 097 105 103 810 092 896 256 054 217 430 596 251 \ \backslash  
 $207 q^{9453} +$   
 647 683 003 982 591 371 131 704 821 526 121 529 088 054 909 970 290 288 839 499 506 581 066 647 572 \ \backslash  
 240 106 757 655 495 329 620 399 002 132 991 244 602 891 065 791 158 463 293 756 976 104 179 939 451 \ \backslash  
 503 205 260 926 957 779 428 046 522 680 716 225 367 153 510 814 682 740 564 664 106 606 020 372 480 \ \backslash  
 $000 q^{9456} -$   
 666 024 477 605 374 663 622 652 248 628 297 109 668 908 512 704 886 392 393 748 546 363 375 019 929 \ \backslash  
 903 404 715 621 942 689 150 866 619 719 237 216 160 055 317 918 094 944 755 844 563 108 165 947 139 \ \backslash  
 978 331 203 587 868 422 477 337 976 181 617 290 443 972 472 194 626 944 483 184 411 829 458 776 260 \ \backslash  
 $608 q^{9457} +$   
 724 218 176 460 721 723 032 109 165 962 206 587 276 123 561 260 489 626 553 815 855 373 322 436 361 \ \backslash  
 693 988 988 391 774 885 601 789 985 472 620 500 733 875 415 970 615 142 257 186 105 051 259 594 718 \ \backslash  
 845 812 585 397 675 489 623 836 488 931 126 805 197 572 928 752 210 350 852 608 059 230 567 536 640 \ \backslash  
 $000 q^{9460} -$   
 744 722 630 122 372 024 678 954 237 116 769 487 227 258 611 419 376 835 854 272 686 026 994 341 749 \ \backslash  
 935 254 233 036 759 106 705 272 414 617 618 718 747 532 980 437 128 276 829 519 816 468 127 228 754 \ \backslash

924 261 744 347 055 342 021 059 434 377 210 016 288 787 820 790 839 916 117 428 036 008 335 403 299 3  
 125  $q^{9461} +$   
 809 778 246 079 320 009 701 139 181 617 772 768 235 099 636 740 979 331 188 247 711 059 981 159 363 3  
 655 069 718 486 928 712 998 798 720 681 788 192 007 928 686 408 396 689 392 198 024 721 392 220 339 3  
 382 570 601 527 291 923 753 672 101 605 623 809 185 750 373 064 875 188 665 314 011 493 687 696 000 3  
 000  $q^{9464} -$   
 832 700 218 380 434 307 031 613 537 129 403 739 310 590 422 456 854 936 993 647 406 248 409 847 914 3  
 835 212 879 582 136 356 450 747 664 544 736 053 446 810 239 206 863 479 468 236 077 178 297 913 409 3  
 380 428 949 379 992 063 335 588 030 335 254 368 236 105 040 457 504 035 943 465 991 344 956 273 459 3  
 200  $q^{9465} +$   
 905 425 168 525 828 693 899 620 032 552 620 165 546 787 936 019 100 085 909 325 175 651 378 554 877 3  
 122 572 079 348 879 591 121 878 574 739 825 056 972 920 788 597 954 695 095 472 532 250 643 402 104 3  
 518 932 887 370 545 615 682 404 421 023 668 769 517 850 907 394 951 668 829 469 268 696 737 216 358 3  
 400  $q^{9468} -$   
 931 049 088 895 847 582 452 602 569 178 839 786 346 742 186 530 044 557 620 669 009 798 875 902 322 3  
 480 404 294 016 079 644 296 425 320 525 225 905 341 494 599 003 468 609 489 731 572 234 052 804 916 3  
 198 965 537 400 241 826 012 695 815 902 992 074 914 511 694 237 096 163 299 081 480 290 160 438 506 3  
 500  $q^{9469} +$   
 1 012 345 595 848 423 165 151 562 789 408 002 091 693 203 037 828 974 213 791 424 850 901 353 717 576 3  
 496 774 223 673 327 157 277 877 636 666 662 853 383 639 100 496 815 882 949 098 746 849 519 517 827 3  
 908 638 125 063 509 356 201 423 494 580 295 304 617 078 688 287 420 876 662 480 188 398 089 897 246 3  
 720  $q^{9472} -$   
 1 040 989 287 268 208 526 735 338 363 044 754 201 072 470 263 508 074 038 613 652 126 104 623 727 991 3  
 863 658 241 971 144 242 291 925 557 781 676 012 122 856 092 482 016 860 926 006 130 350 396 824 856 3  
 515 870 035 359 392 493 478 823 083 946 335 269 508 602 933 959 328 146 744 444 180 115 631 418 245 3  
 120  $q^{9473} +$   
 1 131 865 487 616 958 776 088 281 390 595 144 012 869 760 676 005 493 392 437 368 191 802 201 756 108 3  
 013 487 561 780 596 361 335 114 575 276 751 495 865 046 335 772 864 245 832 138 182 281 141 094 543 3  
 846 545 976 696 431 578 789 567 914 385 295 730 025 166 426 291 284 379 818 044 482 952 466 190 336 3  
 000  $q^{9476} -$   
 1 163 884 078 938 892 814 646 163 873 368 080 207 865 412 058 166 421 631 986 851 752 203 952 784 568 3  
 658 028 829 394 116 241 880 027 155 098 829 514 324 745 373 164 324 196 332 032 786 750 674 246 194 3  
 873 859 132 754 545 529 173 112 811 775 735 424 433 706 147 406 592 191 463 413 689 933 062 790 937 3  
 597  $q^{9477} +$   
 1 265 466 430 523 200 592 186 871 003 885 957 620 928 781 672 317 052 628 242 570 983 987 643 440 624 3  
 268 585 935 547 153 002 270 315 376 477 843 648 546 227 193 048 795 464 885 448 152 144 979 611 126 3  
 215 717 989 456 806 630 845 313 458 509 895 169 492 599 205 657 921 655 405 375 784 494 866 235 545 3  
 600  $q^{9480} -$   
 1 301 256 726 184 966 727 885 242 864 328 704 994 822 193 625 429 321 768 619 244 207 083 026 011 512 3  
 449 600 640 596 187 901 444 666 047 626 564 124 988 852 365 497 974 041 040 787 538 531 094 405 840 3  
 655 970 743 612 385 600 174 498 448 303 337 099 248 872 355 538 790 721 860 157 080 817 281 814 528 3  
 000  $q^{9481} +$   
 1 414 803 865 762 224 874 604 284 773 362 935 334 587 810 747 508 314 425 673 052 176 467 842 054 820 3  
 845 712 438 429 366 066 938 429 797 200 023 426 436 308 994 910 733 441 585 901 826 068 149 055 073 3  
 729 858 797 254 843 842 514 931 231 359 186 355 627 129 797 687 048 358 889 188 997 250 933 537 088 3  
 000  $q^{9484} -$   
 1 454 809 226 256 045 675 100 459 360 612 882 282 279 160 424 295 822 877 334 908 675 903 632 288 155 3  
 533 798 520 576 455 473 008 267 006 445 737 000 389 586 036 568 103 763 162 943 771 741 613 297 414 3  
 339 995 896 005 538 520 296 456 803 692 880 620 606 533 748 349 384 334 210 768 831 277 506 607 582 3  
 125  $q^{9485} +$   
 1 581 727 446 747 253 681 937 398 630 215 662 606 007 548 654 462 922 980 368 500 079 637 155 536 077 3  
 094 277 975 780 810 190 255 940 391 125 477 275 723 234 452 589 721 817 654 461 063 447 030 458 553 3  
 190 443 426 803 382 967 148 571 069 677 776 567 151 693 969 592 563 043 766 335 917 979 894 249 947 3  
 136  $q^{9488} -$   
 1 626 443 239 418 698 260 766 673 996 131 350 260 447 939 893 845 024 535 267 416 809 613 215 812 573 3

274 115 365 466 863 402 743 839 186 902 564 407 158 842 753 370 649 711 166 139 261 189 013 350 326 3  
 792 400 748 654 357 315 030 174 700 380 184 219 481 809 601 960 991 931 353 647 900 894 111 141 888 3  
 000  $q^{9489} +$   
 1 768 303 775 617 367 200 845 056 821 556 947 321 280 872 143 337 531 292 617 977 213 481 781 391 905 3  
 287 021 440 749 931 406 813 113 332 393 591 913 380 189 552 554 839 587 246 110 541 361 414 460 643 3  
 670 249 986 430 810 372 904 881 489 358 699 252 615 111 480 776 927 800 825 609 454 882 291 340 632 3  
 064  $q^{9492} -$   
 1 818 283 462 301 891 135 431 590 188 597 575 119 109 804 323 478 299 624 903 811 074 762 442 978 363 3  
 897 541 424 269 965 052 202 306 505 651 599 897 878 784 963 652 853 314 737 236 360 163 414 905 795 3  
 600 755 595 469 622 714 459 338 967 839 685 755 821 839 746 978 292 564 809 251 675 428 890 313 081 3  
 938  $q^{9493} +$   
 1 976 841 795 914 215 329 296 523 896 785 950 916 242 040 243 269 354 839 072 697 493 048 439 376 670 3  
 658 396 682 624 869 492 698 757 079 485 933 414 349 557 629 666 317 541 617 054 745 338 974 733 877 3  
 352 956 183 173 814 626 721 511 367 458 322 492 368 319 302 070 839 531 983 496 626 495 396 865 856 3  
 000  $q^{9496} -$   
 2 032 703 731 659 028 220 313 967 753 289 395 632 529 986 067 152 171 919 448 651 366 586 766 243 666 3  
 184 317 033 695 277 972 024 618 195 073 929 082 665 896 108 704 447 930 258 734 005 539 072 084 693 3  
 612 584 843 300 487 314 288 692 127 678 820 203 898 574 540 706 055 699 001 315 612 912 170 522 050 3  
 560  $q^{9497} +$   
 2 209 921 151 078 881 348 856 493 092 222 244 552 208 050 692 244 913 102 652 667 170 643 505 788 428 3  
 155 216 355 234 379 411 815 204 618 623 273 490 093 393 602 004 449 017 901 691 007 184 178 733 611 3  
 919 769 642 444 312 422 802 782 924 409 671 496 470 252 378 318 167 303 955 625 480 334 240 070 144 3  
 000  $q^{9500} -$   
 2 272 356 176 835 897 955 156 988 877 584 243 101 757 469 048 354 334 017 076 579 759 458 852 082 269 3  
 010 863 615 300 596 887 428 361 219 469 339 014 407 459 153 332 460 081 923 944 930 696 774 763 842 3  
 098 888 410 568 784 125 412 182 775 104 473 428 875 174 397 422 427 345 486 740 270 866 763 500 494 3  
 250  $q^{9501} +$   
 2 470 423 854 442 651 853 808 678 811 056 357 518 394 272 395 284 366 830 004 378 335 072 370 733 973 3  
 209 818 380 004 917 988 370 265 449 469 682 124 821 828 613 035 749 753 636 450 021 175 470 161 541 3  
 646 029 901 898 118 615 203 183 774 510 113 017 095 791 413 200 959 230 956 228 398 867 160 940 544 3  
 000  $q^{9504} -$   
 2 540 203 776 259 316 206 880 080 669 353 704 604 634 952 261 564 625 873 824 089 012 974 868 571 804 3  
 960 110 832 814 658 659 441 015 896 545 262 285 154 292 901 109 346 126 749 095 588 122 363 538 487 3  
 559 420 110 563 861 233 823 079 347 338 207 967 421 709 421 756 100 346 166 418 133 310 994 461 491 3  
 200  $q^{9505} +$   
 2 761 569 656 589 847 278 452 968 844 602 267 299 304 796 769 376 185 036 489 272 867 826 179 795 410 3  
 810 638 459 307 759 631 865 707 053 814 476 882 311 046 420 132 308 346 924 909 268 716 825 851 802 3  
 205 799 646 583 710 145 538 378 963 649 383 597 454 462 785 742 384 581 997 491 938 905 367 750 246 3  
 400  $q^{9508} -$   
 2 839 556 714 584 711 958 637 493 376 984 079 606 511 841 019 420 934 062 025 674 886 318 483 095 610 3  
 370 411 685 110 406 169 325 825 901 341 636 662 708 492 630 374 889 938 589 879 294 272 020 326 144 3  
 978 844 449 595 305 638 638 070 868 995 018 899 371 062 010 968 406 525 843 104 766 672 298 295 021 3  
 375  $q^{9509} +$   
 3 086 955 540 841 503 290 244 308 489 884 249 769 351 393 235 591 125 434 393 192 920 238 633 046 034 3  
 861 845 095 704 215 042 087 979 977 734 152 892 323 514 376 989 776 103 411 151 970 917 545 673 782 3  
 800 017 716 194 448 638 532 210 315 328 531 149 259 868 825 045 090 820 071 399 775 338 707 996 500 3  
 992  $q^{9512} -$   
 3 174 112 983 260 217 164 295 001 466 642 160 198 819 553 538 638 521 252 460 549 735 046 680 108 584 3  
 327 367 540 692 863 534 518 650 777 485 089 710 723 523 302 717 047 591 037 968 757 366 287 478 212 3  
 836 286 536 377 030 672 389 015 662 876 967 988 126 260 116 690 953 993 112 556 778 136 051 386 286 3  
 080  $q^{9513} +$   
 3 450 599 827 686 003 148 835 124 140 955 084 063 946 660 563 823 193 358 629 537 603 381 943 771 693 3  
 100 623 240 172 740 576 187 368 533 495 773 686 166 367 986 124 205 687 339 307 190 538 724 844 119 3  
 560 994 784 676 757 292 148 067 207 522 333 820 981 536 270 877 046 356 392 143 526 141 058 316 288 3  
 000  $q^{9516} -$

3 548 003 718 735 411 393 986 895 235 419 870 979 913 845 359 541 207 189 050 489 214 141 703 183 153 3  
 389 049 308 035 758 541 371 529 257 951 931 587 169 065 013 258 286 144 707 384 805 926 876 014 759 3  
 586 769 755 193 954 980 076 062 680 799 067 887 623 386 204 834 696 112 546 453 400 050 439 945 111 3  
 225  $q^{9517} +$   
 3 856 991 424 869 644 447 825 803 576 833 175 906 281 772 725 557 627 980 184 602 281 896 979 746 271 3  
 175 734 913 084 572 173 456 799 915 370 157 774 296 580 409 536 786 449 692 726 029 411 758 657 501 3  
 665 930 450 510 046 187 182 322 776 061 551 635 512 626 440 315 282 571 859 482 616 948 188 366 028 3  
 800  $q^{9520} -$   
 3 965 843 829 984 345 793 430 003 633 441 587 441 699 416 107 597 457 961 168 340 286 647 632 367 763 3  
 300 961 397 377 680 807 571 281 556 969 215 093 404 102 731 427 060 954 263 276 452 369 973 148 456 3  
 436 377 920 722 706 918 729 359 548 591 339 746 282 521 814 559 542 165 758 014 935 663 587 753 984 3  
 000  $q^{9521} +$   
 4 311 144 822 229 145 310 557 216 877 542 182 413 401 939 777 724 186 219 590 586 688 813 625 925 618 3  
 795 467 584 126 816 881 308 720 196 880 092 749 317 760 846 394 249 504 124 366 603 873 029 370 709 3  
 877 556 921 606 224 840 502 802 009 639 683 253 815 143 437 103 039 306 562 081 470 138 592 362 240 3  
 000  $q^{9524} -$   
 4 432 788 531 116 031 354 034 479 869 013 233 401 688 528 587 759 315 891 379 520 985 024 998 571 982 3  
 788 661 858 378 851 733 653 966 204 814 116 090 679 676 930 257 807 600 899 453 787 242 492 163 477 3  
 928 744 807 566 939 379 741 088 998 785 131 245 579 942 431 656 447 982 045 488 584 163 079 827 967 3  
 325  $q^{9525} +$   
 4 818 661 499 949 518 178 027 395 637 364 888 298 115 968 945 466 326 563 199 867 789 749 700 003 562 3  
 979 153 150 322 258 257 750 663 741 779 209 393 449 687 367 259 226 262 197 910 292 760 042 717 835 3  
 417 385 919 683 901 780 454 511 093 122 982 387 737 840 187 927 430 807 263 734 661 903 077 822 348 3  
 288  $q^{9528} -$   
 4 954 596 466 382 272 395 243 431 602 282 943 860 818 021 074 724 985 604 474 956 558 979 229 938 673 3  
 931 328 028 862 936 911 841 115 583 580 353 415 496 755 104 130 778 030 735 049 428 594 563 641 311 3  
 840 991 616 107 667 554 163 425 007 315 535 230 347 373 334 650 688 468 571 608 219 841 914 806 272 3  
 000  $q^{9529} +$   
 5 385 798 496 601 482 363 869 177 131 647 395 150 834 038 550 993 994 042 118 295 634 535 328 431 131 3  
 426 028 707 012 599 401 861 376 073 494 529 360 414 652 750 626 976 654 015 226 071 736 299 277 118 3  
 087 899 620 156 072 599 591 381 318 773 371 733 103 261 203 648 083 591 893 346 057 436 212 691 075 3  
 072  $q^{9532} -$   
 5 537 700 194 722 657 751 707 702 051 955 782 441 878 503 371 204 308 959 999 102 360 949 517 057 798 3  
 659 839 632 007 481 834 618 314 641 952 464 385 628 692 323 218 583 107 752 080 761 554 764 829 636 3  
 562 510 709 228 396 882 681 782 946 411 126 559 141 429 503 160 292 286 529 226 795 892 678 507 291 3  
 827  $q^{9533} +$   
 6 019 544 969 986 211 312 690 544 455 194 615 285 121 600 961 196 719 829 510 262 467 452 411 529 231 3  
 114 590 935 421 686 661 526 048 901 816 630 092 316 510 667 337 901 682 752 244 694 786 759 711 741 3  
 259 851 978 228 681 388 522 586 960 627 155 491 941 071 055 711 016 966 880 027 288 756 268 810 240 3  
 000  $q^{9536} -$   
 6 189 284 890 069 104 401 572 412 098 345 029 296 338 107 780 922 274 251 113 656 384 214 192 422 899 3  
 717 113 502 594 403 223 171 373 413 310 502 839 097 307 715 406 720 828 486 912 038 830 076 698 623 3  
 488 103 621 013 290 359 153 989 904 230 963 411 701 191 933 242 816 687 793 355 596 492 548 958 093 3  
 312  $q^{9537} +$   
 6 727 707 680 533 058 393 708 773 884 540 553 697 548 307 329 140 979 410 127 907 010 067 412 077 663 3  
 549 050 673 992 003 890 976 002 800 508 037 704 415 666 010 782 353 322 859 728 950 875 096 985 108 3  
 530 103 467 364 465 408 991 696 883 054 407 423 228 667 867 634 289 454 778 877 605 233 012 617 216 3  
 000  $q^{9540} -$   
 6 917 376 213 037 754 527 241 035 271 310 795 810 721 100 396 110 939 475 866 821 647 065 423 391 058 3  
 550 602 791 600 491 537 115 261 488 054 767 131 857 353 433 927 076 684 574 184 627 495 692 521 782 3  
 012 641 210 889 746 923 702 517 498 826 817 583 681 739 500 485 871 541 302 471 136 694 186 906 939 3  
 250  $q^{9541} +$   
 7 519 006 434 919 514 208 139 778 721 125 646 432 165 586 434 873 198 692 286 338 079 944 028 746 956 3  
 109 443 609 243 384 790 693 143 617 037 526 686 588 499 079 813 687 104 928 034 020 979 283 707 793 3  
 654 403 565 268 213 470 405 124 702 871 554 639 675 984 066 617 139 213 235 953 782 695 065 030 400 3

$000 q^{9544} -$   
7 730 938 420 557 948 552 569 267 805 231 931 527 999 868 705 145 106 926 118 878 512 151 820 106 429 \ \backslash  
892 632 288 667 418 530 096 648 014 524 634 796 431 763 866 959 381 021 461 236 108 330 057 285 555 \ \backslash  
890 070 393 258 092 319 920 335 228 420 158 420 684 692 887 948 482 014 974 593 462 713 379 017 523 \ \backslash  
 $200 q^{9545} +$   
8 403 180 648 007 598 201 865 986 448 893 923 876 879 067 657 435 459 024 328 449 412 163 489 322 349 \ \backslash  
610 903 217 962 869 731 308 886 544 916 573 012 906 043 092 769 722 025 813 192 198 445 000 004 593 \ \backslash  
894 095 053 577 284 810 021 486 634 079 753 822 272 376 512 158 246 019 757 316 464 479 280 304 576 \ \backslash  
 $512 q^{9548} -$   
8 639 983 903 757 869 132 880 769 082 745 597 657 321 810 602 025 848 061 673 664 889 675 720 201 652 \ \backslash  
120 616 527 100 242 730 066 957 509 084 836 249 954 003 214 319 976 240 454 403 913 371 567 077 382 \ \backslash  
267 686 095 726 369 707 104 298 553 402 589 802 312 709 361 847 686 636 383 915 451 834 532 236 355 \ \backslash  
 $125 q^{9549} +$   
9 391 108 315 562 234 476 611 822 819 263 032 077 860 186 749 980 493 139 869 013 886 967 526 694 874 \ \backslash  
585 477 385 330 702 551 722 338 574 803 841 539 579 814 707 326 047 438 438 657 908 977 228 066 859 \ \backslash  
141 752 305 303 393 099 231 639 447 532 910 688 829 262 446 649 832 354 811 214 076 942 054 580 322 \ \backslash  
 $304 q^{9552} -$   
9 655 695 482 529 315 743 216 845 354 526 802 712 559 811 091 111 833 618 490 616 796 985 889 665 860 \ \backslash  
811 832 110 324 423 844 909 360 124 332 824 610 350 890 400 552 880 485 836 401 139 175 163 693 661 \ \backslash  
574 239 691 296 981 353 882 368 455 734 295 365 871 434 700 406 550 834 791 213 666 738 223 501 082 \ \backslash  
 $624 q^{9553} +$   
10 494 938 840 146 649 659 168 187 660 093 854 639 610 132 641 597 087 731 415 050 593 540 176 090 \ \backslash  
250 596 121 498 811 999 816 656 422 358 487 208 186 326 785 392 478 664 902 527 248 391 332 710 757 \ \backslash  
229 174 256 036 362 608 002 814 419 906 844 828 875 131 274 282 035 863 128 266 218 119 410 075 087 \ \backslash  
 $104 000 q^{9556} -$   
10 790 562 939 286 257 671 535 062 901 059 577 979 974 400 421 879 266 764 060 716 849 940 634 008 \ \backslash  
567 903 012 142 273 857 819 673 628 033 344 957 757 342 990 823 482 583 163 824 138 906 550 384 033 \ \backslash  
255 453 194 084 887 224 652 392 411 970 309 114 730 736 946 402 611 298 296 801 848 413 712 211 566 \ \backslash  
 $234 543 q^{9557} +$   
11 728 241 319 875 077 052 470 815 080 117 607 631 716 036 228 608 954 381 905 243 683 169 676 169 \ \backslash  
281 067 167 528 600 417 462 463 013 501 082 739 678 233 317 007 728 618 238 418 846 500 317 086 190 \ \backslash  
982 050 850 439 856 571 508 077 020 292 806 392 193 965 633 046 044 102 365 686 317 092 036 867 730 \ \backslash  
 $124 800 q^{9560} -$   
12 058 535 446 360 661 804 902 830 233 338 389 919 960 336 680 089 851 918 796 700 822 579 055 570 \ \backslash  
742 246 840 565 397 381 021 224 136 308 199 014 667 200 057 648 332 638 519 104 351 546 753 410 564 \ \backslash  
205 617 164 964 810 225 987 535 819 877 914 484 308 218 147 694 035 608 055 218 393 673 604 102 279 \ \backslash  
 $168 000 q^{9561} +$   
13 106 170 096 348 938 499 289 500 550 189 301 880 795 675 864 058 607 754 524 305 723 835 100 176 \ \backslash  
023 449 968 878 528 191 995 643 054 090 148 428 863 302 911 009 253 081 133 427 899 851 653 723 133 \ \backslash  
428 433 009 592 437 923 087 466 355 674 770 976 705 314 667 421 865 117 262 797 761 661 676 941 500 \ \backslash  
 $160 000 q^{9564} -$   
13 475 191 733 304 923 537 308 425 314 215 436 013 569 865 651 572 395 554 723 152 359 630 132 833 \ \backslash  
827 237 680 315 183 246 866 205 854 583 311 988 029 192 597 298 962 613 219 384 040 028 921 464 609 \ \backslash  
950 576 873 640 548 873 401 043 905 230 996 856 775 070 730 164 243 071 535 877 082 378 066 721 353 \ \backslash  
 $267 875 q^{9565} +$   
14 645 649 566 345 198 330 158 736 824 956 543 101 125 457 480 273 315 726 985 204 741 581 891 740 \ \backslash  
305 225 243 390 838 539 272 208 910 727 125 415 944 775 654 868 523 958 093 701 062 434 466 640 882 \ \backslash  
034 528 163 634 041 469 102 560 935 326 207 275 472 165 969 024 978 076 667 996 867 057 372 455 246 \ \backslash  
 $315 520 q^{9568} -$   
15 057 930 054 390 857 848 824 387 448 734 703 533 027 330 032 485 563 691 692 975 832 482 312 708 \ \backslash  
976 239 160 732 337 340 854 047 760 428 503 998 474 012 847 402 821 148 371 307 836 317 818 416 223 \ \backslash  
081 448 321 156 154 657 540 092 295 581 632 285 182 918 401 968 290 984 972 114 723 540 259 449 659 \ \backslash  
 $392 000 q^{9569} +$   
16 365 580 494 158 435 423 986 775 969 025 631 324 705 823 975 832 946 927 557 314 049 558 319 604 \ \backslash  
086 619 284 628 661 013 743 487 419 995 621 662 958 356 364 823 749 412 225 032 196 173 640 645 416 \ \backslash

391 629 726 339 084 780 913 853 095 716 297 178 866 842 677 097 642 491 135 126 684 854 799 580 377 \\  
 169 920  $q^{9572}$  -

16 826 180 255 373 254 866 511 318 709 080 569 374 537 109 189 421 704 695 881 131 544 129 729 405 \\  
 238 961 075 676 500 200 962 016 287 084 351 244 206 369 716 246 037 297 329 502 243 044 810 621 854 \\  
 930 848 557 208 552 498 643 266 093 299 630 395 854 699 088 854 674 561 863 516 536 440 578 551 496 \\  
 346 554  $q^{9573}$  +

18 287 070 320 702 388 332 894 929 595 741 767 863 132 338 588 492 700 445 422 744 467 591 067 054 \\  
 927 435 875 721 516 714 885 109 680 598 126 592 051 425 440 213 614 234 167 642 752 721 736 550 765 \\  
 359 644 306 869 935 857 540 003 290 503 076 745 795 812 634 924 928 634 888 269 166 591 653 188 976 \\  
 256 000  $q^{9576}$  -

18 801 640 504 979 353 686 700 723 259 844 456 676 475 664 549 531 402 041 621 031 830 529 293 585 \\  
 798 633 024 671 081 469 830 037 471 592 091 702 573 473 088 225 618 305 336 071 541 424 316 192 521 \\  
 656 817 064 594 914 725 464 213 816 384 729 536 319 688 747 459 607 776 427 303 475 748 412 962 451 \\  
 095 552  $q^{9577}$  +

20 433 690 254 653 697 636 334 105 316 448 814 777 425 461 248 886 520 832 865 627 510 111 783 721 \\  
 748 114 066 377 619 105 475 677 908 165 400 916 937 135 239 071 402 423 568 703 345 727 467 445 138 \\  
 598 494 486 841 098 284 504 696 113 387 779 491 914 702 187 000 020 383 881 962 258 469 446 873 644 \\  
 748 800  $q^{9580}$  -

21 008 541 553 781 333 968 451 997 547 523 616 219 226 215 193 830 425 361 861 083 345 622 068 043 \\  
 318 226 548 623 168 054 963 224 392 545 769 743 745 767 126 343 937 070 470 042 337 935 717 435 718 \\  
 640 165 949 537 241 241 005 933 045 785 241 254 768 856 728 994 062 332 525 580 391 337 962 974 202 \\  
 766 000  $q^{9581}$  +

22 831 762 253 528 906 581 749 025 266 936 543 082 351 154 149 943 692 956 840 966 175 864 626 740 \\  
 713 757 609 323 922 072 076 575 362 046 861 278 408 610 178 906 642 328 930 940 397 979 193 881 843 \\  
 019 412 325 563 679 482 583 393 417 144 076 192 766 190 764 435 029 339 743 821 106 895 074 485 946 \\  
 368 000  $q^{9584}$  -

23 473 941 714 661 214 849 903 561 769 272 718 972 062 950 115 874 141 289 536 395 377 929 052 179 \\  
 582 345 746 162 073 642 296 867 235 447 022 381 871 388 355 460 513 226 211 539 811 530 137 667 453 \\  
 412 142 956 912 988 683 432 878 558 260 876 241 470 594 340 059 135 436 645 791 078 232 896 092 648 \\  
 243 200  $q^{9585}$  +

25 510 679 362 482 352 347 741 824 007 626 960 686 976 445 728 046 178 939 594 335 640 391 429 024 \\  
 696 098 178 334 750 418 639 031 279 900 058 077 553 185 293 433 412 729 953 665 102 357 022 619 165 \\  
 237 030 991 157 061 566 008 518 147 977 380 649 713 971 195 455 367 014 464 611 246 150 818 099 913 \\  
 326 592  $q^{9588}$  -

26 228 056 128 949 771 881 347 068 863 252 782 493 921 971 836 622 192 593 627 451 352 593 879 076 \\  
 366 764 794 697 433 137 549 206 228 489 097 711 092 948 376 121 913 428 191 637 233 284 177 667 731 \\  
 608 828 834 121 935 540 858 236 494 704 638 973 868 518 171 498 820 378 714 069 993 608 056 557 785 \\  
 619 500  $q^{9589}$  +

28 503 263 280 098 275 656 301 151 437 338 362 391 868 157 220 048 798 163 187 896 370 591 931 946 \\  
 217 869 852 192 385 149 217 994 058 972 500 232 900 651 394 108 080 805 800 726 569 552 716 592 569 \\  
 722 674 871 636 380 899 223 747 168 505 823 946 688 725 067 544 577 657 301 888 445 641 284 088 775 \\  
 181 312  $q^{9592}$  -

29 304 624 294 932 883 238 125 846 867 898 193 491 916 273 566 051 045 692 518 251 107 277 853 085 \\  
 360 564 408 246 384 861 830 185 229 842 015 178 044 030 597 100 772 112 604 151 277 802 041 123 503 \\  
 781 429 488 508 627 258 629 926 027 274 146 816 393 878 367 209 232 520 890 095 114 887 008 612 357 \\  
 505 024  $q^{9593}$  +

31 846 163 468 321 220 081 800 382 991 033 113 856 714 117 664 192 217 972 866 979 709 215 030 735 \\  
 515 074 207 674 034 383 423 045 407 891 376 985 450 141 542 478 315 618 576 867 252 490 249 182 453 \\  
 567 577 794 588 132 139 333 533 433 391 987 436 743 099 080 933 324 371 307 512 286 720 413 968 602 \\  
 112 000  $q^{9596}$  -

32 741 320 295 698 420 906 508 427 467 178 626 545 244 801 417 576 800 030 740 724 757 022 852 610 \\  
 241 655 053 673 091 592 321 959 500 920 305 390 149 526 932 919 022 417 463 943 887 860 161 889 002 \\  
 554 342 714 434 147 280 589 743 393 219 590 715 772 192 285 591 793 292 849 980 514 962 392 602 013 \\  
 313 943  $q^{9597}$  +

35 580 302 623 272 402 308 057 388 946 452 378 800 898 035 500 942 355 741 492 485 154 907 373 594 \

231 627 108 739 167 151 882 305 395 571 786 435 066 916 560 765 742 837 243 021 643 023 484 646 304 \\  
 746 668 645 132 300 924 454 426 652 373 756 569 286 641 738 839 503 889 483 693 143 726 900 135 633 \\  
 715 200  $q^{9600}$  -

36 580 210 676 739 834 644 762 947 195 924 311 022 616 349 798 651 733 000 839 421 496 690 070 714 \\  
 902 677 935 924 155 606 146 565 862 762 250 681 012 689 470 396 492 796 074 523 789 801 452 897 682 \\  
 464 166 419 991 858 892 553 872 118 539 402 148 981 026 186 297 858 593 272 314 024 718 670 443 200 \\  
 512 000  $q^{9601}$  +

39 751 373 880 999 299 518 777 922 448 542 327 396 470 322 572 846 827 184 848 857 548 327 854 224 \\  
 489 338 260 369 721 915 443 005 371 407 669 558 943 958 850 612 441 932 761 105 079 979 508 052 715 \\  
 353 240 557 056 766 139 991 090 973 108 874 810 189 979 983 406 940 646 178 112 590 681 792 357 814 \\  
 298 752  $q^{9604}$  -

40 868 265 496 466 578 888 452 841 841 115 698 318 126 162 944 834 625 004 545 670 319 671 922 693 \\  
 543 237 366 730 950 423 462 734 590 904 576 392 703 566 996 993 539 273 710 373 263 984 043 235 996 \\  
 001 379 796 531 405 643 048 020 503 348 466 070 774 124 653 671 222 082 179 480 496 960 011 267 640 \\  
 571 875  $q^{9605}$  +

44 410 395 753 850 218 941 520 322 296 598 027 125 011 774 685 572 057 853 463 780 256 221 052 690 \\  
 641 743 682 496 552 510 340 401 251 225 953 628 470 142 457 299 482 409 937 917 432 950 548 434 165 \\  
 602 889 318 632 962 378 315 353 755 337 019 073 785 043 043 081 186 266 143 511 968 969 987 767 471 \\  
 171 584  $q^{9608}$  -

45 657 928 711 628 948 066 060 711 990 067 324 412 500 654 495 256 874 198 818 195 463 011 116 539 \\  
 788 140 369 648 499 226 868 318 387 701 353 487 254 551 804 103 137 108 416 959 200 171 188 871 654 \\  
 045 400 276 224 071 005 427 587 824 303 096 209 812 304 289 401 133 886 229 272 421 443 755 630 858 \\  
 240 000  $q^{9609}$  +

49 614 331 486 568 728 910 147 710 620 480 277 010 986 246 094 463 974 424 461 158 573 650 219 133 \\  
 193 885 615 572 821 175 954 086 542 430 487 664 443 213 347 318 440 027 050 061 767 390 573 287 370 \\  
 474 442 982 125 753 967 828 971 196 204 718 395 511 233 850 311 184 281 254 885 240 935 732 086 112 \\  
 481 280  $q^{9612}$  -

51 007 754 772 263 853 347 255 935 735 446 976 421 430 379 820 301 683 339 621 100 555 634 653 465 \\  
 228 633 621 600 465 748 467 798 476 787 264 464 565 265 949 261 215 222 620 909 249 657 908 058 232 \\  
 765 795 543 674 068 165 715 459 232 198 325 388 327 235 699 744 702 936 261 992 833 574 408 470 172 \\  
 291 183  $q^{9613}$  +

55 426 780 294 630 576 124 181 465 456 557 889 666 088 598 682 241 961 139 661 825 354 895 415 686 \\  
 694 926 200 897 495 234 288 422 904 745 996 782 191 458 163 024 885 874 112 813 507 141 420 115 037 \\  
 200 229 921 205 157 305 786 228 446 913 402 949 097 887 134 751 671 696 208 755 114 879 681 149 255 \\  
 680 000  $q^{9616}$  -

56 983 119 095 602 592 076 630 240 059 883 514 284 791 782 519 975 320 564 738 446 853 520 642 465 \\  
 205 474 596 889 250 245 639 274 977 786 051 036 072 565 357 060 490 806 355 728 735 659 259 485 235 \\  
 501 761 136 104 379 586 252 353 289 769 467 190 093 895 920 607 755 381 238 360 049 543 394 369 415 \\  
 118 848  $q^{9617}$  +

61 918 748 810 014 319 851 900 150 679 005 516 434 360 989 879 298 806 940 913 073 897 400 252 328 \\  
 925 416 484 296 534 888 050 770 491 597 245 351 857 224 359 356 888 621 288 255 801 173 020 940 970 \\  
 067 340 272 544 471 322 922 946 118 435 557 217 852 971 032 474 946 200 336 006 942 967 938 561 947 \\  
 443 200  $q^{9620}$  -

63 657 010 974 922 074 943 518 730 938 852 444 717 274 431 421 071 516 895 799 671 752 288 670 387 \\  
 320 061 844 915 174 320 251 347 512 335 296 220 483 045 014 540 959 590 995 701 809 178 369 407 543 \\  
 524 870 005 217 752 043 018 350 348 072 963 466 044 578 237 241 460 444 733 407 464 019 579 998 680 \\  
 675 000  $q^{9621}$  +

69 169 512 021 781 803 071 515 022 778 646 001 595 599 316 746 956 286 454 962 950 702 819 634 080 \\  
 064 315 206 284 555 534 865 876 231 288 537 589 607 010 440 445 019 290 920 851 271 641 799 499 669 \\  
 487 658 692 603 661 117 099 316 692 886 811 013 402 396 446 162 274 347 220 188 603 755 214 555 836 \\  
 032 000  $q^{9624}$  -

71 110 918 468 125 968 923 191 869 284 404 176 583 252 728 551 898 741 735 096 253 779 764 183 174 \\  
 808 964 052 333 841 469 029 013 482 291 971 625 193 912 220 668 765 668 763 434 275 456 716 070 565 \\  
 433 951 012 029 248 965 720 884 127 505 126 475 897 510 558 392 749 598 981 808 455 849 866 408 542 \\  
 208 000  $q^{9625}$  +

77 267 574 072 001 843 613 340 183 660 691 482 947 938 456 514 345 650 437 012 455 522 281 618 653 \

654 399 139 216 149 811 830 946 366 072 033 955 432 540 899 006 316 373 280 541 300 368 908 148 958 \

912 369 490 158 993 893 481 687 996 924 969 564 176 321 616 848 465 977 977 930 847 216 357 895 931 \

443 200  $q^{9628}$  -

79 435 815 913 683 620 097 051 311 554 467 192 165 894 535 144 957 487 835 352 327 267 430 493 817 \

596 218 637 279 730 455 172 302 963 373 990 887 715 138 277 421 479 013 136 091 807 033 445 366 260 \

465 517 935 684 703 949 865 455 675 093 645 786 434 631 086 691 036 428 725 873 887 334 030 240 658 \

492 375  $q^{9629}$  +

86 311 740 464 452 302 285 629 483 378 592 732 610 268 215 134 410 455 242 932 292 904 259 742 671 \

305 403 855 557 698 946 110 536 176 753 718 119 574 992 383 418 132 704 616 137 447 951 116 351 896 \

545 151 092 598 803 412 364 168 490 770 292 199 578 200 182 241 329 204 834 434 437 434 491 647 106 \

170 880  $q^{9632}$  -

88 733 265 951 556 518 974 943 806 764 719 664 866 323 965 739 904 747 758 617 974 405 767 868 242 \

177 402 552 302 147 710 764 140 977 333 532 268 271 123 820 270 949 238 965 179 592 982 873 972 227 \

818 303 073 302 330 842 826 207 841 001 982 291 330 785 709 132 379 855 380 281 113 720 911 568 293 \

822 464  $q^{9633}$  +

96 412 314 578 421 021 714 389 954 616 009 636 528 354 239 796 024 051 204 030 160 232 977 229 034 \

900 879 409 432 730 519 282 327 592 094 914 294 566 788 281 597 288 245 287 334 080 118 279 167 644 \

178 103 789 876 818 693 519 595 114 018 193 723 952 457 011 120 024 064 272 981 120 993 260 045 570 \

048 000  $q^{9636}$  -

99 116 649 298 535 796 732 153 040 386 887 741 995 919 820 584 883 079 240 401 093 794 140 163 249 \

647 718 354 650 503 127 791 417 564 488 341 541 476 629 683 809 179 086 227 734 546 036 443 534 985 \

330 375 409 611 777 436 090 018 699 358 451 830 756 066 634 340 626 843 716 057 421 672 712 810 354 \

335 963  $q^{9637}$  +

107 692 432 868 669 123 834 841 213 484 388 173 527 266 142 810 246 184 159 844 374 168 771 628 187 \

467 140 888 131 829 532 281 804 901 319 451 565 151 108 971 941 399 000 029 605 985 224 497 901 970 \

606 639 315 218 435 980 358 411 243 159 664 993 267 159 695 486 154 587 684 511 649 638 938 433 167 \

155 200  $q^{9640}$  -

110 712 537 057 311 126 142 022 297 164 913 400 371 388 658 958 613 964 785 781 530 361 736 217 758 \

587 149 251 371 180 635 781 402 010 230 523 566 876 552 802 412 394 002 929 201 929 343 831 189 684 \

131 807 538 087 789 149 277 032 958 198 604 698 631 954 943 664 853 846 216 196 936 463 306 961 485 \

824 000  $q^{9641}$  +

120 289 554 792 917 300 089 744 134 165 756 775 834 634 574 027 026 156 501 781 521 131 452 826 403 \

007 764 196 206 388 849 759 286 175 260 703 862 580 169 841 773 816 911 625 976 747 435 080 191 491 \

739 733 148 251 990 923 878 192 361 198 838 126 305 880 339 065 165 543 420 185 362 782 085 077 401 \

792 000  $q^{9644}$  -

123 662 222 044 775 273 863 627 455 716 429 555 019 464 379 017 168 435 359 771 950 701 810 068 994 \

806 254 093 916 553 801 264 985 472 994 368 197 694 892 104 777 229 345 783 356 530 001 917 529 077 \

273 147 726 339 891 305 050 937 262 414 907 985 416 066 855 036 608 146 023 452 014 471 048 542 471 \

991 850  $q^{9645}$  +

134 357 125 359 794 702 071 674 259 622 861 251 685 112 527 845 184 616 027 286 757 860 551 513 898 \

658 588 189 415 153 089 248 800 956 623 562 553 993 874 322 355 506 386 881 982 307 450 481 533 816 \

211 408 010 994 182 293 687 281 215 030 981 300 962 267 057 593 318 283 957 343 249 841 504 372 067 \

987 456  $q^{9648}$  -

138 123 427 527 810 243 756 045 182 873 386 162 433 918 250 092 566 080 322 103 470 303 048 534 209 \

644 376 078 637 971 022 240 076 675 953 846 607 083 926 794 517 657 552 042 282 836 990 240 740 402 \

528 090 060 300 232 030 481 430 033 865 249 646 305 382 635 237 551 611 509 194 980 369 341 011 255 \

296 000  $q^{9649}$  +

150 066 430 255 042 348 802 192 253 282 043 634 063 288 736 227 731 792 703 253 210 925 372 397 219 \

041 210 069 414 277 040 078 209 821 653 663 553 638 329 424 245 291 510 172 840 843 639 929 459 719 \

111 805 260 333 667 189 607 033 630 503 994 071 659 912 257 215 518 230 382 198 073 537 775 942 159 \

753 216  $q^{9652}$  -

154 272 213 876 697 332 892 978 249 871 536 299 971 775 284 525 171 174 893 669 096 547 123 252 052 \

725 812 563 470 072 409 567 584 886 036 008 927 949 625 659 385 032 813 941 489 815 214 309 905 428 \

099 329 000 379 209 062 728 815 408 292 551 865 653 744 661 115 329 779 898 564 266 654 864 844 710 \

$376\,783\,q^{9653} +$   
 167 608 665 806 403 191 292 415 105 369 225 734 712 865 705 374 420 078 260 479 278 322 927 245 393 999 121 075 374 976 100 745 752 775 706 587 141 729 445 729 934 384 483 519 622 312 787 428 386 197 817 379 331 153 939 581 029 018 146 591 782 383 886 574 591 451 613 514 089 679 129 384 200 005 503 232 000  $q^{9656} -$   
 172 305 106 012 533 749 592 260 501 487 000 774 405 805 008 097 156 055 596 443 340 016 478 997 814 471 931 102 491 065 243 253 988 846 995 867 711 887 501 614 834 333 423 547 645 533 353 189 946 841 836 468 917 100 914 995 745 733 664 733 000 136 633 973 314 279 242 650 510 072 784 413 252 742 792 282 112  $q^{9657} +$   
 187 197 248 615 385 638 435 464 960 356 128 305 335 596 032 195 127 086 631 092 413 739 855 109 375 395 864 540 151 886 198 080 177 678 746 811 712 069 062 543 510 325 149 238 530 974 810 171 507 755 614 375 864 482 258 558 601 847 709 775 547 030 367 098 265 975 046 980 645 909 190 029 168 349 814 374 400  $q^{9660} -$   
 192 441 467 163 701 148 098 720 647 957 969 201 145 567 647 694 037 157 401 214 739 356 866 295 211 720 094 938 990 817 033 576 732 674 725 964 418 693 795 849 597 553 292 647 734 983 721 504 906 061 646 016 569 951 528 084 467 088 653 886 218 704 133 821 658 160 776 303 943 493 440 588 135 585 078 083 500  $q^{9661} +$   
 209 070 392 547 416 786 746 248 564 322 682 904 858 889 638 317 992 310 079 291 804 233 694 057 934 657 773 249 677 836 524 580 268 674 602 783 274 217 164 578 544 569 187 462 328 304 145 571 071 375 837 352 349 405 984 177 068 895 309 489 384 049 463 483 965 147 317 618 774 205 489 012 948 228 227 072 000  $q^{9664} -$   
 214 926 147 388 814 819 345 304 826 184 346 001 921 200 456 521 375 949 966 812 438 227 768 085 764 031 342 545 301 570 220 273 956 508 493 380 212 810 460 007 505 697 986 426 873 602 840 031 224 856 224 820 432 816 323 549 090 622 212 158 244 798 476 034 829 601 752 166 146 506 103 410 012 363 761 254 400  $q^{9665} +$   
 233 493 983 964 758 597 211 837 219 283 589 486 833 595 492 965 319 986 726 275 029 954 946 566 703 344 267 903 776 931 737 241 443 609 781 381 311 056 258 494 904 428 389 122 449 938 129 586 148 293 828 175 969 383 797 371 341 983 163 739 423 075 314 669 963 910 960 932 794 259 390 639 527 797 587 656 704  $q^{9668} -$   
 240 032 438 604 572 979 688 346 136 790 506 953 270 792 643 179 199 035 894 370 952 114 184 434 513 691 905 238 563 929 689 642 759 776 329 490 225 958 606 945 721 807 692 153 877 826 735 291 357 152 399 500 750 674 071 367 765 068 598 296 630 574 157 692 184 735 083 553 171 326 464 229 908 284 115 718 125  $q^{9669} +$   
 260 764 789 646 789 659 436 672 469 520 686 994 799 167 378 598 743 277 272 542 469 864 674 959 237 931 679 545 148 111 853 202 154 123 792 474 594 533 366 001 180 219 047 581 303 194 029 061 529 105 928 417 544 927 276 316 122 322 430 331 741 361 901 678 190 499 397 871 915 635 618 514 278 990 050 756 608  $q^{9672} -$   
 268 065 371 515 409 138 842 609 206 837 500 947 984 135 261 012 837 834 460 082 405 605 129 307 913 595 248 383 684 926 952 398 520 256 035 526 643 429 621 804 344 842 984 800 675 861 534 445 507 769 048 727 630 569 759 235 105 422 170 525 293 383 326 453 528 598 439 808 295 524 355 858 695 297 550 909 440  $q^{9673} +$   
 291 214 035 812 039 077 785 327 996 906 322 319 823 748 970 132 246 045 330 181 814 800 233 281 909 692 266 029 032 241 151 716 904 753 340 642 499 928 594 760 269 890 069 569 300 992 489 906 676 634 558 931 487 182 518 033 018 825 738 646 545 852 430 124 248 573 657 561 978 232 214 579 709 885 566 464 000  $q^{9676} -$   
 299 365 393 921 168 722 025 337 425 502 318 826 688 932 856 836 879 139 037 706 829 758 467 685 636 759 094 315 108 015 404 664 060 562 619 032 587 650 602 844 583 284 554 984 027 729 942 677 779 033 418 827 670 258 600 096 045 087 956 621 408 459 062 266 386 257 353 713 018 755 985 905 647 925 857 617 276  $q^{9677} +$   
 325 211 401 082 712 820 089 737 515 386 307 798 446 384 846 935 884 053 033 516 876 720 900 604 644 500 450 290 101 407 898 823 372 978 049 460 450 114 501 591 914 545 884 576 517 899 656 705 355 952 909 204 691 564 270 055 628 837 446 368 595 424 479 339 736 835 802 022 018 131 104 417 058 960 239 738 880  $q^{9680} -$   
 334 312 474 427 491 716 475 234 083 903 238 033 624 135 708 986 430 732 481 827 280 258 277 759 451 962 360 473 493 429 312 696 647 585 458 206 197 002 471 645 707 507 646 467 197 606 146 623 410 890

290 299 445 780 102 225 422 003 480 520 509 164 141 897 894 811 712 892 710 568 285 583 070 627 127 \
 296 000  $q^{9681}$  +

363 169 471 167 777 971 184 990 839 204 441 795 504 960 756 787 708 264 372 762 664 000 764 055 667 \
 483 700 680 963 662 718 497 034 771 320 863 246 534 582 478 812 430 062 398 521 035 399 579 352 087 \
 061 065 243 988 618 967 577 083 073 974 902 512 103 284 412 699 266 520 425 367 070 728 354 147 059 \
 968 000  $q^{9684}$  -

373 330 680 655 027 577 299 652 618 775 686 265 726 108 040 336 276 040 556 308 005 139 622 159 663 \
 653 631 031 489 613 044 703 278 941 258 010 134 362 288 802 363 990 085 837 413 834 640 691 051 960 \
 557 895 021 020 580 904 435 326 785 129 586 803 858 184 243 375 611 877 957 888 629 847 628 171 721 \
 453 950  $q^{9685}$  +

405 548 708 543 369 806 213 418 678 533 493 880 536 085 443 445 868 046 772 039 524 527 199 056 765 \
 600 803 835 290 272 284 034 793 347 984 161 649 979 571 581 303 194 276 161 760 073 401 464 803 285 \
 552 085 841 128 467 479 603 610 352 810 010 552 055 621 422 912 546 215 869 466 119 033 714 666 270 \
 379 008  $q^{9688}$  -

416 893 286 698 044 728 514 701 706 952 425 796 634 960 922 198 104 108 730 654 910 803 972 697 381 \
 134 220 894 278 247 987 567 901 656 092 989 524 095 405 375 818 315 724 815 995 436 357 977 284 309 \
 217 859 756 282 005 515 754 918 760 146 751 177 050 578 531 605 969 523 979 961 500 970 678 615 826 \
 432 000  $q^{9689}$  +

452 862 996 544 451 170 232 990 347 179 722 705 302 546 282 413 961 955 166 496 197 545 281 547 636 \
 758 239 293 106 707 962 124 986 515 977 323 144 007 380 958 082 943 358 101 011 073 563 906 948 101 \
 966 727 839 986 674 198 893 861 545 971 232 282 462 756 772 167 344 621 675 364 417 709 393 137 927 \
 550 976  $q^{9692}$  -

465 528 470 887 303 535 252 117 011 892 914 459 954 437 520 598 043 376 669 910 791 426 534 448 122 \
 787 231 488 308 366 758 519 745 281 087 511 679 272 601 184 530 545 966 106 367 371 942 957 071 316 \
 770 164 494 378 098 485 895 672 144 723 429 444 280 256 642 473 825 224 180 521 133 520 440 550 241 \
 025 120  $q^{9693}$  +

505 685 824 121 825 902 954 832 288 963 672 117 309 109 496 494 988 218 023 860 096 461 046 827 926 \
 261 942 736 285 210 977 487 557 537 534 887 021 727 881 387 461 466 099 454 932 667 109 972 560 873 \
 752 114 155 672 714 501 857 468 004 460 580 740 555 154 064 392 016 882 469 460 940 920 241 160 307 \
 712 000  $q^{9696}$  -

519 825 671 940 773 556 588 948 520 651 692 416 382 329 571 551 906 613 099 378 475 556 912 605 206 \
 128 127 865 737 703 674 493 315 151 960 706 658 581 179 143 031 522 112 387 864 226 620 283 104 344 \
 997 964 974 636 434 256 744 739 222 100 594 470 498 946 240 187 642 496 936 008 950 357 255 311 951 \
 724 544  $q^{9697}$  +

564 657 185 144 633 761 101 335 335 651 832 253 577 435 945 697 139 743 473 012 996 977 659 398 770 \
 848 979 247 744 771 322 209 471 676 880 992 311 130 849 186 679 957 872 014 049 886 169 988 229 738 \
 581 131 782 699 748 511 162 364 833 609 874 368 342 718 984 728 685 699 004 647 788 272 246 559 024 \
 332 800  $q^{9700}$  -

580 442 679 421 958 959 224 668 330 371 398 497 527 622 912 451 054 464 364 704 906 390 532 270 479 \
 277 903 934 464 929 328 236 384 737 167 559 988 943 182 608 244 803 209 537 267 014 021 843 261 114 \
 342 454 314 069 172 968 725 921 971 665 144 563 296 840 210 292 651 569 770 195 728 190 842 394 418 \
 537 000  $q^{9701}$  +

630 491 274 630 430 851 292 470 679 795 794 402 786 349 906 546 533 491 009 188 330 581 544 250 549 \
 604 724 064 932 499 730 501 181 871 530 030 136 012 588 903 878 969 906 956 941 592 401 823 792 494 \
 776 418 229 623 534 390 303 628 495 367 051 281 749 261 641 408 348 253 167 570 781 387 865 303 553 \
 344 000  $q^{9704}$  -

648 113 543 161 821 063 625 492 943 573 665 541 698 087 459 172 183 687 210 465 116 066 273 705 832 \
 840 194 305 719 710 503 671 129 983 171 269 703 314 158 060 171 531 387 563 812 860 140 314 954 246 \
 487 876 258 259 585 020 528 917 796 957 928 741 317 465 750 920 247 386 070 053 701 355 206 662 063 \
 718 400  $q^{9705}$  +

703 985 073 763 292 492 818 341 829 731 904 803 404 941 206 672 621 932 269 293 023 183 287 357 652 \
 095 429 131 969 880 806 334 895 183 775 671 434 729 467 540 625 401 473 684 876 230 159 764 753 431 \
 421 209 448 379 898 856 809 226 771 079 764 181 360 484 588 730 547 796 179 571 761 875 916 535 334 \
 067 200  $q^{9708}$  -

723 657 396 039 715 533 487 042 600 212 512 689 765 897 514 386 199 506 199 353 978 267 550 695 861 \

307 944 837 214 816 705 122 177 743 763 592 632 902 987 780 842 666 860 302 086 652 720 323 791 882 \
 276 556 464 043 540 851 825 949 956 838 448 909 180 368 452 351 517 109 138 486 024 625 368 151 570 \
 700 250  $q^{9709}$  +

786 027 926 126 955 204 531 212 788 884 275 436 842 926 514 261 132 494 159 101 274 164 117 623 942 \
 686 696 188 810 468 968 597 981 319 139 380 435 105 832 436 142 631 212 647 989 240 134 043 513 269 \
 837 510 900 826 589 730 317 556 952 100 001 287 959 987 680 196 184 237 988 297 681 215 636 505 204 \
 129 792  $q^{9712}$  -

807 988 295 376 354 768 252 987 565 415 867 542 576 980 665 583 466 583 277 968 278 607 463 194 798 \
 436 297 887 044 512 349 967 441 960 083 736 899 487 475 113 084 533 827 216 069 699 592 934 761 556 \
 957 220 775 277 369 708 418 227 758 799 496 909 915 860 299 397 668 637 516 990 369 751 296 904 463 \
 024 128  $q^{9713}$  +

877 612 219 359 527 700 351 091 974 571 728 777 271 890 615 415 507 245 258 733 418 418 260 591 156 \
 005 840 076 178 548 327 499 514 232 248 171 508 739 573 680 154 552 770 521 360 563 862 478 349 574 \
 052 916 975 721 761 524 239 337 988 628 086 490 768 235 233 920 666 413 672 159 364 314 529 859 212 \
 288 000  $q^{9716}$  -

902 126 200 295 671 155 729 824 265 651 646 822 322 659 224 764 633 400 713 710 339 774 486 996 082 \
 483 397 297 251 088 665 320 338 363 984 232 174 245 661 011 859 111 499 696 676 583 263 025 780 427 \
 640 465 618 790 022 343 137 230 869 481 713 994 366 444 964 920 247 553 808 964 917 966 816 511 730 \
 455 556  $q^{9717}$  +

979 845 299 567 690 295 003 500 816 827 791 334 058 532 761 671 965 773 259 681 980 152 321 929 481 \
 985 536 966 907 984 607 188 774 727 135 777 912 826 782 305 859 506 039 818 894 256 908 455 563 417 \
 515 708 641 777 755 198 160 432 286 485 464 834 674 890 456 402 036 930 044 752 539 780 449 963 448 \
 345 600  $q^{9720}$  -

1 007 209 215 905 348 258 626 135 869 037 648 601 861 142 264 944 729 039 084 272 744 536 917 154 875 \
 652 028 601 710 423 100 166 335 255 222 146 871 660 889 556 252 542 336 234 162 050 813 542 999 326 \
 715 783 358 870 323 425 384 404 222 287 243 365 166 578 927 088 183 401 525 291 531 214 784 670 068 \
 736 000  $q^{9721}$  +

1 093 962 760 476 393 896 119 038 176 533 826 930 956 141 059 436 676 484 959 858 989 964 921 913 820 \
 893 142 518 400 194 899 702 220 221 069 607 183 300 736 200 465 615 189 409 216 846 491 045 862 408 \
 278 519 091 860 365 768 089 753 601 195 713 588 011 938 800 528 347 099 817 942 758 801 406 509 249 \
 024 000  $q^{9724}$  -

1 124 507 250 186 776 855 250 038 017 913 015 136 857 308 347 769 571 897 647 360 761 933 872 560 205 \
 698 459 572 621 543 062 054 788 383 270 520 430 903 578 388 153 763 725 856 728 339 801 569 010 117 \
 753 452 561 284 841 658 090 614 343 141 471 453 019 884 155 978 002 485 524 137 330 200 540 139 102 \
 394 200  $q^{9725}$  +

1 221 343 265 607 384 611 253 661 368 777 335 190 364 824 325 061 965 463 365 679 655 528 255 434 363 \
 718 843 159 566 104 939 836 000 647 738 116 178 868 337 025 027 189 011 832 383 017 121 918 651 330 \
 322 035 452 610 659 938 654 472 821 525 720 169 569 582 631 688 768 665 933 143 882 106 051 997 830 \
 217 728  $q^{9728}$  -

1 255 437 246 251 532 354 394 429 086 776 914 068 581 622 782 286 641 701 162 714 519 983 880 320 843 \
 078 171 888 306 013 896 980 605 729 192 492 857 771 372 899 455 389 622 976 444 193 956 009 800 166 \
 868 114 466 697 697 058 924 845 671 446 364 188 704 940 604 862 857 131 406 748 267 547 922 984 386 \
 560 000  $q^{9729}$  +

1 363 525 079 968 651 772 298 544 845 634 351 577 721 432 194 389 306 410 699 044 980 237 274 756 728 \
 537 910 842 156 802 706 316 774 587 588 134 378 447 236 056 874 147 259 532 759 291 528 507 859 384 \
 417 116 419 768 680 524 700 558 135 031 415 708 169 118 042 131 709 210 499 633 126 744 689 208 677 \
 056 512  $q^{9732}$  -

1 401 580 171 310 663 255 900 348 799 536 511 891 880 621 396 762 232 280 082 390 979 475 442 833 467 \
 225 256 275 331 587 357 159 884 196 442 776 508 911 088 915 263 170 825 098 204 683 244 063 354 091 \
 587 066 170 688 157 628 575 358 562 007 704 613 142 838 997 345 141 186 209 588 099 319 806 653 950 \
 928 430  $q^{9733}$  +

1 522 224 508 011 320 568 823 549 788 513 953 838 842 325 931 153 925 324 940 990 265 461 847 723 798 \
 286 130 576 803 521 835 069 551 457 763 578 474 787 427 630 714 526 423 597 824 333 072 515 038 869 \
 059 467 506 777 661 152 102 660 289 453 299 054 375 946 687 598 692 785 285 347 313 648 853 810 992 \
 128 000  $q^{9736}$  -

1 564 699 964 535 192 521 096 098 691 440 285 576 288 382 393 838 242 194 274 423 900 573 249 235 150 632 519 788 158 878 346 097 336 252 986 711 772 658 749 580 612 164 740 730 765 130 309 352 667 857 167 708 774 536 323 925 696 700 496 968 340 617 401 714 935 389 206 342 862 093 762 364 347 641 841 516 544  $q^{9737} +$   
 1 699 356 457 209 244 639 552 359 094 215 738 527 601 224 128 821 707 785 087 996 218 564 448 246 508 555 425 351 604 320 289 170 353 445 077 047 719 071 624 960 343 436 462 677 011 928 125 764 141 726 141 572 927 687 037 825 807 488 250 152 550 393 711 416 117 899 662 365 678 428 234 774 767 426 323 430 400  $q^{9740} -$   
 1 746 764 669 206 464 103 154 114 151 483 545 634 436 314 093 646 908 576 909 765 495 964 359 619 839 582 345 705 696 521 039 558 163 686 382 252 144 432 729 687 266 319 923 030 502 875 325 093 487 884 948 380 260 281 110 206 792 116 389 208 951 120 480 854 057 689 760 625 680 706 191 059 396 552 425 605 625  $q^{9741} +$   
 1 897 057 371 805 510 948 067 556 030 124 744 851 140 800 956 525 210 308 251 763 947 228 482 493 564 679 218 293 757 081 146 919 739 495 243 658 815 832 980 126 796 892 567 833 621 564 604 641 922 562 480 633 011 953 147 938 571 809 521 809 147 579 674 890 476 762 566 867 964 370 554 119 826 216 386 560 000  $q^{9744} -$   
 1 949 970 000 436 512 841 277 894 278 087 927 531 407 722 232 838 763 842 067 357 131 790 140 156 539 012 634 186 294 918 653 559 856 915 504 000 733 978 542 796 522 310 497 259 613 417 298 416 992 448 483 537 933 581 940 504 508 060 964 283 721 529 483 807 979 278 675 448 666 106 012 821 013 971 120 947 200  $q^{9745} +$   
 2 117 710 809 345 519 615 174 258 188 769 007 349 270 678 038 398 925 149 158 420 055 872 626 973 937 706 072 683 922 620 180 022 405 096 529 714 509 911 039 078 953 682 320 760 485 390 786 868 857 338 691 446 999 237 452 565 795 025 265 835 535 137 630 719 171 080 274 325 886 518 488 431 493 461 341 906 944  $q^{9748} -$   
 2 176 765 628 585 883 409 062 510 338 669 522 738 571 168 021 253 315 376 175 253 126 273 247 473 160 441 181 066 567 906 939 572 679 503 253 059 897 046 956 306 511 425 820 522 984 637 789 856 926 818 949 742 334 972 443 206 426 643 265 478 373 354 085 526 879 003 281 913 725 052 651 979 573 266 881 410 250  $q^{9749} +$   
 2 363 975 963 908 332 913 259 413 009 613 548 800 568 247 490 232 606 653 728 353 687 124 550 980 557 680 596 370 044 046 515 570 394 063 551 944 840 694 671 743 835 039 745 236 992 584 911 911 862 950 793 125 426 760 061 754 793 325 509 157 354 681 365 186 421 812 936 034 499 953 104 165 658 457 491 788 800  $q^{9752} -$   
 2 429 884 490 658 400 732 482 815 707 077 613 880 552 283 938 010 123 662 093 115 286 415 402 892 753 841 166 618 495 810 824 531 863 504 327 461 432 340 656 265 542 808 244 004 682 184 488 276 660 010 317 000 415 973 987 743 346 684 746 260 537 261 782 932 279 052 828 979 022 823 185 422 875 368 302 280 704  $q^{9753} +$   
 2 638 819 474 824 357 442 502 135 760 980 659 014 042 201 075 289 485 051 778 235 436 563 073 806 129 831 232 994 673 800 469 180 779 259 627 183 371 687 987 094 761 780 954 500 157 833 679 020 578 014 323 023 083 803 421 832 454 912 445 416 924 288 074 729 306 827 966 251 348 151 424 177 287 074 501 120 000  $q^{9756} -$   
 2 712 375 477 787 126 809 517 037 953 468 757 437 369 068 023 273 838 096 863 498 864 809 860 151 911 867 610 419 586 792 476 137 051 756 166 507 455 109 175 442 426 308 003 819 130 238 790 011 385 085 533 982 025 572 681 006 326 171 441 927 382 041 681 268 541 903 220 753 364 707 036 002 641 502 380 713 074  $q^{9757} +$   
 2 945 550 898 537 847 849 300 707 850 745 317 560 007 377 143 049 677 667 247 733 793 257 154 955 582 890 544 604 592 500 390 716 139 048 840 540 209 730 637 192 603 943 710 397 654 006 468 643 993 969 690 974 599 165 307 934 935 817 759 297 029 566 713 928 612 191 350 383 702 370 608 258 832 555 280 998 400  $q^{9760} -$   
 3 027 639 886 864 059 458 769 590 550 146 470 531 144 865 335 024 077 585 259 484 681 309 002 162 010 458 341 712 080 306 149 778 506 485 911 813 725 665 913 740 822 828 088 229 438 504 483 481 539 484 608 360 201 557 617 497 448 173 541 751 970 124 123 052 116 121 589 299 863 999 321 325 952 336 334 848 000  $q^{9761} +$   
 3 287 862 264 593 652 108 340 620 843 248 000 598 108 298 204 055 780 085 544 156 573 162 393 195 601 757 984 988 914 663 759 187 677 232 495 408 987 499 648 334 967 958 906 879 035 637 873 676 808 095 023 156 772 904 411 964 642 613 917 316 951 040 602 829 469 027 599 444 232 563 219 037 896 583 141

$376\,000 q^{9764} -$   
3 379 472 068 876 982 909 943 718 035 057 965 338 915 130 207 578 139 307 437 679 955 521 503 580 067 325 094 899 429 322 126 950 915 456 022 475 324 896 054 239 098 354 736 361 721 988 725 913 640 611 918 064 807 701 801 069 893 785 943 796 252 854 708 409 717 174 598 044 241 357 130 061 854 626 466 147 875  $q^{9765} +$   
3 669 872 185 007 566 937 584 288 571 498 228 045 691 939 007 120 568 487 686 667 104 385 047 473 191 492 088 480 528 669 532 383 263 060 624 753 106 812 192 521 509 292 867 255 662 896 430 854 688 257 866 342 262 781 765 820 340 420 759 809 009 297 175 778 343 710 507 699 326 979 559 096 951 336 670 056 448  $q^{9768} -$   
3 772 104 756 122 692 744 267 076 839 687 145 367 579 035 126 207 680 707 466 840 945 305 044 763 754 842 193 480 477 735 360 658 338 269 039 641 058 375 371 720 380 504 342 221 892 927 264 464 566 421 045 942 491 326 746 170 341 149 788 036 111 874 331 230 442 572 184 763 657 175 008 835 515 562 872 832 000  $q^{9769} +$   
4 096 175 040 085 128 279 290 752 349 918 054 548 512 752 549 157 345 272 571 667 115 916 242 937 955 475 050 513 115 871 194 634 925 347 552 274 251 395 286 520 667 707 577 227 889 265 165 943 510 033 643 023 897 327 202 922 228 052 067 263 279 175 540 707 286 652 661 334 164 584 918 432 499 066 817 989 632  $q^{9772} -$   
4 210 259 605 748 577 726 143 679 099 533 877 280 162 633 551 767 022 619 666 898 761 229 414 175 578 242 160 074 816 855 251 523 303 158 529 654 950 277 554 618 677 316 902 096 717 645 330 169 817 358 221 137 569 486 544 012 269 287 691 421 214 682 434 144 731 424 487 215 945 382 155 548 136 736 047 230 612  $q^{9773} +$   
4 571 895 823 715 695 726 480 733 042 719 996 653 391 532 820 950 879 732 562 849 072 353 001 370 888 312 038 937 973 583 448 588 992 186 242 317 922 706 069 993 077 493 152 020 369 024 754 531 894 647 591 381 680 524 732 445 472 920 389 528 422 431 607 161 043 998 598 279 603 047 895 753 466 587 806 720 000  $q^{9776} -$   
4 699 203 558 682 579 865 292 091 866 348 305 390 382 754 503 889 365 351 332 878 287 389 147 594 421 384 067 974 184 861 271 352 774 254 933 675 182 288 225 514 298 673 346 739 420 965 622 294 223 871 021 827 000 448 796 385 507 843 616 079 712 153 832 269 495 294 778 175 226 638 032 887 206 786 223 276 032  $q^{9777} +$   
5 102 751 297 990 296 528 793 173 581 671 330 658 884 394 353 736 391 116 624 834 082 668 703 133 005 900 106 575 721 969 878 896 675 653 519 627 346 530 072 623 873 180 201 539 308 433 803 378 119 586 463 308 254 083 931 007 678 865 781 916 477 791 601 939 916 381 893 545 516 154 948 341 786 590 373 888 000  $q^{9780} -$   
5 244 811 681 667 091 852 408 563 379 159 066 816 920 869 014 840 424 208 548 855 692 571 339 205 973 660 895 628 308 211 064 426 141 063 372 913 629 021 485 040 602 784 735 659 654 046 066 981 238 406 775 752 851 962 445 584 516 932 489 881 836 771 018 139 300 725 534 521 911 159 404 913 989 937 918 972 875  $q^{9781} +$   
5 695 118 181 455 975 719 018 586 632 727 869 356 449 959 106 582 593 250 871 052 591 840 573 962 537 397 359 279 911 097 604 693 478 720 634 666 755 967 086 760 914 208 609 760 495 439 371 996 862 141 698 487 266 318 501 722 846 467 921 681 445 629 012 964 209 748 075 998 231 973 464 231 067 836 937 600 000  $q^{9784} -$   
5 853 637 236 619 900 511 174 524 587 421 451 748 035 364 327 905 035 550 211 971 469 274 962 417 025 236 092 485 593 587 241 183 247 690 445 546 672 545 890 346 362 994 918 085 045 236 661 642 957 484 477 574 725 946 493 965 465 191 633 955 163 283 145 689 181 721 880 671 866 617 464 949 672 564 862 156 800  $q^{9785} +$   
6 356 109 178 298 670 612 183 056 530 522 501 468 317 185 113 756 484 428 015 017 127 198 260 796 255 571 846 752 263 013 455 270 534 778 654 110 730 014 346 545 195 607 827 286 618 747 909 861 516 156 320 511 360 476 632 553 547 998 026 073 082 248 071 072 946 430 174 234 679 186 292 142 961 983 344 046 080  $q^{9788} -$   
6 532 989 806 801 008 553 939 468 880 320 076 025 187 889 082 244 563 760 098 107 705 632 962 937 511 663 845 037 749 181 830 379 832 396 955 619 737 006 492 337 038 933 366 182 461 685 095 800 649 051 622 245 573 184 695 893 493 648 391 981 836 949 769 666 967 027 141 970 945 470 141 109 430 845 885 516 625  $q^{9789} +$   
7 093 657 748 212 565 286 118 627 574 836 355 907 898 782 607 594 387 898 004 422 758 381 504 269 489 608 903 270 289 390 331 550 960 838 085 302 398 167 441 835 833 026 029 401 427 283 362 719 939 107

704 695 823 645 650 599 546 035 817 995 948 252 278 374 069 030 582 830 283 756 297 073 320 060 653 \
 666 304  $q^{9792}$  -

7 291 022 404 266 296 034 779 251 407 200 247 932 548 841 719 877 018 985 342 905 645 623 442 018 618 \
 781 701 879 959 823 853 627 260 748 554 617 159 593 892 207 414 877 045 548 575 720 092 408 176 877 \
 325 486 854 875 528 533 953 467 592 208 136 940 794 873 642 922 985 666 523 729 303 155 973 816 215 \
 994 368  $q^{9793}$  +

7 916 612 619 748 810 339 394 004 409 622 532 554 312 567 462 478 120 546 008 143 743 641 583 496 813 \
 408 704 934 676 045 309 466 133 566 613 833 093 663 806 775 290 490 143 774 307 897 490 192 475 750 \
 646 883 398 337 019 428 026 206 006 162 891 933 461 029 488 285 470 075 115 436 488 553 095 970 508 \
 800 000  $q^{9796}$  -

8 136 828 588 949 418 794 331 533 046 051 076 832 131 699 620 385 721 282 081 959 055 468 343 325 731 \
 102 777 887 148 053 589 977 596 546 106 703 790 769 012 163 533 522 156 258 462 801 001 926 069 607 \
 232 491 772 640 697 639 887 834 369 657 045 626 369 515 406 093 324 034 997 501 633 981 921 387 716 \
 048 179  $q^{9797}$  +

8 834 843 164 745 968 460 338 795 181 607 675 995 297 218 614 291 342 006 369 448 130 770 474 701 441 \
 571 639 865 942 934 289 498 584 940 757 017 344 541 680 970 327 863 708 875 130 569 884 091 993 516 \
 673 823 557 972 296 173 690 408 746 232 995 329 638 638 193 035 953 728 118 656 457 238 000 659 036 \
 102 400  $q^{9800}$  -

9 080 550 747 670 572 241 406 089 164 047 178 248 148 684 468 315 773 305 268 514 790 960 266 346 342 \
 266 663 965 350 622 621 532 801 072 304 923 580 910 316 876 800 961 944 069 788 861 455 111 917 661 \
 994 977 176 959 782 874 078 092 928 979 432 076 860 933 865 911 440 242 912 005 951 773 977 734 053 \
 888 248  $q^{9801}$  +

9 859 356 879 371 347 646 455 649 921 435 798 263 016 395 489 230 212 771 152 109 245 526 353 413 555 \
 330 559 304 555 561 414 996 453 213 060 839 272 655 285 400 219 228 566 689 841 979 538 851 716 671 \
 986 447 119 202 706 073 114 294 650 237 385 316 118 356 181 156 954 719 735 950 776 357 835 367 574 \
 528 000  $q^{9804}$  -

10 133 500 812 804 232 207 229 265 848 734 721 785 851 364 659 984 477 150 346 247 075 069 024 079 \
 929 937 179 001 033 943 990 219 980 756 143 760 871 679 917 479 279 611 623 393 134 952 921 546 908 \
 286 989 076 177 102 267 611 957 637 865 758 107 509 580 231 615 128 508 089 045 308 537 730 722 718 \
 106 703 650  $q^{9805}$  +

11 002 430 359 842 107 309 385 970 005 160 834 560 466 517 797 901 608 499 898 715 216 076 767 146 \
 650 210 151 326 914 586 779 893 089 647 757 857 836 790 902 611 852 344 010 880 550 266 557 595 772 \
 967 452 936 812 431 837 439 604 696 613 425 873 826 091 051 901 518 328 502 893 886 798 561 230 330 \
 771 980 288  $q^{9808}$  -

11 308 294 846 784 158 747 557 256 364 926 088 025 594 469 888 022 065 645 996 733 358 638 230 880 \
 828 388 888 285 060 442 686 135 589 255 984 873 541 893 241 036 906 583 095 300 511 840 389 048 084 \
 684 368 188 993 959 649 296 685 272 556 636 528 545 213 841 476 151 500 288 462 062 343 187 916 519 \
 243 776 000  $q^{9809}$  +

12 277 755 319 713 434 796 071 346 722 104 085 311 569 638 920 250 292 852 080 002 511 595 187 885 \
 008 671 516 206 642 827 516 035 086 995 459 134 067 519 667 331 598 499 531 779 966 166 412 479 322 \
 644 938 794 506 049 997 370 498 326 178 862 971 963 927 823 524 426 168 223 316 012 062 559 481 773 \
 371 265 024  $q^{9812}$  -

12 619 003 081 794 060 724 321 437 124 083 366 233 107 711 598 999 803 257 722 637 888 307 855 297 \
 959 029 285 370 495 909 750 365 267 791 561 190 914 970 265 504 106 300 550 275 950 096 823 572 075 \
 287 280 216 776 794 219 857 196 804 402 356 495 481 364 698 007 435 779 159 752 731 808 876 412 767 \
 966 691 836  $q^{9813}$  +

13 700 601 372 573 450 899 951 916 561 419 674 106 871 858 103 390 298 036 056 782 855 311 536 019 \
 394 853 884 816 278 399 227 934 080 080 683 192 031 859 221 105 315 003 242 618 897 388 157 978 061 \
 180 732 132 414 281 541 817 052 079 224 595 155 059 114 104 270 332 349 302 752 884 823 440 609 811 \
 028 992 000  $q^{9816}$  -

14 081 317 185 792 272 321 005 700 102 952 873 775 481 348 919 181 531 644 081 669 408 009 345 275 \
 510 690 657 851 406 672 815 620 747 064 479 169 430 858 069 205 880 206 883 416 773 821 621 484 826 \
 598 712 867 473 206 356 616 493 583 087 635 873 970 380 547 717 046 470 101 259 021 554 200 864 278 \
 146 449 408  $q^{9817}$  +

15 287 997 501 137 077 304 963 207 709 014 848 727 532 109 696 029 377 032 039 323 724 248 161 186 \

923 271 537 307 896 400 683 385 896 512 255 578 482 830 806 972 059 878 872 743 512 554 417 964 865 \\  
 190 723 168 483 012 894 060 858 105 445 625 302 107 366 556 268 589 203 024 778 871 999 533 995 286 \\  
 250 444 800  $q^{9820}$  -

15 712 736 728 571 244 058 235 692 991 641 014 977 532 652 501 630 920 528 706 748 958 307 853 882 \\  
 586 914 949 305 874 280 749 777 606 343 096 774 002 971 820 198 792 476 332 081 091 231 176 431 748 \\  
 694 601 389 086 360 114 598 922 307 104 453 483 524 405 921 810 896 296 739 573 953 720 896 651 242 \\  
 858 432 875  $q^{9821}$  +

17 058 934 353 385 104 614 768 150 582 252 869 767 357 330 643 486 072 673 759 242 335 642 878 692 \\  
 837 468 927 556 852 415 264 467 428 741 726 076 107 635 071 838 608 671 143 883 883 957 029 418 787 \\  
 417 787 049 005 563 591 606 715 272 677 534 516 525 506 446 092 863 325 704 769 685 589 725 065 301 \\  
 613 056 000  $q^{9824}$  -

17 532 777 047 221 610 128 821 101 165 633 907 794 878 708 481 794 058 059 392 654 595 433 652 183 \\  
 746 874 835 999 316 270 881 831 127 886 813 117 806 874 033 850 173 894 715 547 817 199 692 785 187 \\  
 686 242 415 591 455 759 942 631 669 377 312 976 626 276 742 014 770 641 931 026 904 052 823 829 158 \\  
 544 179 200  $q^{9825}$  +

19 034 589 751 112 969 360 322 115 936 976 104 117 050 971 938 706 022 170 906 470 406 331 386 970 \\  
 809 164 152 523 324 970 554 437 028 776 620 773 726 970 719 726 771 403 726 059 155 737 974 140 954 \\  
 549 108 886 561 779 694 993 292 282 210 380 058 387 699 374 568 473 130 711 335 706 100 378 398 250 \\  
 959 241 216  $q^{9828}$  -

19 563 200 961 788 809 731 317 695 636 396 905 236 396 580 567 970 399 542 508 281 814 214 749 791 \\  
 593 981 732 541 341 204 760 089 531 606 790 184 182 089 372 069 063 906 412 457 618 025 508 432 332 \\  
 347 944 119 193 294 564 904 495 532 959 536 050 537 780 003 703 068 511 320 034 632 092 625 965 630 \\  
 510 211 250  $q^{9829}$  +

21 238 580 068 890 409 883 901 882 297 937 887 659 884 655 607 788 489 963 105 152 694 120 366 361 \\  
 424 459 514 131 543 766 852 297 072 167 620 542 085 735 676 785 032 609 351 377 934 391 099 008 665 \\  
 053 883 325 532 879 166 834 186 011 428 769 258 841 660 176 923 303 074 518 049 219 526 389 380 424 \\  
 511 792 640  $q^{9832}$  -

21 828 277 072 009 687 357 380 645 509 754 784 862 178 329 633 309 596 039 205 786 123 182 950 212 \\  
 938 216 688 854 433 825 827 993 409 489 459 284 361 181 126 239 293 582 375 909 414 049 548 536 191 \\  
 973 992 671 618 685 829 139 629 251 723 569 335 118 018 196 228 858 575 095 874 573 182 499 094 539 \\  
 520 114 688  $q^{9833}$  +

23 697 240 445 166 687 723 753 528 613 614 160 265 412 994 758 389 187 195 320 339 462 940 169 736 \\  
 578 748 801 855 238 272 813 168 005 923 578 563 778 510 548 352 243 225 958 034 044 426 607 783 410 \\  
 068 469 484 235 723 949 554 382 315 567 607 424 427 766 292 713 179 768 257 644 323 804 931 274 229 \\  
 227 968 000  $q^{9836}$  -

24 355 067 678 062 315 018 030 509 871 073 193 496 414 417 436 975 822 447 657 039 598 392 896 649 \\  
 409 894 090 288 667 971 667 660 406 601 127 903 529 311 741 411 464 050 147 080 884 953 658 818 392 \\  
 196 321 898 558 714 049 286 167 673 367 329 904 485 883 254 560 224 632 355 008 858 068 922 442 531 \\  
 321 261 810  $q^{9837}$  +

26 439 937 125 626 012 901 353 268 886 954 604 997 738 350 186 780 544 674 573 373 645 668 371 551 \\  
 833 489 331 250 257 210 790 071 814 478 287 888 080 877 781 846 262 421 262 111 259 702 802 621 183 \\  
 509 845 881 903 997 290 205 978 547 645 582 271 587 521 431 537 155 990 382 924 176 080 012 145 918 \\  
 141 235 200  $q^{9840}$  -

27 173 749 715 890 551 922 570 561 172 981 953 799 626 544 453 280 688 045 342 989 735 289 458 613 \\  
 359 260 389 954 777 116 894 471 989 345 970 935 849 741 561 820 298 152 648 110 135 975 101 468 751 \\  
 216 572 514 920 184 902 207 333 302 182 176 365 517 751 552 458 349 611 888 785 065 530 280 134 978 \\  
 019 328 000  $q^{9841}$  +

29 499 415 615 845 837 635 221 949 082 090 719 542 212 082 203 086 616 123 135 696 008 242 230 053 \\  
 897 948 158 434 060 600 698 672 559 279 398 910 797 946 272 388 504 432 176 093 692 523 422 893 154 \\  
 344 091 662 110 302 444 608 094 200 815 801 953 240 303 432 069 418 204 539 451 761 849 070 203 016 \\  
 815 104 000  $q^{9844}$  -

30 317 972 484 924 667 478 336 820 318 798 487 398 224 083 614 954 703 128 021 975 169 873 107 805 \\  
 584 944 173 666 155 065 138 958 918 057 997 651 100 982 565 304 101 662 680 946 168 308 172 423 341 \\  
 849 047 078 433 604 314 441 551 896 784 044 264 200 859 296 395 051 417 586 067 577 329 185 962 885 \\  
 599 689 250  $q^{9845}$  +

32 912 188 740 226 057 837 153 240 481 769 155 687 821 143 850 094 177 100 801 485 427 199 357 474 \\  
 809 998 265 760 976 647 052 746 042 501 145 075 209 349 549 345 218 001 663 304 117 631 782 981 603 \\  
 072 735 383 267 552 363 919 258 293 365 289 406 895 682 970 356 616 964 295 015 594 868 056 980 339 \\  
 292 037 120  $q^{9848}$  -

33 825 256 377 419 597 845 987 888 630 446 046 885 660 478 763 809 112 723 423 488 503 426 163 456 \\  
 750 133 563 637 356 316 136 877 512 320 123 889 157 045 831 219 513 486 809 532 214 745 213 735 619 \\  
 073 933 886 107 541 430 365 239 498 754 968 809 022 345 721 290 288 289 986 671 578 688 141 751 304 \\  
 998 912 000  $q^{9849}$  +

36 718 969 171 927 525 934 019 618 402 505 784 172 976 761 079 362 825 006 702 774 950 557 458 381 \\  
 392 670 460 444 908 184 894 583 785 483 931 181 436 120 021 247 729 168 797 867 660 889 750 399 108 \\  
 170 577 251 763 125 131 923 333 016 031 737 444 983 044 308 225 026 189 510 396 213 187 864 138 117 \\  
 703 387 136  $q^{9852}$  -

37 737 437 299 193 902 309 847 704 199 175 068 719 585 385 963 443 993 166 878 315 607 409 197 427 \\  
 073 179 296 351 956 979 745 818 616 164 091 897 195 929 669 964 636 196 049 311 685 145 586 087 833 \\  
 317 357 354 928 785 812 386 148 565 622 413 841 825 365 428 003 144 179 833 914 792 393 673 360 677 \\  
 443 762 819  $q^{9853}$  +

40 965 151 519 626 107 834 106 105 872 821 014 714 566 830 028 589 028 084 608 210 485 637 494 741 \\  
 523 832 628 358 437 439 137 391 408 625 901 802 556 691 617 371 436 038 939 581 213 764 176 317 477 \\  
 136 778 560 976 850 462 721 878 759 771 624 162 909 475 940 751 064 214 512 181 998 194 467 603 491 \\  
 078 144 000  $q^{9856}$  -

42 101 162 006 865 974 187 210 766 287 966 392 765 670 323 516 864 900 407 850 197 716 848 931 323 \\  
 197 159 264 212 892 772 431 256 404 386 124 580 622 200 880 982 627 659 142 116 581 283 682 607 884 \\  
 221 019 184 414 469 170 121 628 857 285 996 962 747 584 979 721 033 340 378 972 039 528 446 221 246 \\  
 747 738 112  $q^{9857}$  +

45 701 349 637 313 976 027 402 452 430 010 507 284 073 799 517 347 537 463 724 929 690 517 940 464 \\  
 466 781 231 987 629 957 872 502 888 792 788 044 960 318 721 671 678 149 221 855 580 735 064 545 552 \\  
 601 226 390 735 808 645 893 818 627 251 447 252 847 846 065 166 869 041 528 682 278 606 584 044 488 \\  
 192 819 200  $q^{9860}$  -

46 968 440 182 974 765 658 326 746 060 451 065 349 365 798 602 221 705 917 834 582 165 814 817 243 \\  
 090 754 633 978 638 526 226 455 950 183 906 838 773 048 989 946 945 580 132 634 474 124 741 836 205 \\  
 764 154 108 889 239 178 923 938 208 859 446 696 804 246 375 925 697 250 264 147 376 148 187 135 852 \\  
 336 893 000  $q^{9861}$  +

50 983 995 469 910 733 429 785 517 989 271 091 466 736 318 289 940 648 862 538 084 695 168 994 605 \\  
 895 495 947 064 321 203 814 974 730 363 653 620 699 810 386 756 562 653 625 608 698 382 843 197 464 \\  
 946 990 809 503 264 015 992 377 257 456 164 082 501 452 671 238 880 720 076 627 803 961 898 322 164 \\  
 428 160 000  $q^{9864}$  -

52 397 259 734 571 771 470 484 352 811 997 162 951 843 300 265 252 025 427 195 075 188 067 589 771 \\  
 557 020 301 761 004 612 621 258 003 573 372 982 772 853 658 645 357 271 131 242 449 670 137 521 536 \\  
 499 219 856 509 382 418 204 045 075 436 596 026 505 662 324 278 729 822 868 641 796 242 177 838 742 \\  
 513 254 400  $q^{9865}$  +

56 876 006 467 596 637 972 271 621 654 545 280 882 836 836 373 602 350 305 381 110 402 465 801 092 \\  
 855 938 736 544 204 308 489 576 498 094 181 513 123 883 083 876 492 988 111 032 841 540 170 533 711 \\  
 649 395 107 808 024 373 098 100 364 962 818 869 420 467 809 555 381 587 474 763 667 436 850 078 870 \\  
 154 397 184  $q^{9868}$  -

58 452 272 540 697 168 113 683 487 679 267 384 369 087 438 652 043 637 023 527 066 841 029 155 959 \\  
 921 963 591 367 073 626 673 033 997 176 987 012 411 453 155 658 768 135 574 484 840 756 205 633 547 \\  
 942 355 400 578 818 973 655 714 519 560 858 983 951 305 602 997 133 935 779 736 707 461 261 838 223 \\  
 526 196 750  $q^{9869}$  +

63 447 529 403 914 157 445 310 584 400 735 158 089 746 329 804 802 560 120 967 652 253 214 711 682 \\  
 962 188 354 227 357 997 116 528 446 363 371 750 821 978 556 712 697 142 224 052 980 958 448 451 407 \\  
 882 717 854 788 032 671 769 001 252 777 067 792 813 251 239 698 671 178 190 874 161 726 750 604 526 \\  
 712 651 776  $q^{9872}$  -

65 205 558 698 199 045 336 530 074 620 360 418 268 968 697 679 939 633 602 038 661 548 150 939 923 \\  
 015 628 557 364 261 548 631 337 554 207 268 060 947 646 054 113 003 331 808 396 170 381 446 431 840 \\  
 446 234 613 153 831 170 496 815 785 056 062 256 190 987 801 018 436 203 176 607 673 603 183 798 095 \

029 829 632  $q^{9873} +$   
 70 776 769 326 116 478 911 254 487 482 684 620 753 711 326 697 280 102 224 322 279 173 475 535 796 \ \backslash  
 235 361 234 523 773 273 019 179 695 350 204 828 536 184 843 854 068 433 698 592 564 110 366 019 967 \ \backslash  
 486 356 893 305 242 513 363 321 373 310 930 146 330 257 640 621 766 810 098 853 292 840 778 527 803 \ \backslash  
 113 984 000  $q^{9876} -$   
 72 737 478 233 188 229 277 947 905 167 598 847 237 019 818 962 622 650 914 709 214 496 473 734 322 \ \backslash  
 077 439 129 938 974 268 348 959 055 946 339 105 984 420 957 443 112 737 277 924 742 294 364 246 421 \ \backslash  
 270 234 510 085 614 596 606 586 567 422 641 443 093 781 507 378 877 217 720 940 971 993 232 796 396 \ \backslash  
 624 506 036  $q^{9877} +$   
 78 950 913 361 342 571 420 917 053 087 155 118 241 538 479 489 539 456 206 542 414 017 068 149 971 \ \backslash  
 206 094 635 013 122 072 359 110 681 115 400 282 960 665 742 799 193 742 249 957 186 477 435 337 303 \ \backslash  
 745 697 571 619 280 503 675 325 883 717 569 724 933 774 496 788 204 866 311 525 056 176 066 774 870 \ \backslash  
 646 374 400  $q^{9880} -$   
 81 137 620 267 694 589 449 637 530 695 061 196 720 263 304 093 904 579 226 679 135 675 634 198 596 \ \backslash  
 175 893 388 685 310 549 852 613 920 903 248 917 412 073 144 784 991 171 256 285 759 023 526 868 726 \ \backslash  
 945 061 750 771 607 100 059 679 950 114 315 831 624 618 007 012 020 466 453 541 991 853 150 380 625 \ \backslash  
 084 416 000  $q^{9881} +$   
 88 067 160 210 513 569 304 091 028 523 001 139 674 755 326 417 860 229 537 559 117 731 346 348 713 \ \backslash  
 203 491 390 825 631 785 693 145 380 608 924 987 158 034 548 288 926 702 577 706 651 149 607 091 318 \ \backslash  
 095 596 084 926 354 928 926 273 051 218 521 742 220 880 773 950 373 355 922 467 713 927 119 240 394 \ \backslash  
 757 632 000  $q^{9884} -$   
 90 505 860 769 663 644 349 629 045 482 849 305 589 742 302 548 277 791 030 526 640 188 744 028 999 \ \backslash  
 659 868 871 420 679 211 937 287 846 663 045 806 058 586 051 431 308 094 011 576 012 140 563 425 234 \ \backslash  
 744 239 240 427 219 209 842 546 880 975 524 861 306 498 230 989 348 616 439 160 526 280 005 963 618 \ \backslash  
 790 603 225  $q^{9885} +$   
 98 233 867 396 228 657 670 344 123 862 956 112 958 588 201 212 286 238 754 037 360 721 682 714 049 \ \backslash  
 153 626 051 438 694 238 381 578 527 745 641 801 341 001 030 517 668 414 364 200 817 682 716 594 480 \ \backslash  
 327 446 880 581 894 410 717 350 087 927 732 336 571 425 486 424 427 306 921 879 022 469 103 507 721 \ \backslash  
 223 233 536  $q^{9888} -$   
 100 953 541 282 508 392 979 613 321 268 740 842 660 154 470 828 248 824 896 125 570 856 960 779 935 \ \backslash  
 265 058 121 155 256 414 454 304 206 348 609 590 532 944 828 270 528 172 166 811 246 124 358 857 609 \ \backslash  
 553 824 893 301 699 368 770 805 798 381 549 437 478 932 269 764 311 508 741 176 379 816 783 882 802 \ \backslash  
 765 824 000  $q^{9889} +$   
 109 571 829 705 700 768 032 971 784 582 300 416 360 653 959 669 649 653 297 410 541 451 926 593 893 \ \backslash  
 364 454 445 729 817 828 659 775 425 892 707 325 405 747 379 363 982 216 435 775 884 279 095 418 871 \ \backslash  
 445 296 673 636 076 391 136 323 908 951 275 427 335 052 202 921 211 806 583 668 407 791 280 057 157 \ \backslash  
 477 744 640  $q^{9892} -$   
 112 604 782 442 710 210 434 766 614 926 930 455 881 077 141 039 579 292 356 695 551 740 937 420 903 \ \backslash  
 979 071 347 477 436 031 554 299 785 002 551 163 102 129 250 930 594 156 545 652 773 091 365 736 833 \ \backslash  
 862 484 385 631 012 252 492 520 163 416 402 138 852 642 957 467 634 351 457 324 970 627 679 067 717 \ \backslash  
 774 678 480  $q^{9893} +$   
 122 215 703 800 844 788 715 264 966 741 034 939 304 774 823 062 806 855 377 200 192 777 427 681 572 \ \backslash  
 103 694 900 678 324 461 392 255 822 764 762 538 773 579 974 189 427 268 197 283 867 710 500 176 065 \ \backslash  
 560 517 437 283 437 396 979 244 643 322 732 102 323 834 754 833 552 451 493 633 309 668 646 960 134 \ \backslash  
 778 176 000  $q^{9896} -$   
 125 597 947 666 809 050 997 581 576 799 000 060 672 465 284 793 073 625 871 743 847 210 791 033 533 \ \backslash  
 078 743 771 045 441 292 635 020 675 118 033 963 832 647 352 517 852 387 315 050 062 803 206 443 304 \ \backslash  
 294 727 943 263 713 956 455 422 990 327 291 857 905 447 096 641 035 848 603 384 448 431 066 268 123 \ \backslash  
 338 539 008  $q^{9897} +$   
 136 315 595 672 749 573 115 608 580 063 577 767 481 859 557 675 250 974 271 690 671 405 910 342 266 \ \backslash  
 864 011 501 349 576 872 906 042 906 627 382 703 441 006 612 739 813 611 594 695 433 279 603 259 814 \ \backslash  
 703 428 001 395 246 656 640 610 222 591 642 721 627 667 640 963 479 412 979 077 926 568 902 562 926 \ \backslash  
 860 582 400  $q^{9900} -$   
 140 087 274 140 755 109 120 857 704 626 829 640 145 464 254 146 966 968 483 019 290 674 896 948 817 \ \backslash  
 272 903 428 526 918 444 834 356 646 223 654 073 091 125 667 339 950 893 635 765 515 588 851 551 791 \ \backslash

415 291 476 678 305 249 076 852 717 583 179 485 860 145 309 597 044 099 198 098 977 830 203 463 819 \
 682 864 375  $q^{9901}$  +

152 038 829 516 673 987 493 667 609 741 764 328 623 344 731 280 503 873 693 489 971 028 431 506 170 \
 445 371 566 772 231 123 805 016 575 404 122 640 459 485 158 463 634 119 712 437 860 390 125 066 870 \
 332 079 994 460 580 707 536 747 015 389 984 367 646 401 384 316 700 799 985 573 069 126 484 220 546 \
 283 008 000  $q^{9904}$  -

156 244 690 195 292 273 237 116 354 464 767 752 343 702 434 165 081 472 126 655 909 486 111 535 055 \
 485 139 861 977 857 962 779 986 235 445 655 855 383 309 325 353 137 294 769 622 431 307 502 551 647 \
 392 158 893 825 135 226 030 154 333 557 283 385 623 103 585 575 209 189 829 128 635 425 073 767 790 \
 646 067 200  $q^{9905}$  +

169 571 918 718 386 001 237 480 073 811 684 789 430 568 252 194 125 696 228 602 261 130 373 711 547 \
 245 419 596 620 641 029 099 891 901 480 127 263 986 180 523 761 545 067 469 649 481 034 681 748 338 \
 955 958 594 765 195 018 297 952 227 893 655 599 863 474 240 662 575 089 849 108 181 881 139 054 762 \
 528 086 016  $q^{9908}$  -

174 261 840 323 384 794 960 922 107 700 708 890 123 073 866 867 412 473 973 586 305 683 710 804 362 \
 111 144 659 302 072 404 104 240 834 612 409 809 052 649 574 032 063 363 999 564 461 058 856 206 275 \
 663 363 927 260 440 301 691 906 835 432 236 553 930 734 144 753 913 669 172 778 041 538 701 904 387 \
 304 328 500  $q^{9909}$  +

189 122 761 997 579 561 128 605 267 945 651 131 163 015 237 482 626 177 930 794 887 695 102 491 526 \
 767 093 409 299 902 510 915 080 540 973 926 837 987 678 272 885 073 773 625 755 036 177 873 290 514 \
 380 337 221 028 958 600 157 760 355 668 223 639 073 933 367 788 622 578 171 056 723 998 395 929 234 \
 354 274 304  $q^{9912}$  -

194 352 341 514 814 425 707 950 176 307 638 055 178 754 207 720 517 201 053 056 335 576 491 360 928 \
 214 546 351 022 068 176 239 427 154 173 370 611 487 276 753 164 233 230 160 640 809 782 482 383 469 \
 292 171 799 325 785 406 780 432 199 618 354 301 152 339 682 699 696 059 574 092 700 095 754 427 202 \
 479 128 576  $q^{9913}$  +

210 923 090 376 492 632 602 539 625 630 235 384 713 264 648 722 412 196 414 092 432 063 041 274 613 \
 049 107 097 188 212 248 794 271 867 904 259 692 436 711 889 886 048 205 376 309 810 057 143 250 426 \
 083 864 023 429 307 768 104 631 705 904 651 767 240 731 126 943 059 293 169 567 757 214 696 343 351 \
 533 312 000  $q^{9916}$  -

216 754 297 276 941 500 088 907 302 694 805 498 042 638 642 531 617 510 061 487 935 619 536 841 161 \
 772 985 994 300 646 826 486 243 484 025 096 808 247 305 959 844 983 720 674 597 729 282 903 154 453 \
 389 761 001 246 504 819 340 989 621 956 645 025 105 570 138 759 338 962 578 711 078 229 457 616 860 \
 023 745 918  $q^{9917}$  +

235 231 193 562 028 685 822 388 012 071 303 383 812 118 945 700 680 552 805 146 644 155 817 630 574 \
 590 322 303 921 527 284 988 252 694 749 217 362 801 351 502 355 496 511 414 879 695 320 327 344 568 \
 856 958 656 001 814 742 711 155 053 050 363 656 865 626 357 172 358 685 848 535 078 978 220 839 328 \
 458 342 400  $q^{9920}$  -

241 733 098 710 380 678 091 839 286 395 431 956 652 145 238 823 904 065 809 797 406 541 969 296 051 \
 531 901 880 860 669 840 845 803 607 532 997 658 138 533 942 645 691 755 124 946 132 830 108 028 519 \
 129 157 652 289 131 134 088 301 350 711 644 007 731 548 455 663 441 382 182 315 463 393 370 542 547 \
 251 200 000  $q^{9921}$  +

262 334 957 581 399 738 947 271 932 022 126 910 408 368 098 020 518 431 754 915 873 937 459 780 089 \
 270 822 617 049 117 911 362 787 870 140 502 850 201 423 273 605 282 390 994 143 005 887 783 983 675 \
 400 537 637 360 323 605 394 207 793 996 152 026 405 461 567 733 178 682 620 458 726 242 073 800 476 \
 968 960 000  $q^{9924}$  -

269 584 545 348 653 178 162 351 420 631 422 908 066 411 939 713 108 181 952 886 092 213 917 090 866 \
 335 739 617 878 448 423 771 398 087 947 861 381 478 980 071 817 568 214 934 372 803 231 987 327 572 \
 383 681 073 276 341 616 483 049 785 244 227 386 176 456 962 422 500 602 290 620 321 320 427 590 530 \
 317 873 975  $q^{9925}$  +

292 555 249 132 124 979 532 073 223 085 101 857 452 420 181 119 881 852 274 260 064 332 321 356 182 \
 959 931 002 897 323 601 762 782 391 265 218 506 991 194 565 876 690 769 877 440 776 679 516 872 911 \
 628 176 847 156 478 958 536 260 411 968 066 930 491 552 362 741 876 505 507 901 351 860 041 281 497 \
 012 647 936  $q^{9928}$  -

300 638 322 190 325 079 939 999 334 970 705 442 784 309 023 806 485 100 286 717 882 101 842 715 082 \

809 873 117 456 709 665 555 823 266 016 557 275 045 674 917 157 080 004 684 988 657 751 631 540 006  
 196 747 995 485 930 410 983 146 345 941 401 150 004 069 700 130 312 396 427 983 731 865 854 105 141  
 944 320 000  $q^{9929} +$   
 326 249 686 138 945 269 974 278 061 466 847 030 581 654 819 753 301 742 560 811 112 336 614 151 576  
 382 301 996 978 331 260 121 019 631 500 108 303 998 605 636 131 018 275 025 552 883 914 476 731 914  
 211 516 599 069 187 932 980 817 098 744 211 704 083 681 498 095 121 387 653 348 095 063 298 246 663  
 630 055 424  $q^{9932} -$   
 335 261 873 493 670 612 686 482 474 550 951 284 522 180 995 758 107 038 691 726 202 019 462 151 757  
 221 938 870 904 841 309 304 981 234 667 060 581 116 701 385 096 073 940 756 243 410 223 334 991 095  
 931 776 708 782 010 236 659 527 742 341 281 229 486 824 339 301 415 546 541 513 423 187 515 543 133  
 203 274 258  $q^{9933} +$   
 363 816 838 499 387 206 207 725 979 363 891 149 500 099 946 140 329 267 863 475 204 912 074 537 325  
 861 345 351 268 827 316 696 533 838 040 905 368 789 146 840 190 851 883 615 351 033 102 614 920 601  
 022 356 474 435 118 499 389 159 814 420 466 095 525 518 432 371 060 916 233 662 928 001 828 369 681  
 711 104 000  $q^{9936} -$   
 373 864 718 515 309 650 543 163 183 397 085 208 645 439 475 374 159 513 266 696 702 367 022 487 811  
 119 550 716 099 430 136 094 125 784 888 870 638 116 739 108 368 364 974 048 424 267 682 075 969 587  
 971 474 338 953 241 480 245 360 462 472 978 367 560 590 499 078 594 613 384 441 826 077 975 243 952  
 490 512 384  $q^{9937} +$   
 405 700 907 998 127 136 411 582 830 009 087 421 003 258 196 829 113 392 685 507 749 032 222 091 873  
 398 751 346 090 711 620 504 157 607 120 081 435 217 814 324 073 503 546 850 368 691 666 967 879 383  
 398 612 377 359 625 055 941 472 850 078 528 284 442 145 953 927 948 042 256 614 749 700 537 847 696  
 829 440 000  $q^{9940} -$   
 416 903 259 508 761 306 662 255 383 193 803 791 672 576 057 006 883 652 707 861 250 334 015 877 051  
 668 723 747 937 767 764 307 505 140 671 158 422 016 136 663 002 101 404 919 959 341 853 856 146 726  
 354 898 307 317 196 576 517 776 476 183 347 512 045 371 753 270 170 241 600 639 734 908 549 629 795  
 754 878 000  $q^{9941} +$   
 452 396 941 935 614 770 508 005 719 969 198 795 034 729 706 510 286 929 553 129 363 043 722 614 621  
 323 590 872 128 962 506 118 543 333 350 611 685 319 372 744 746 180 000 078 127 254 890 322 661 750  
 356 781 430 243 200 211 623 695 995 136 844 915 591 097 416 454 462 215 851 412 415 693 524 379 482  
 067 200 000  $q^{9944} -$   
 464 886 138 015 643 228 250 304 887 537 970 916 169 946 775 161 269 231 904 811 386 355 383 652 621  
 153 799 959 343 325 953 608 674 301 874 105 167 850 550 804 281 354 192 879 095 543 720 552 799 413  
 231 971 271 323 535 932 320 662 841 341 713 266 980 678 067 962 124 077 961 212 692 308 587 951 864  
 725 504 000  $q^{9945} +$   
 504 456 641 212 779 643 562 251 943 793 952 159 408 357 734 026 381 684 418 287 436 515 582 257 166  
 548 610 108 178 969 948 913 557 043 573 946 933 006 340 260 870 283 228 862 124 973 675 683 437 647  
 213 338 055 659 321 247 189 301 043 553 822 806 016 420 903 602 390 712 990 387 213 851 790 065 472  
 470 218 752  $q^{9948} -$   
 518 380 201 847 230 719 260 474 283 665 300 004 677 474 904 736 675 444 874 393 096 539 271 082 463  
 657 404 671 078 319 317 460 193 663 481 464 532 564 317 590 747 353 643 065 749 631 831 666 444 668  
 172 609 877 743 879 986 258 983 865 399 931 465 950 250 535 664 818 150 820 527 647 226 586 725 954  
 150 406 125  $q^{9949} +$   
 562 494 830 512 470 733 813 547 584 417 283 431 758 115 507 431 343 221 191 244 594 782 512 231 486  
 497 345 796 549 235 944 564 952 917 156 664 005 715 869 975 595 576 885 035 812 732 664 900 489 275  
 758 291 953 034 746 136 475 930 827 409 613 969 237 852 727 351 846 511 220 951 878 962 797 097 411  
 335 102 464  $q^{9952} -$   
 578 017 152 240 616 136 490 874 044 622 692 694 896 464 474 424 781 774 667 251 457 121 327 254 994  
 931 389 486 202 540 060 806 096 015 318 476 264 350 793 564 993 832 195 224 857 600 759 561 252 589  
 381 789 812 849 561 158 128 373 731 610 907 836 352 776 715 321 312 773 261 199 268 557 431 190 957  
 514 883 072  $q^{9953} +$   
 627 196 665 899 042 928 917 948 206 437 012 277 974 348 571 148 285 459 407 728 537 456 590 227 626  
 149 456 273 113 069 425 138 688 724 929 028 785 508 808 485 074 356 704 909 361 970 184 902 199 065  
 961 575 254 323 022 518 883 645 435 780 538 843 971 284 292 300 248 548 418 313 198 451 759 324 018  
 759 680 000  $q^{9956} -$

644 500 948 563 404 243 580 425 714 260 479 016 293 761 913 921 785 411 100 098 394 085 707 542 301 \
 264 488 679 836 587 808 823 492 456 147 715 107 589 704 452 204 072 011 378 363 117 538 864 801 358 \
 888 152 158 142 019 691 088 063 318 142 850 059 309 694 233 762 526 892 420 207 575 857 767 854 210 \
 815 190 551  $q^{9957} +$

699 325 663 708 649 451 509 400 011 948 508 317 247 478 255 782 764 821 036 674 422 478 665 877 420 \
 195 659 545 465 386 439 015 662 229 190 713 070 581 858 708 387 912 287 518 419 209 591 634 344 820 \
 545 196 035 908 150 164 553 259 798 053 794 184 995 650 924 246 764 098 670 080 976 822 481 826 446 \
 276 300 800  $q^{9960} -$

718 616 056 724 585 944 242 973 235 756 557 063 151 544 785 852 200 827 978 216 796 253 177 866 574 \
 476 834 298 468 216 155 379 632 774 872 999 600 636 084 942 128 236 581 471 519 066 710 282 280 053 \
 536 541 074 411 363 641 996 268 851 625 128 690 126 899 571 335 077 393 021 559 066 236 608 864 013 \
 615 104 000  $q^{9961} +$

779 732 644 122 756 156 313 976 793 079 202 896 983 348 629 062 528 116 370 448 257 080 540 350 325 \
 510 104 694 171 285 075 378 626 551 273 235 091 553 247 201 526 869 631 191 490 038 259 310 685 157 \
 983 444 889 445 215 984 784 661 906 349 220 252 061 098 783 708 424 429 282 561 740 121 579 571 404 \
 507 904 000  $q^{9964} -$

801 236 637 228 047 347 804 862 473 351 942 967 615 049 162 487 102 495 724 778 493 147 966 216 367 \
 229 943 961 027 886 847 807 543 209 317 959 805 967 299 989 585 125 980 988 673 213 762 598 945 028 \
 805 916 571 217 431 390 719 671 055 130 005 900 758 084 331 259 976 088 010 111 184 526 019 271 396 \
 921 670 025  $q^{9965} +$

869 365 693 415 699 488 524 169 958 219 258 453 090 548 743 242 360 301 847 914 864 122 356 001 315 \
 268 631 143 895 074 204 552 445 086 062 752 141 906 689 747 422 896 770 683 454 760 227 078 019 460 \
 010 242 517 700 053 501 626 646 372 520 192 762 366 879 306 770 645 253 127 965 211 649 334 546 058 \
 318 118 912  $q^{9968} -$

893 336 779 691 598 464 526 745 701 900 141 825 224 514 114 711 335 046 675 107 130 445 098 391 421 \
 973 506 176 037 160 742 491 645 993 806 165 468 927 200 103 419 215 500 091 759 190 817 732 683 138 \
 878 945 507 004 510 481 703 948 479 053 470 758 801 692 465 579 809 954 128 898 869 996 702 628 018 \
 630 656 000  $q^{9969} +$

969 281 260 665 661 947 555 414 189 864 913 538 700 946 283 173 138 814 208 480 912 193 048 615 209 \
 471 875 503 691 110 262 292 136 261 477 295 673 071 632 990 807 822 375 624 314 900 389 730 013 298 \
 471 762 880 843 318 574 161 447 856 813 126 455 966 820 157 461 999 087 786 087 729 829 134 181 185 \
 155 201 024  $q^{9972} -$

996 001 902 773 644 562 708 454 266 380 453 197 419 286 906 850 925 313 835 966 103 689 110 124 605 \
 797 624 457 727 287 475 967 376 560 422 069 432 443 622 856 950 709 393 613 637 862 652 861 288 763 \
 406 281 036 433 572 826 143 546 580 109 979 437 340 059 596 986 137 294 940 751 718 777 795 889 970 \
 574 926 169  $q^{9973} +$

1 080 656 517 852 885 327 756 044 264 005 971 543 621 728 109 355 003 246 860 326 329 386 049 596 690 \
 859 272 041 645 937 737 138 271 368 468 860 977 136 542 576 690 859 669 010 278 439 320 414 678 079 \
 479 943 759 814 458 305 581 975 267 117 775 511 249 518 109 981 472 090 532 979 680 777 596 797 434 \
 094 208 000  $q^{9976} -$

1 110 441 451 940 994 720 789 719 803 970 087 423 925 349 862 947 379 791 589 371 304 340 464 241 778 \
 832 525 333 717 153 852 033 120 275 825 485 381 179 756 356 886 492 799 027 070 450 422 669 654 038 \
 405 390 158 956 515 609 420 814 570 395 795 551 293 949 480 548 172 249 693 706 992 346 966 179 016 \
 134 852 608  $q^{9977} +$

1 204 803 126 890 230 172 734 527 708 314 147 748 608 693 967 302 141 353 159 347 835 447 127 160 865 \
 072 385 894 851 036 420 833 414 924 823 817 814 170 724 036 259 420 056 885 705 654 979 058 877 239 \
 217 846 670 834 783 853 284 647 638 679 286 406 901 169 293 690 936 773 221 113 314 550 349 213 792 \
 277 760 000  $q^{9980} -$

1 238 003 042 529 840 387 784 310 729 306 956 413 712 014 684 975 924 143 473 973 736 234 404 471 858 \
 638 727 823 763 877 126 747 548 532 635 606 236 789 747 696 781 674 791 173 338 842 562 089 890 353 \
 879 822 457 156 437 593 407 403 722 077 711 183 064 476 655 049 665 588 577 766 922 852 047 949 549 \
 620 943 500  $q^{9981} +$

1 343 182 573 407 288 311 505 775 065 381 717 823 490 049 686 592 480 371 379 817 376 237 891 514 589 \
 012 505 807 489 339 662 040 975 789 455 529 777 957 614 193 491 102 611 374 320 248 103 187 172 064 \
 623 866 836 748 591 537 841 800 357 428 418 933 045 165 033 595 061 105 179 826 315 002 854 237 800

$366\,080\,000\,q^{9984} -$   
 $1\,380\,188\,212\,270\,156\,914\,142\,038\,350\,315\,991\,562\,859\,370\,455\,158\,304\,944\,831\,423\,693\,175\,571\,381\,357\,054\,598\,238\,190\,186\,081\,736\,330\,956\,832\,743\,869\,581\,939\,441\,398\,054\,627\,140\,228\,026\,318\,058\,076\,314\,818\,916\,320\,747\,139\,112\,074\,304\,293\,233\,095\,353\,201\,151\,462\,289\,994\,838\,078\,463\,544\,303\,134\,836\,975\,334\,195\,200\,q^{9985} +$   
 $1\,497\,423\,245\,227\,069\,153\,816\,823\,799\,245\,254\,366\,736\,300\,495\,635\,208\,321\,988\,051\,272\,483\,827\,494\,147\,718\,732\,361\,182\,387\,902\,572\,054\,188\,609\,074\,275\,642\,275\,491\,682\,513\,134\,361\,163\,510\,095\,677\,521\,145\,096\,608\,856\,507\,414\,604\,731\,132\,083\,732\,039\,028\,200\,166\,449\,114\,242\,327\,622\,111\,130\,278\,999\,917\,606\,360\,694\,784\,q^{9988} -$   
 $1\,538\,669\,966\,053\,646\,270\,940\,460\,908\,148\,915\,917\,939\,430\,789\,835\,049\,272\,577\,105\,394\,667\,680\,772\,536\,076\,317\,583\,264\,181\,699\,723\,515\,736\,900\,684\,182\,554\,212\,546\,627\,786\,478\,265\,598\,736\,900\,435\,074\,563\,783\,978\,355\,934\,280\,989\,294\,421\,352\,863\,779\,789\,549\,575\,117\,131\,881\,397\,829\,492\,261\,473\,396\,080\,832\,997\,122\,250\,q^{9989} +$   
 $1\,669\,339\,453\,641\,781\,824\,715\,787\,035\,800\,933\,635\,334\,011\,802\,791\,507\,297\,055\,385\,979\,271\,355\,040\,191\,685\,129\,570\,470\,504\,414\,962\,779\,401\,186\,283\,480\,190\,180\,789\,384\,437\,718\,495\,060\,078\,831\,096\,677\,816\,031\,194\,735\,536\,692\,115\,526\,638\,726\,000\,186\,519\,613\,643\,296\,206\,379\,744\,487\,154\,204\,237\,054\,736\,157\,129\,713\,664\,q^{9992} -$   
 $1\,715\,312\,316\,440\,448\,889\,971\,379\,458\,512\,608\,009\,540\,193\,769\,724\,429\,918\,983\,011\,083\,429\,434\,532\,415\,913\,484\,972\,256\,626\,084\,661\,541\,057\,408\,034\,284\,342\,319\,510\,305\,628\,713\,330\,058\,439\,745\,011\,978\,054\,871\,643\,075\,056\,051\,517\,565\,579\,603\,611\,129\,719\,762\,201\,990\,620\,833\,830\,956\,384\,062\,438\,381\,838\,708\,831\,453\,184\,q^{9993} +$   
 $1\,860\,952\,618\,042\,833\,269\,043\,666\,904\,380\,713\,084\,061\,280\,767\,182\,710\,481\,592\,741\,614\,132\,536\,647\,843\,546\,063\,749\,745\,623\,861\,373\,324\,021\,458\,711\,542\,985\,000\,286\,074\,287\,877\,975\,343\,566\,649\,412\,644\,358\,629\,014\,952\,073\,038\,114\,232\,676\,046\,292\,520\,571\,291\,015\,012\,182\,726\,192\,636\,449\,769\,319\,018\,231\,261\,431\,424\,000\,q^{9996} -$   
 $1\,912\,192\,046\,457\,875\,808\,854\,231\,903\,936\,756\,069\,812\,564\,128\,262\,752\,601\,396\,138\,209\,672\,062\,598\,454\,786\,939\,337\,823\,450\,420\,706\,855\,329\,419\,108\,608\,846\,514\,497\,871\,575\,156\,273\,259\,647\,035\,852\,114\,788\,356\,332\,098\,522\,270\,419\,459\,653\,632\,210\,021\,865\,331\,411\,118\,937\,550\,299\,252\,436\,804\,860\,708\,915\,296\,134\,788\,849\,q^{9997} +$   
 $2\,074\,514\,859\,447\,338\,796\,208\,141\,712\,518\,764\,438\,686\,335\,016\,902\,030\,321\,543\,956\,259\,869\,099\,515\,024\,744\,684\,658\,279\,684\,238\,447\,302\,398\,305\,398\,285\,899\,183\,968\,229\,051\,707\,076\,970\,759\,449\,073\,734\,312\,796\,927\,621\,932\,295\,734\,732\,570\,745\,767\,511\,851\,265\,303\,195\,054\,086\,603\,529\,721\,350\,022\,824\,551\,391\,571\,840\,000\,q^{10000} -$   
 $2\,131\,622\,946\,909\,794\,682\,246\,232\,048\,132\,183\,700\,199\,854\,906\,471\,947\,860\,388\,698\,250\,930\,096\,381\,906\,506\,280\,410\,282\,994\,095\,475\,451\,960\,981\,286\,073\,145\,696\,111\,414\,523\,870\,227\,510\,741\,541\,959\,988\,613\,834\,265\,078\,981\,786\,303\,157\,310\,216\,788\,483\,543\,030\,664\,666\,480\,460\,297\,171\,502\,698\,841\,797\,615\,376\,039\,936\,000\,q^{10001} + O[q]^{10002}$

In[11]:=
